# Supplementary material for: Emergent domain topology in the multiferroic hexagonal manganites
Source: arXiv:2510.13020 ancillary file (2025-10-14)

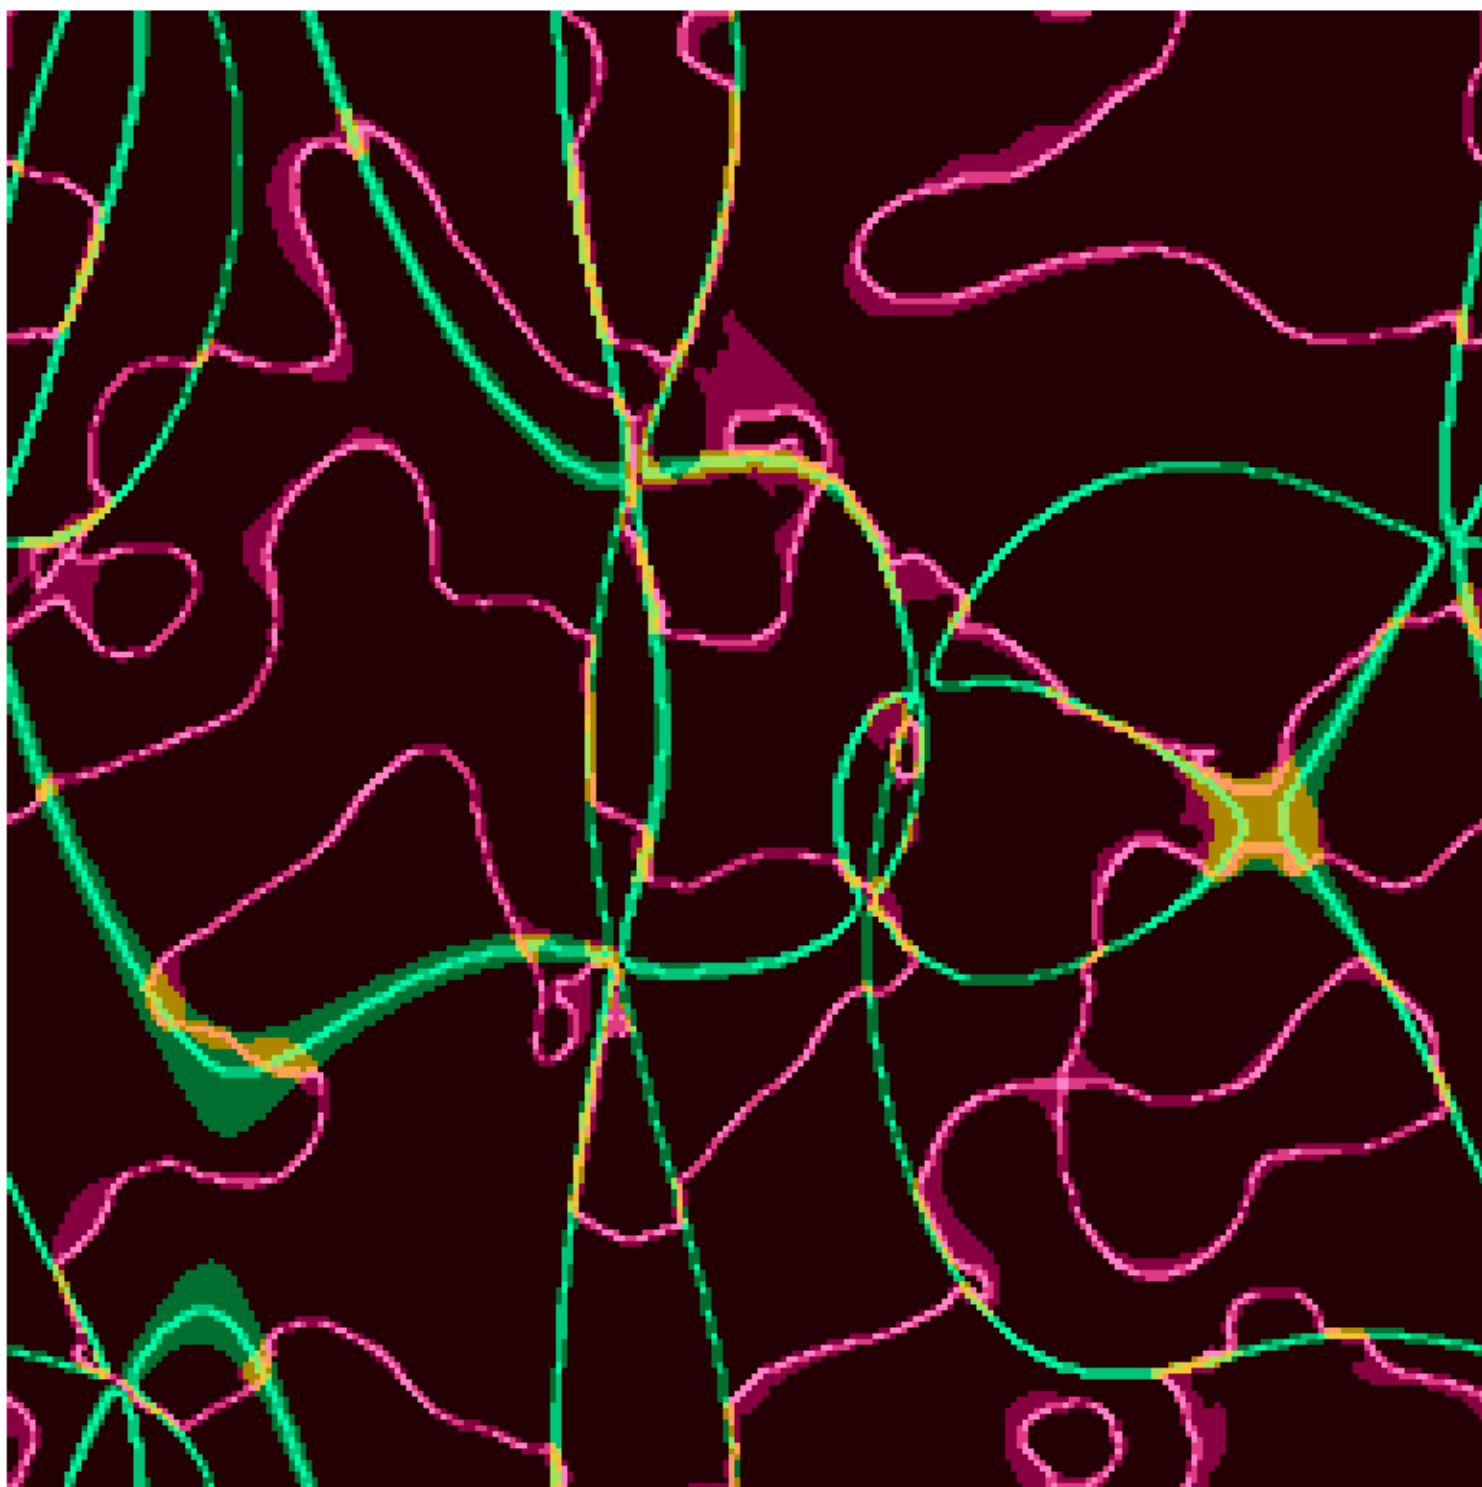

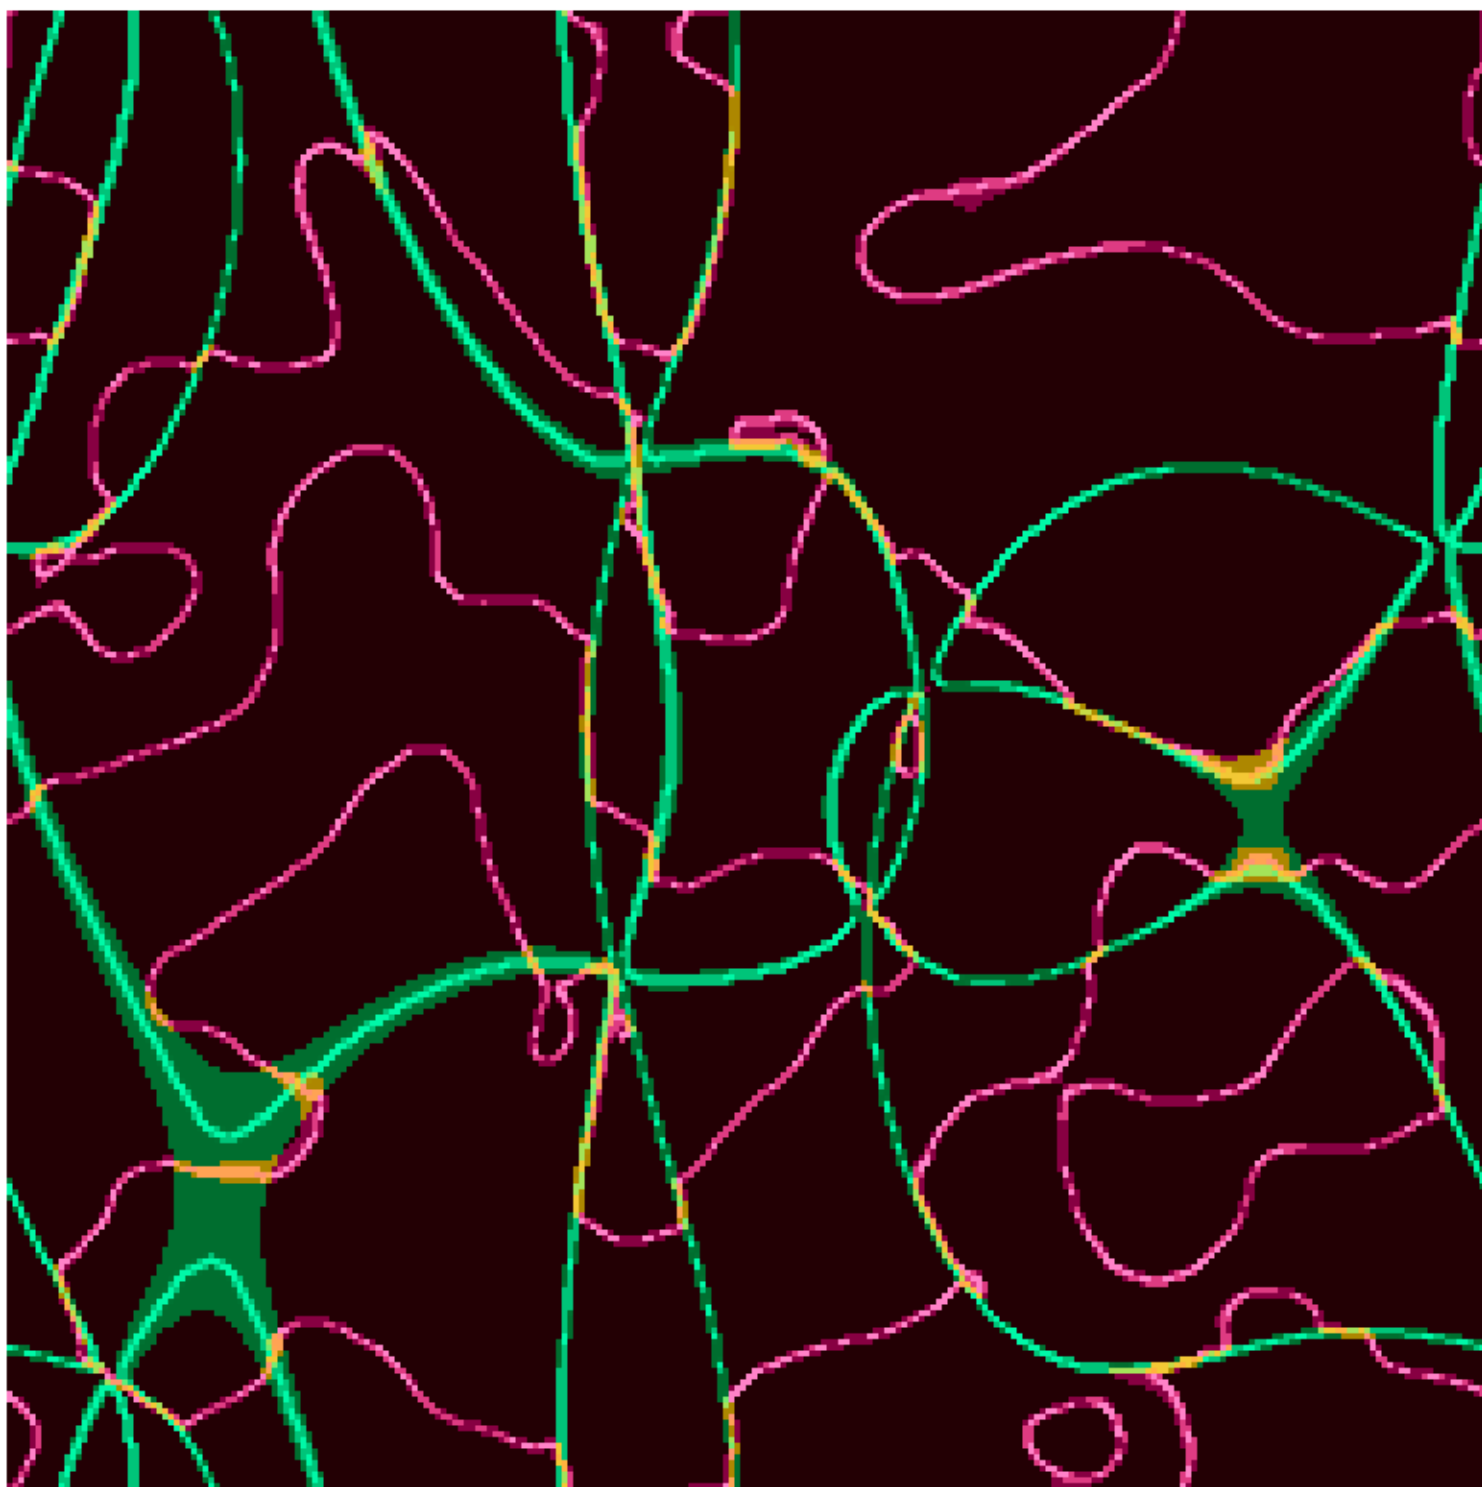

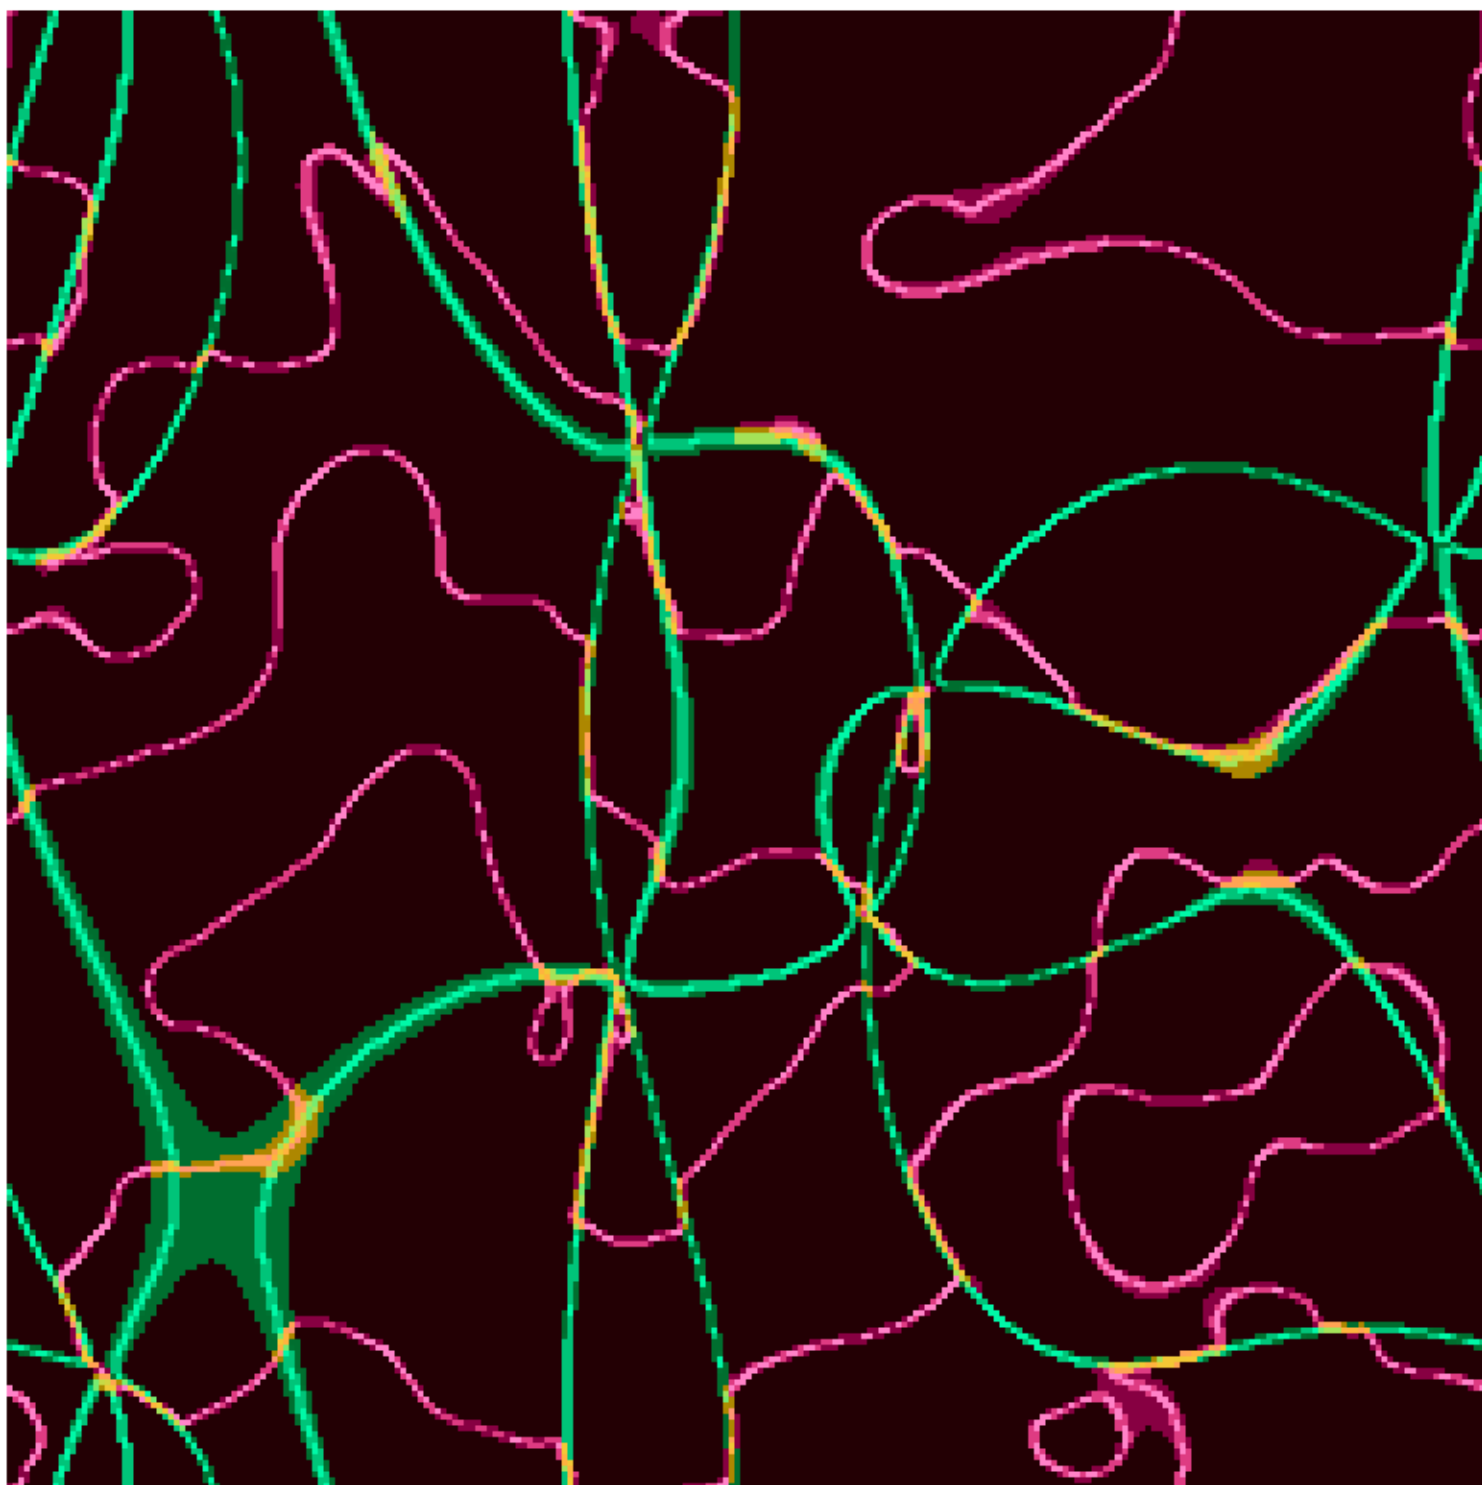

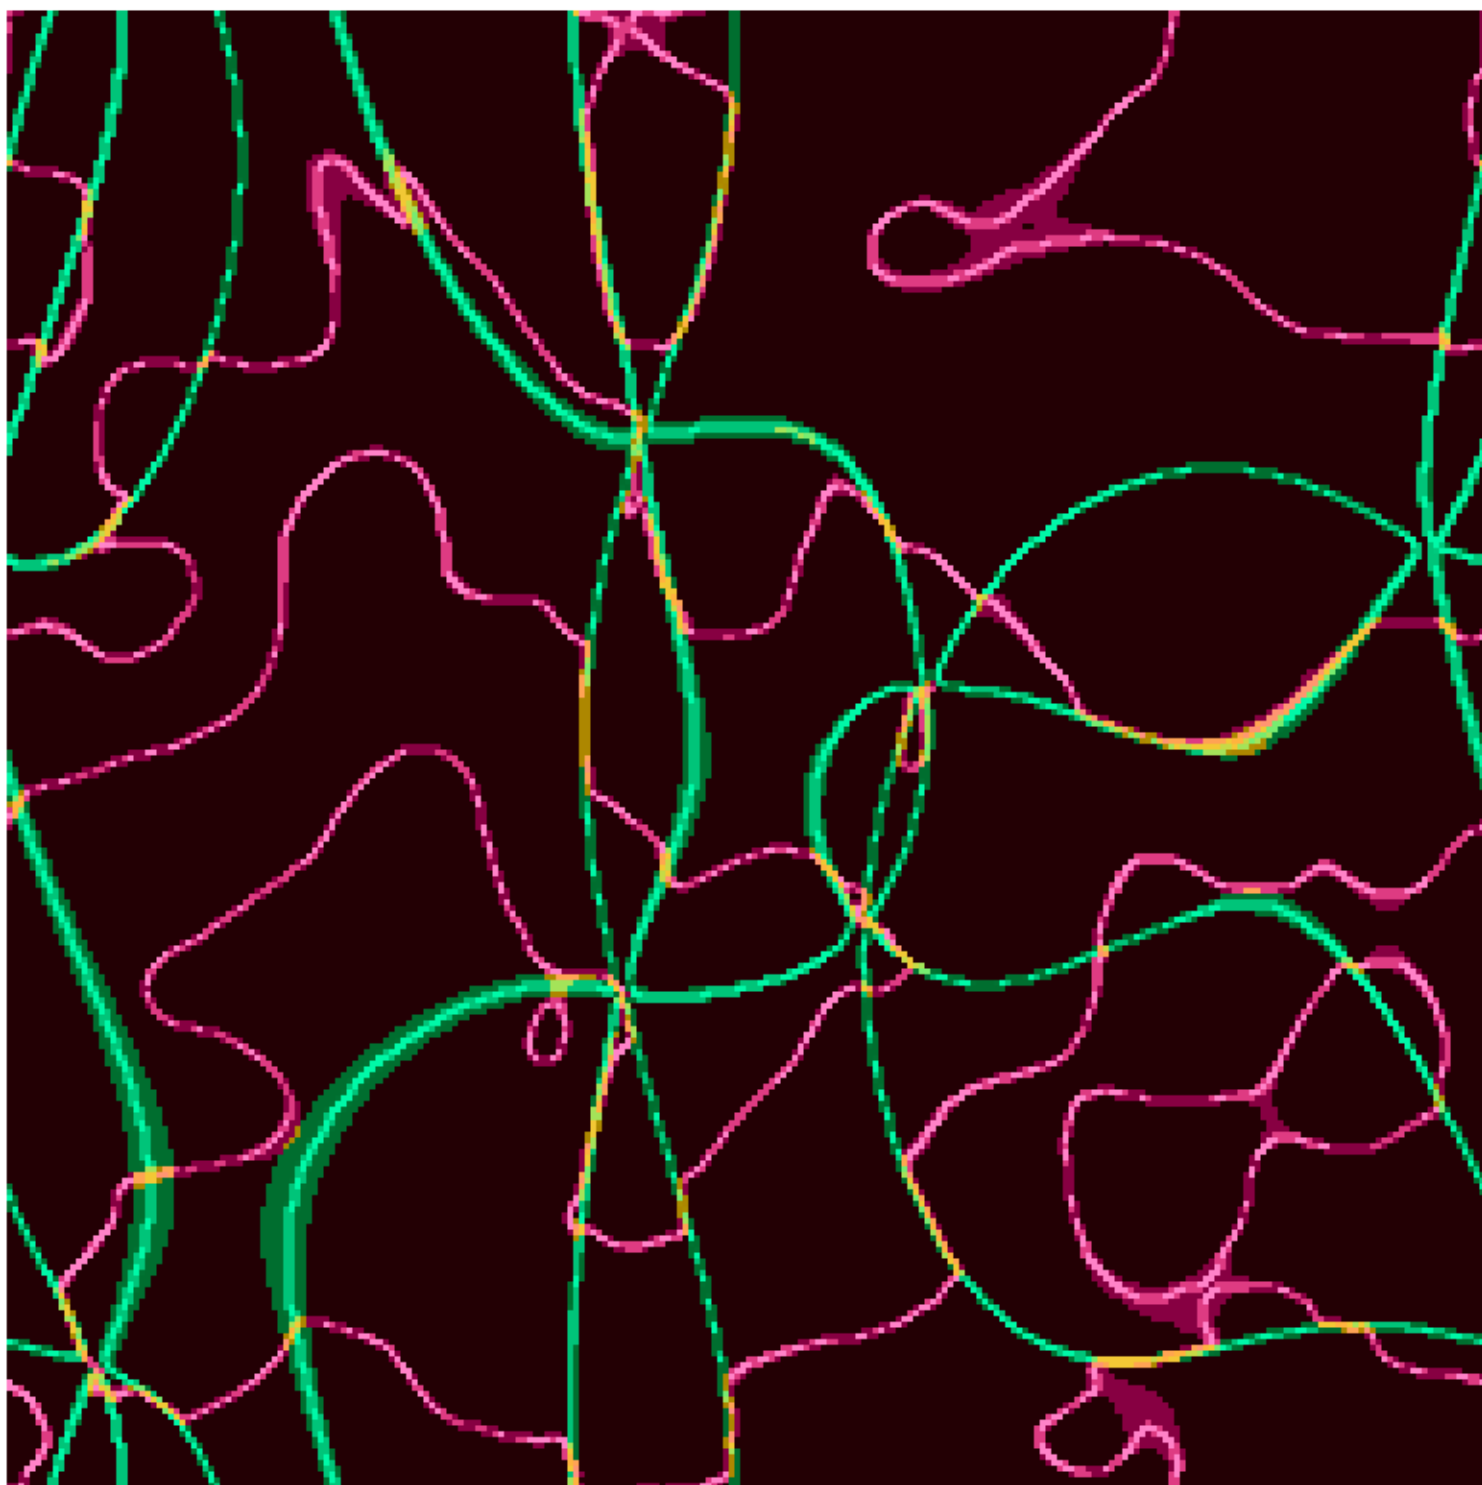



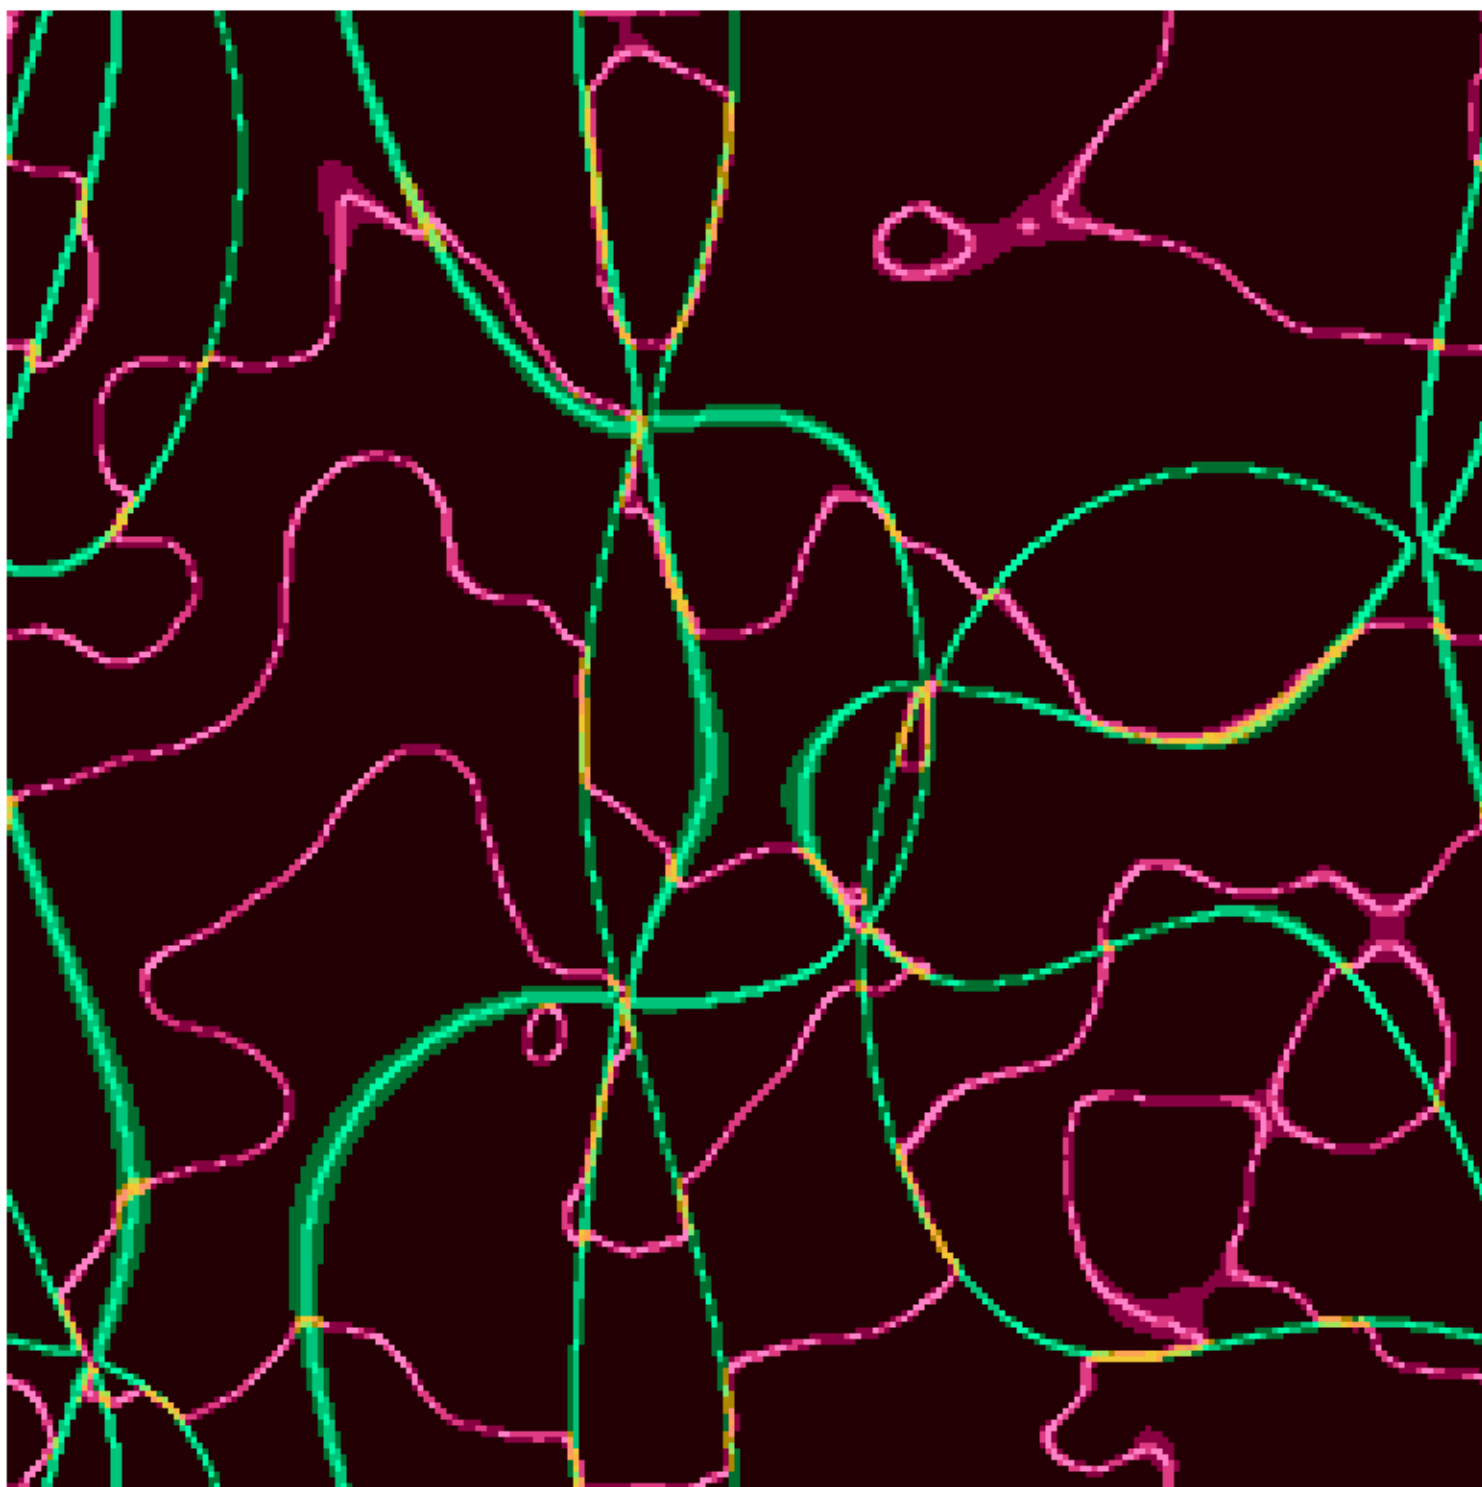

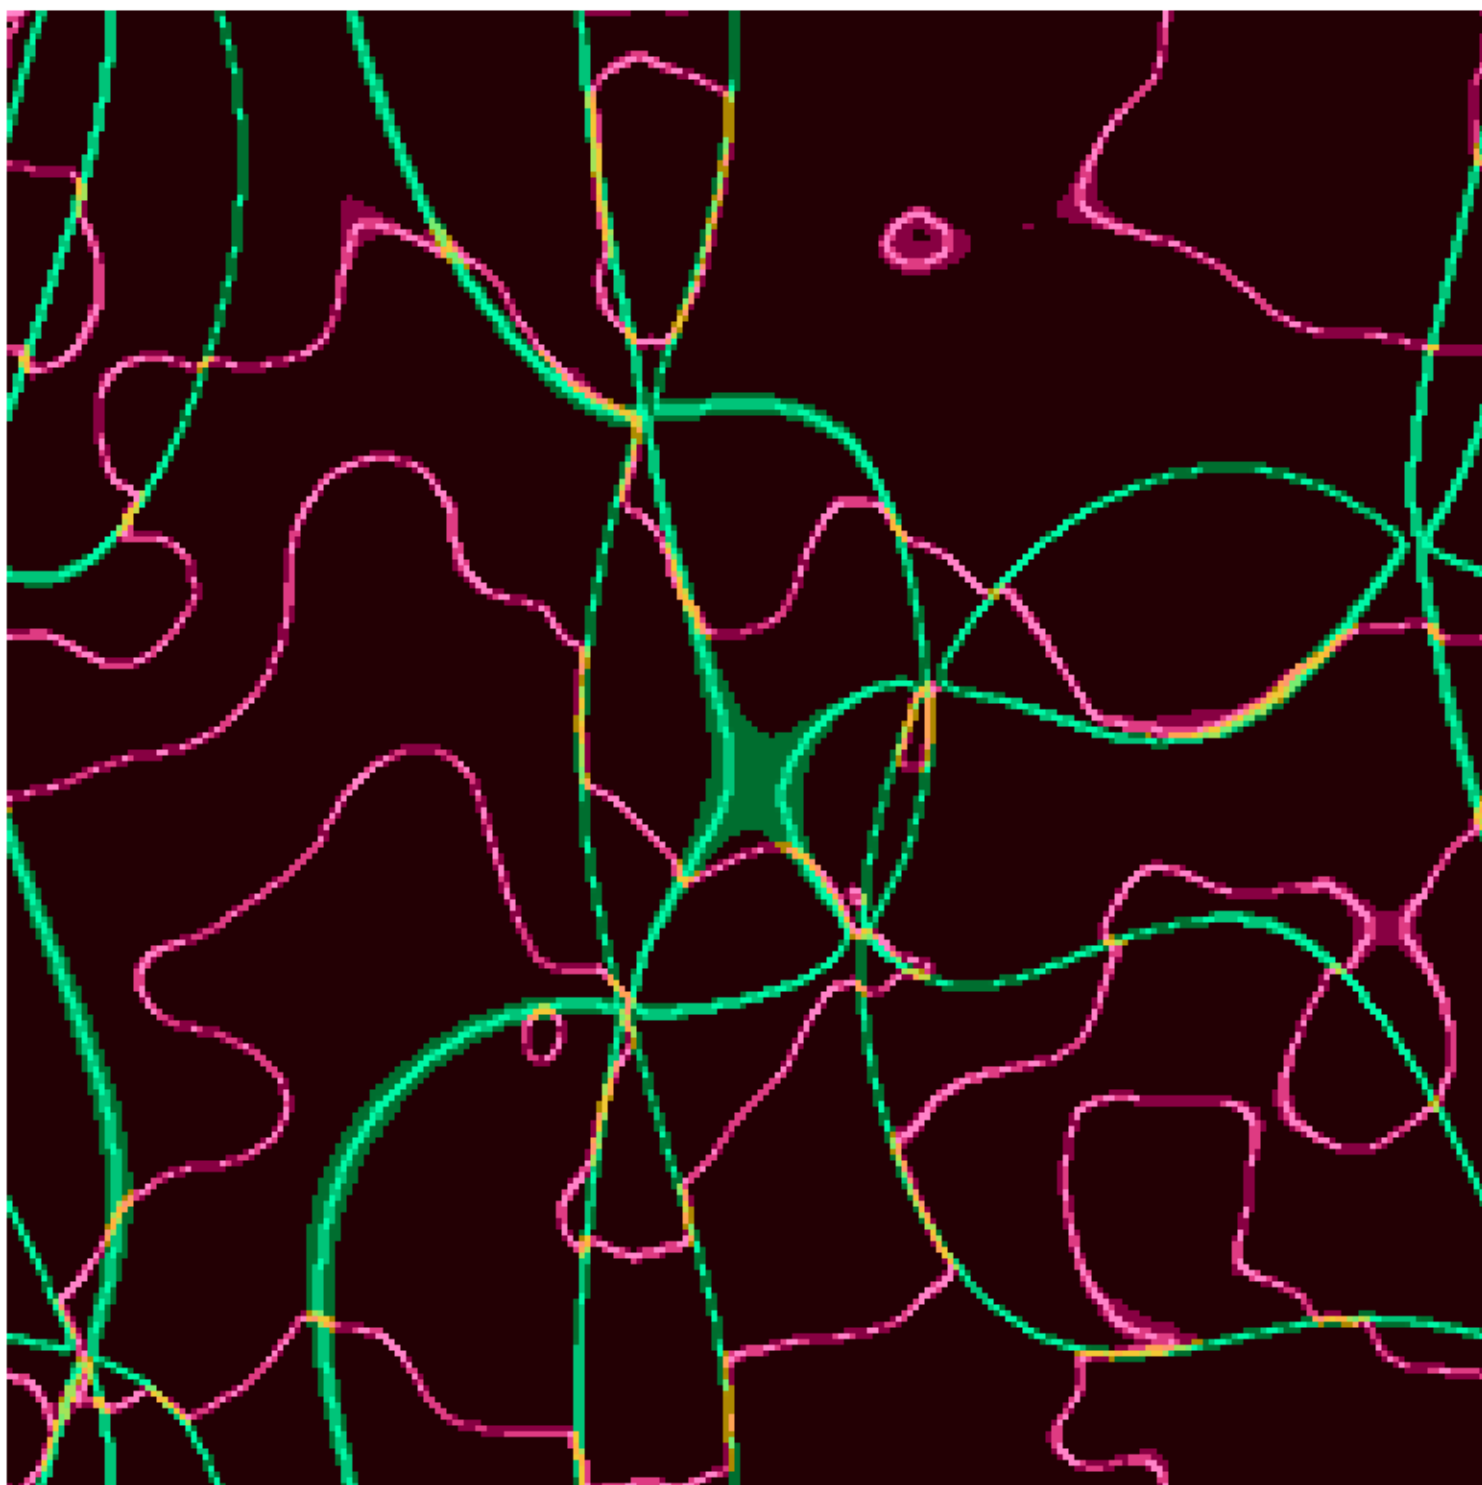

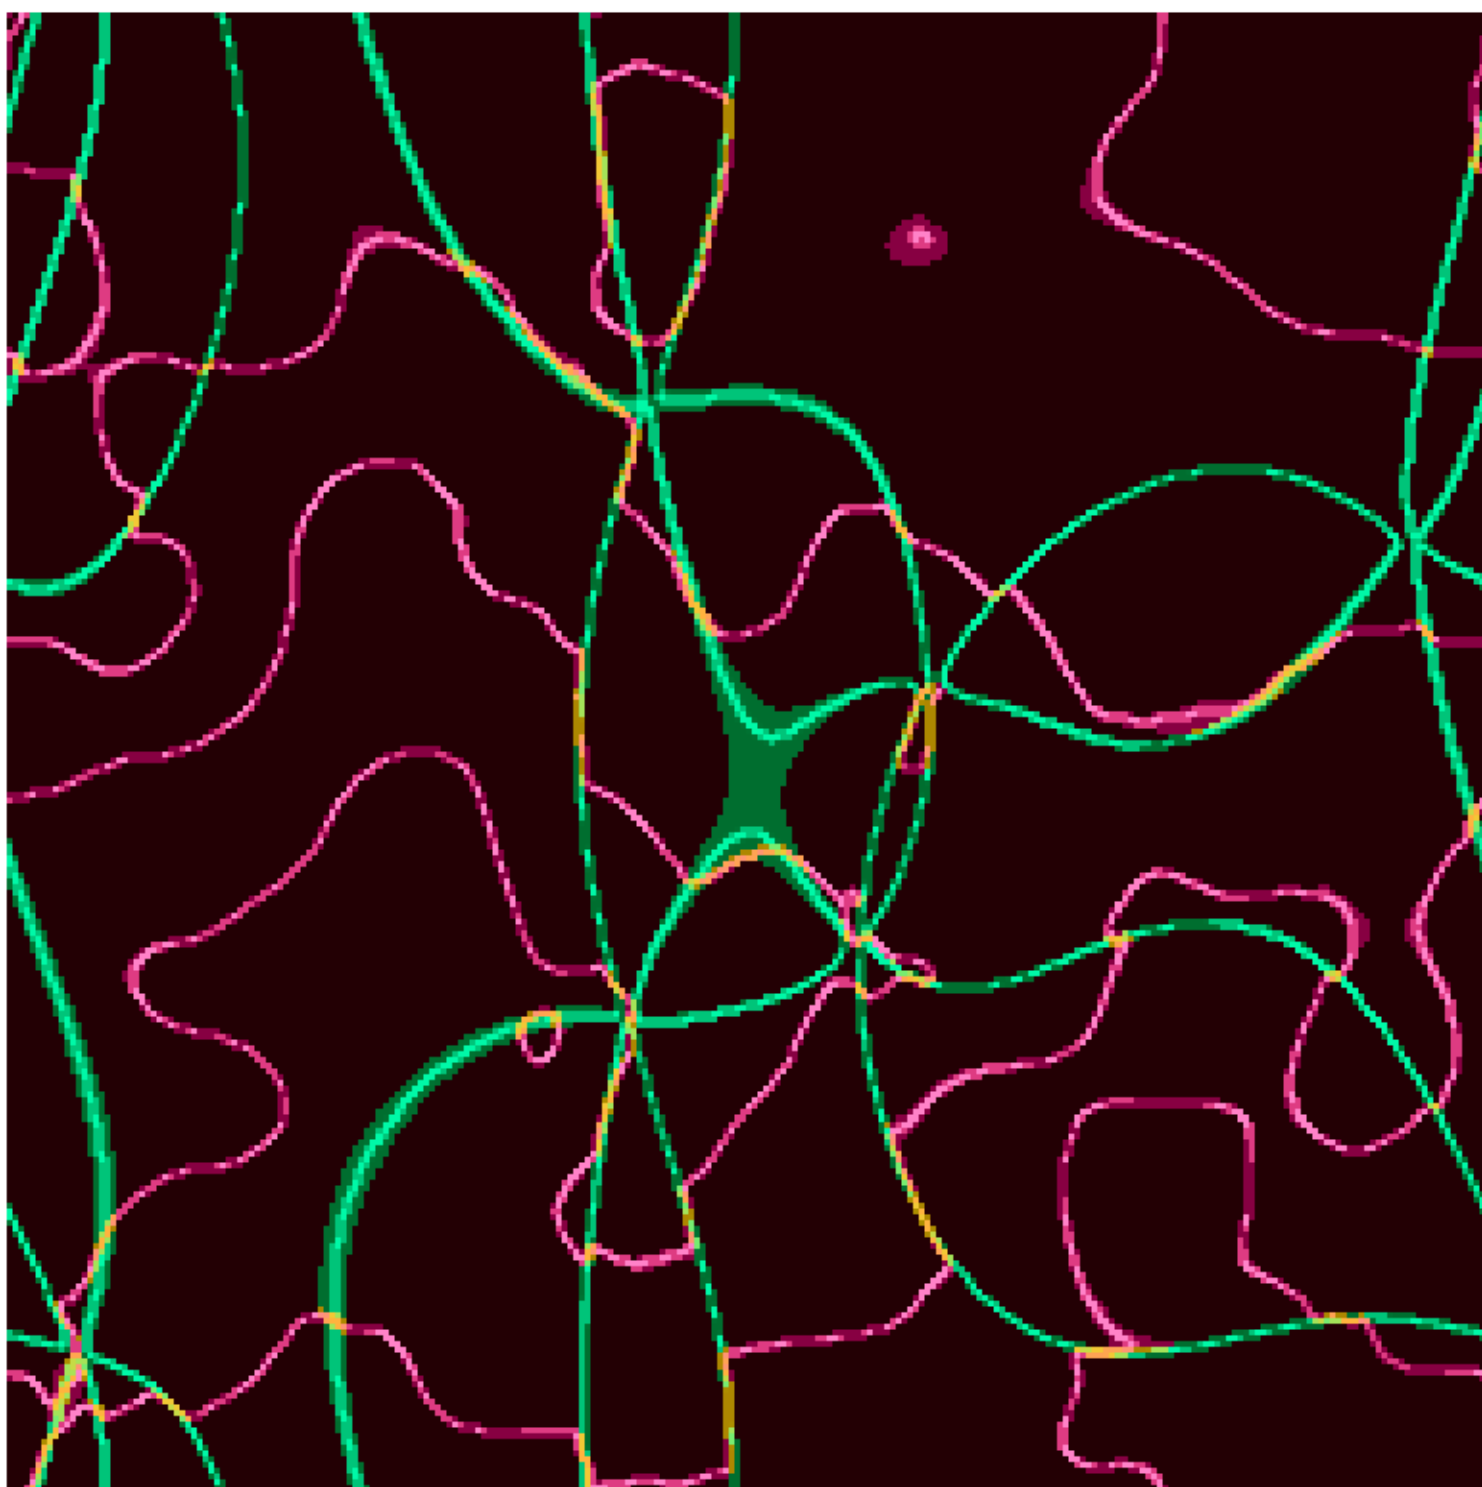

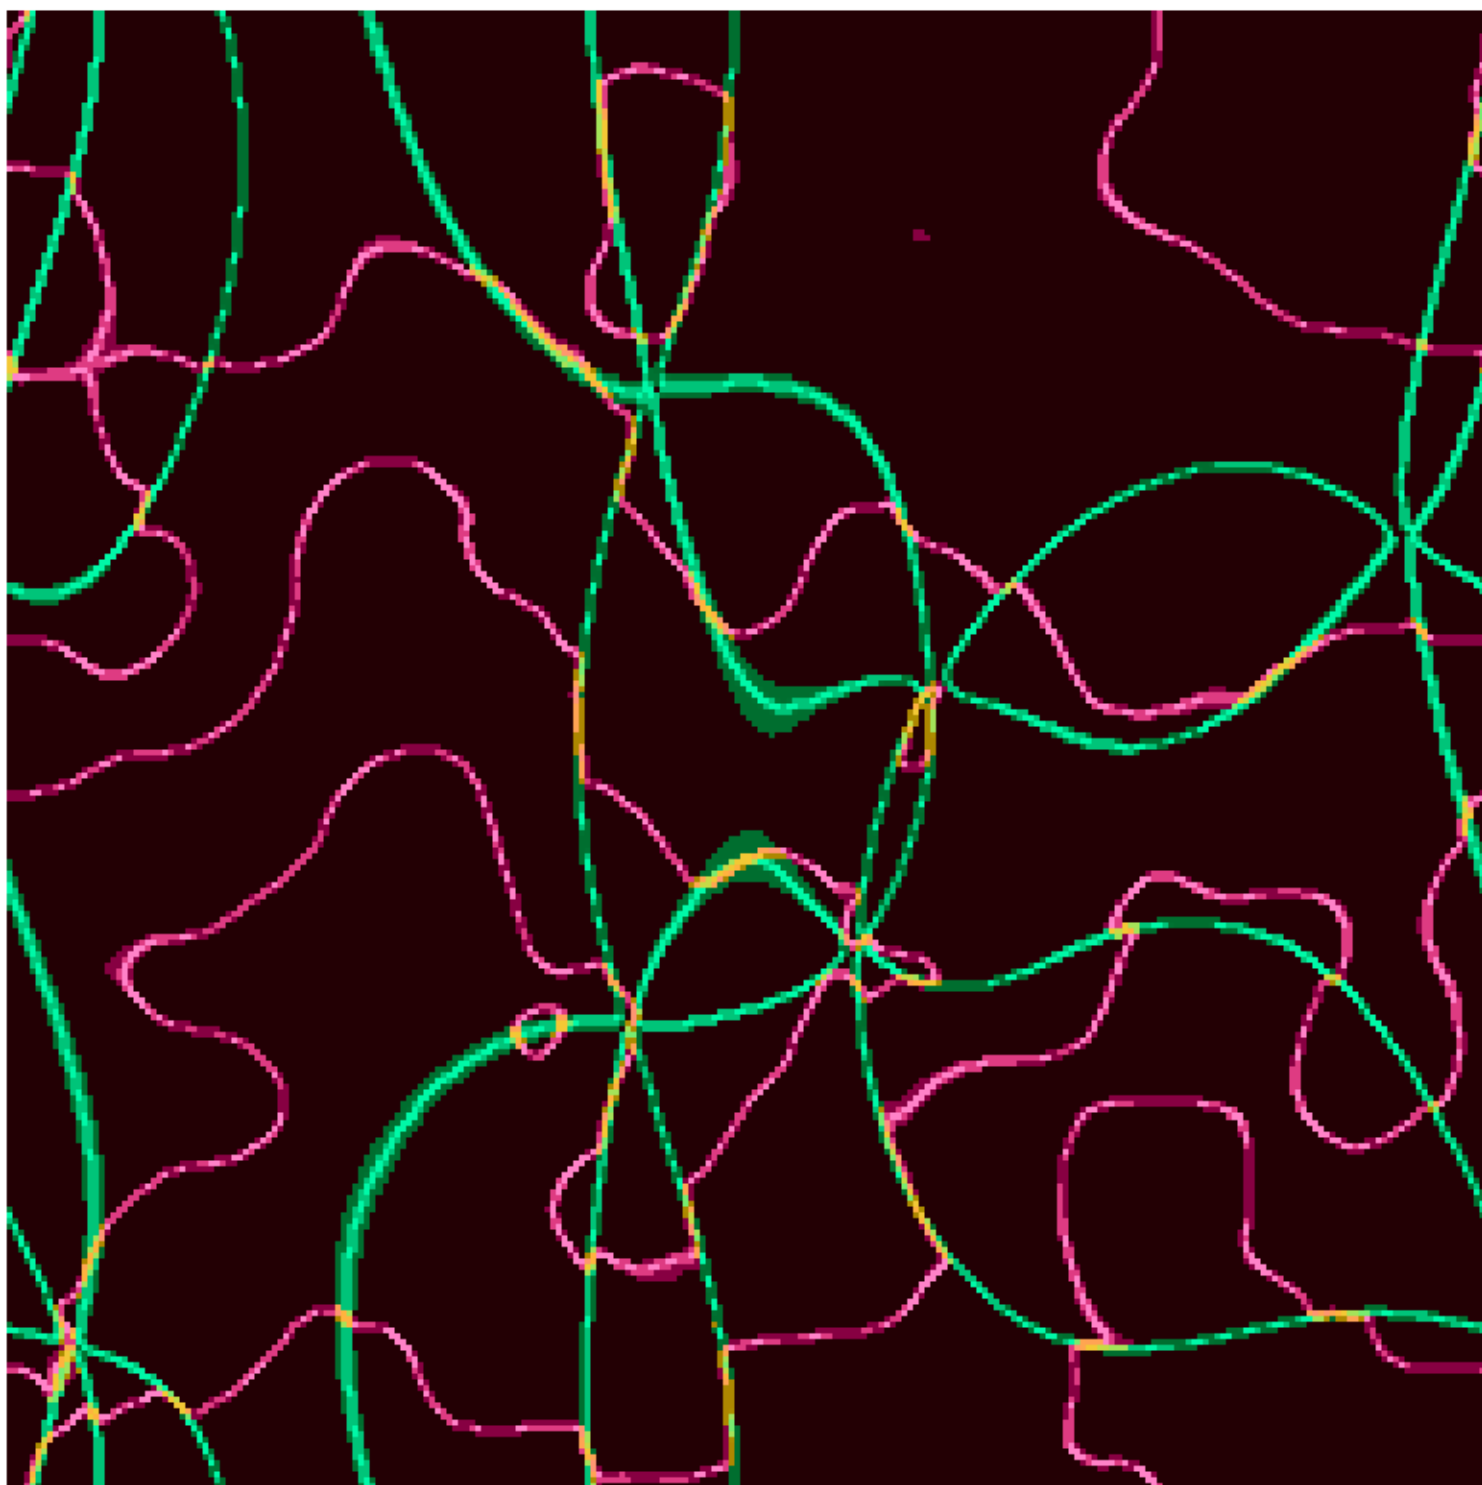

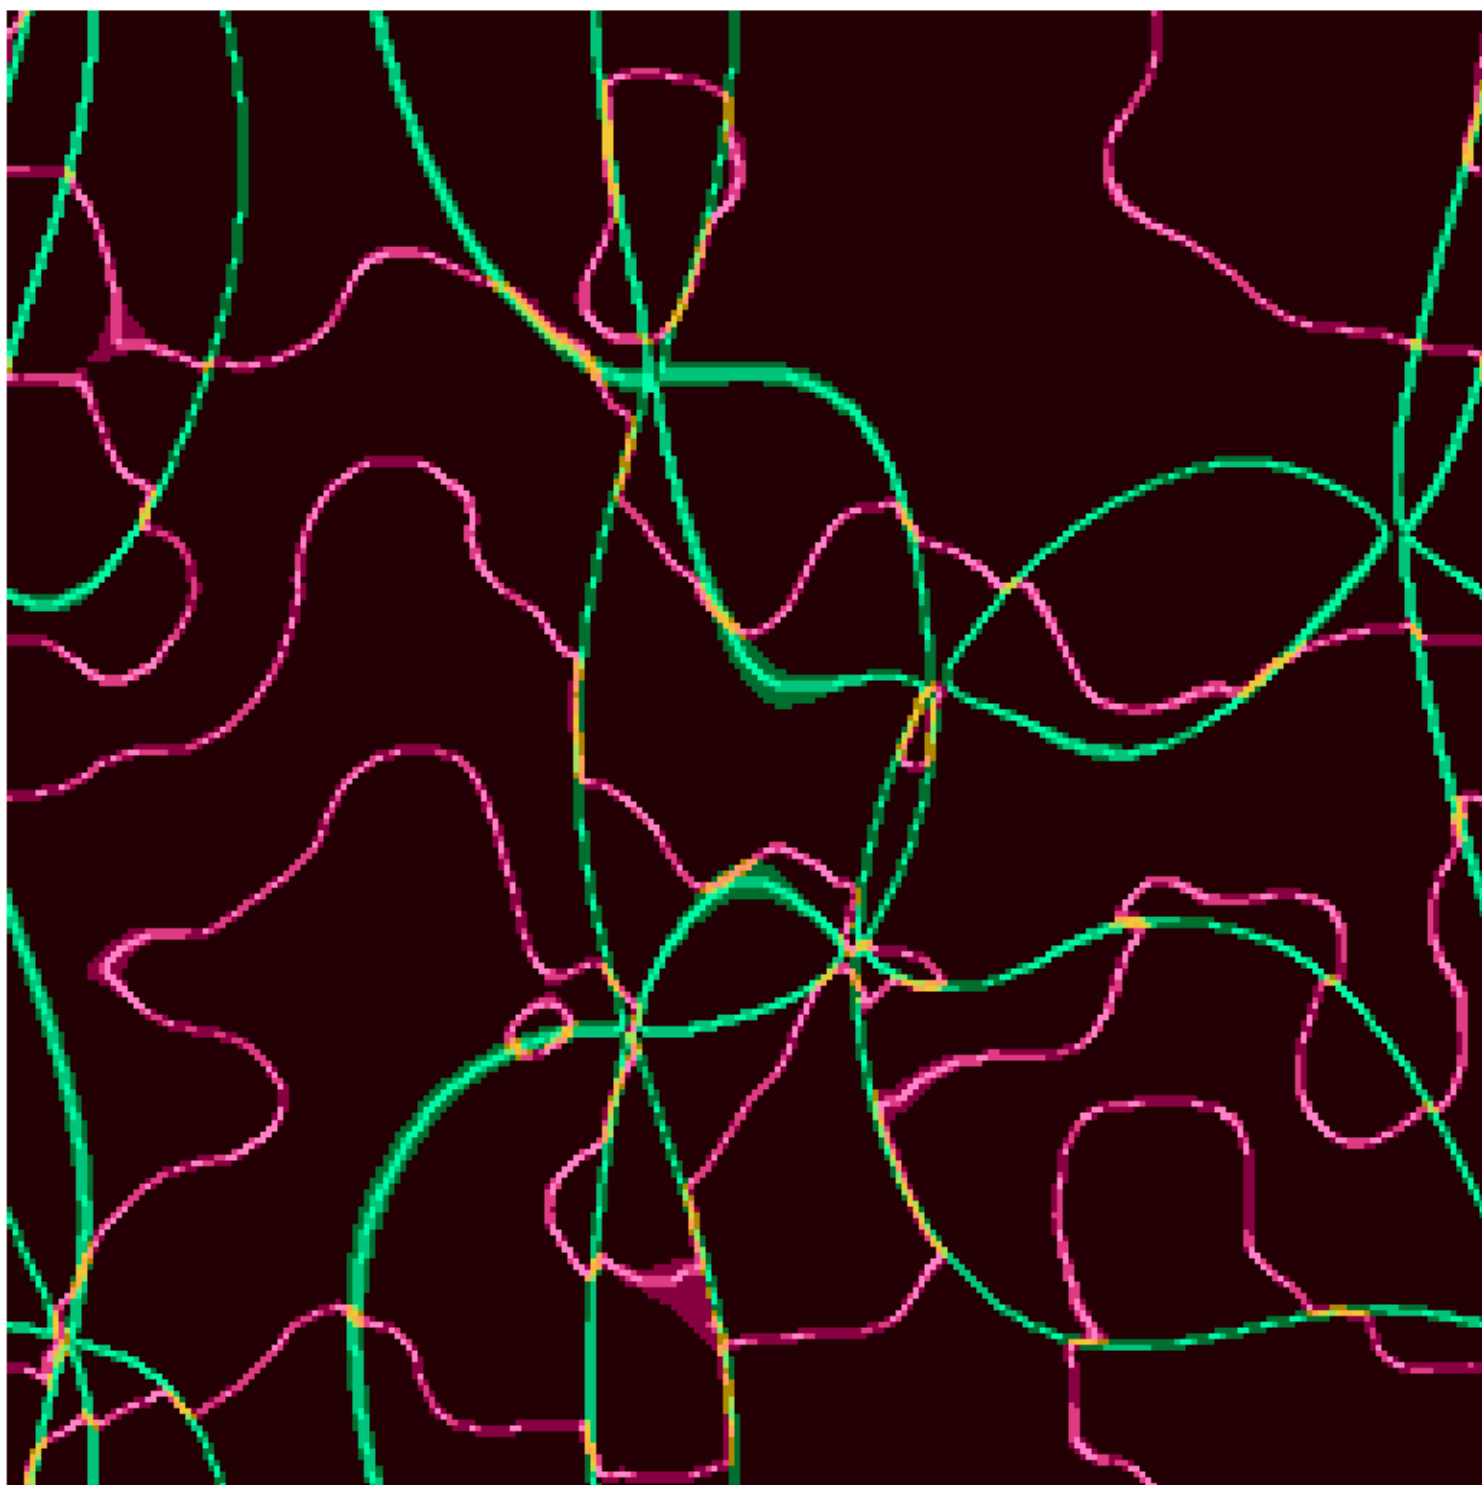

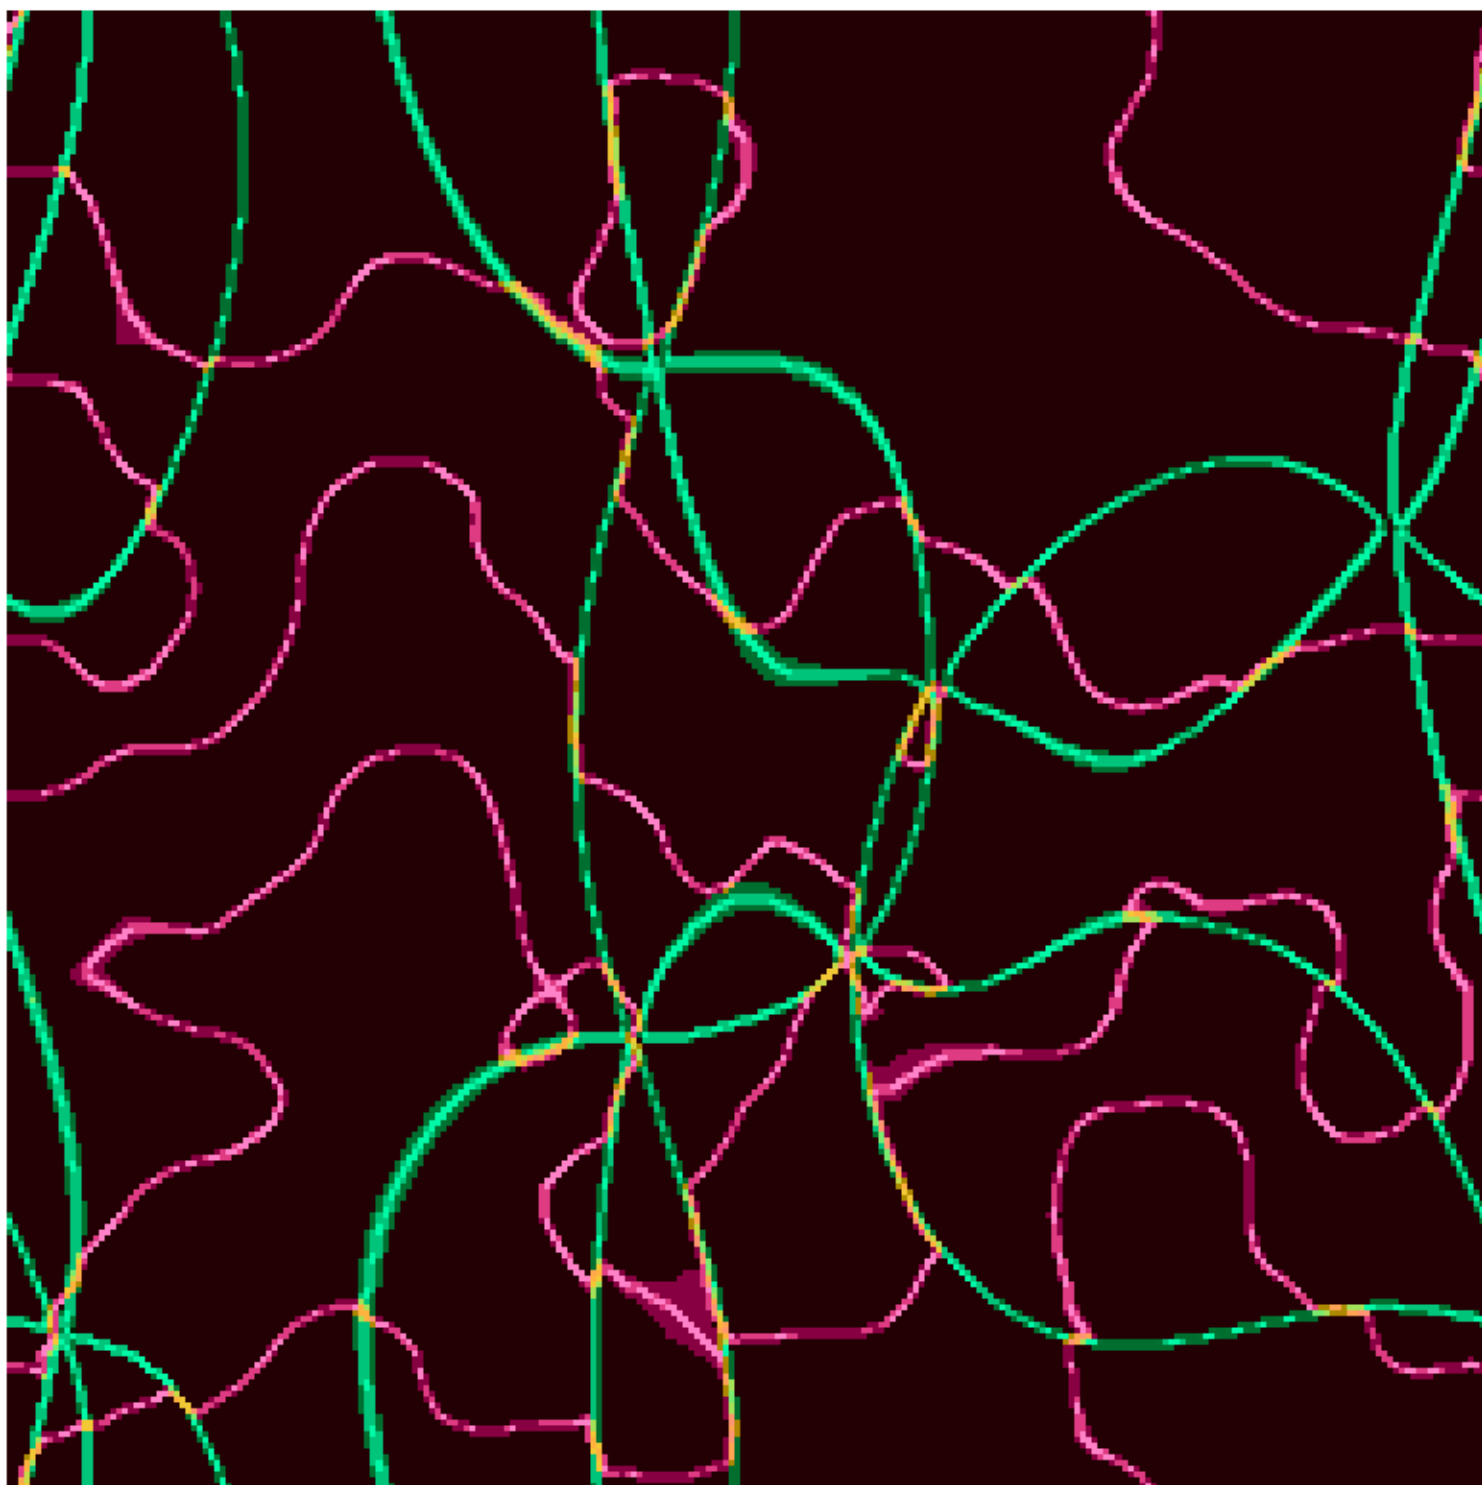

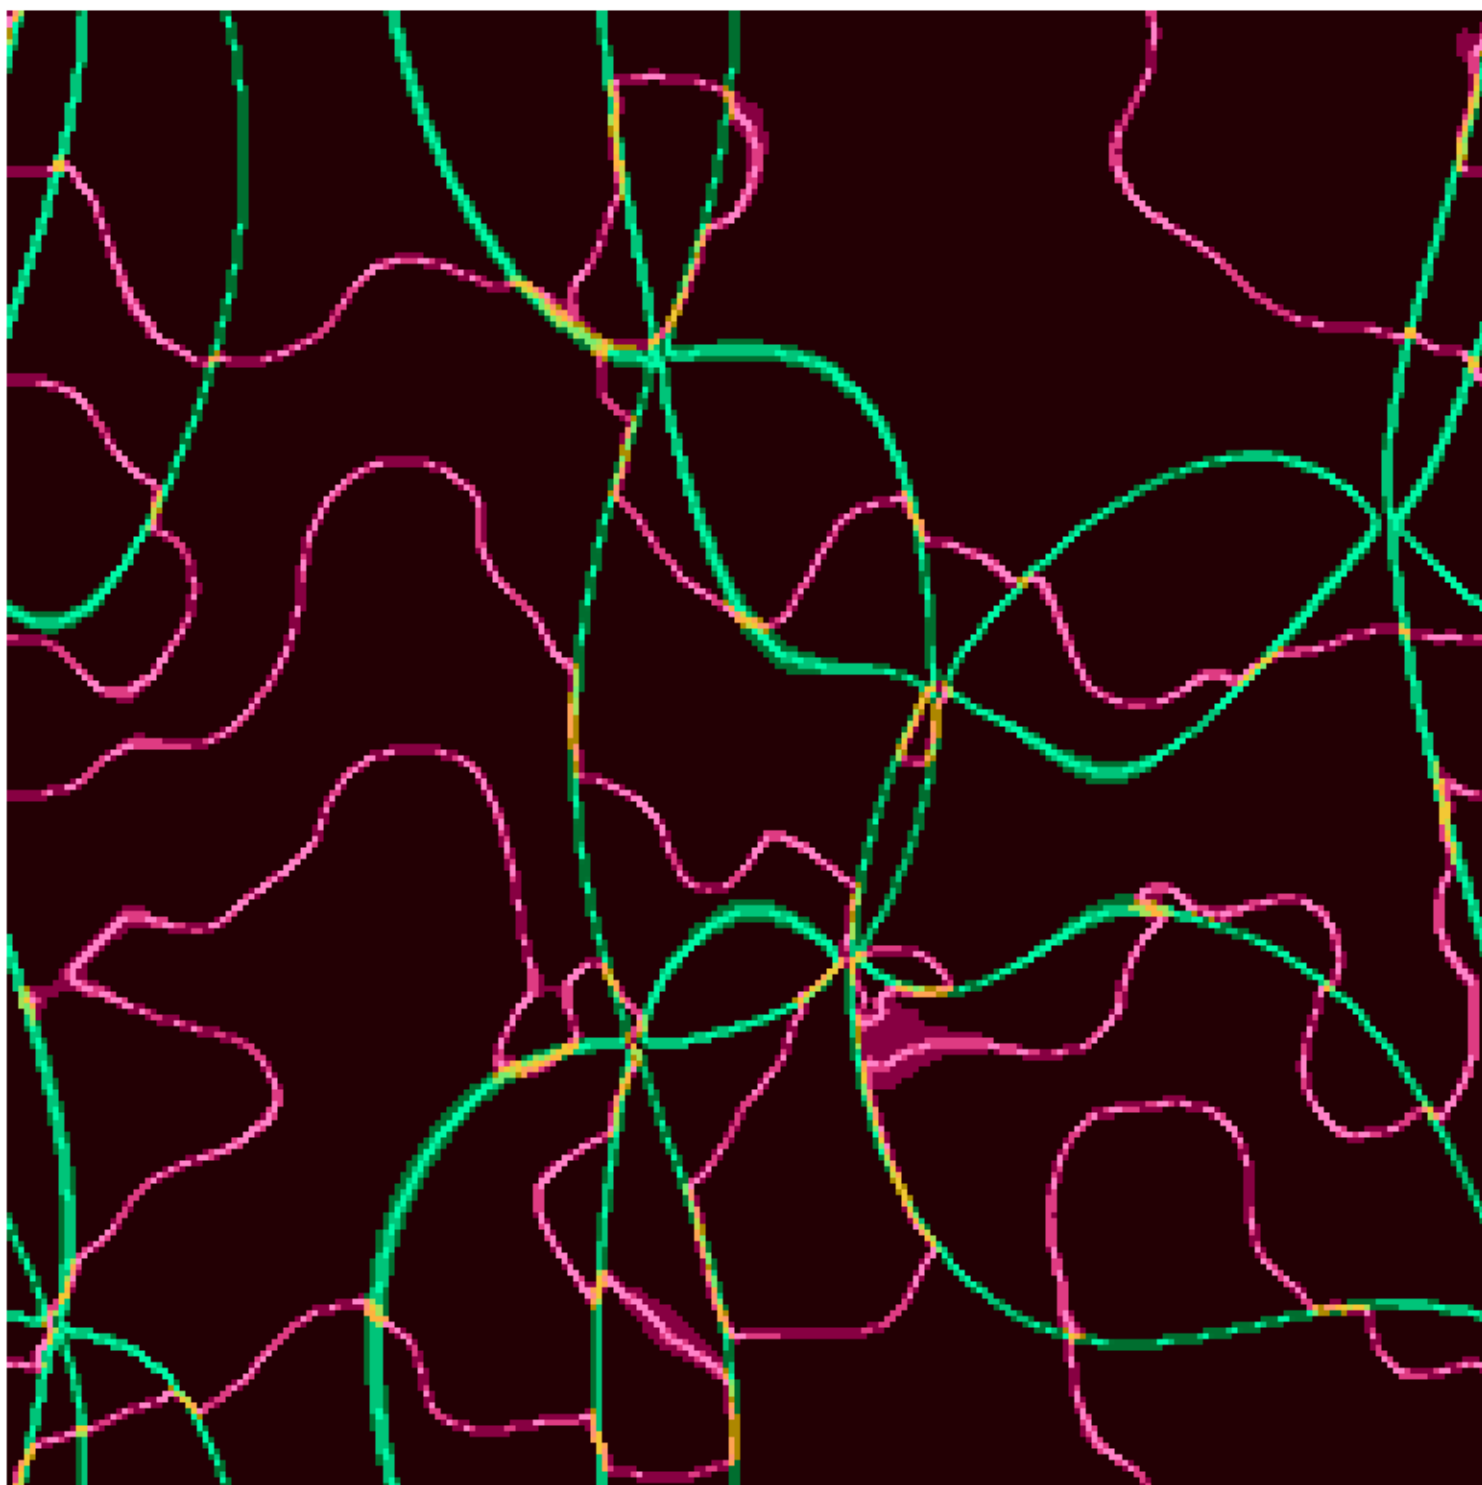

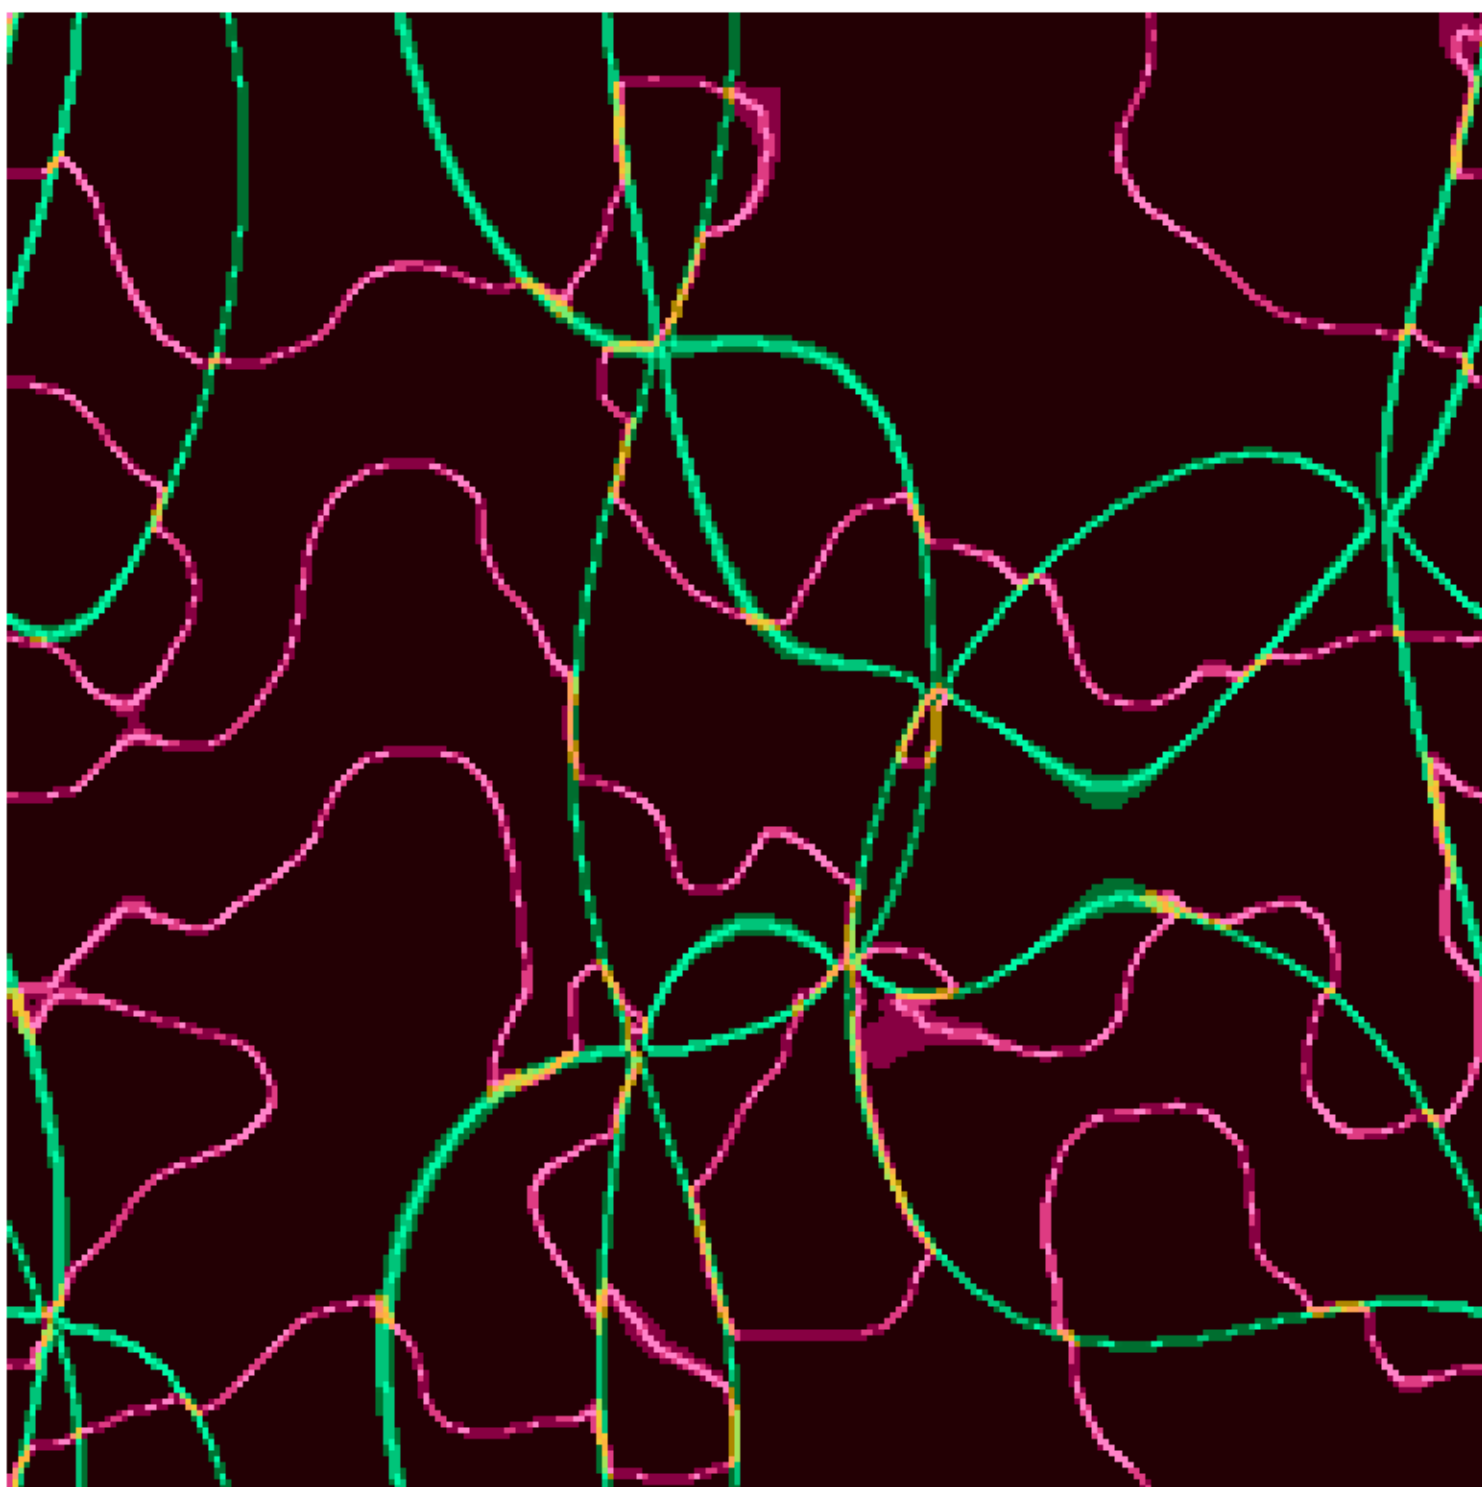



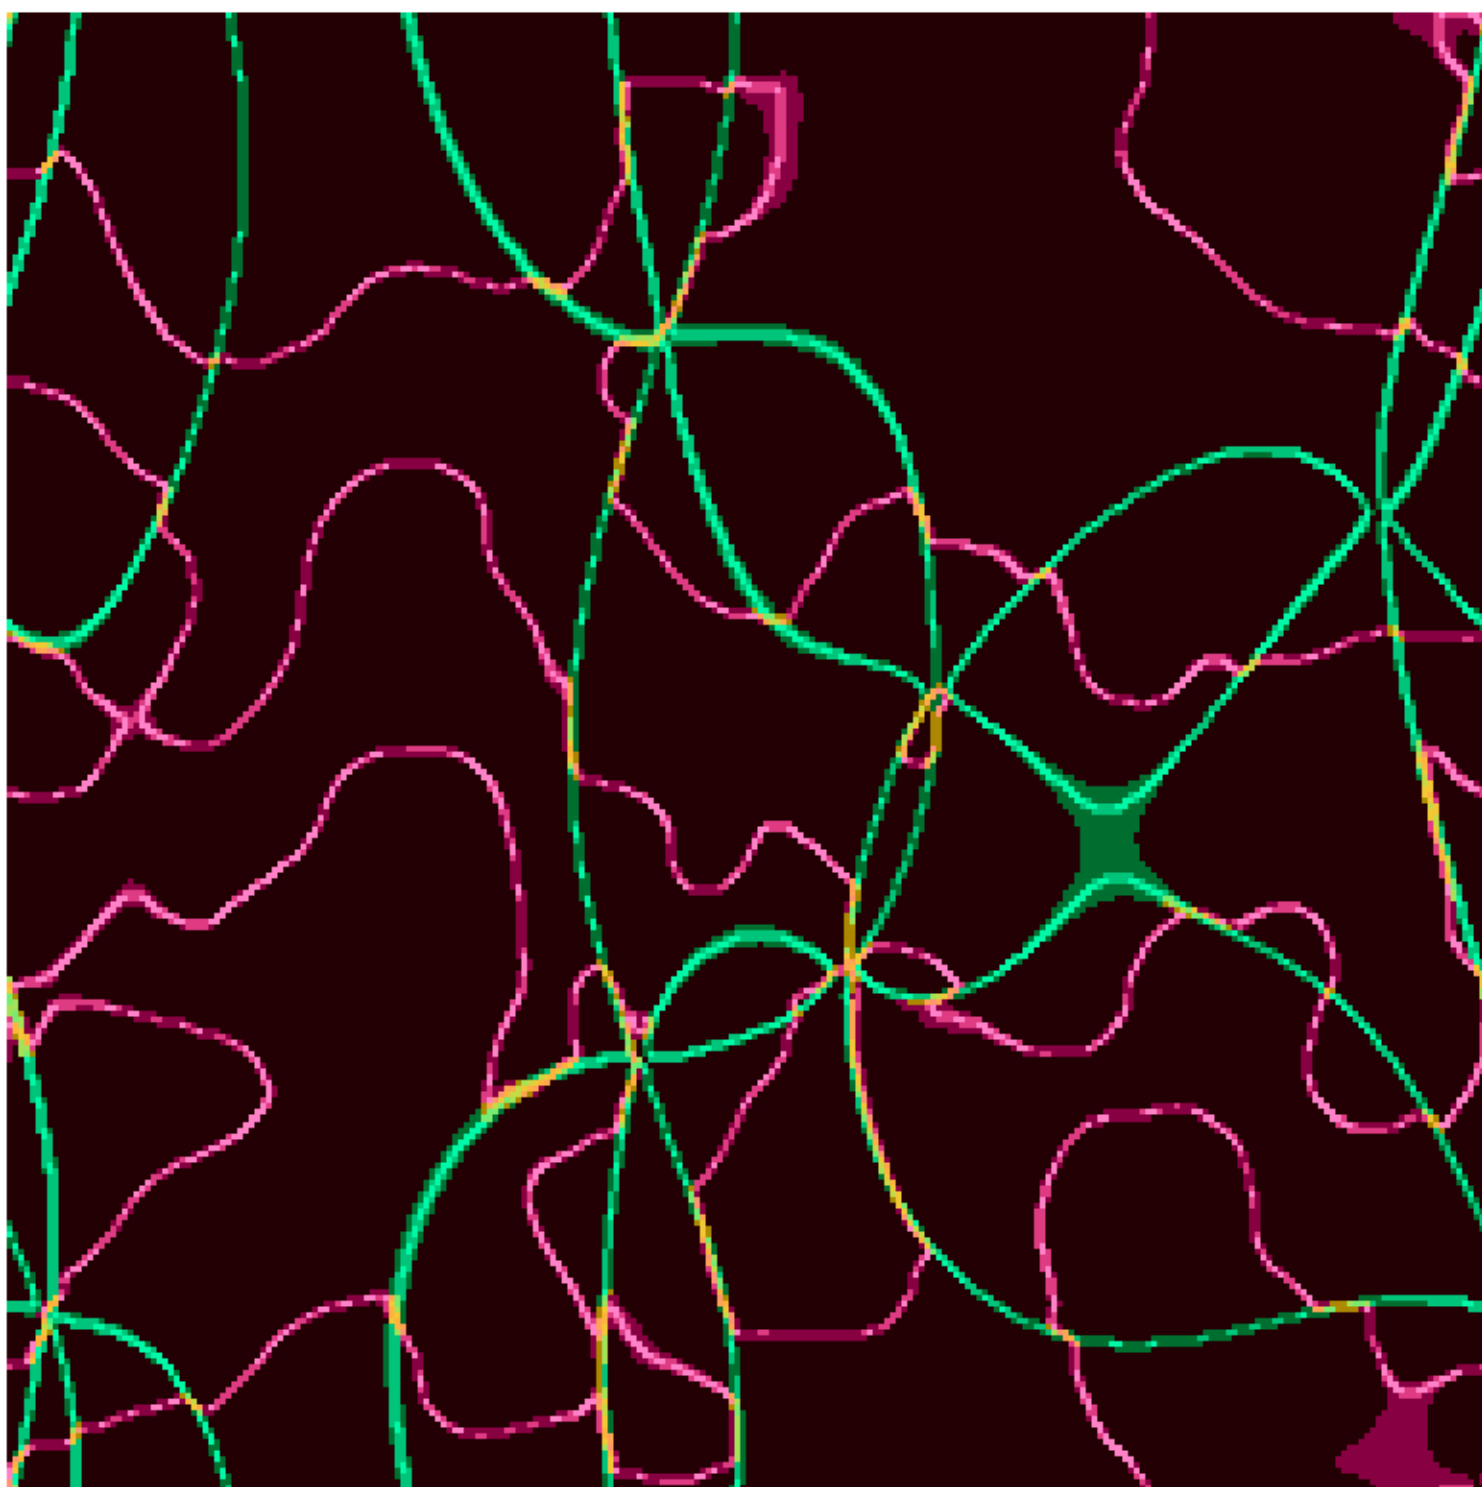

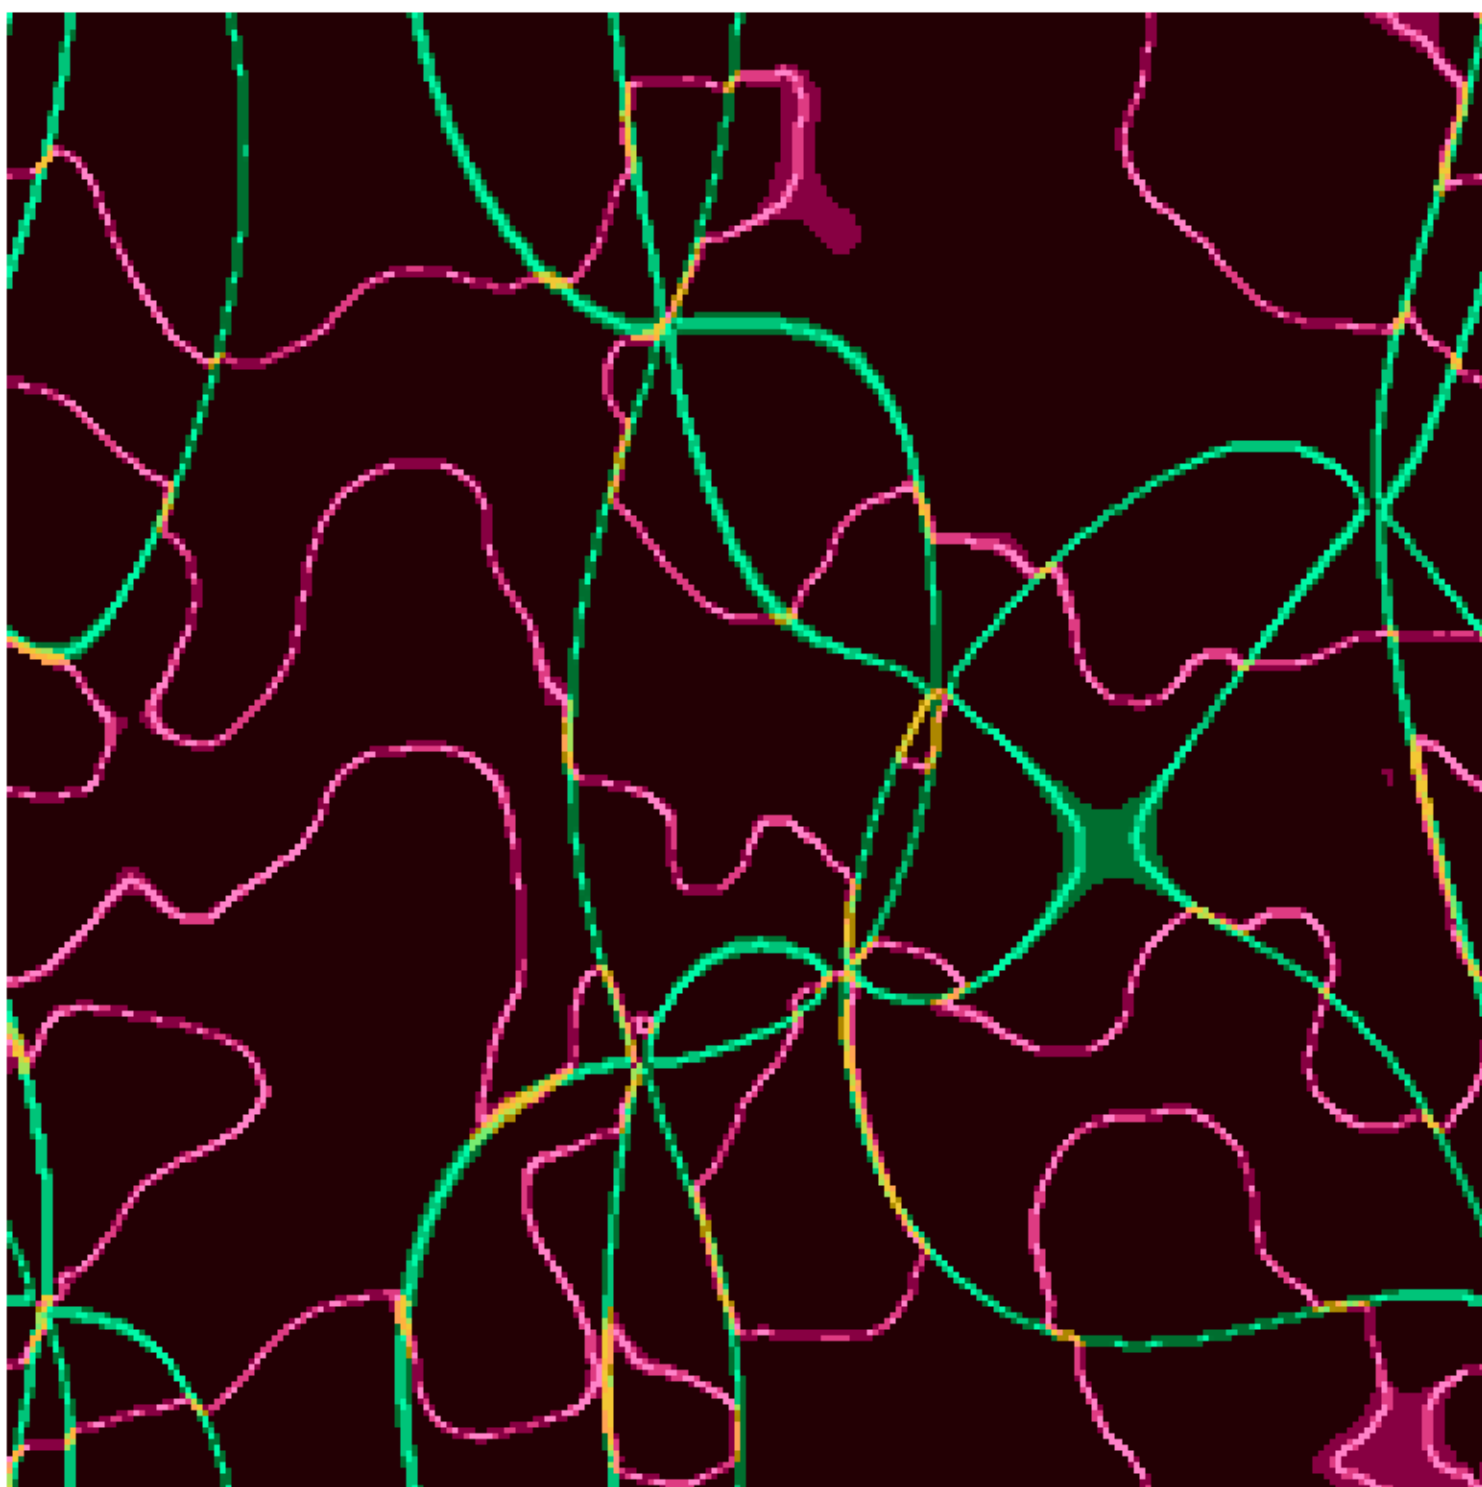

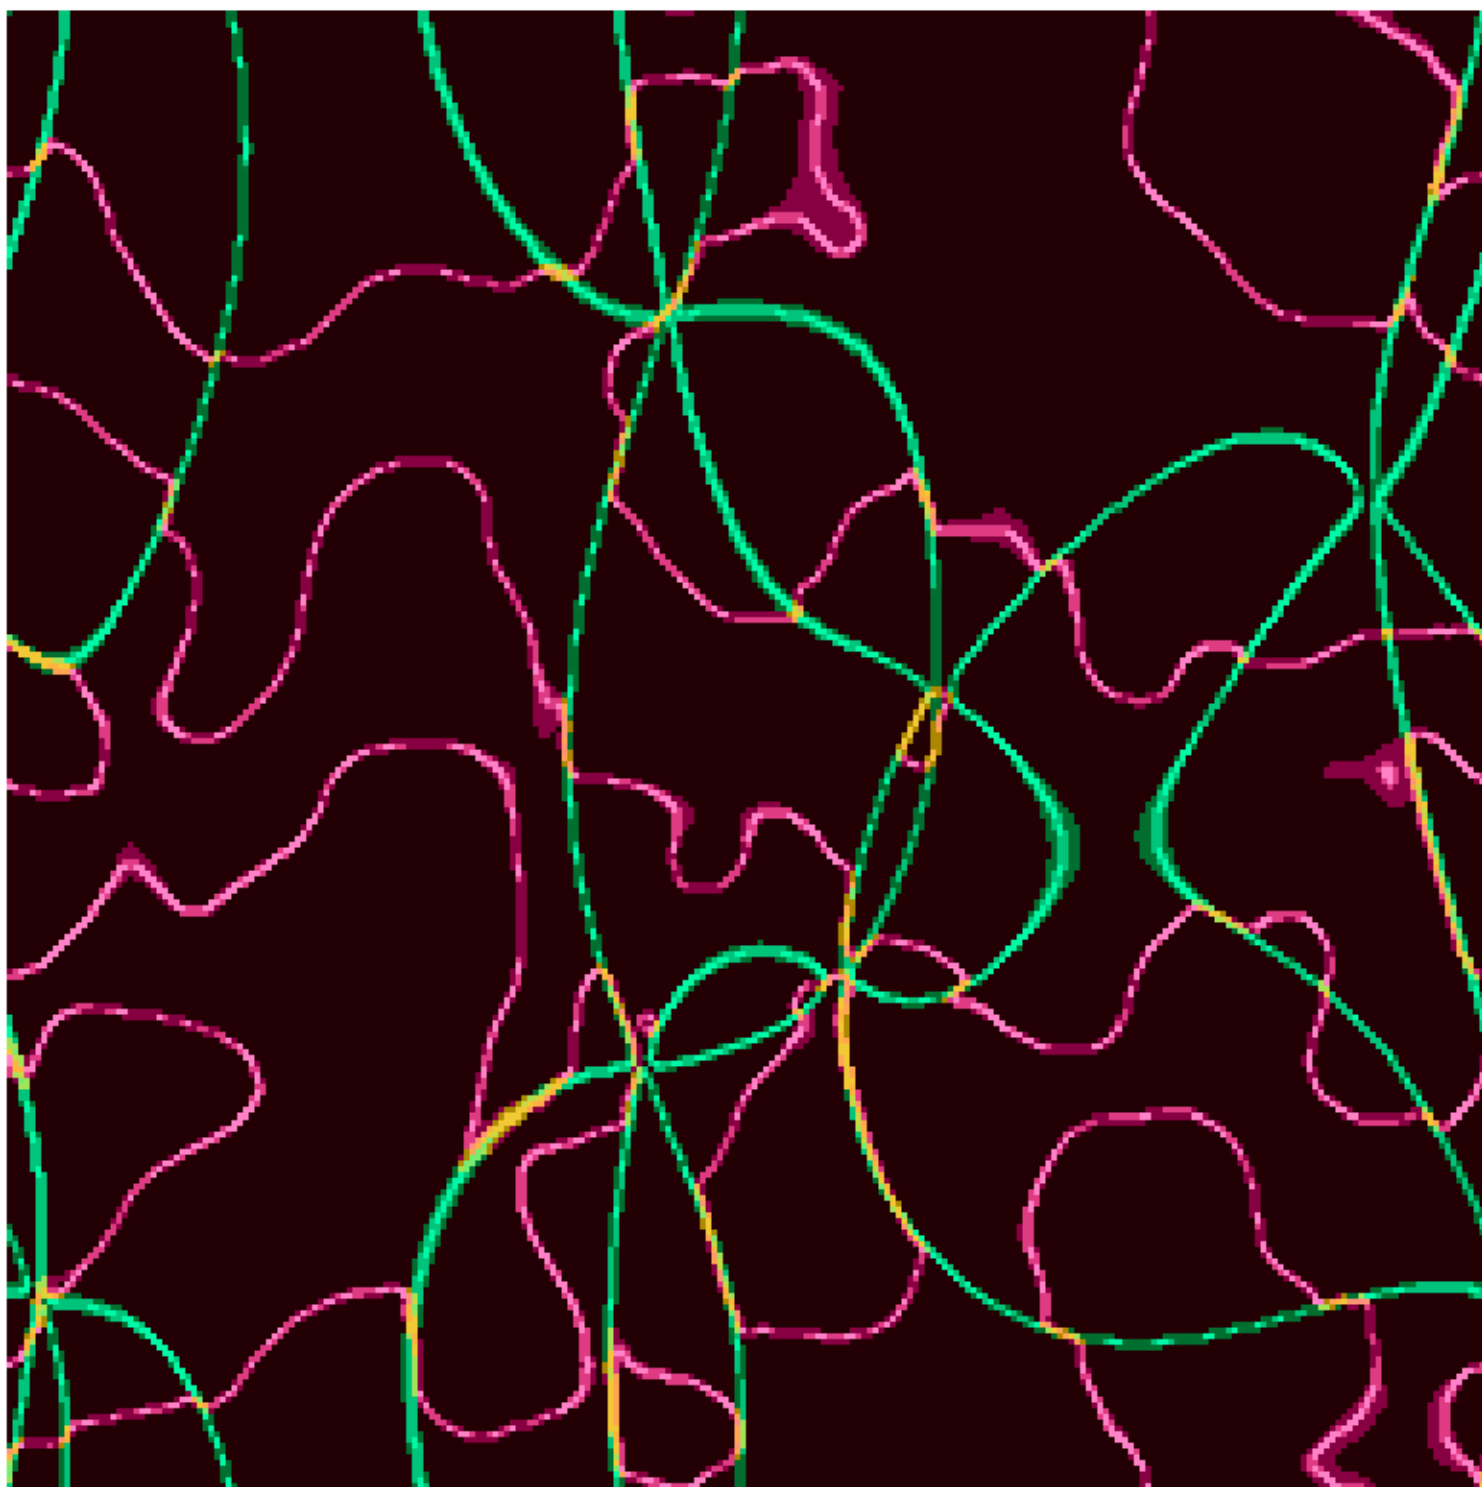

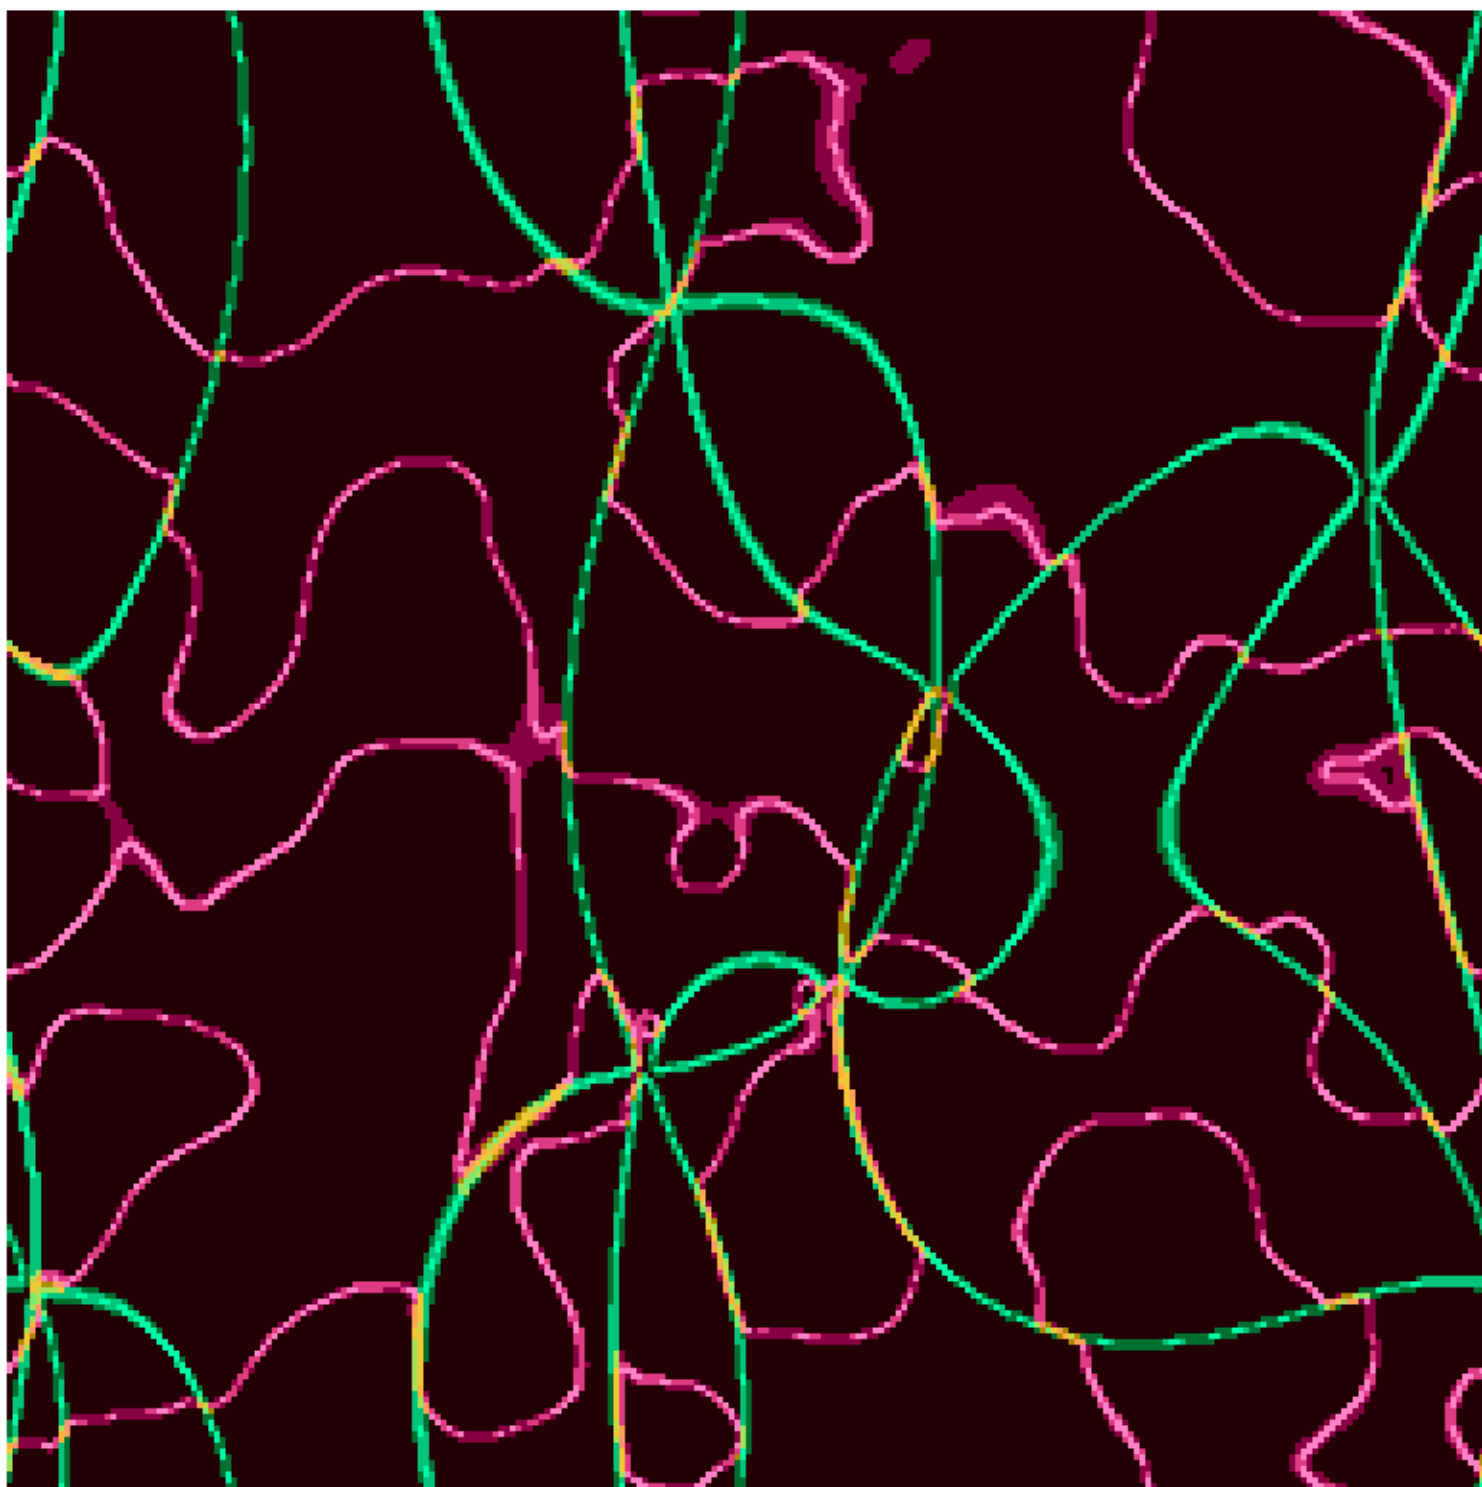

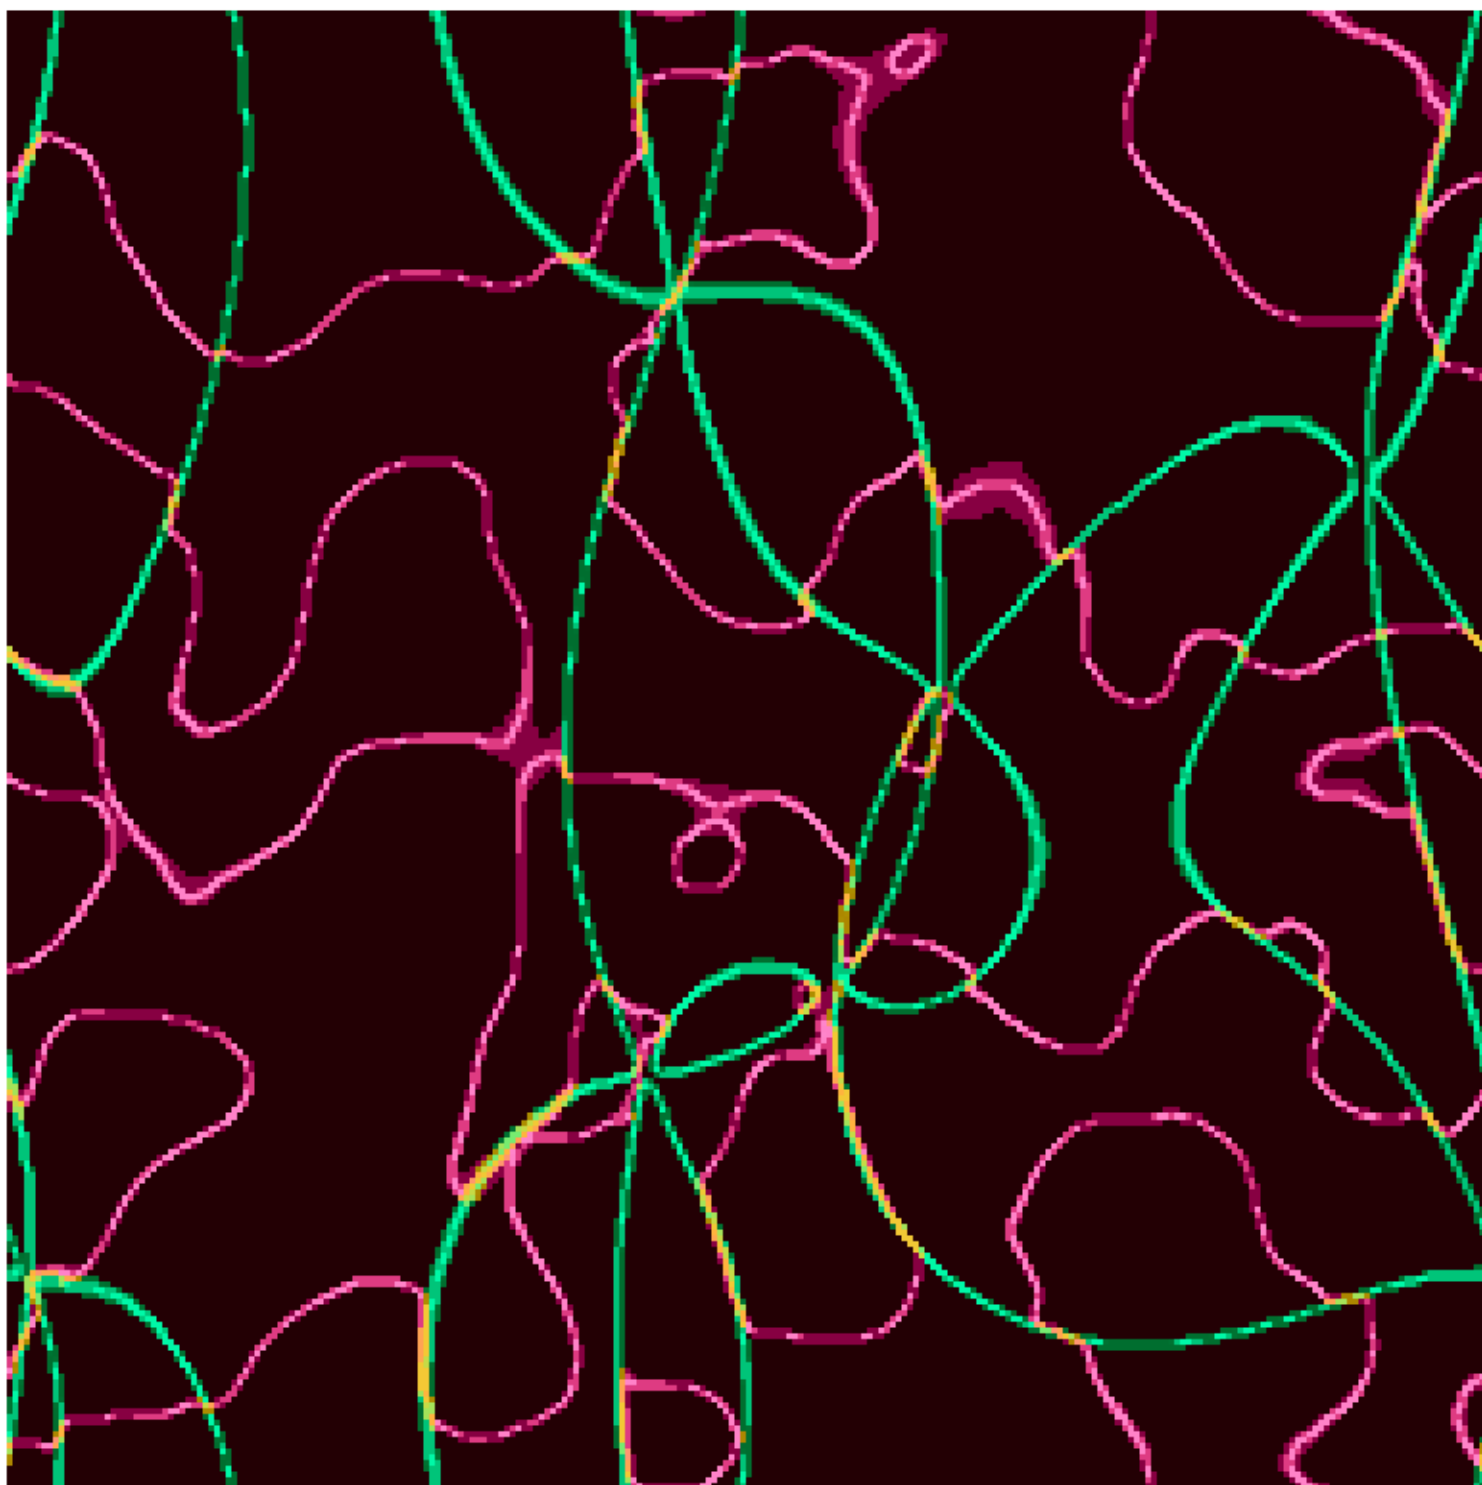

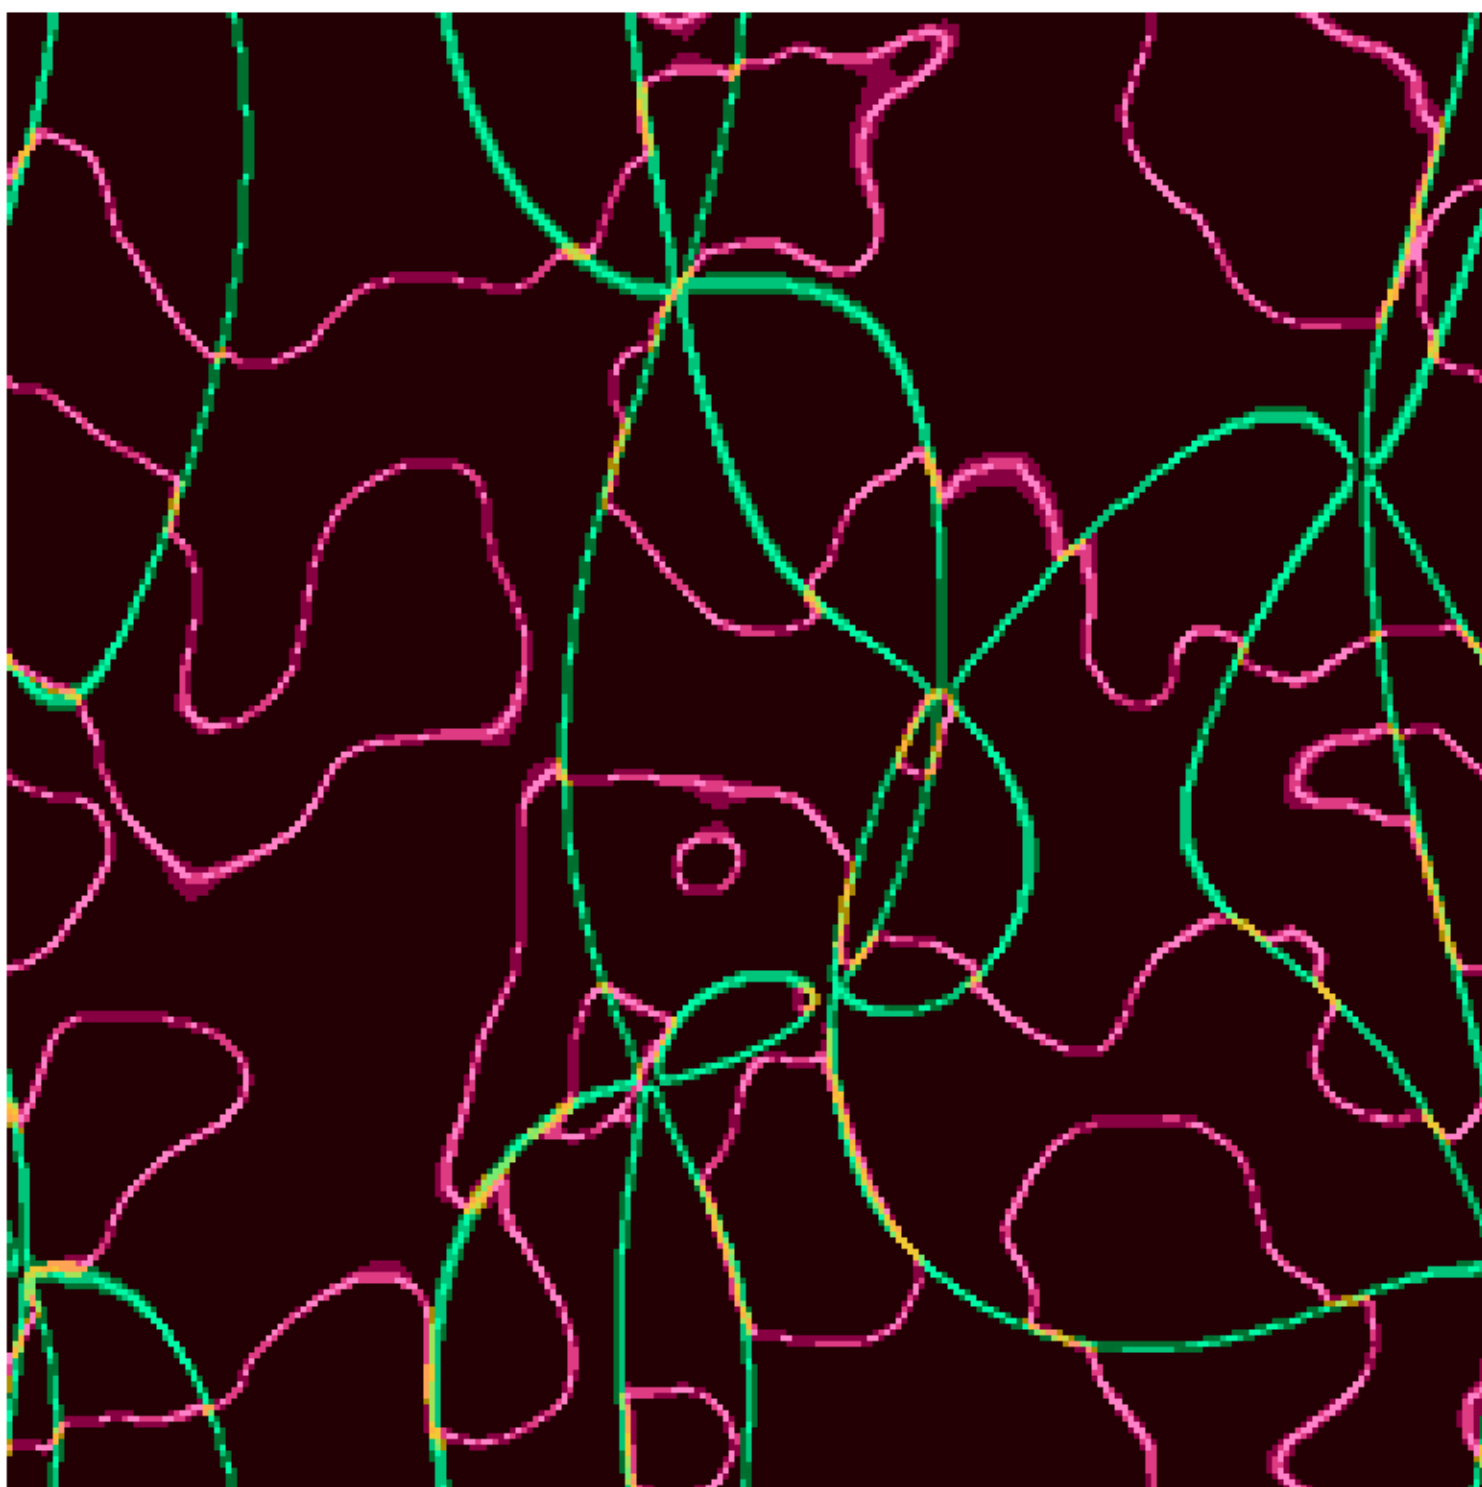

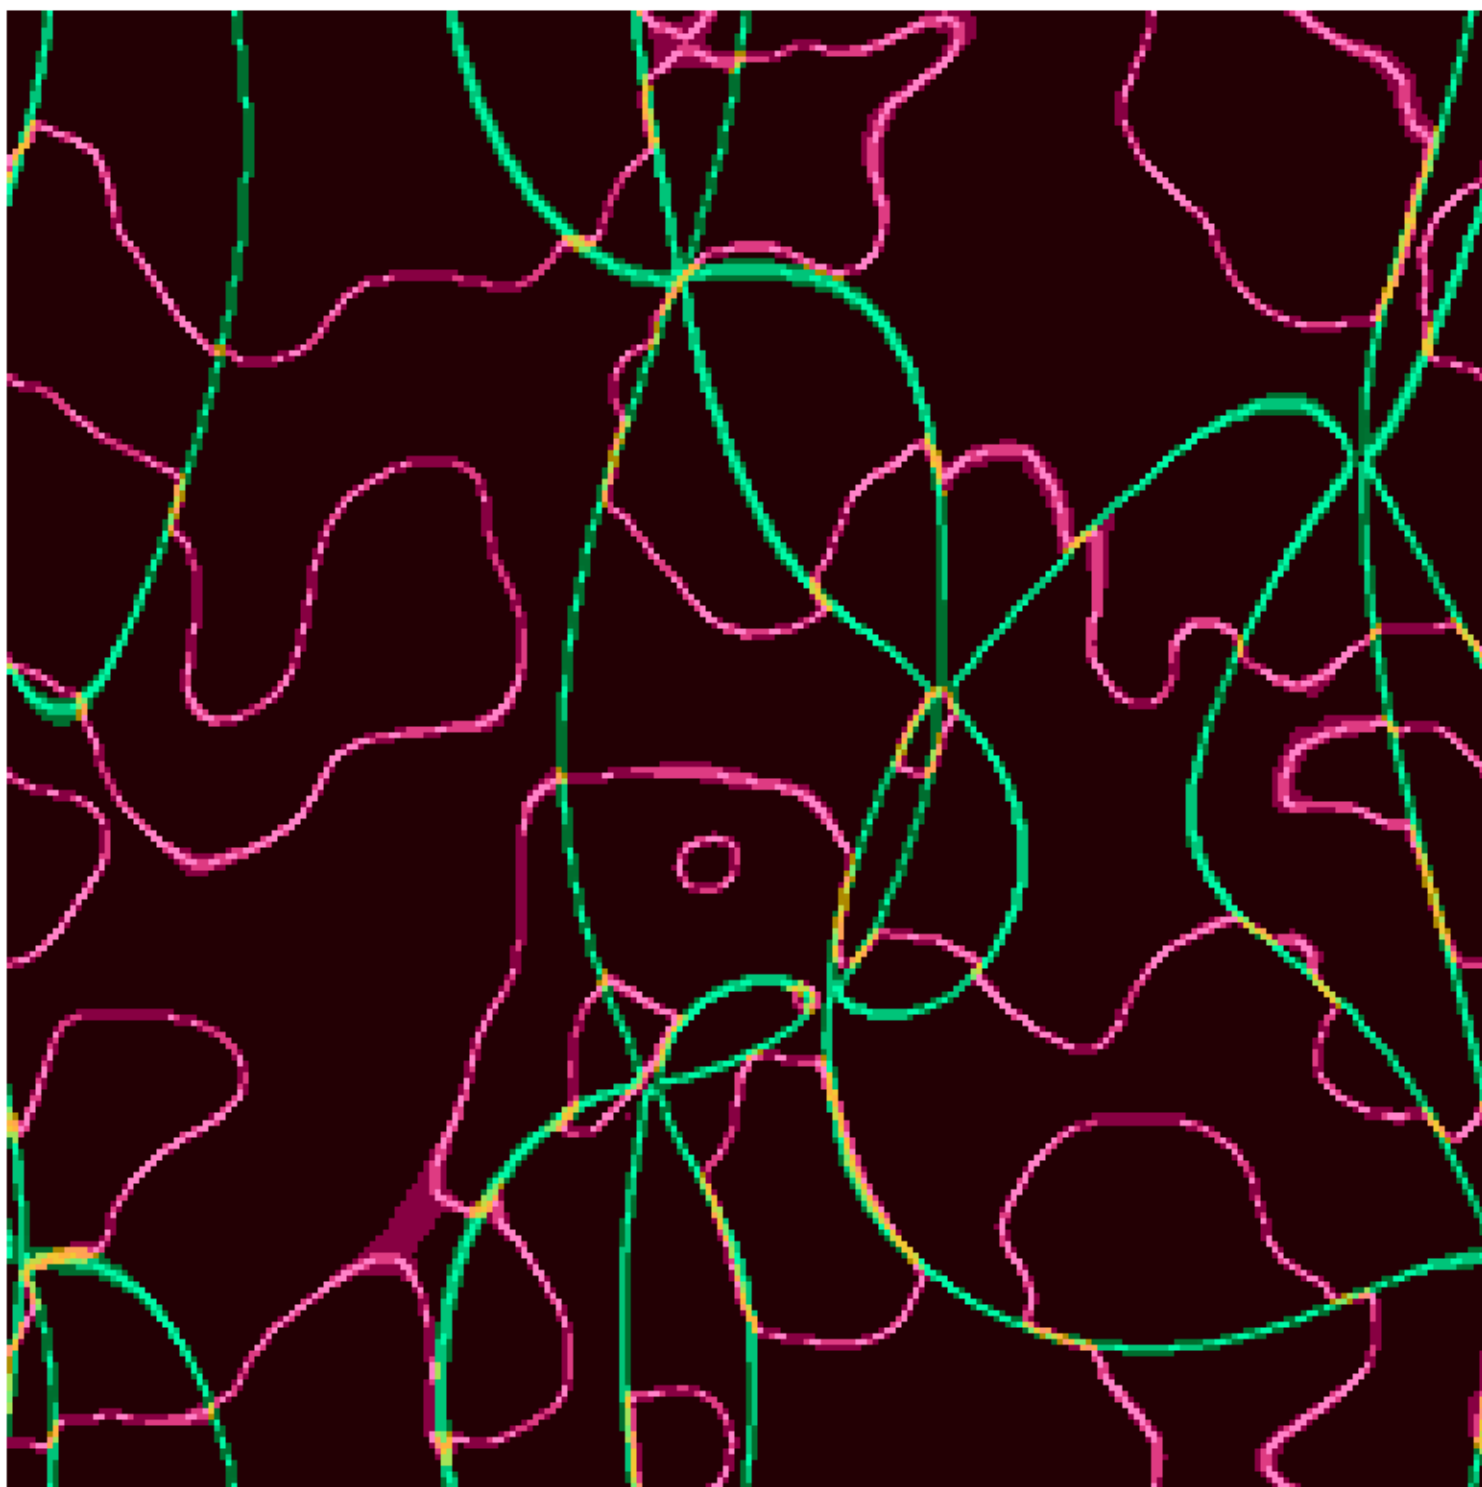

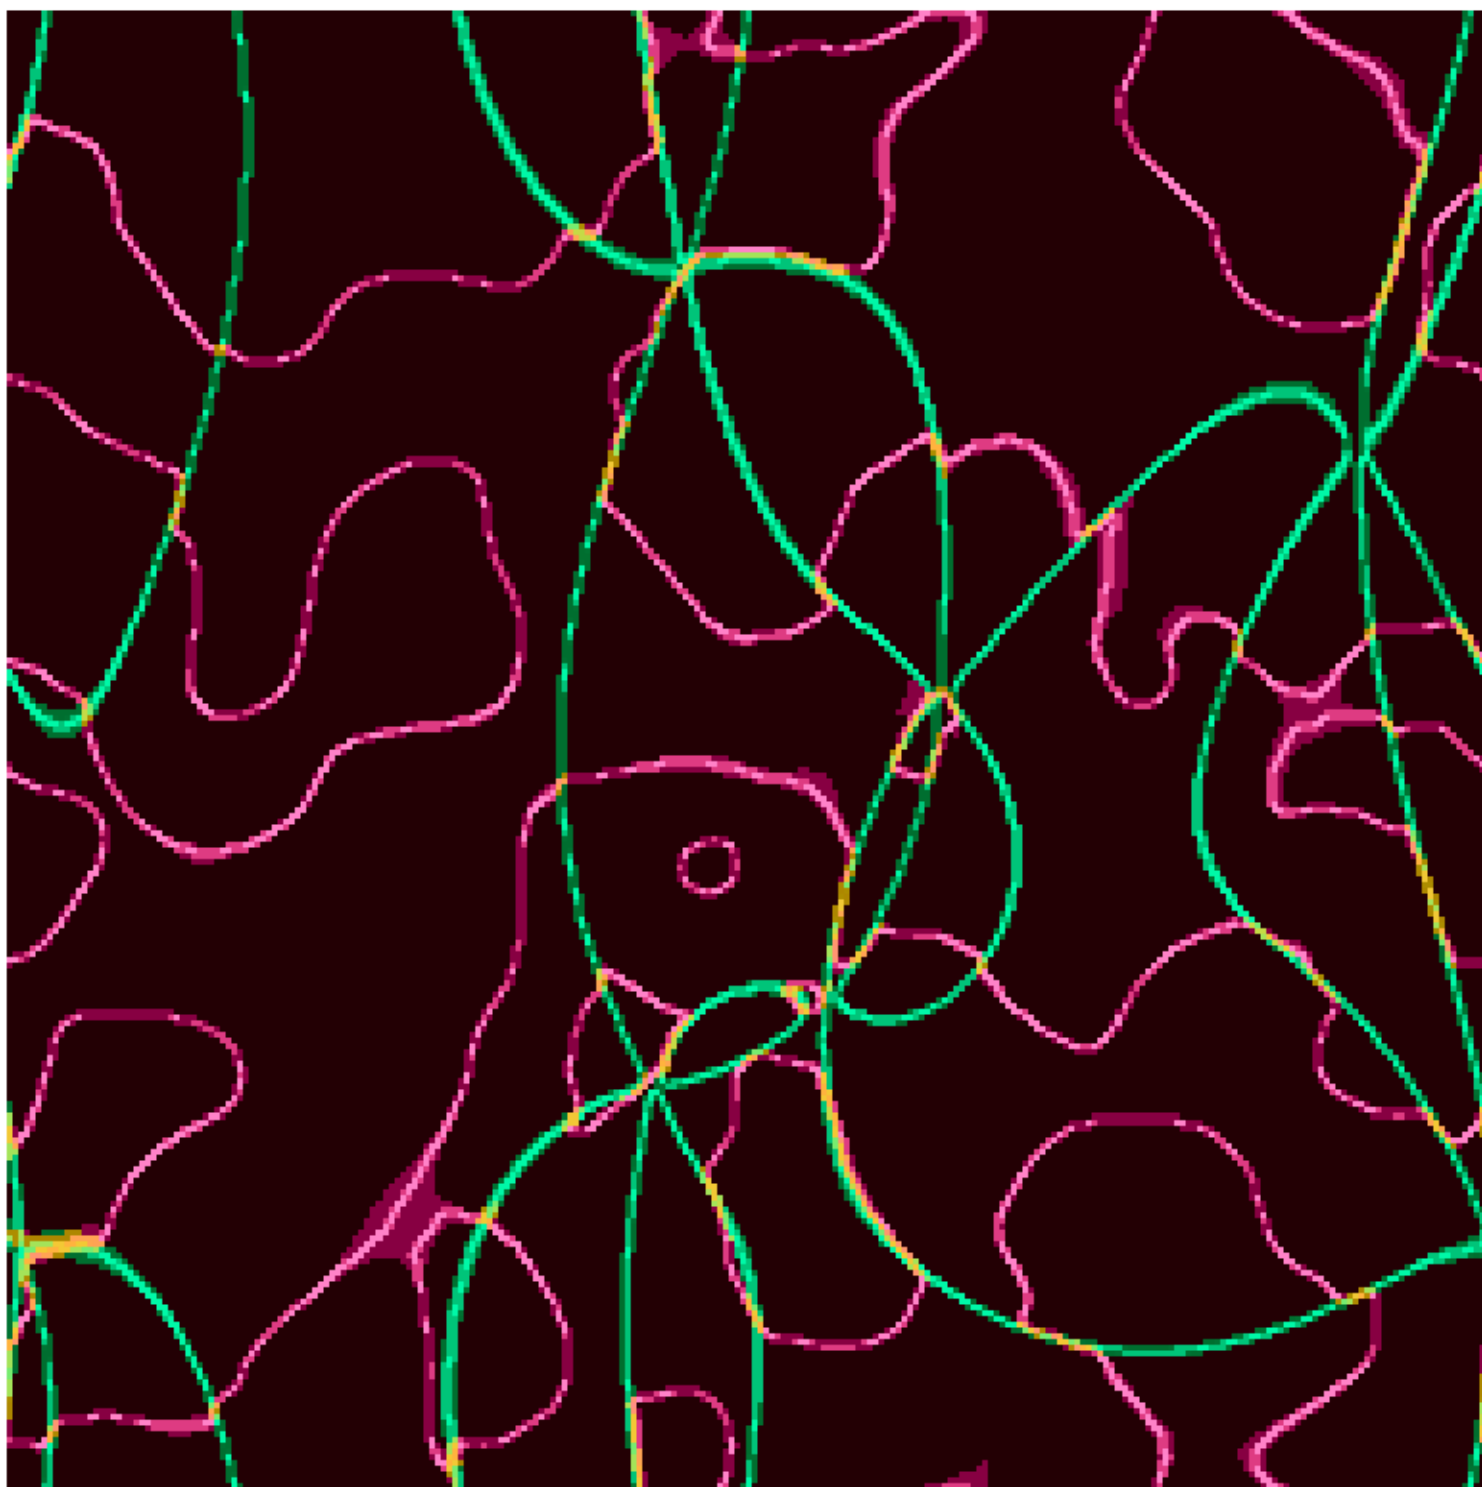



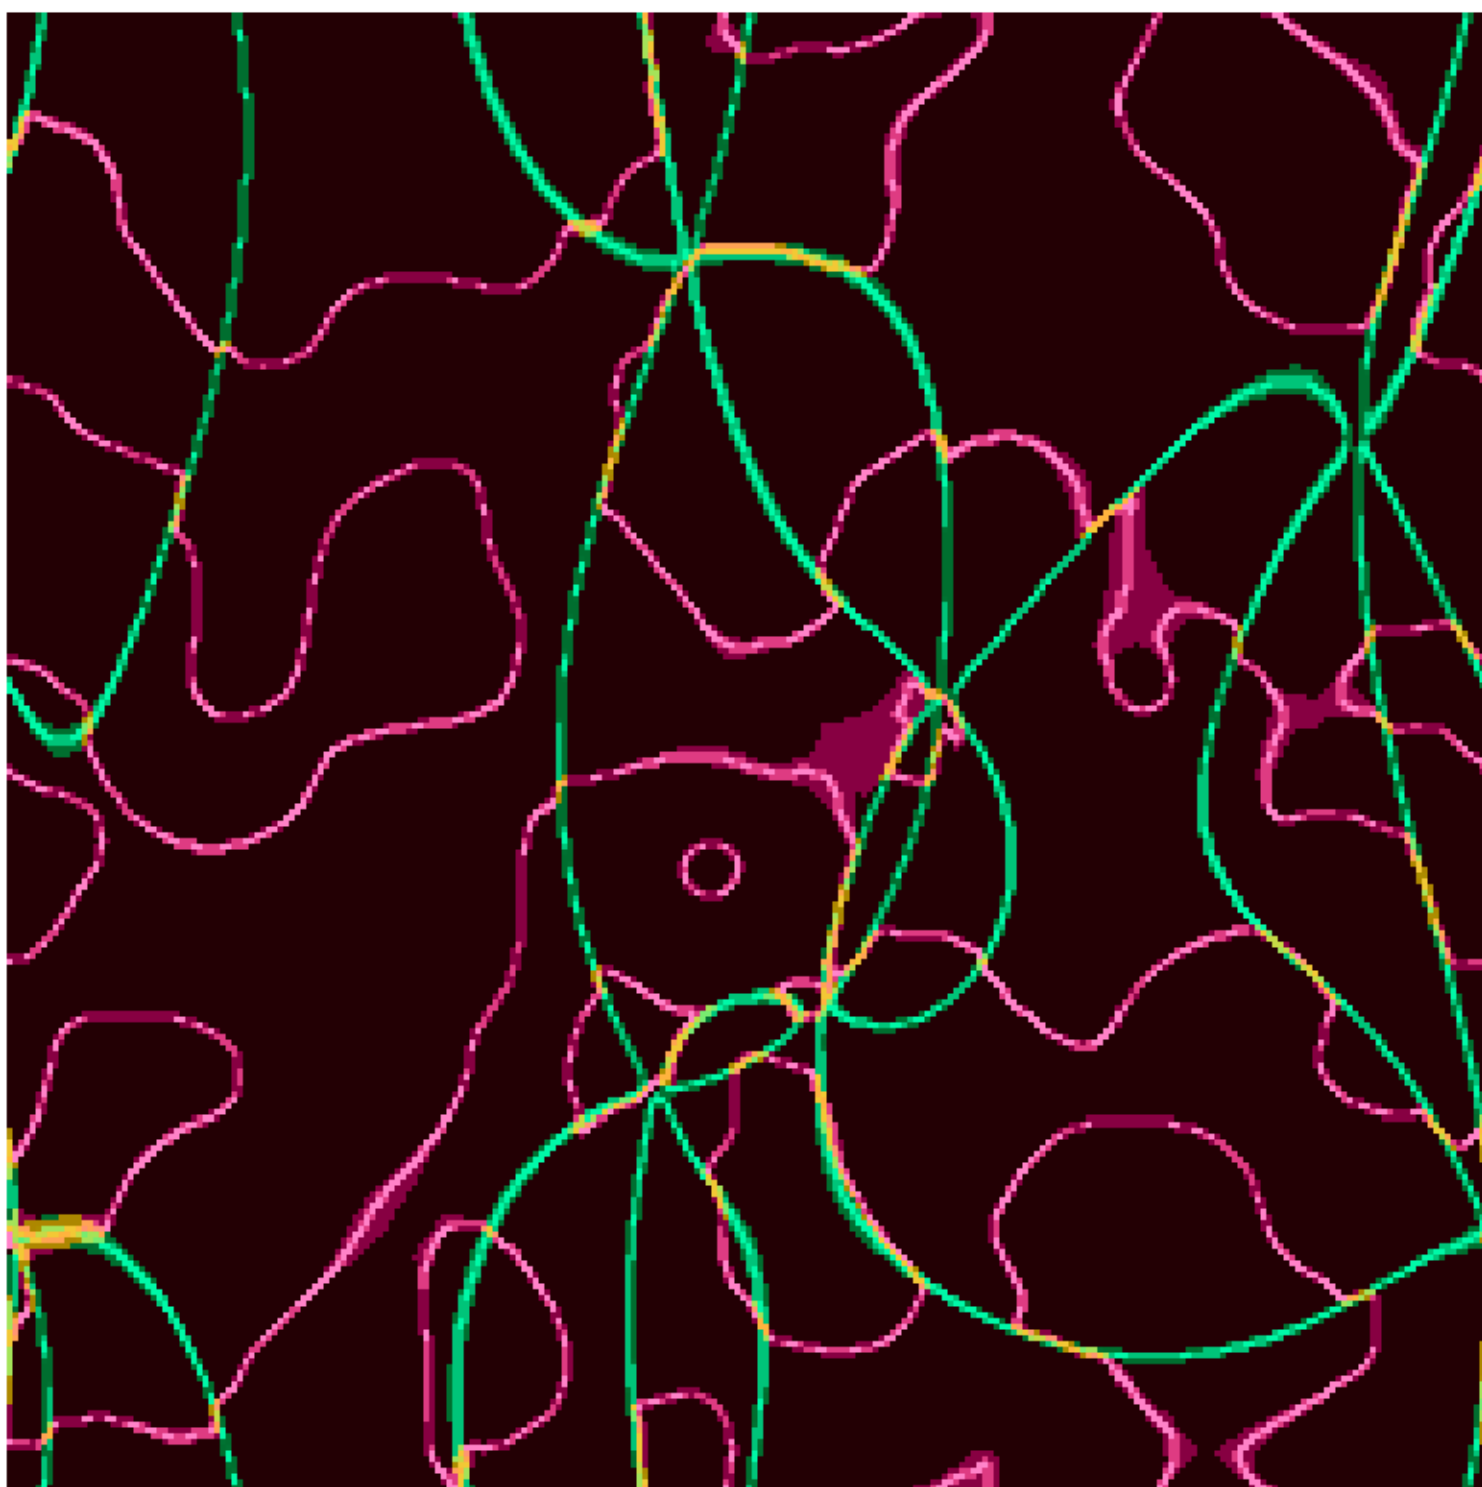

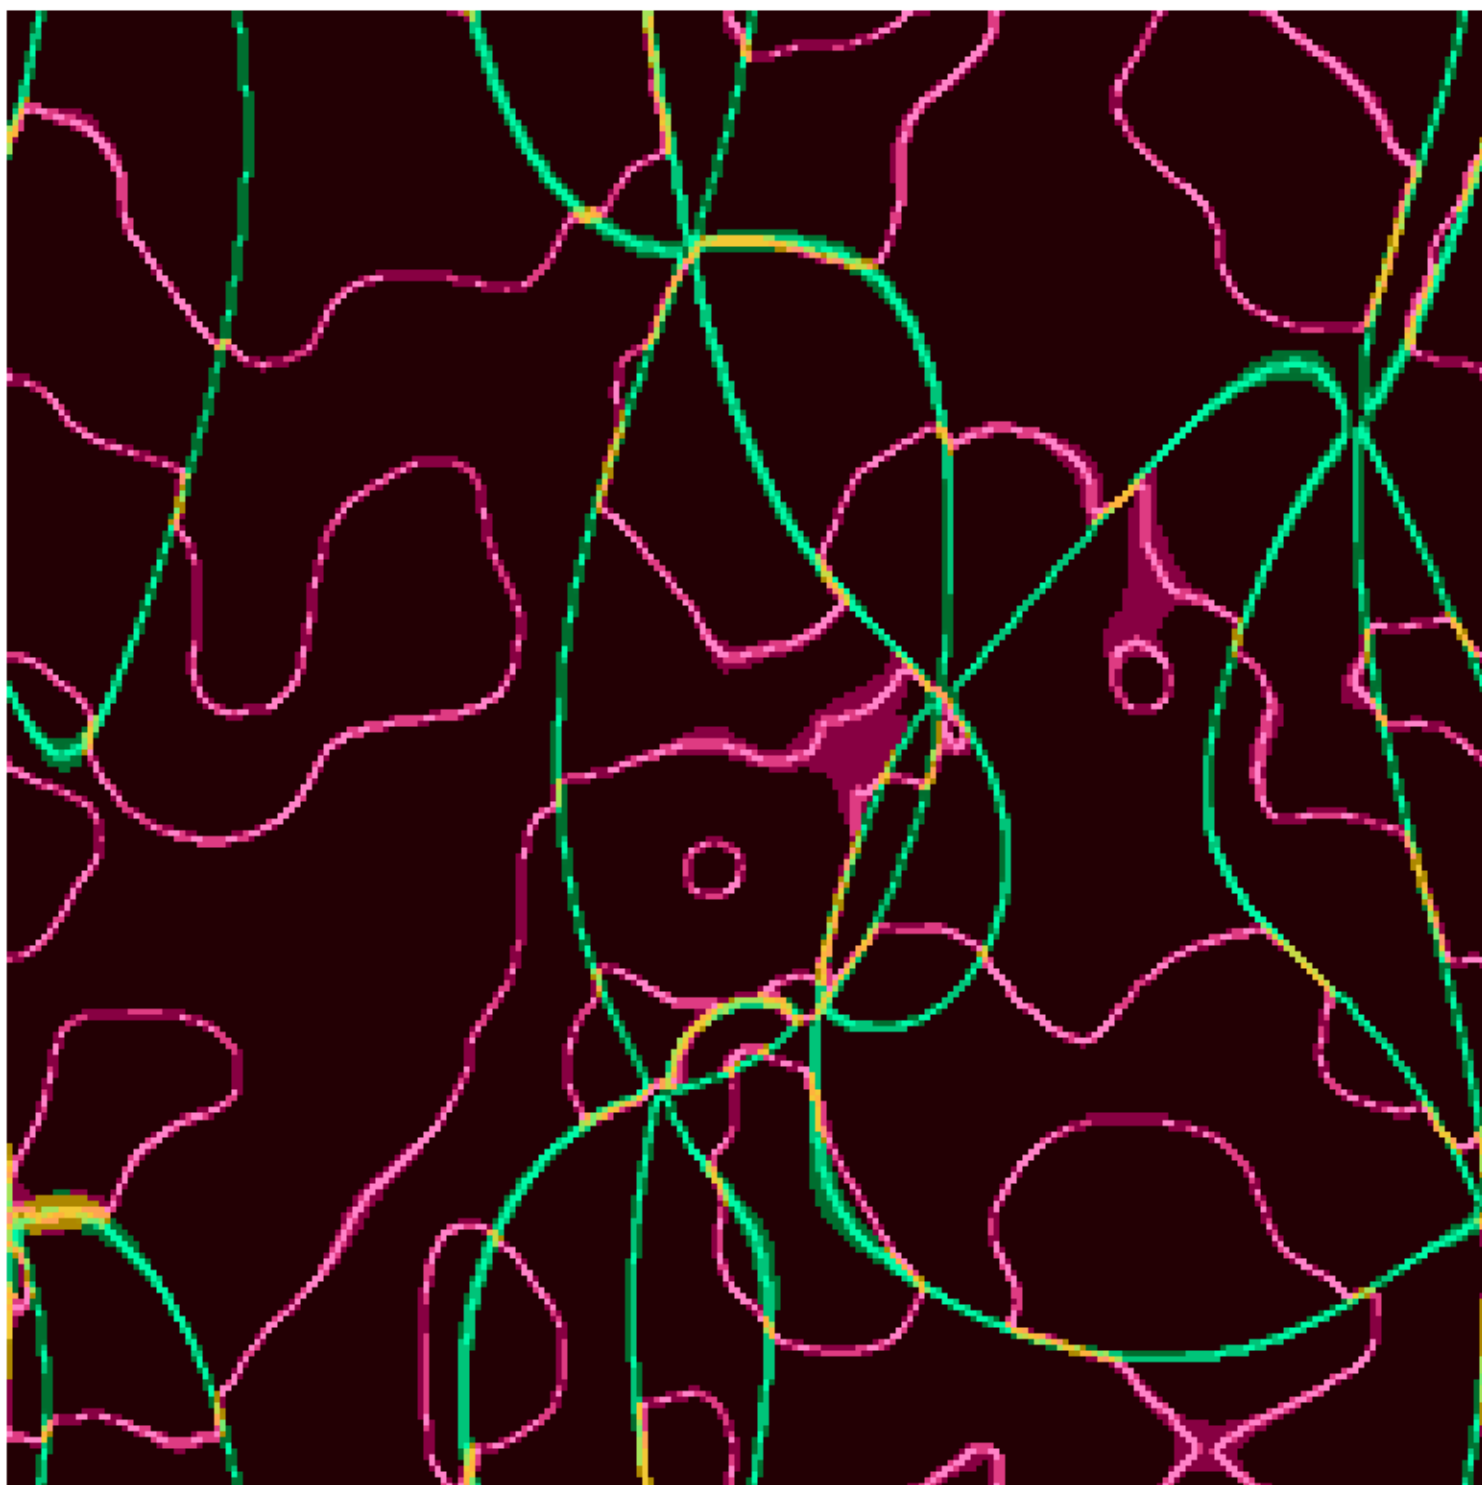

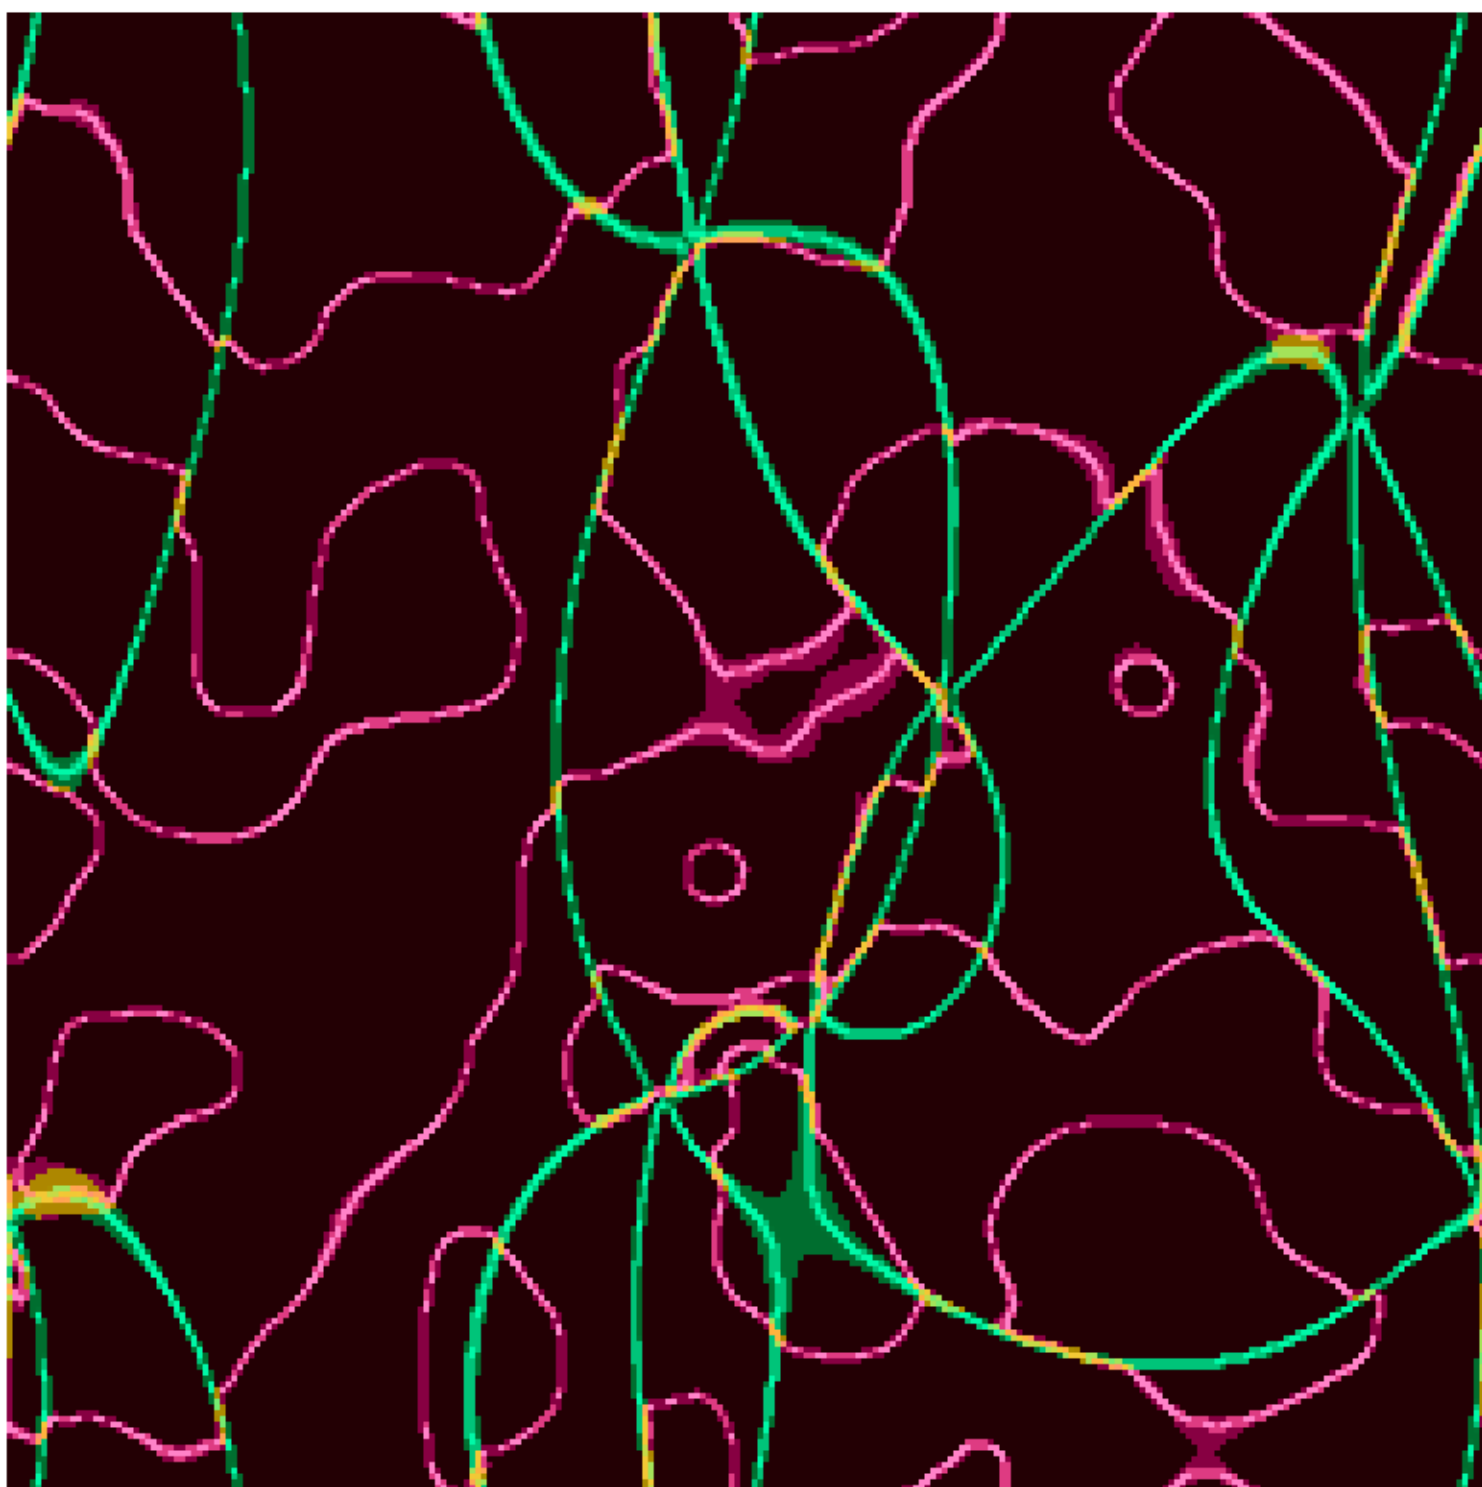

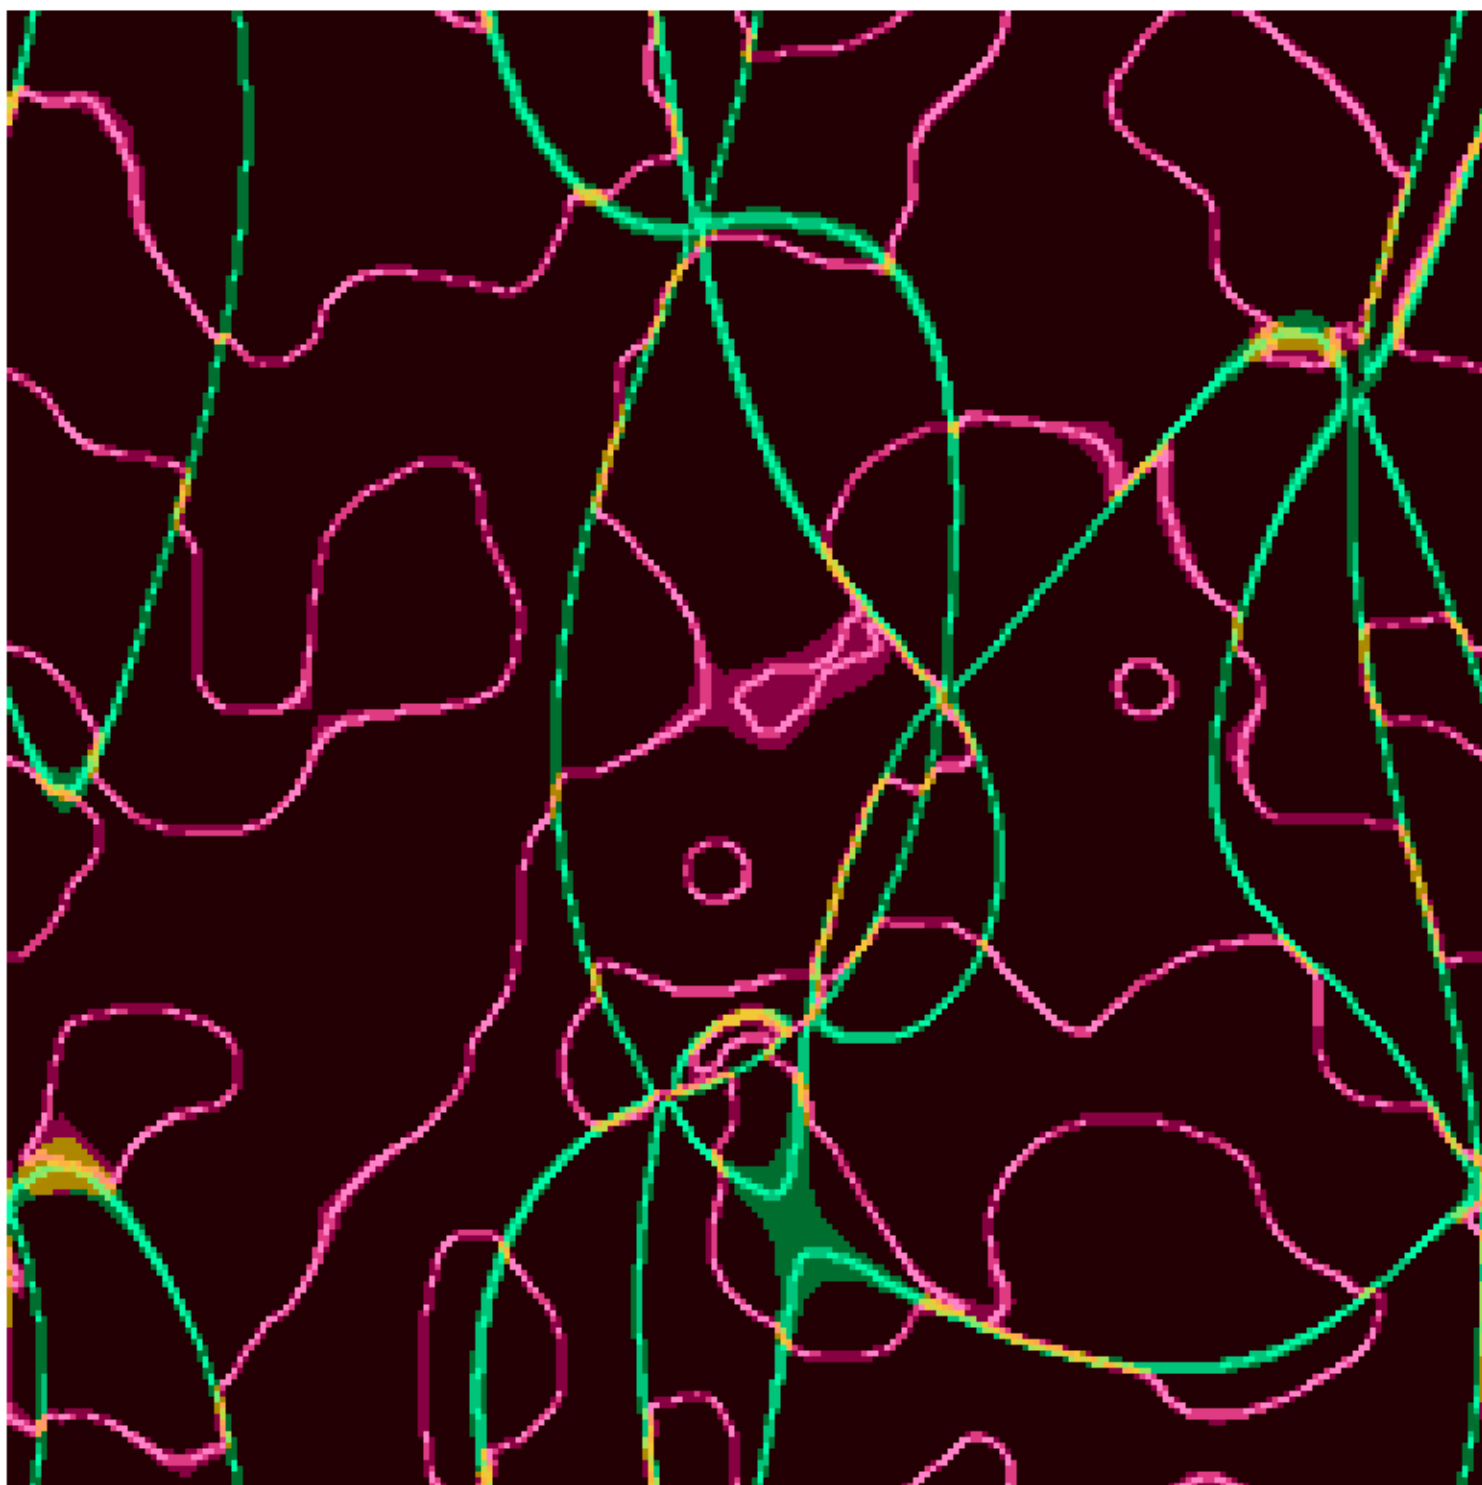

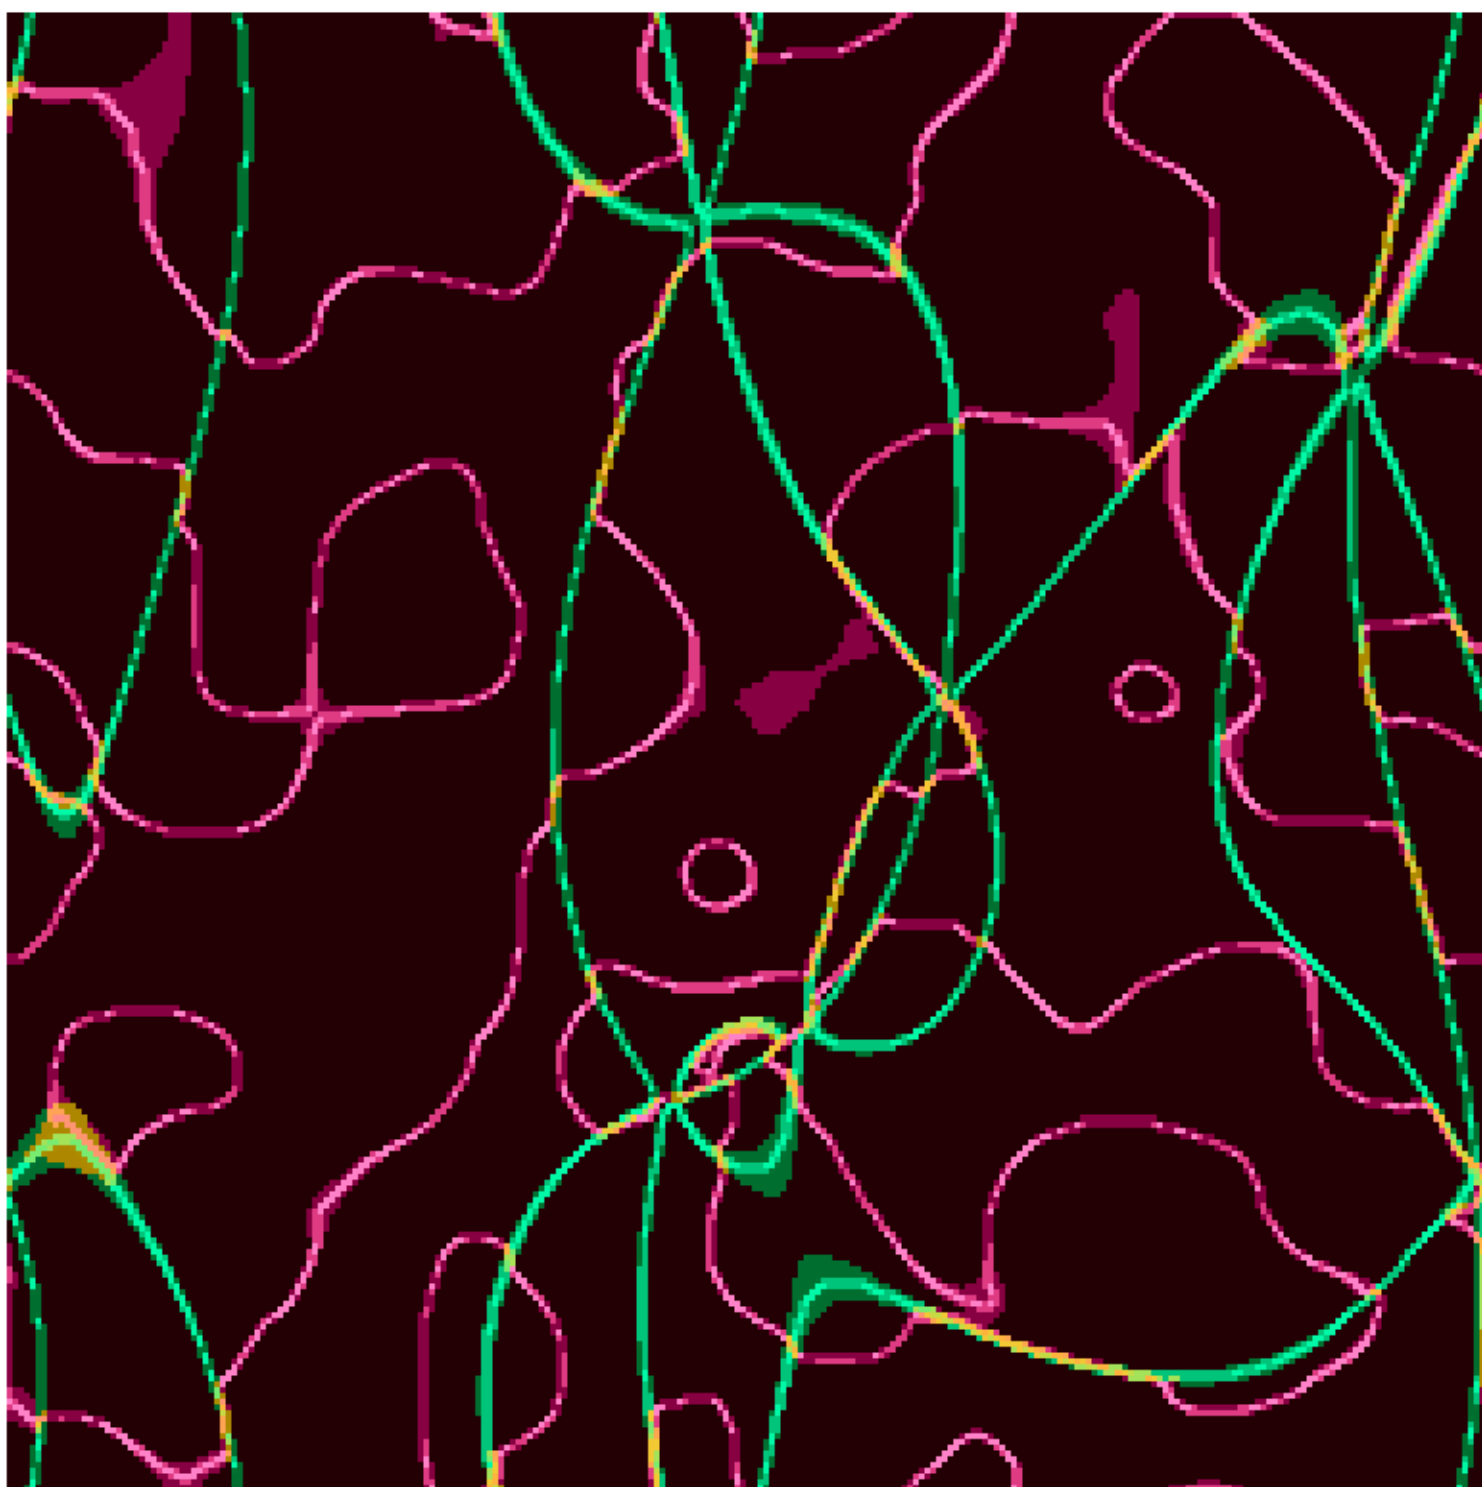

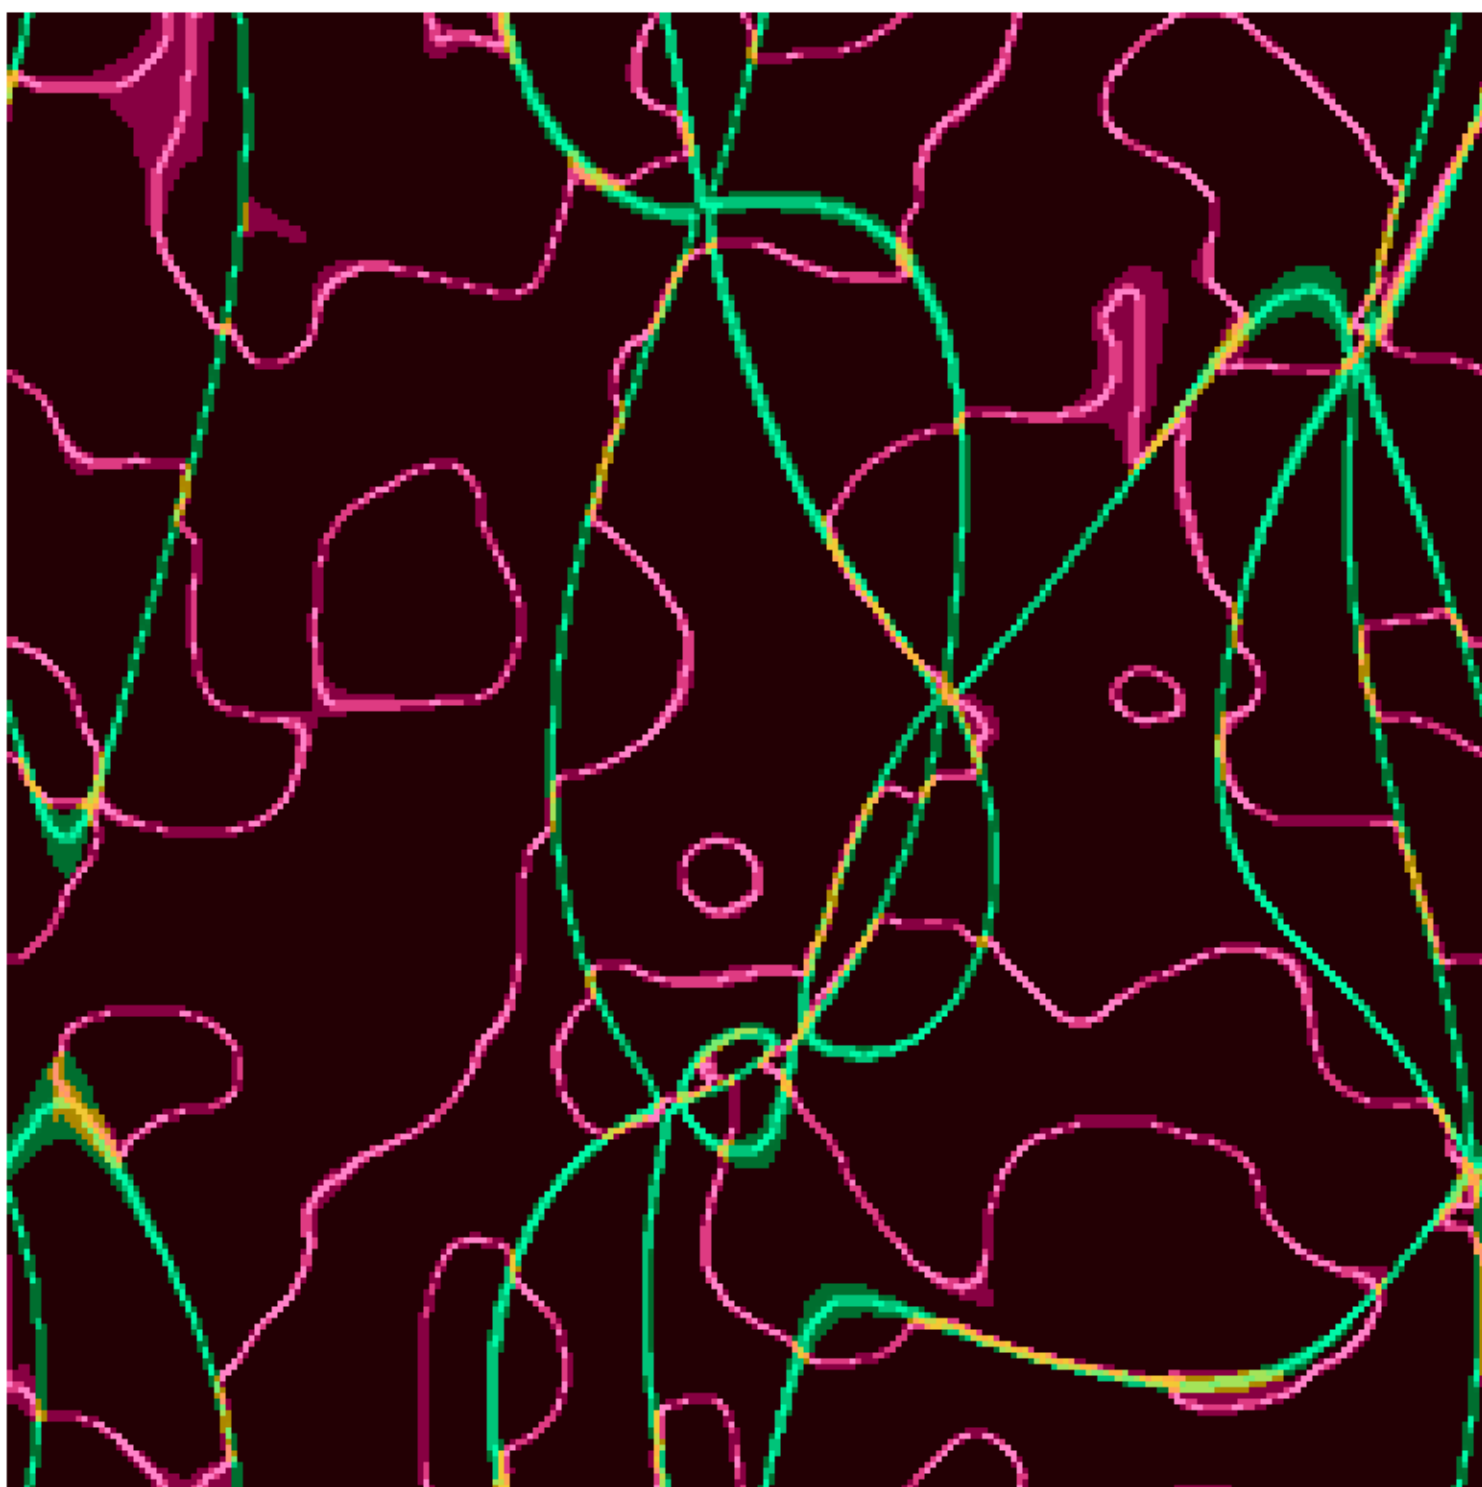

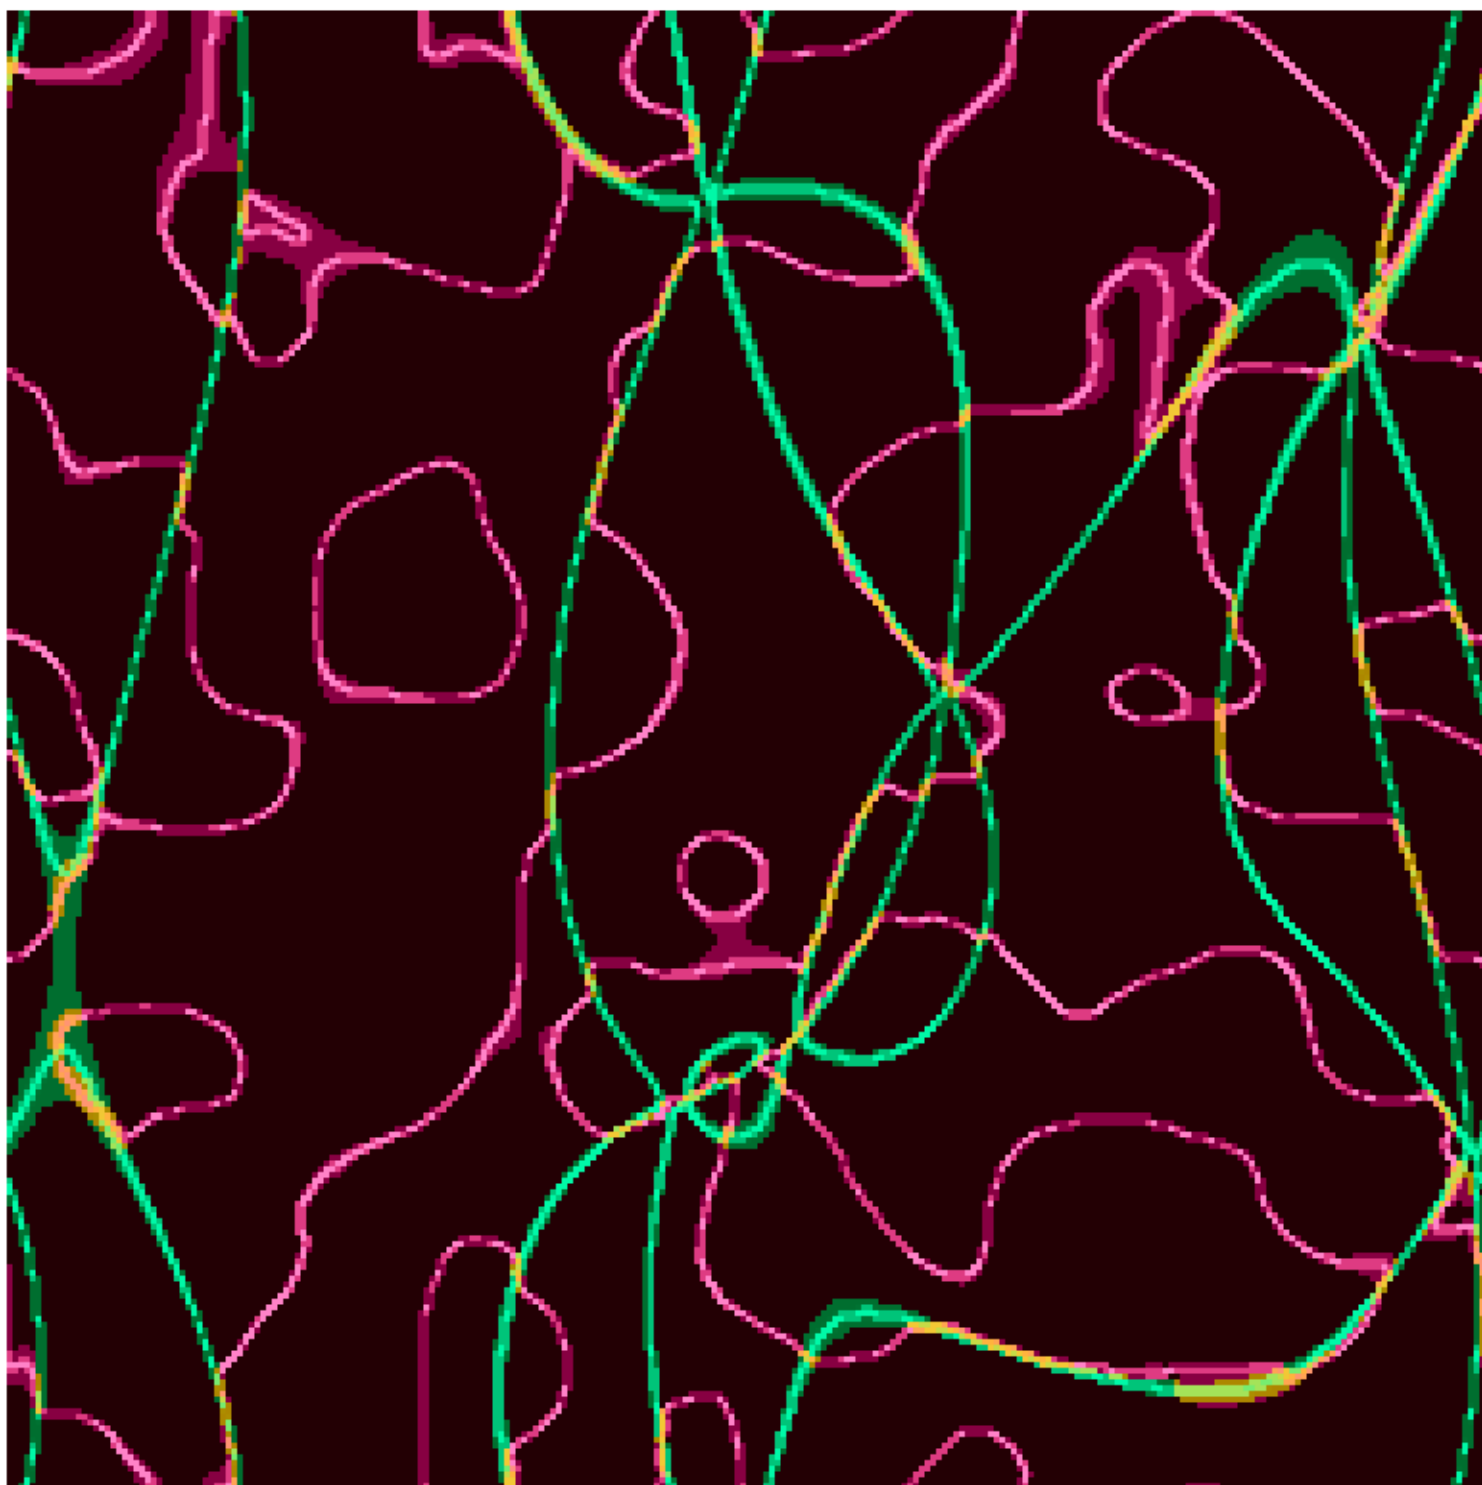

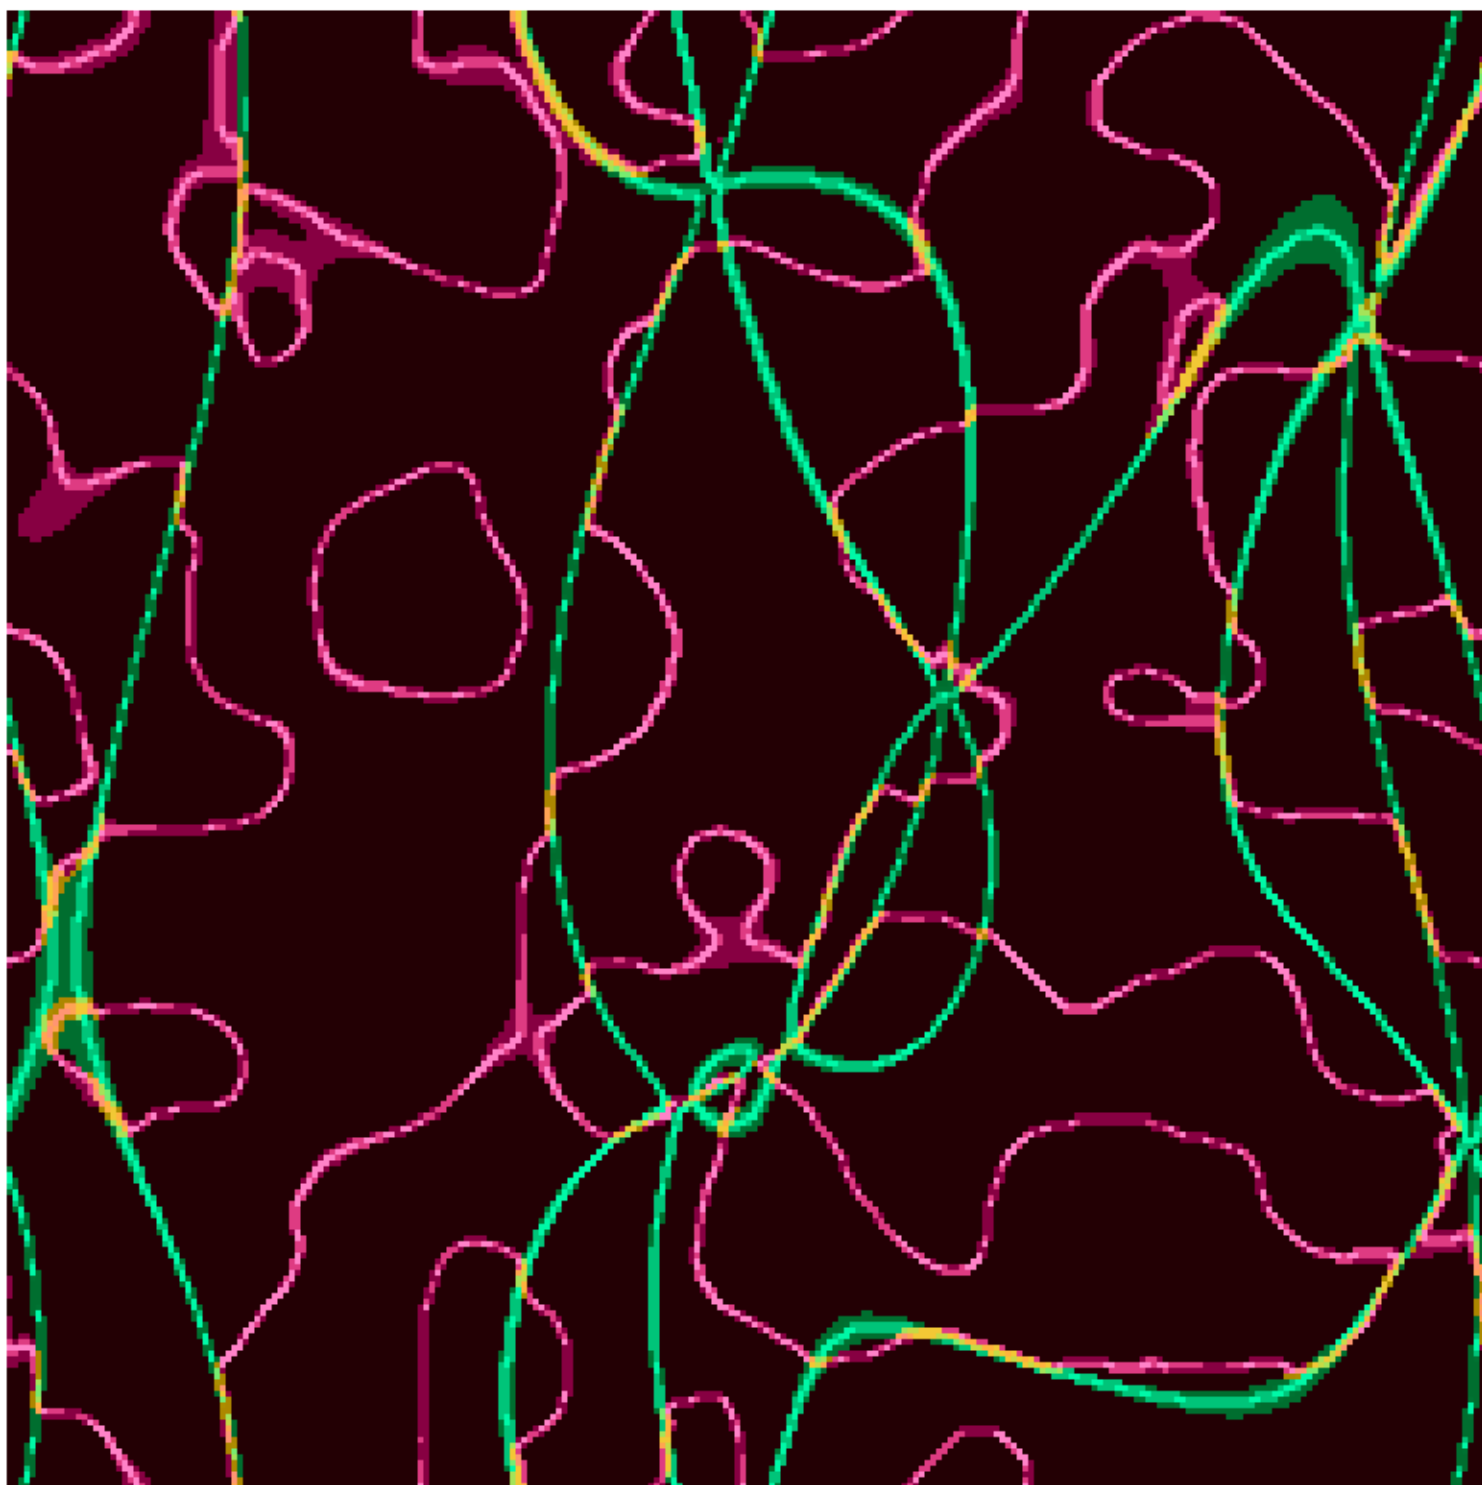



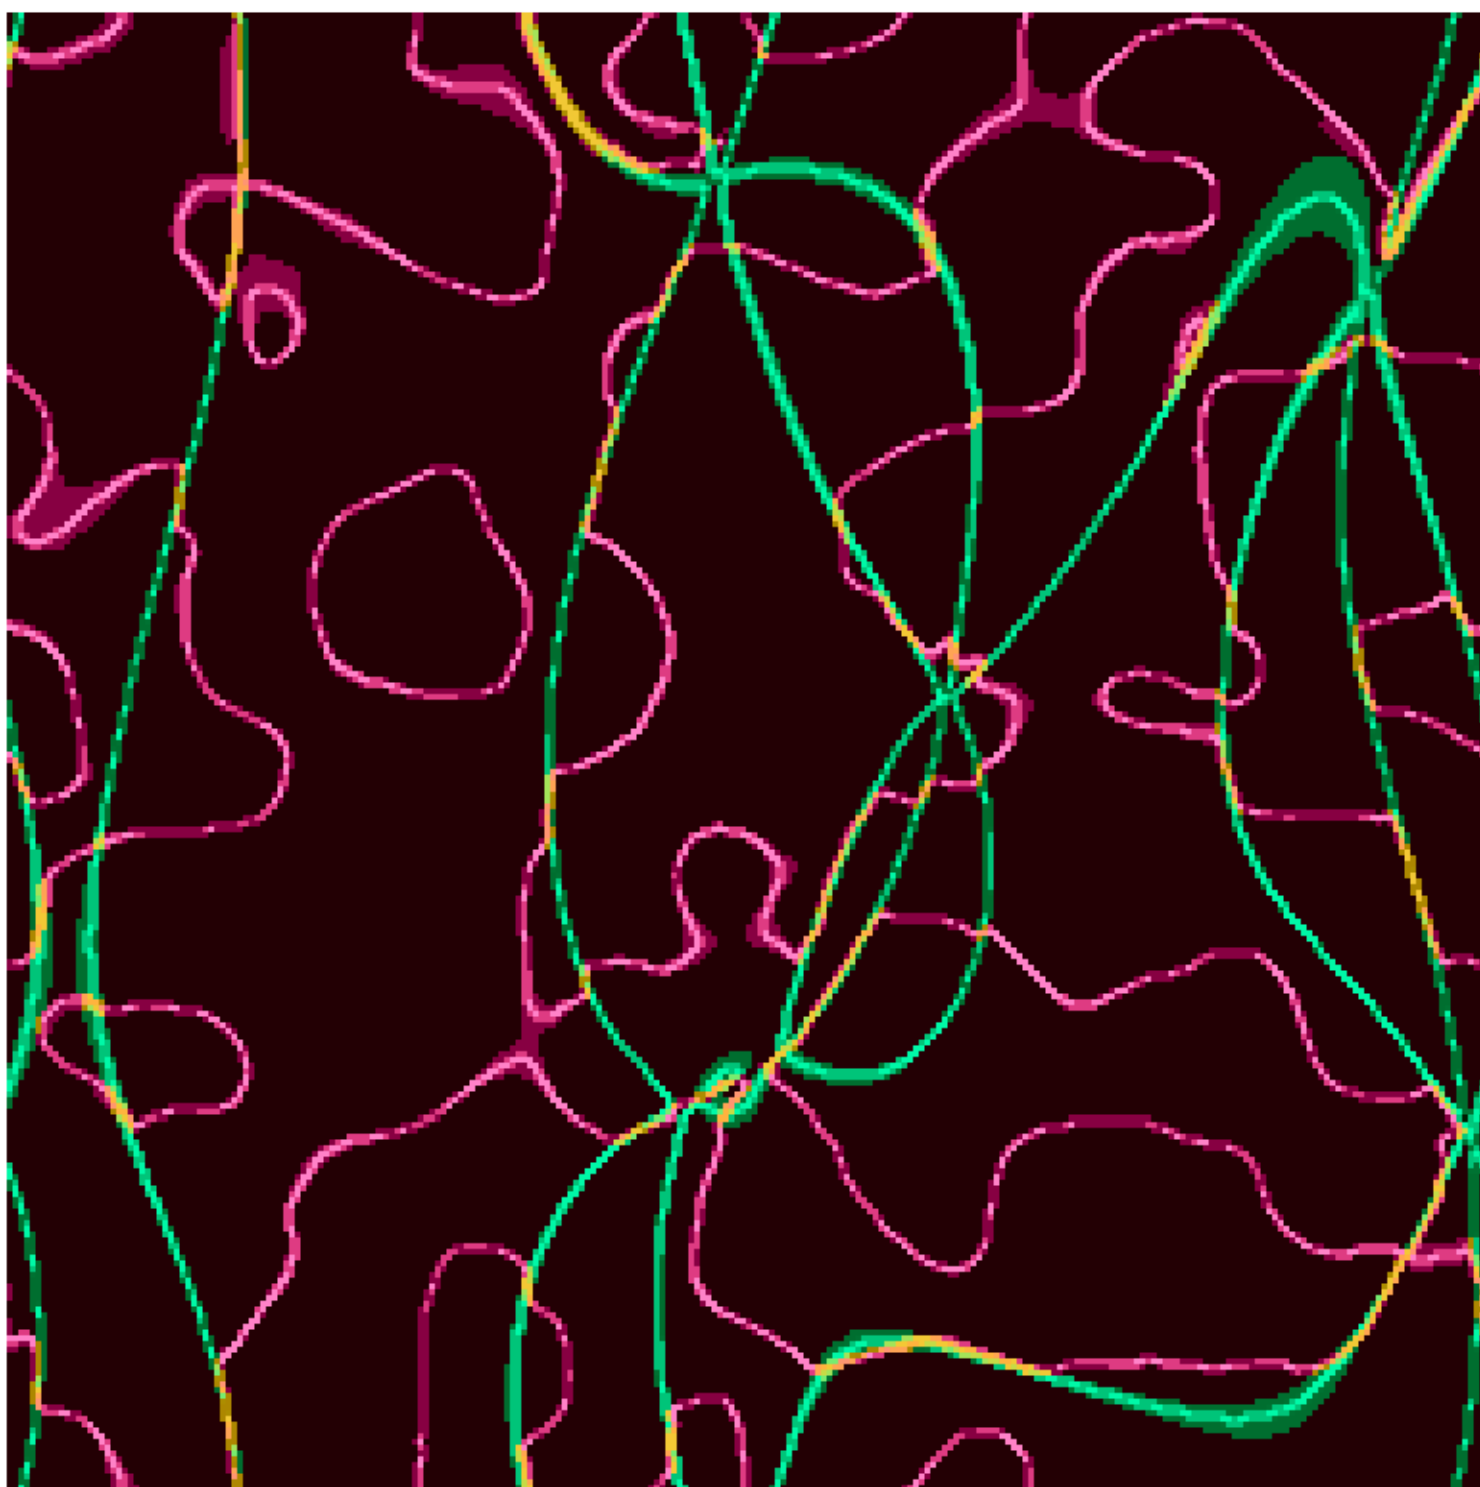

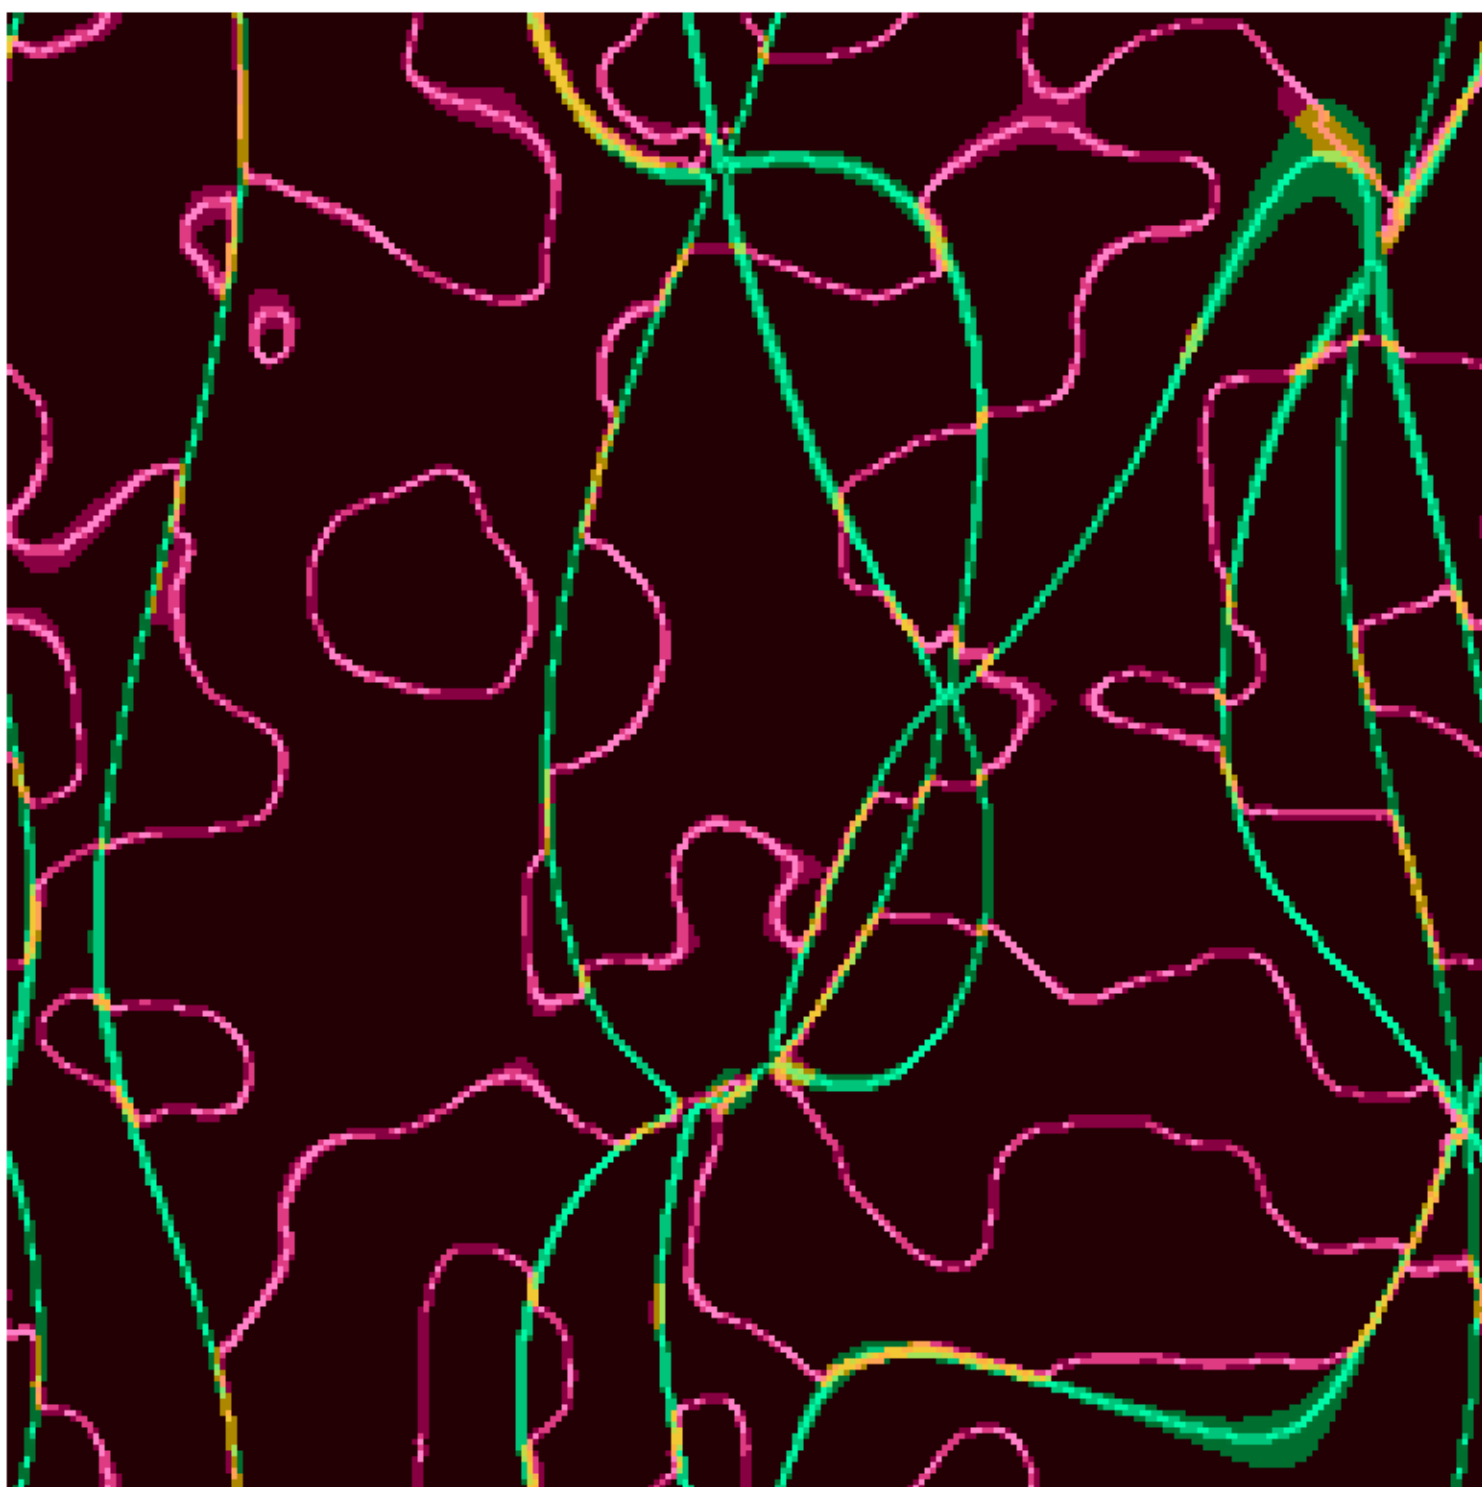

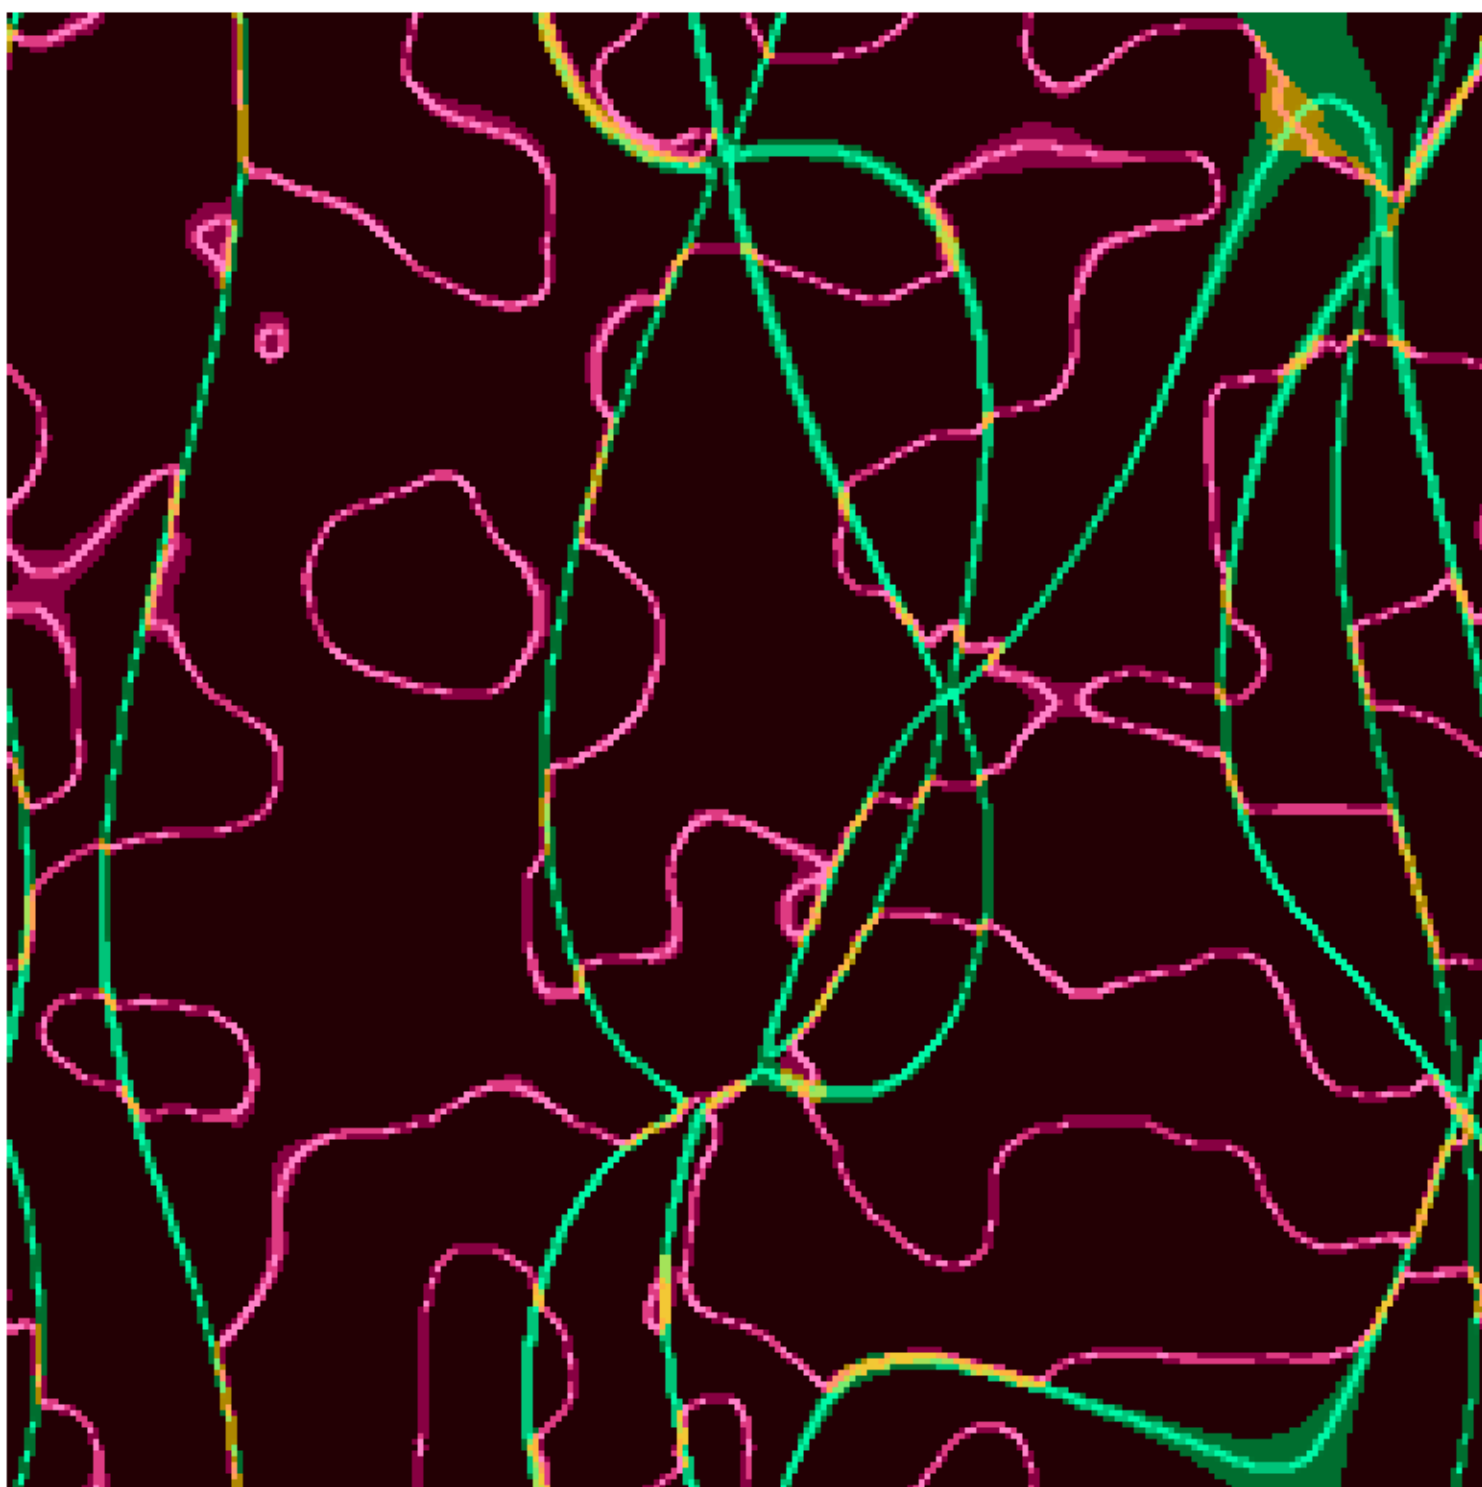

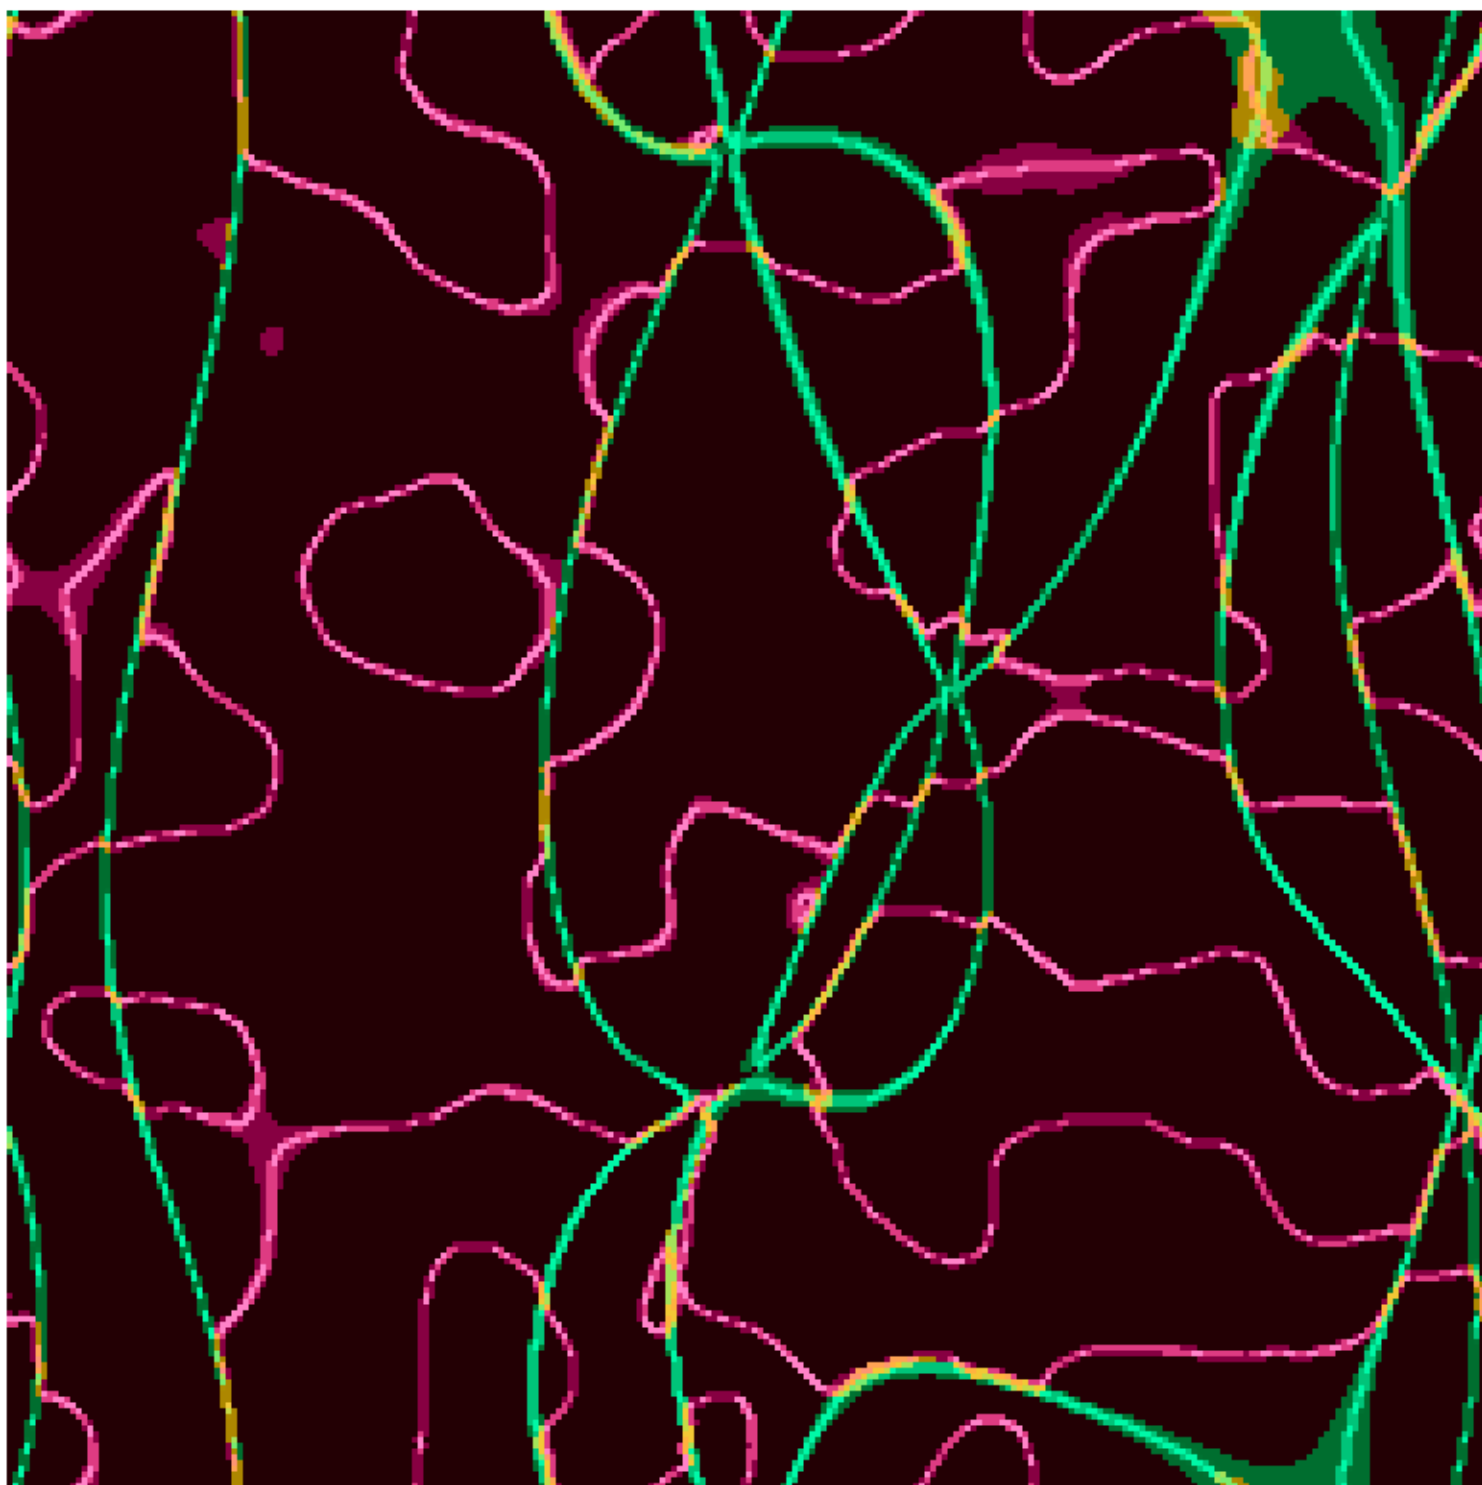

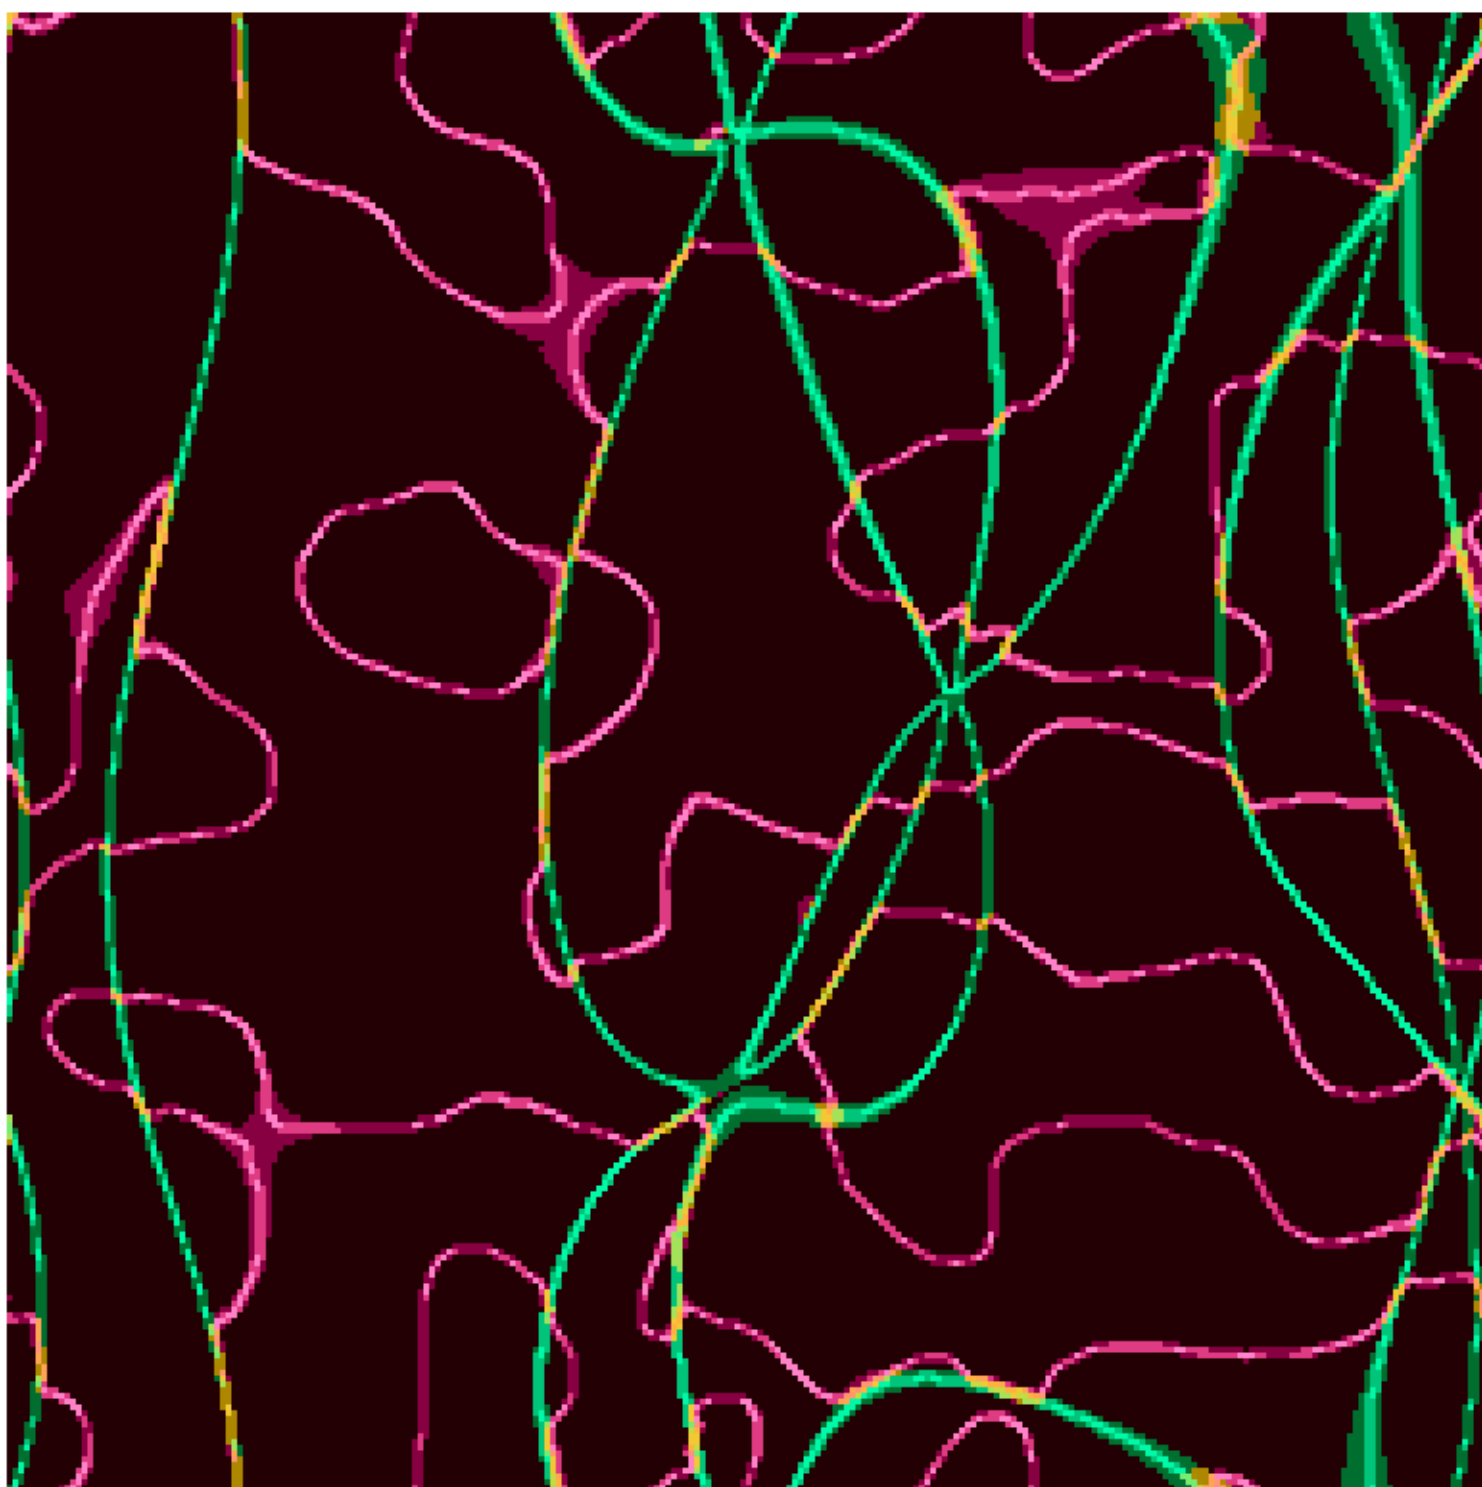

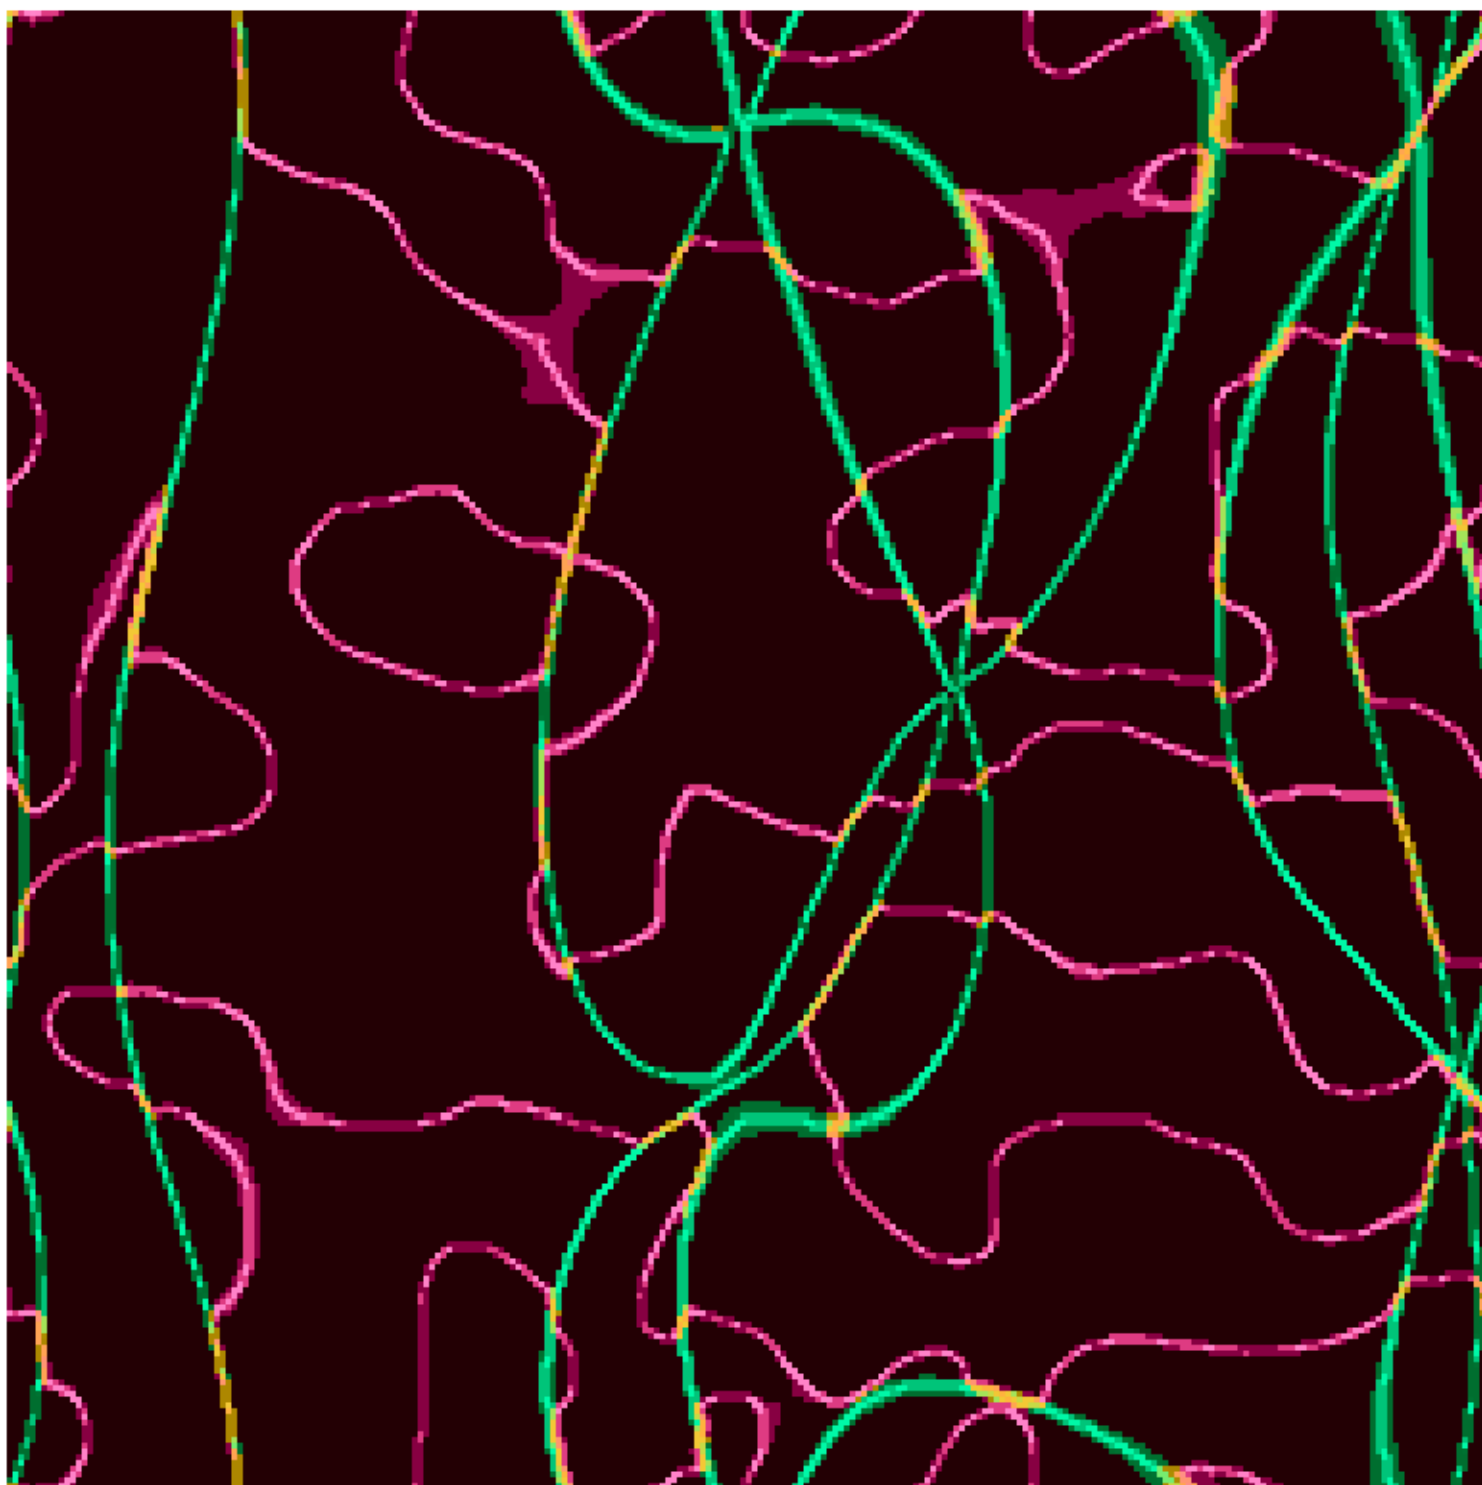

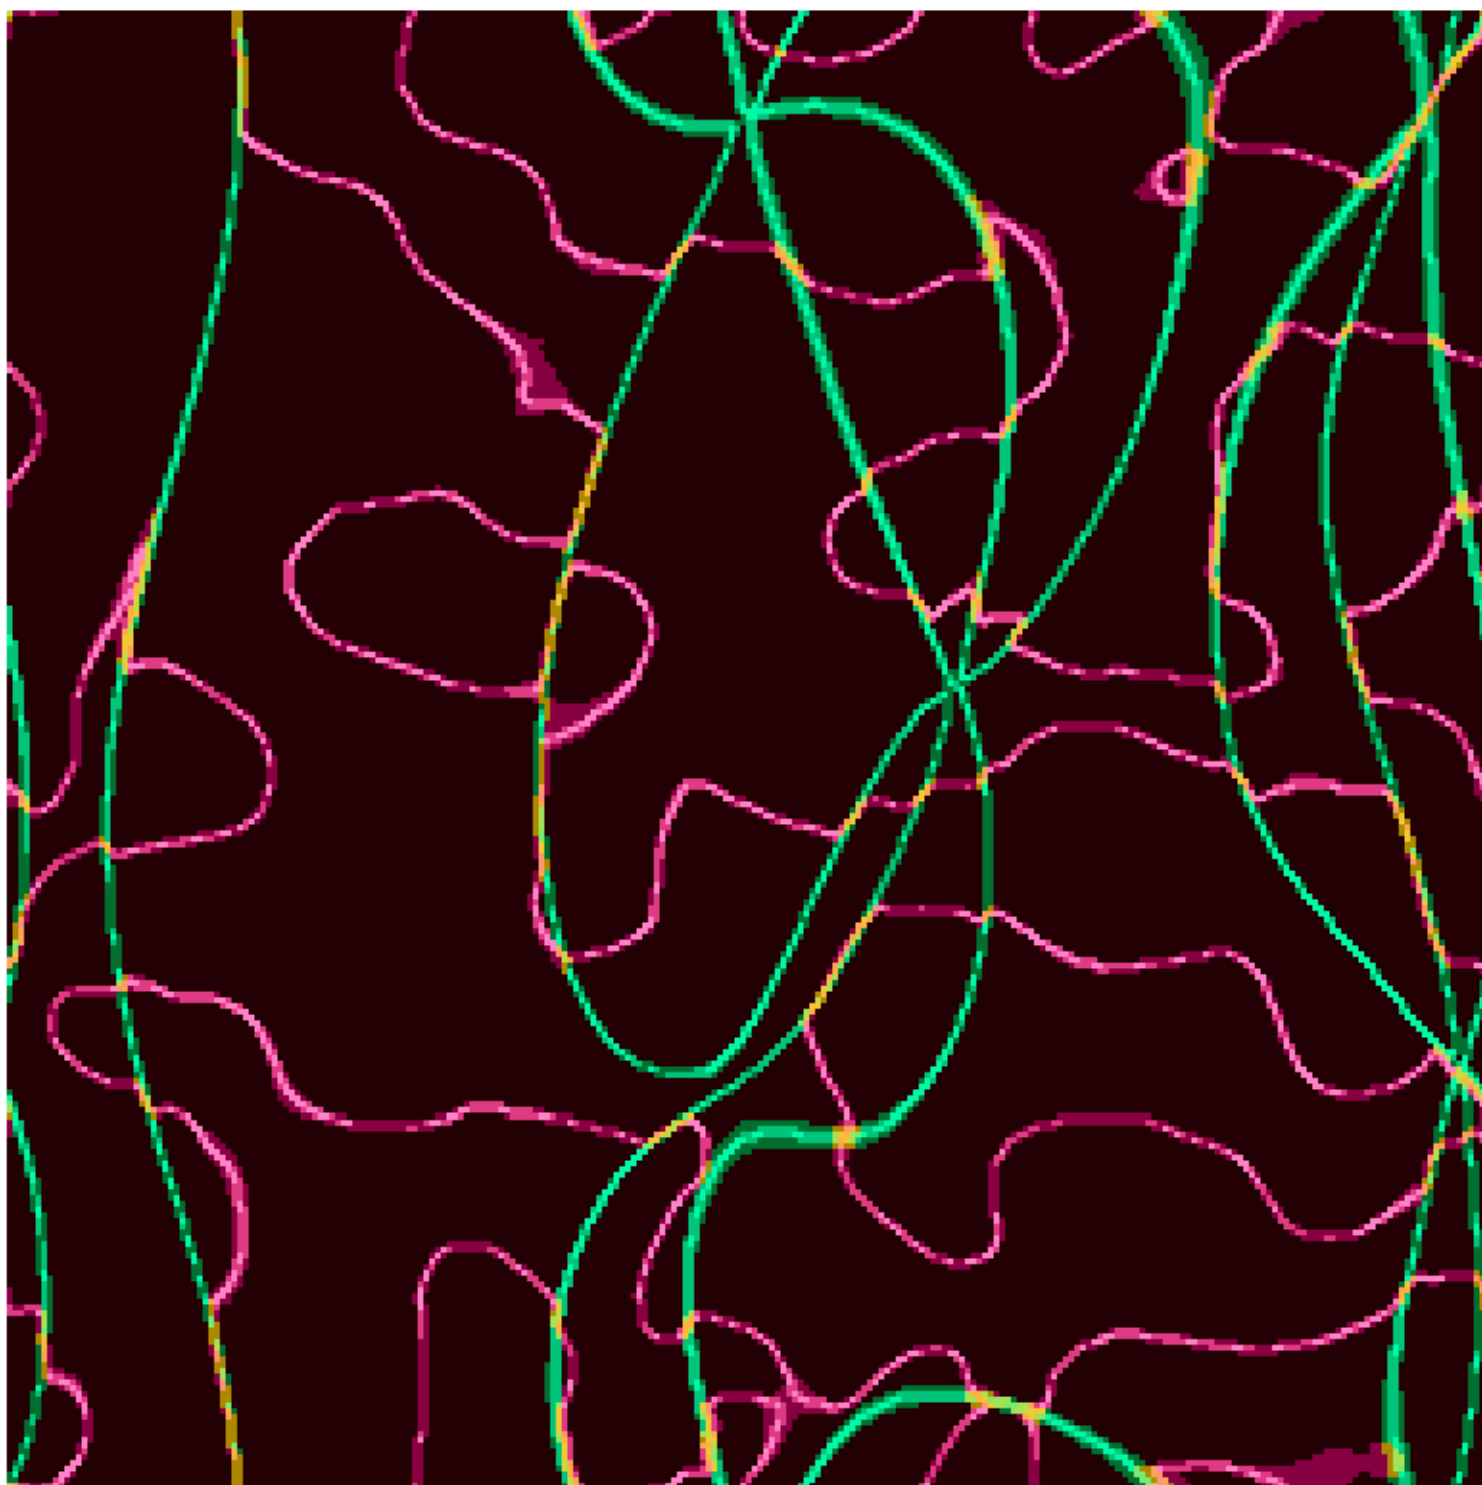

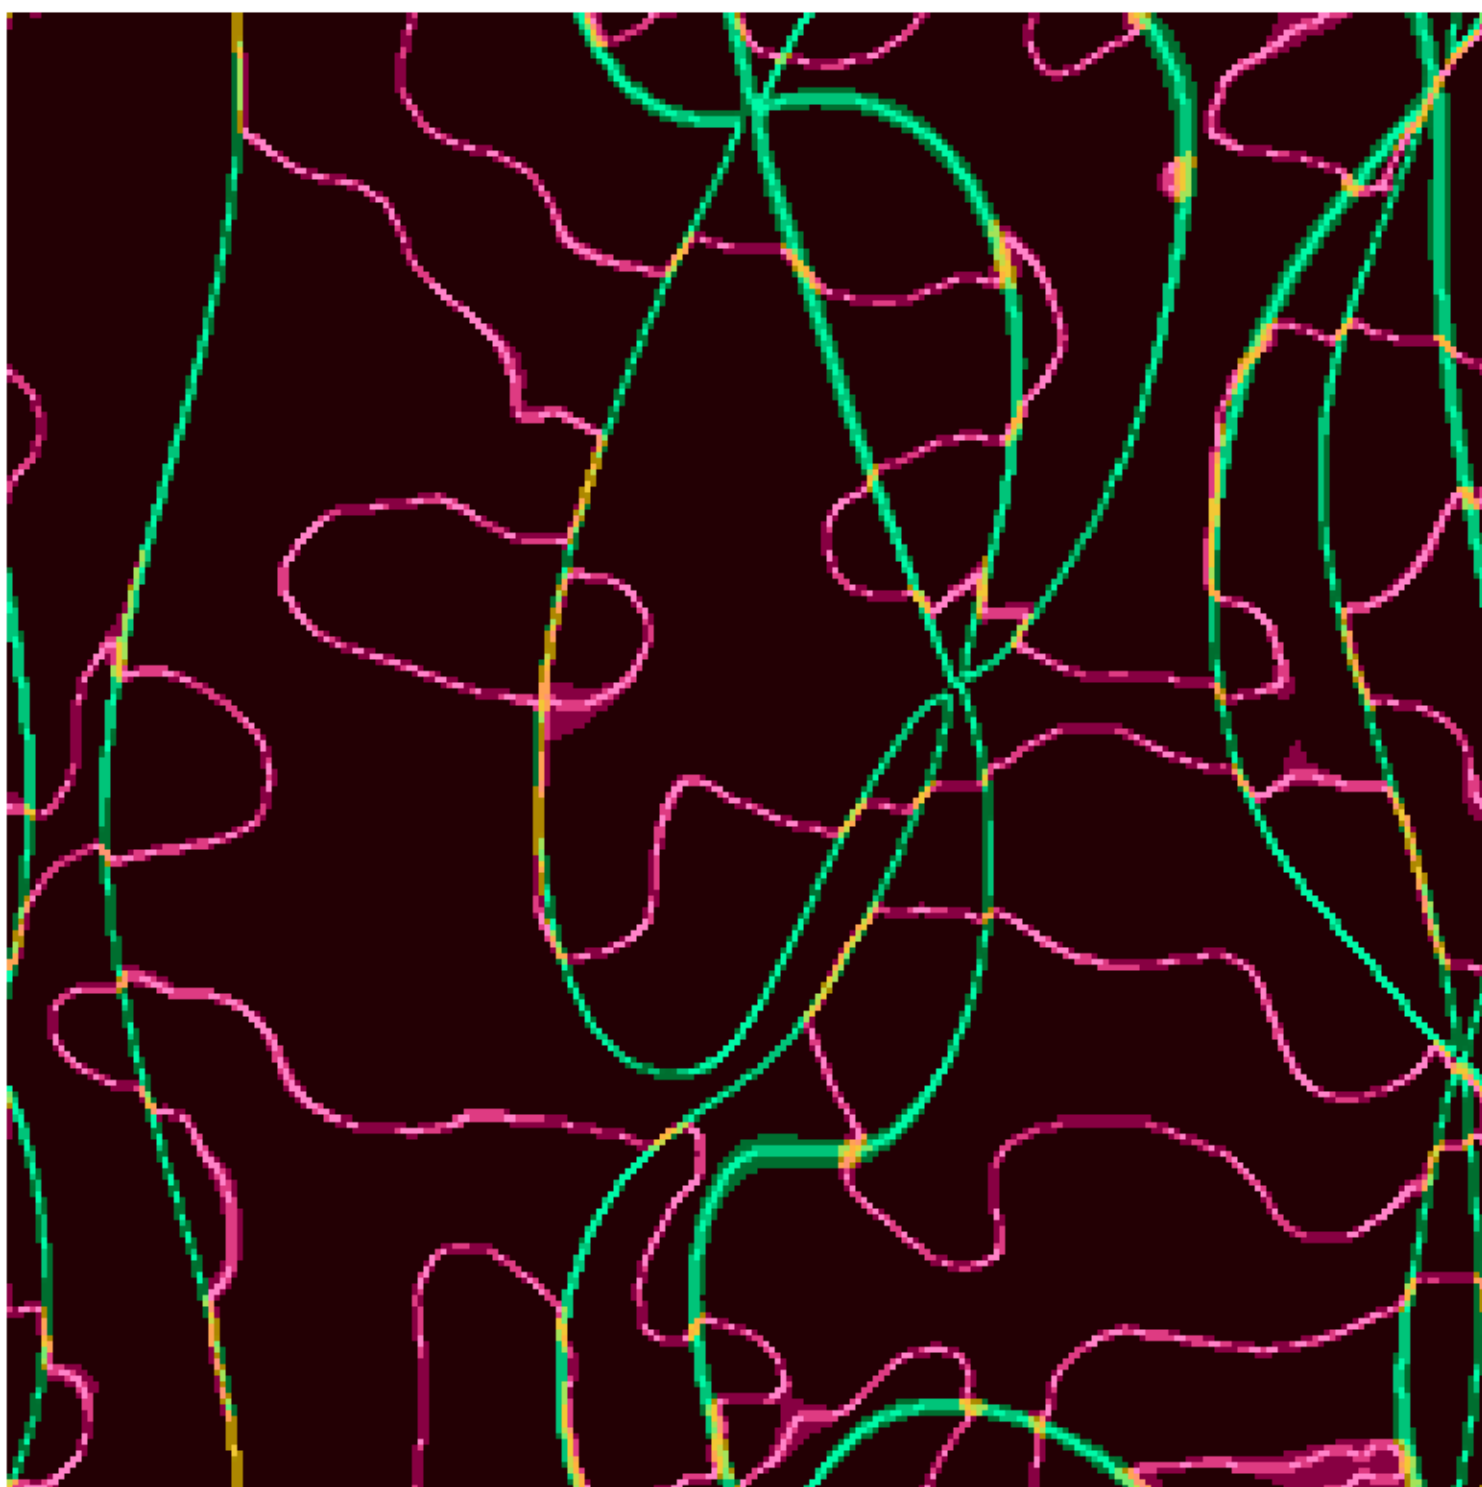



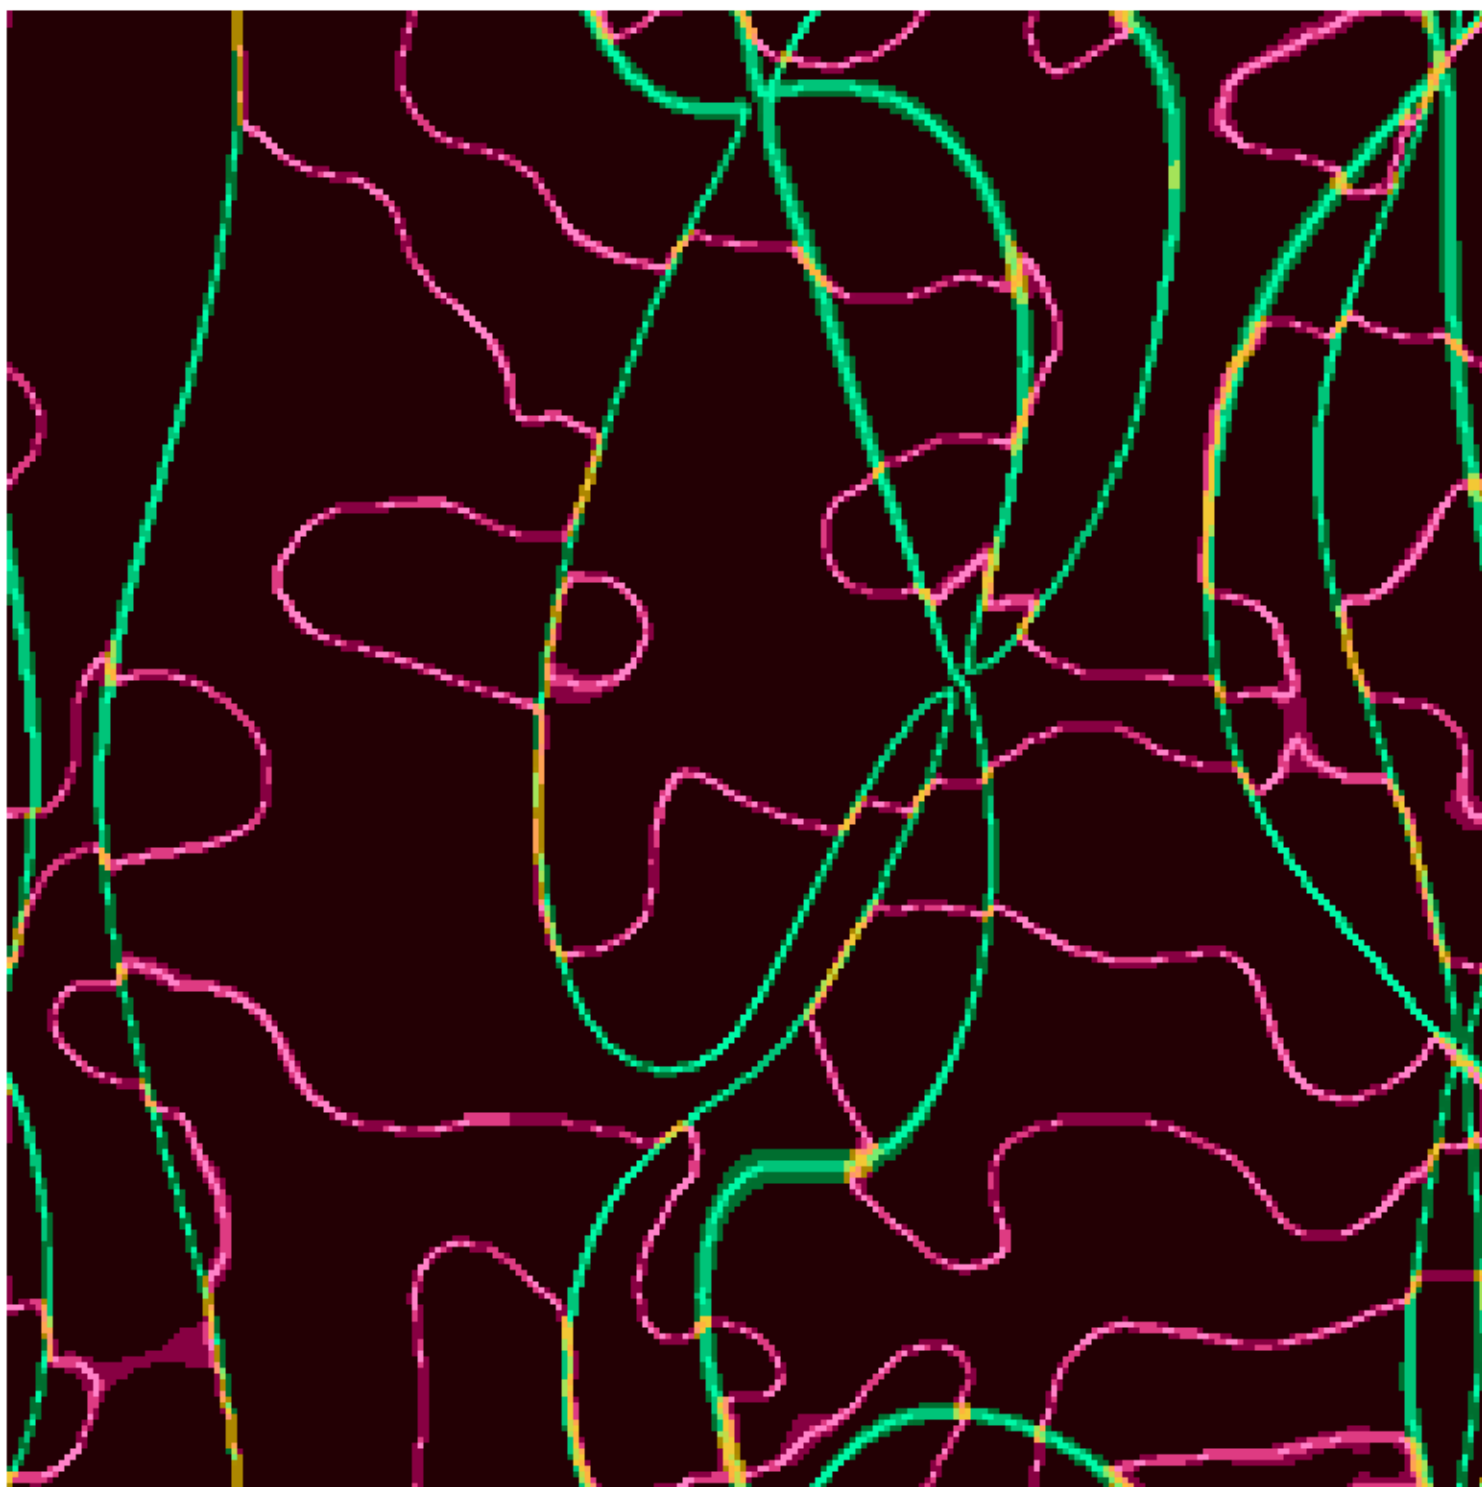

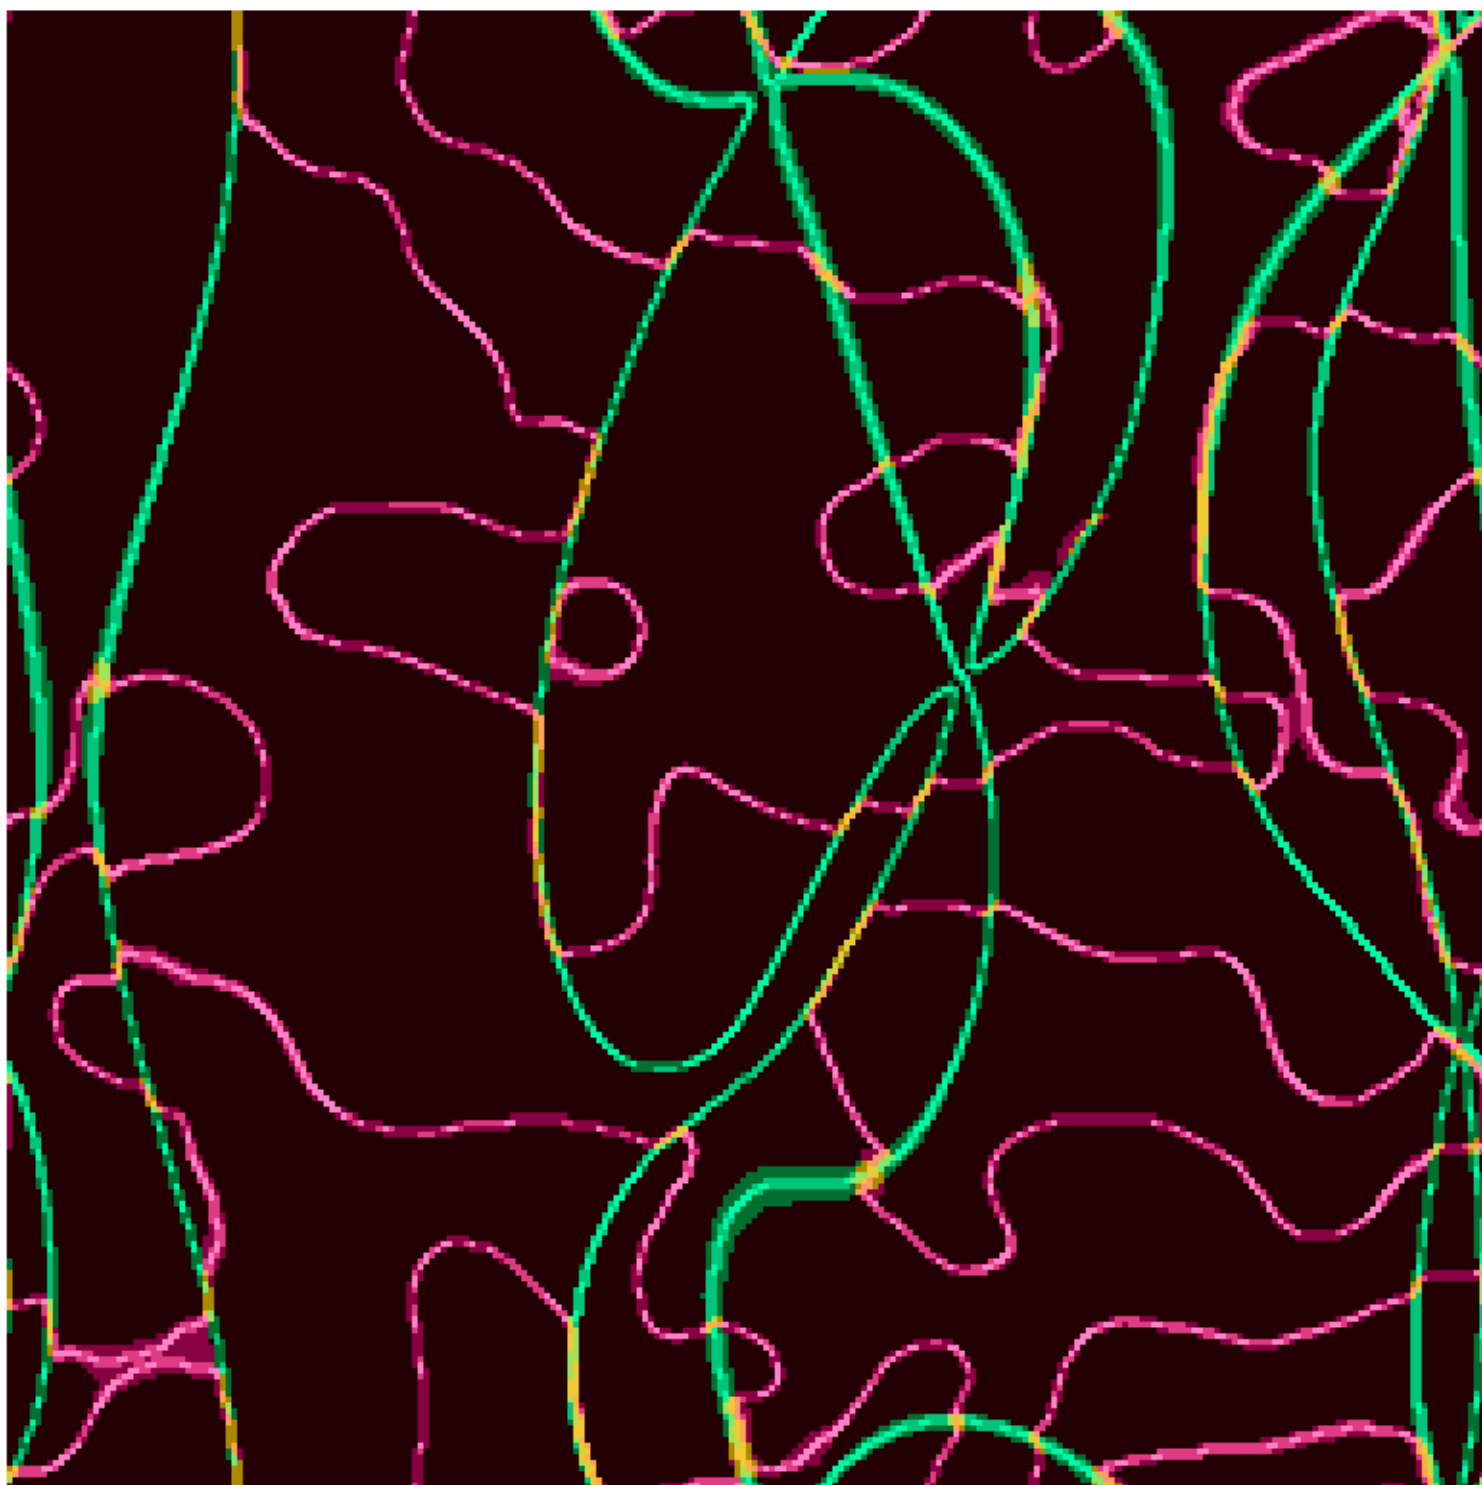

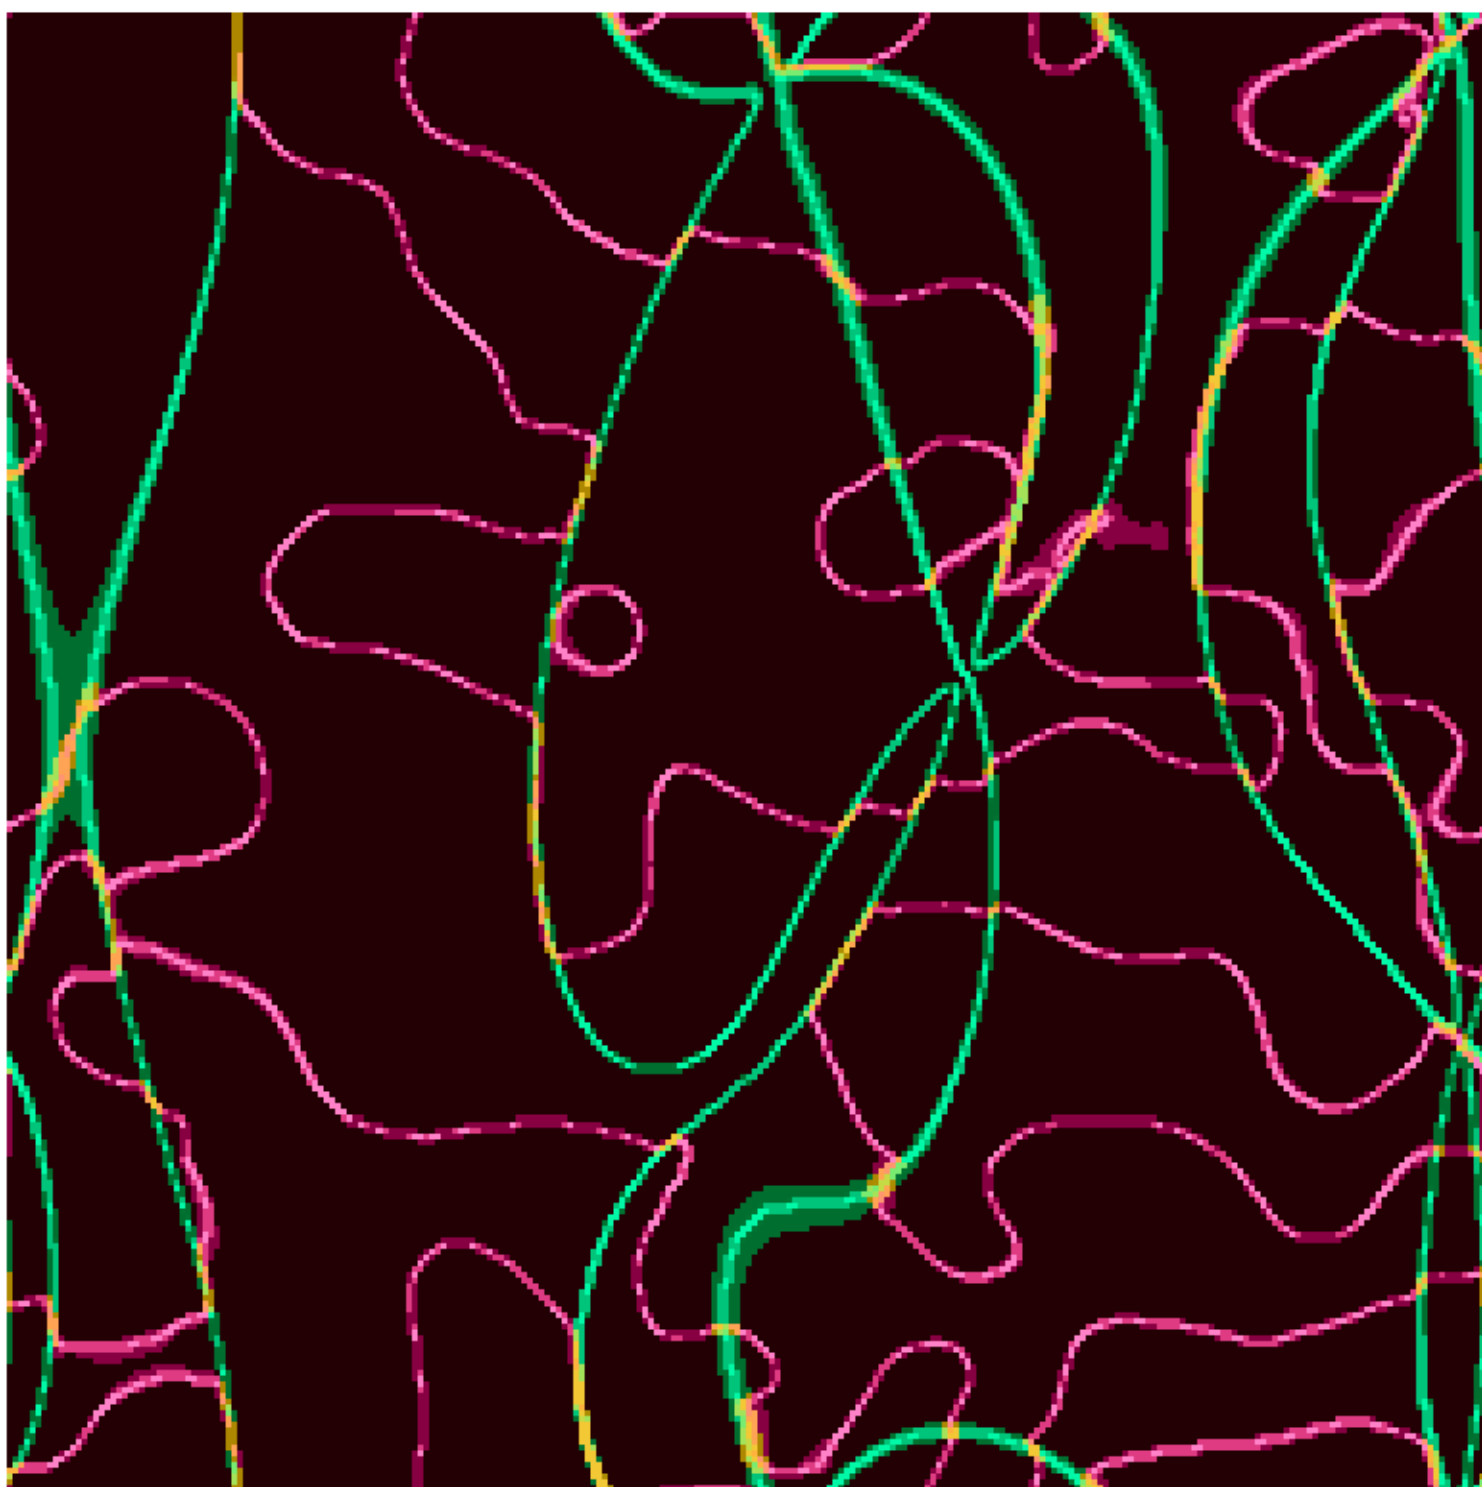

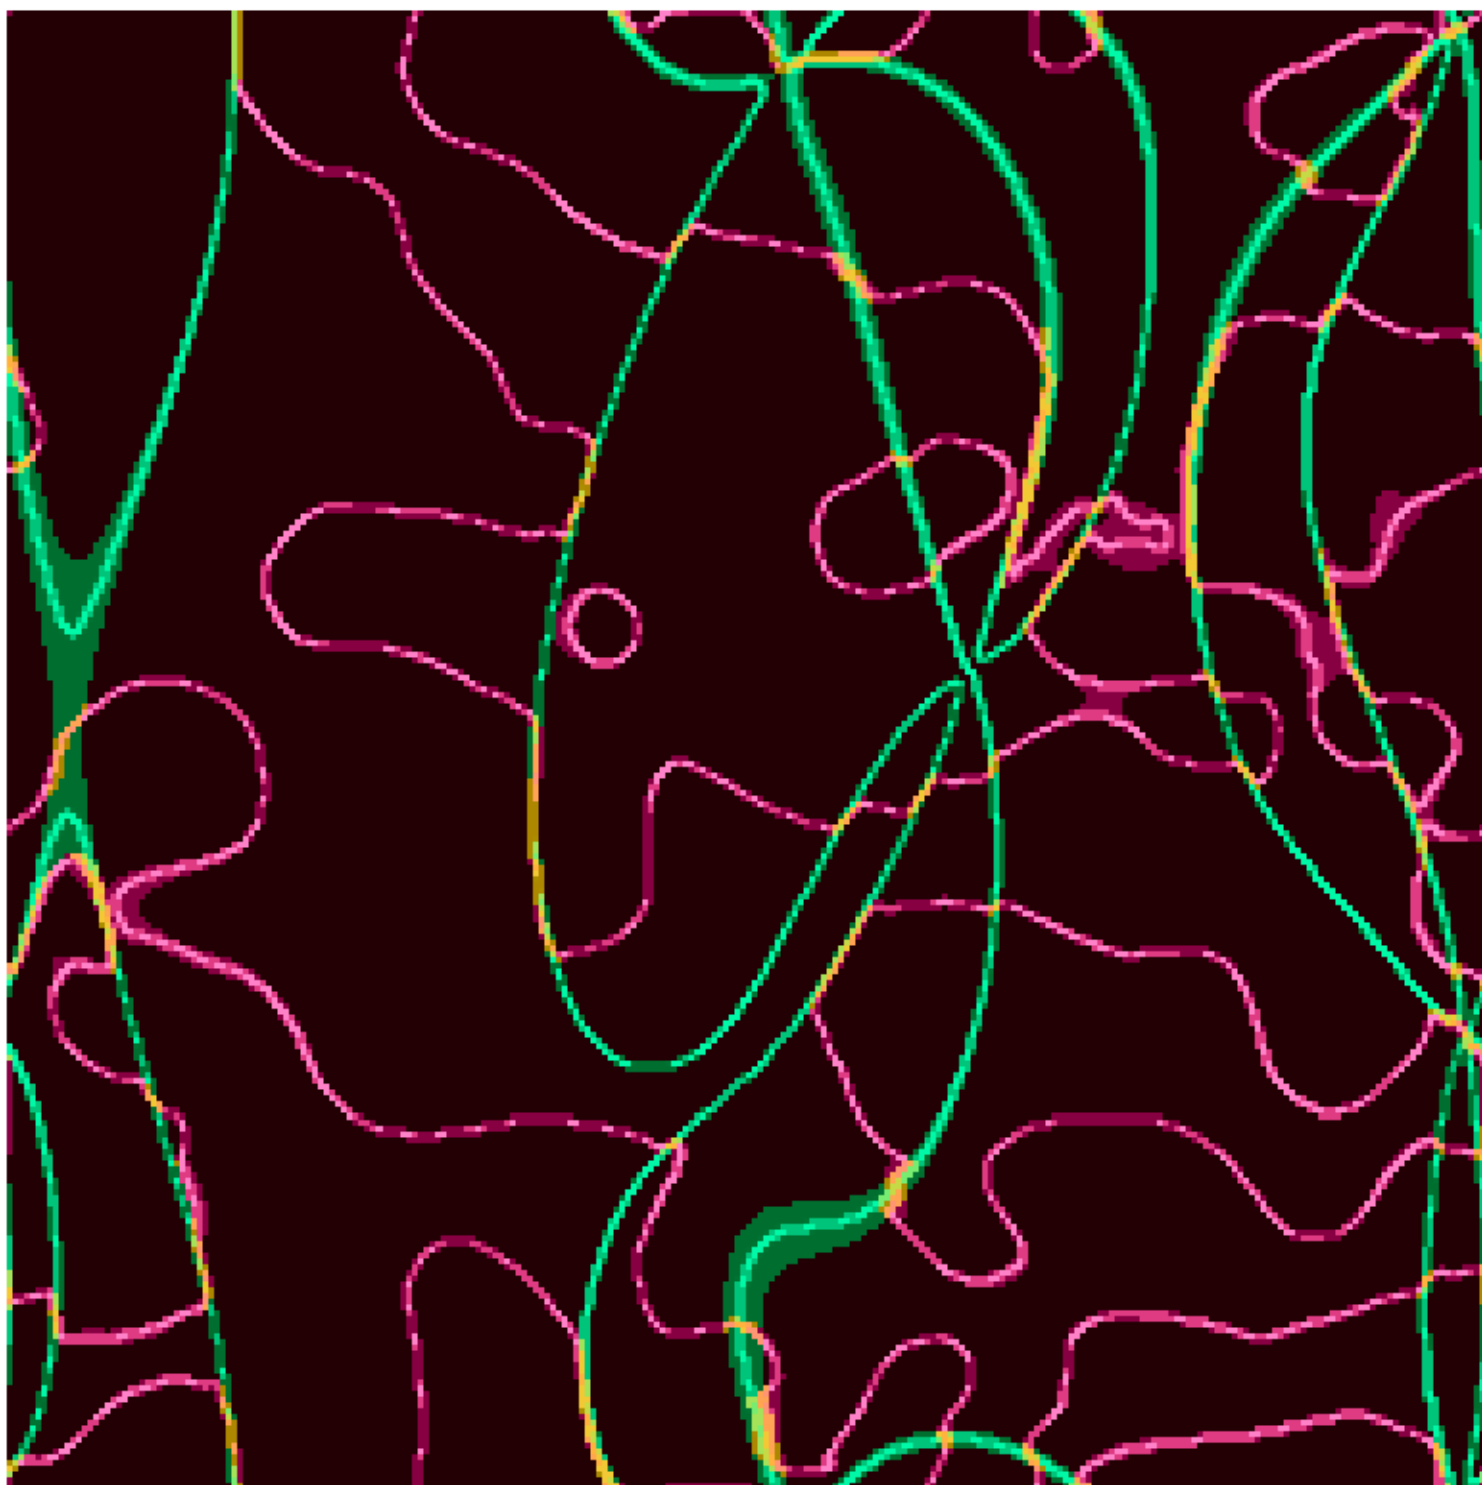

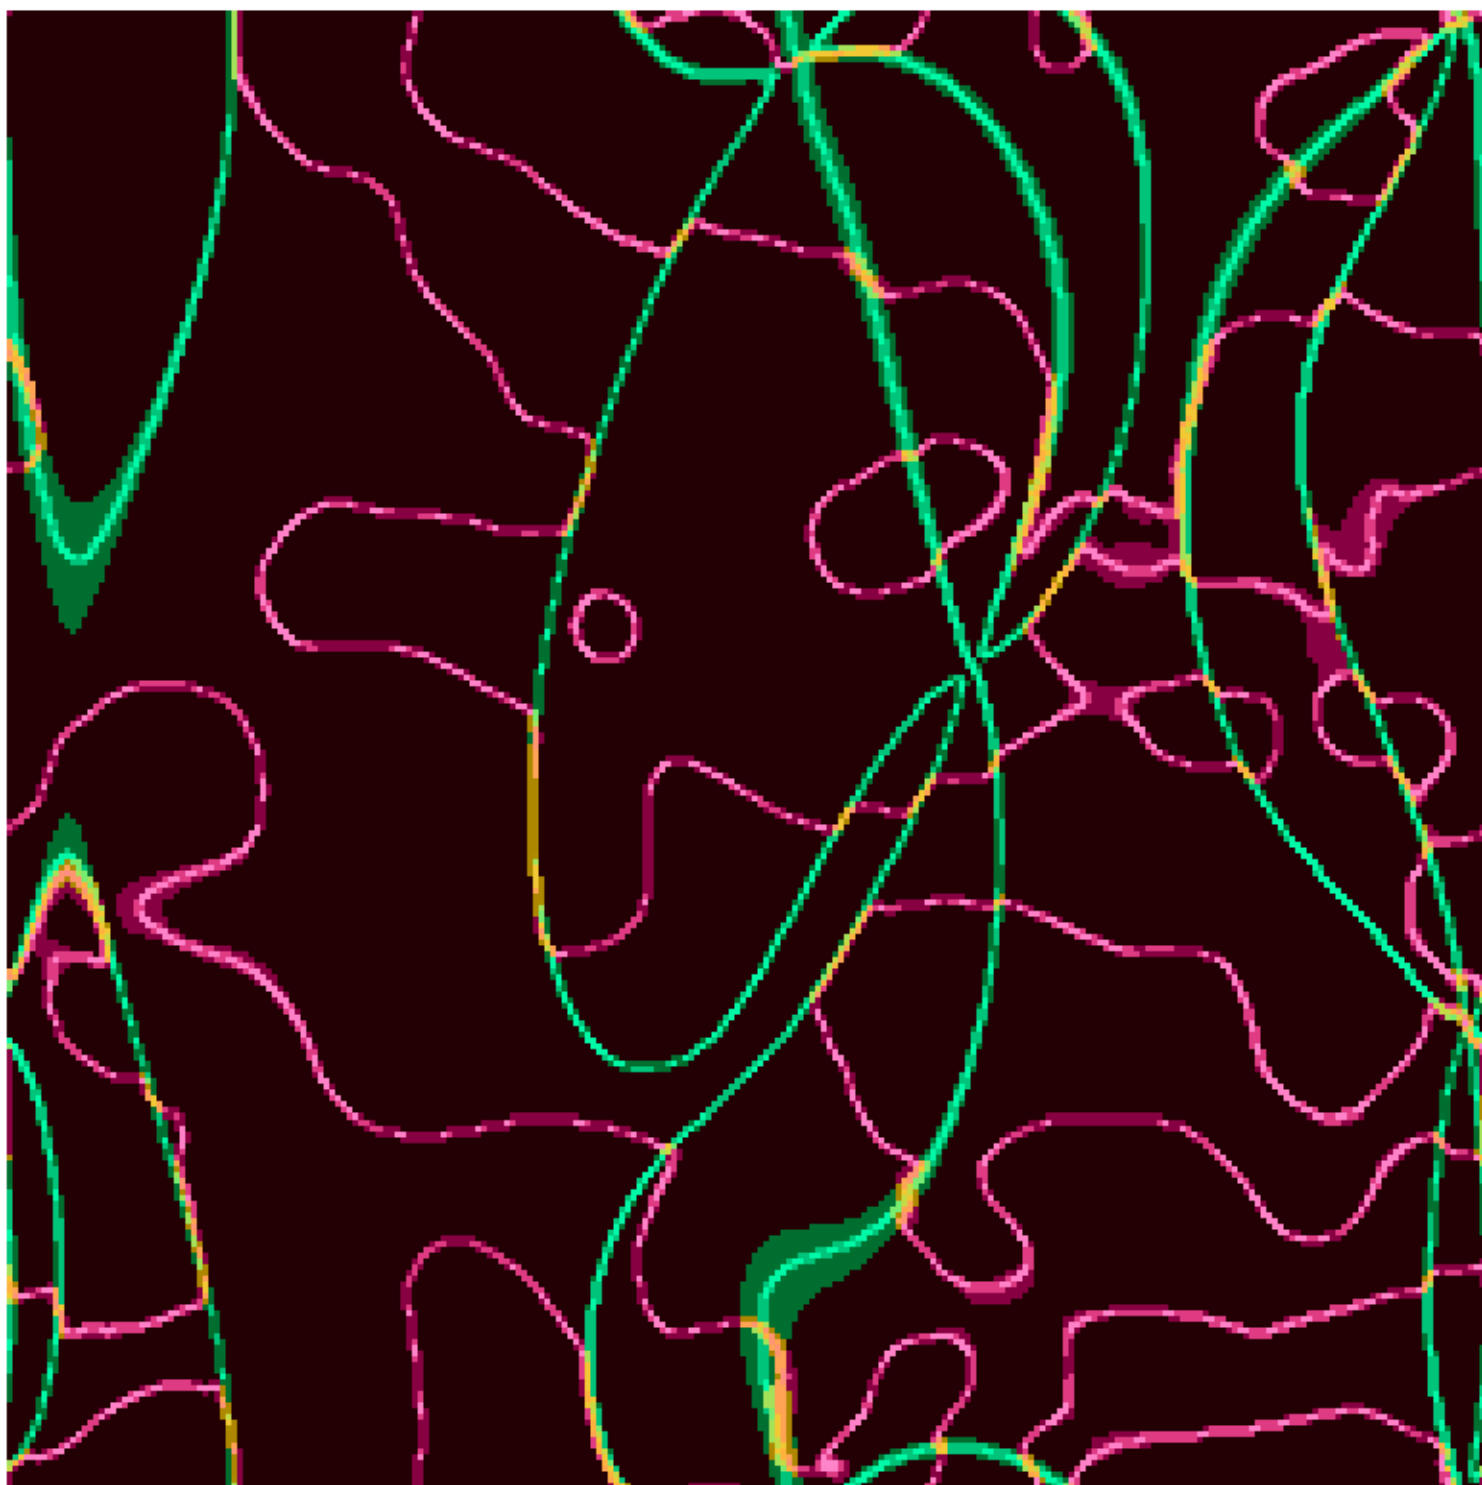

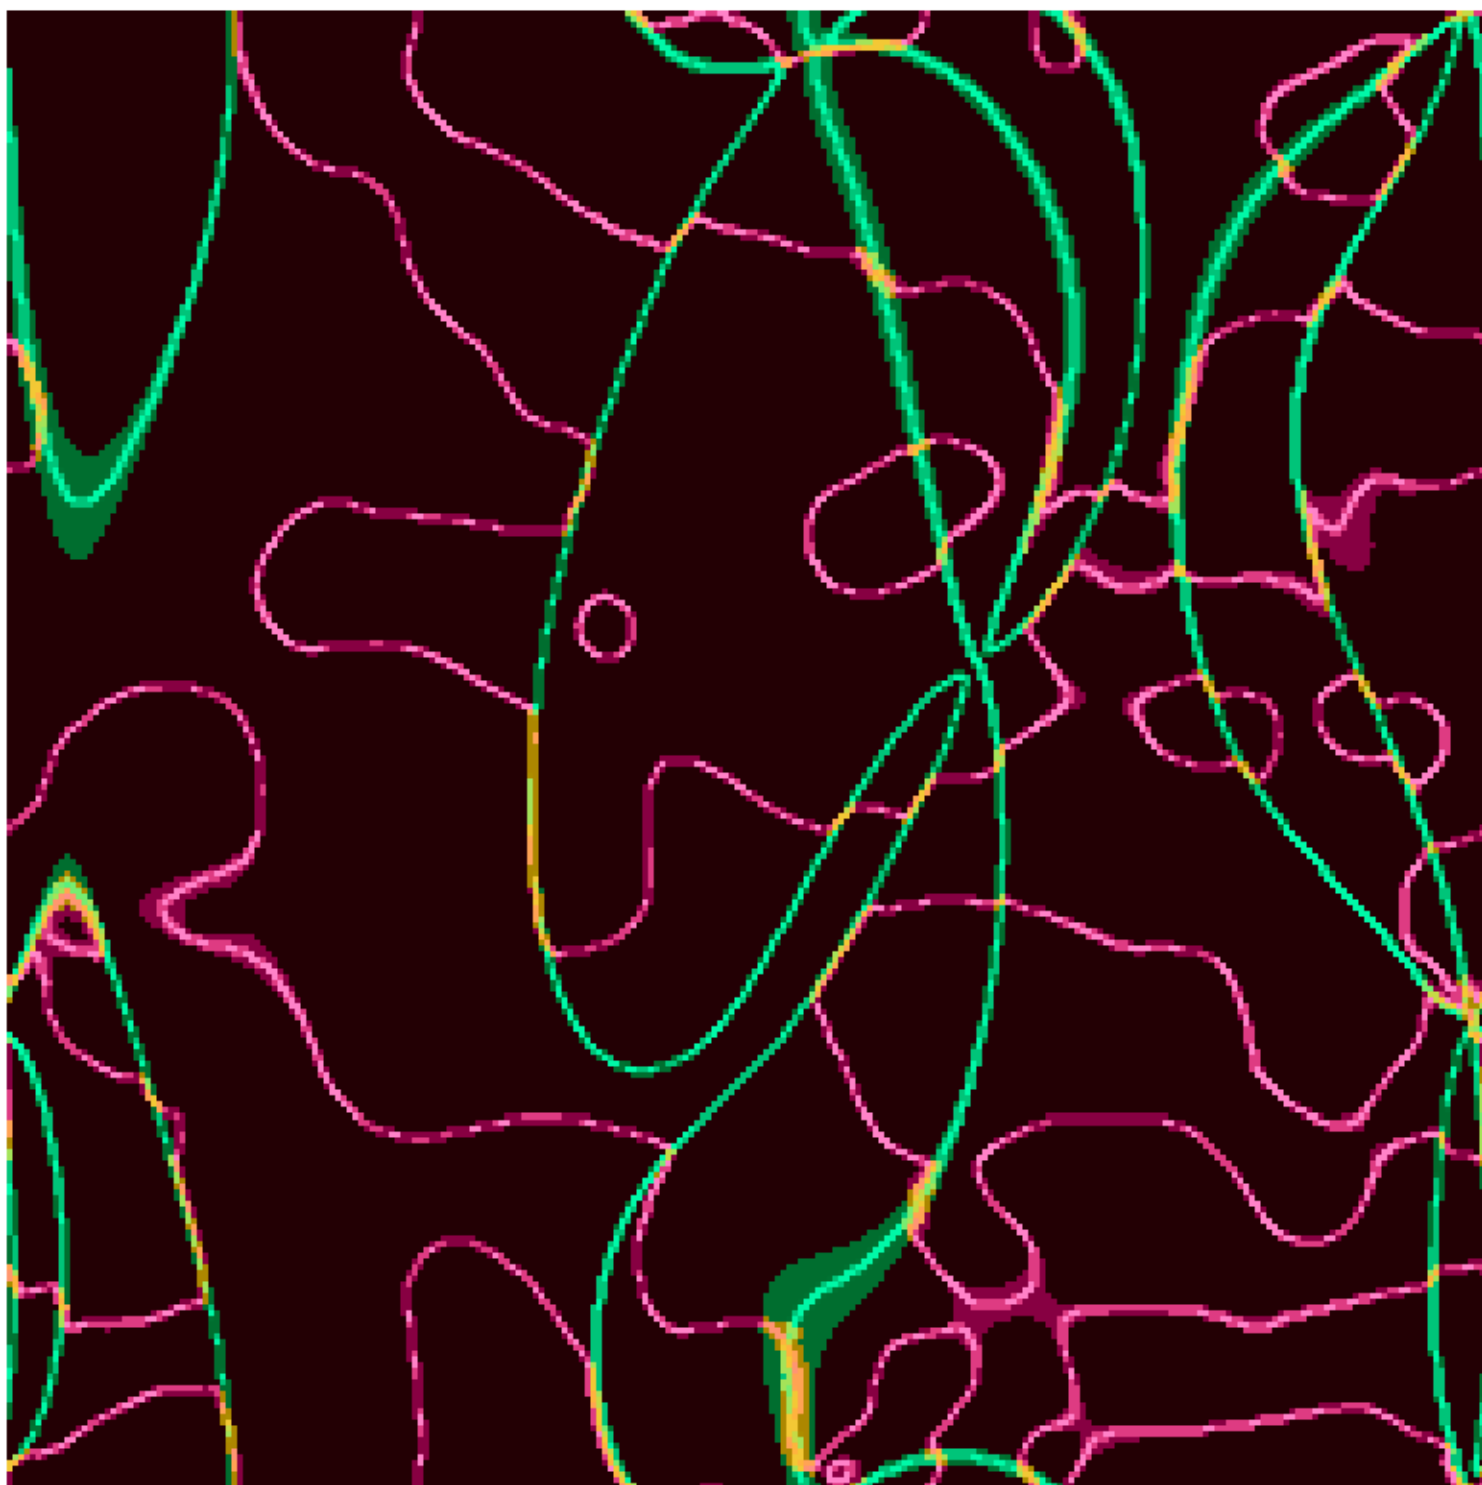

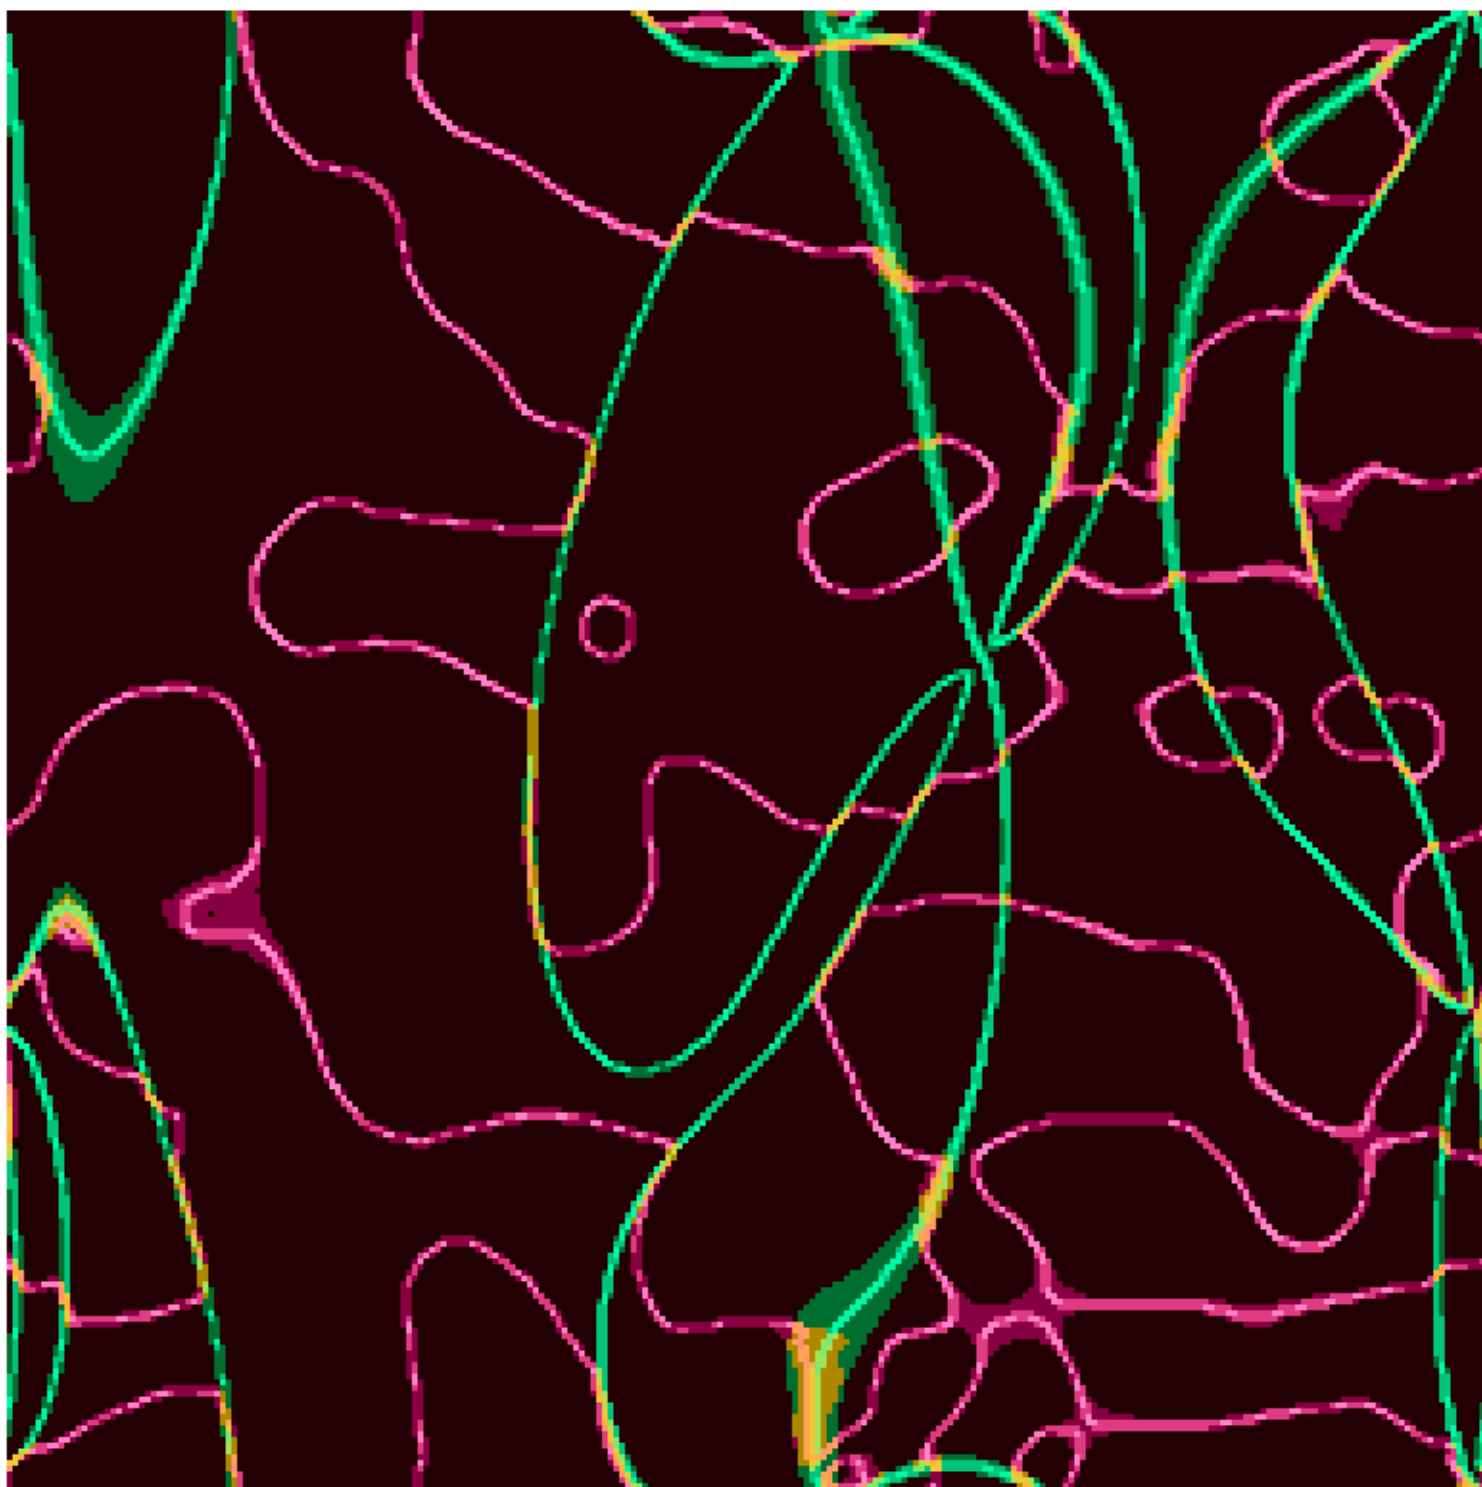

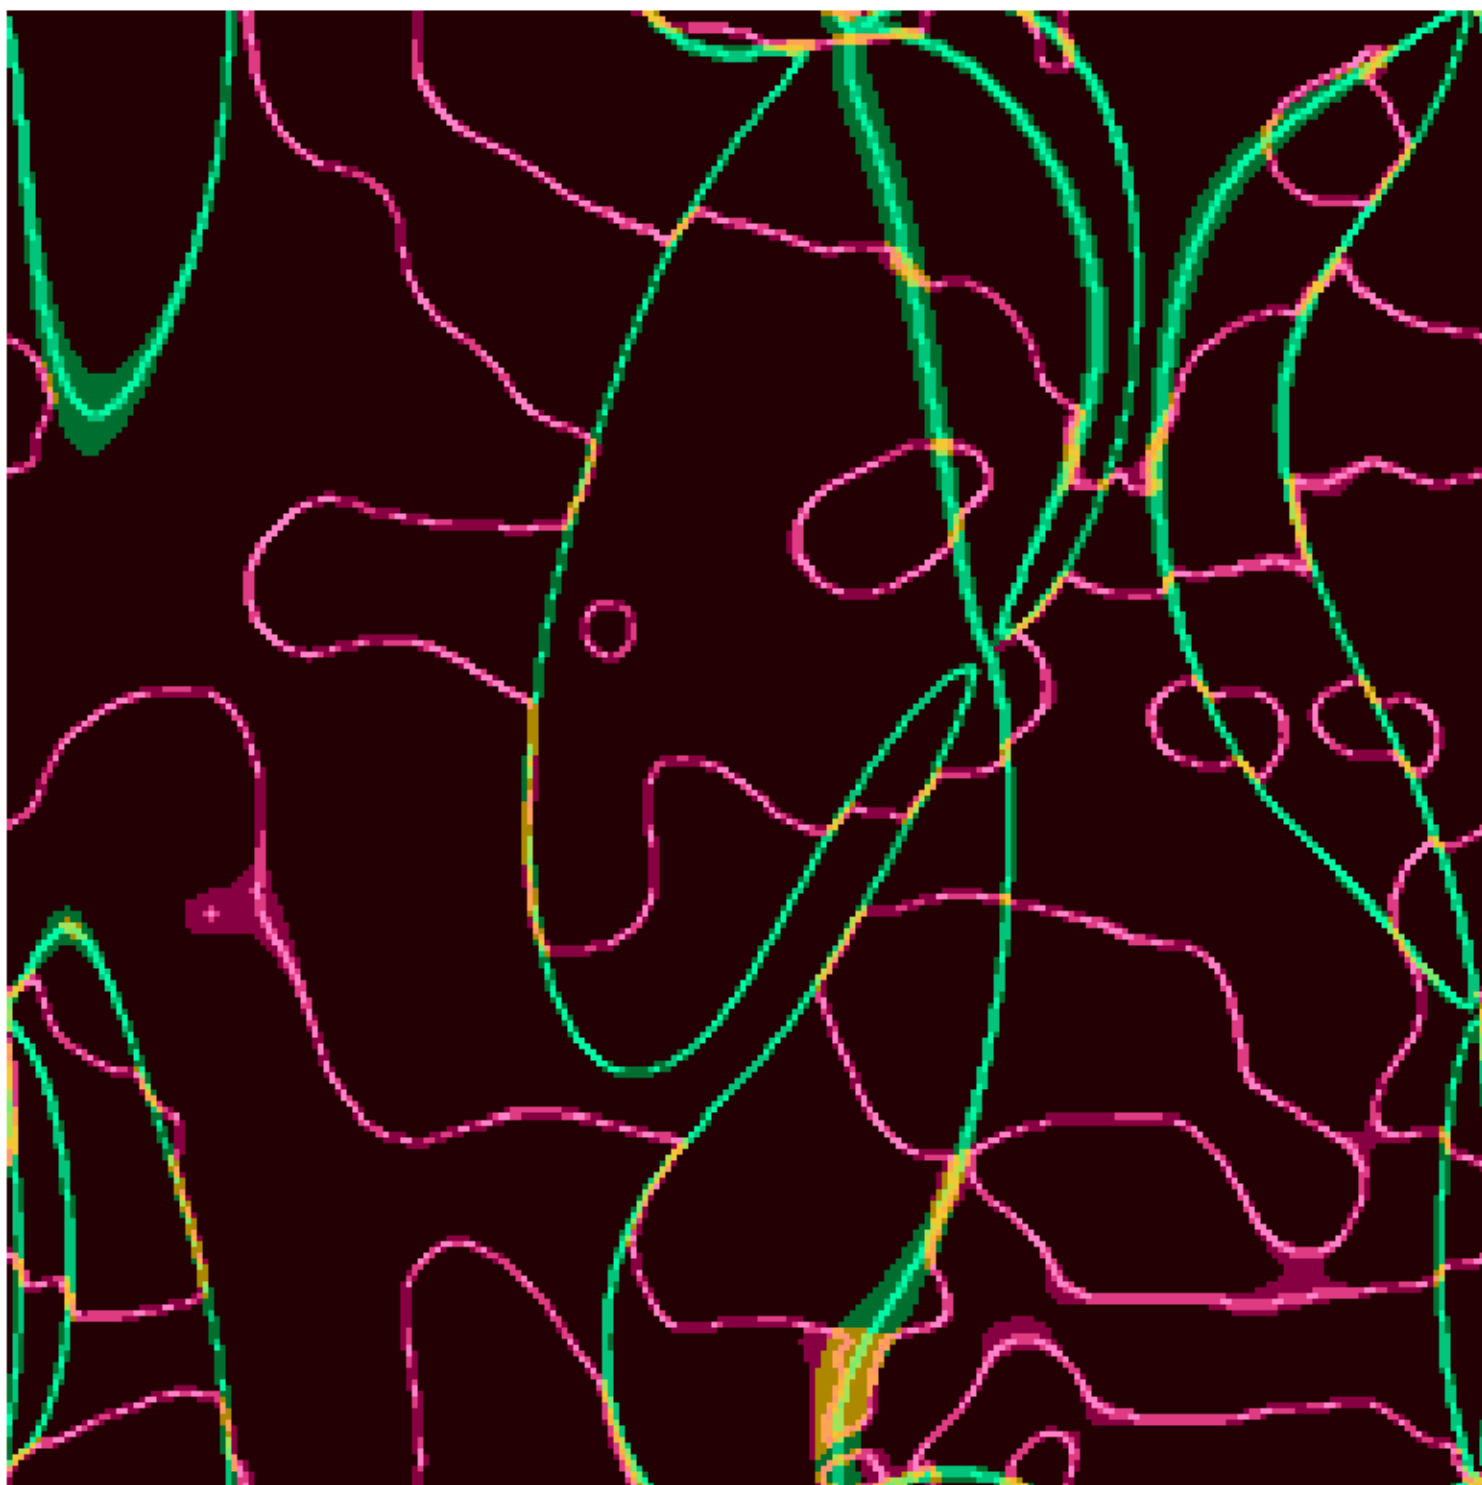



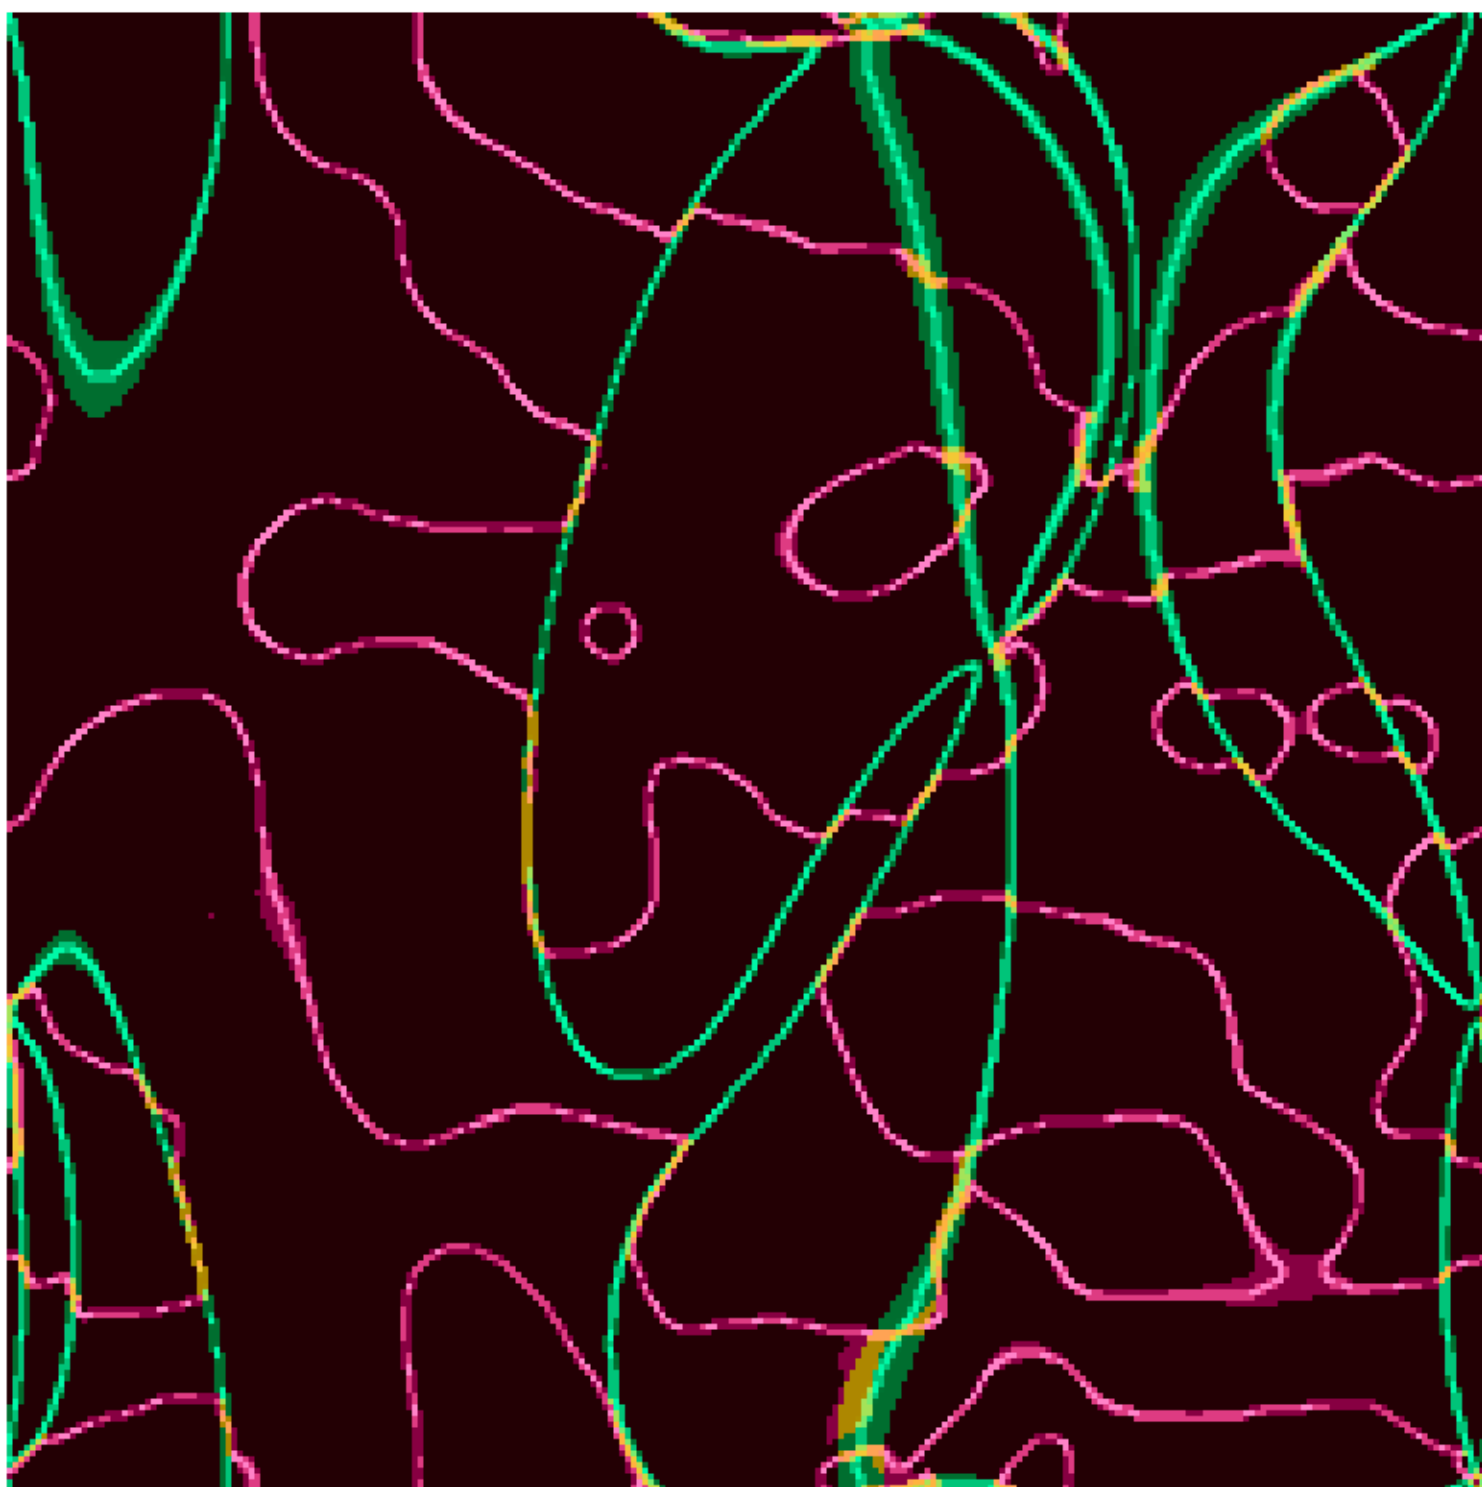

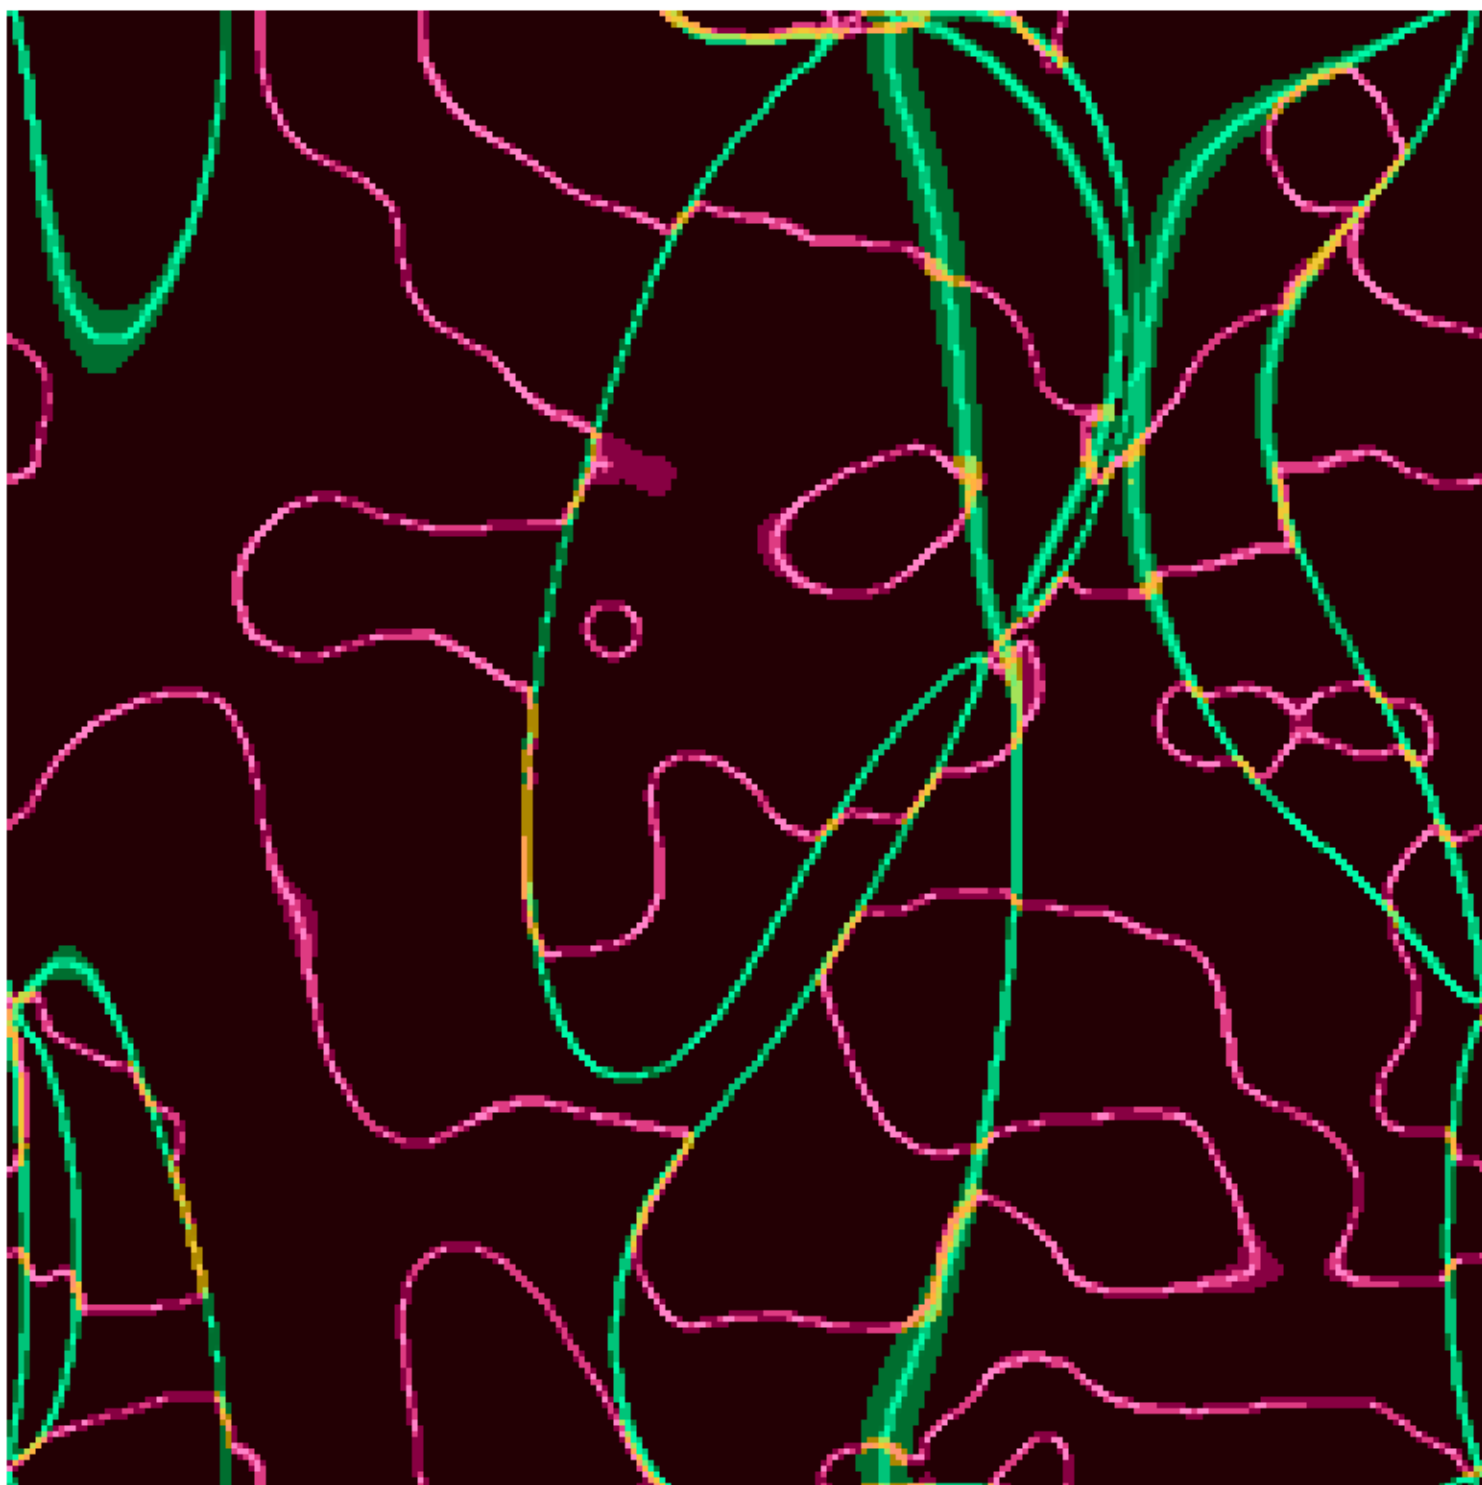

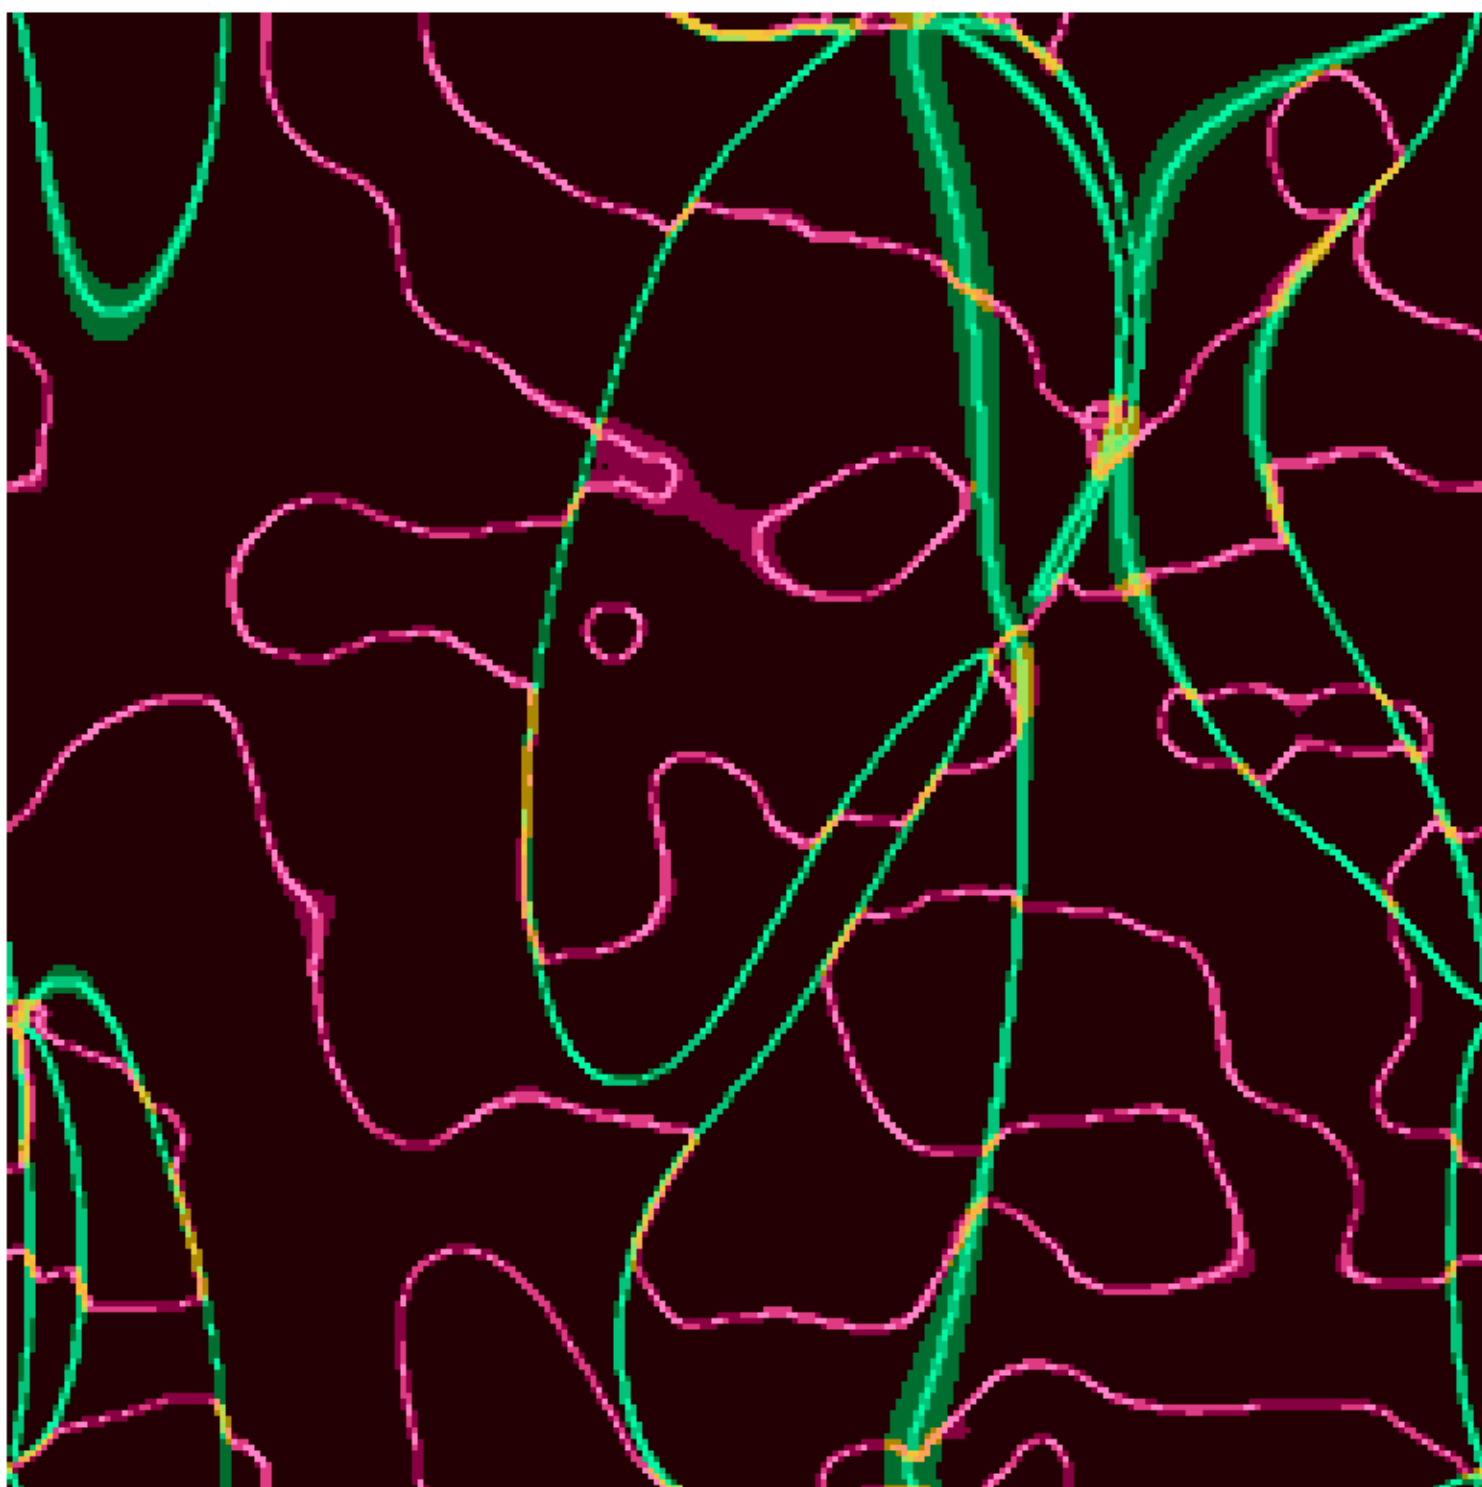

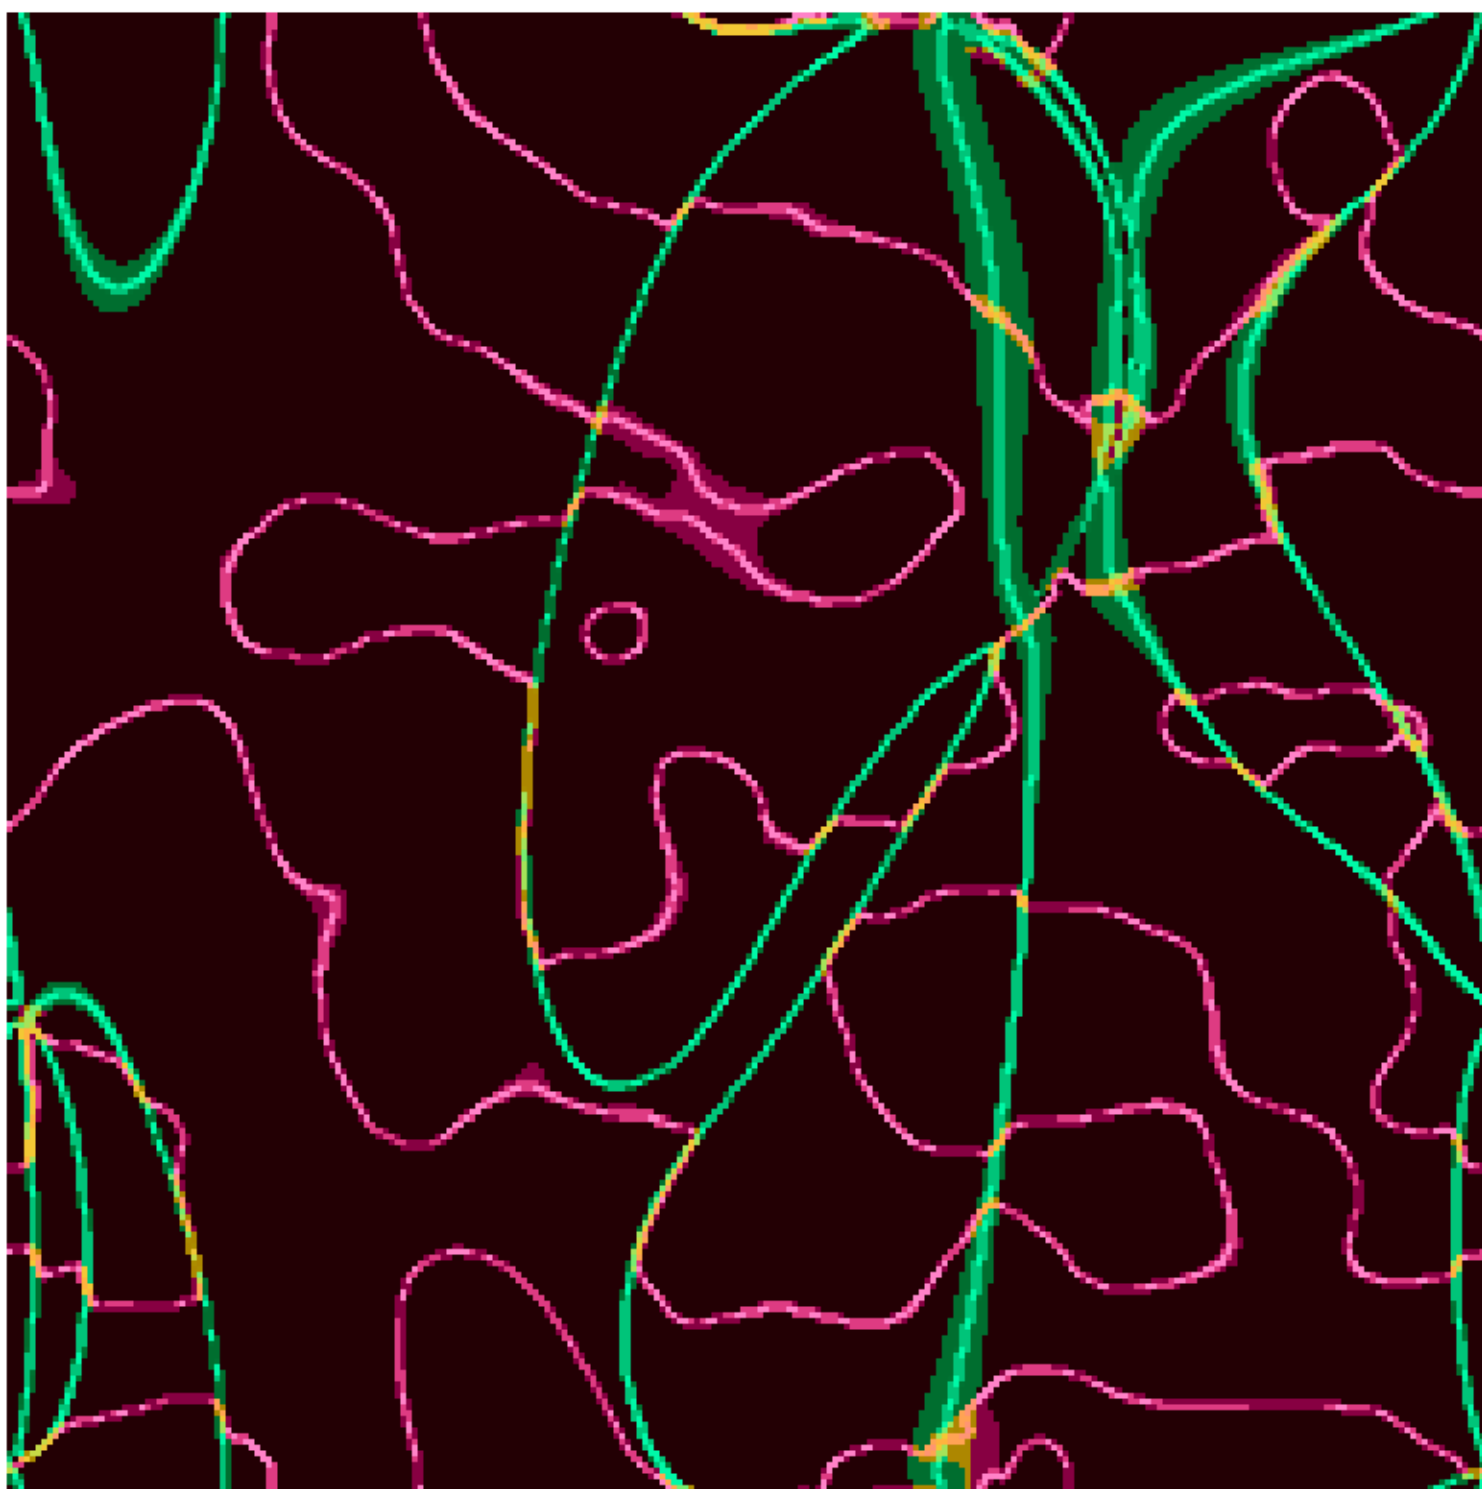

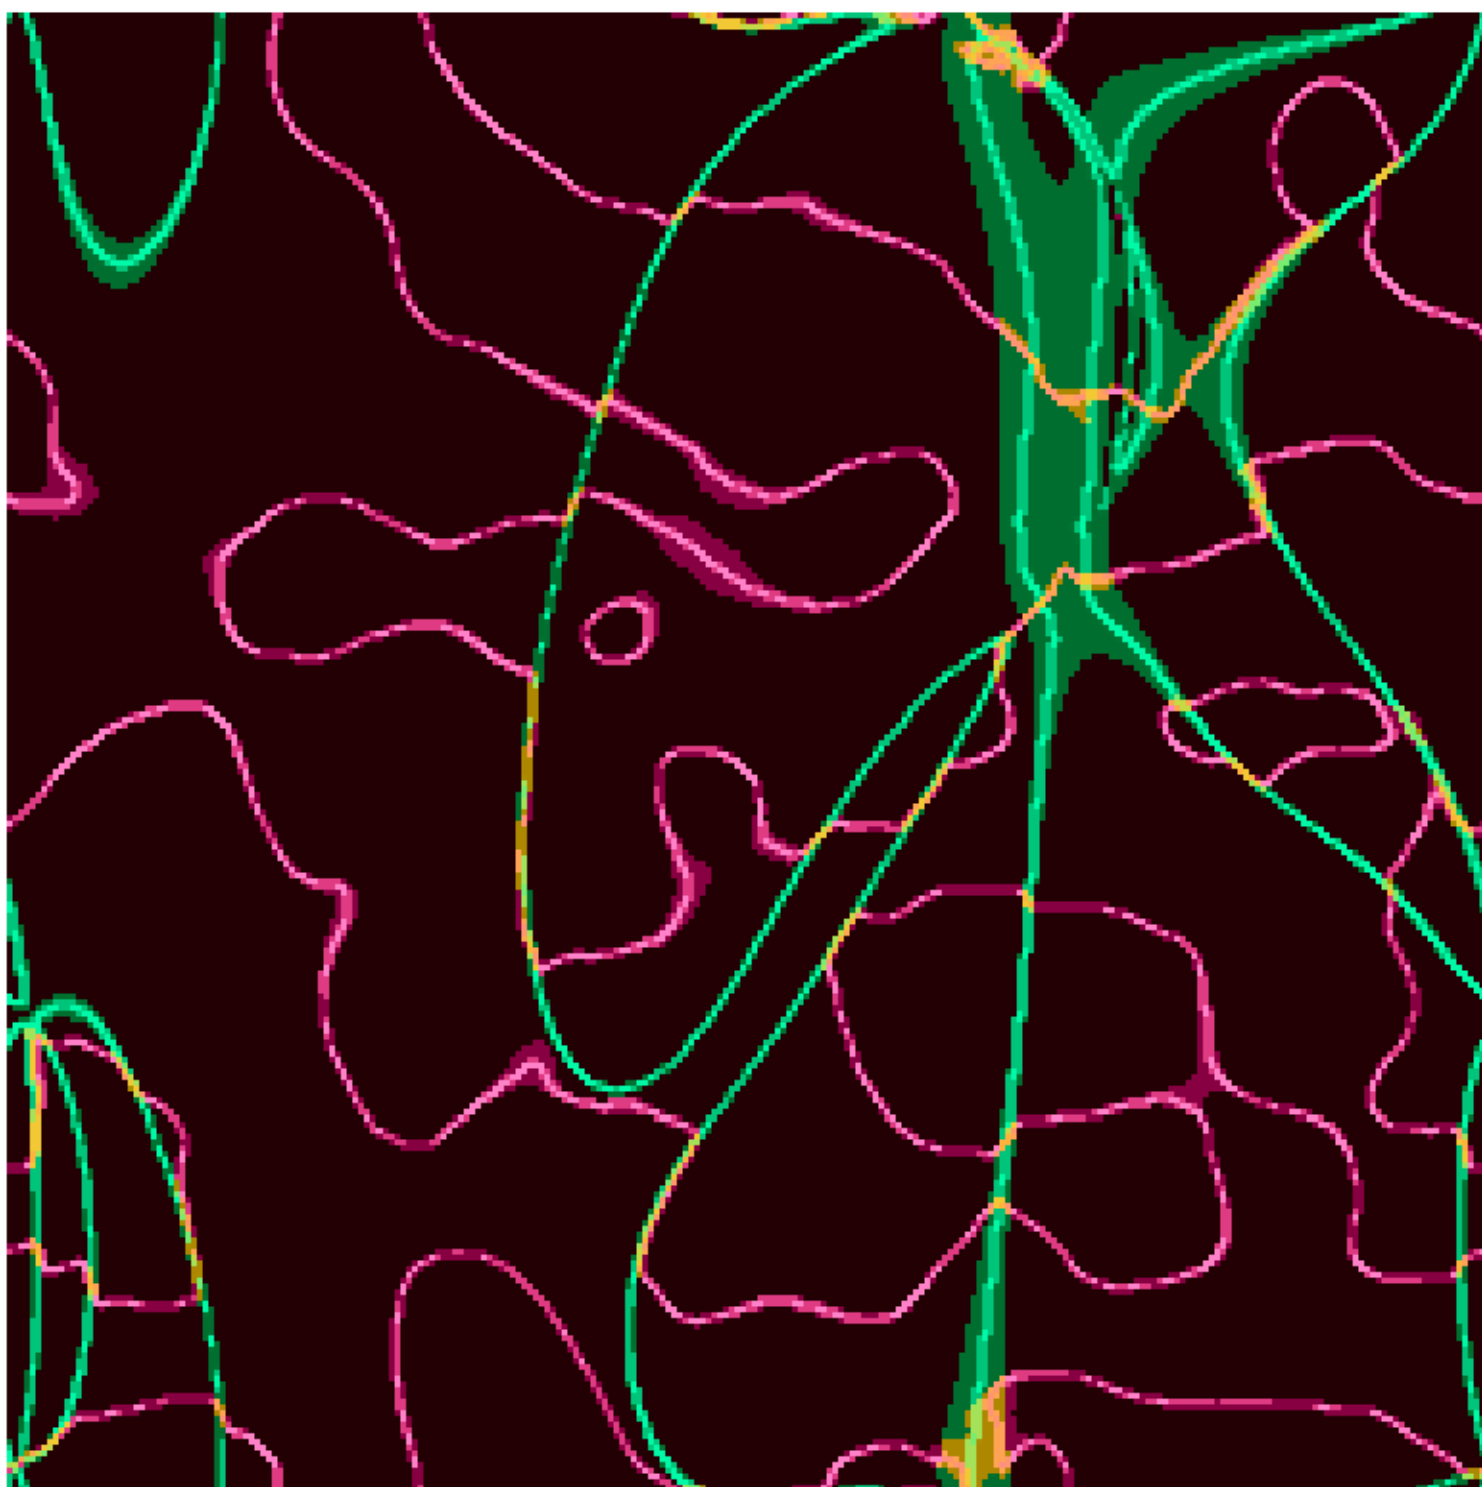

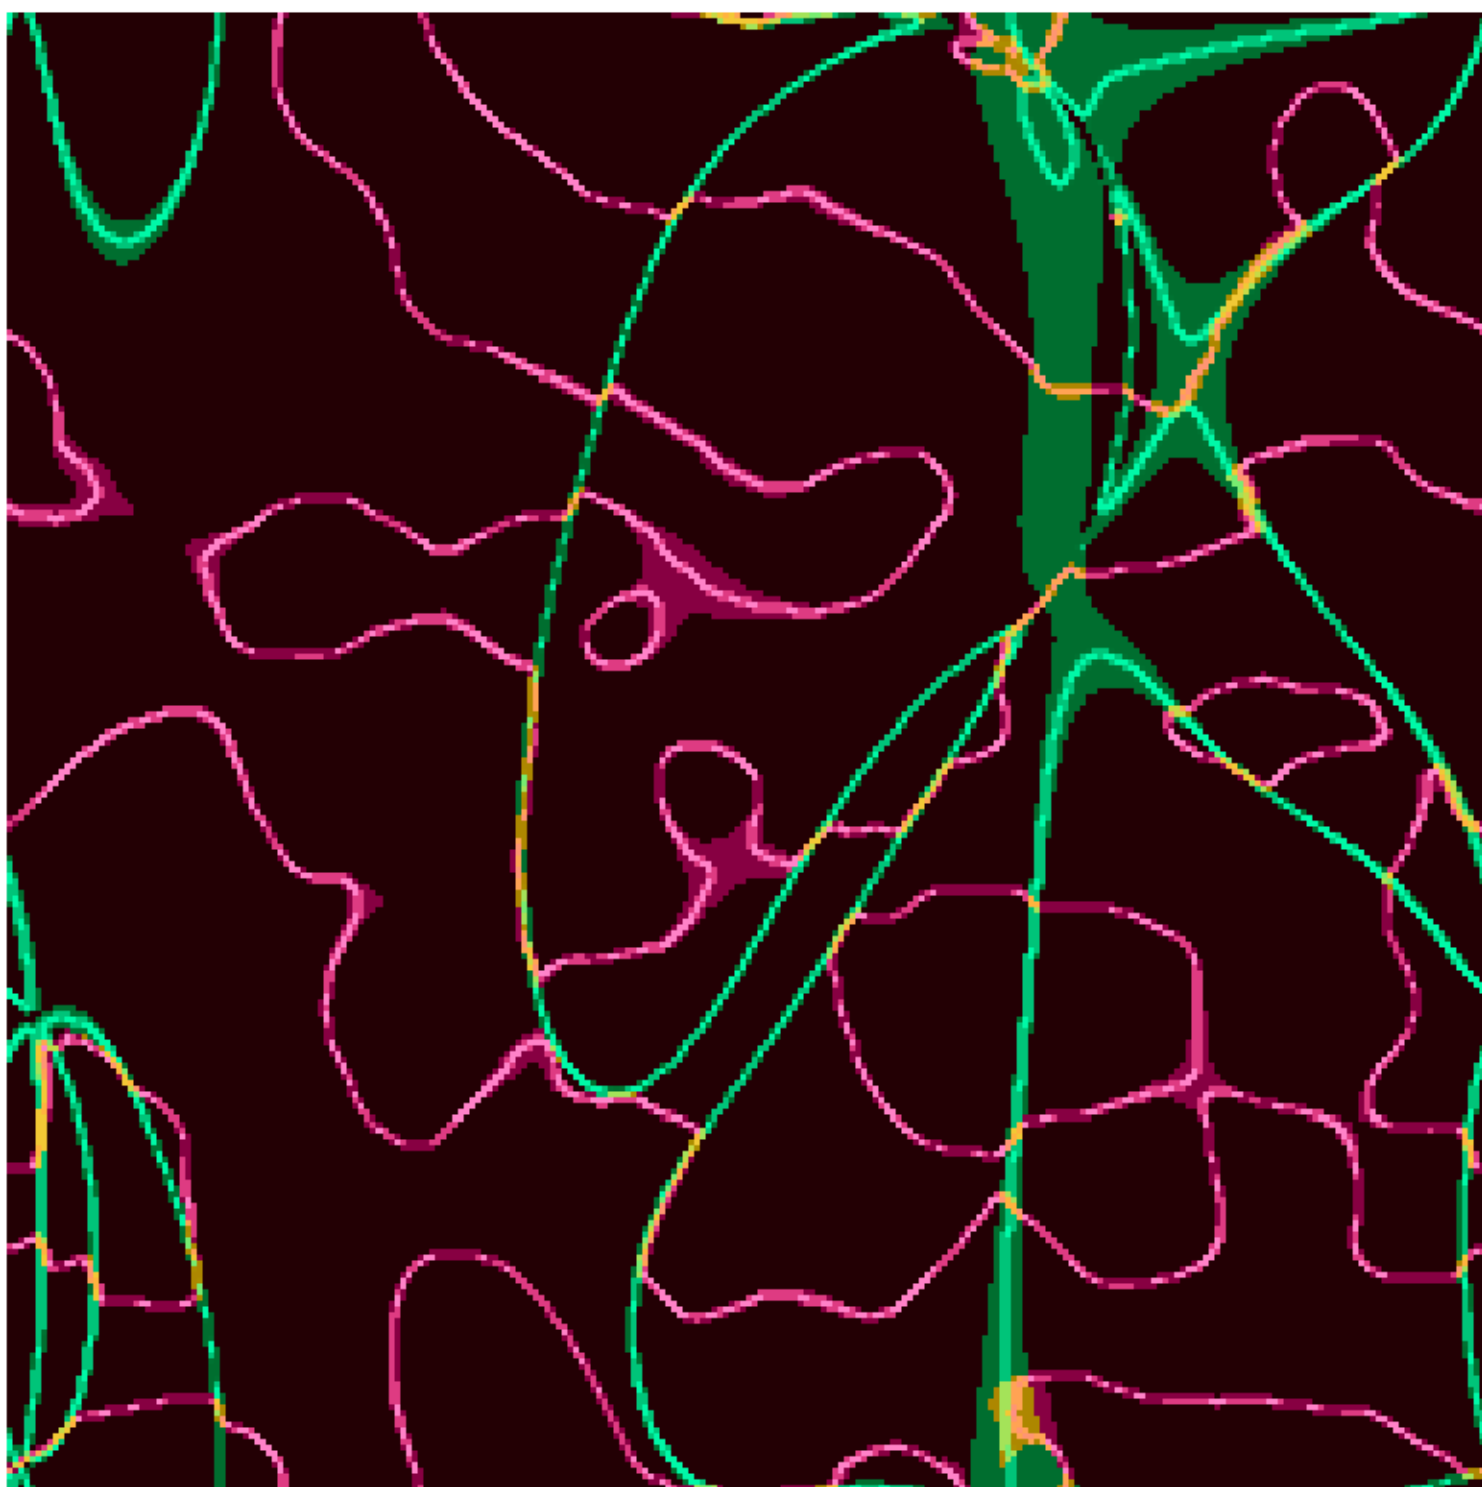

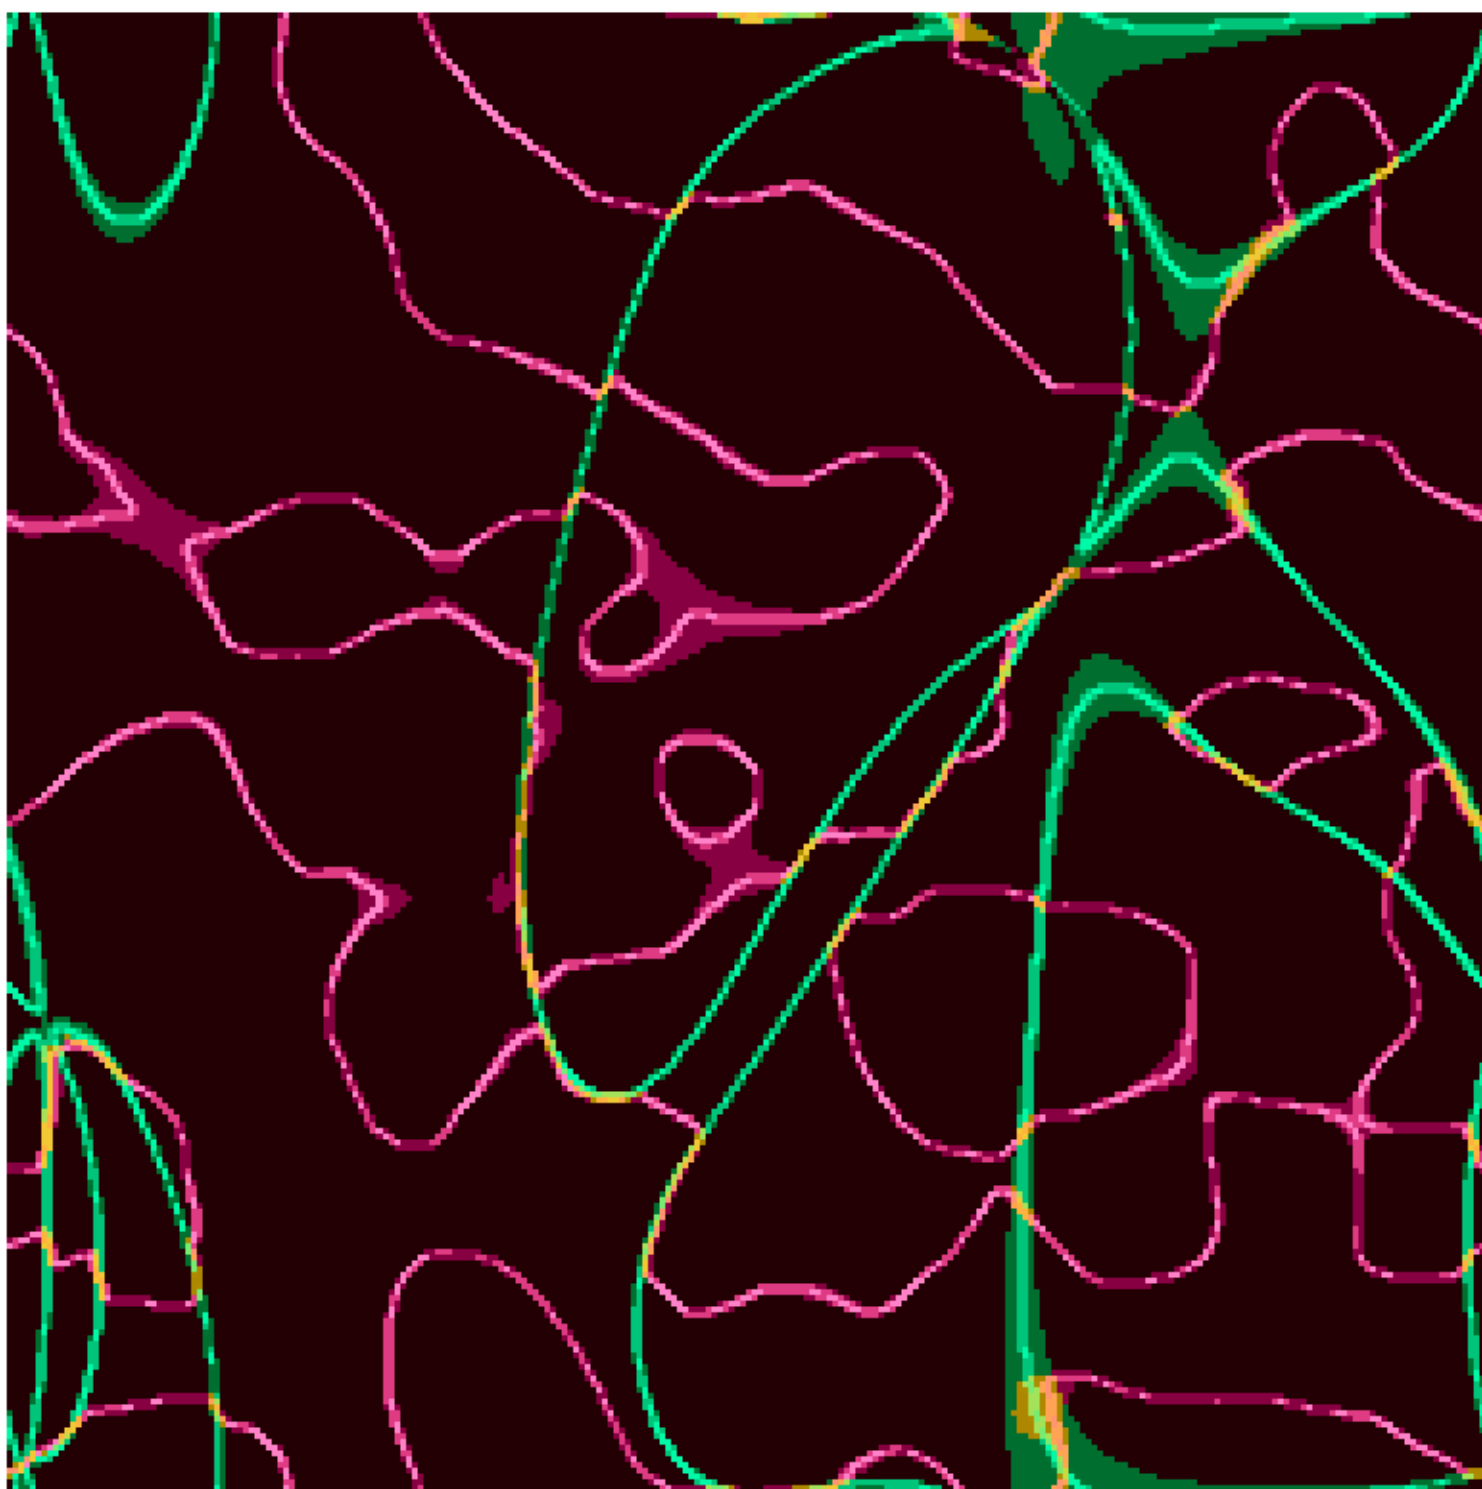

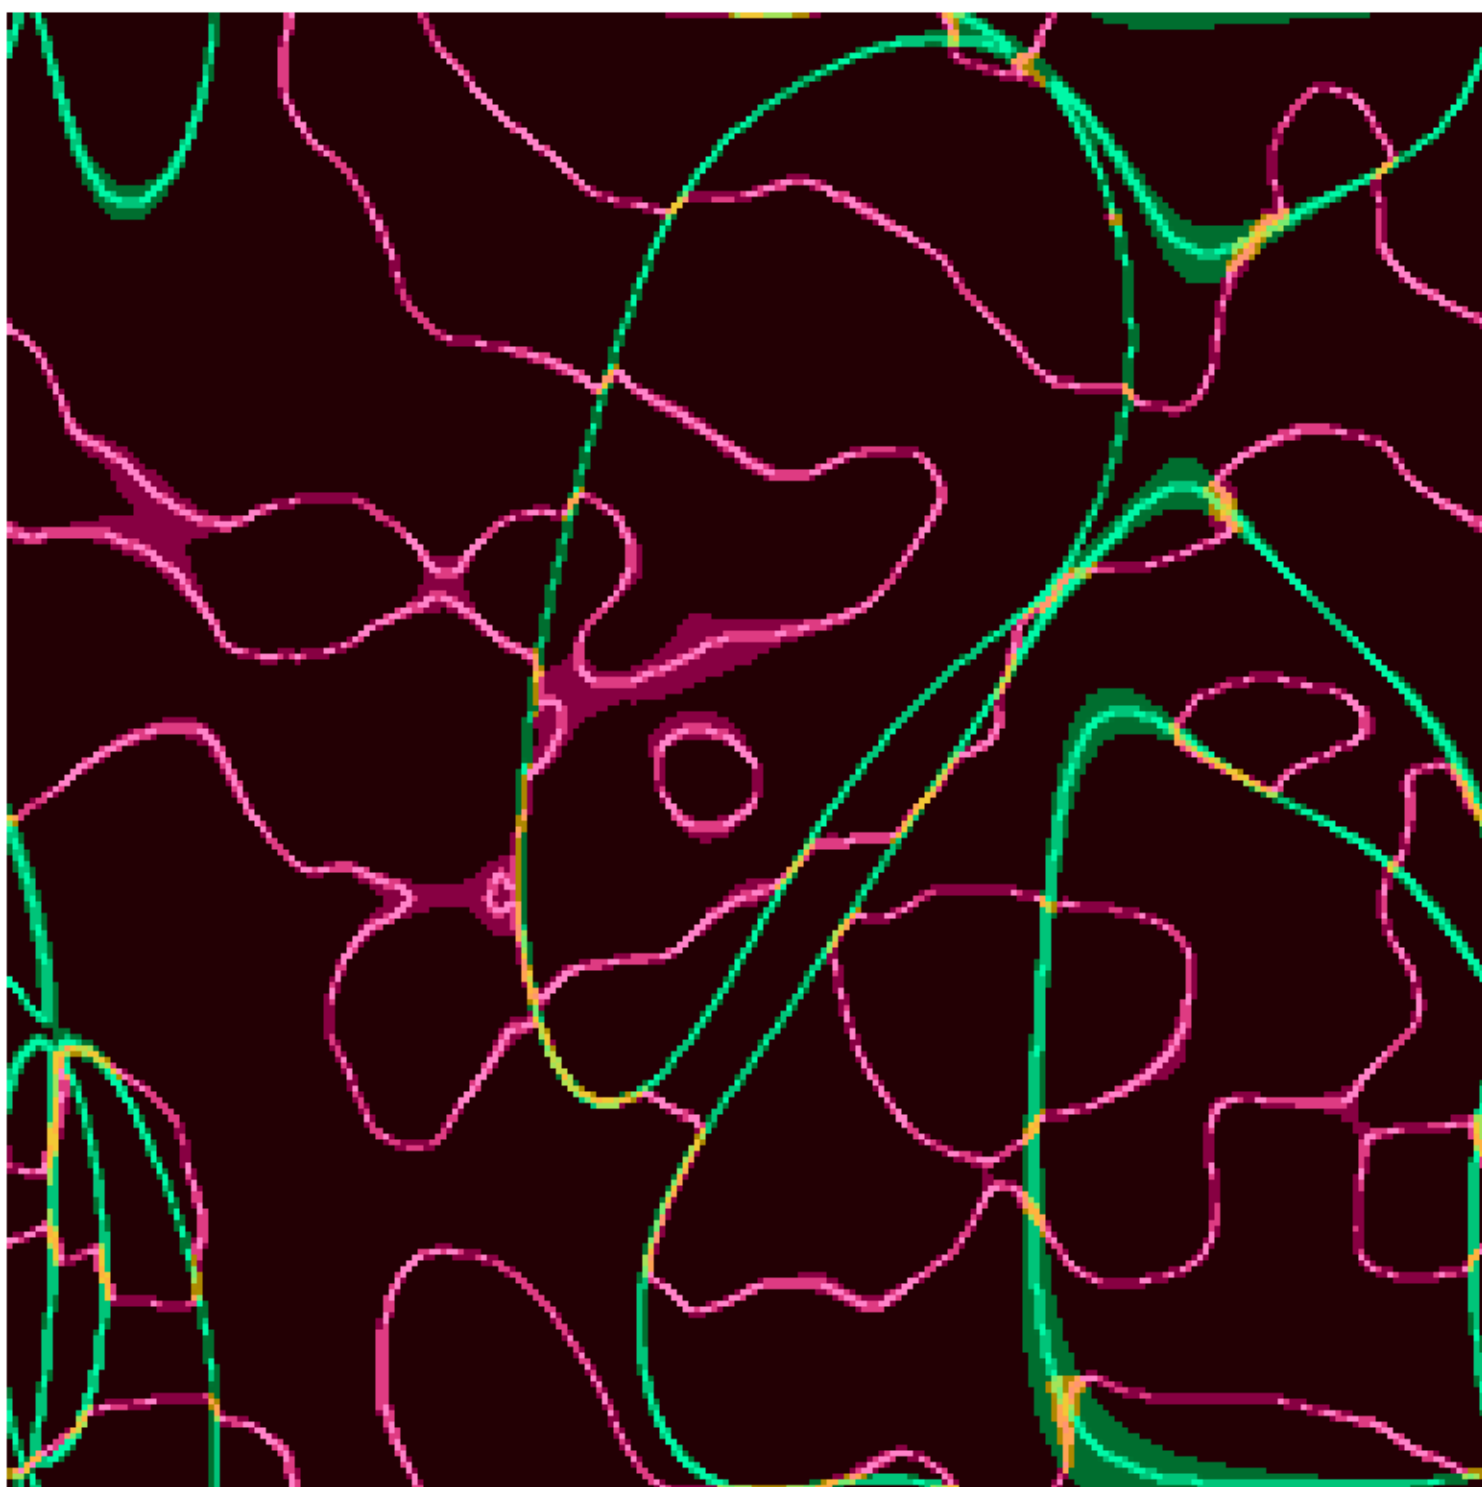



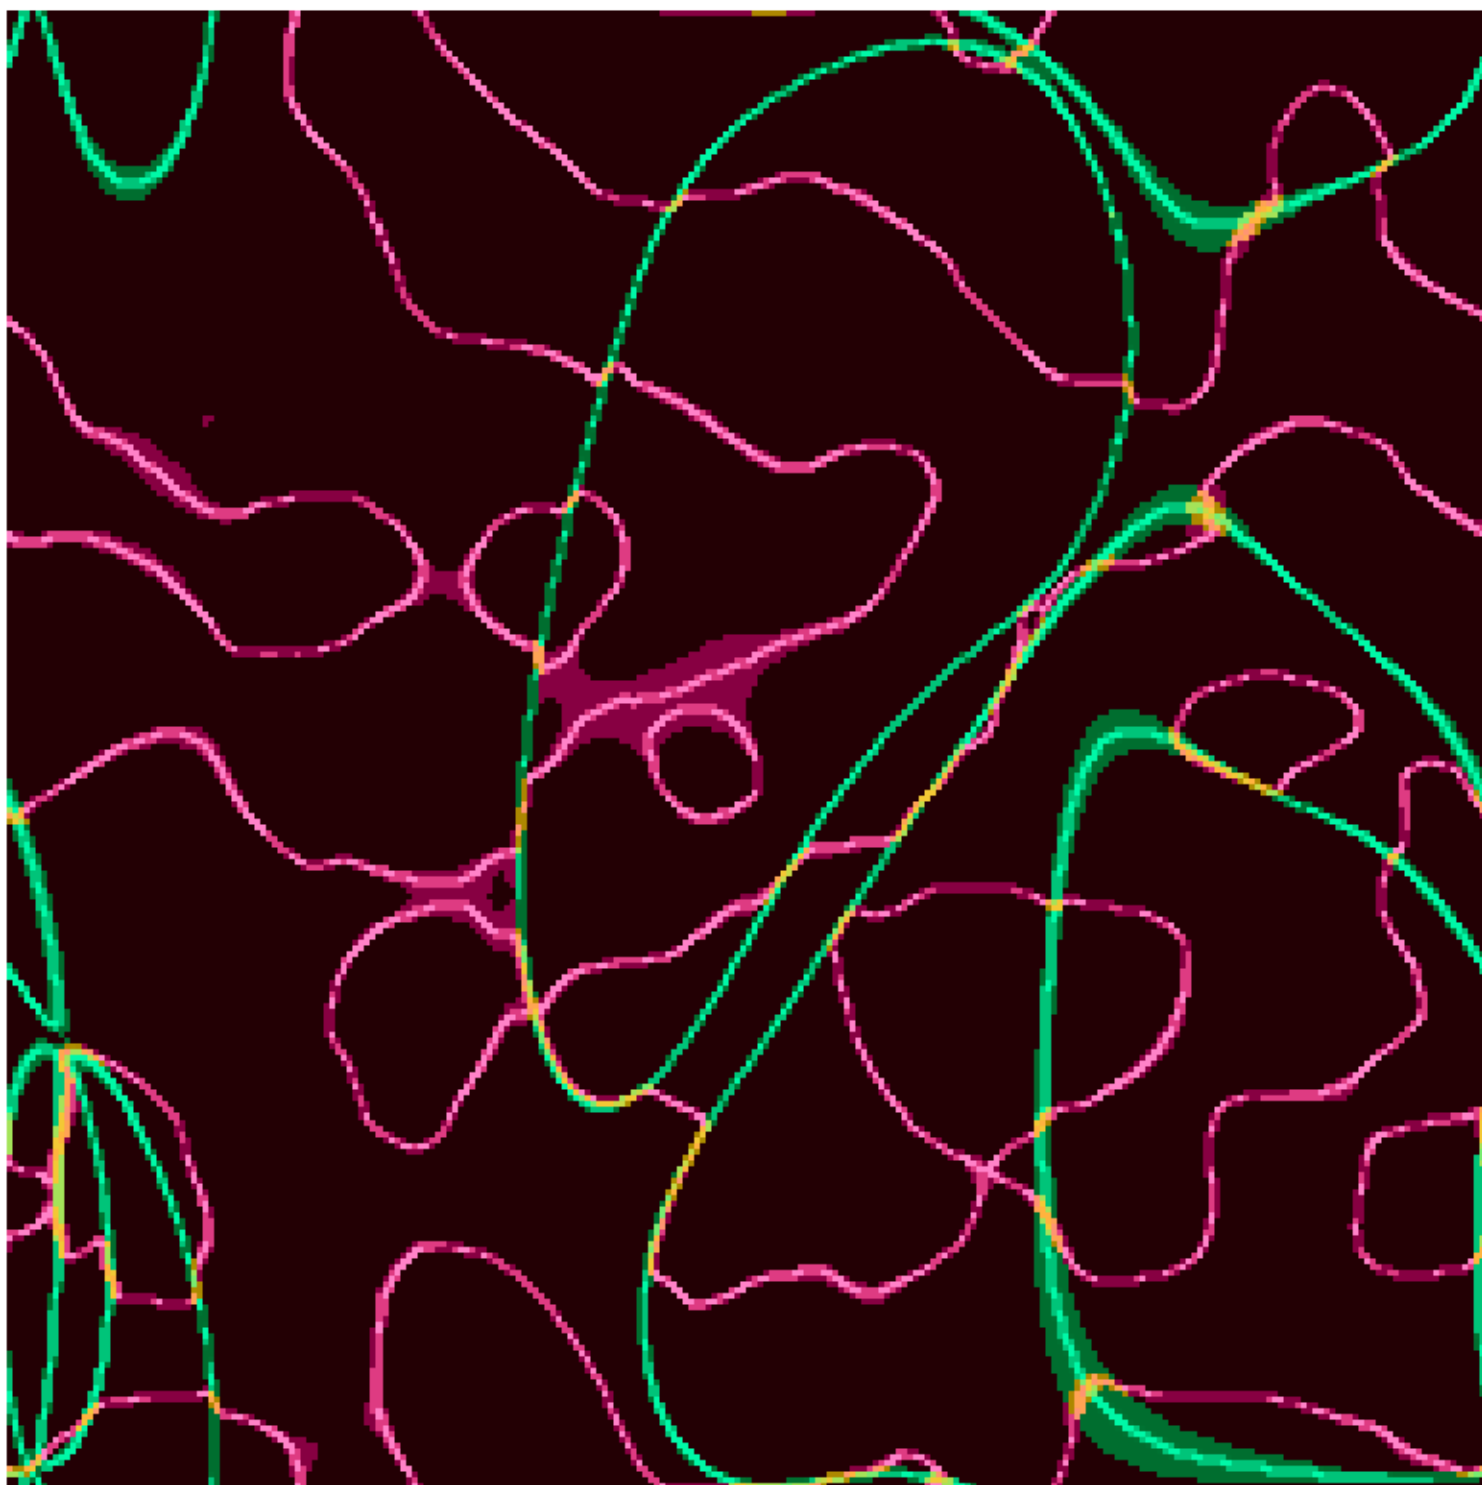

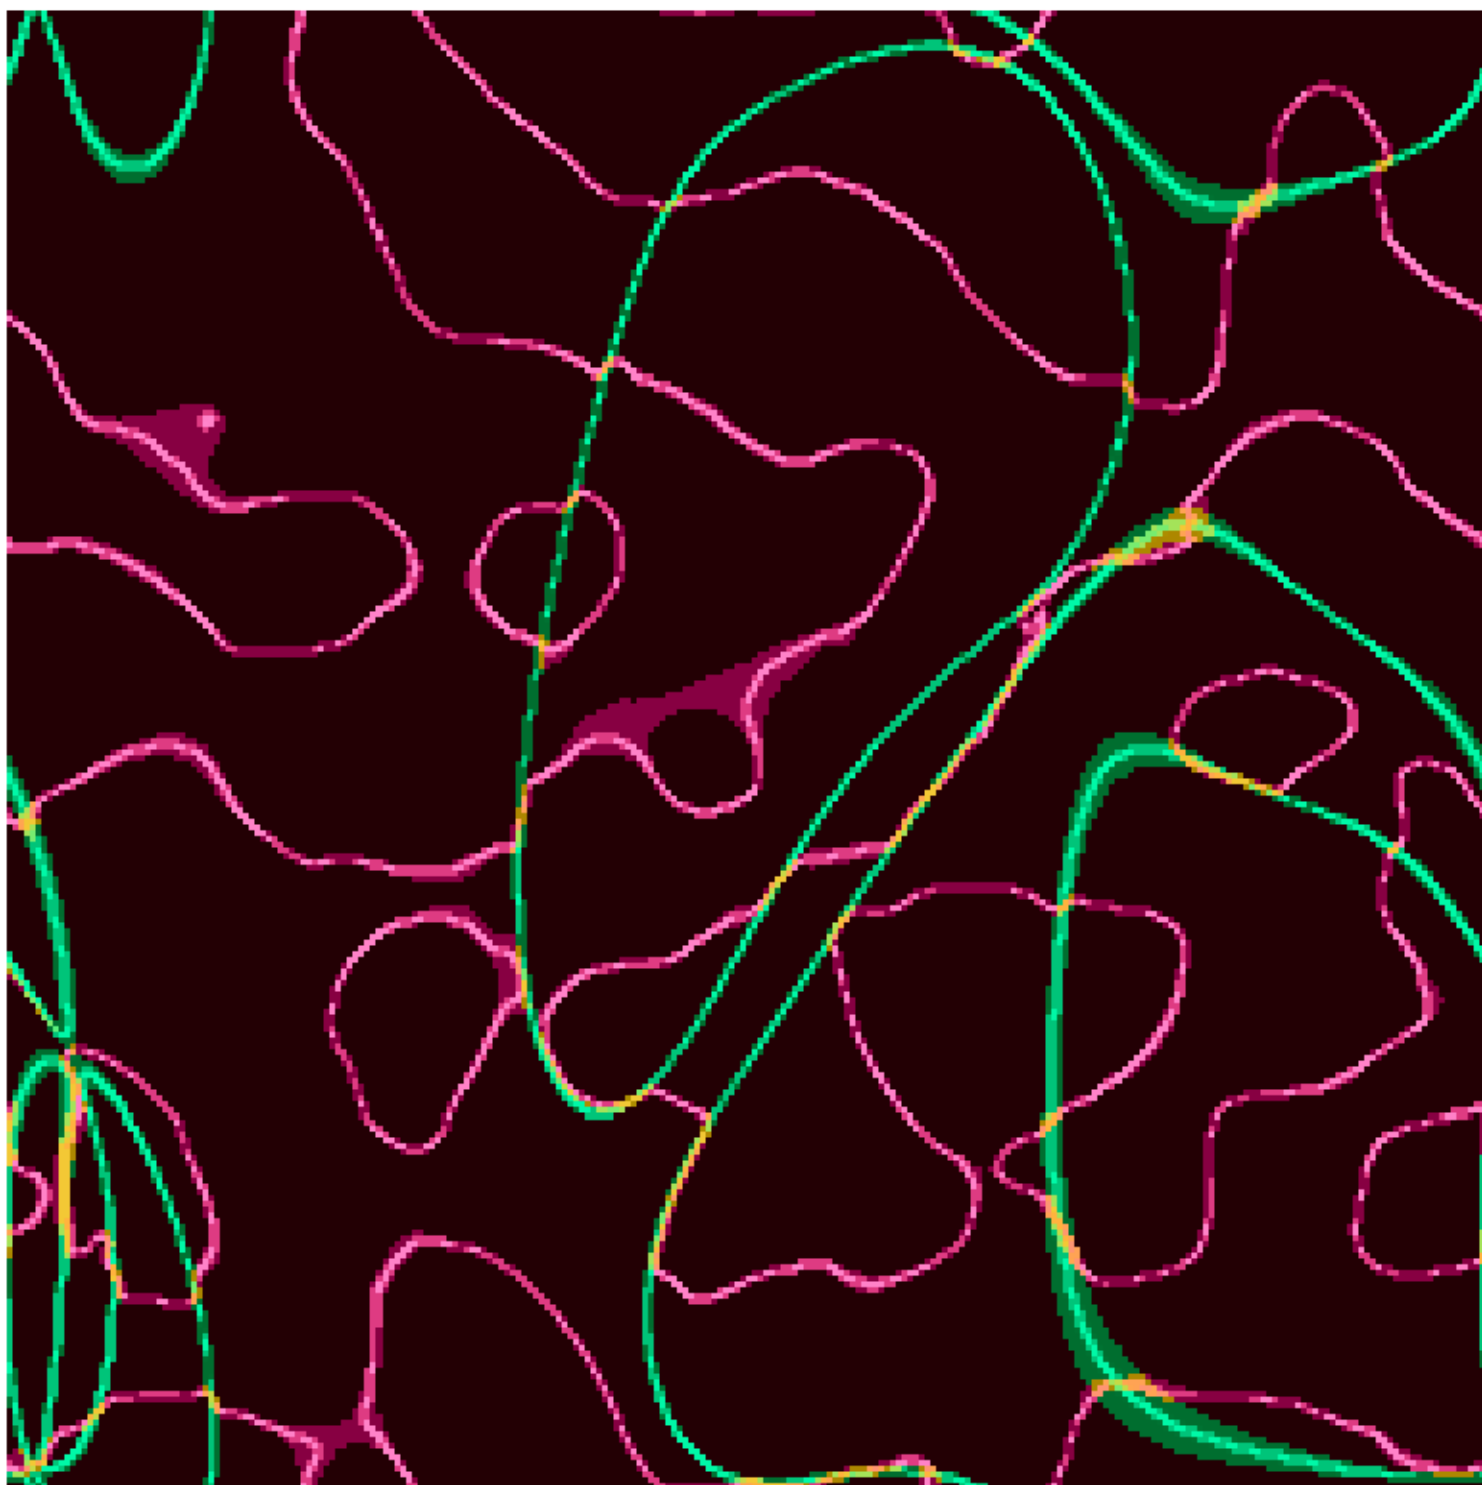

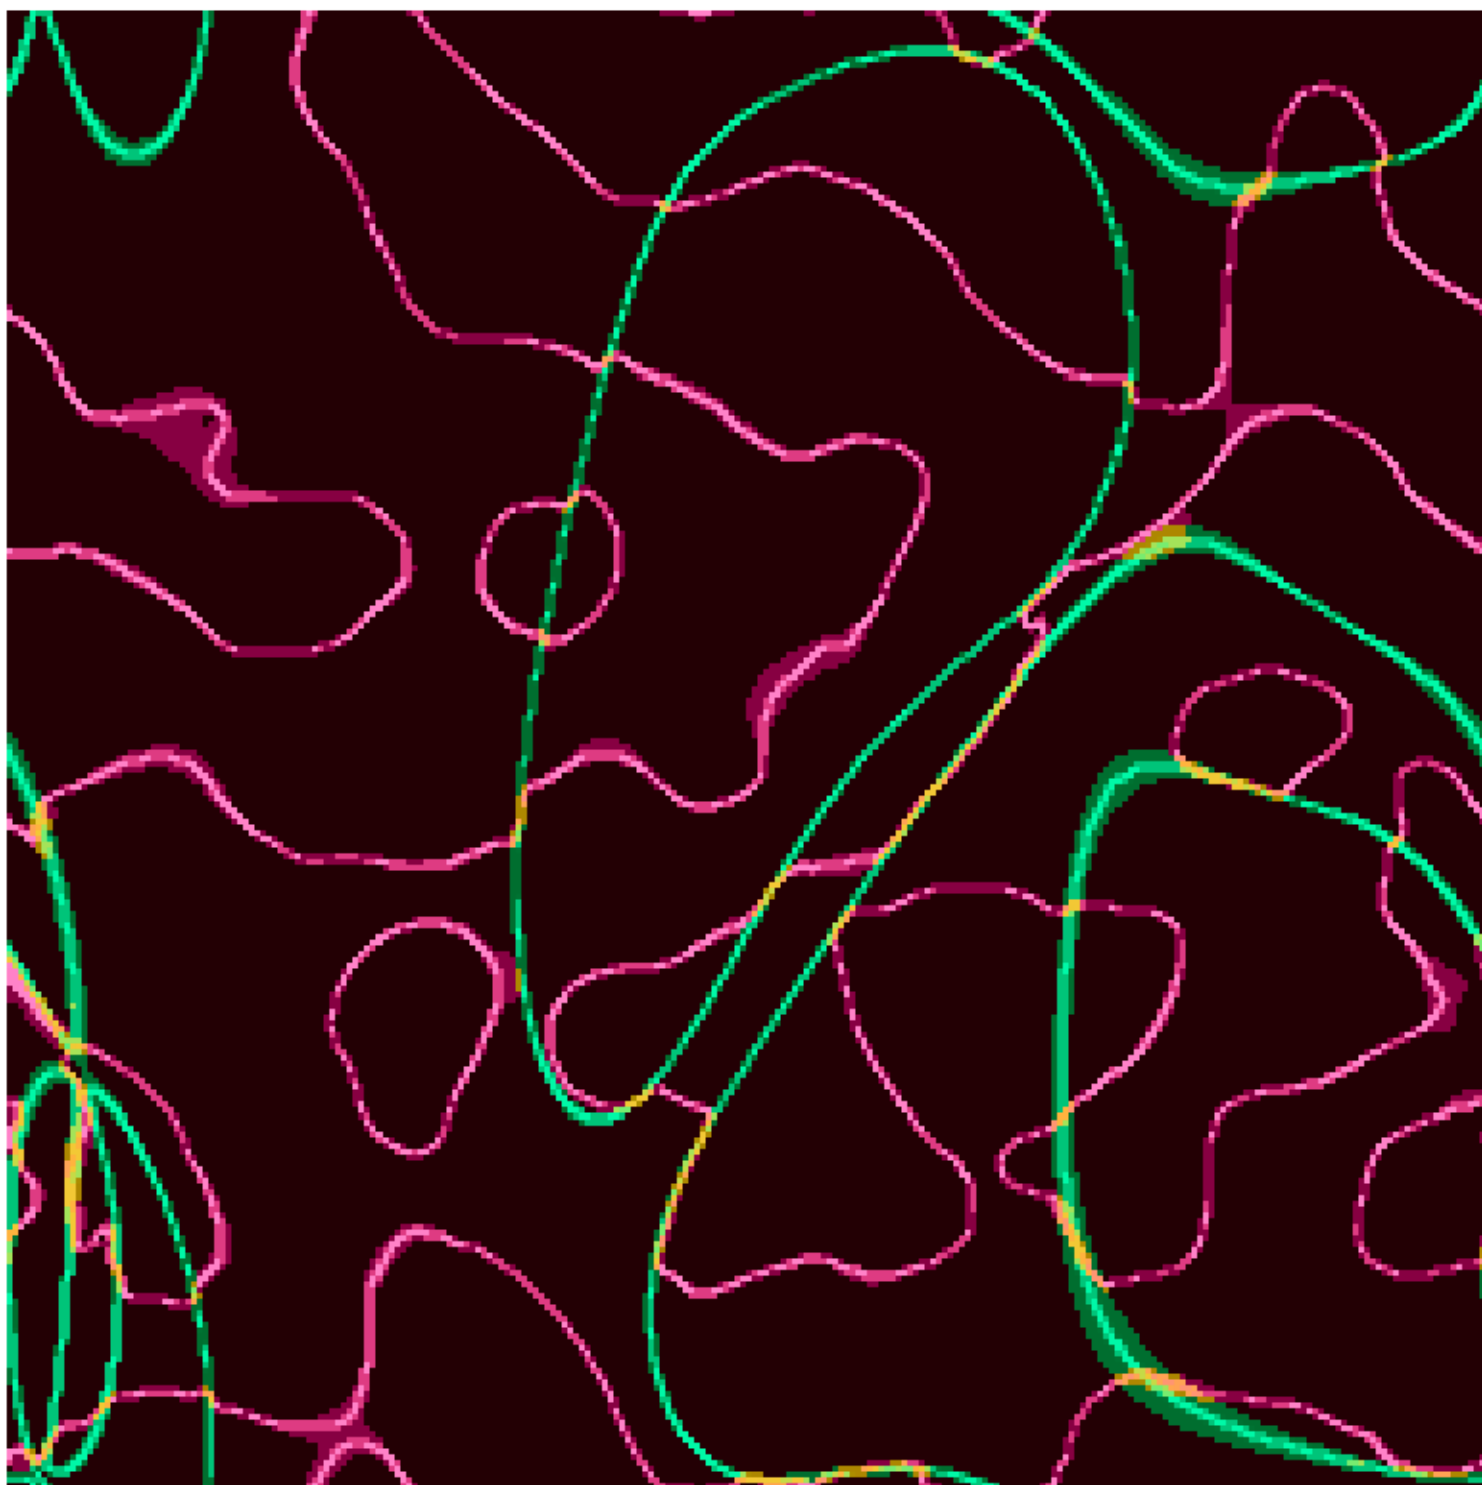

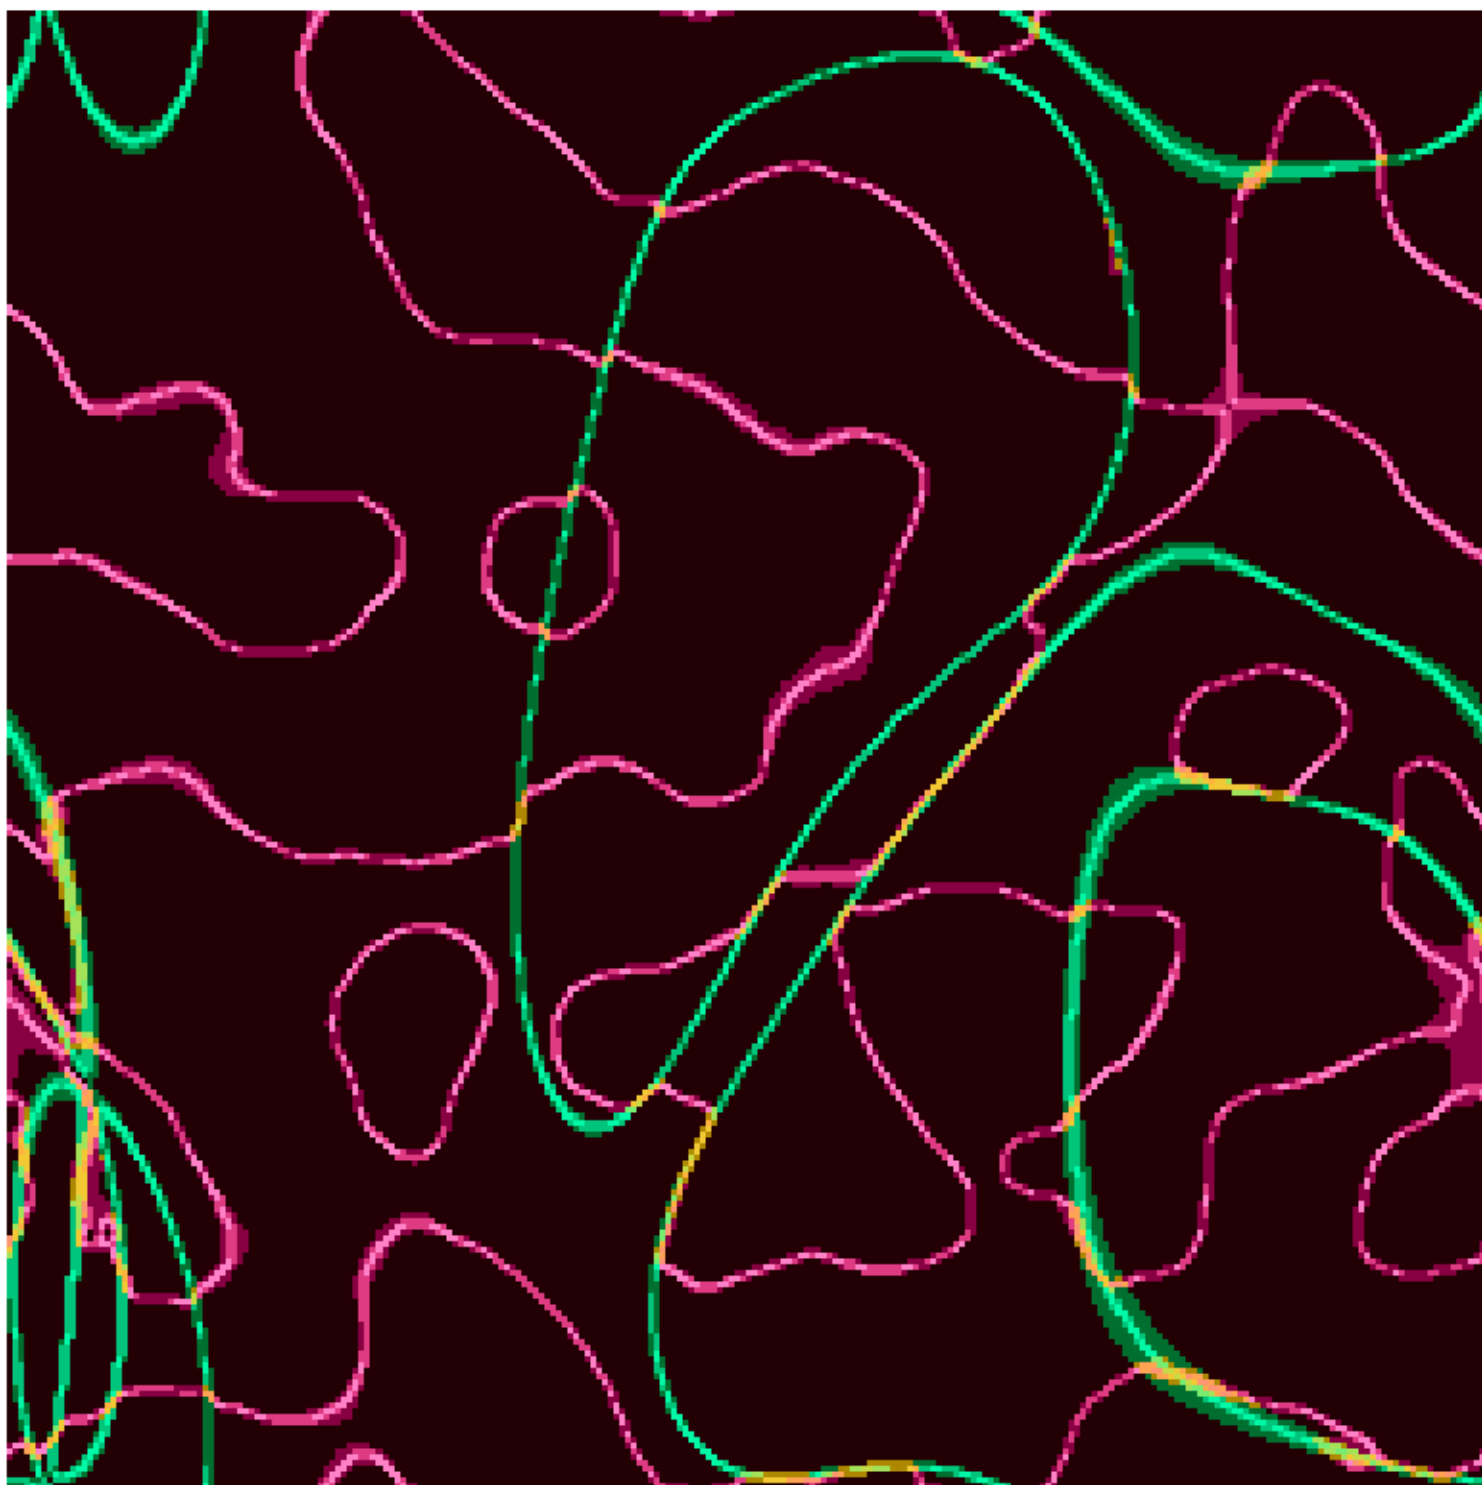

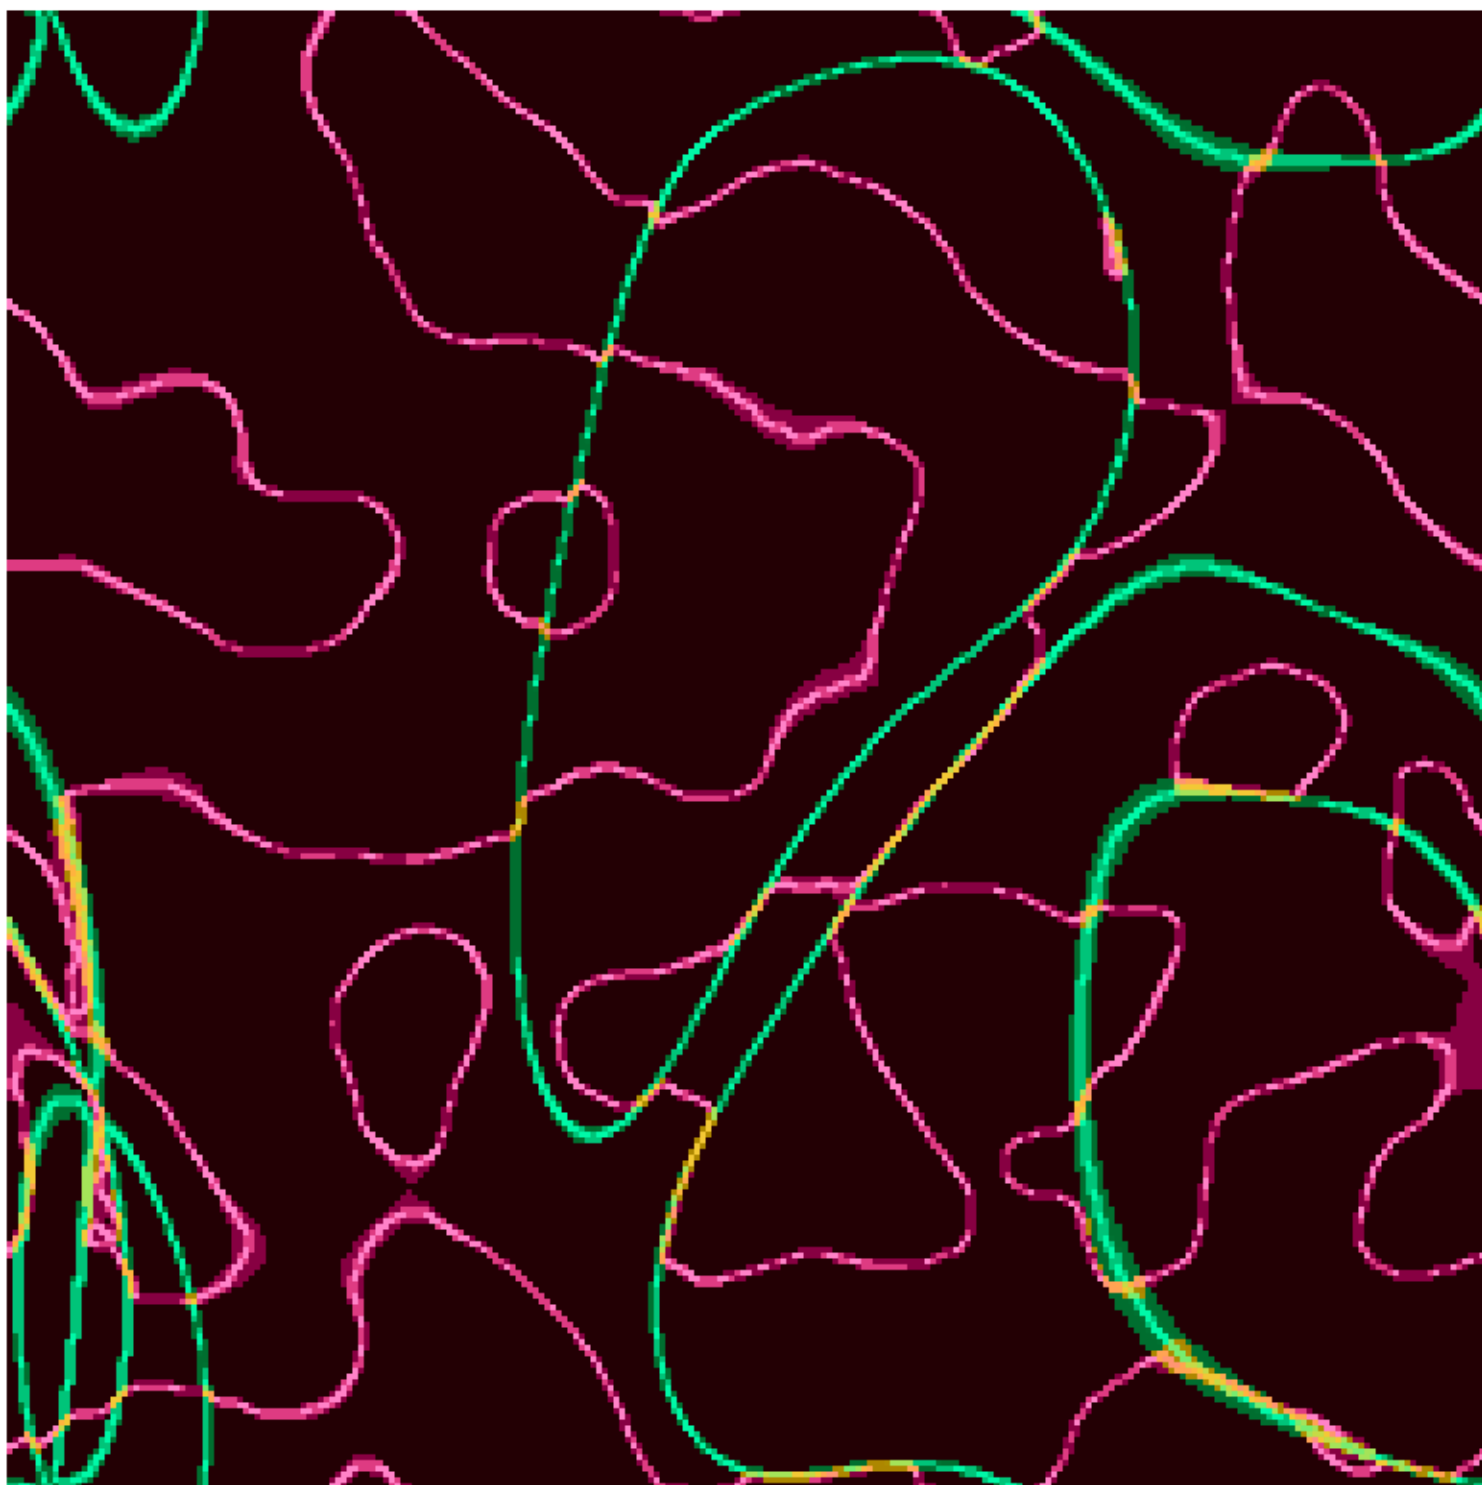

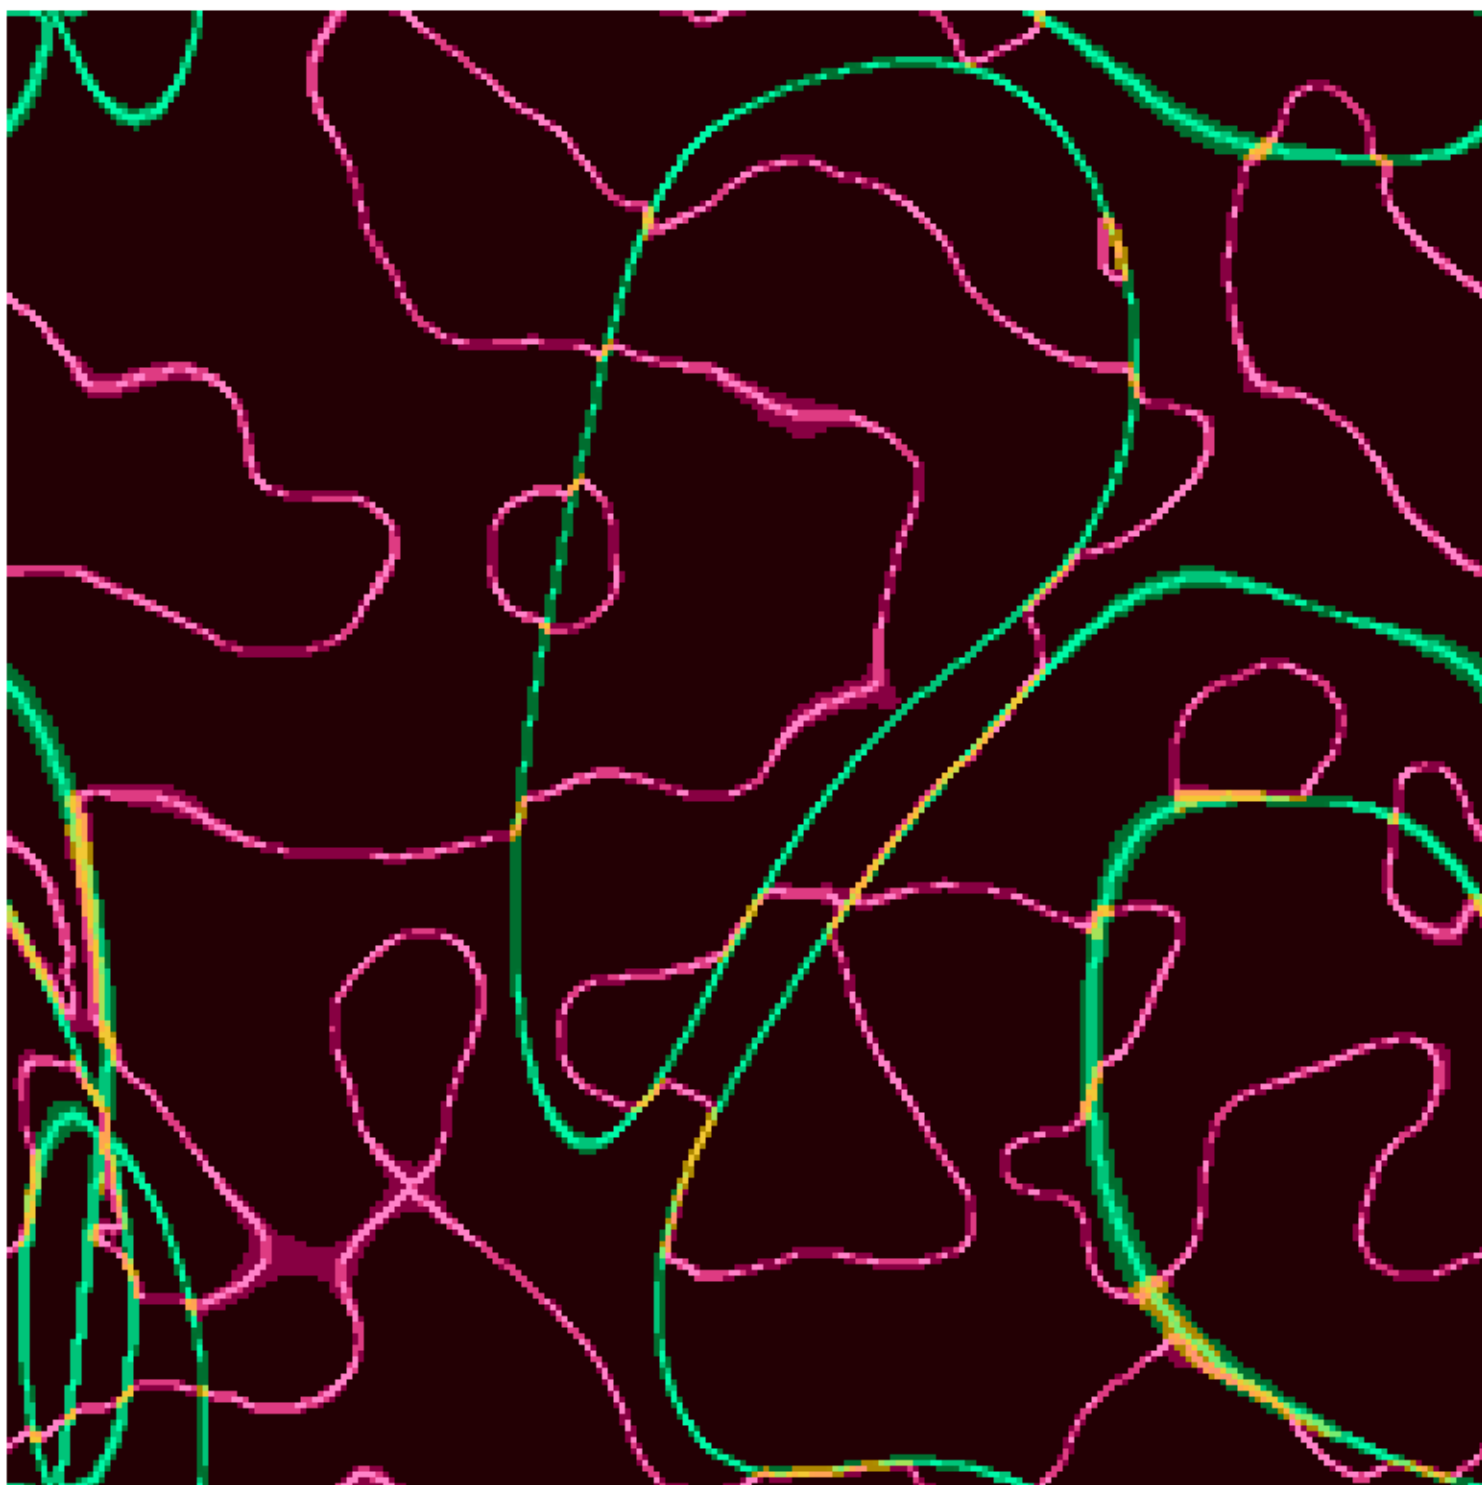

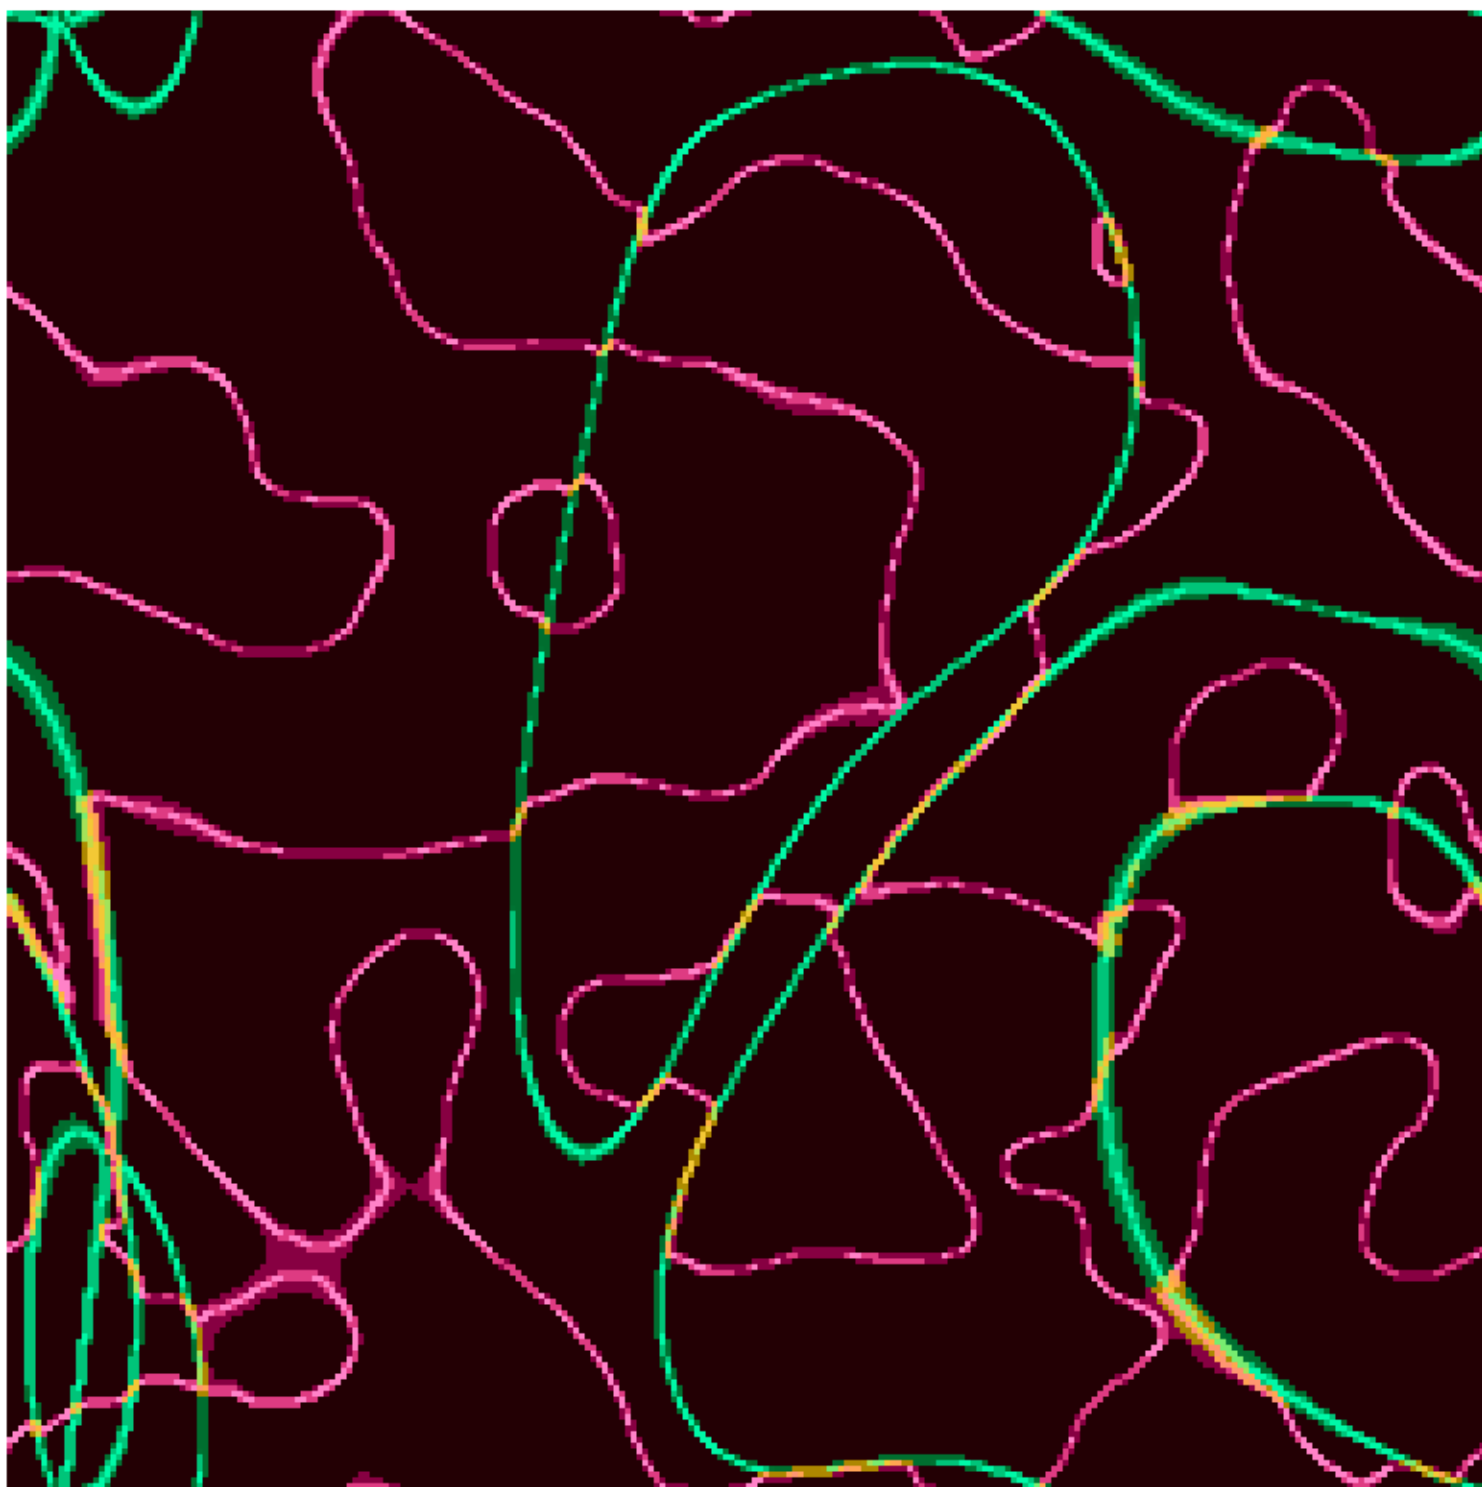

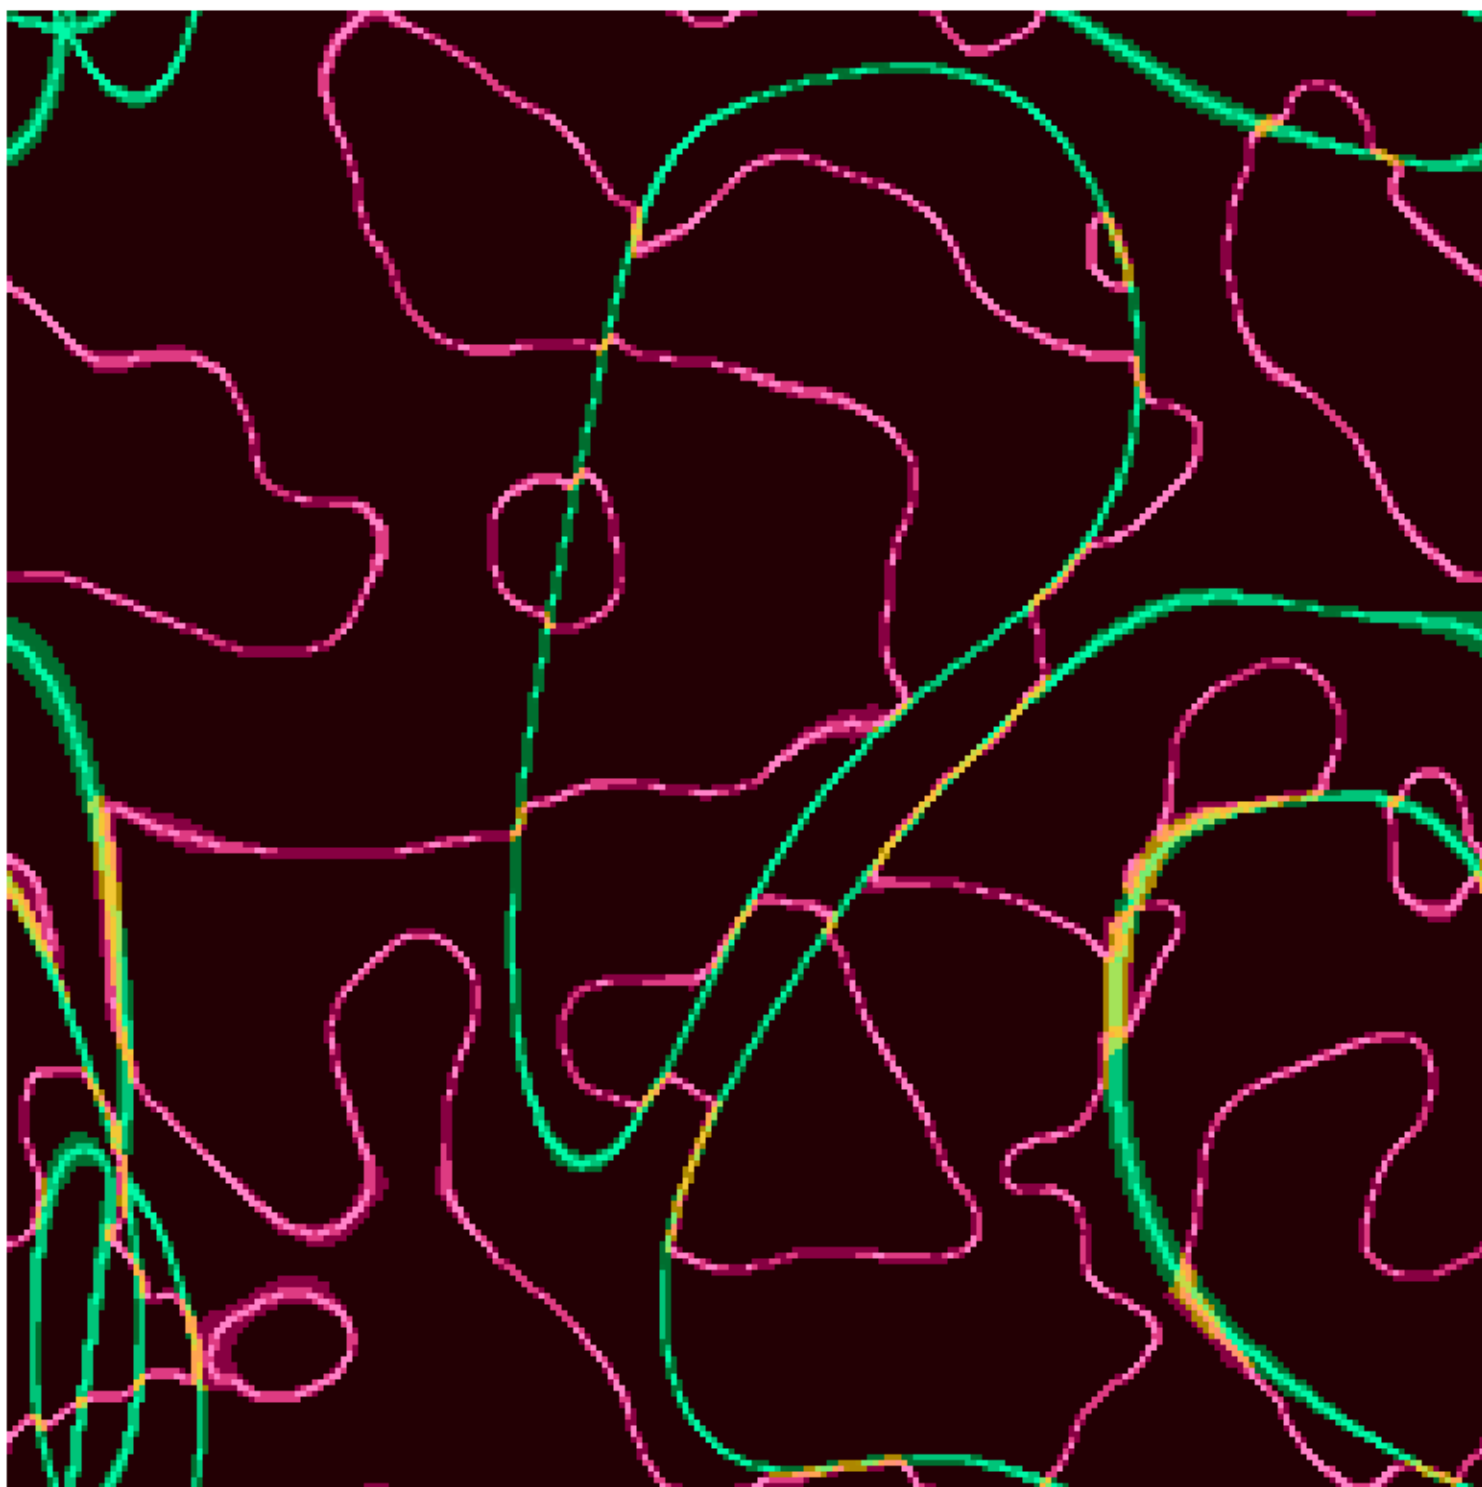



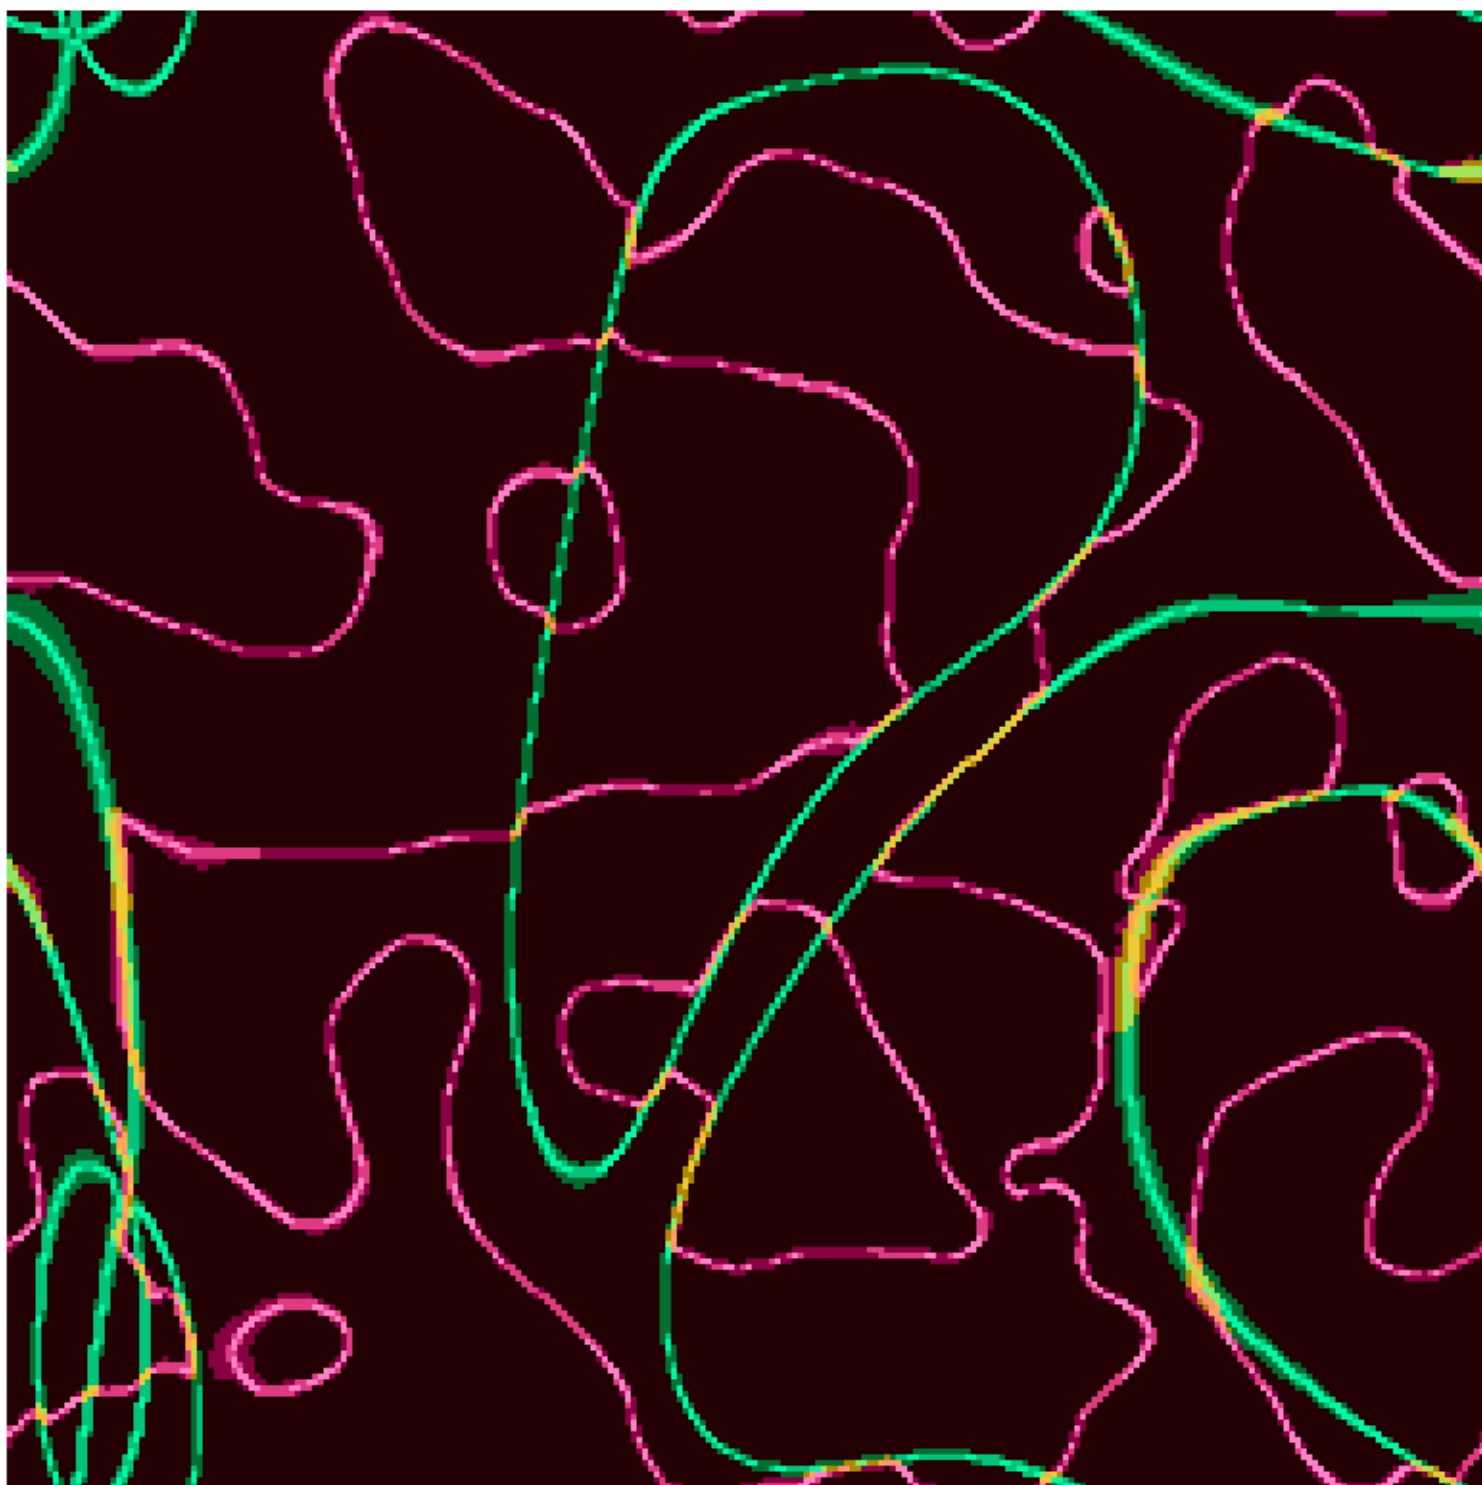

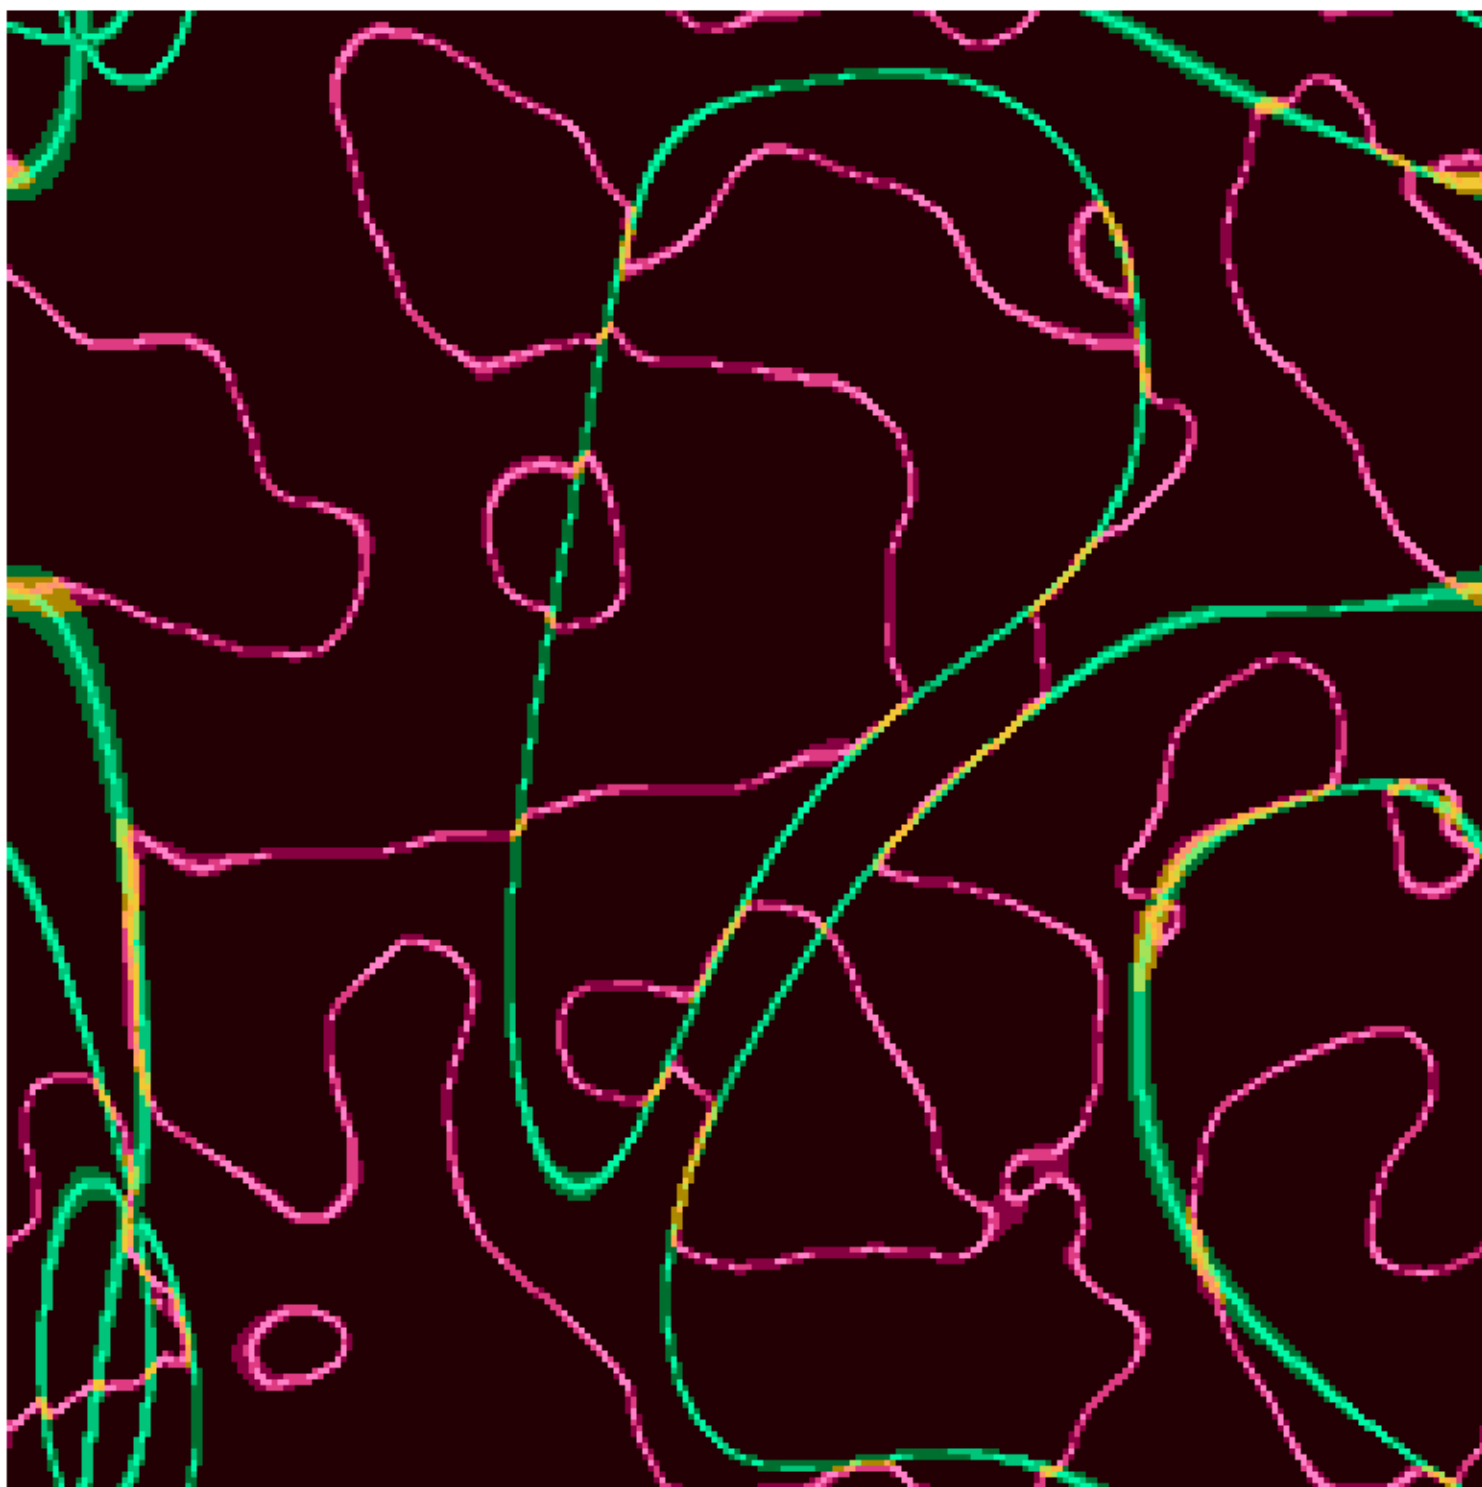

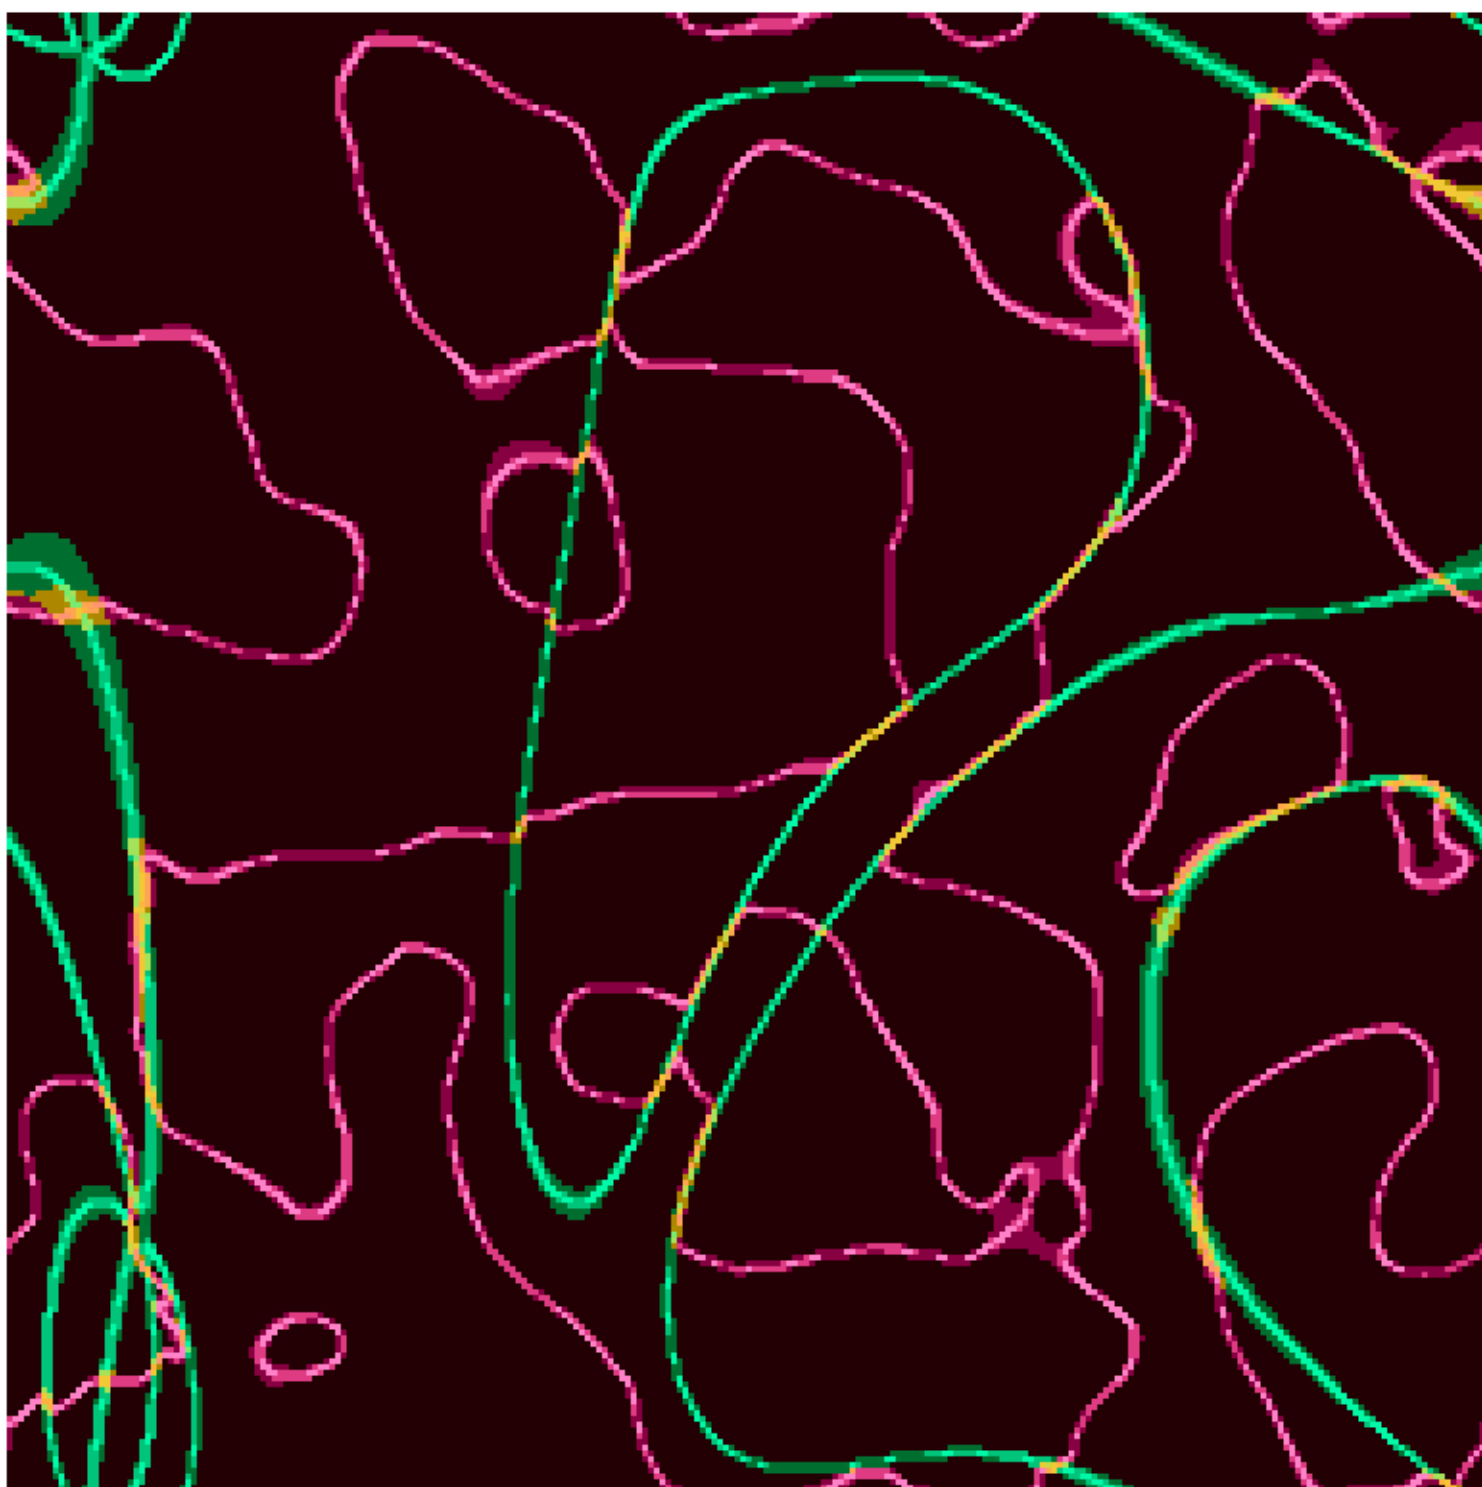

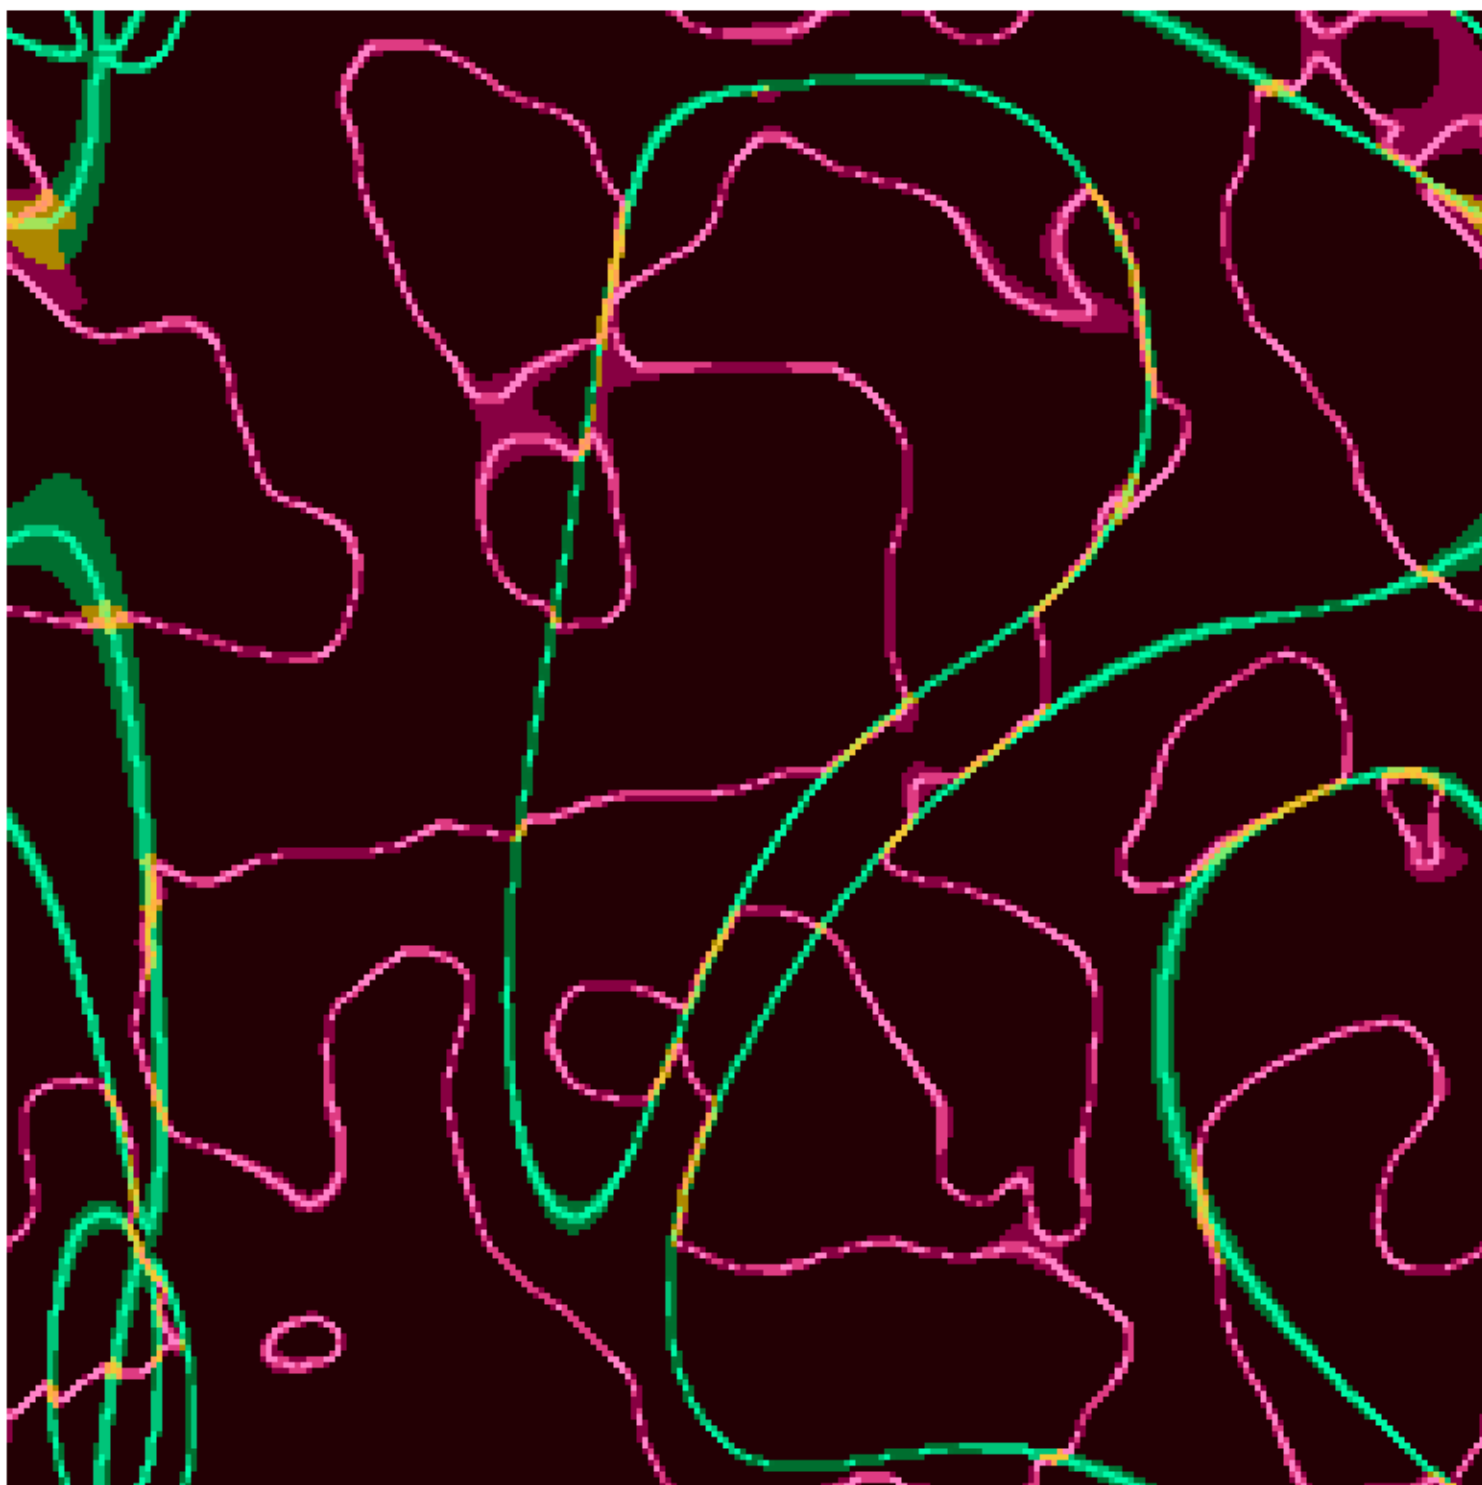

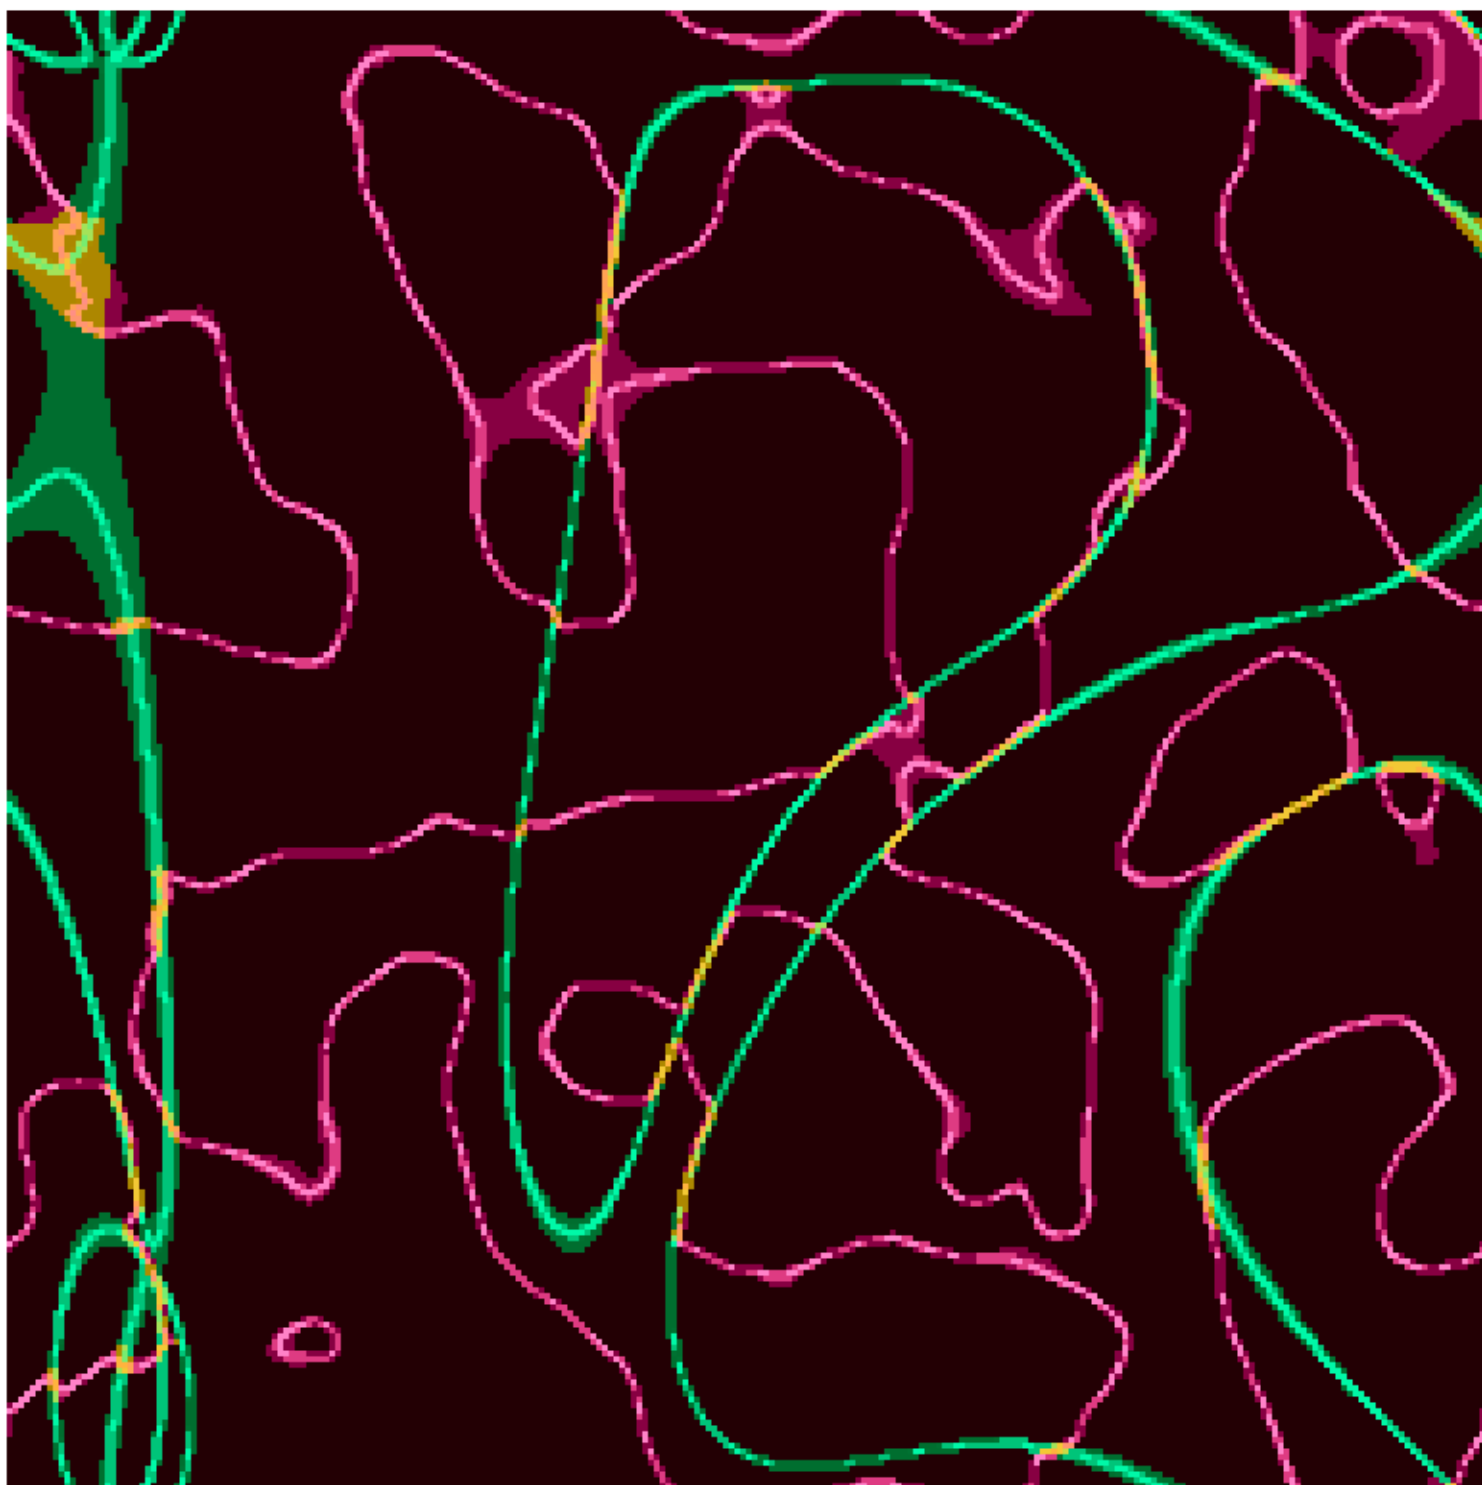

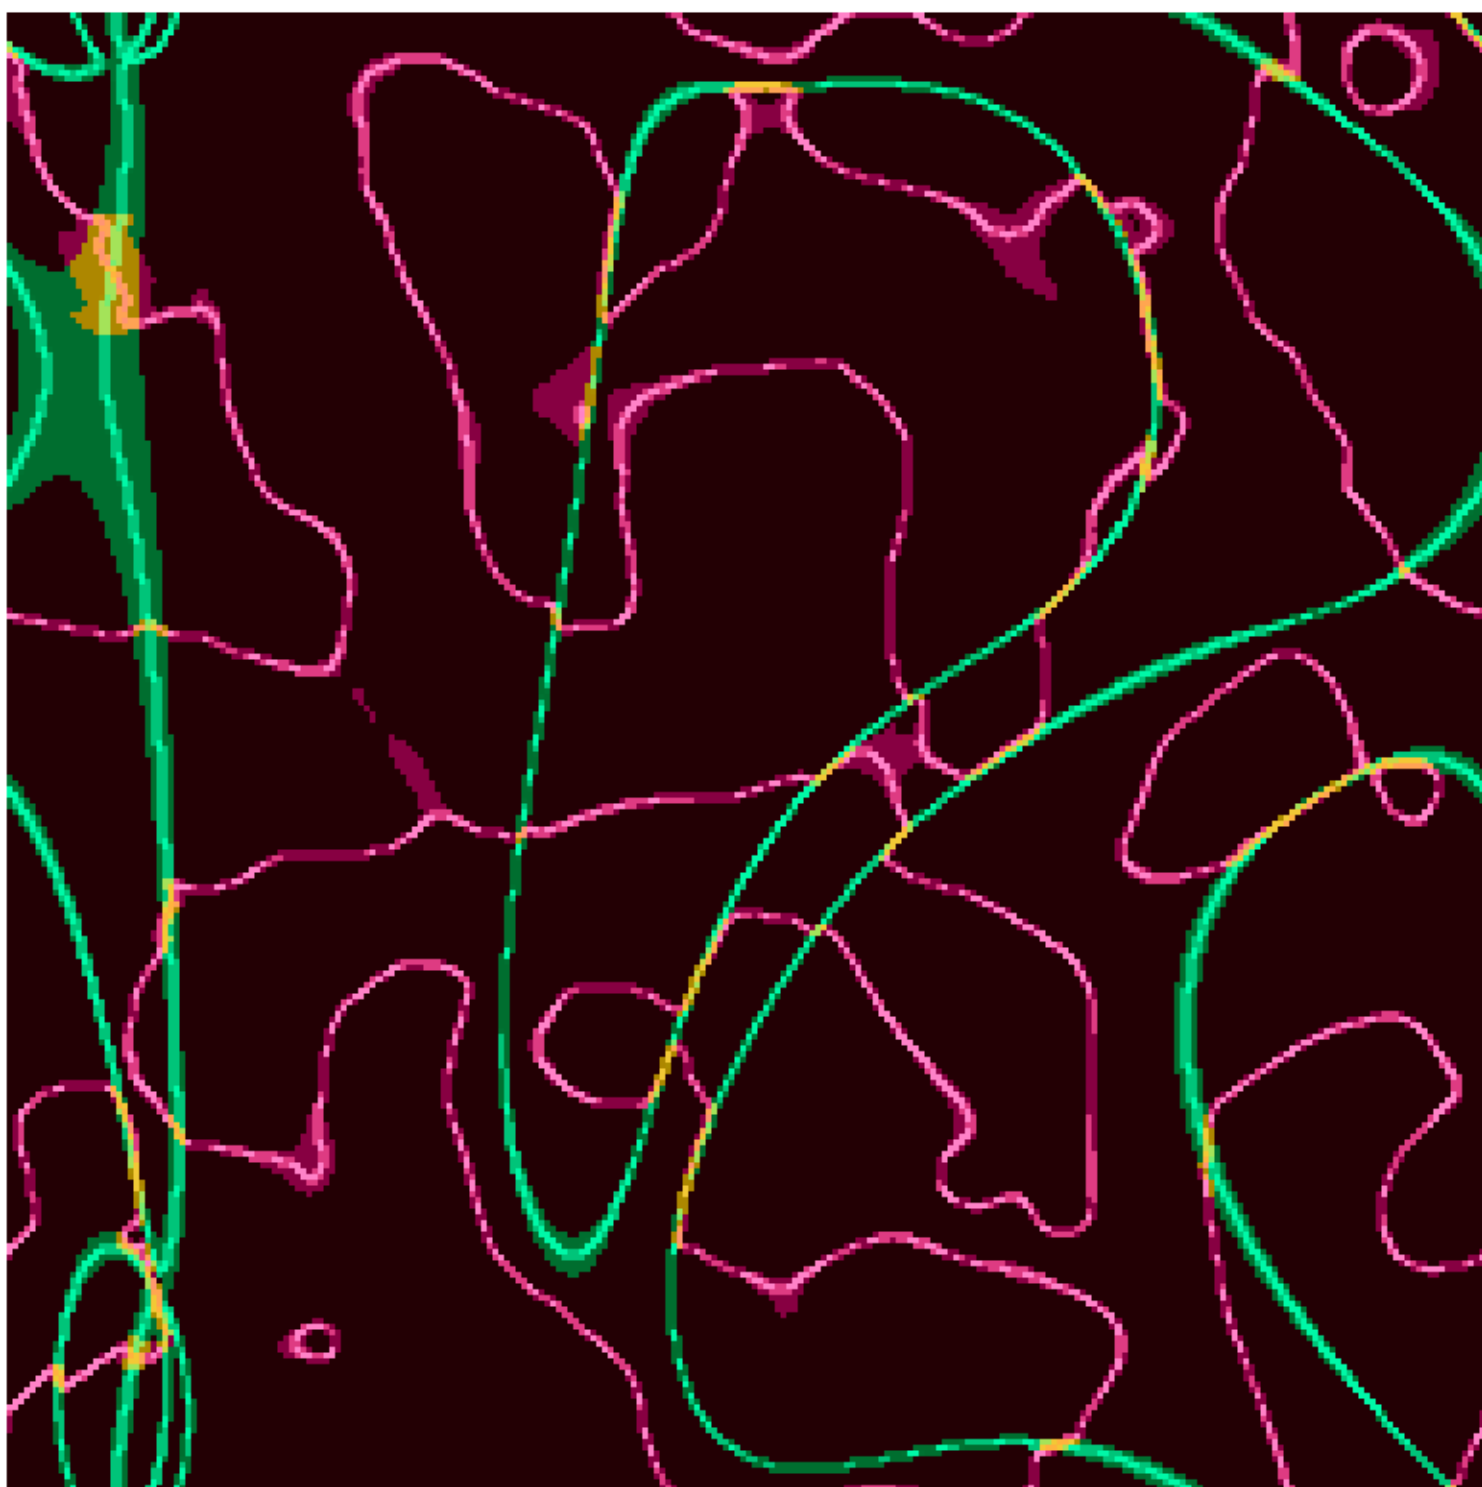

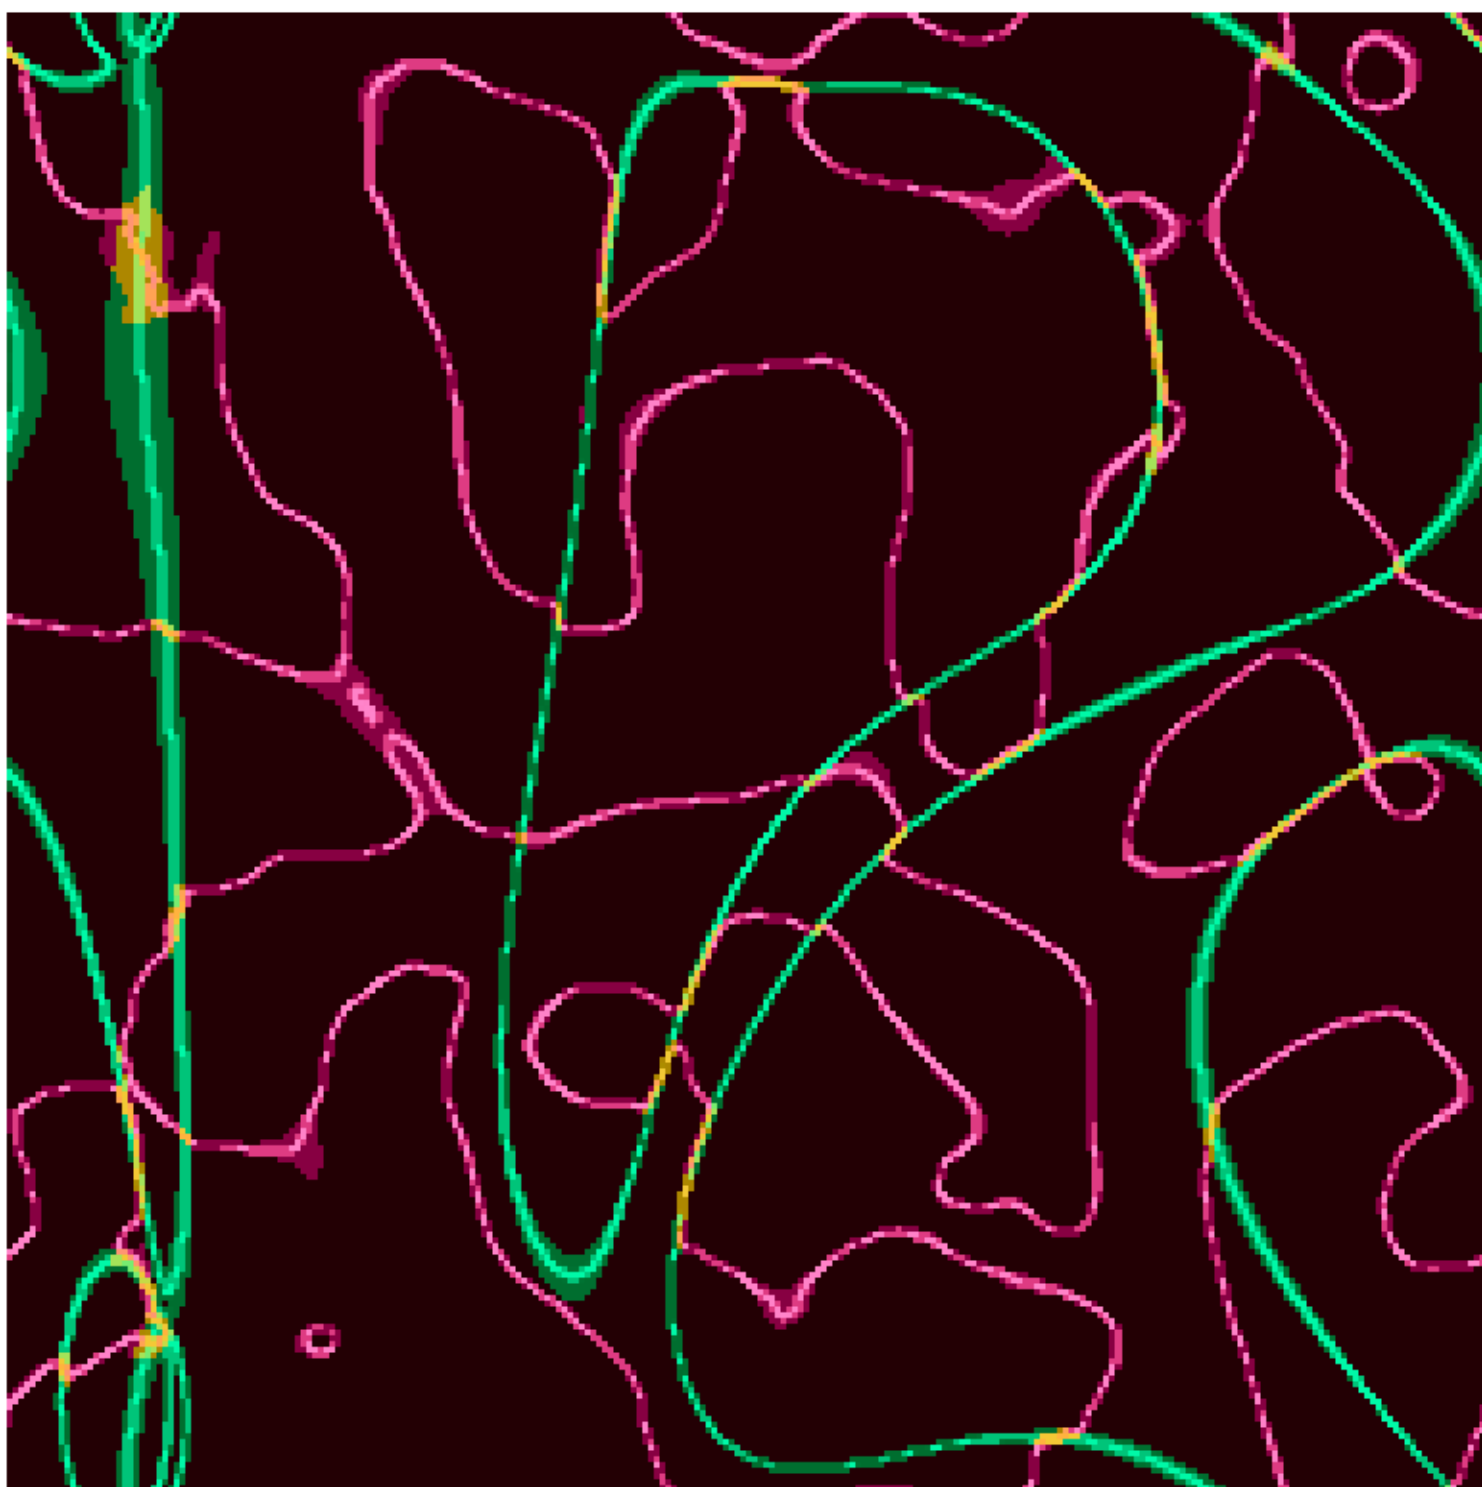

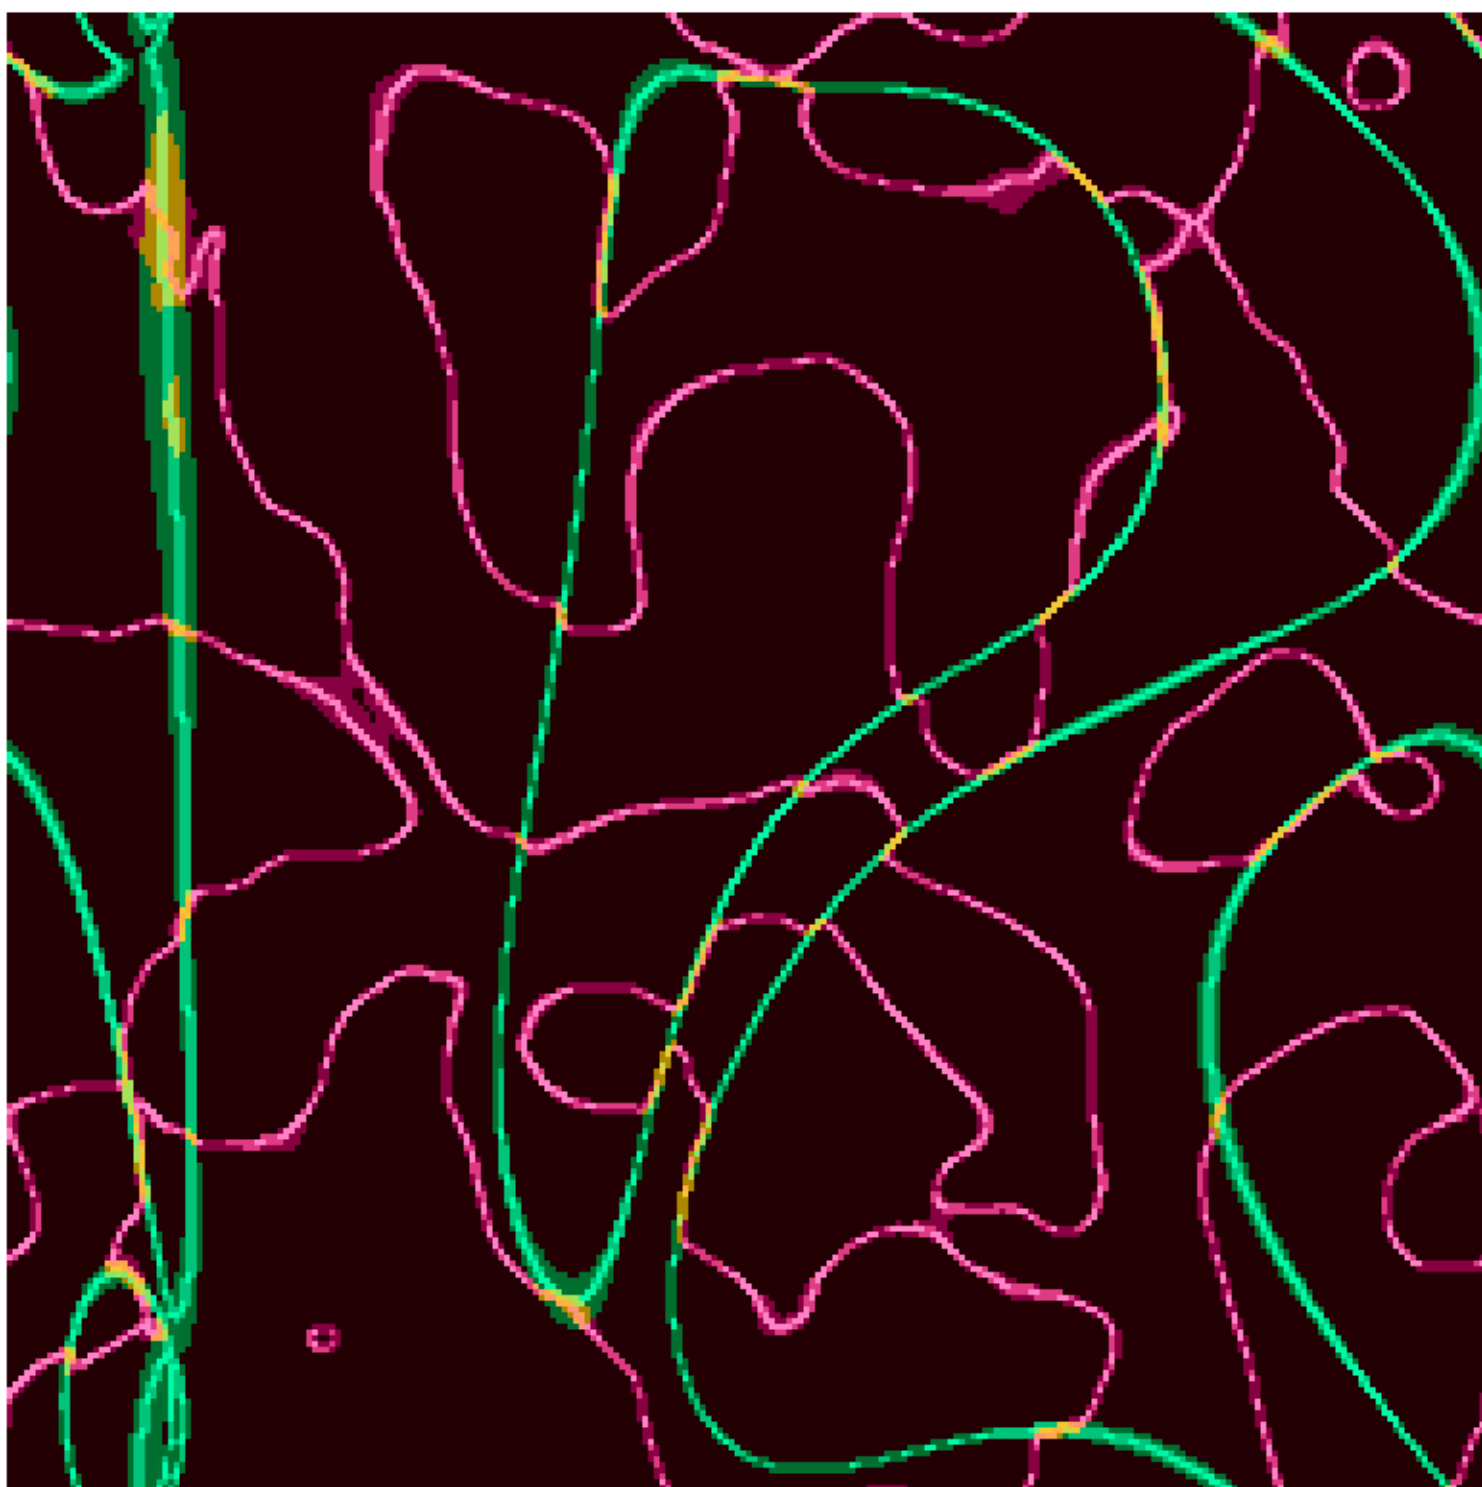



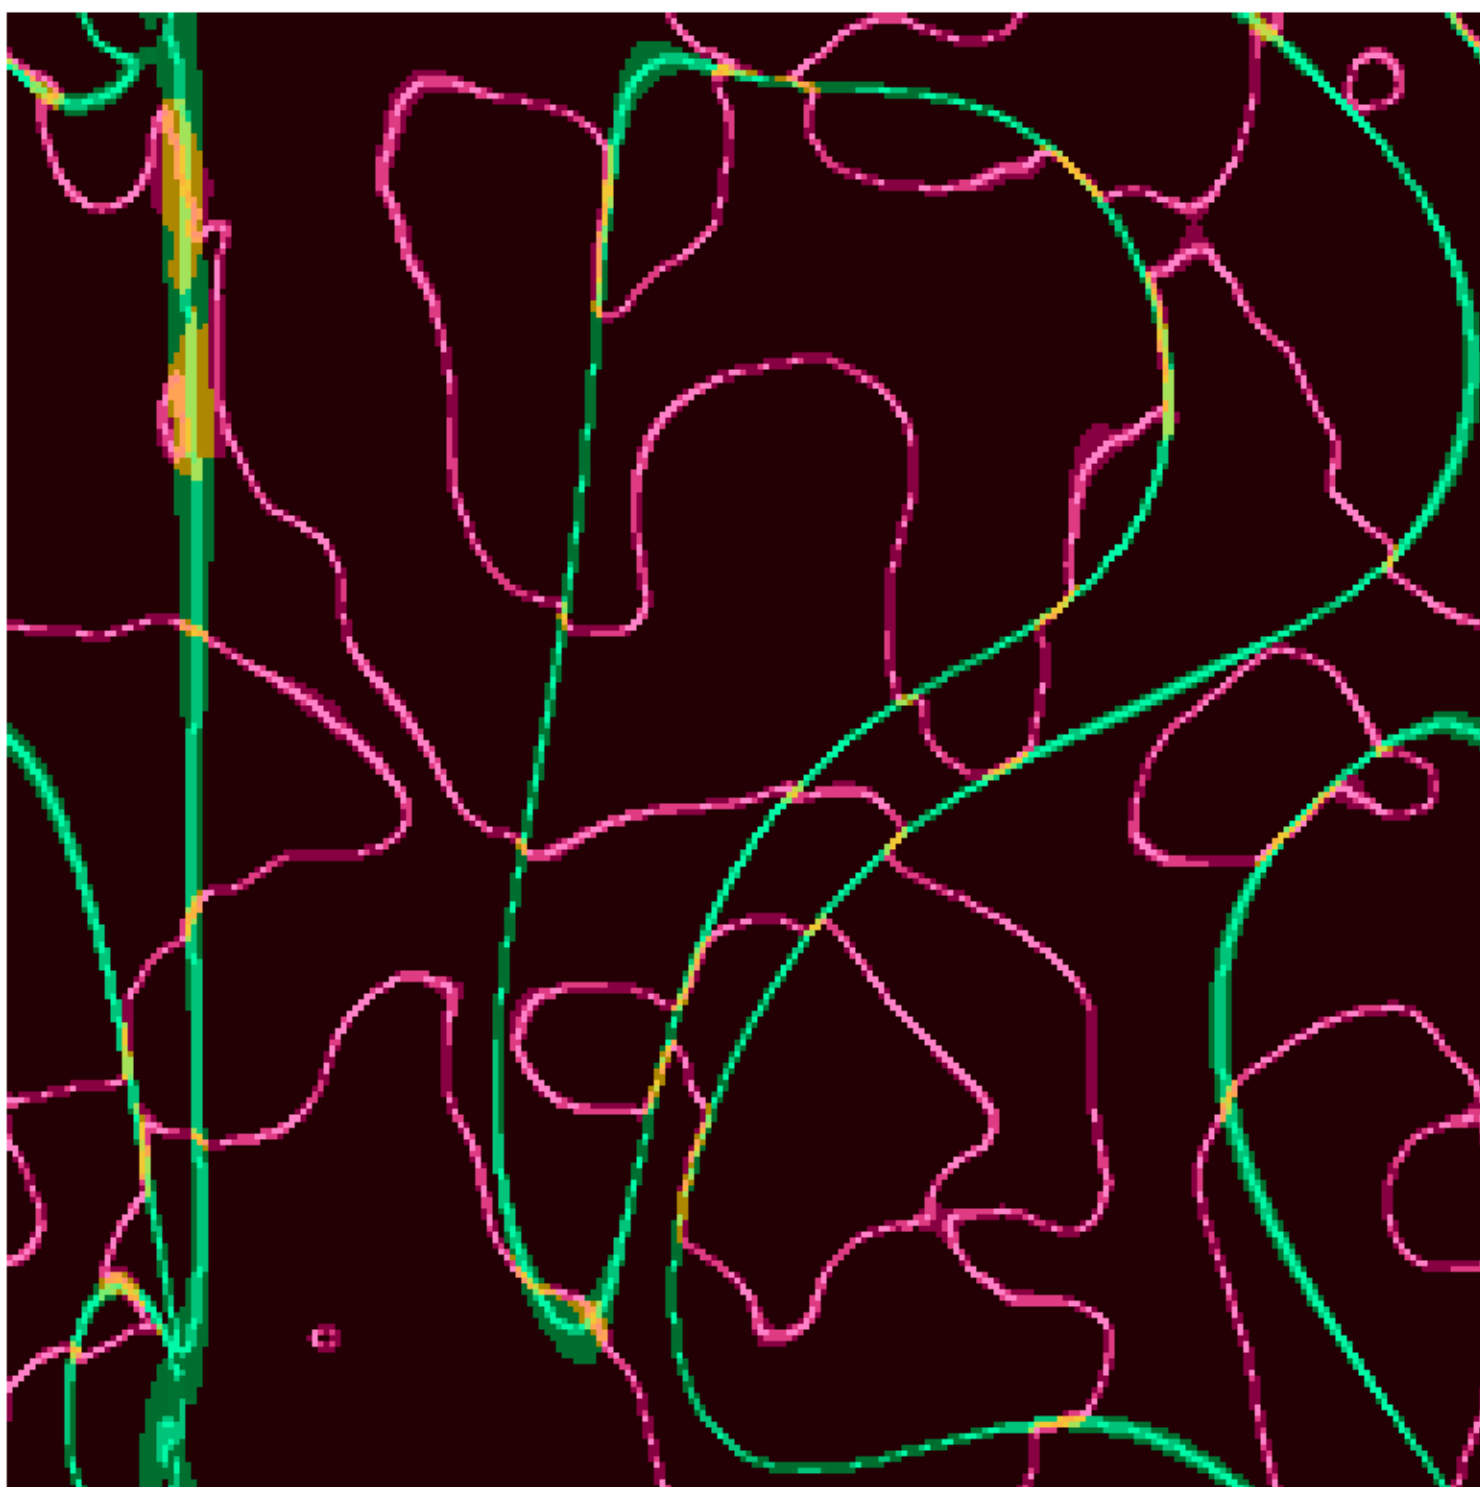

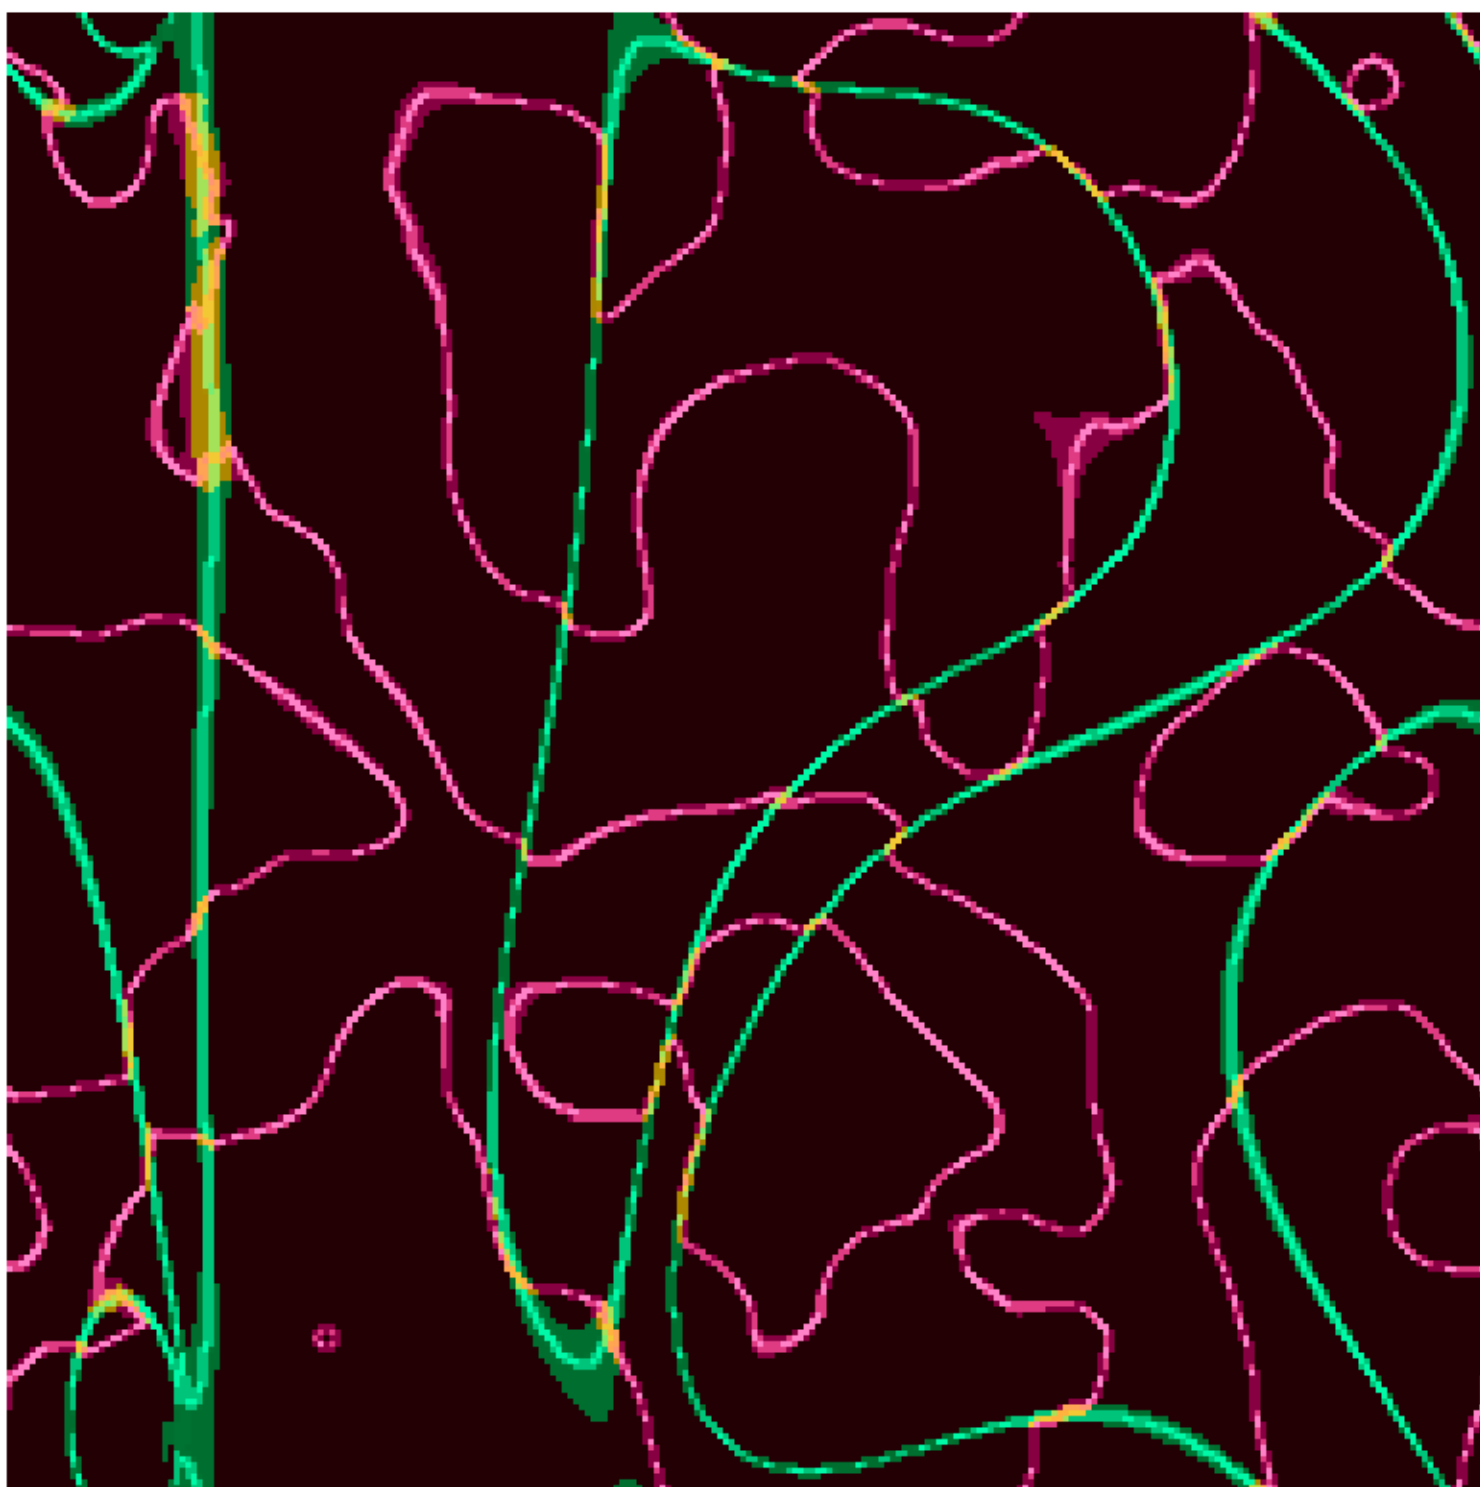

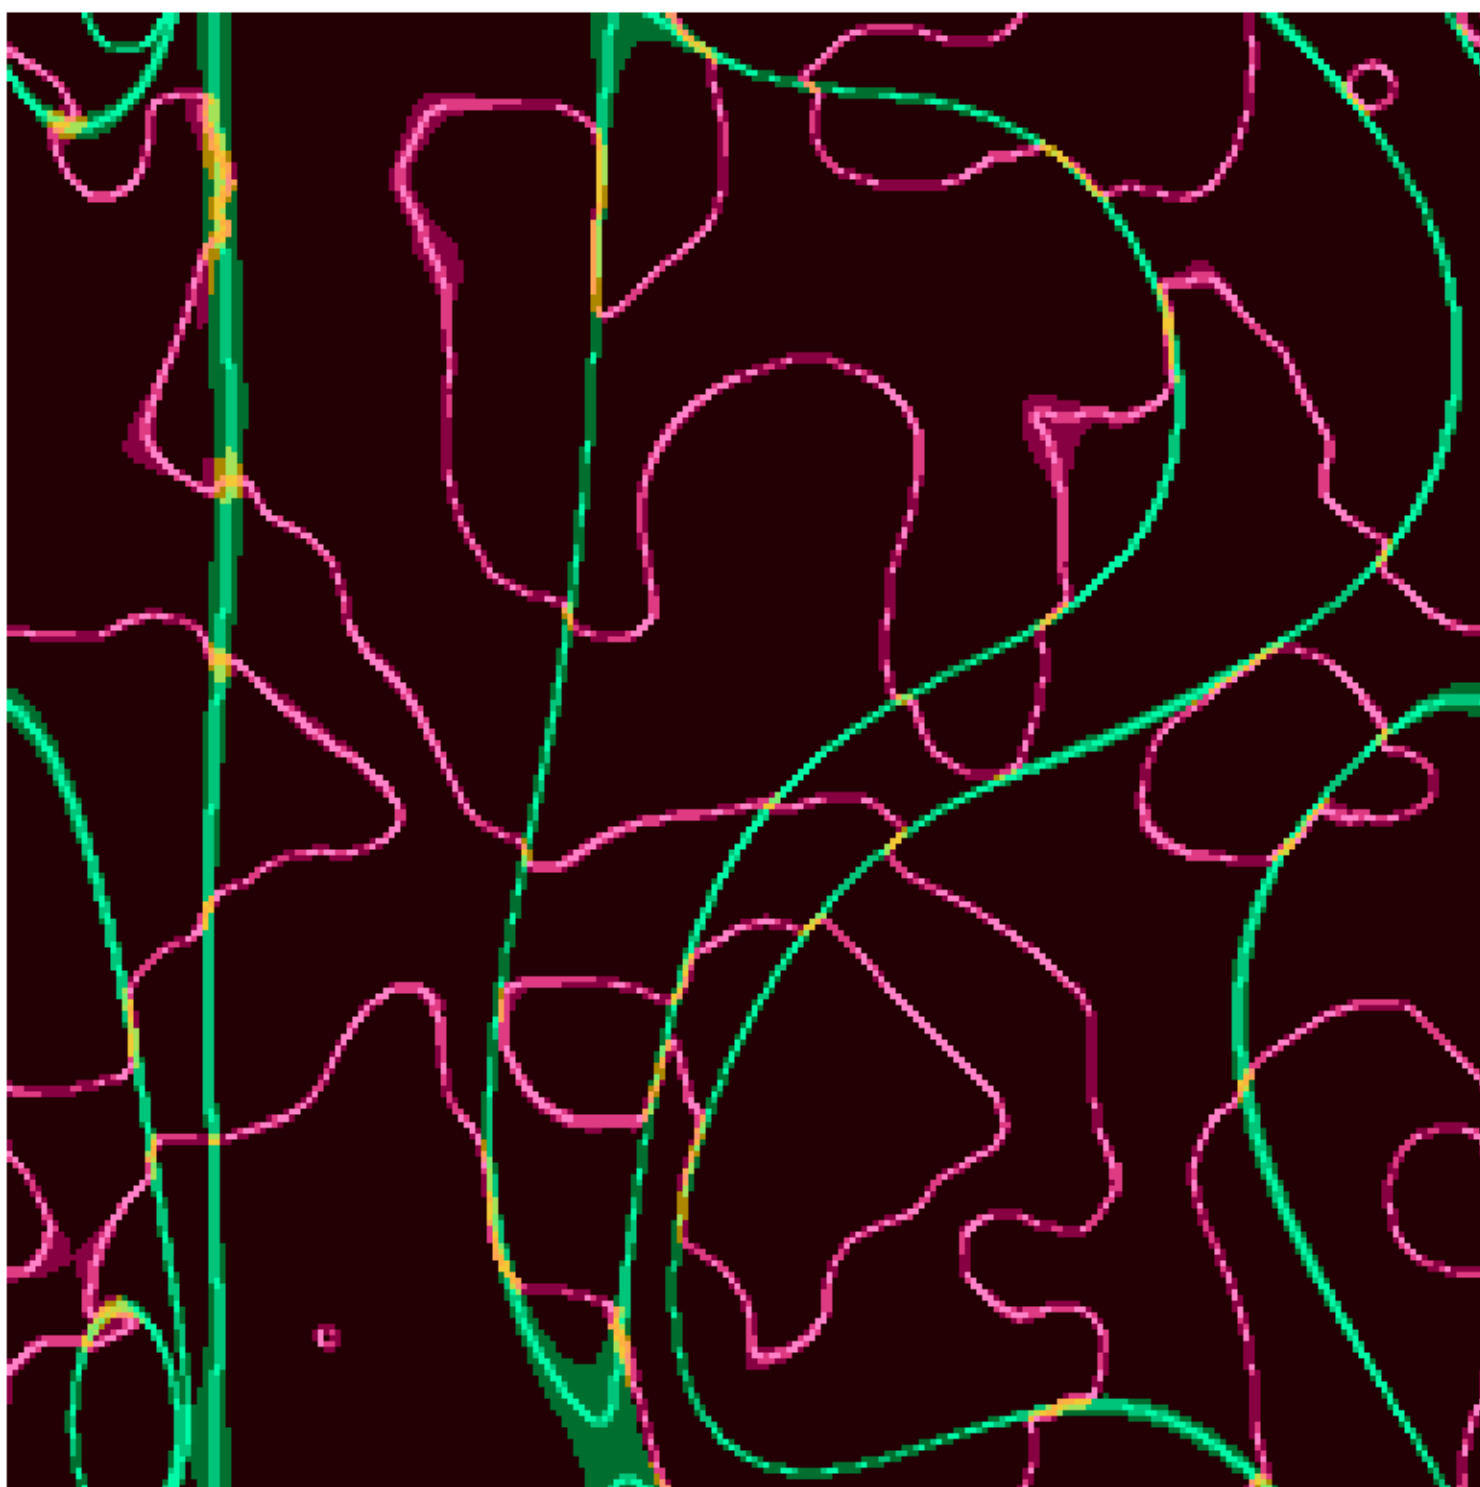

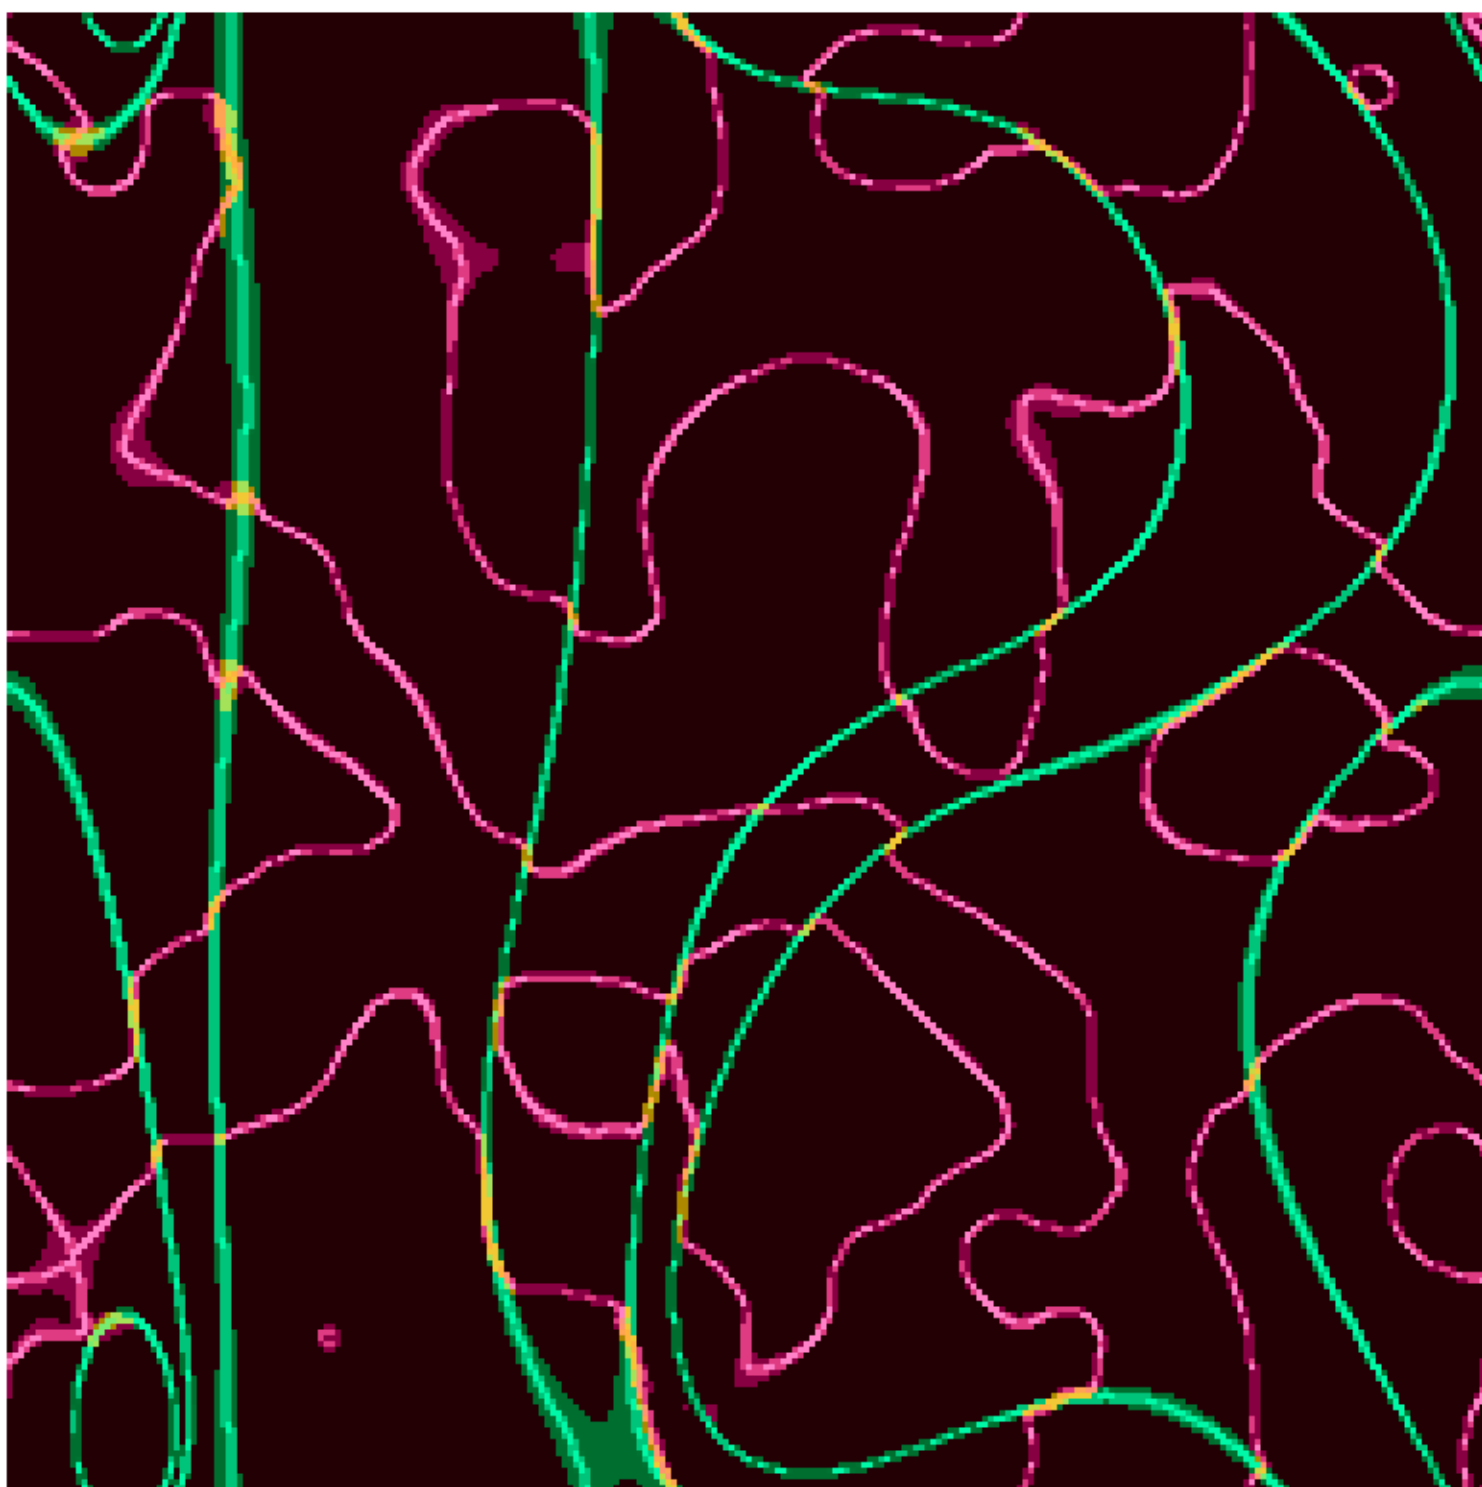

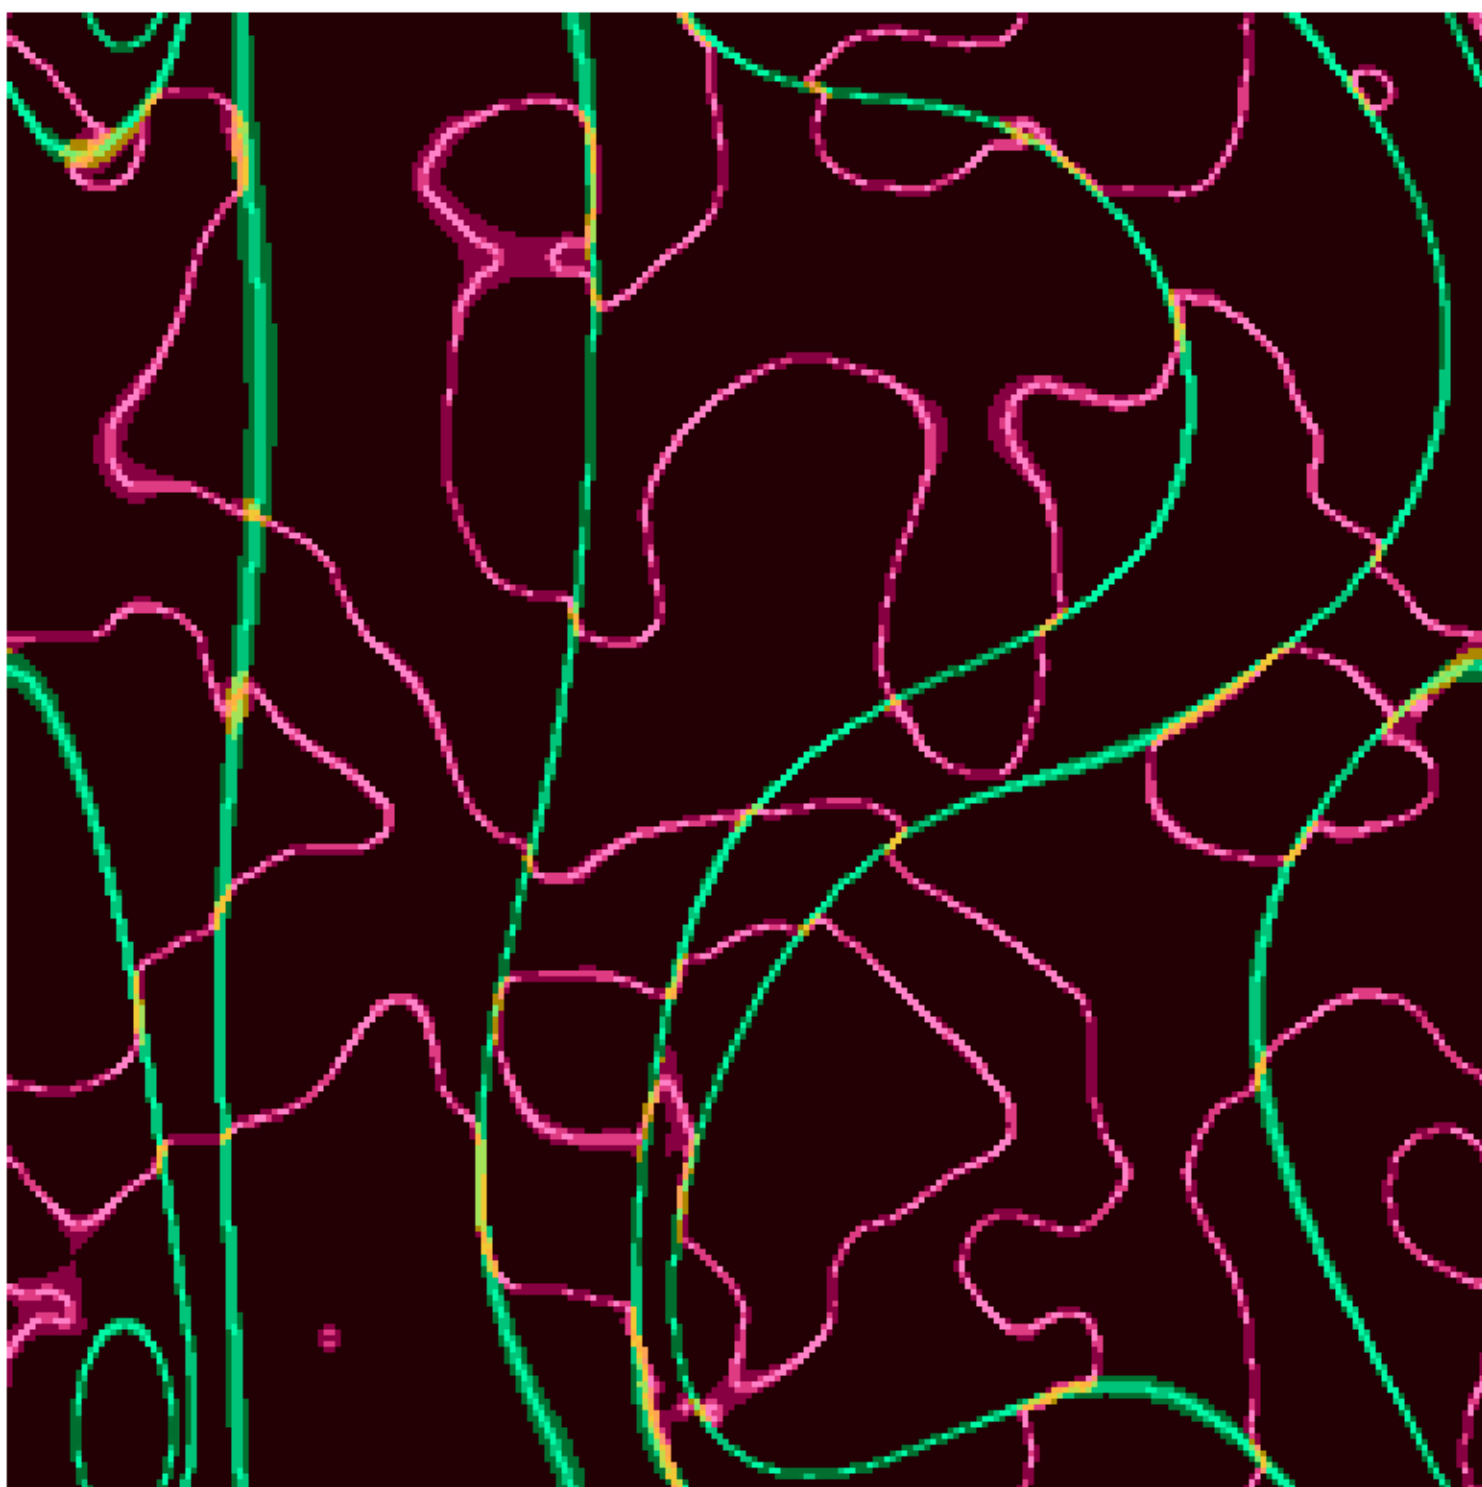

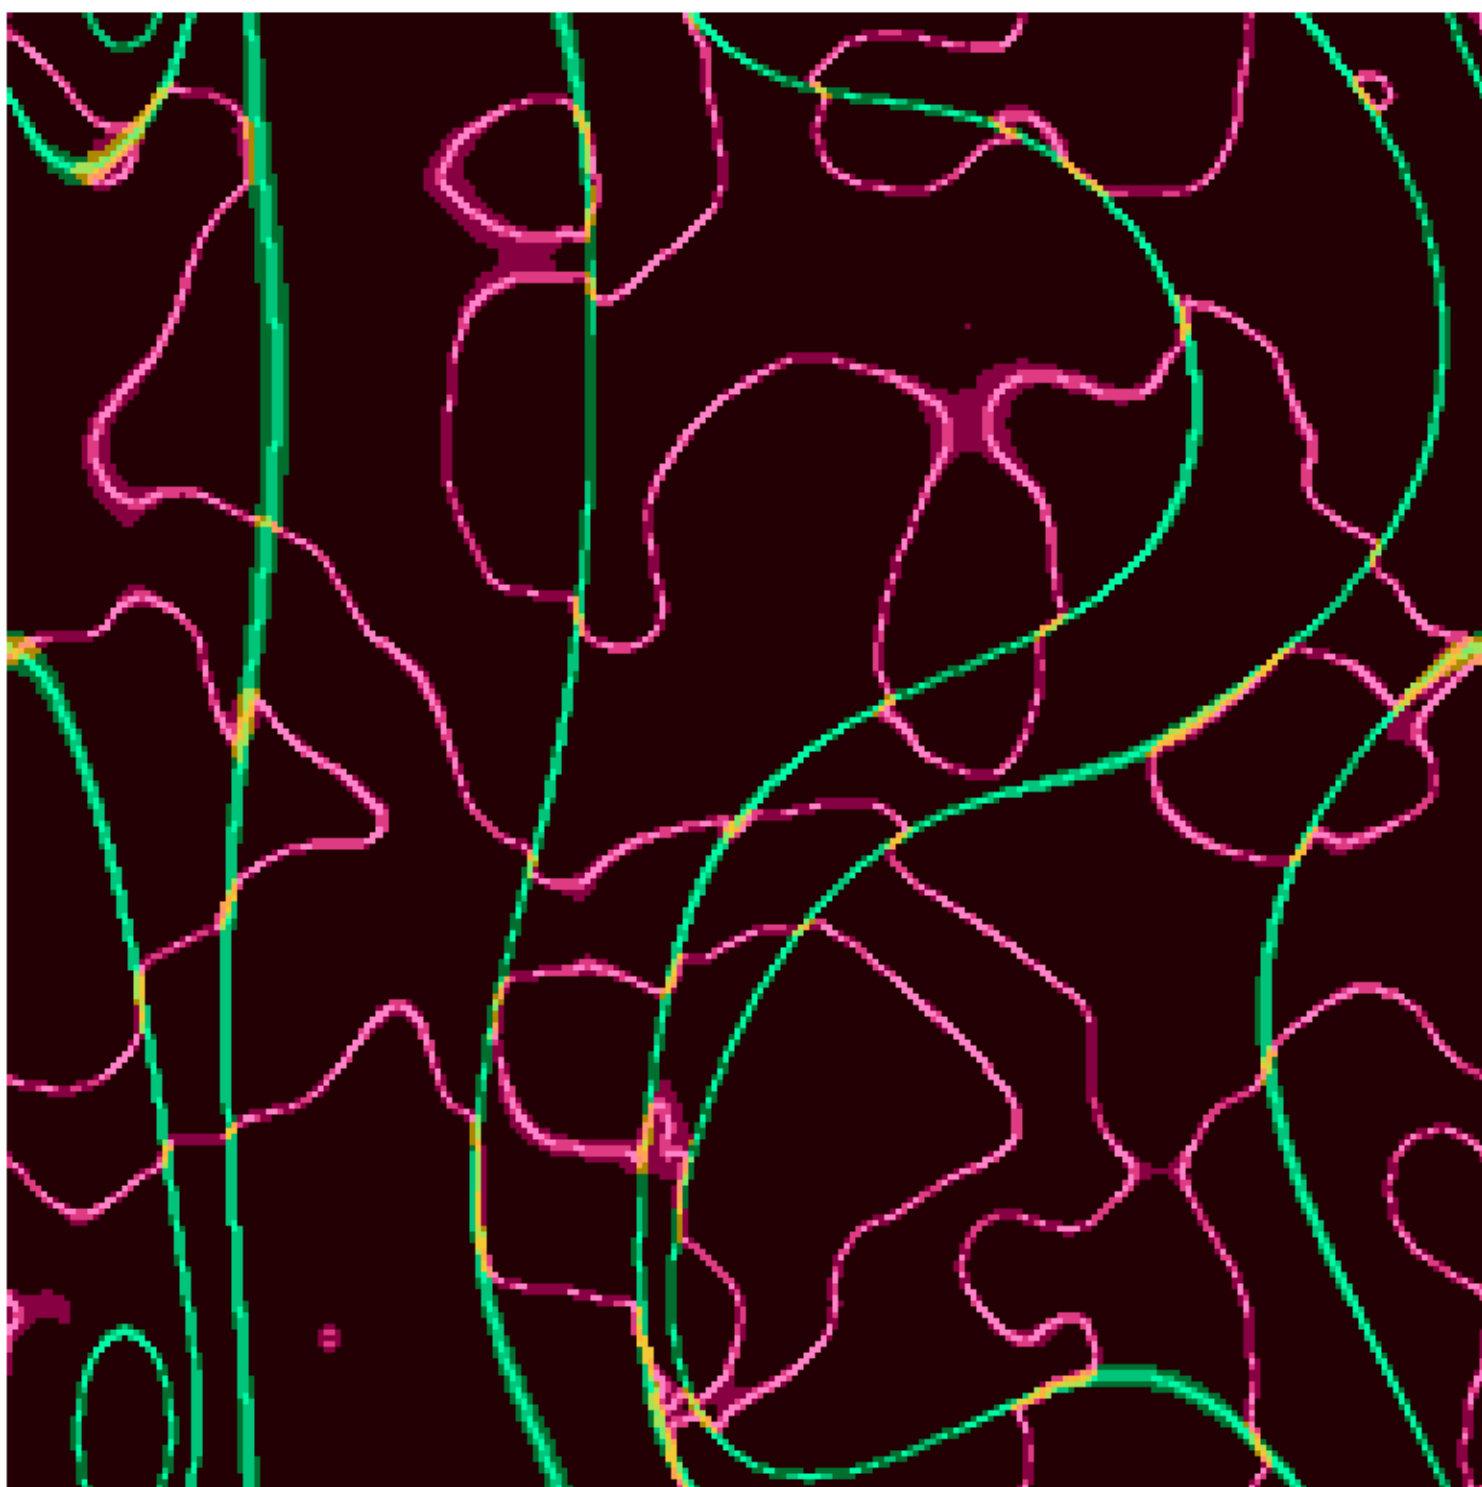

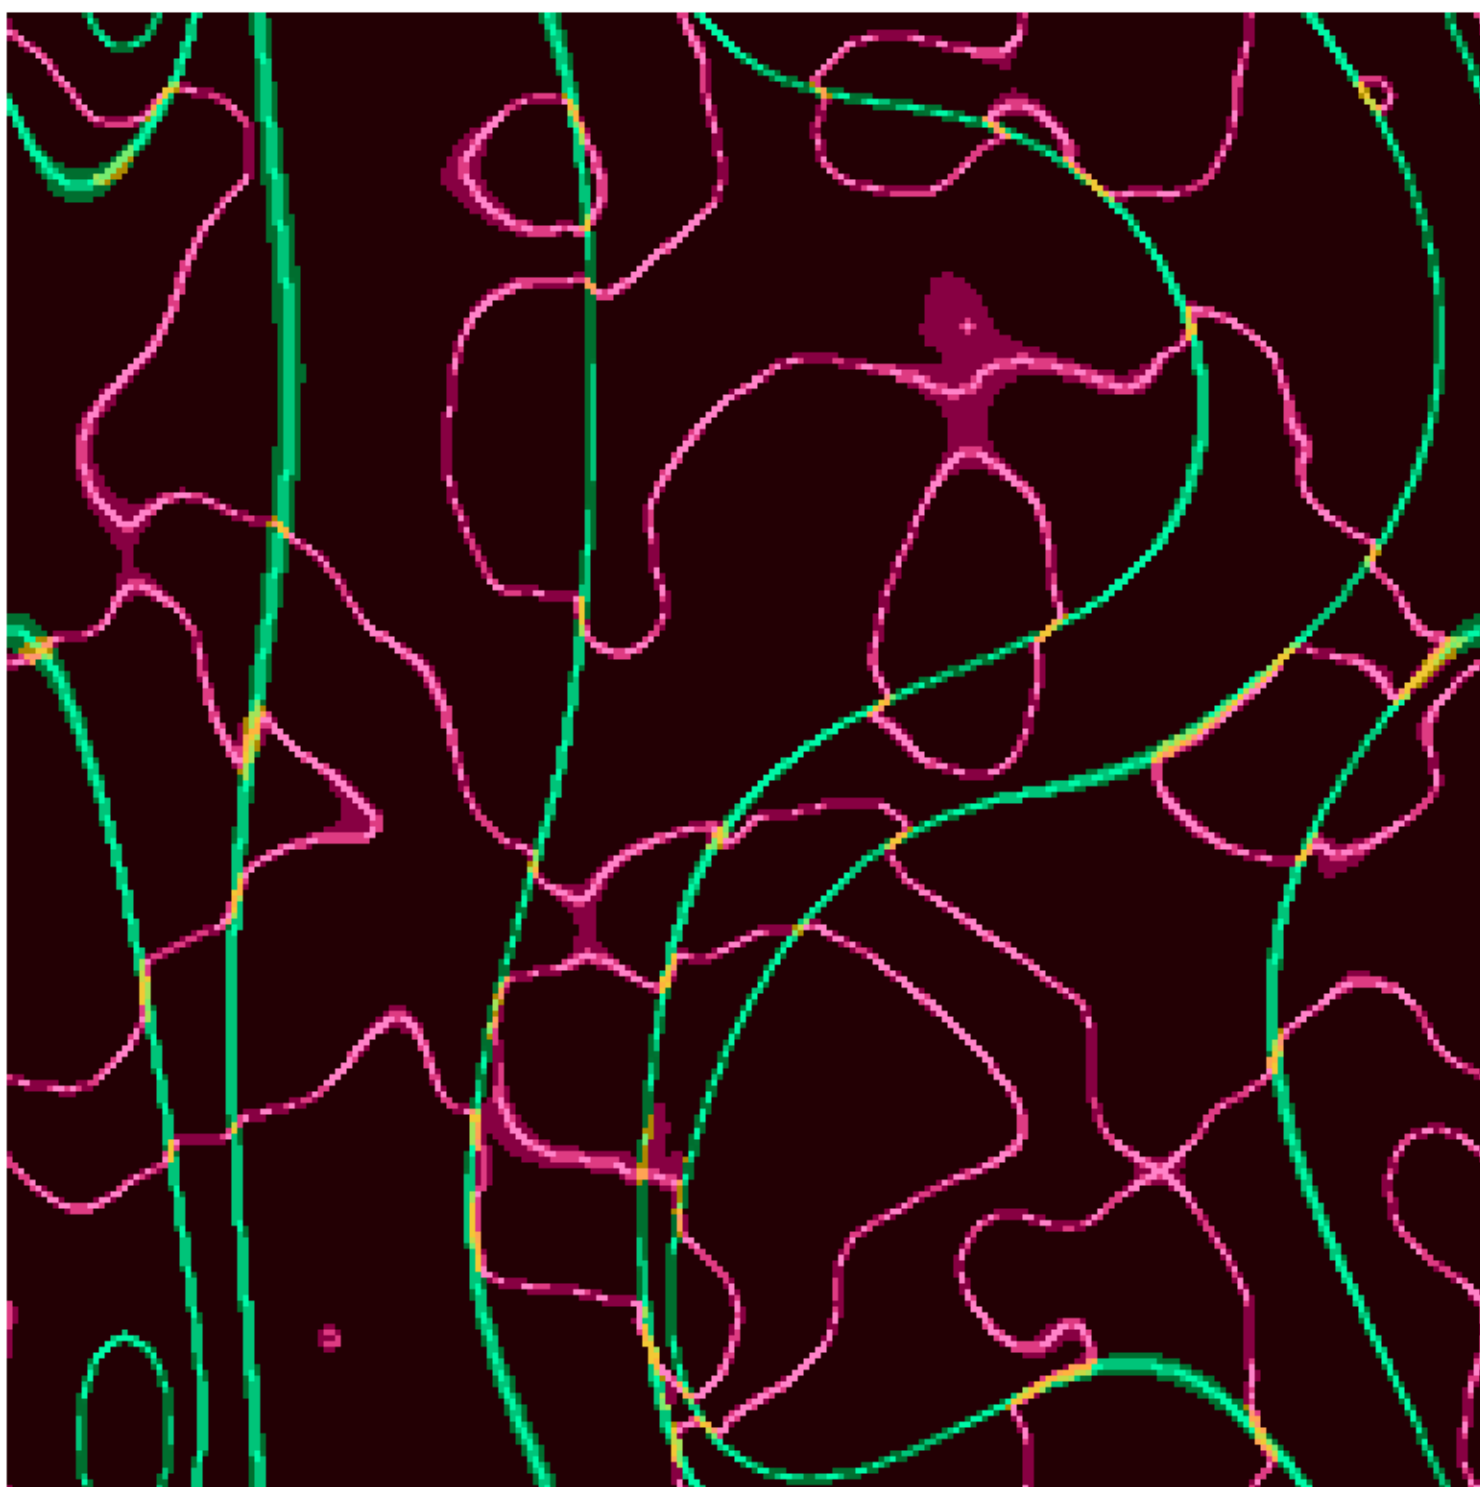

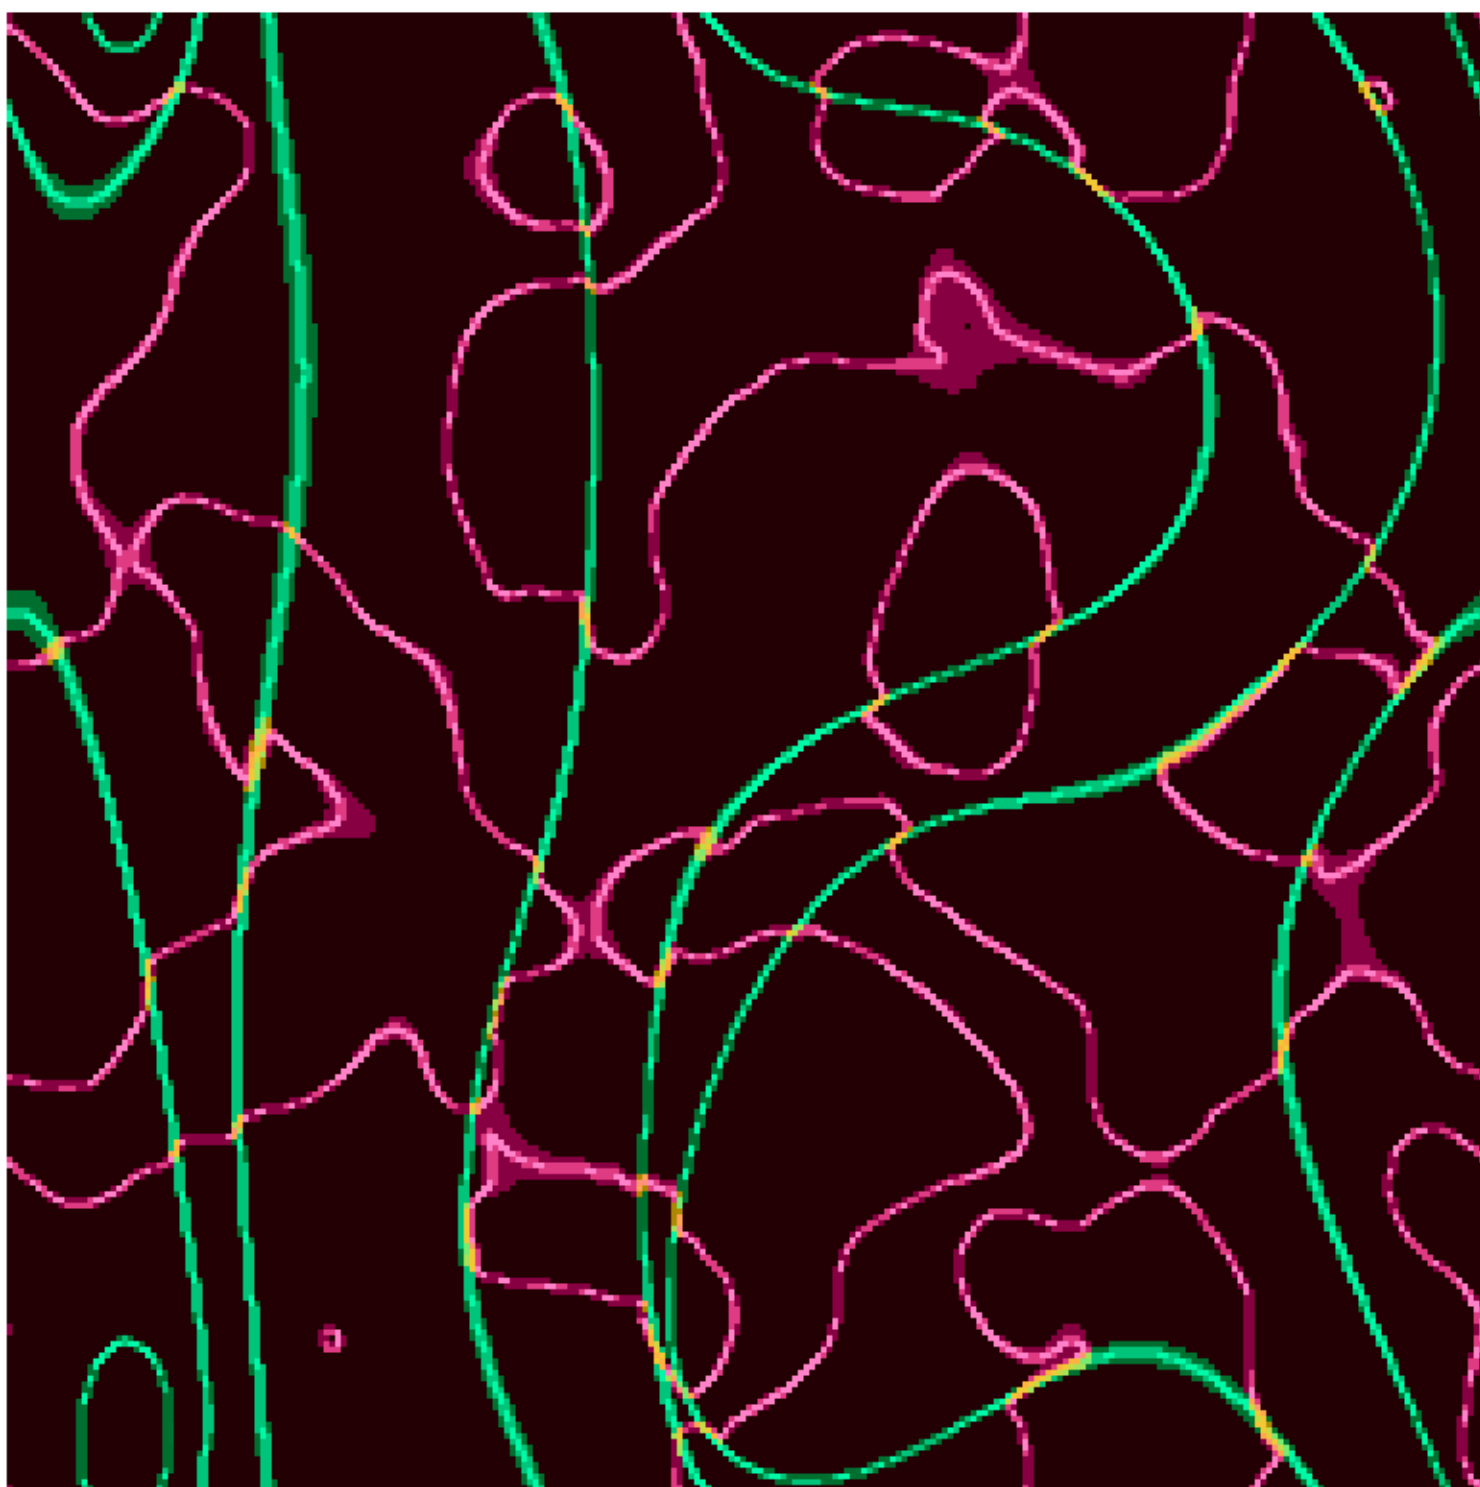



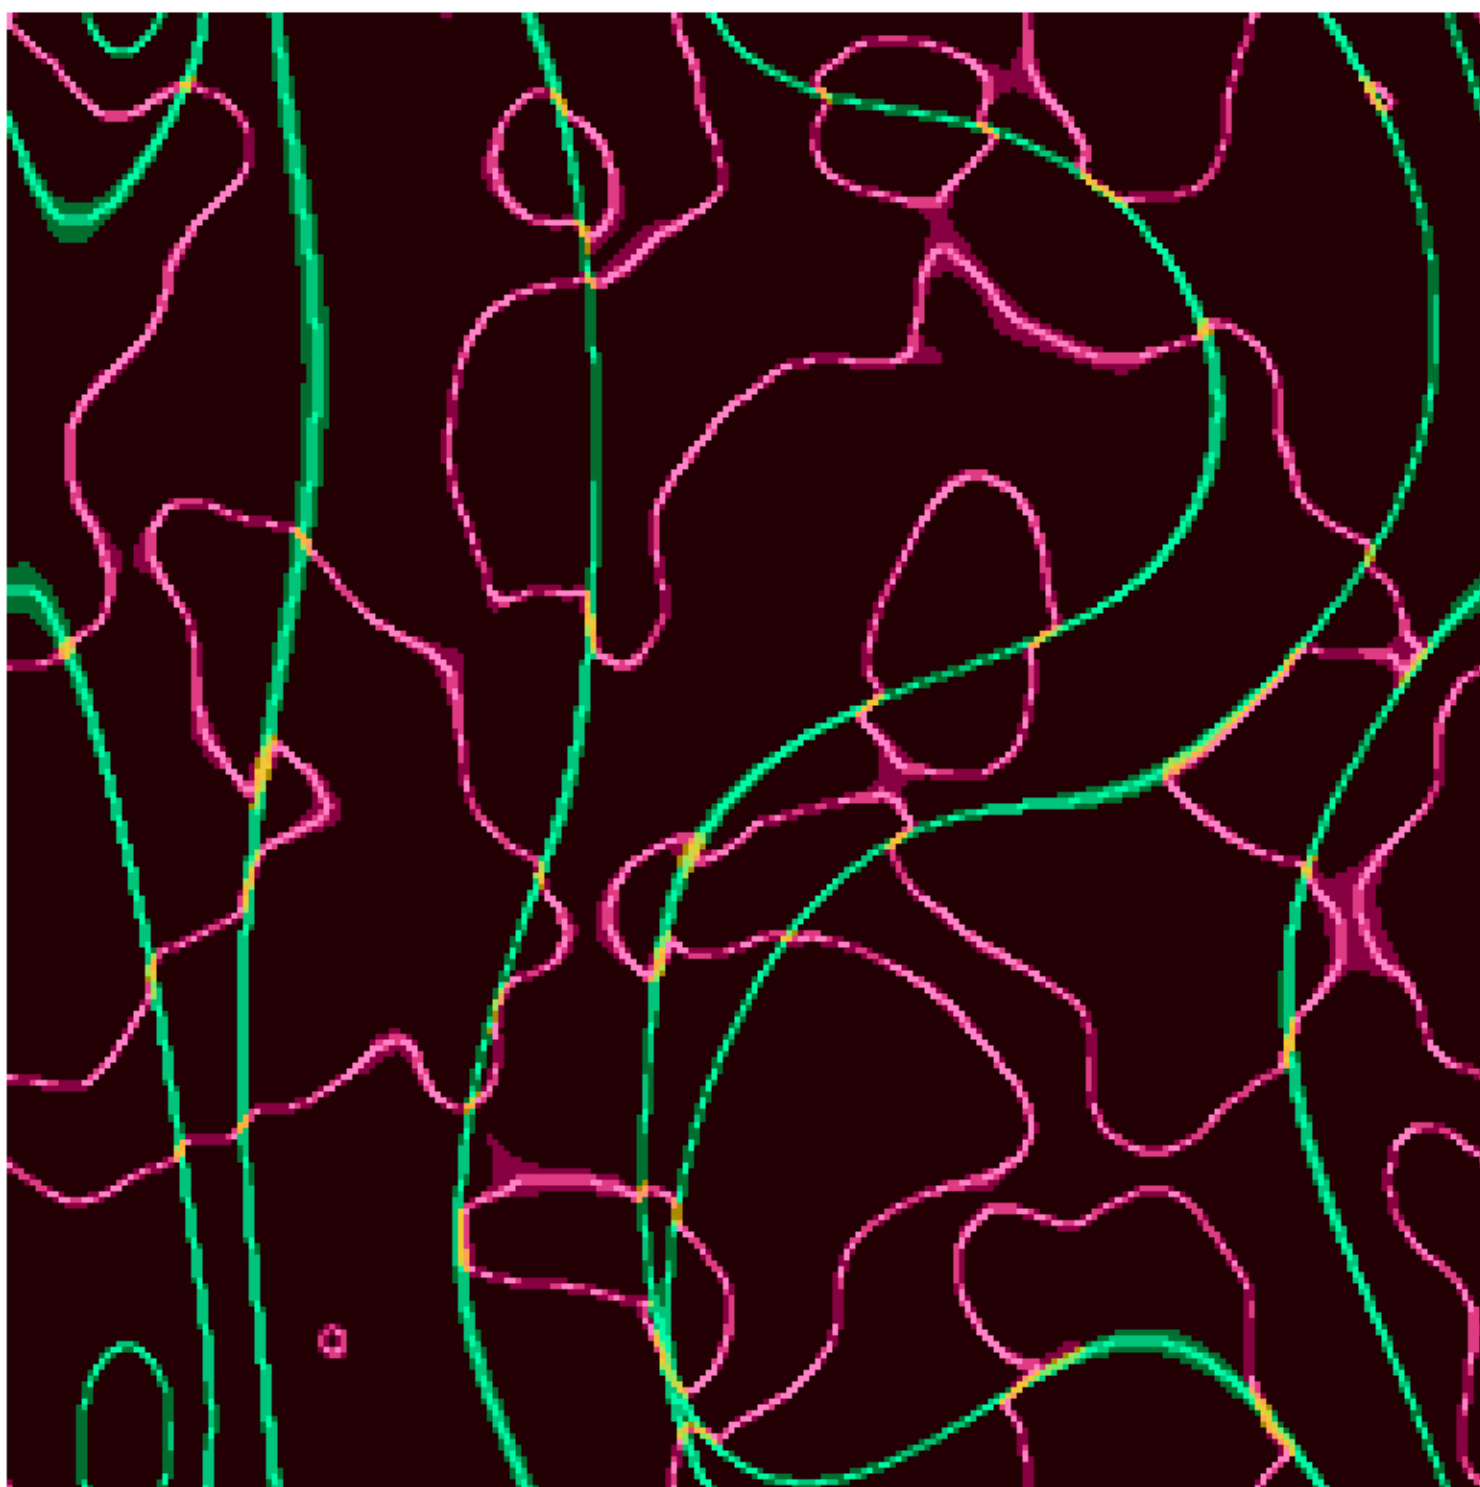

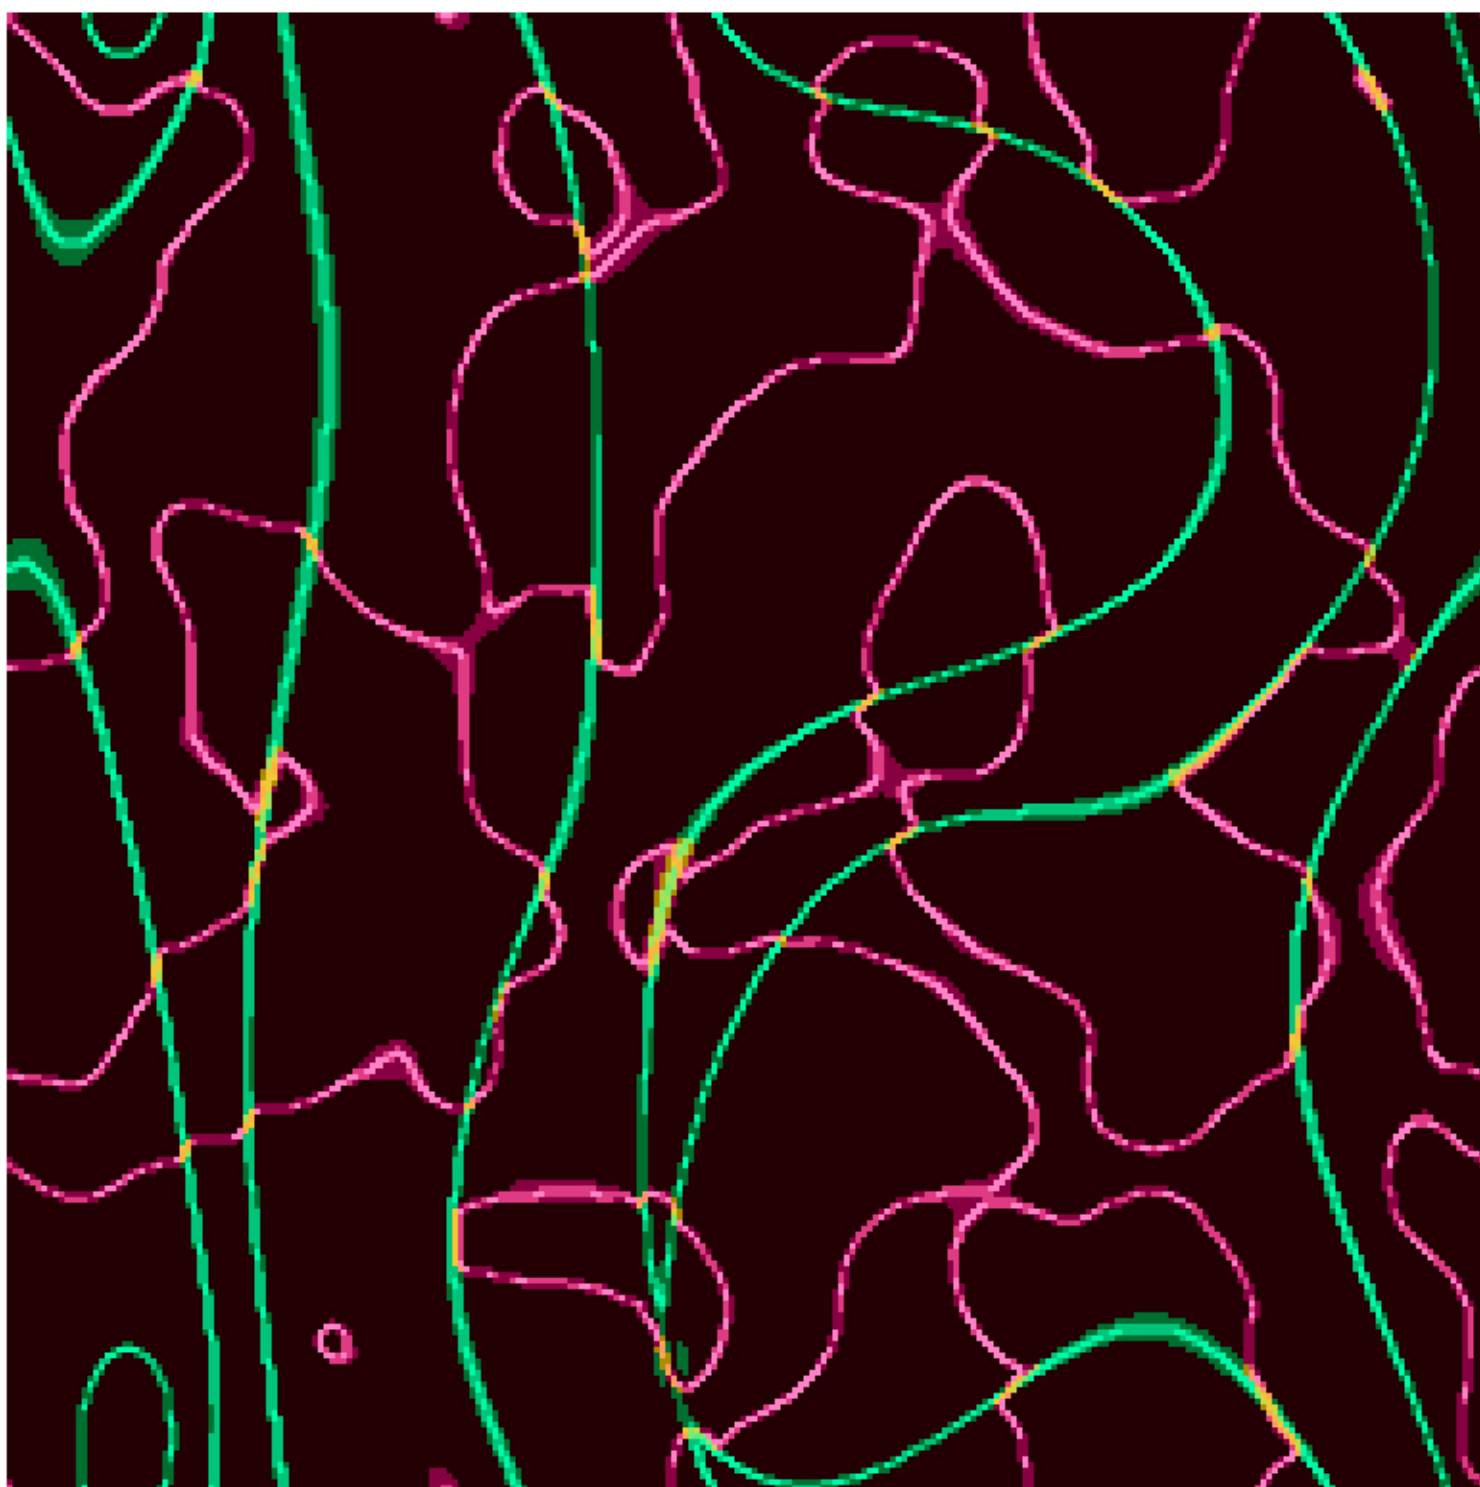

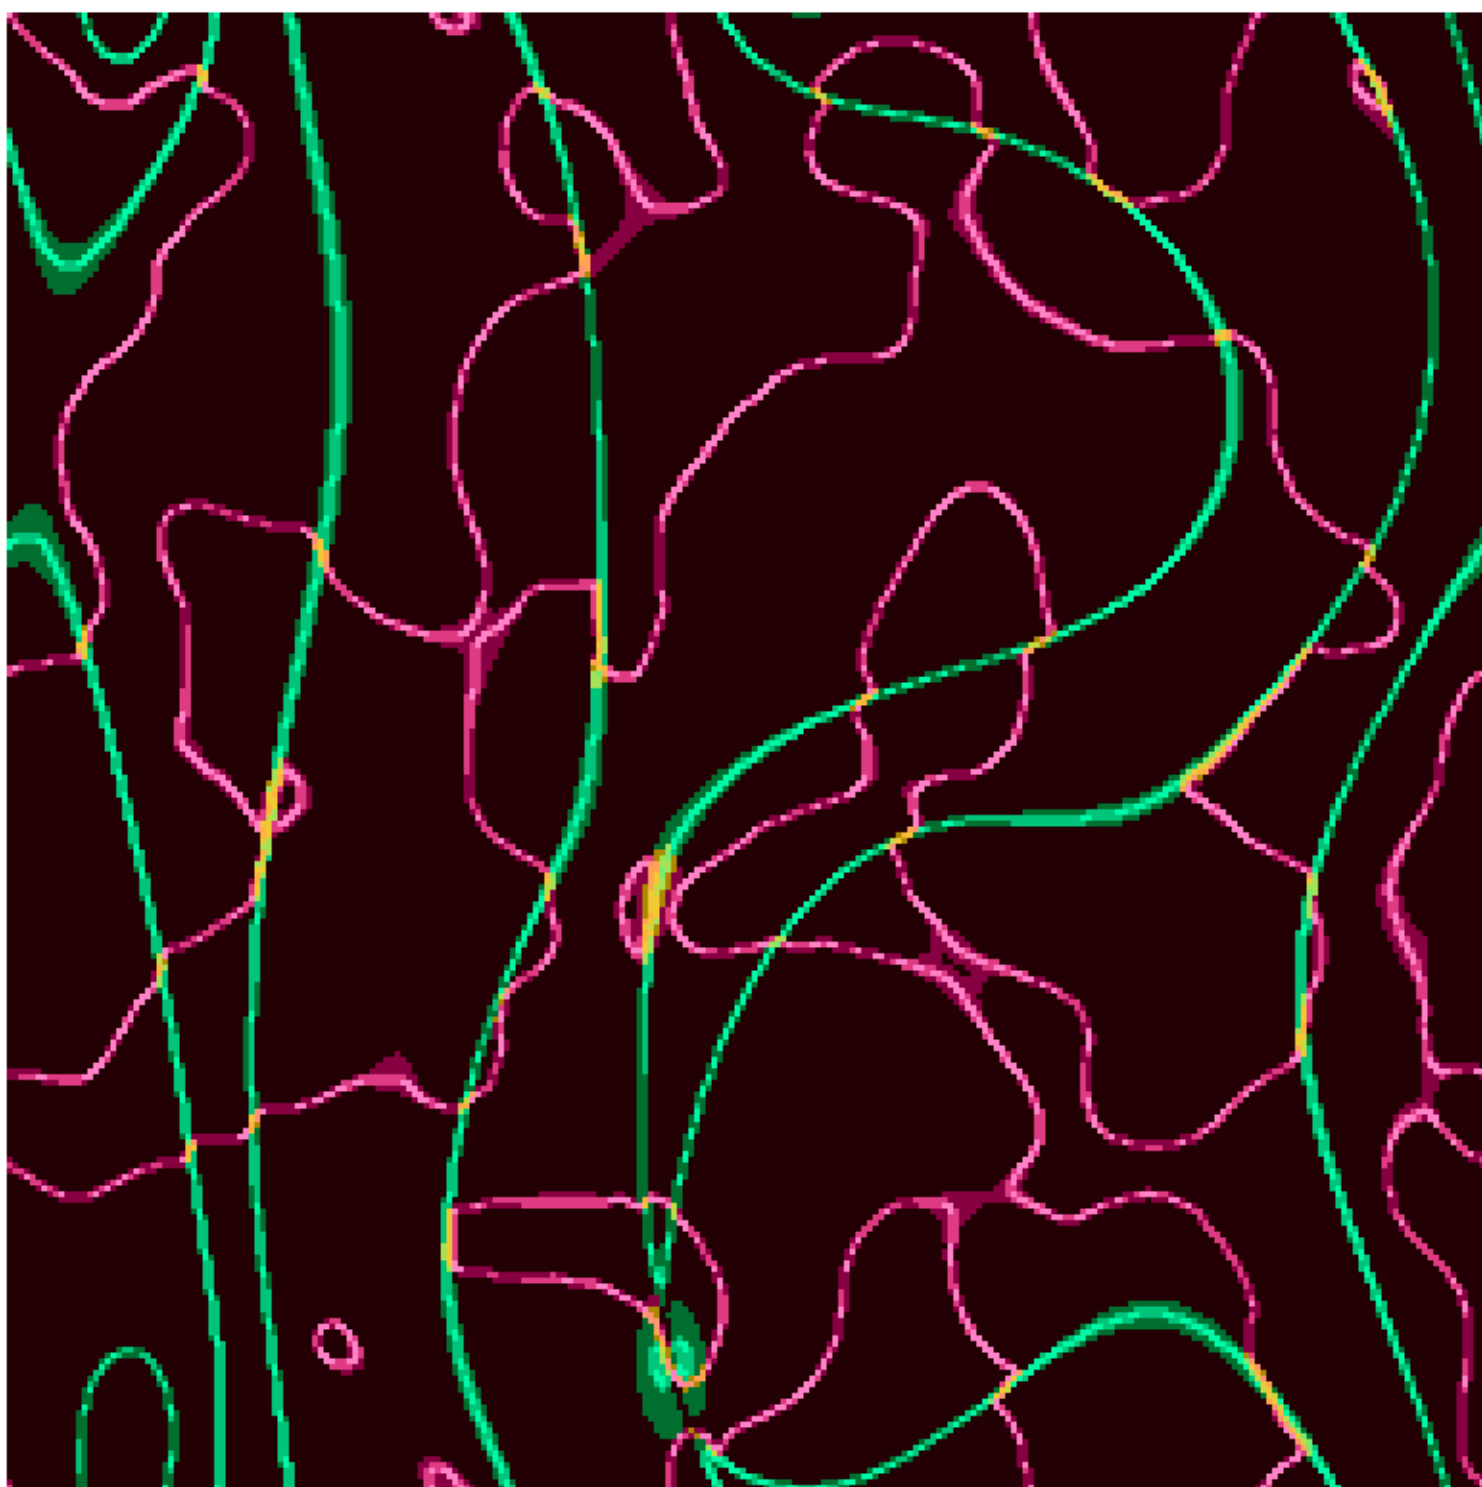

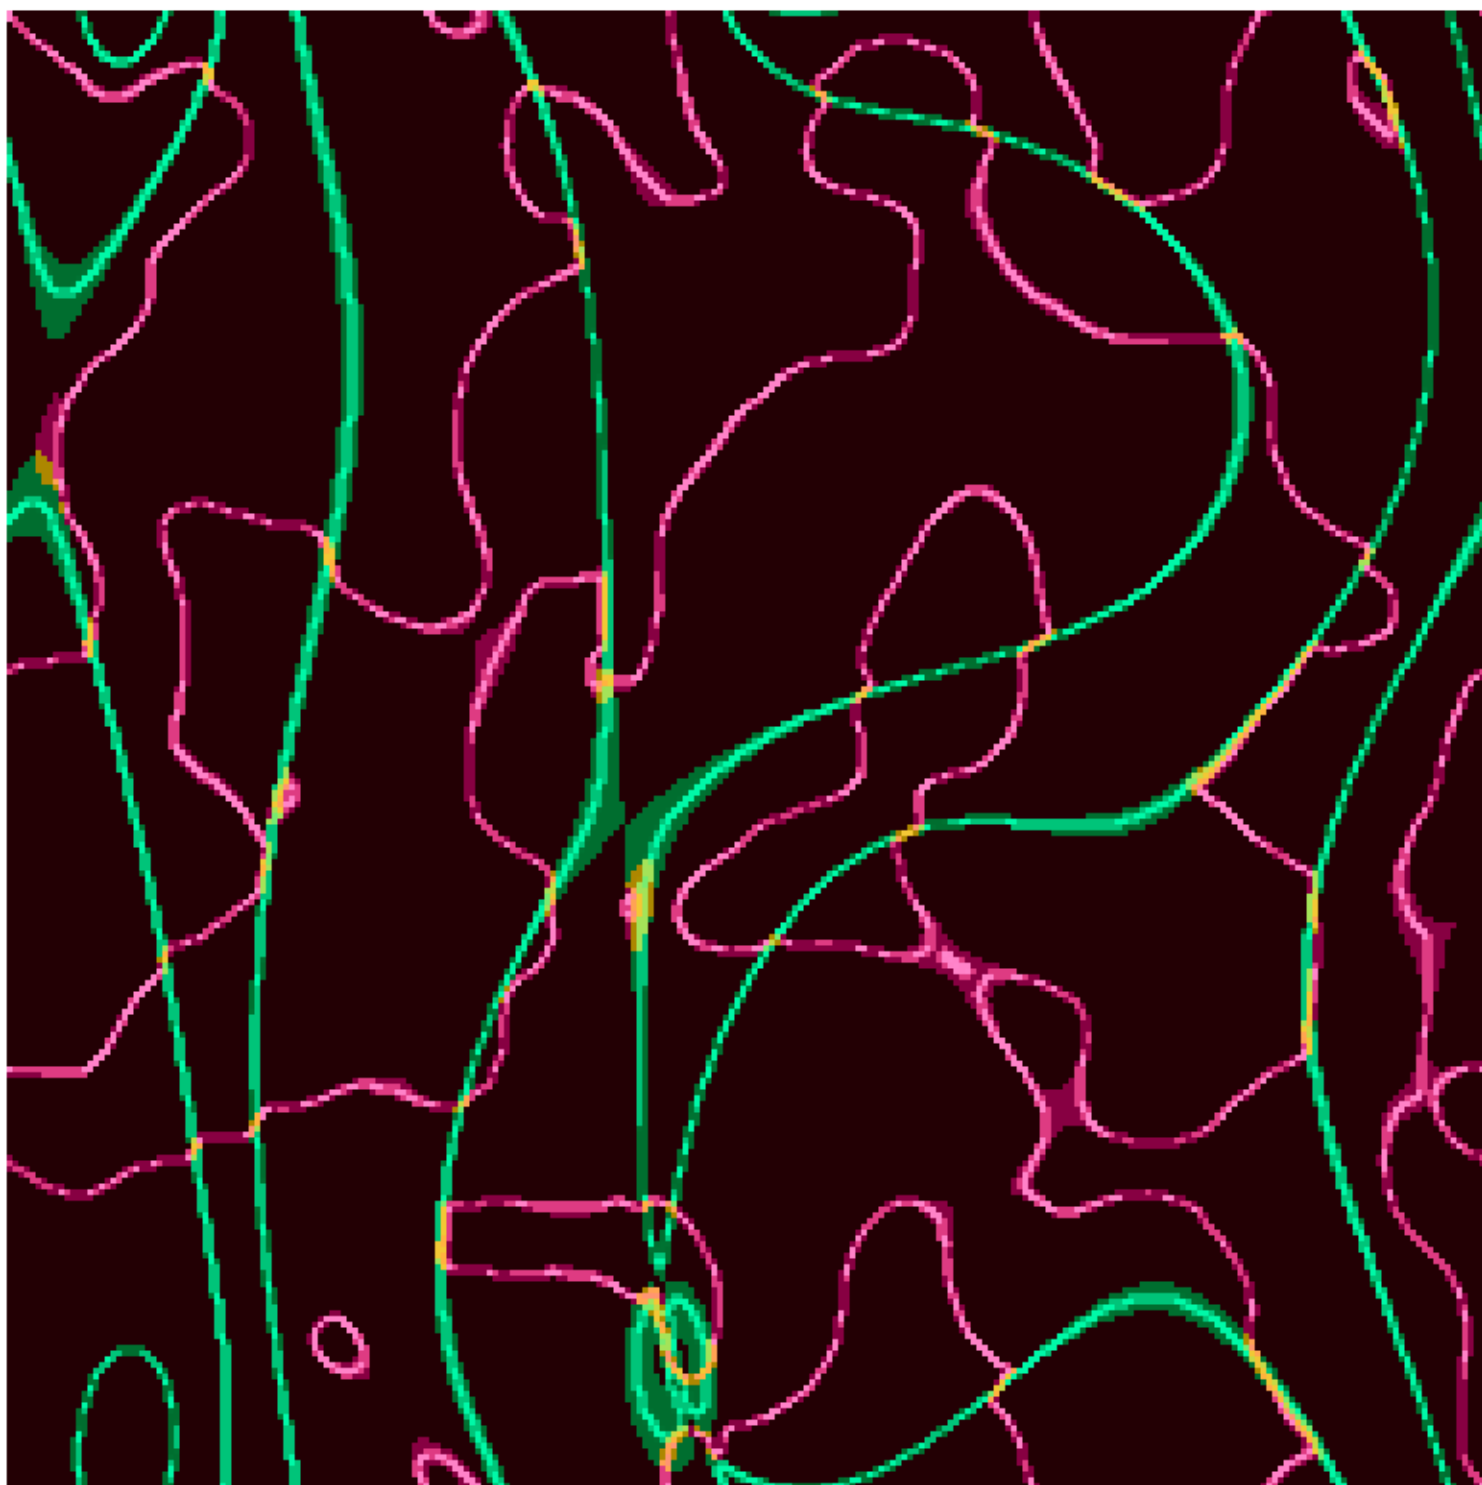

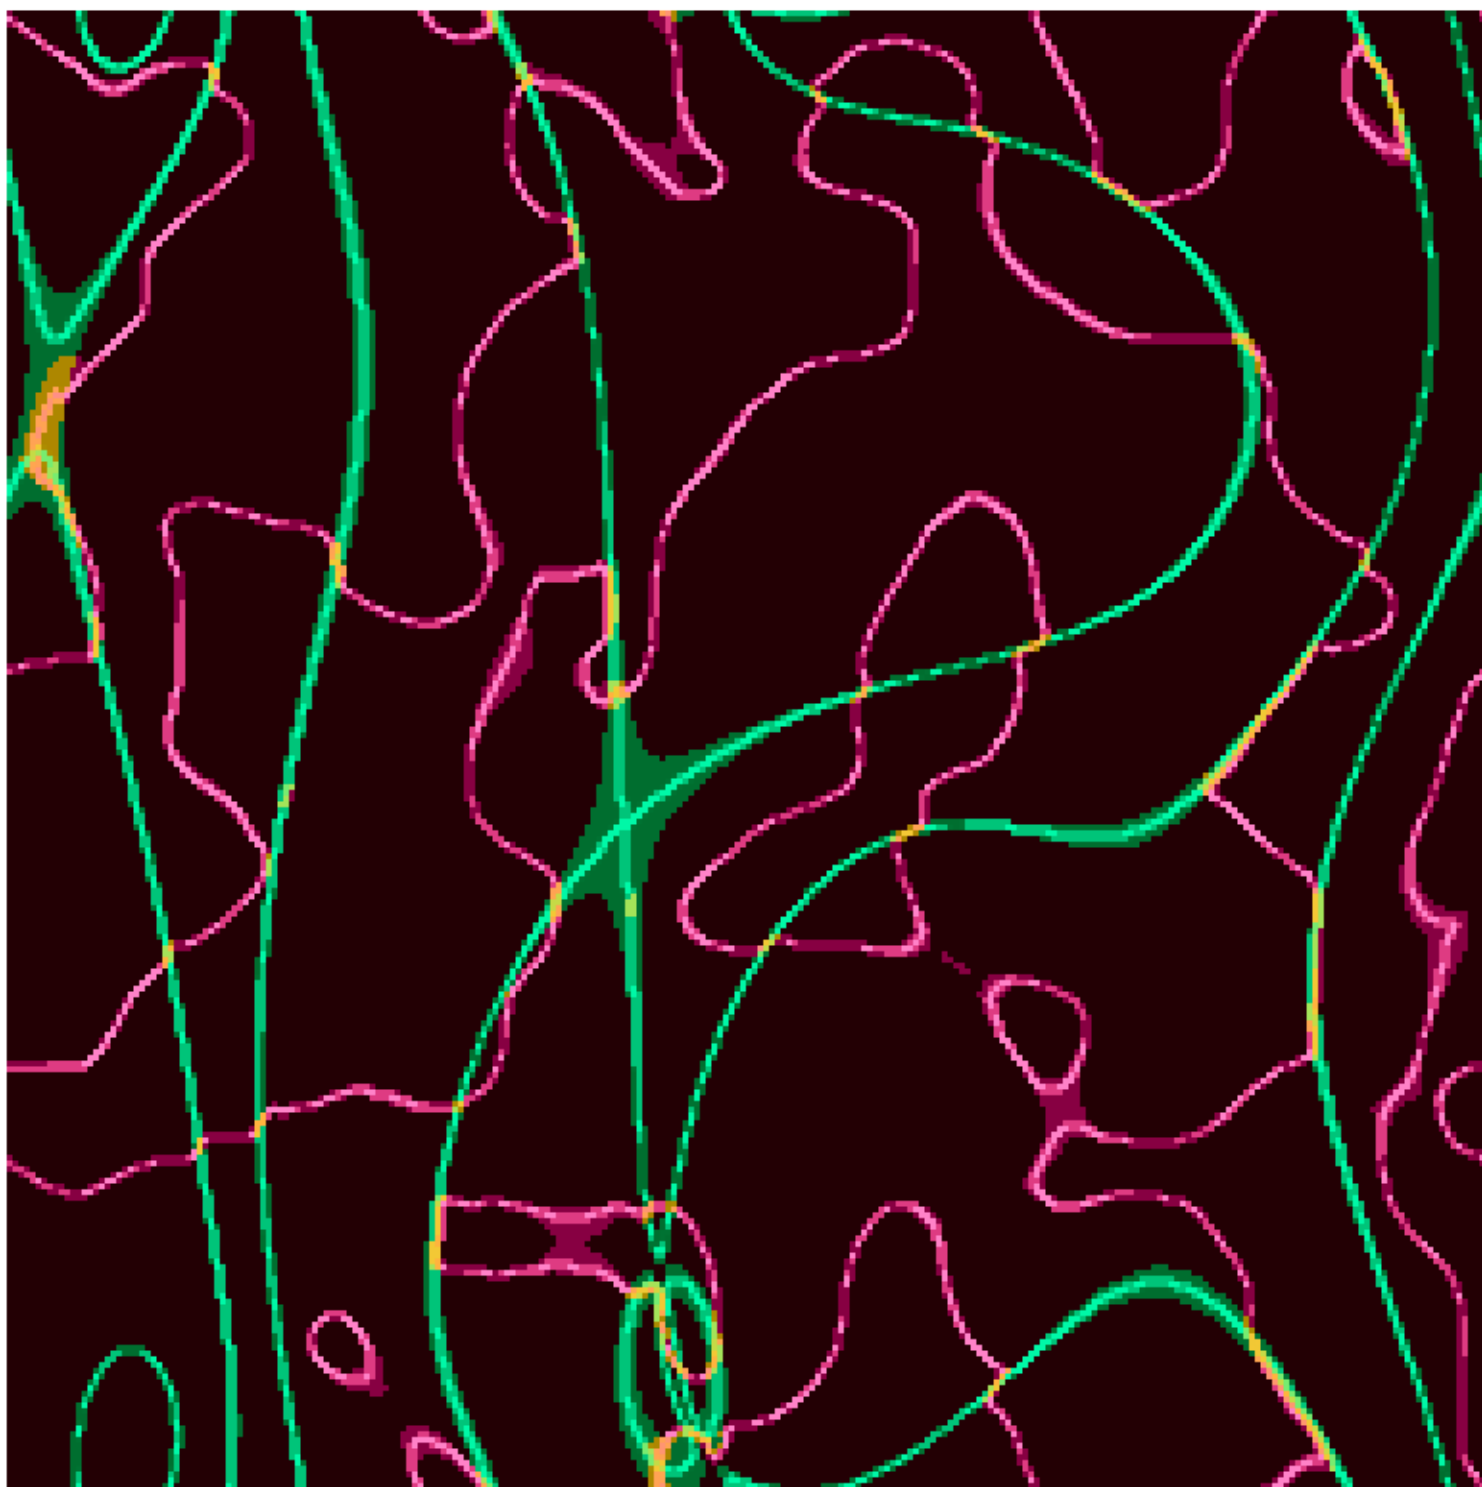

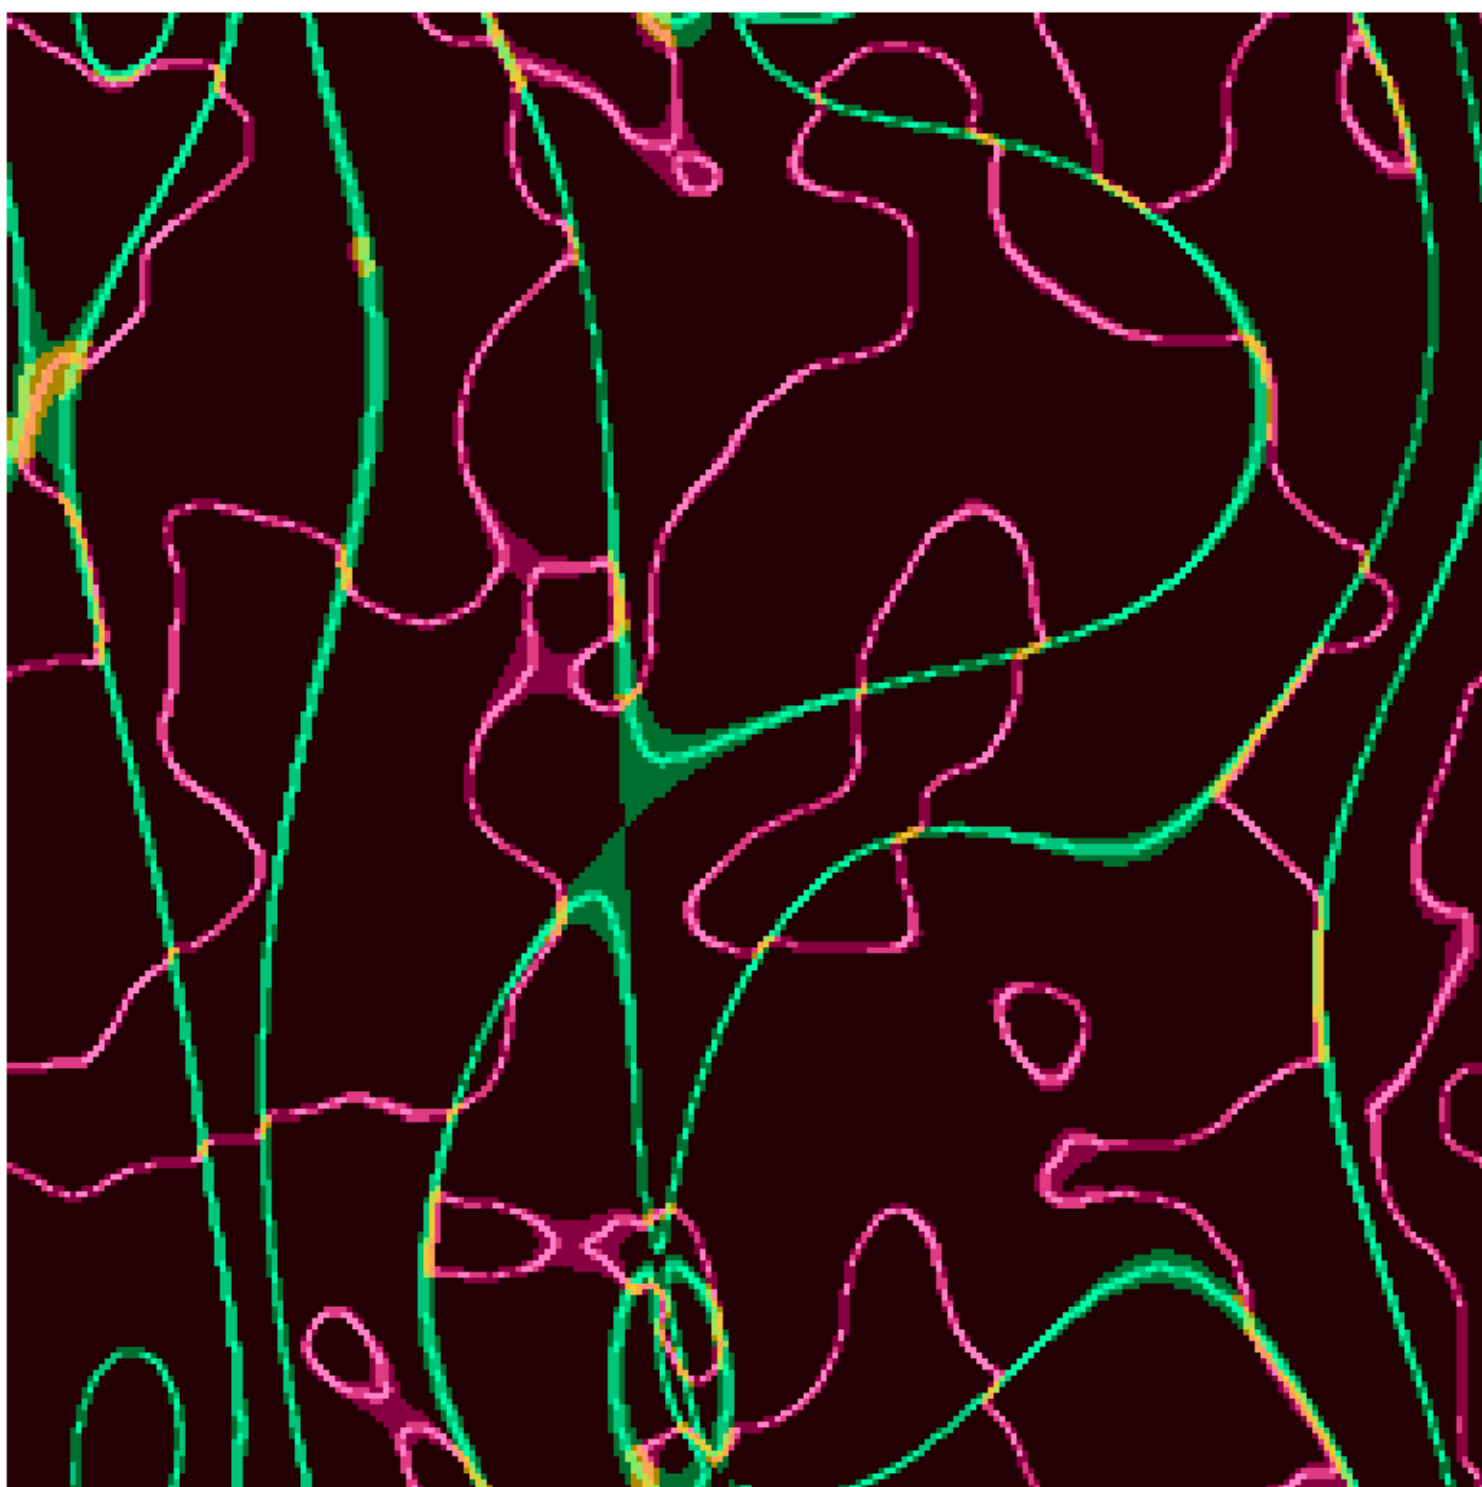

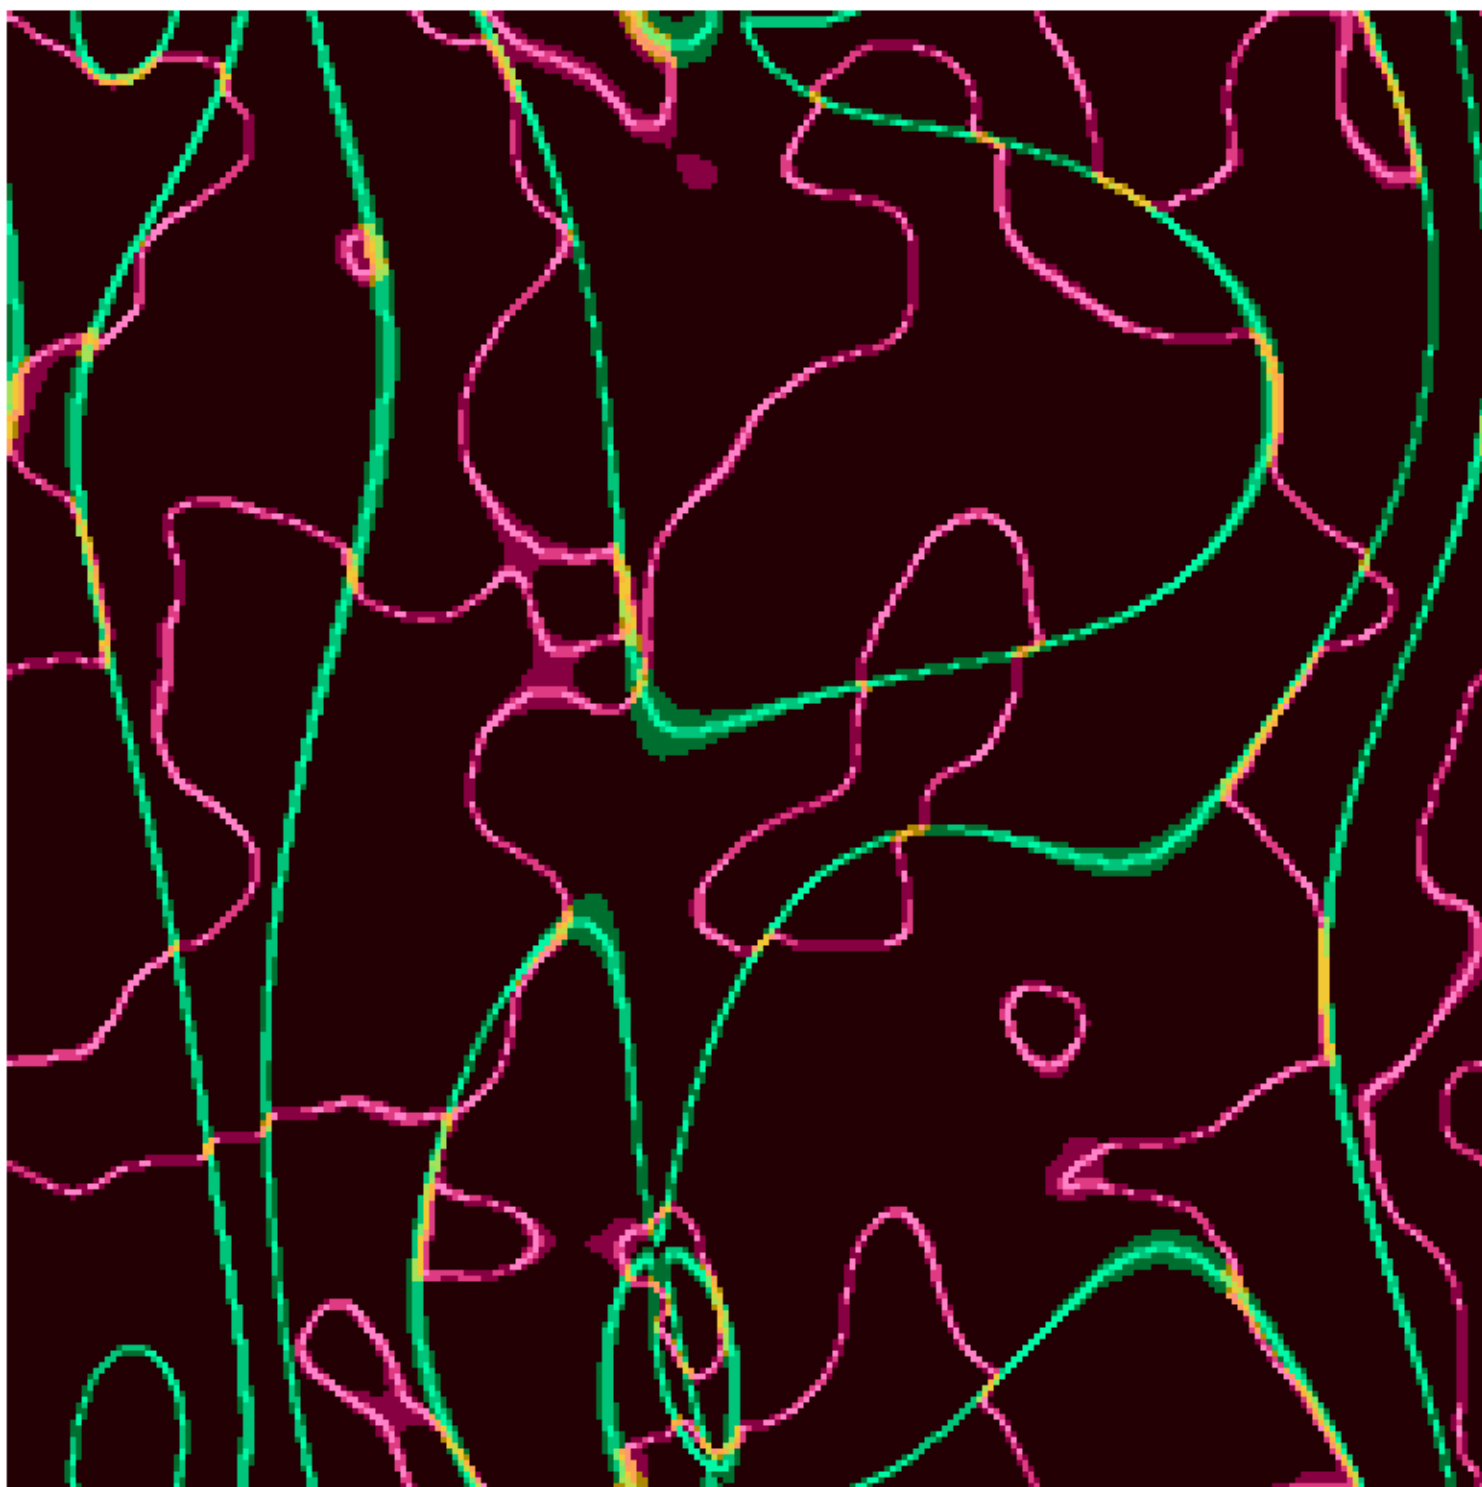

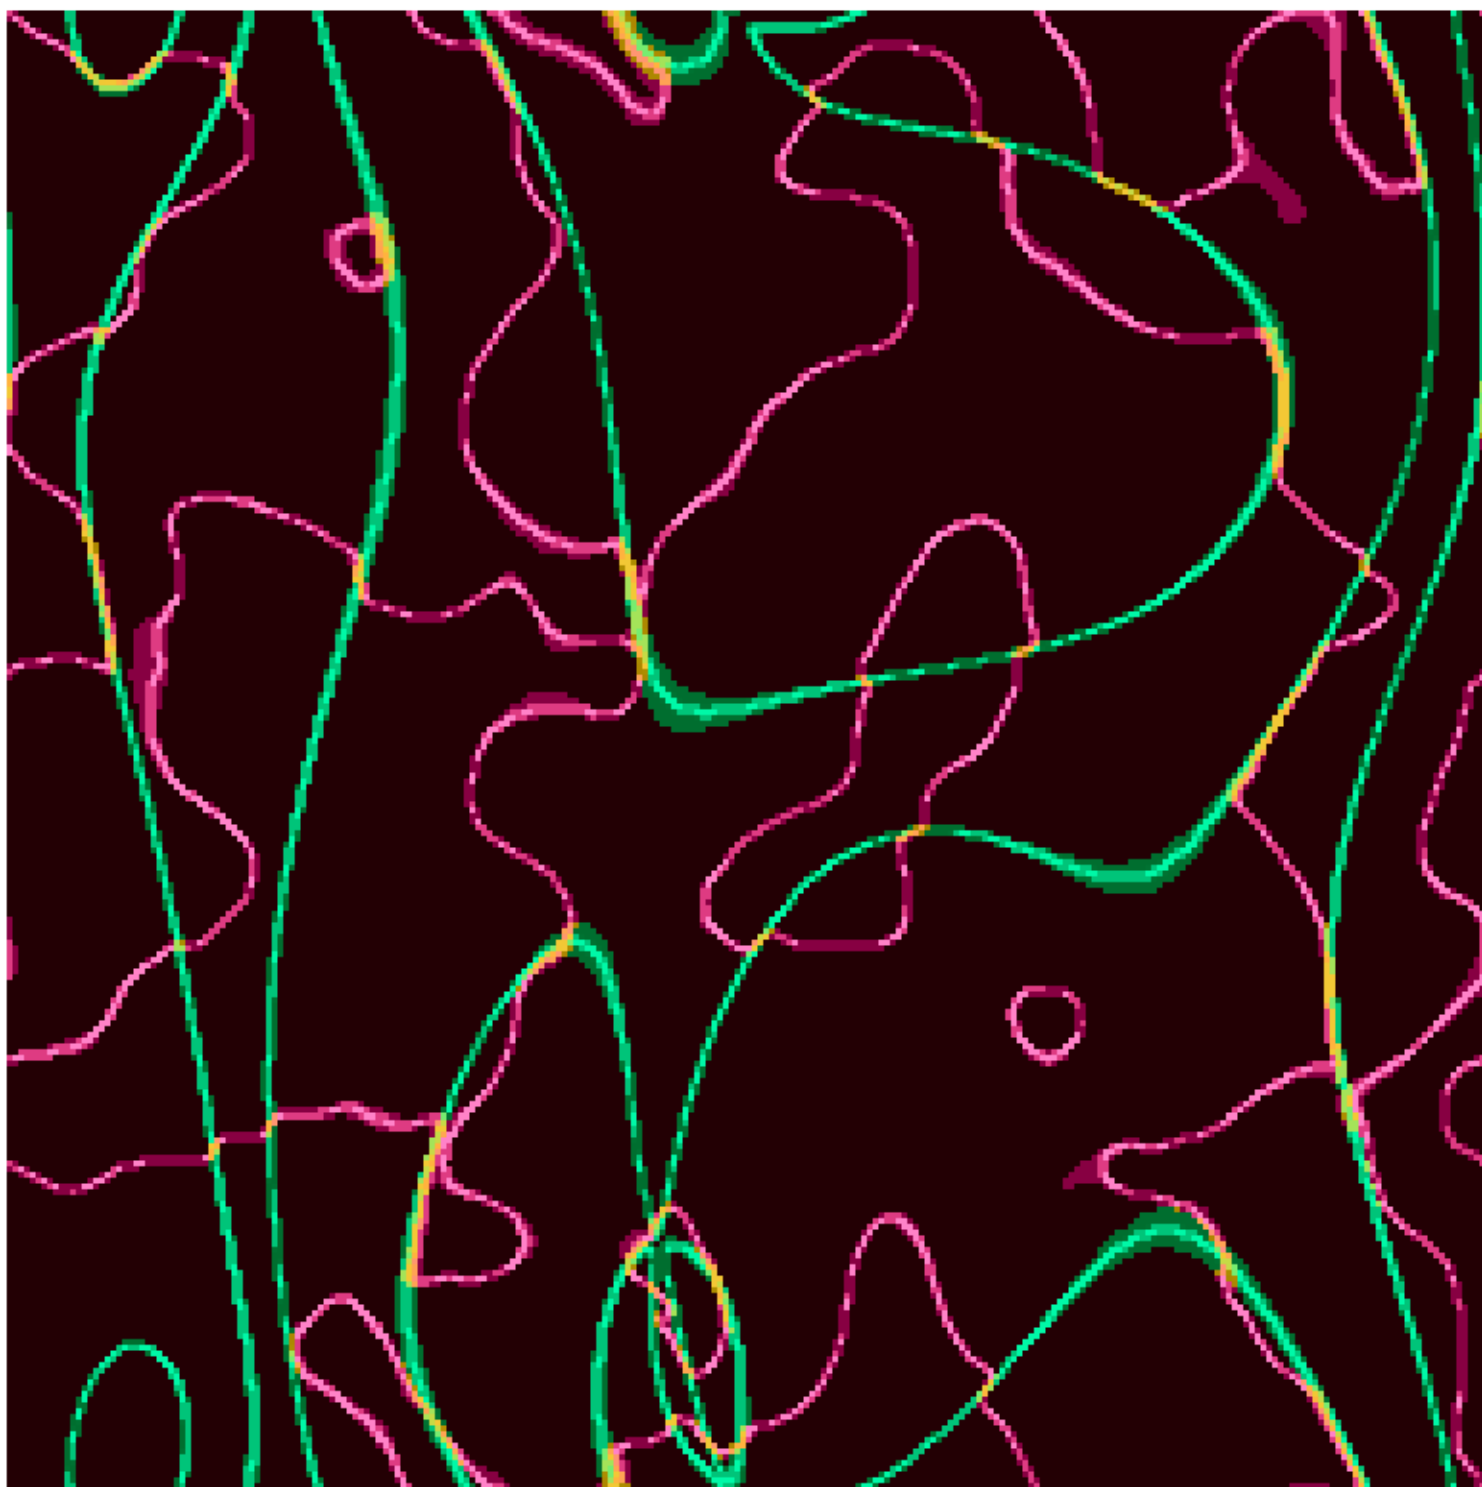



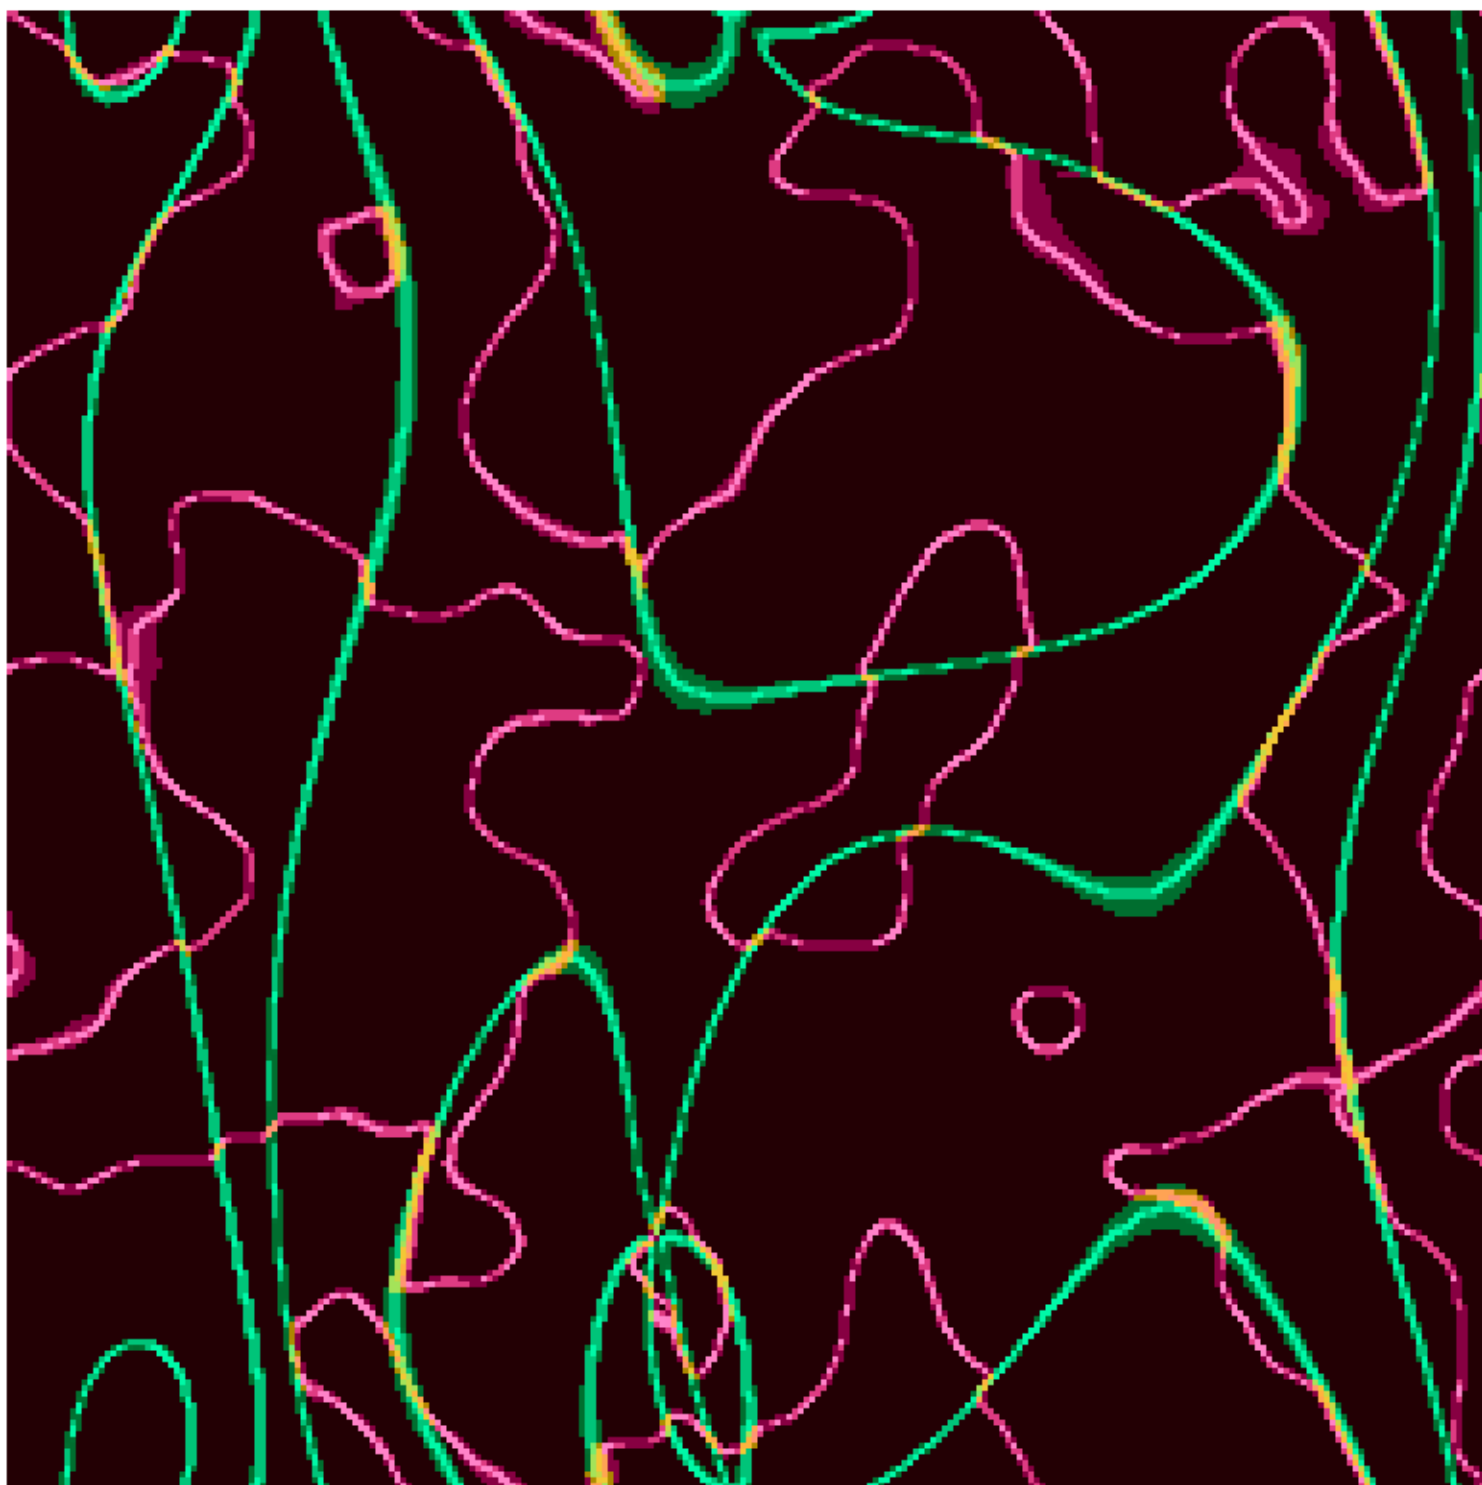

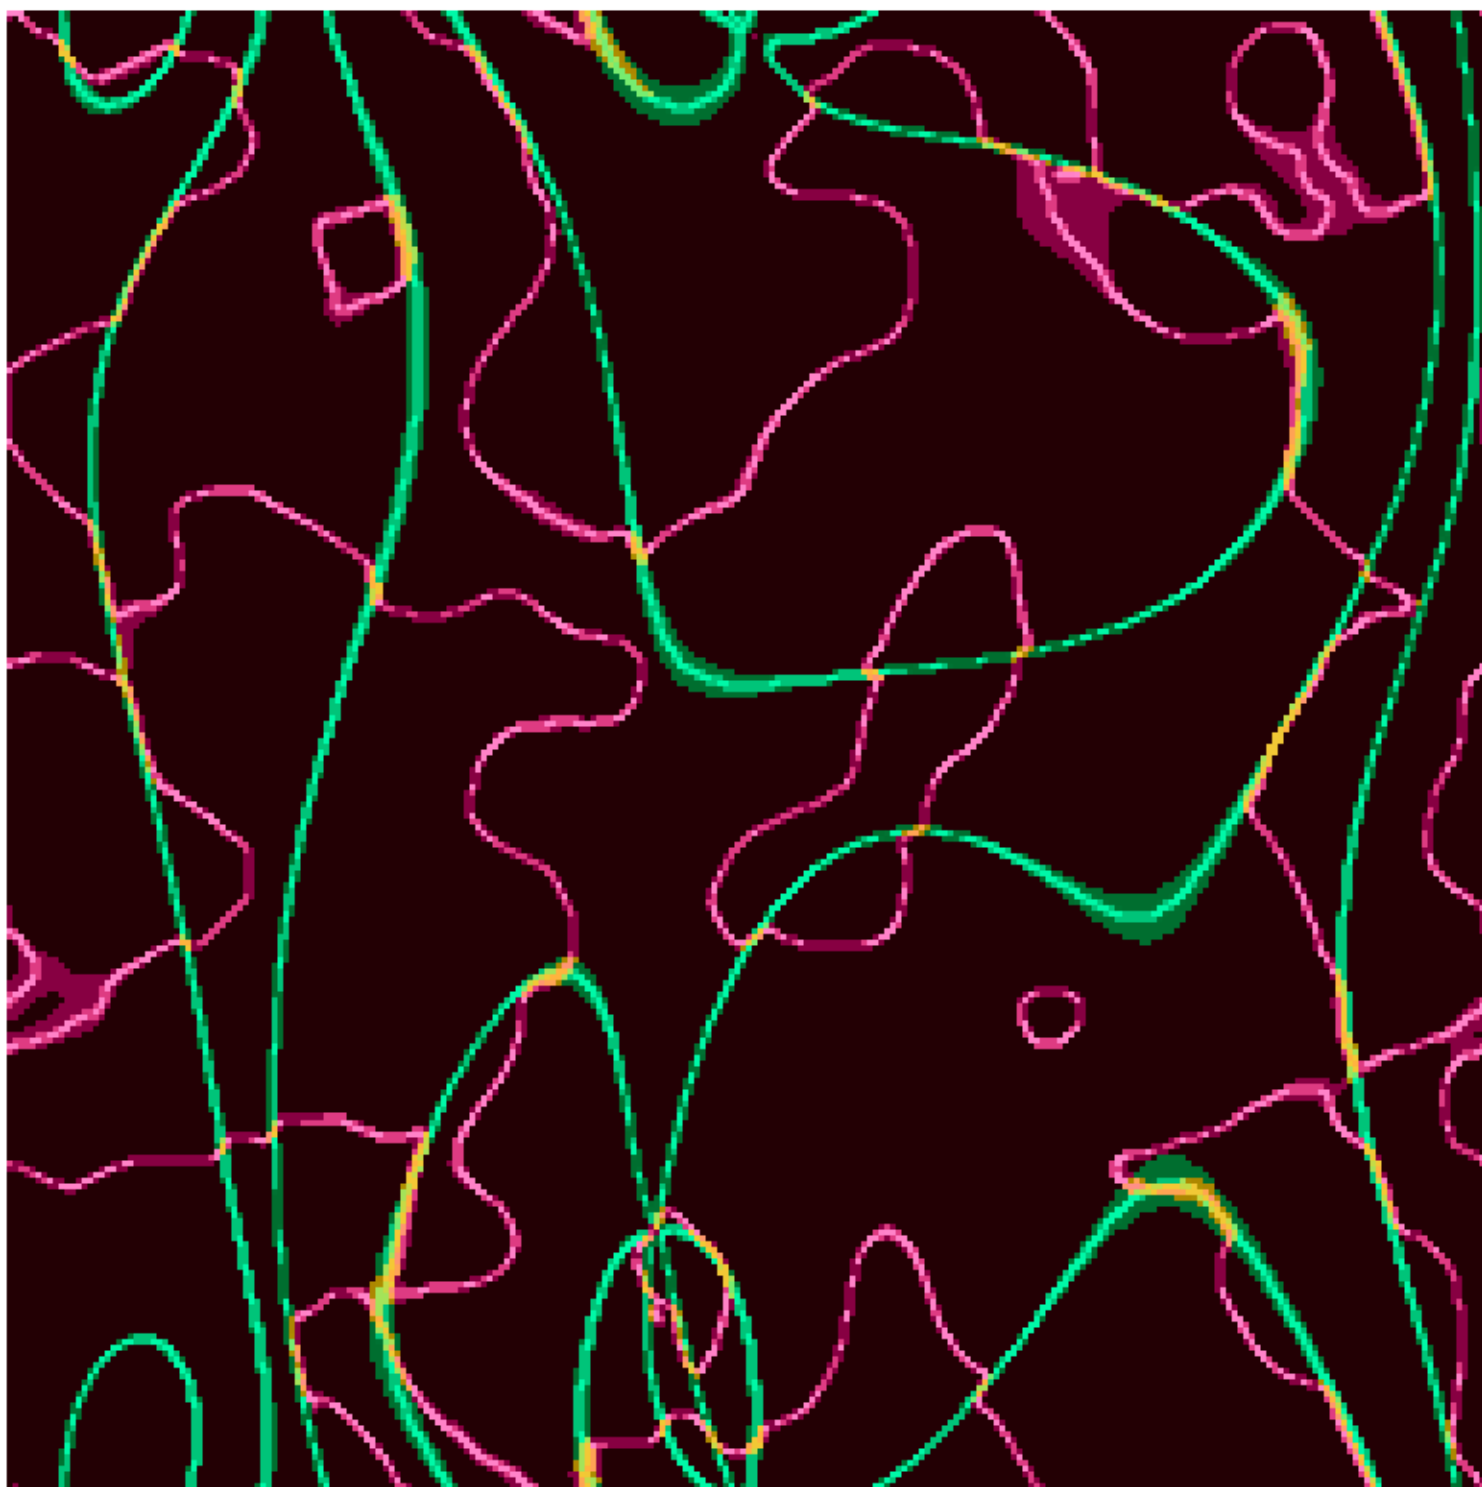

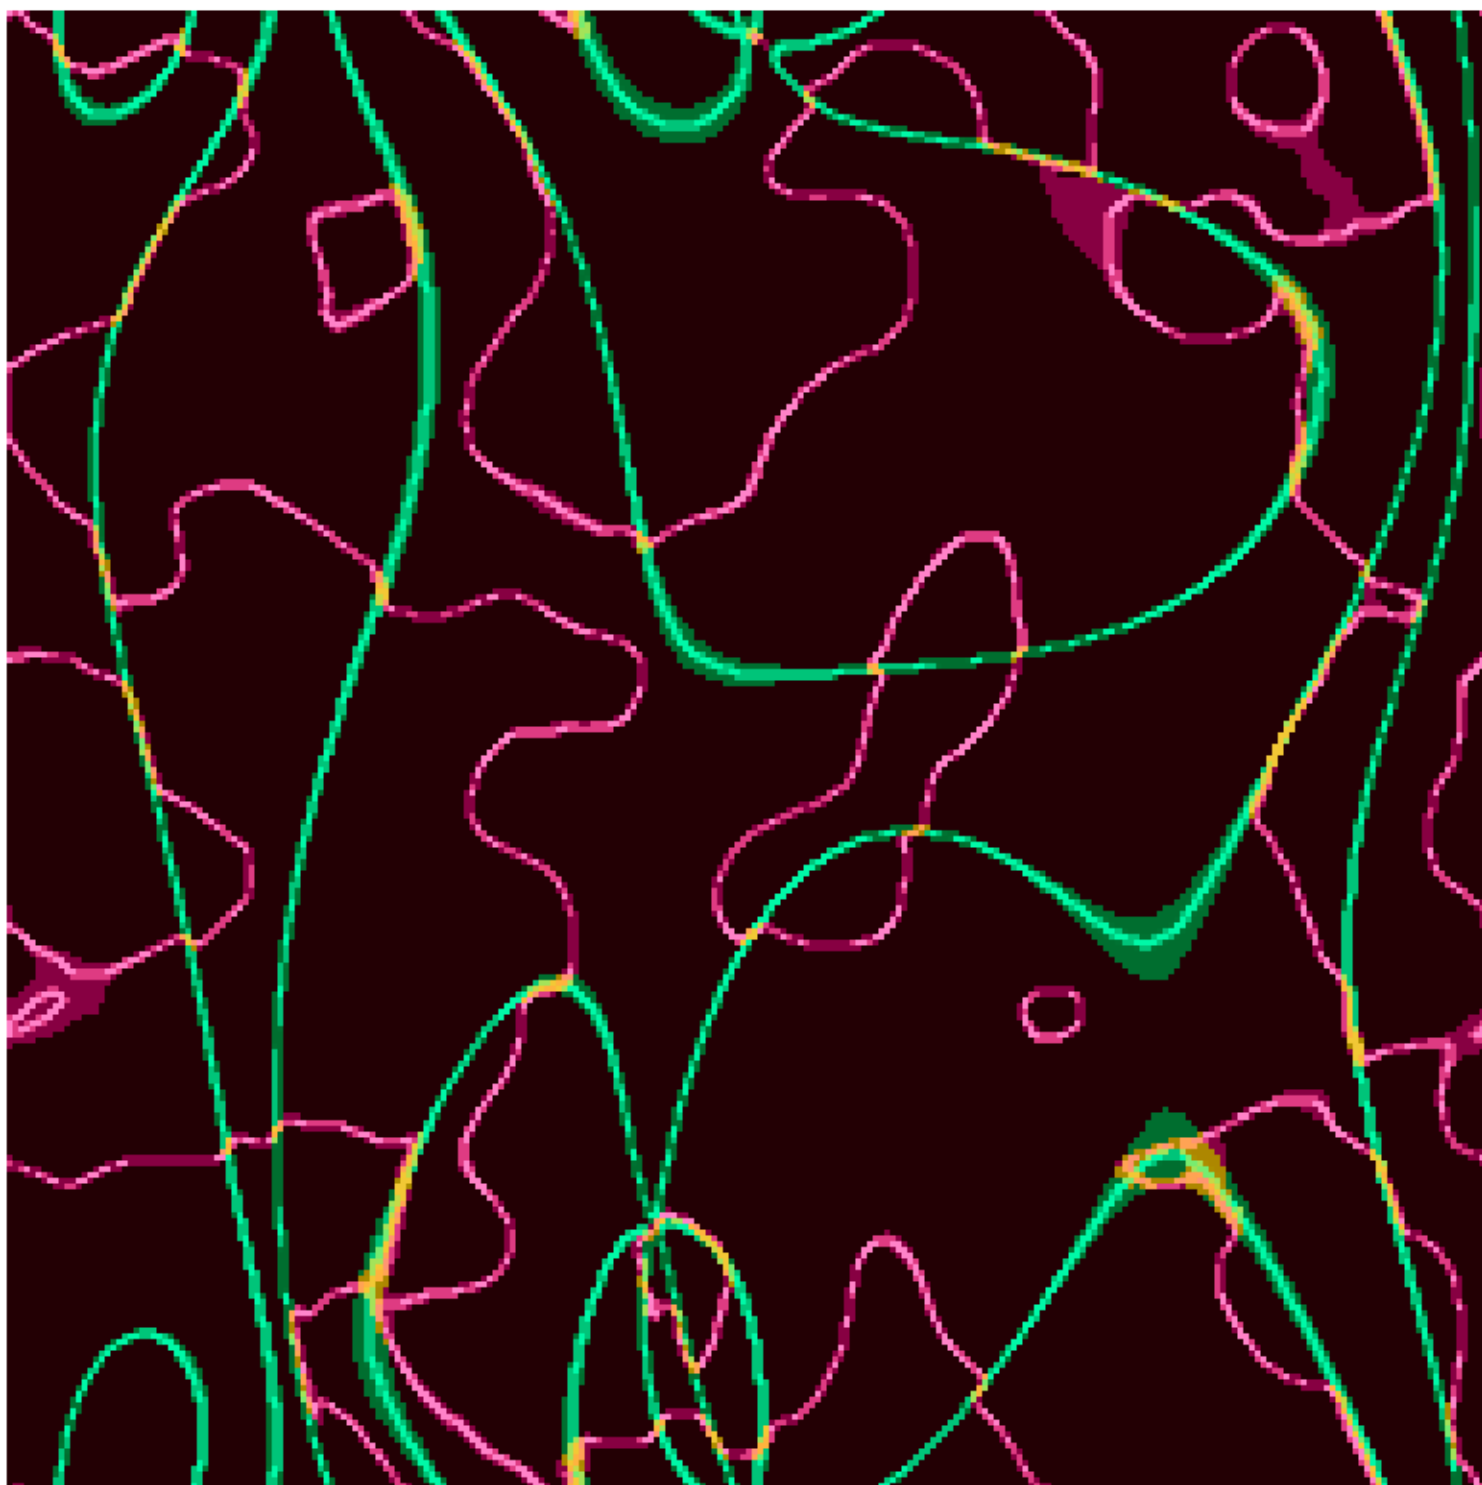

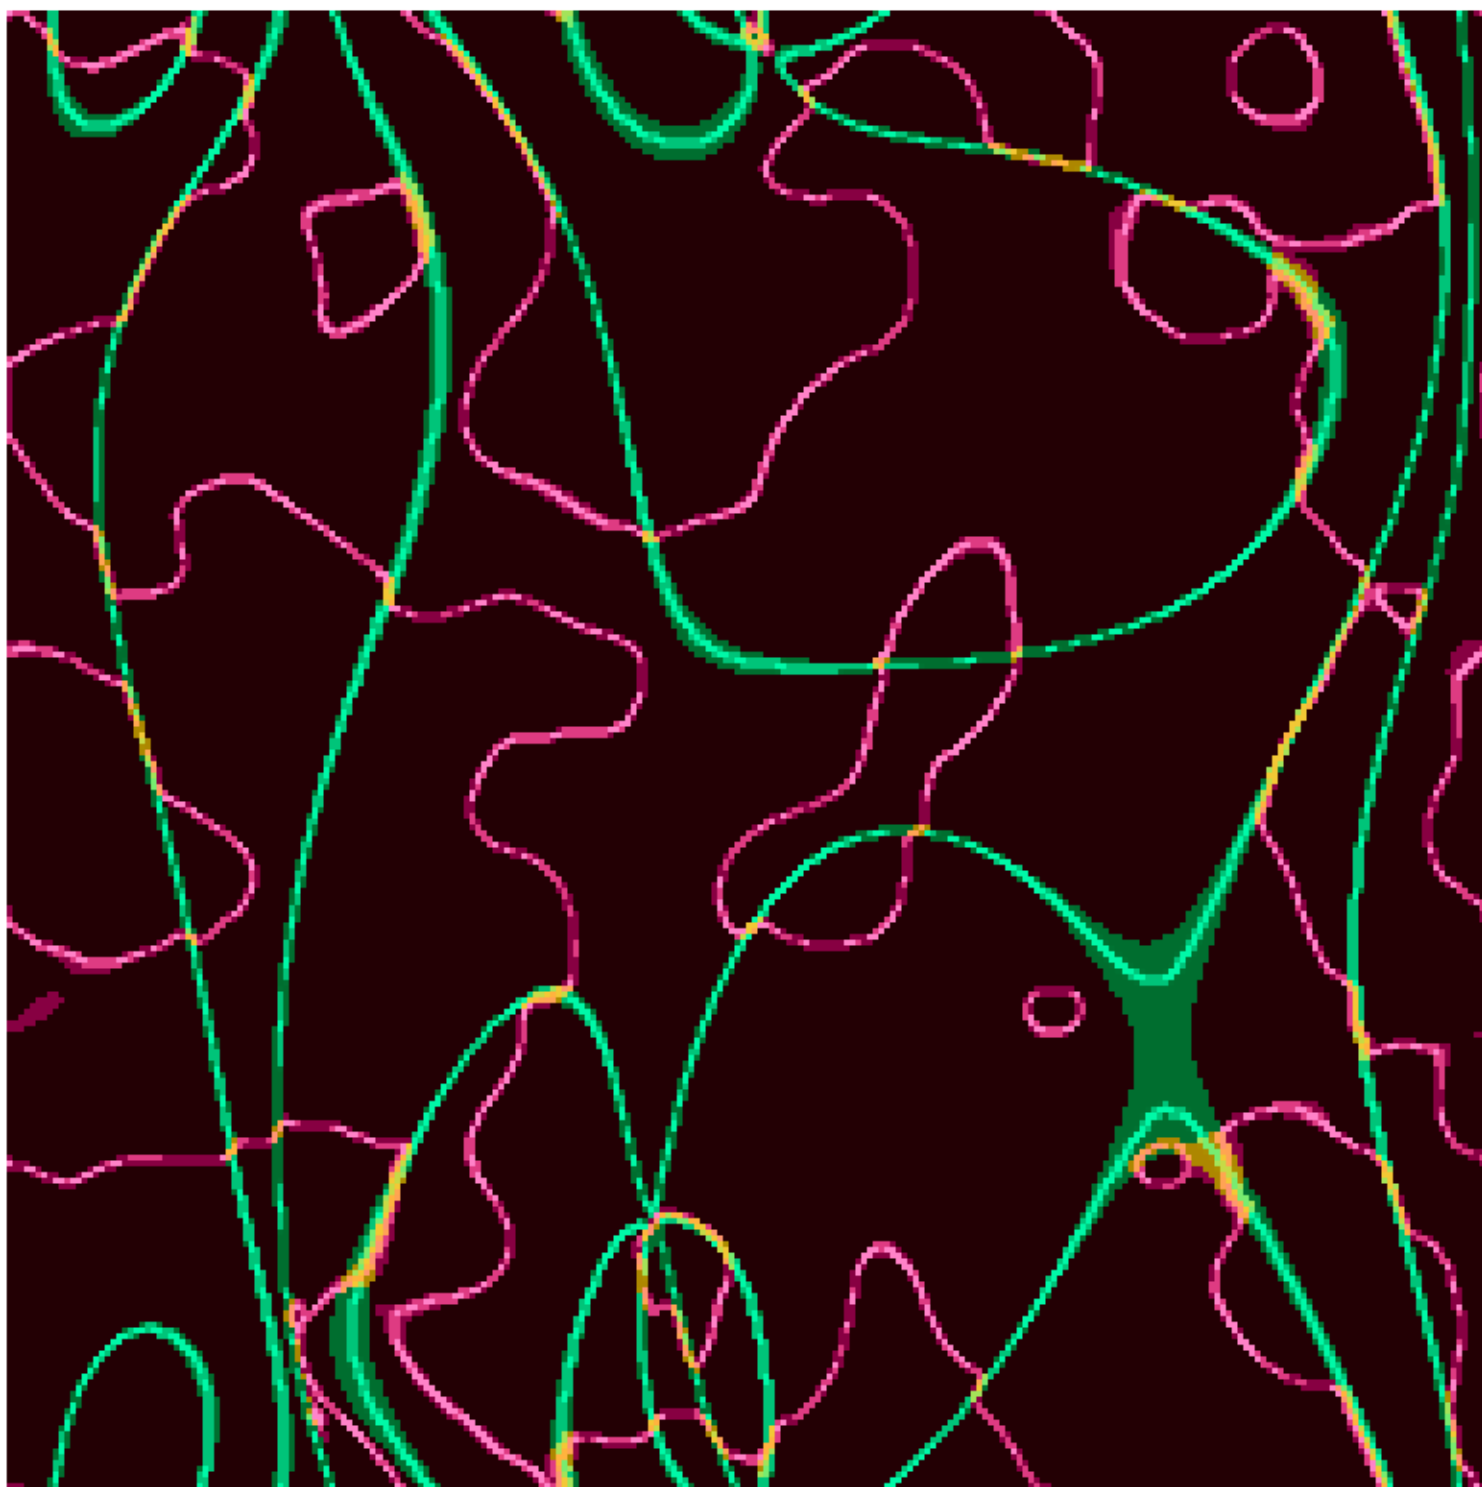

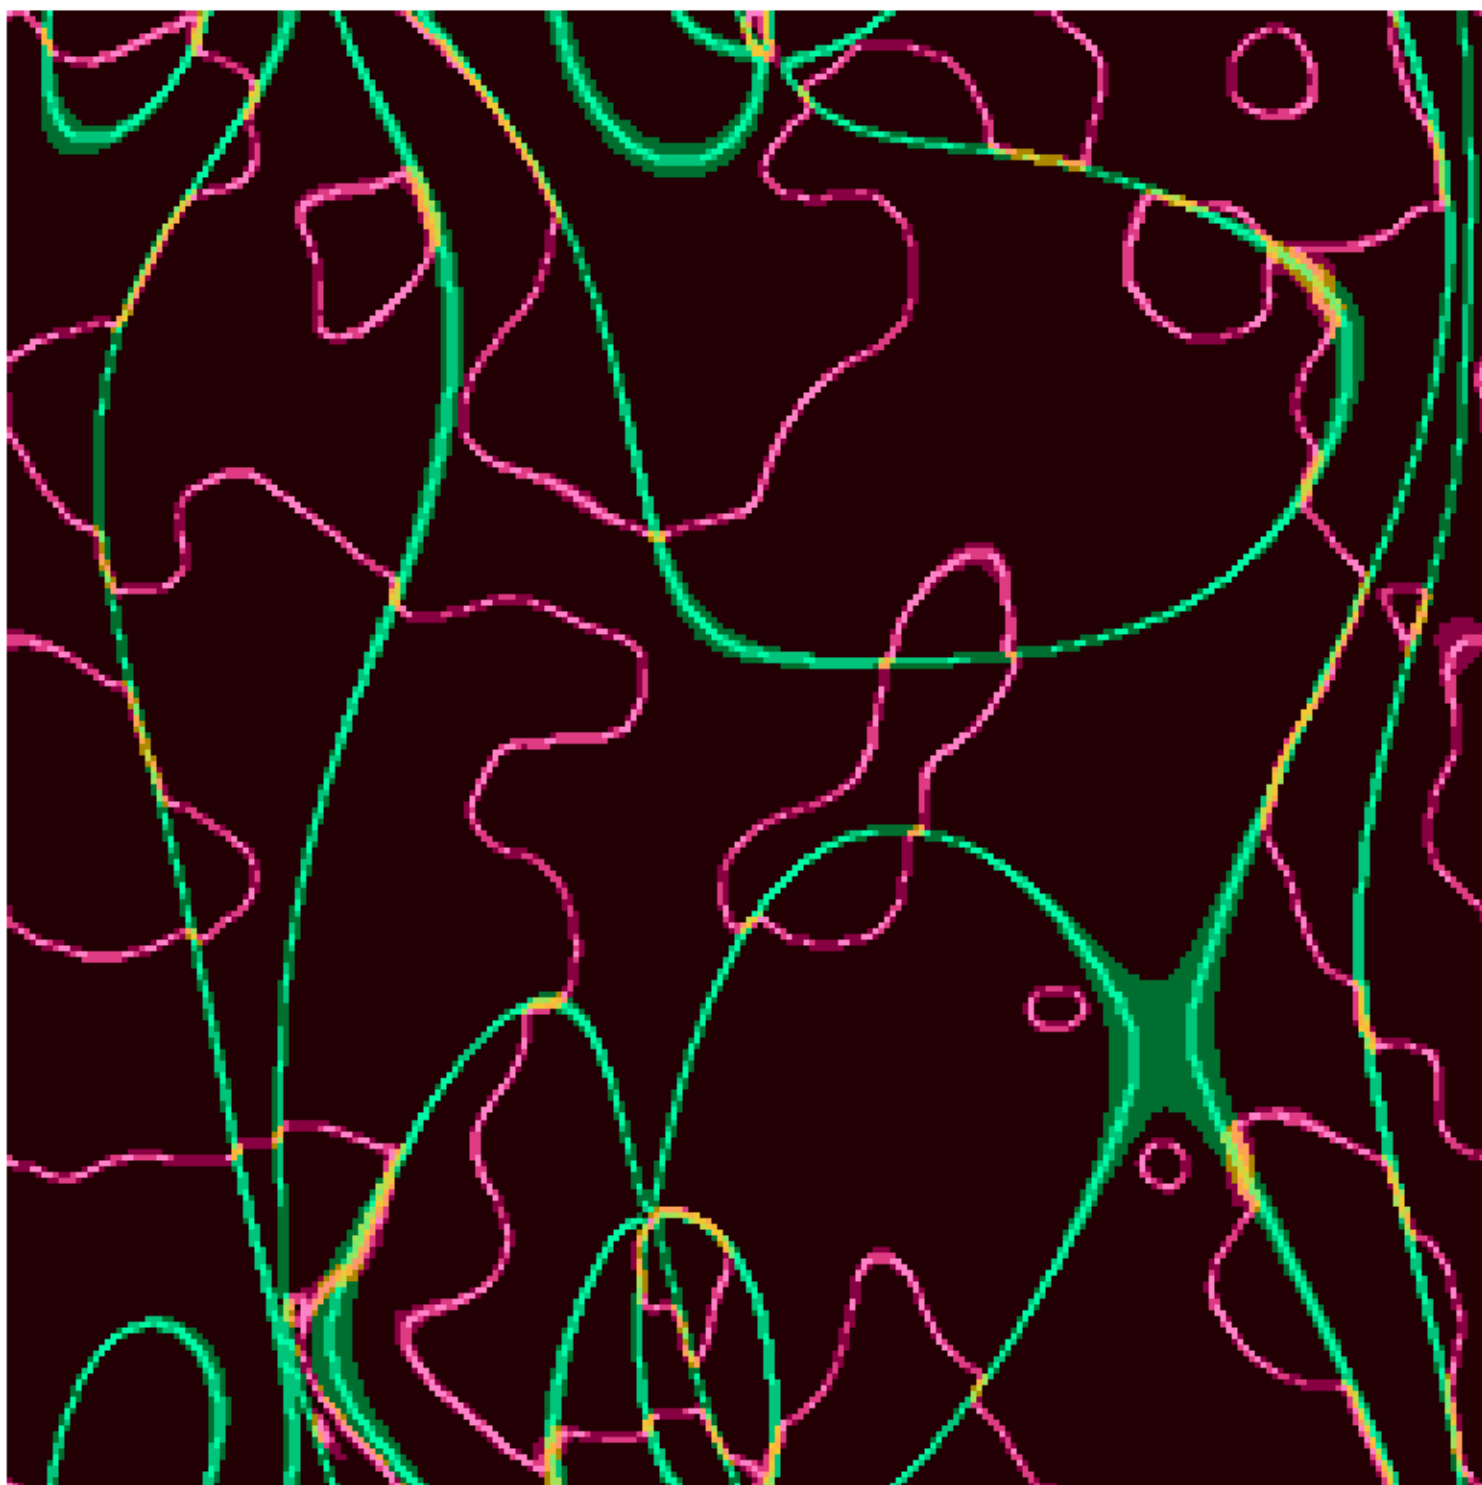

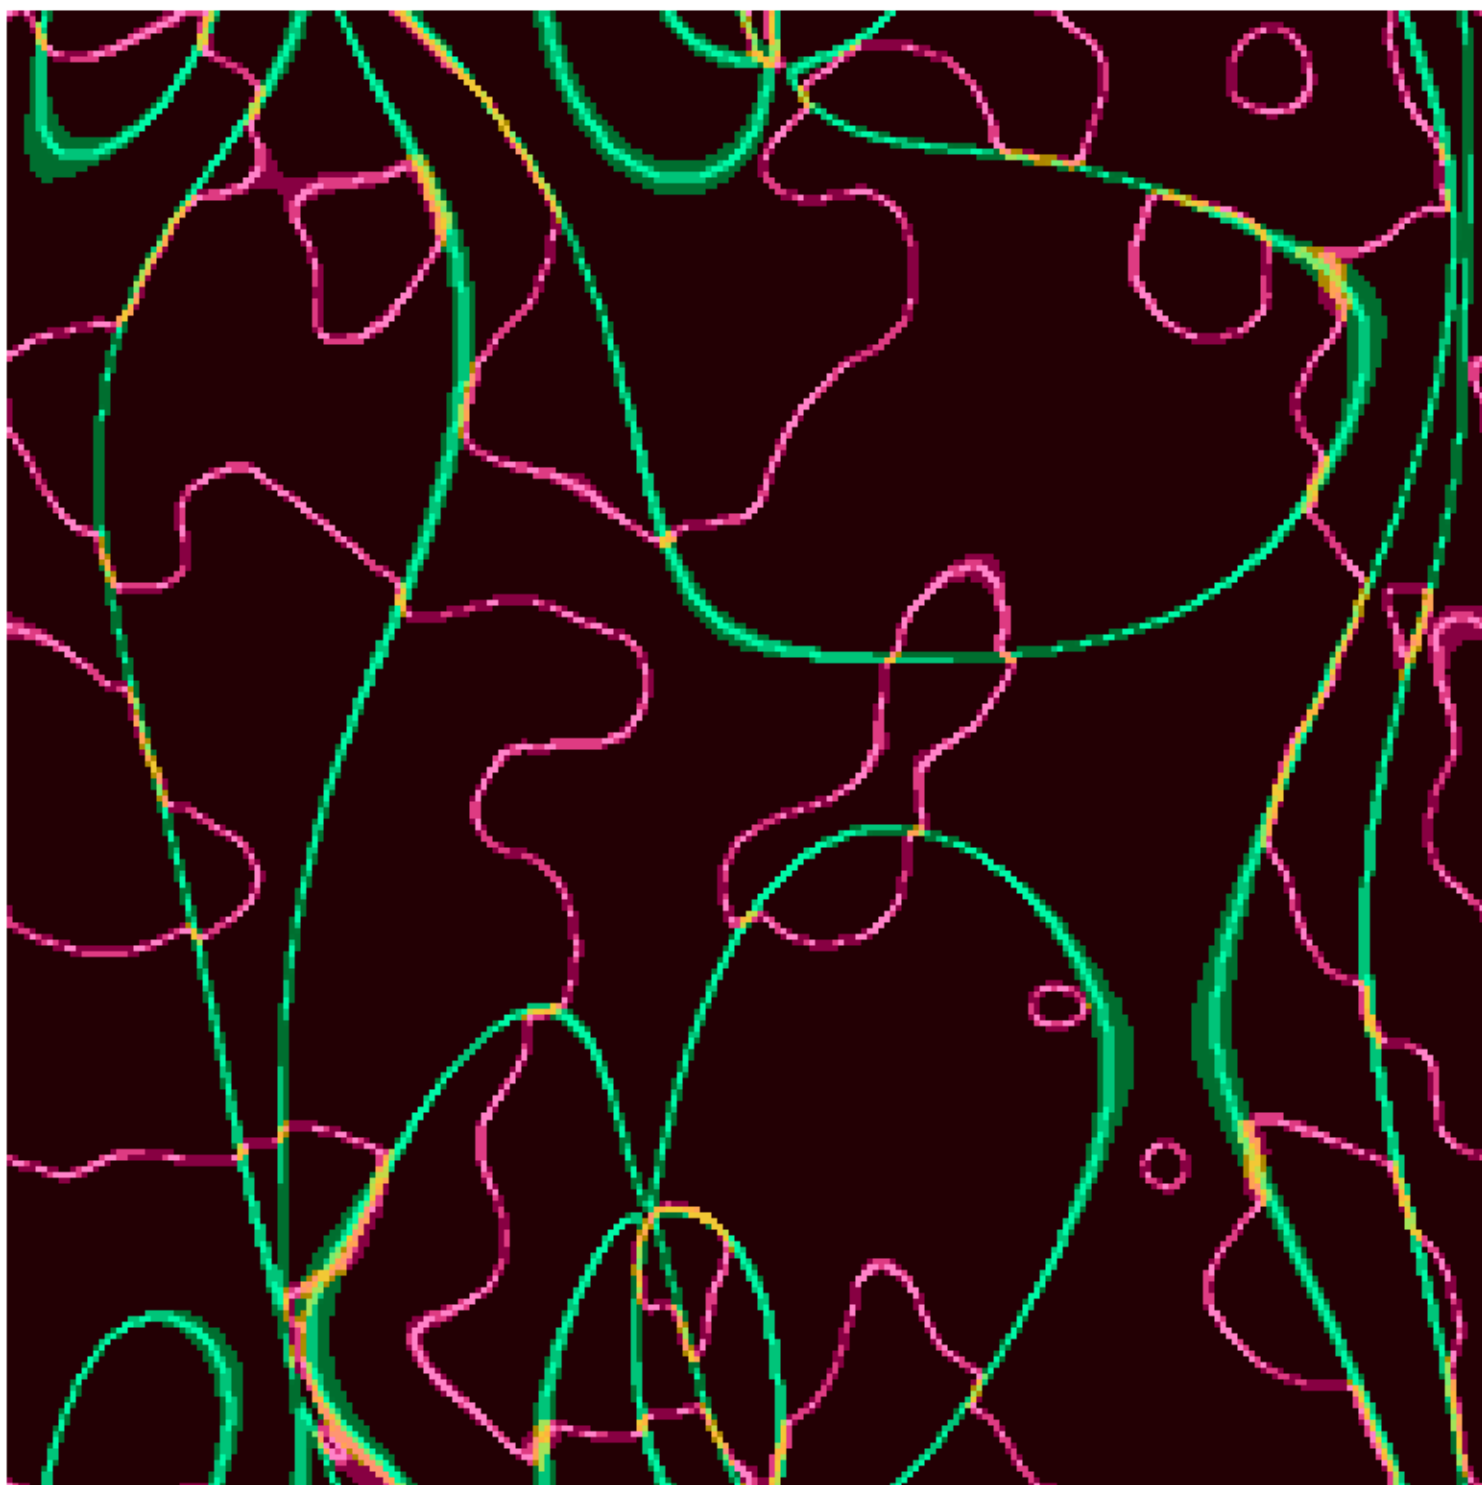

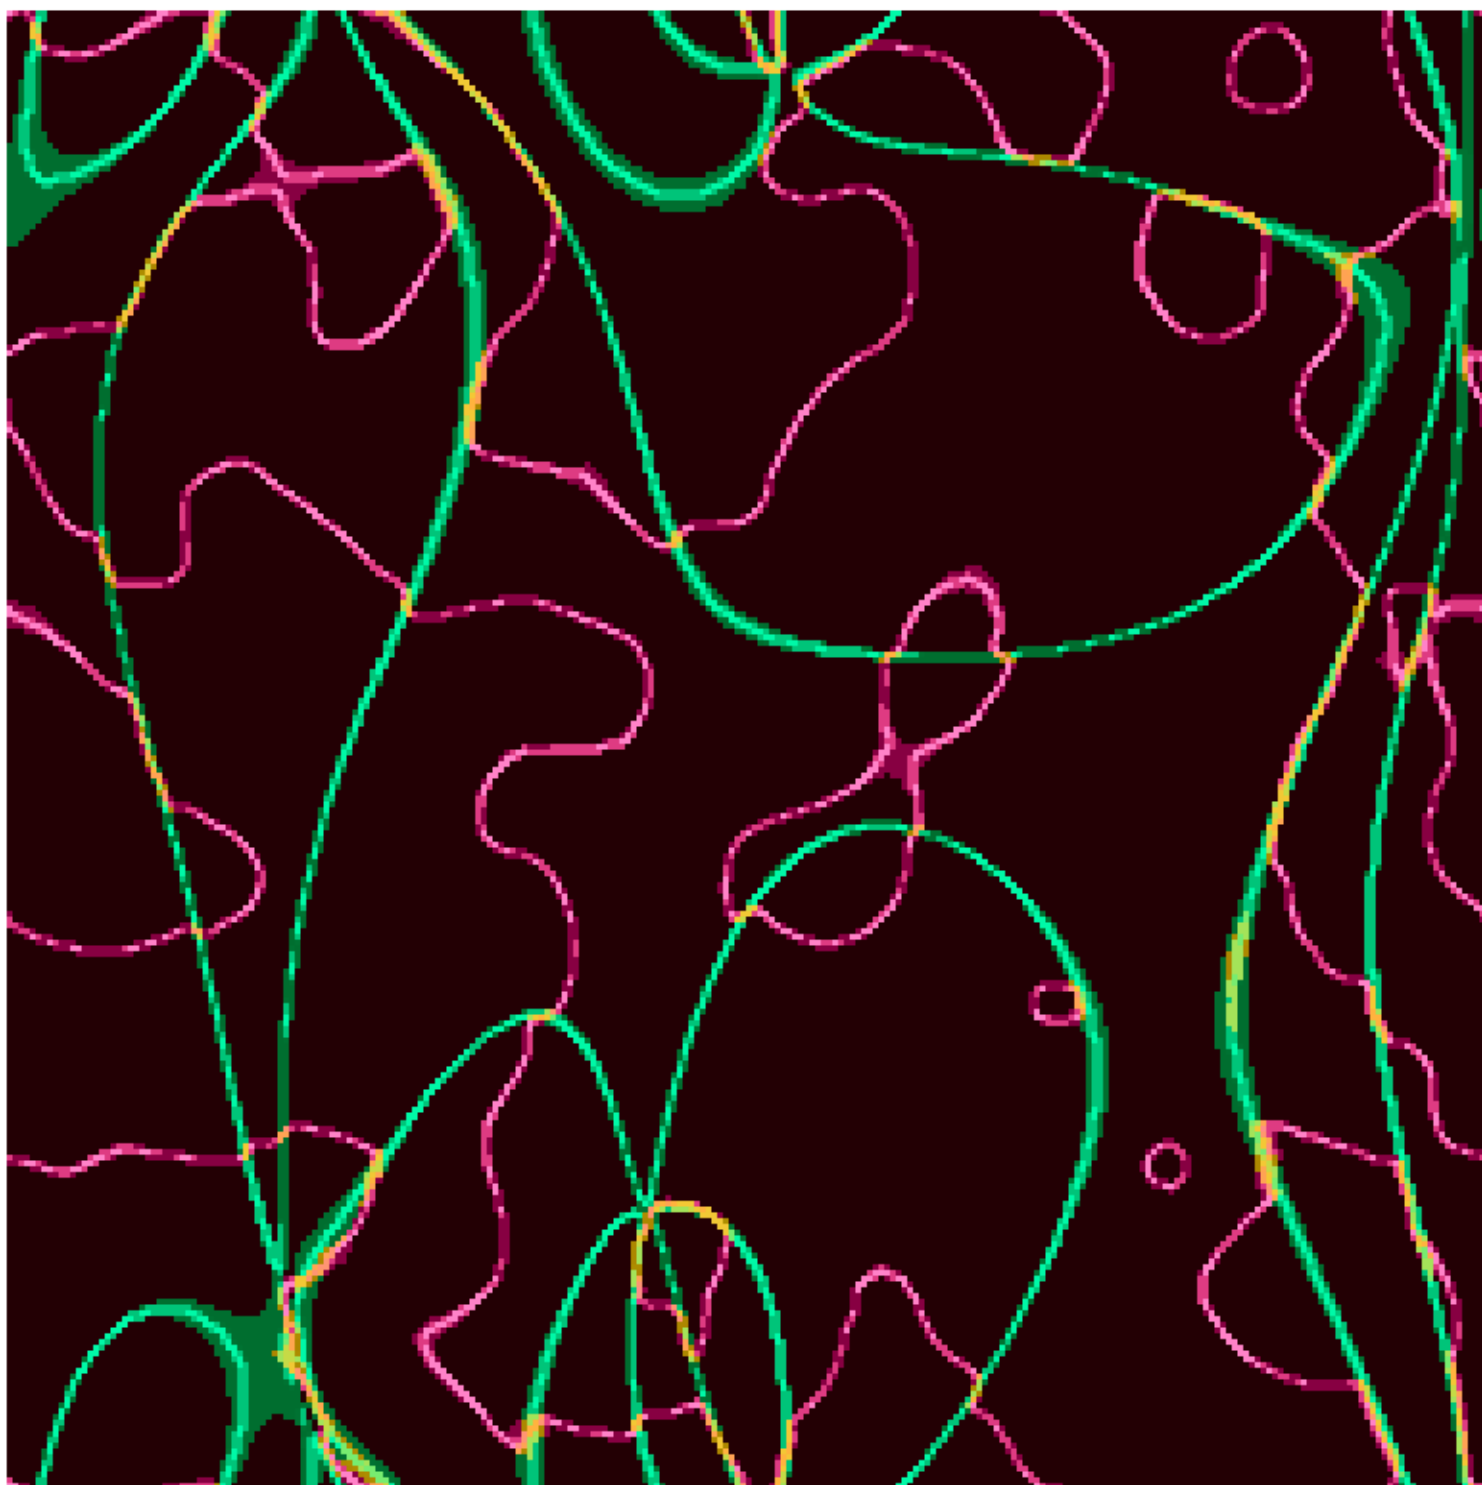

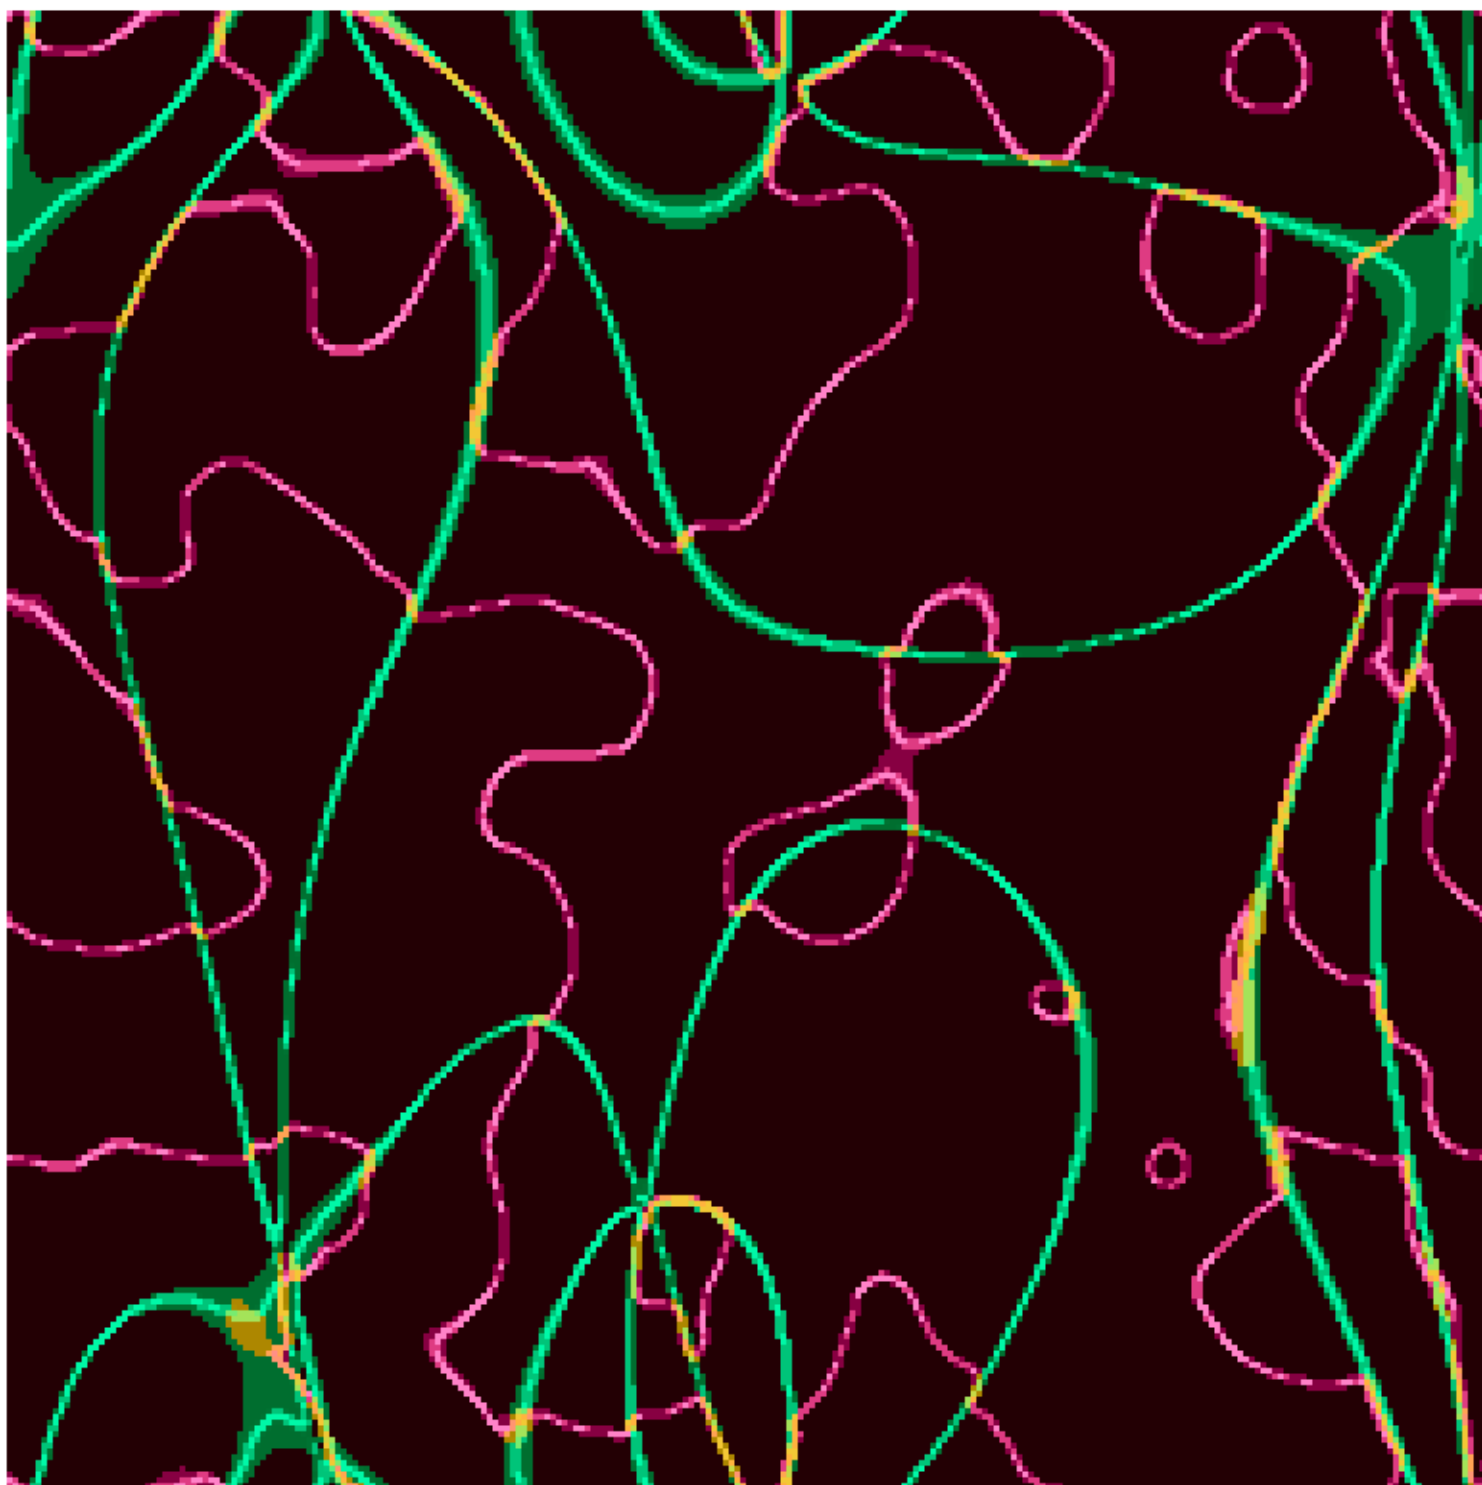



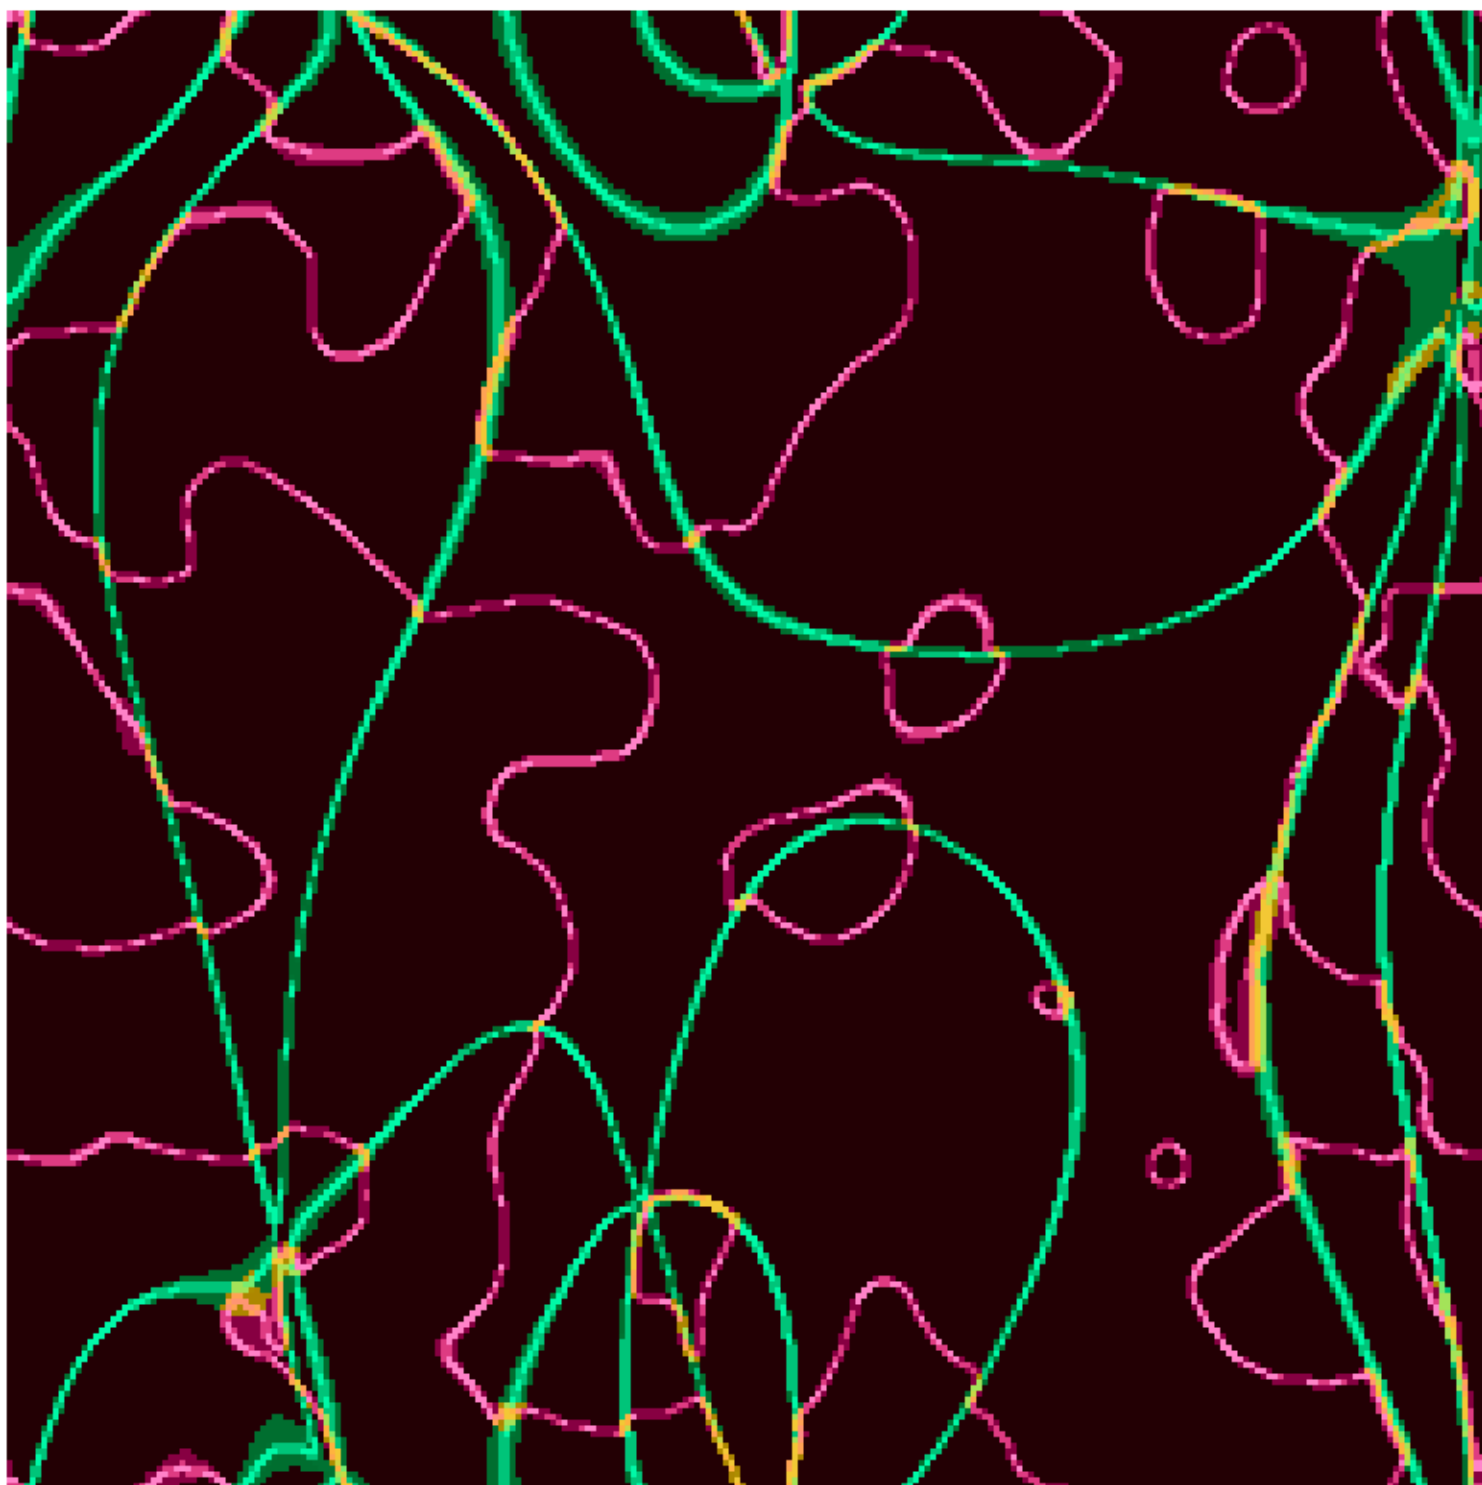

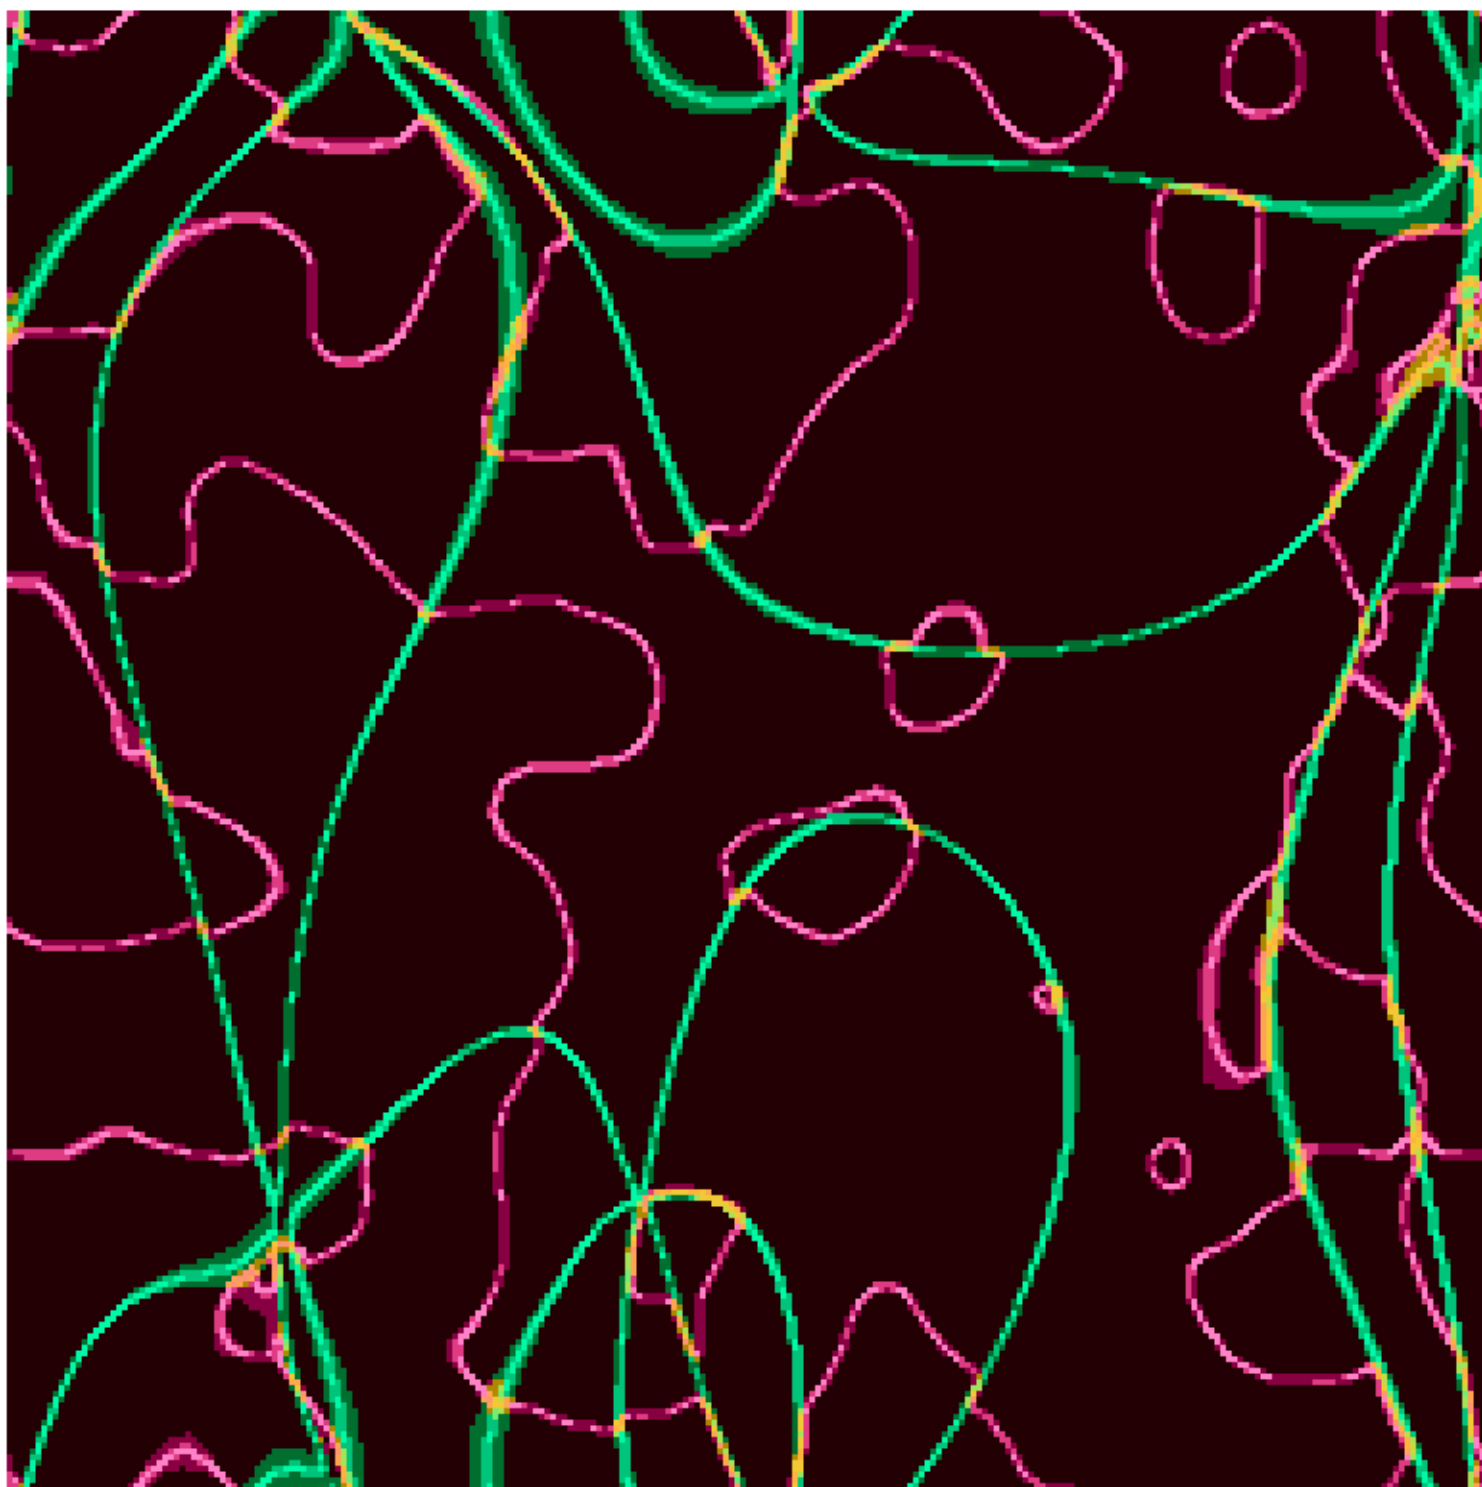

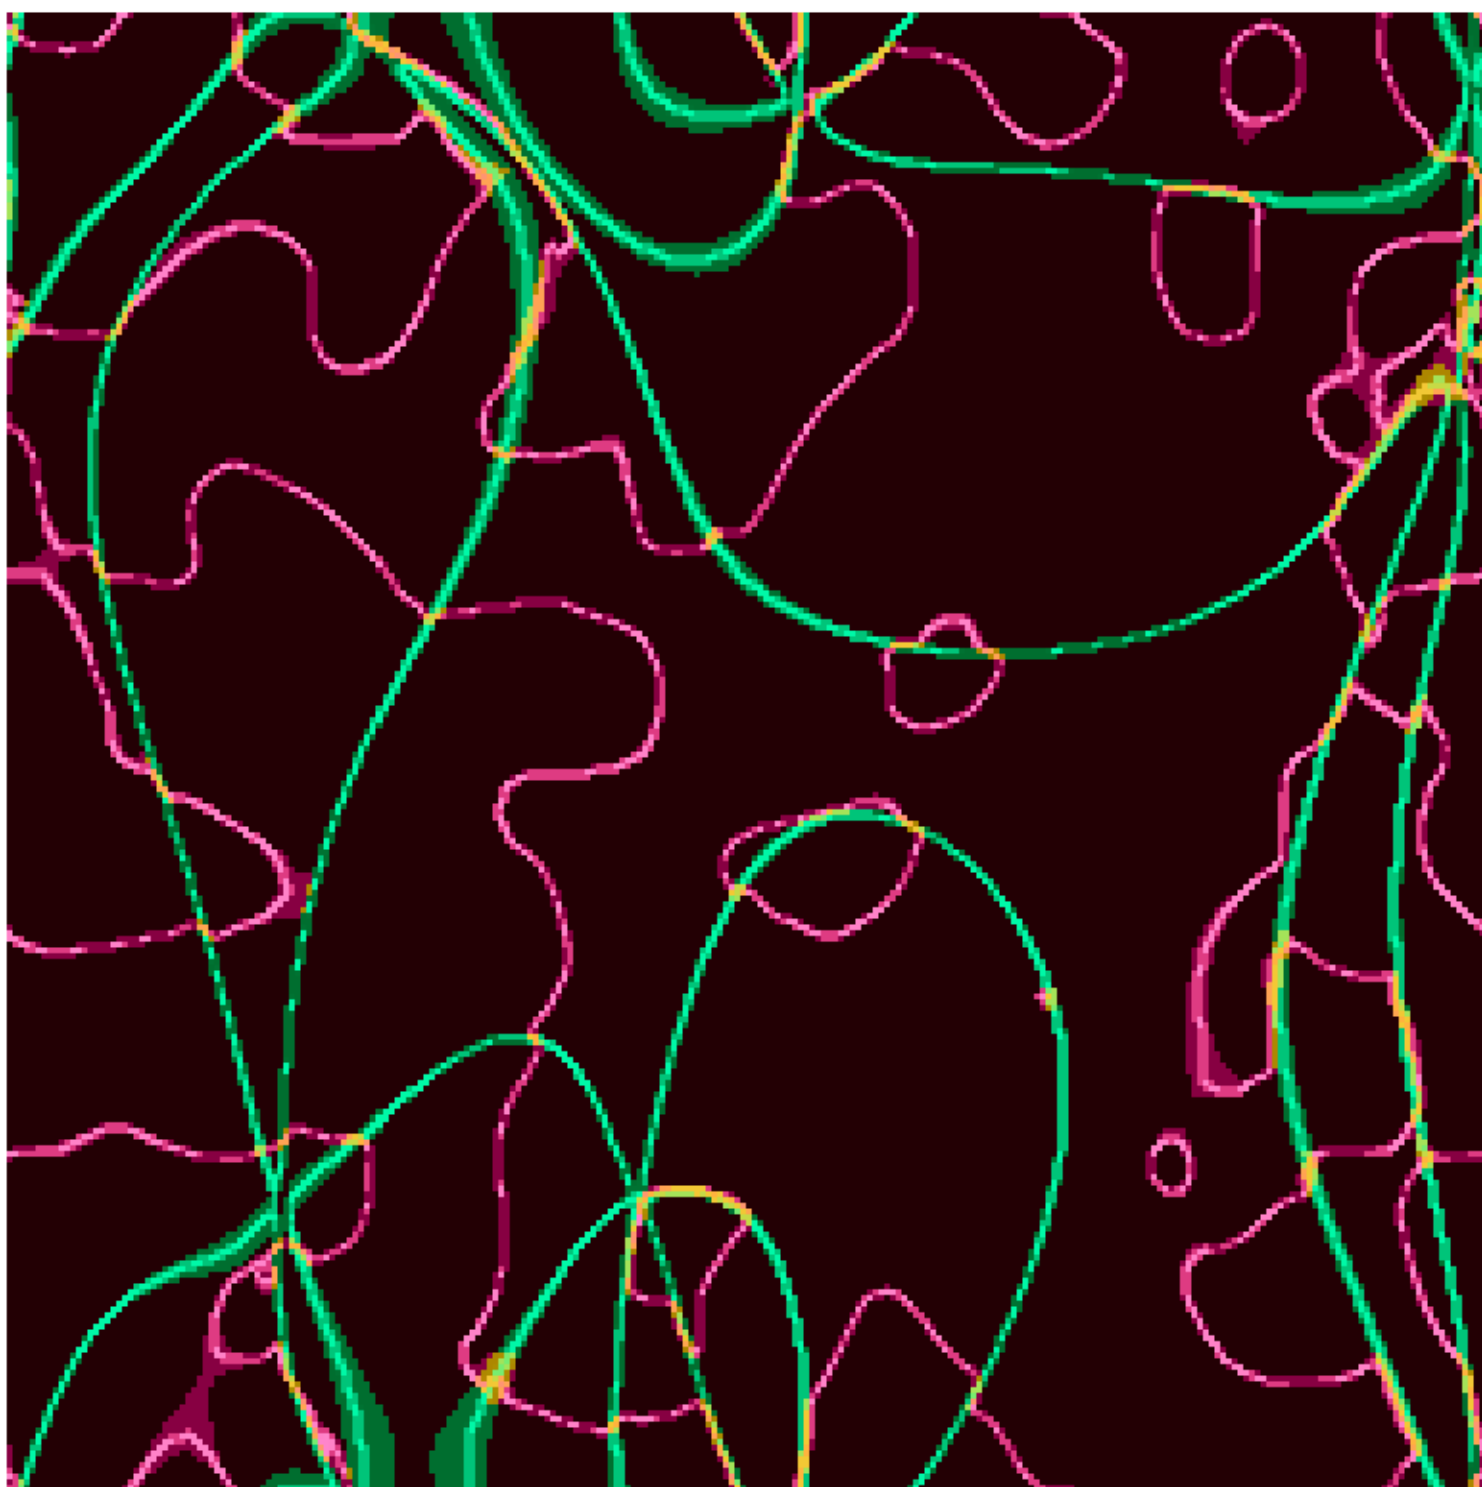

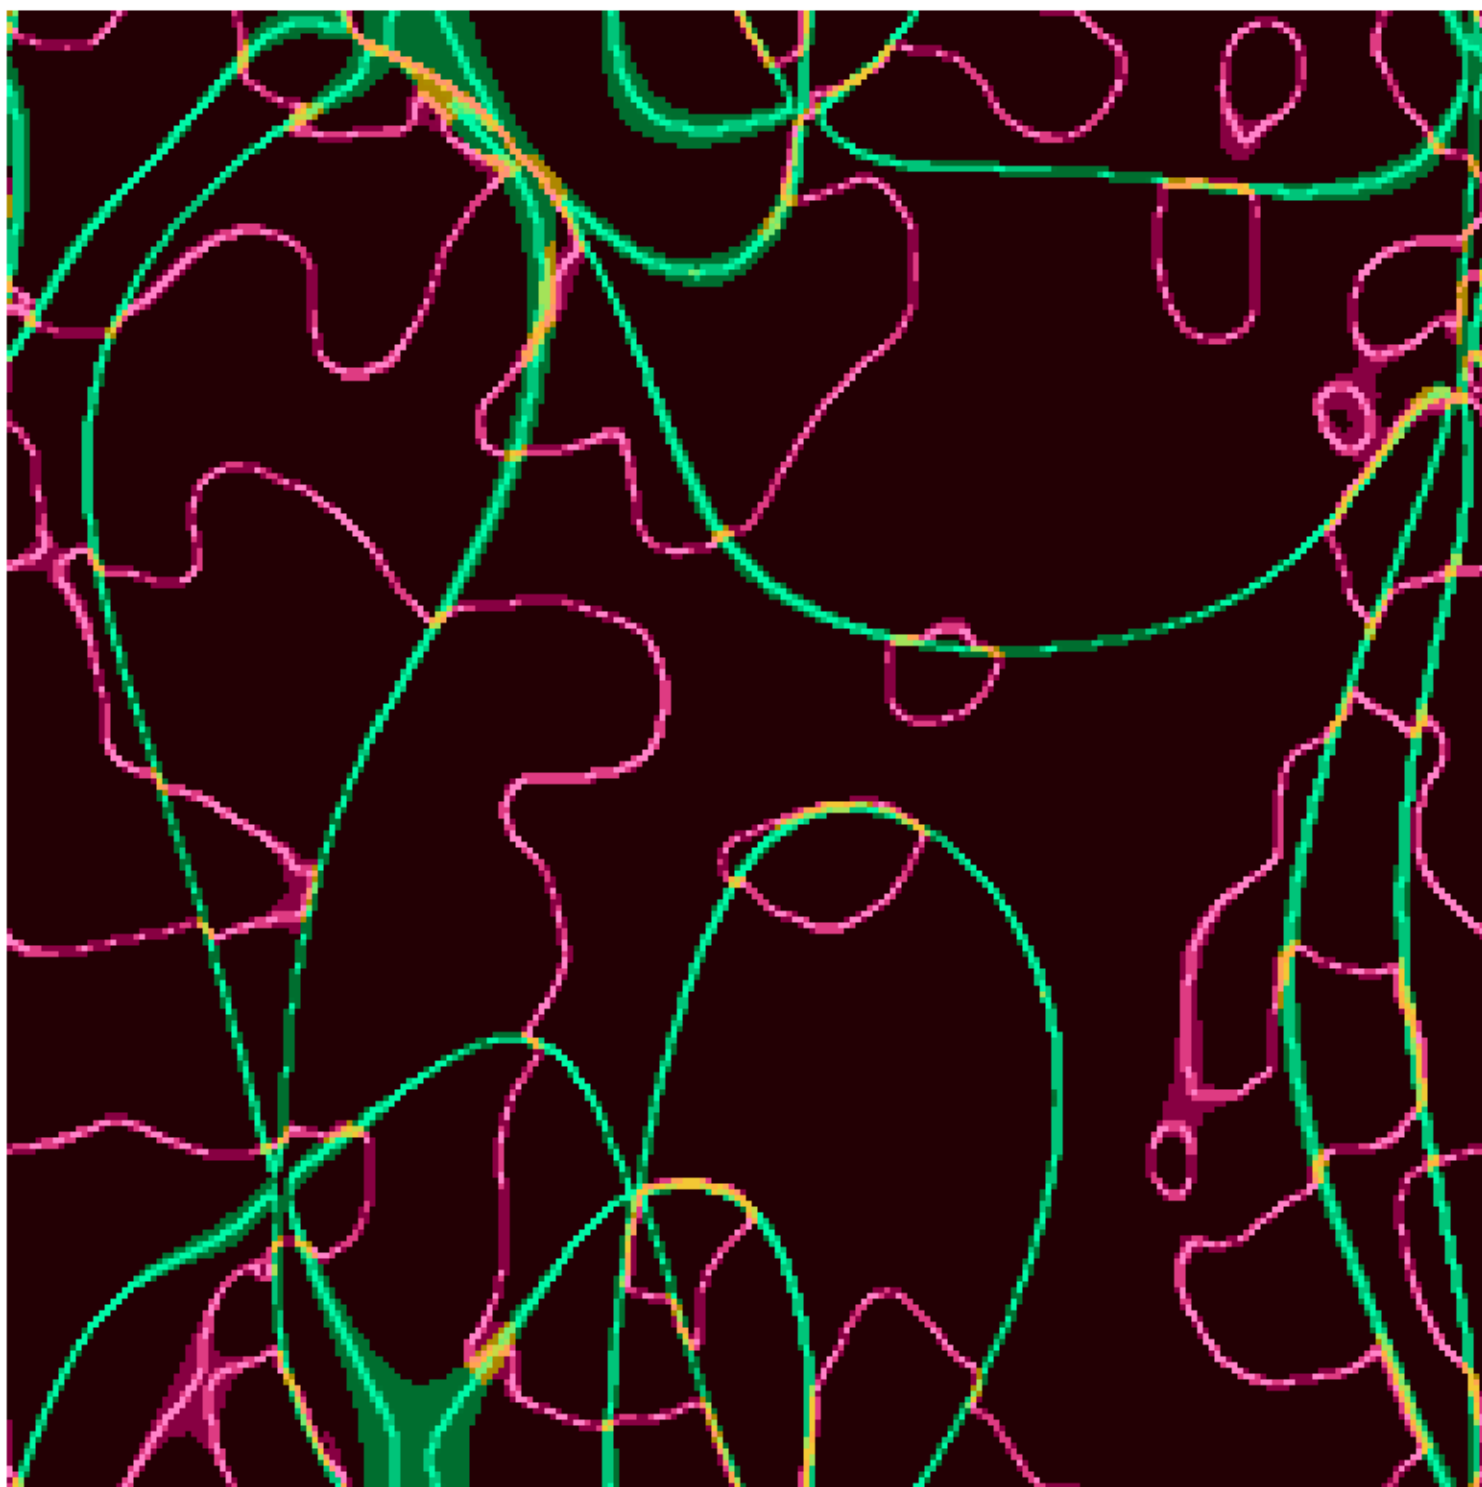

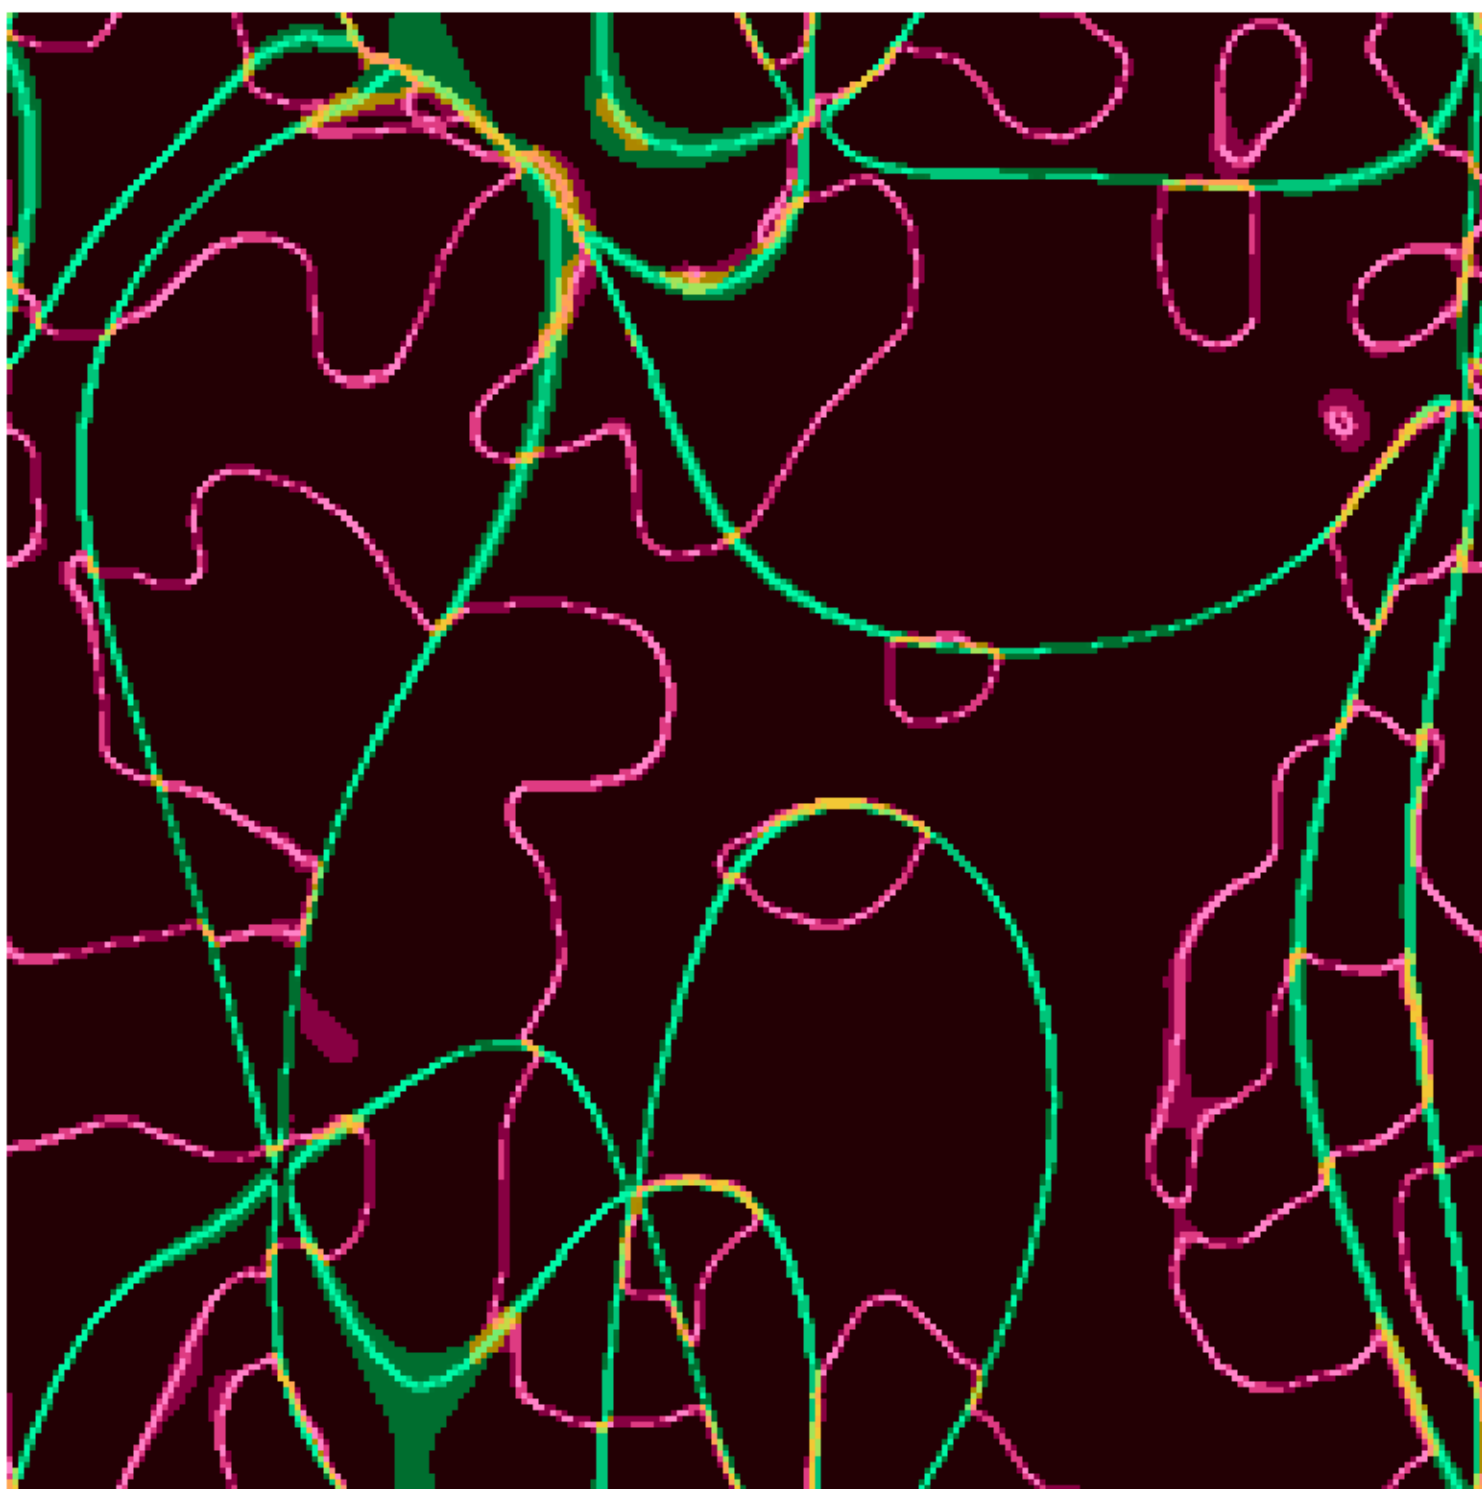

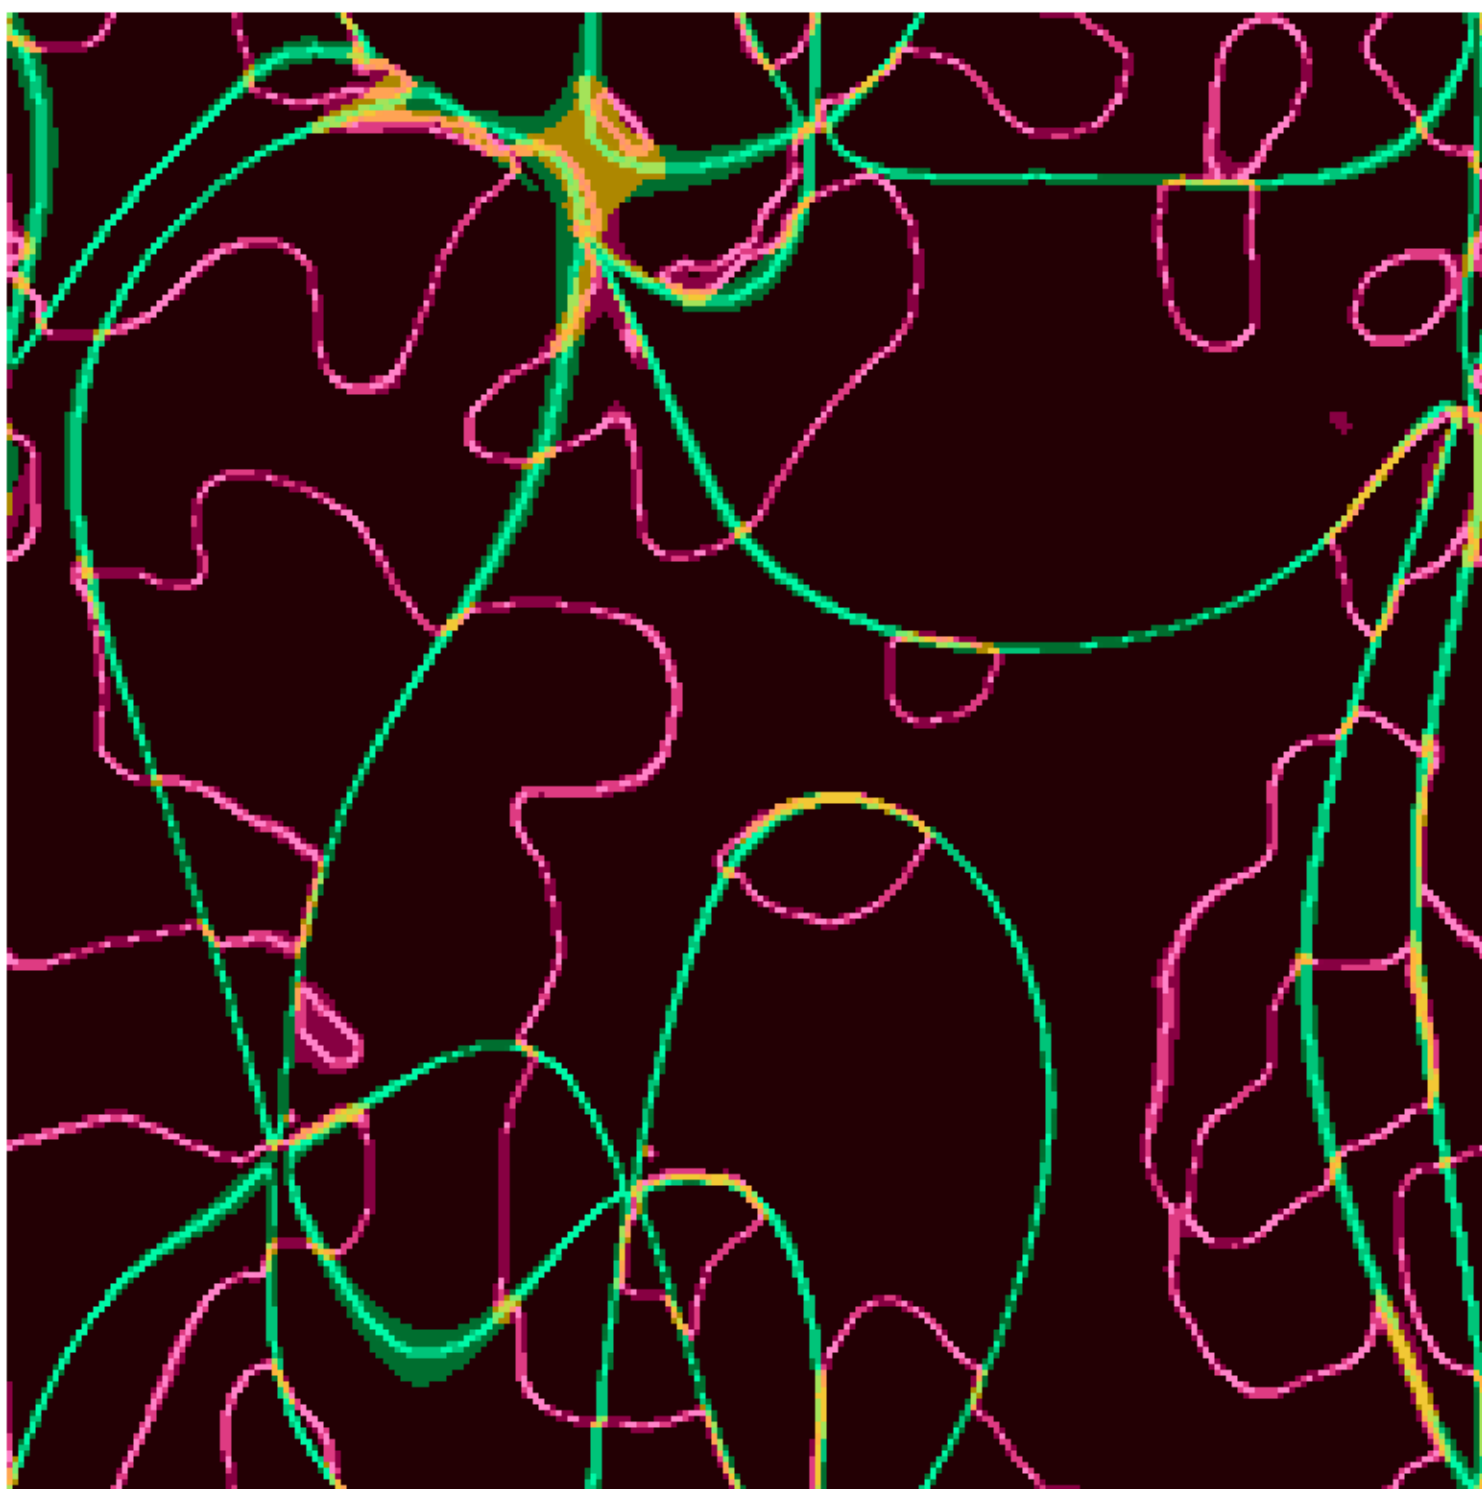

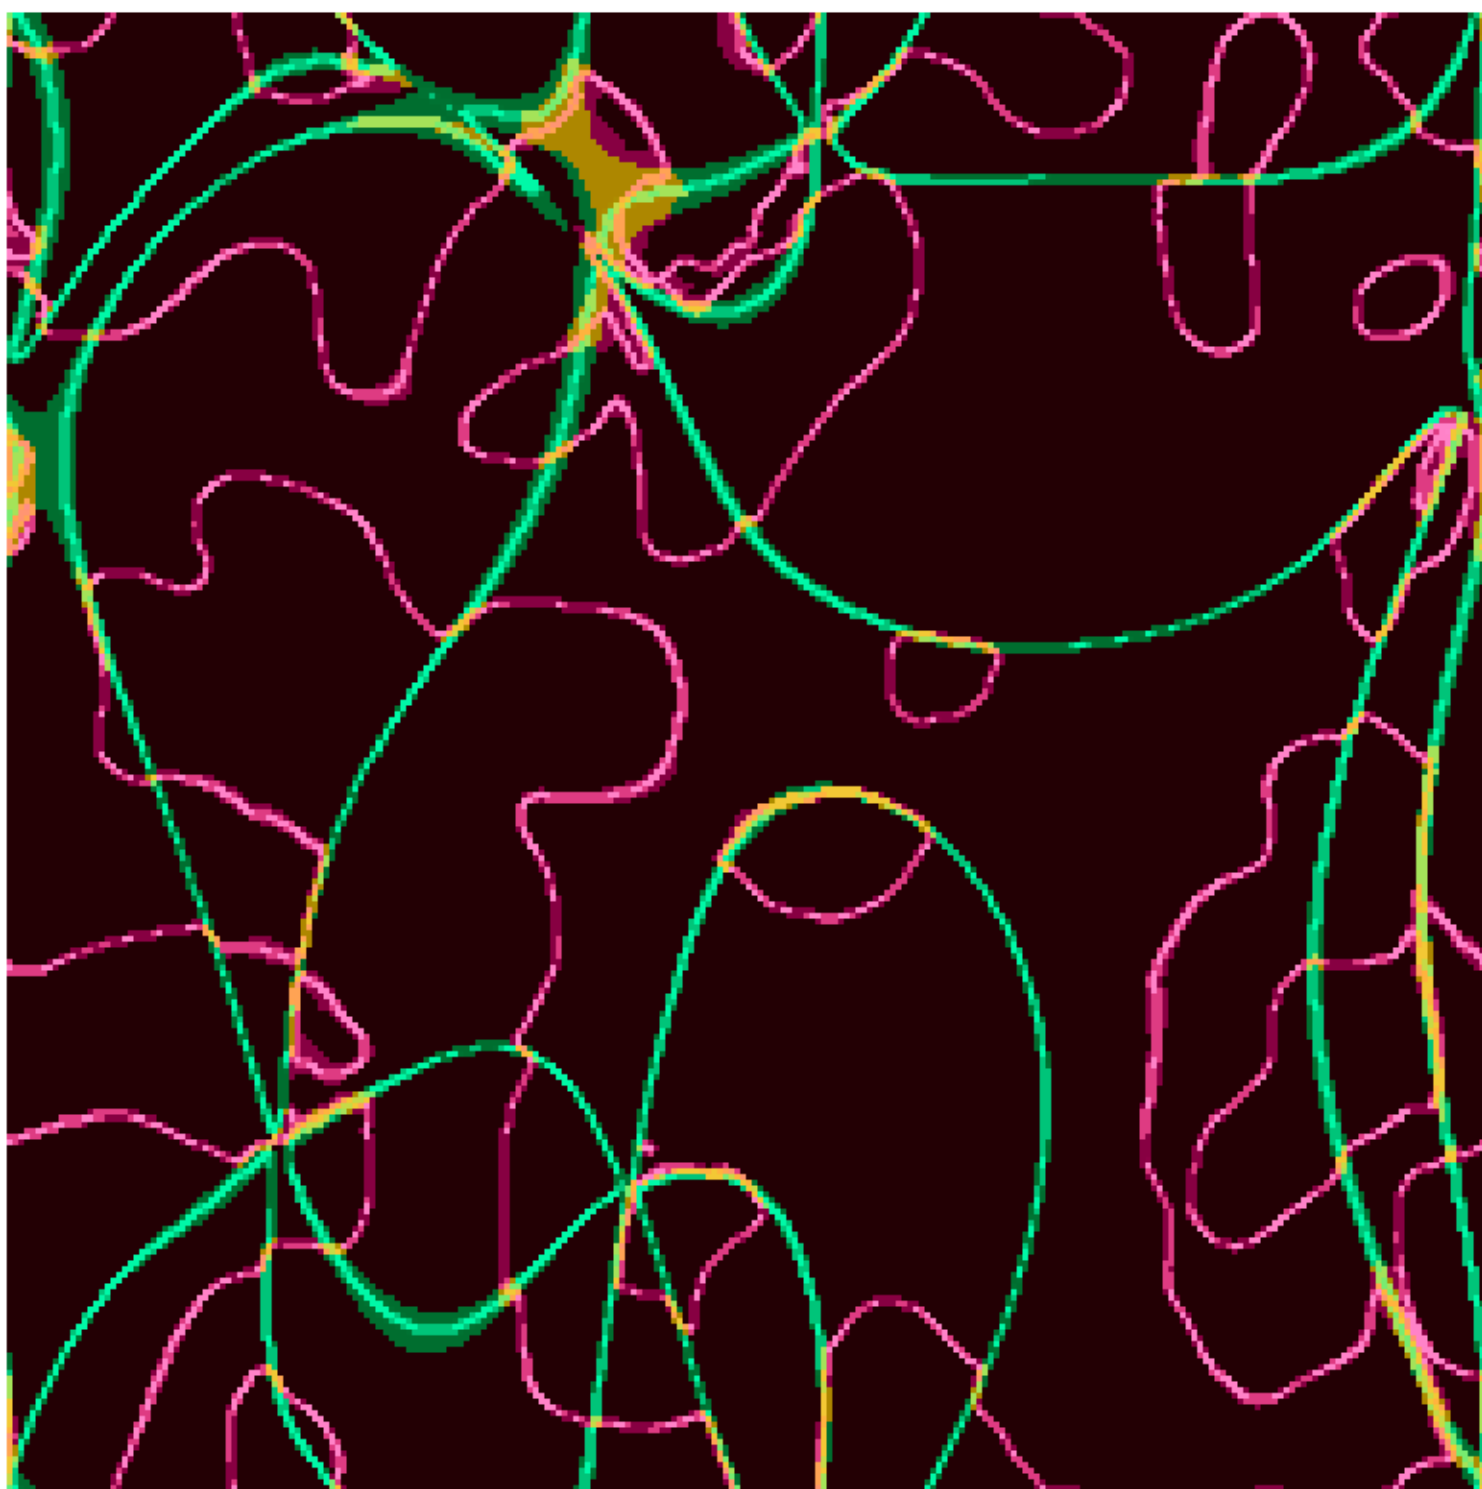

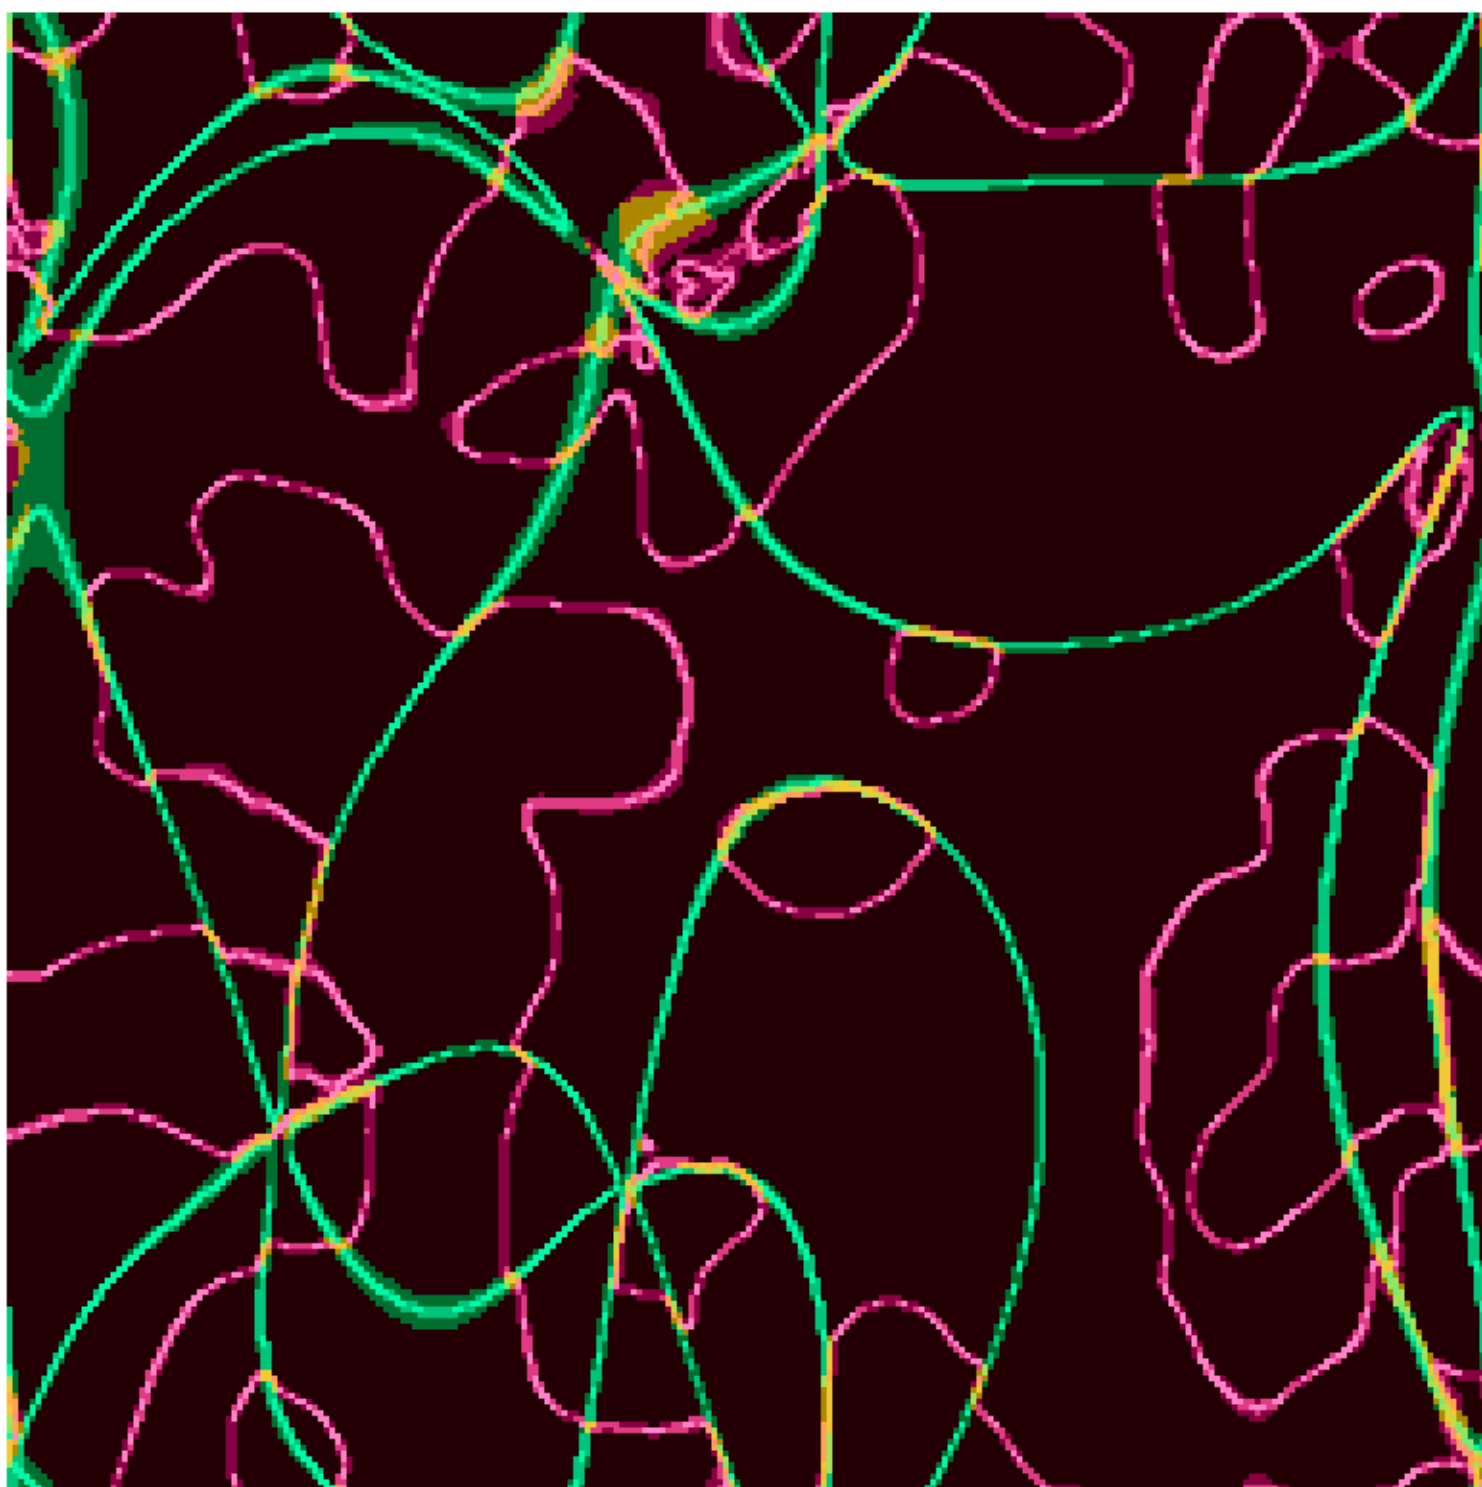



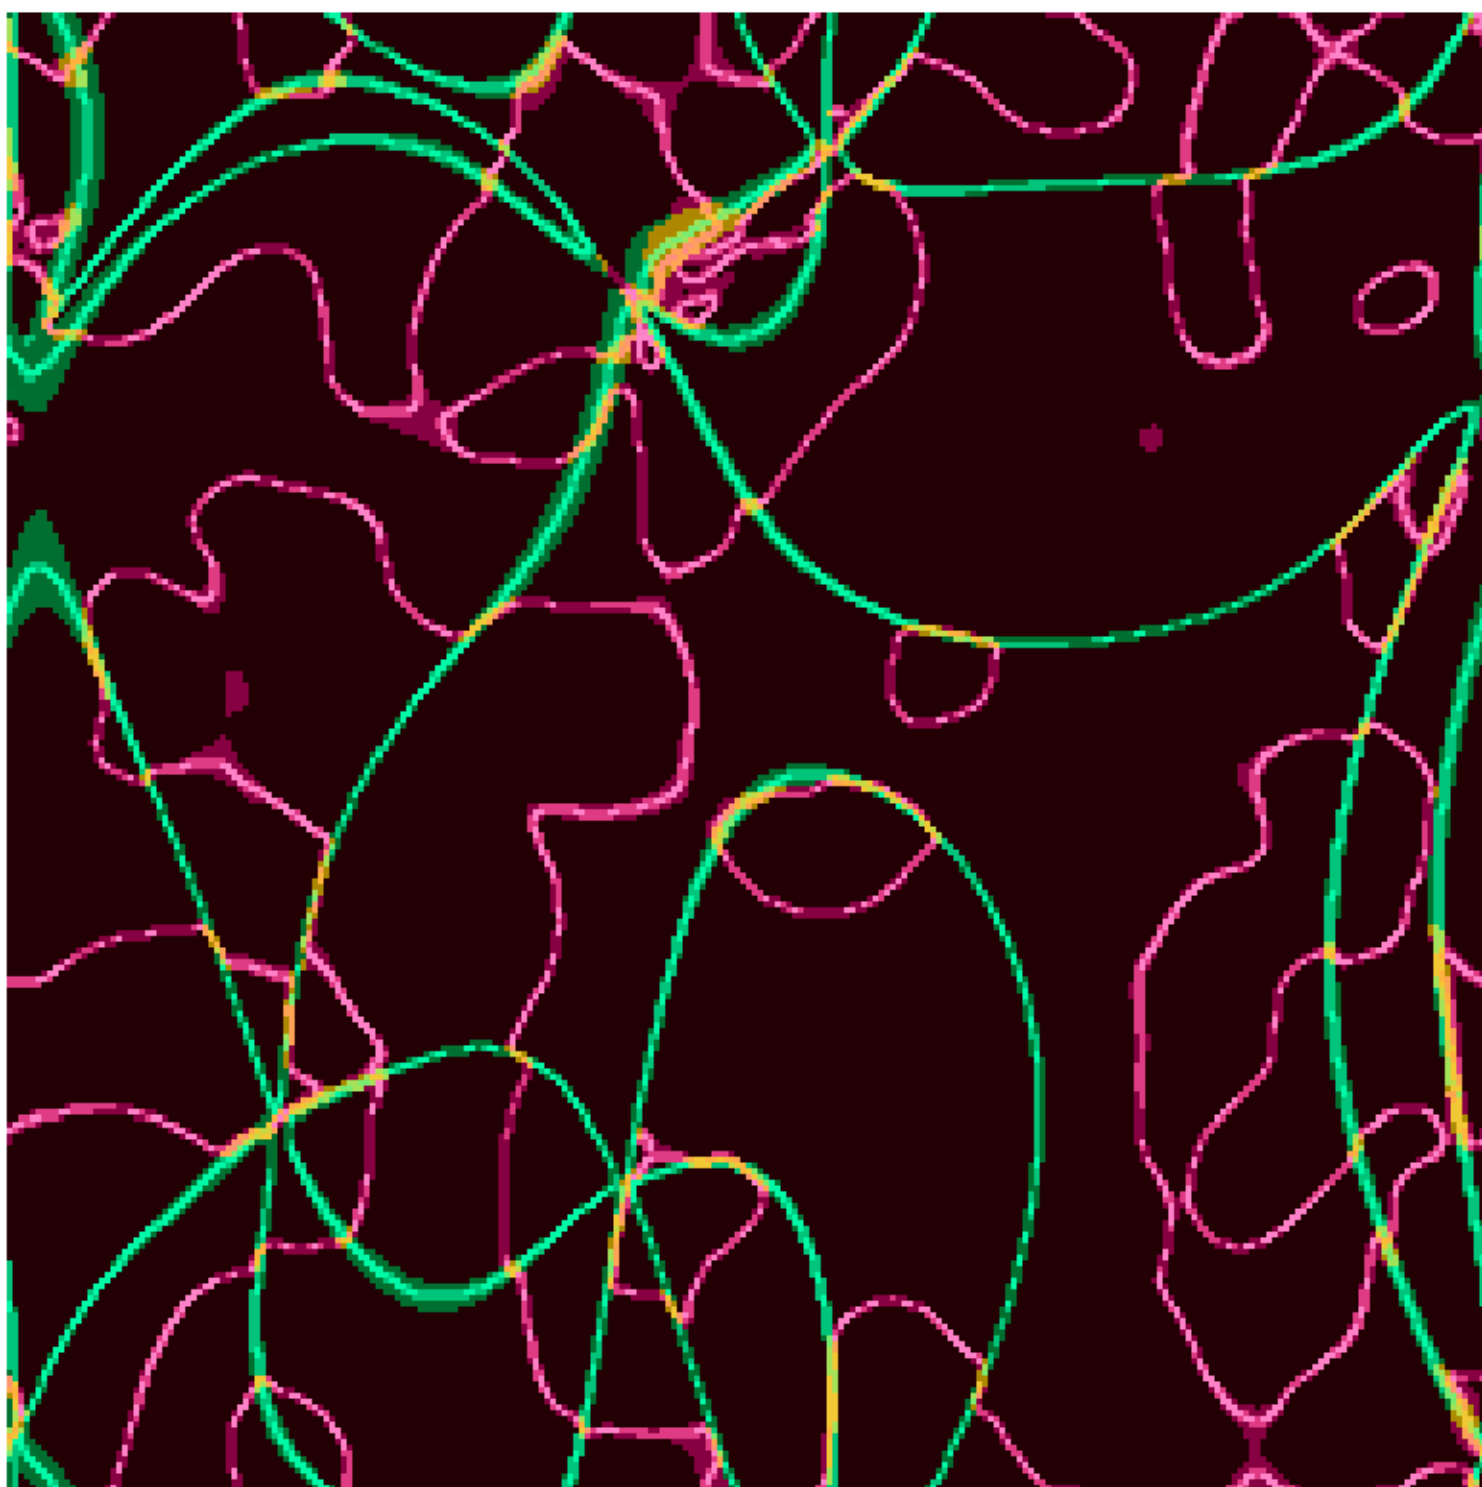

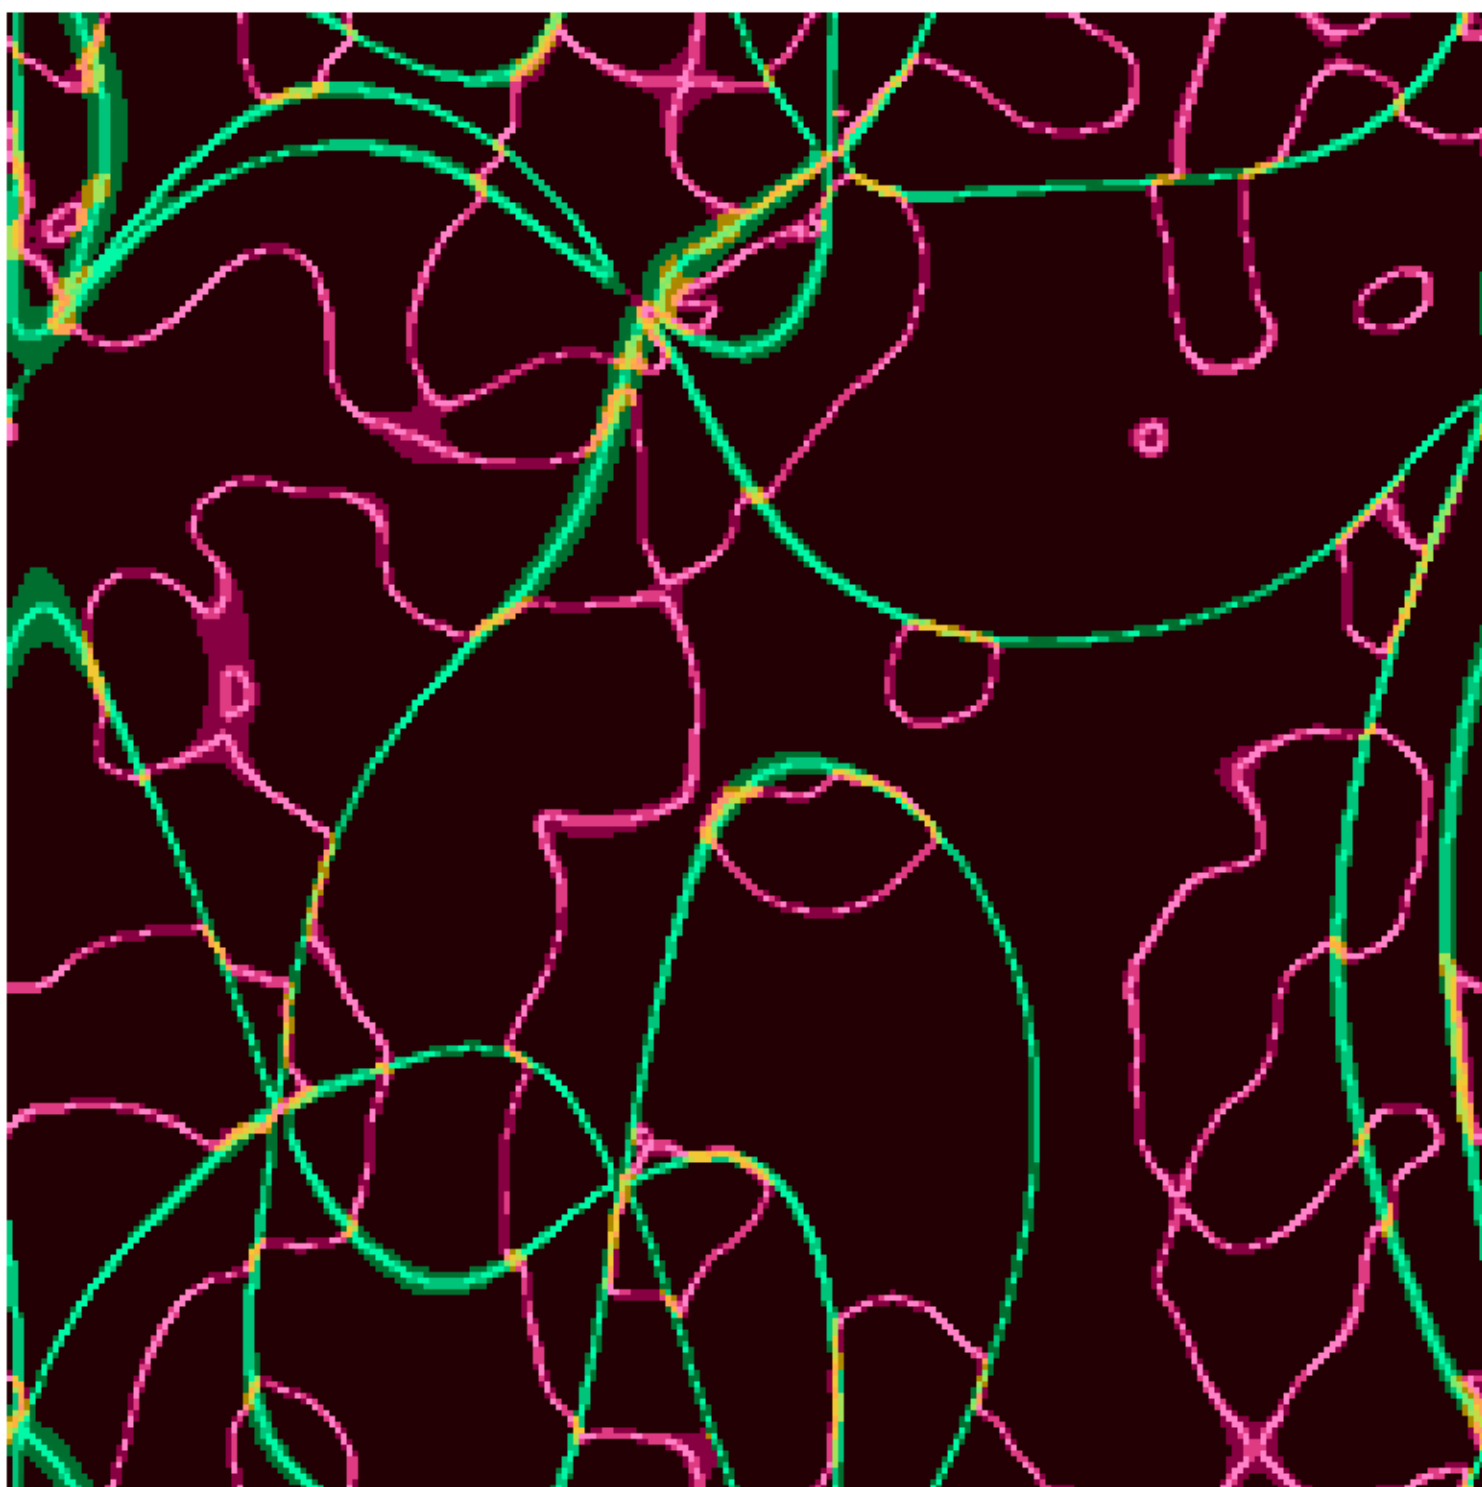

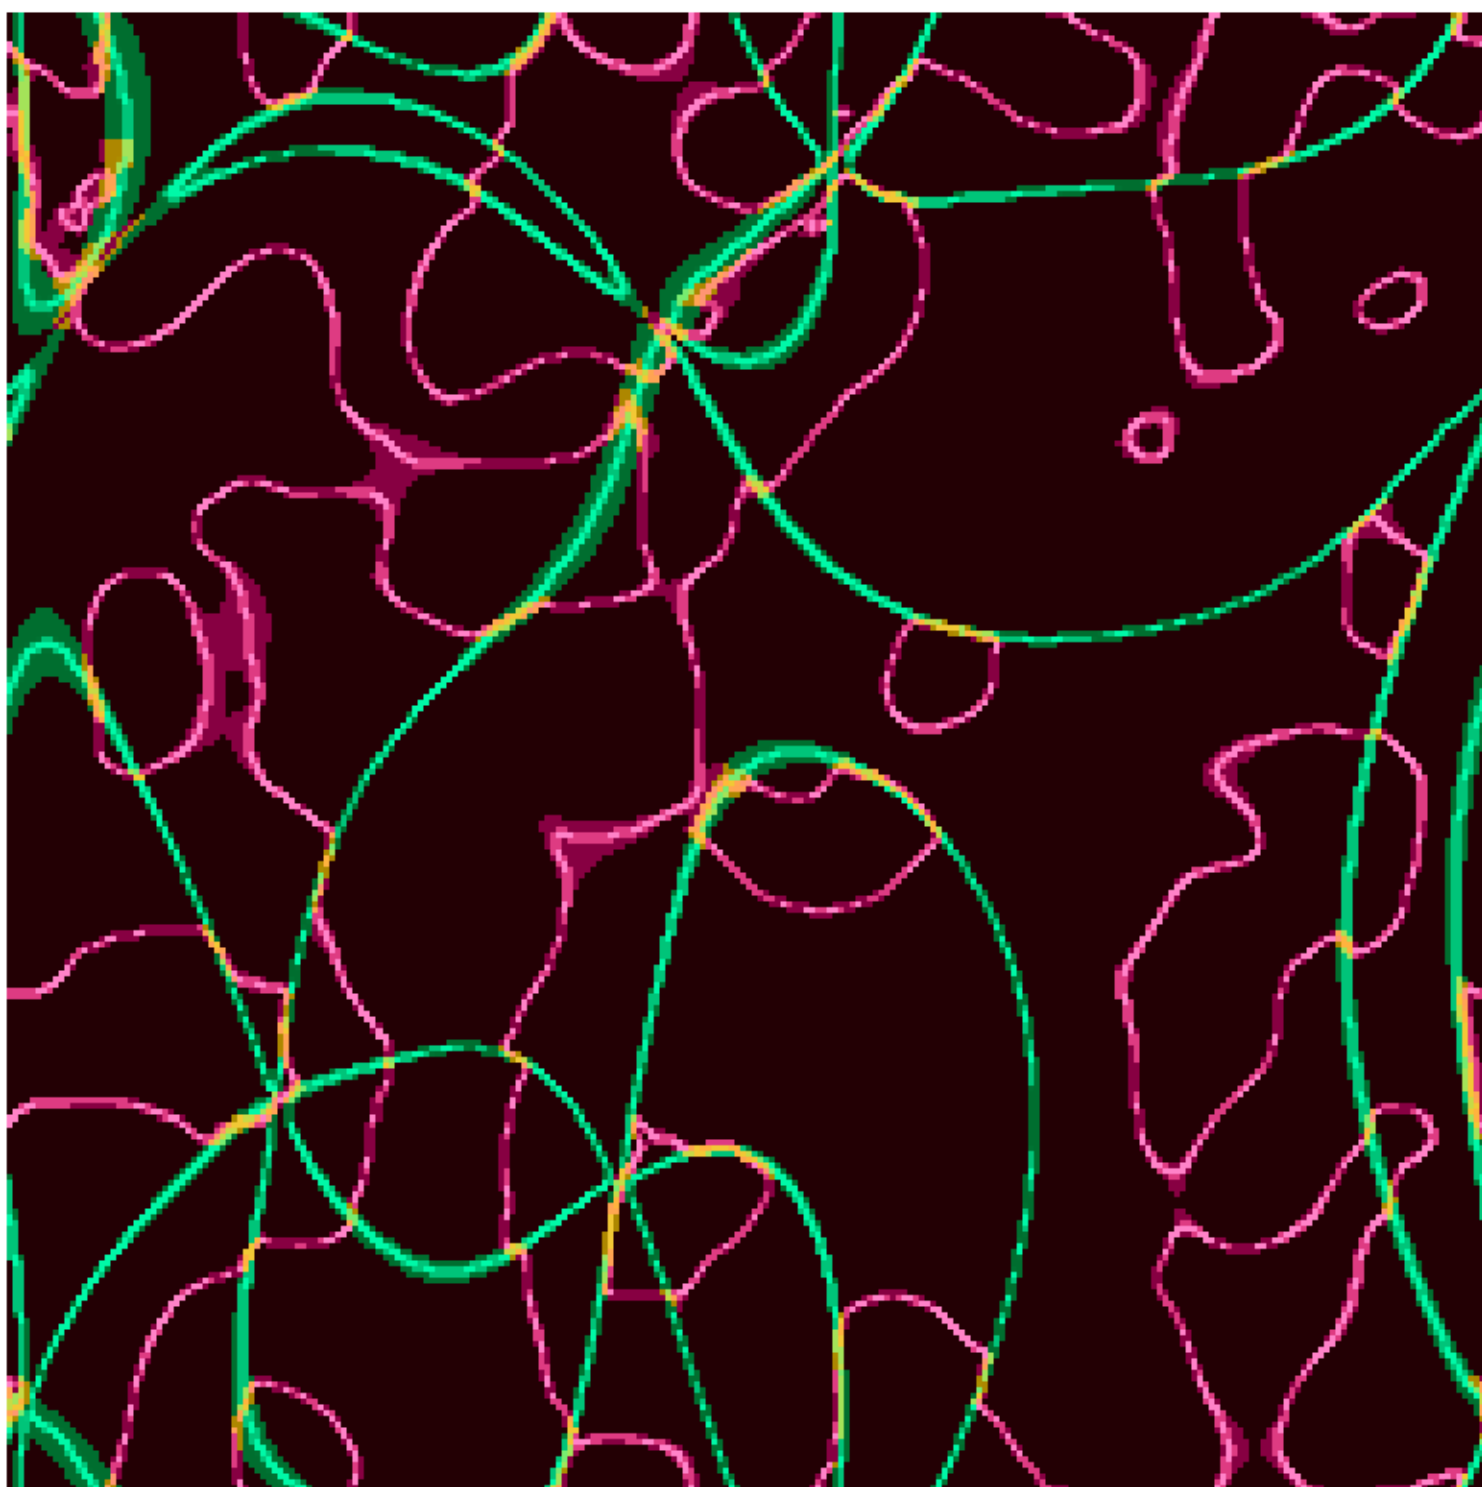

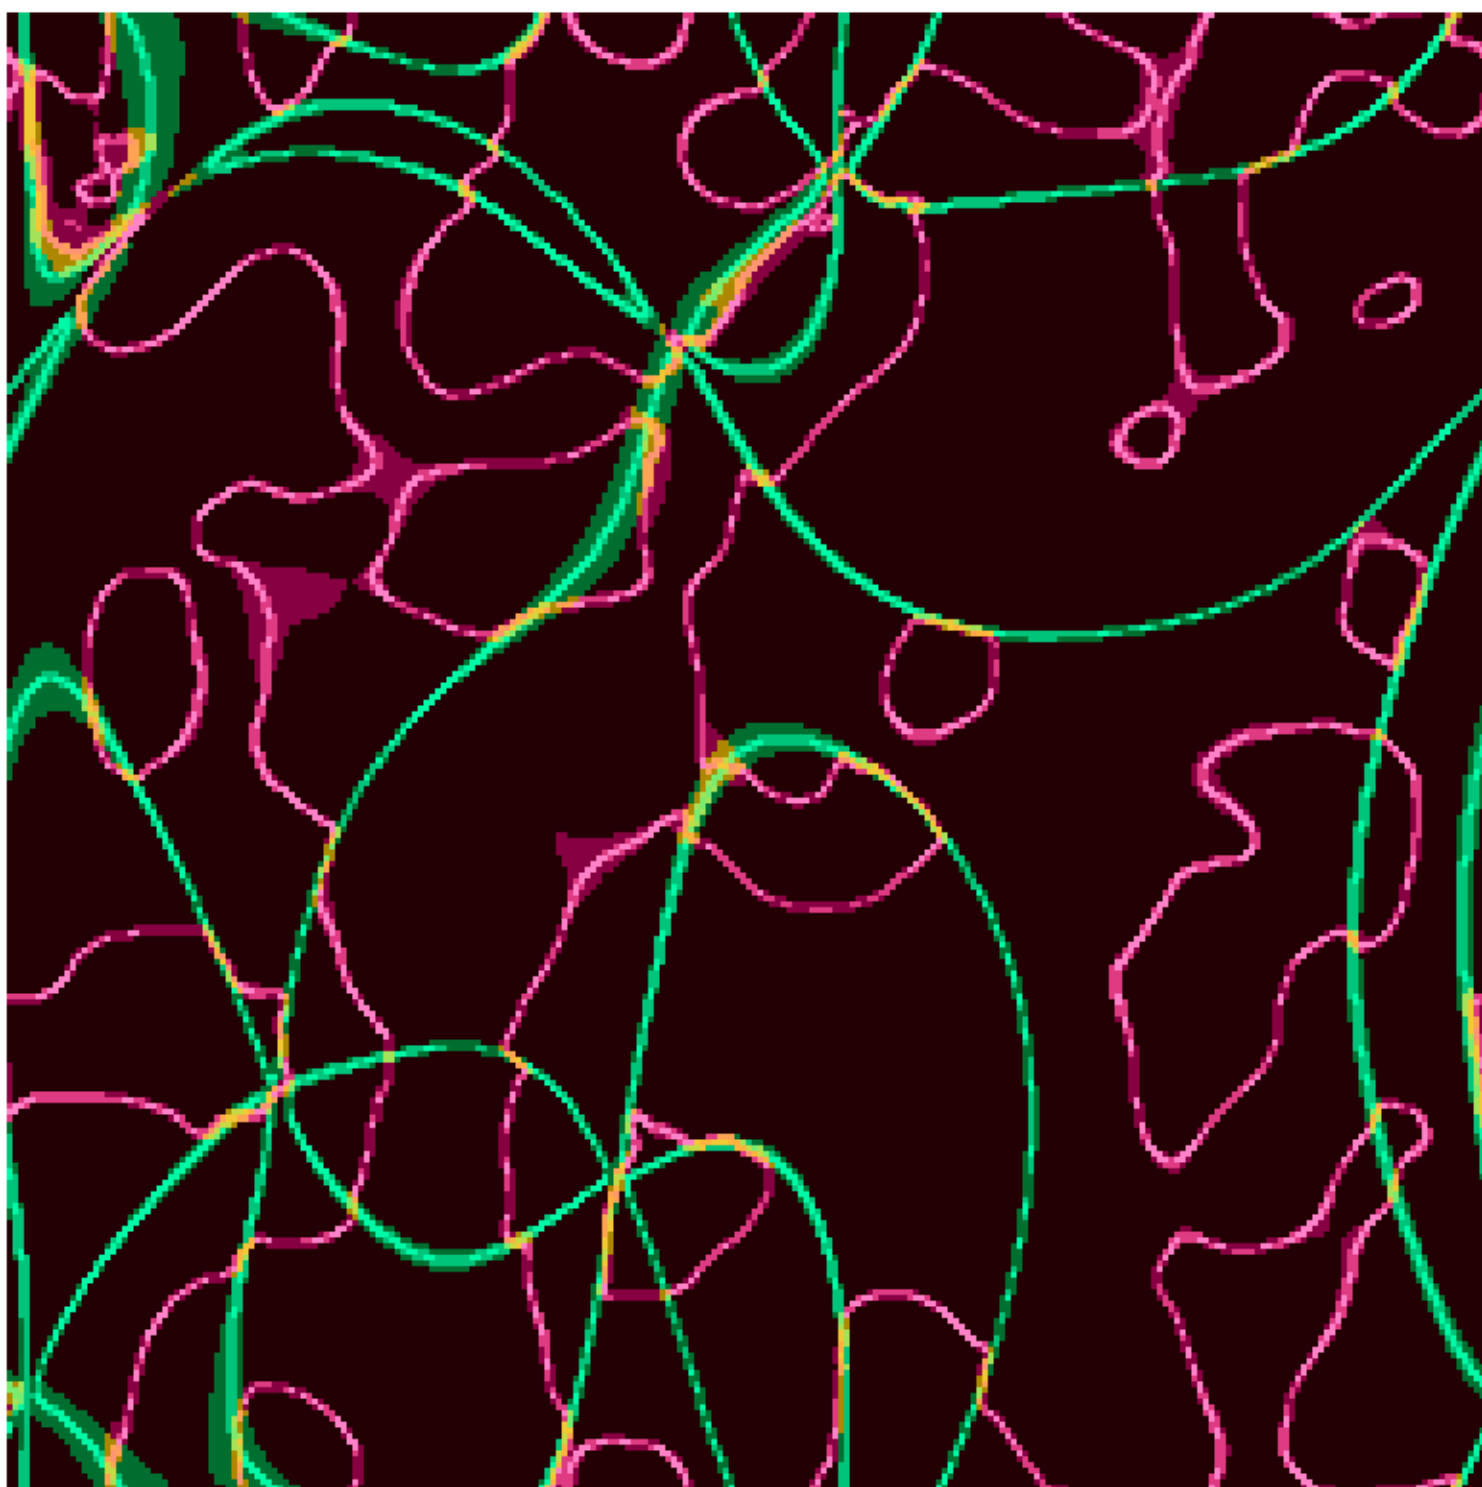

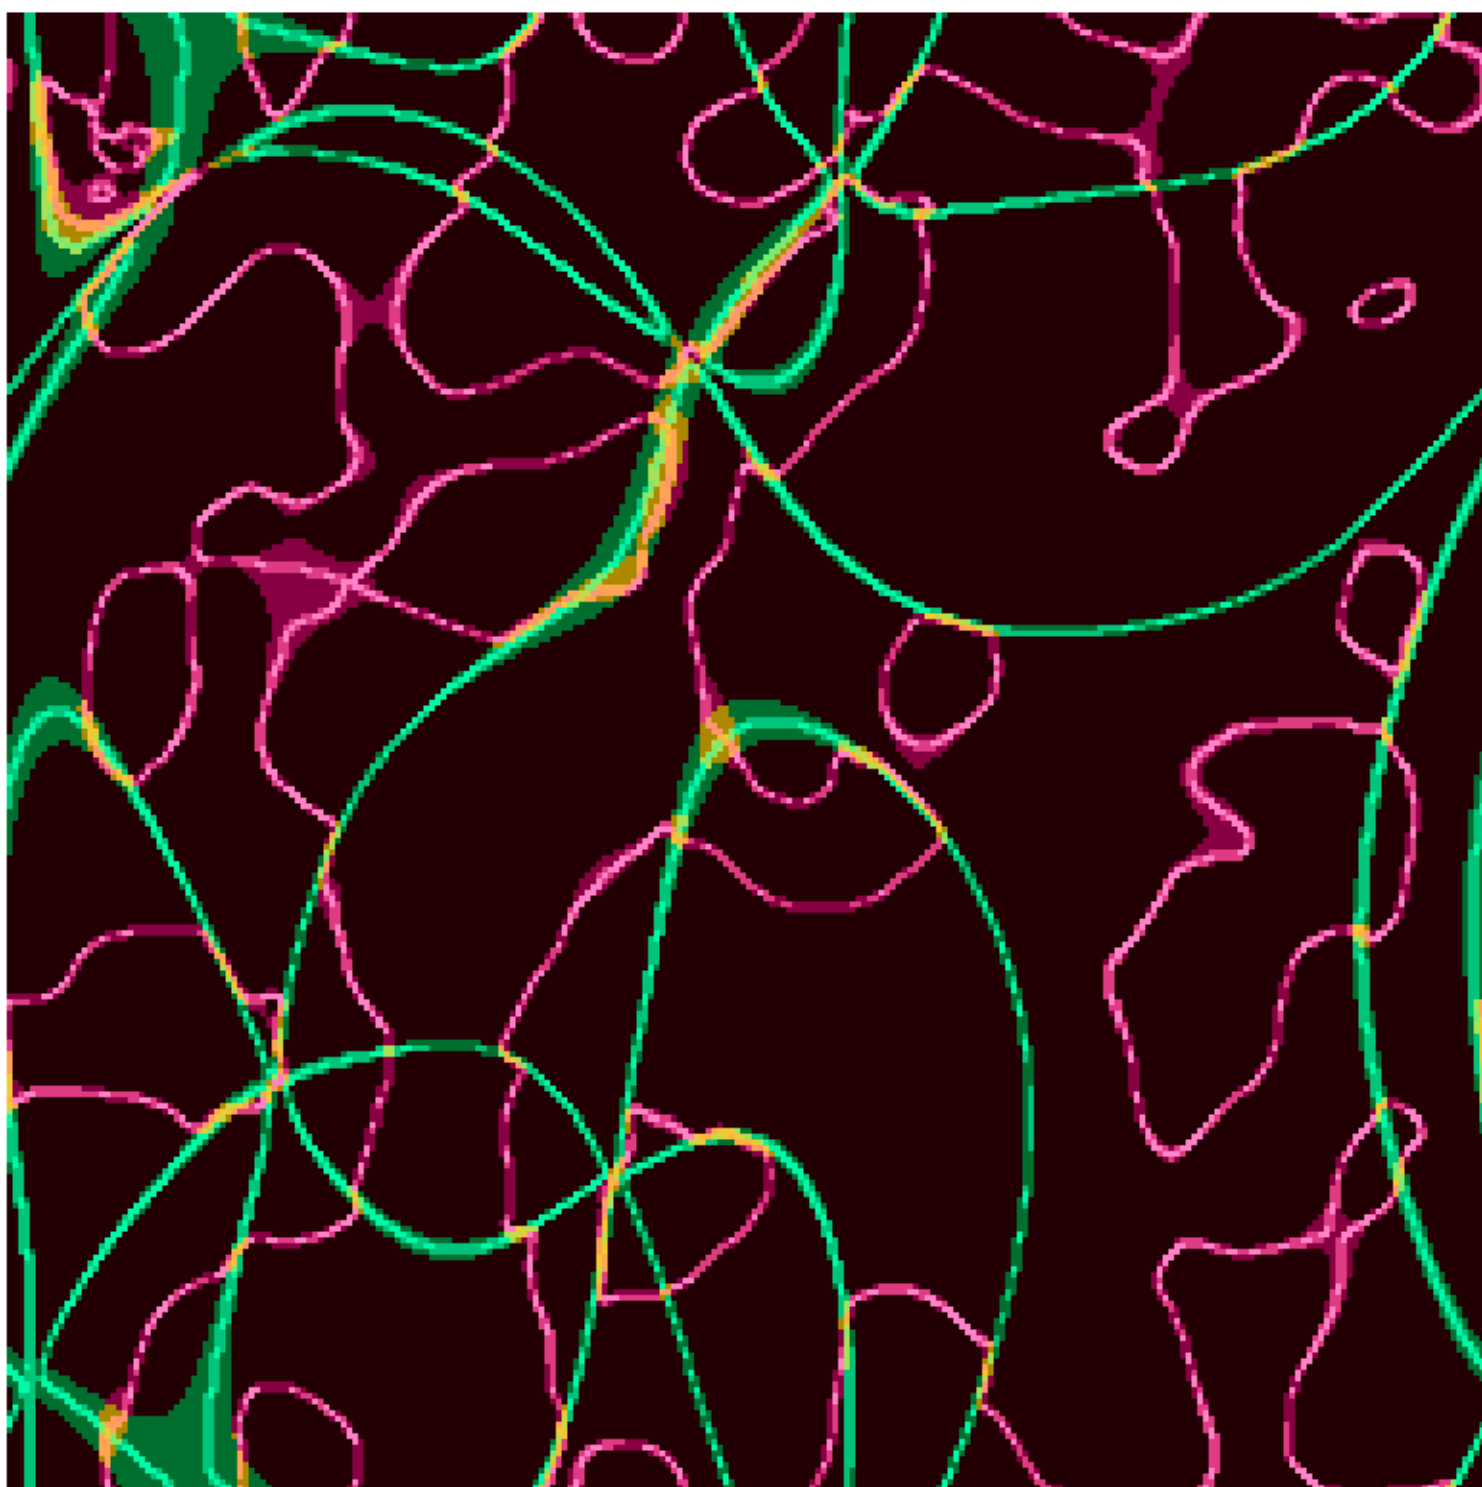

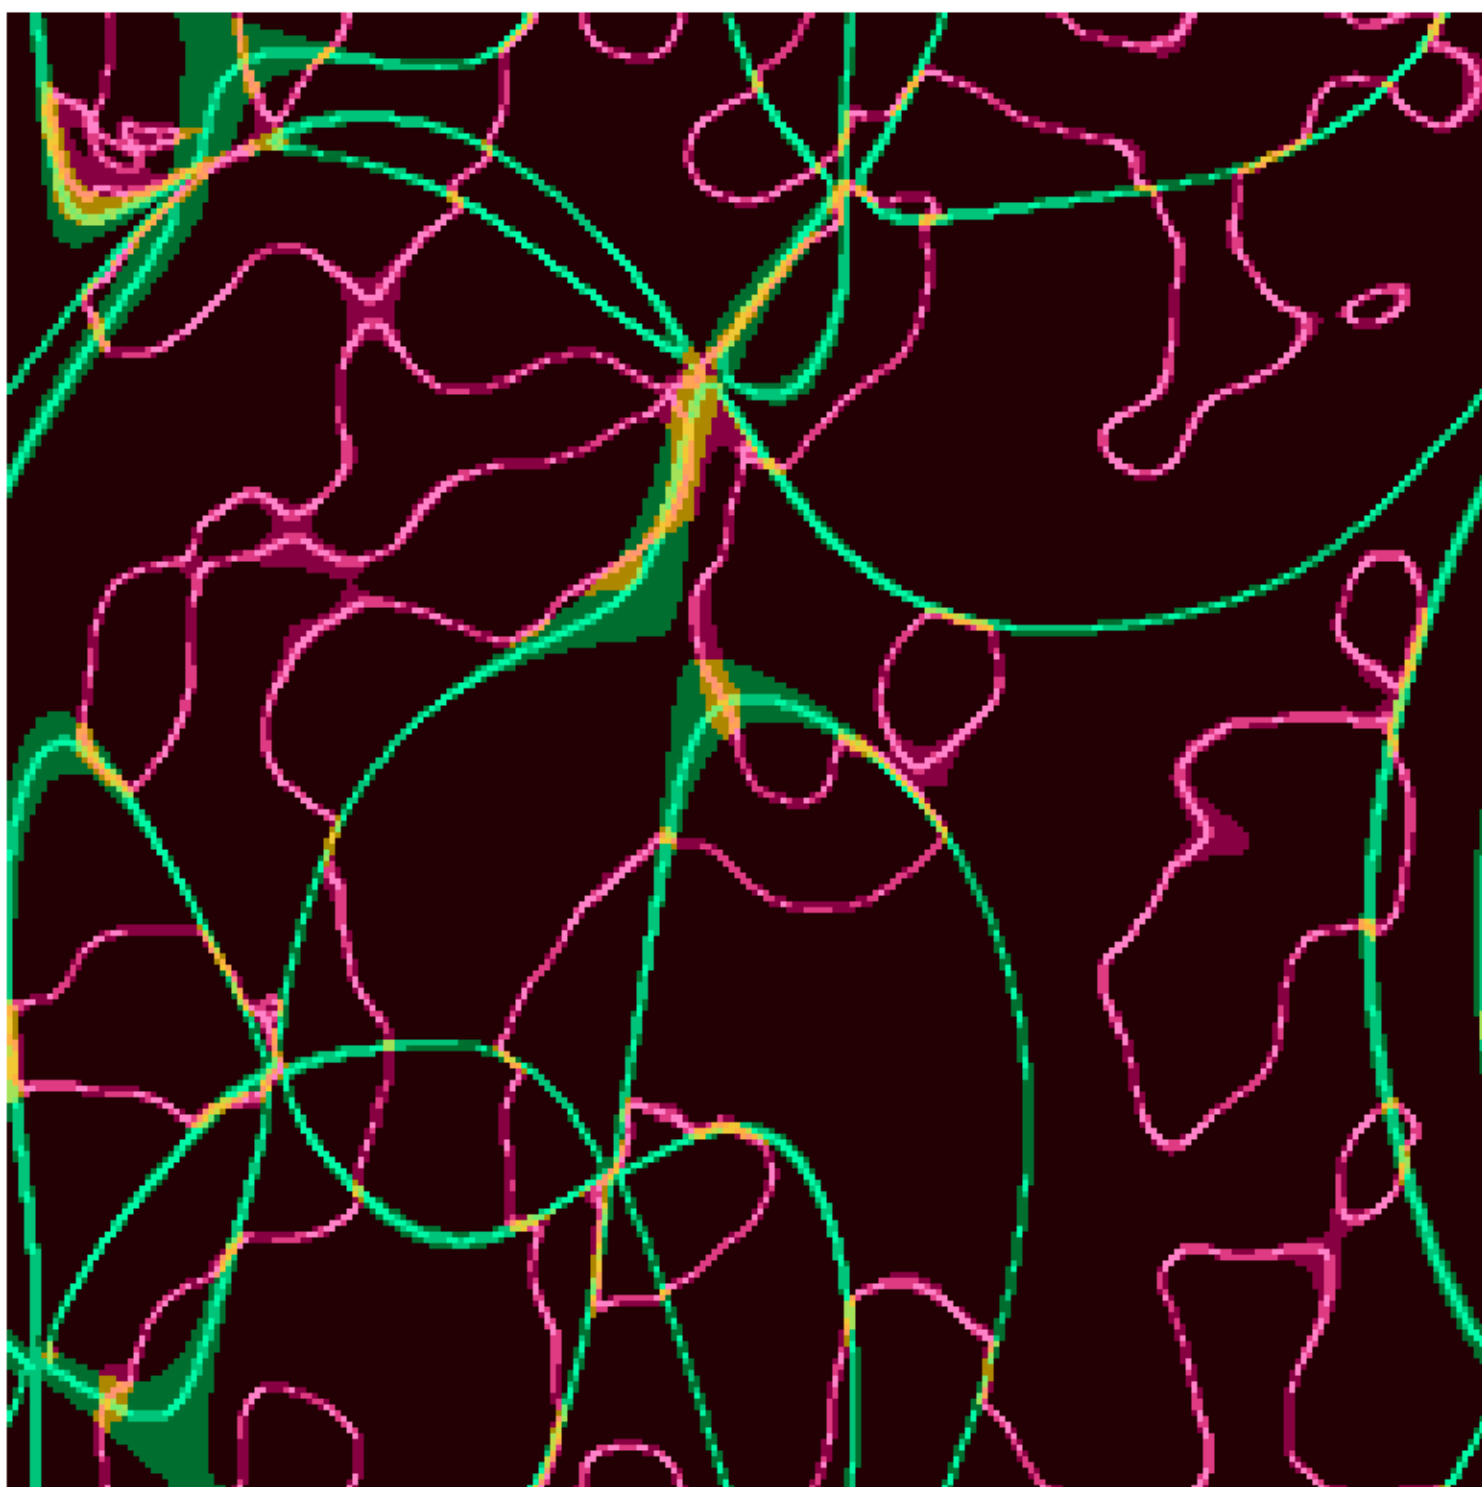

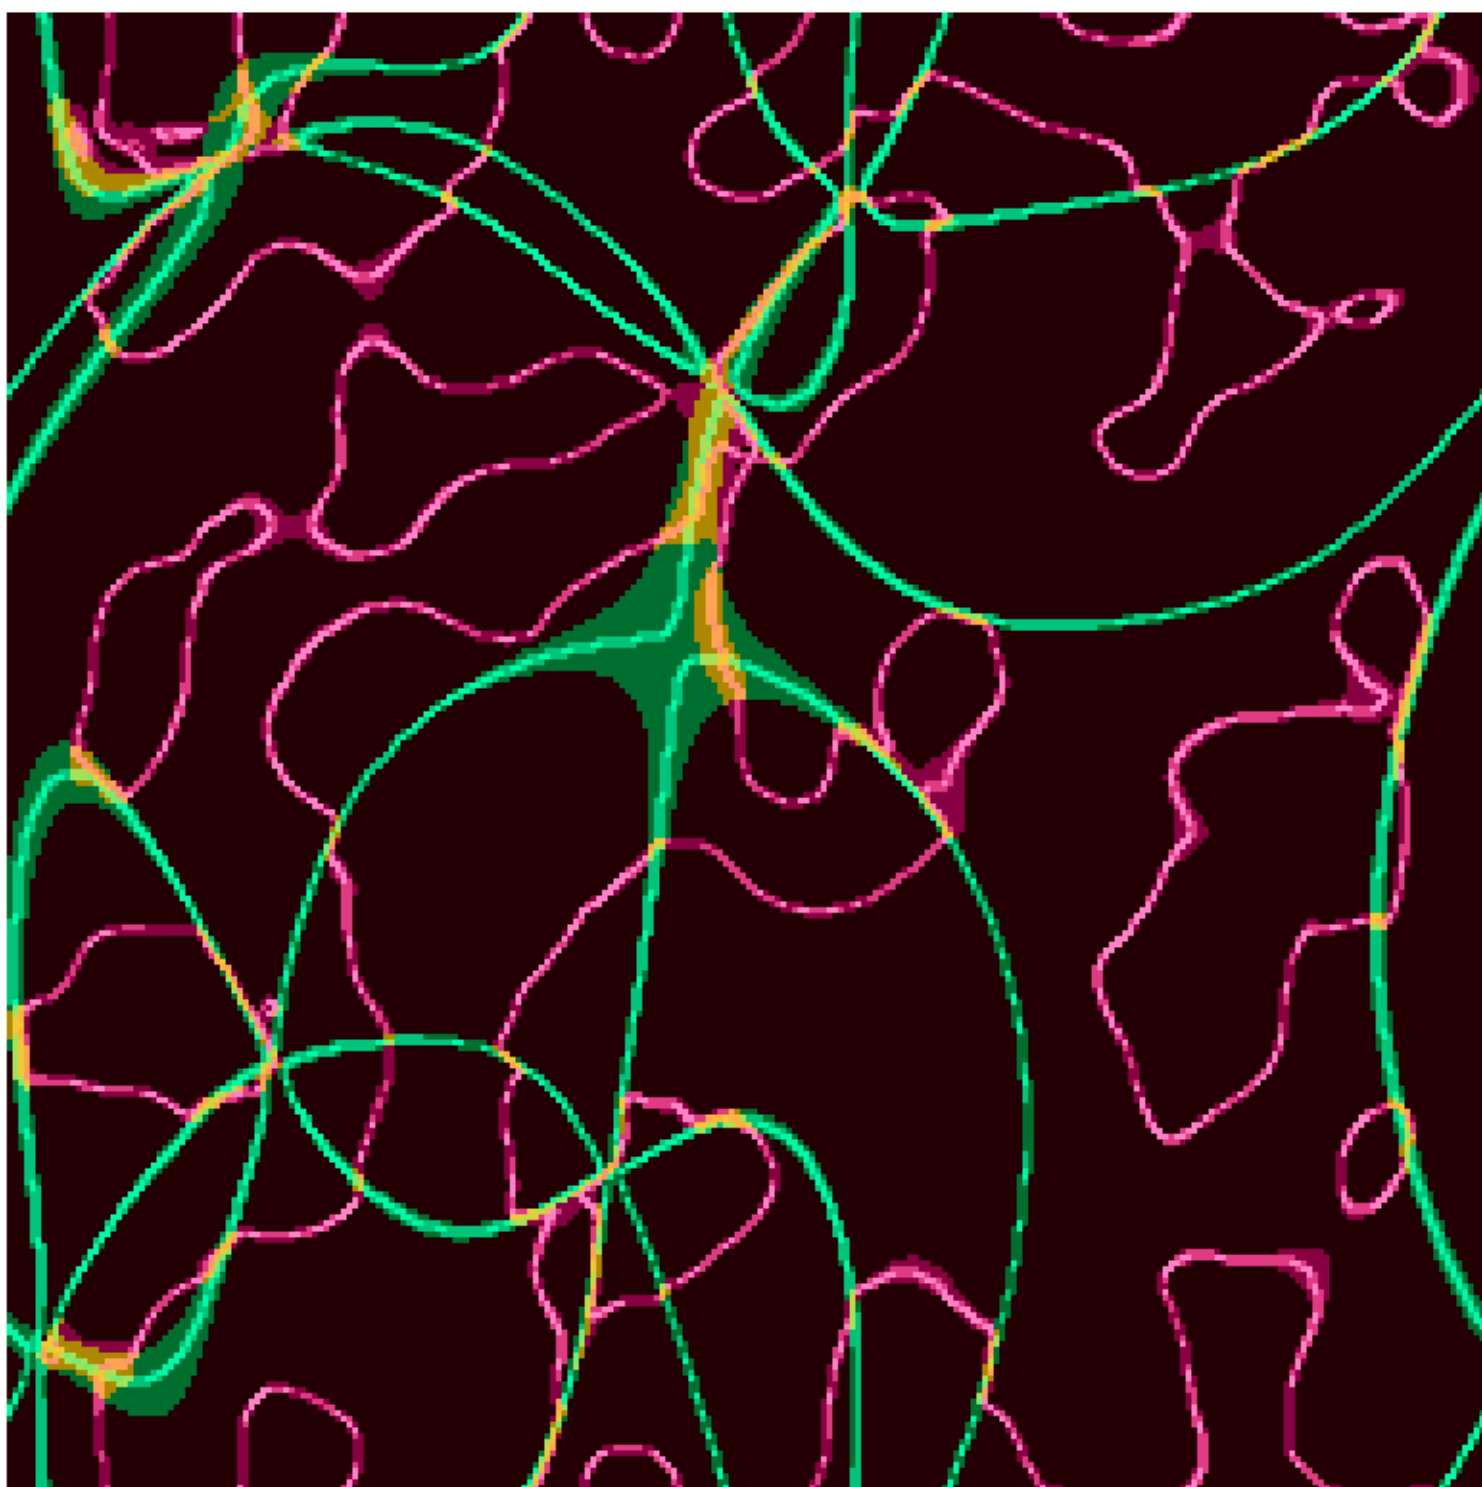

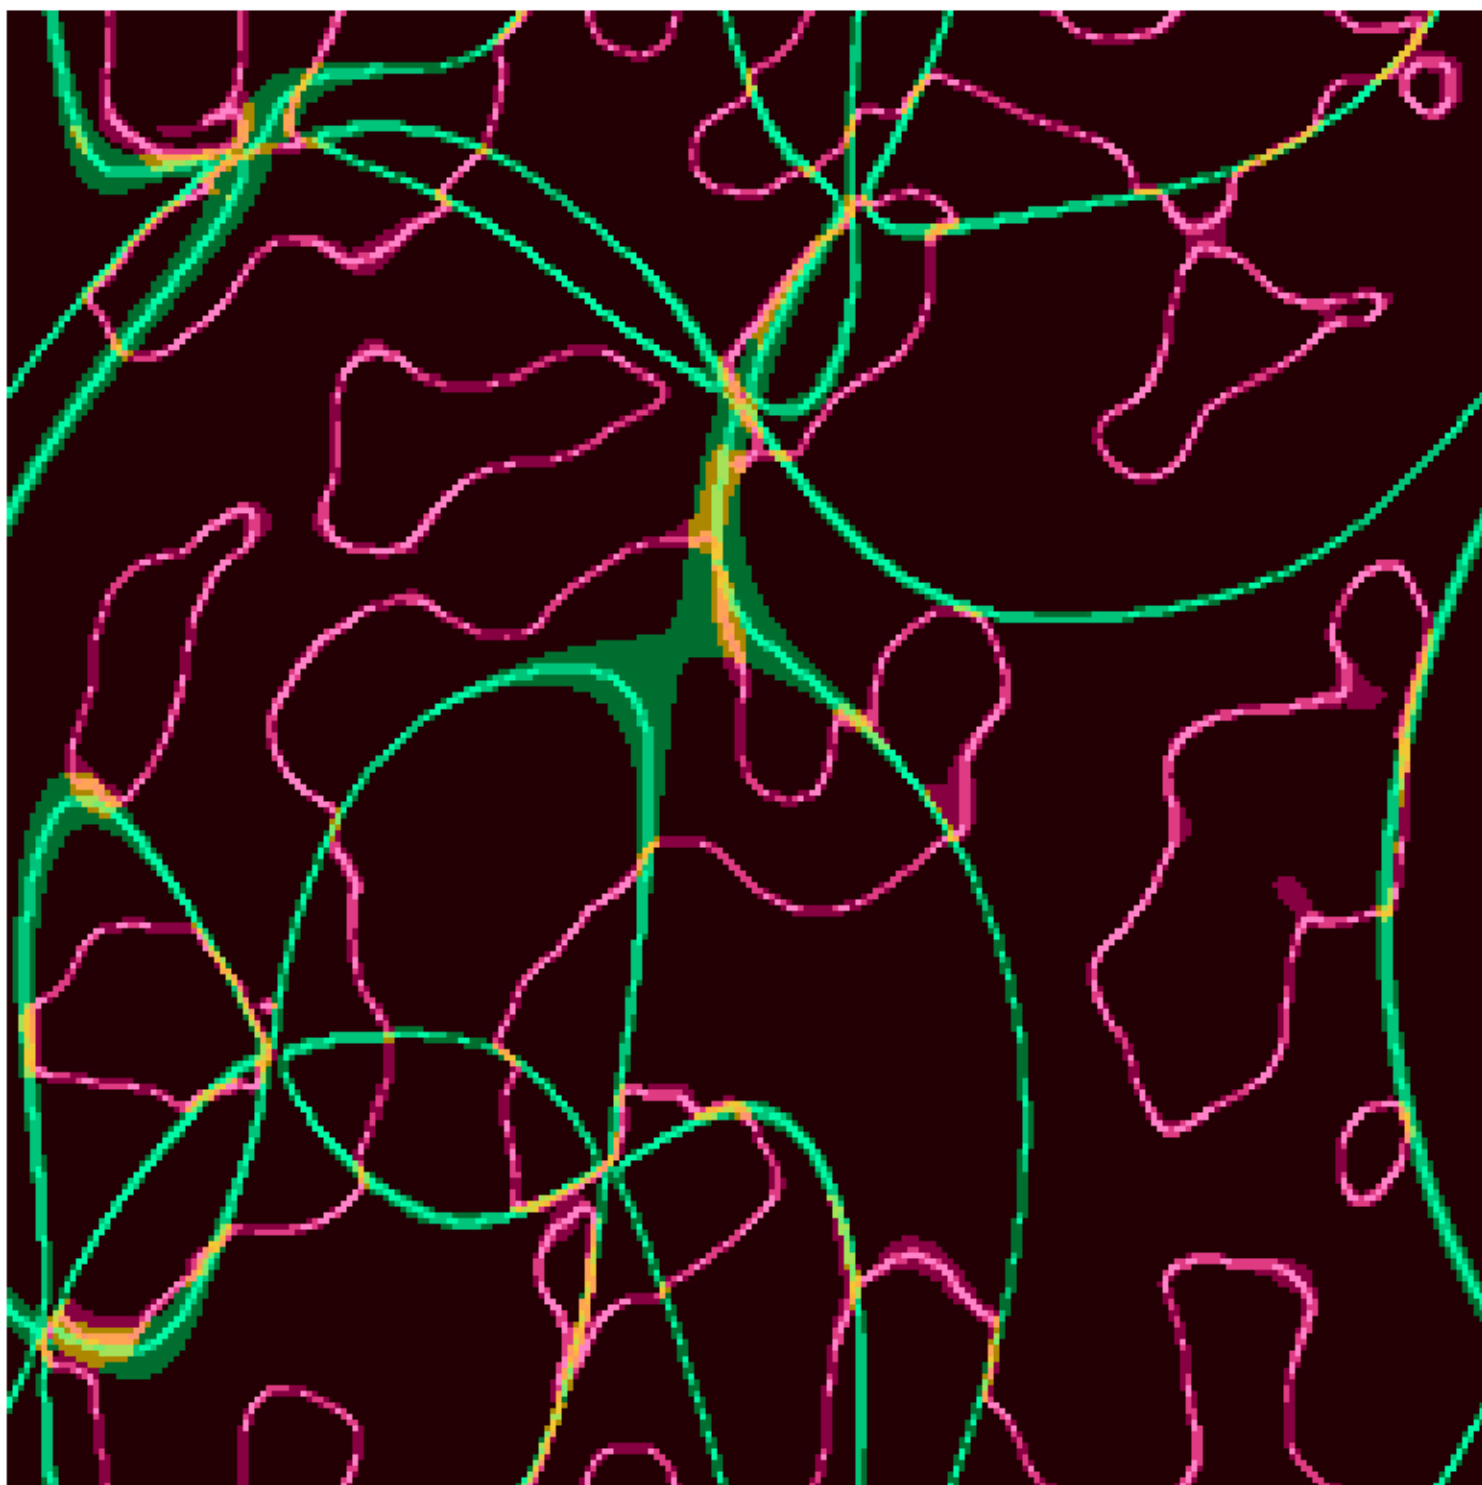



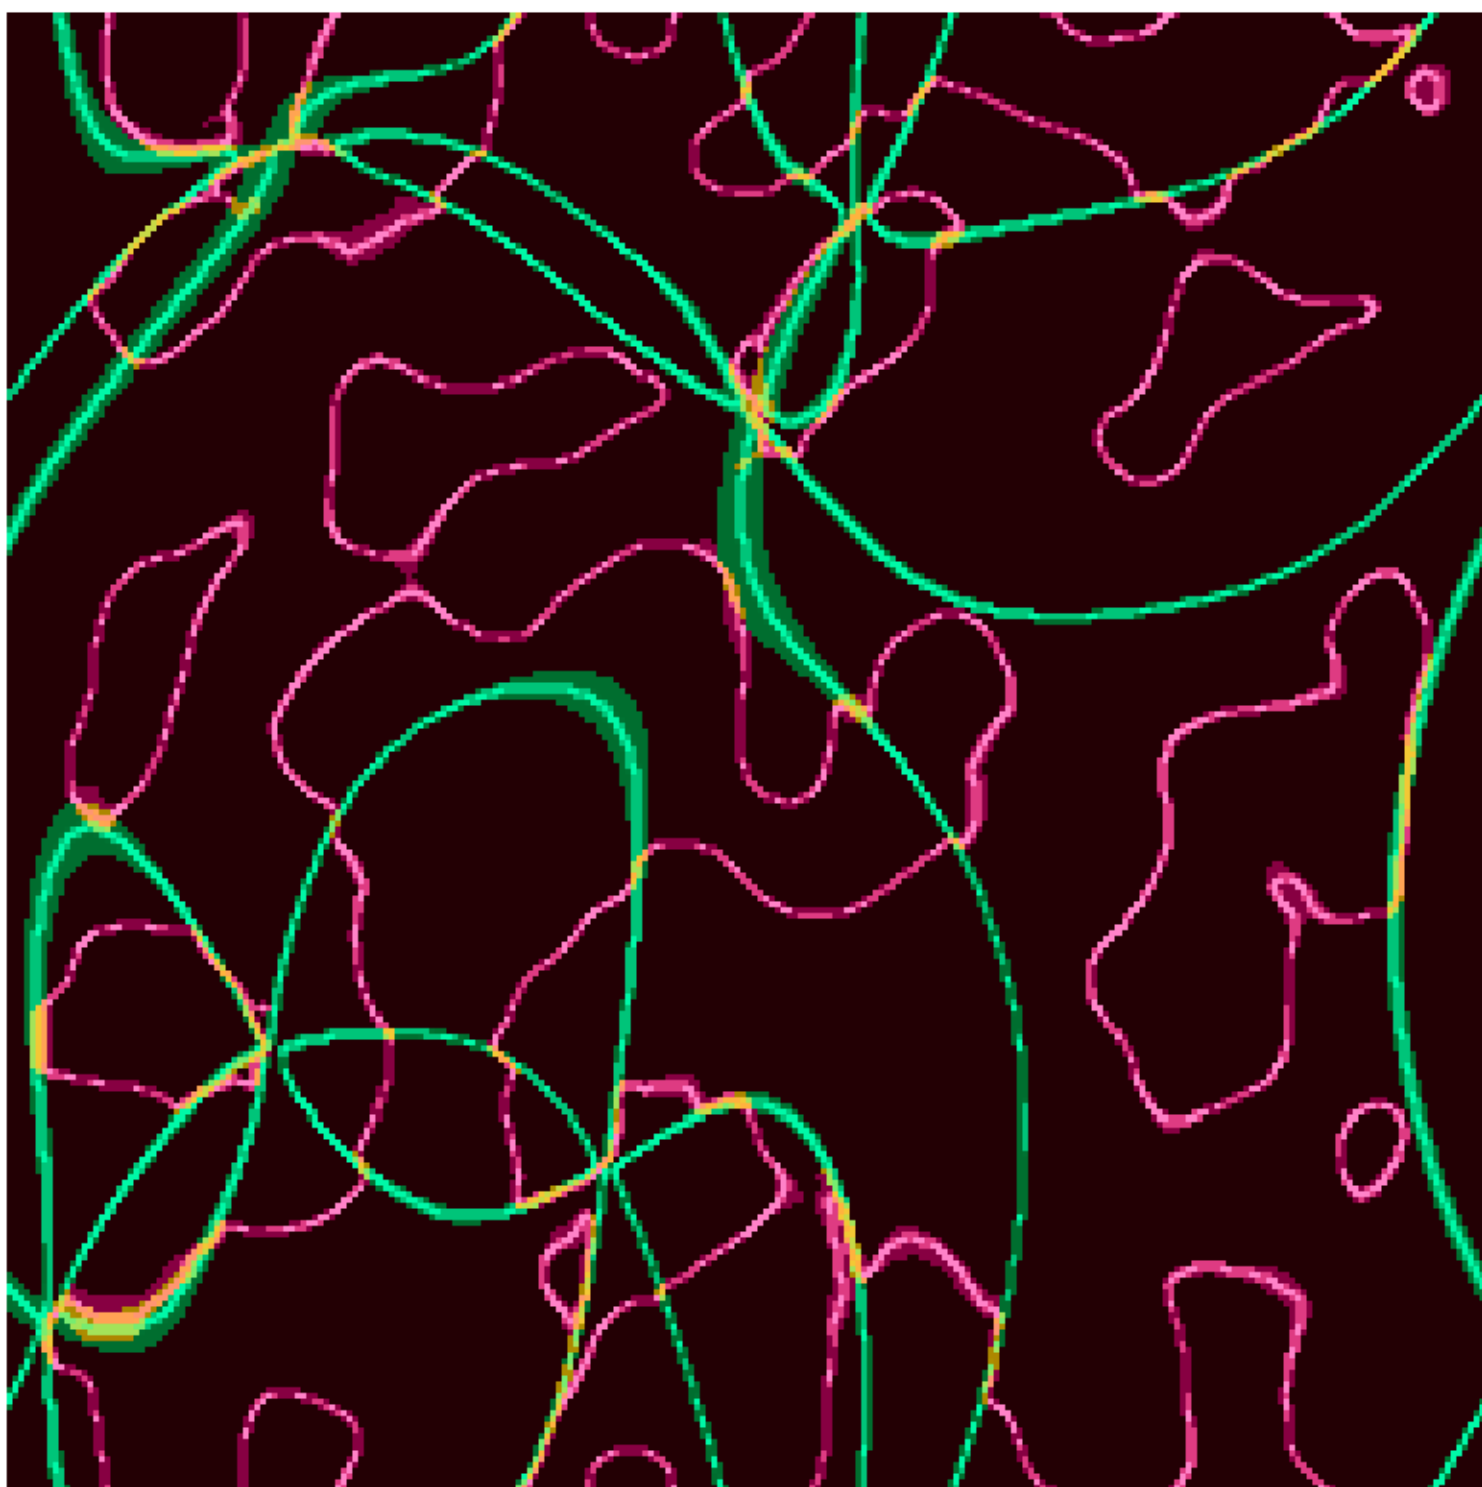

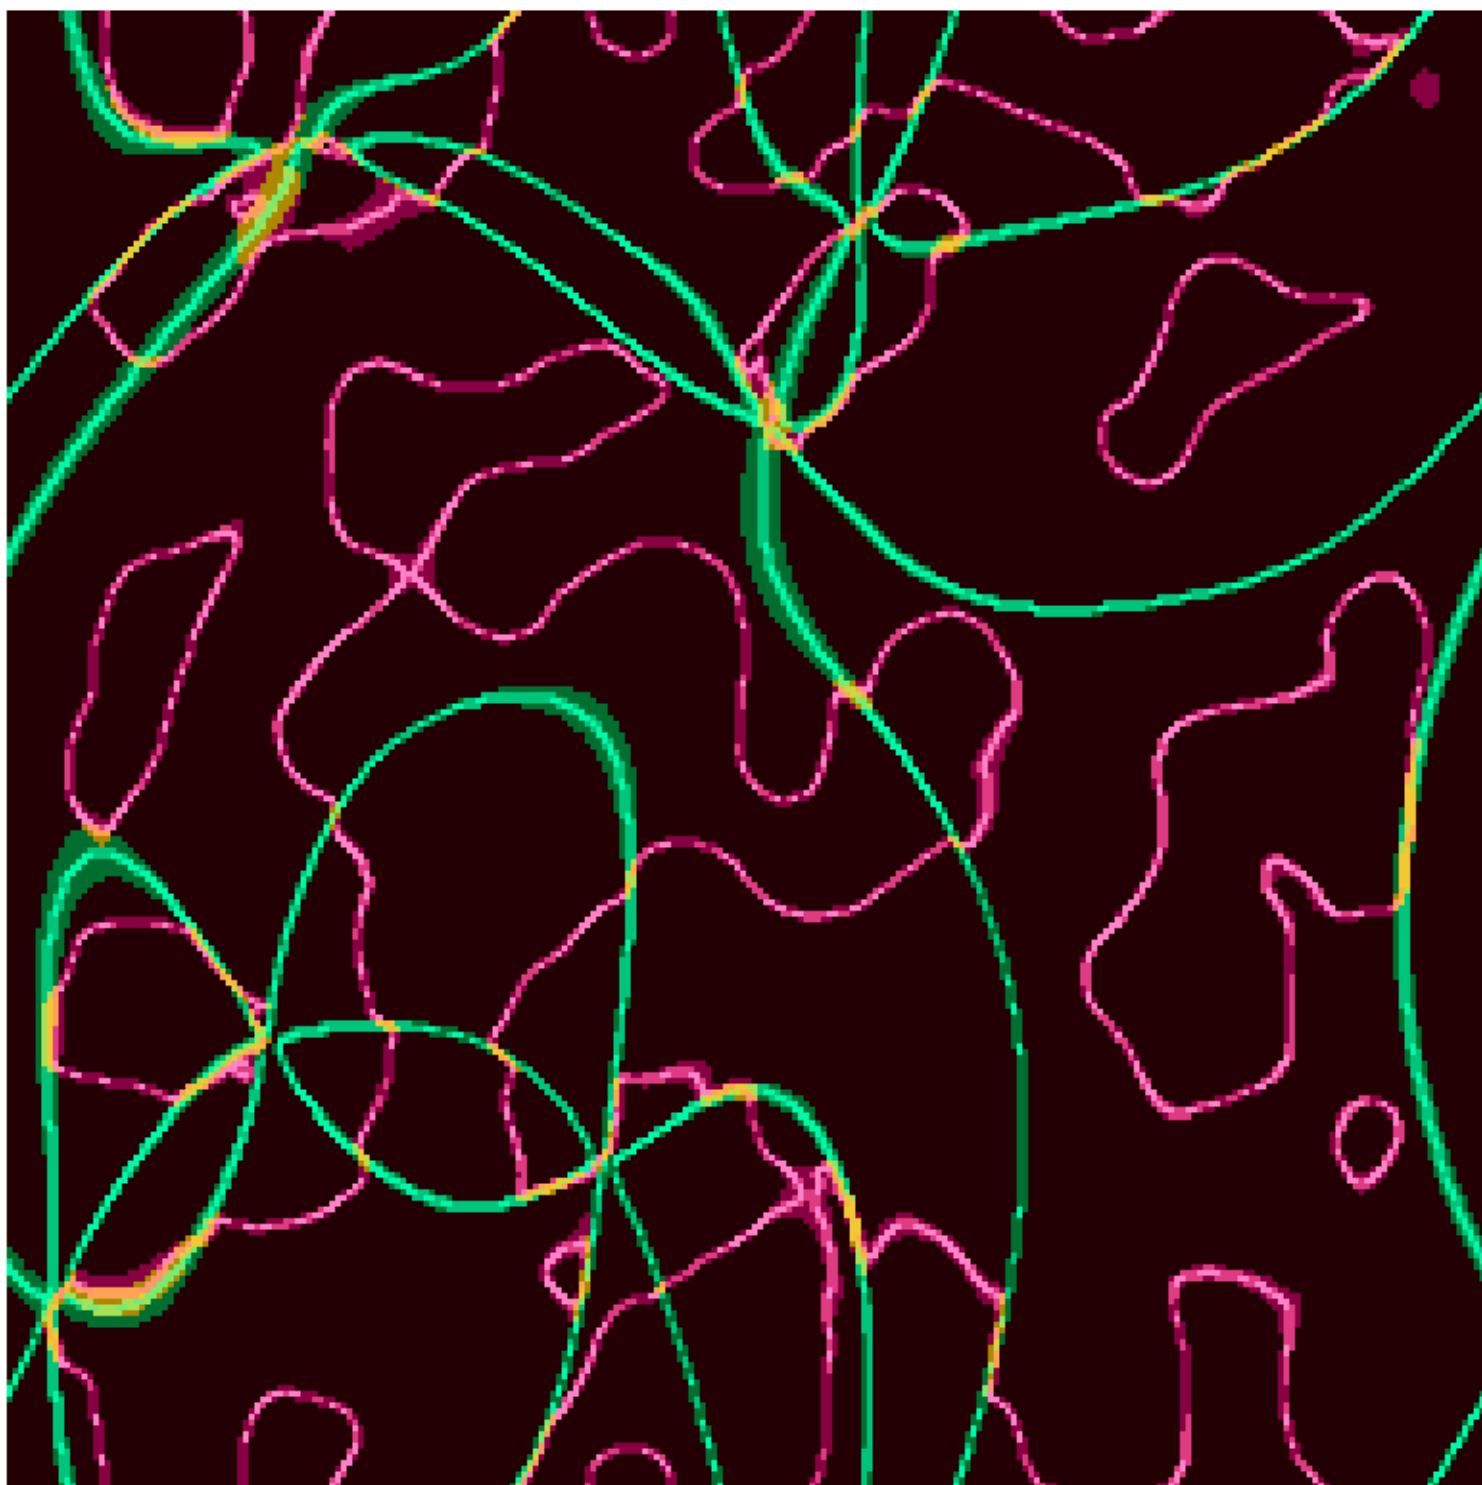

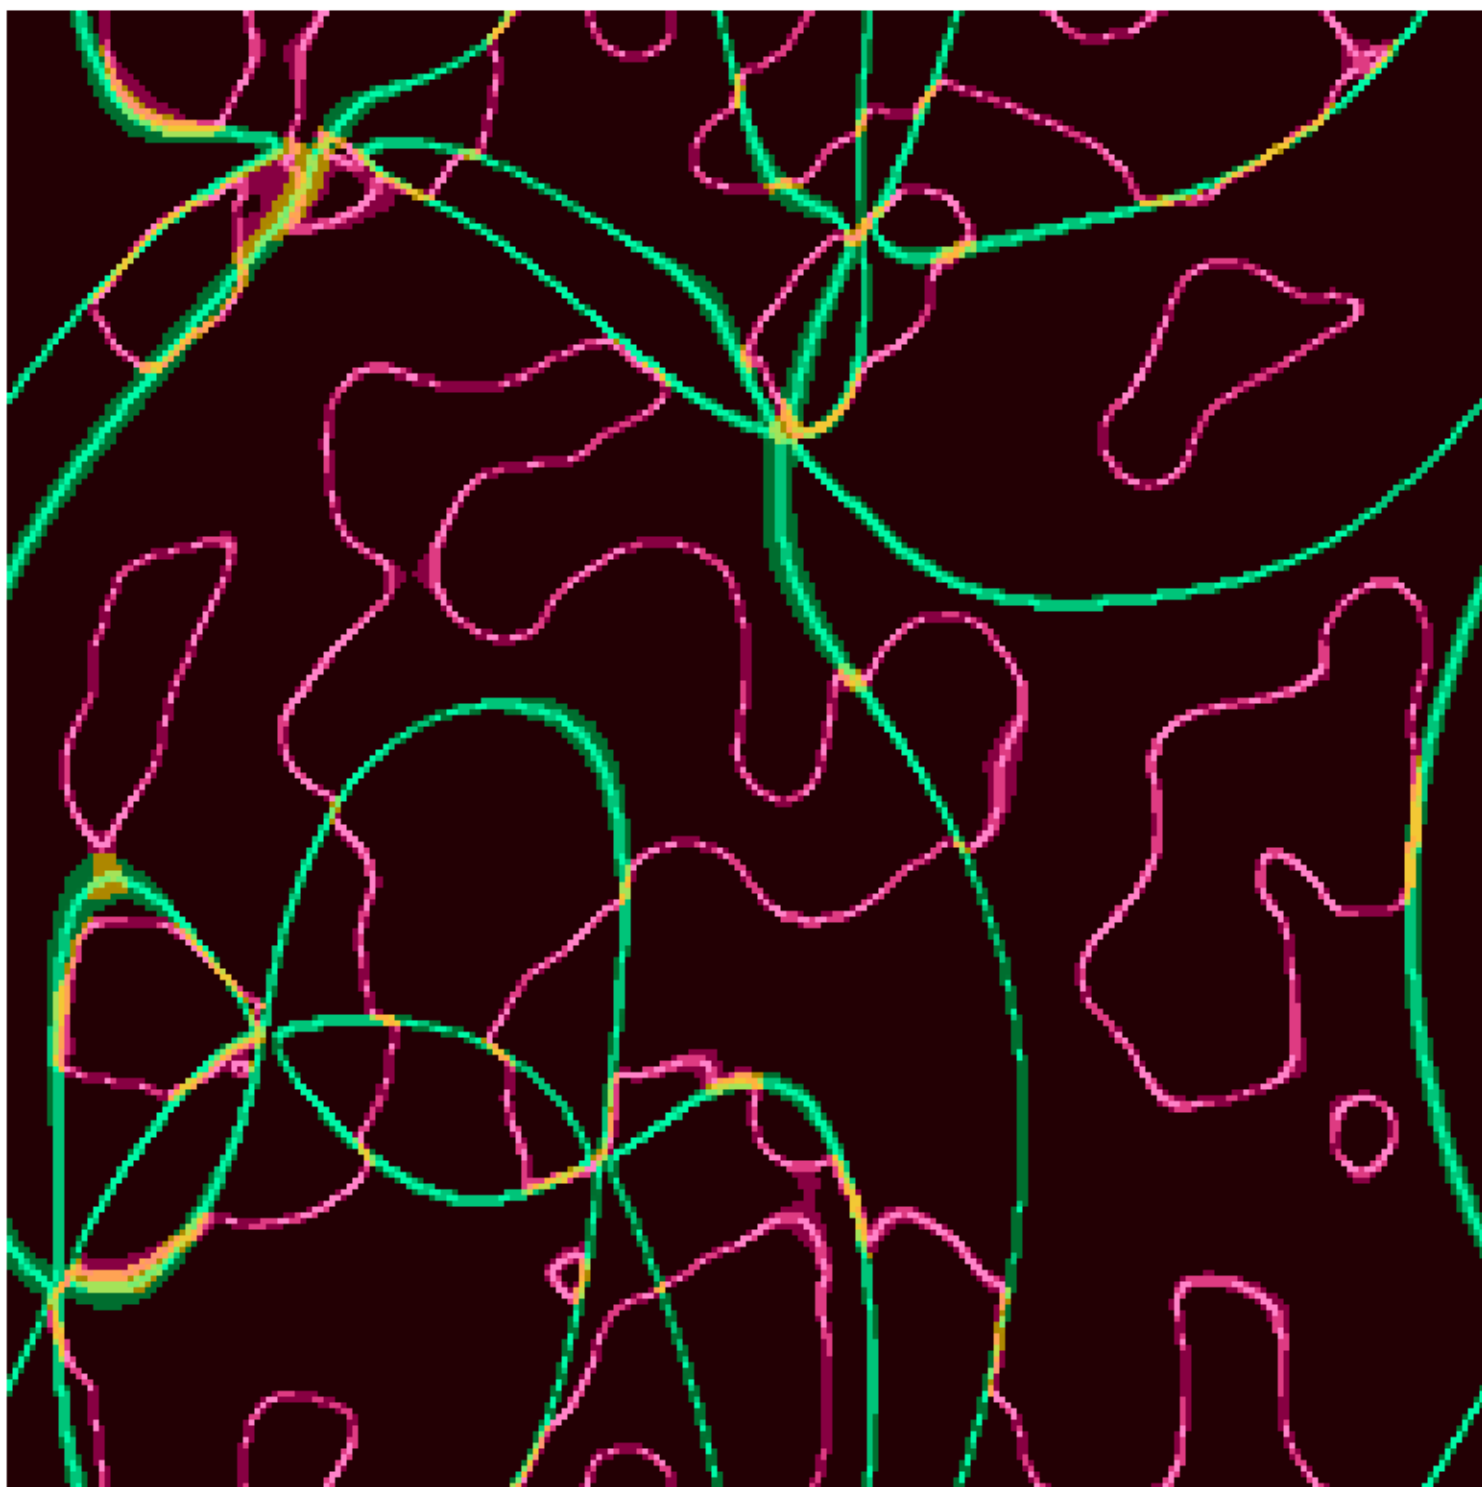

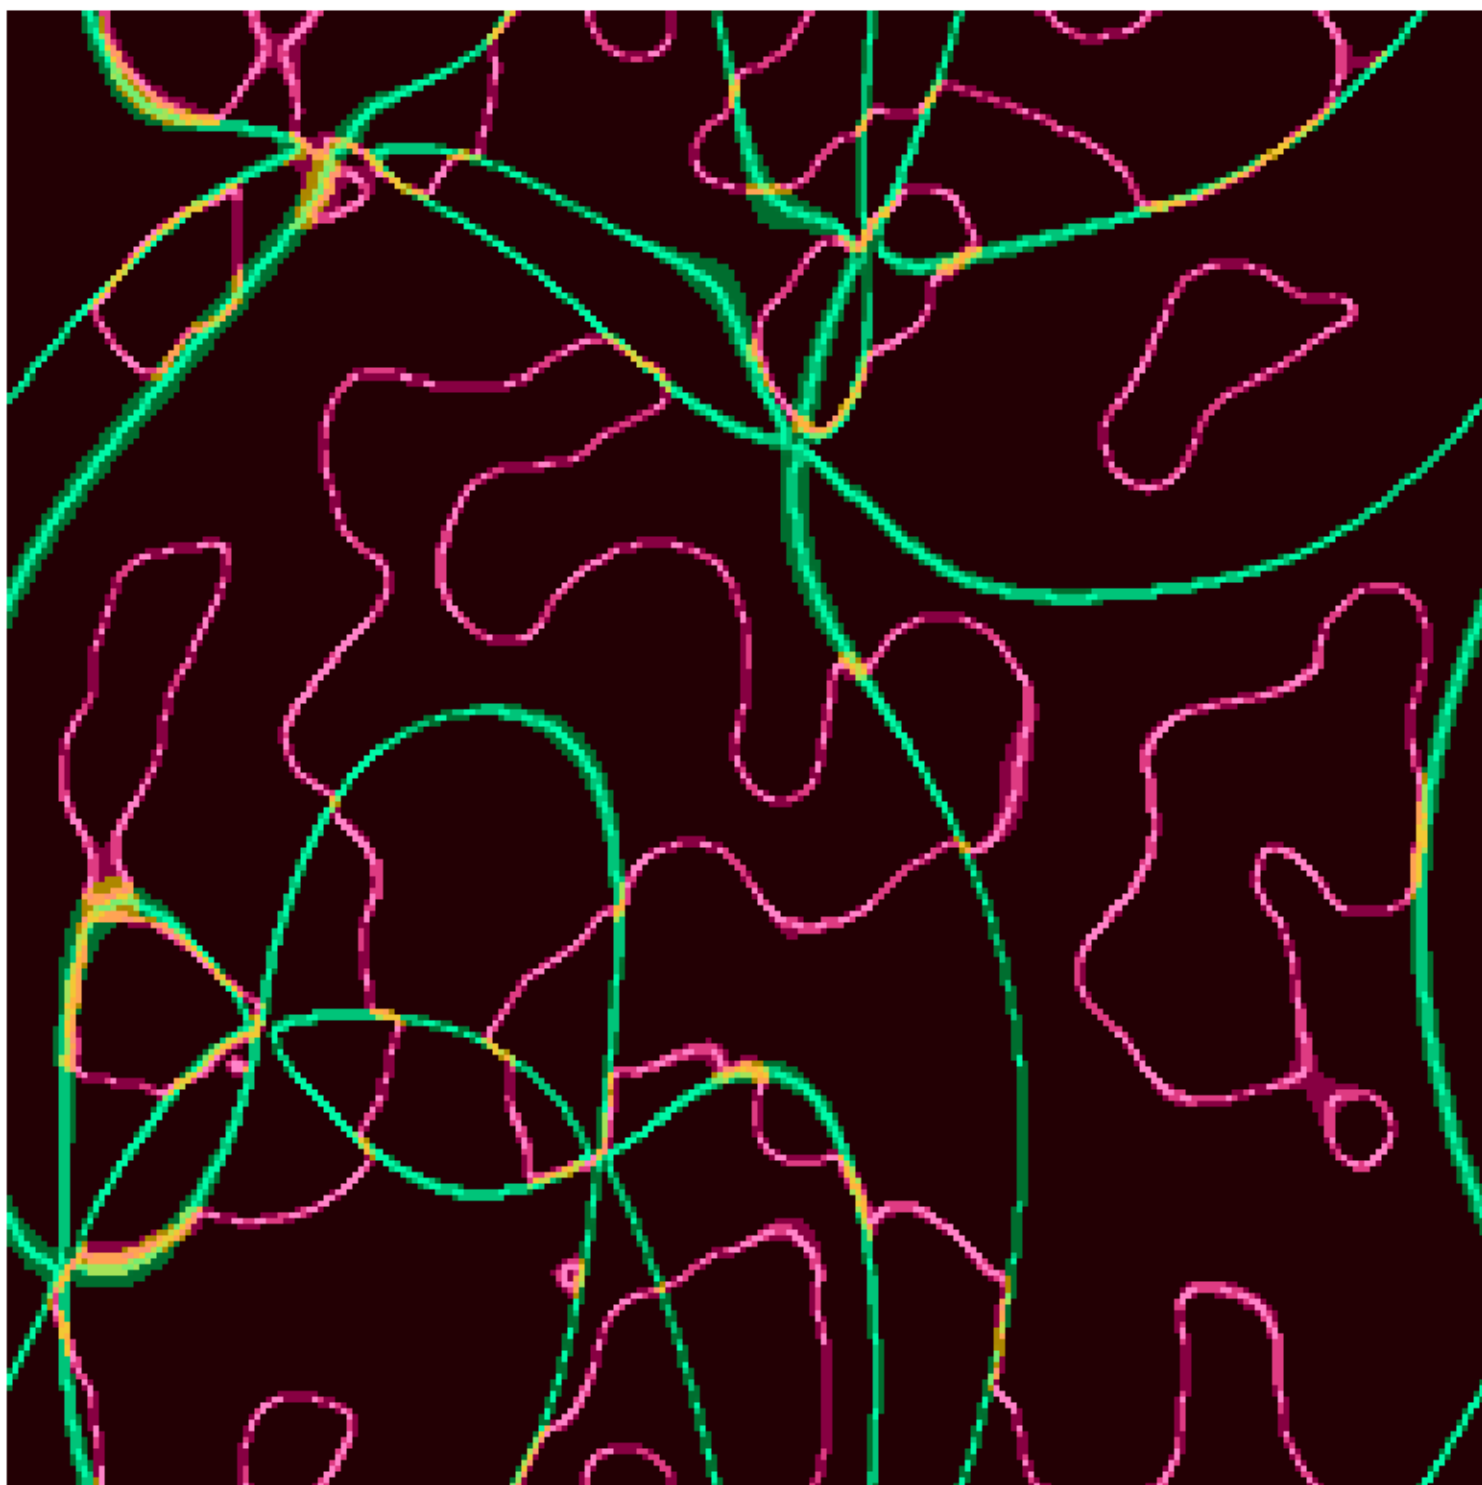

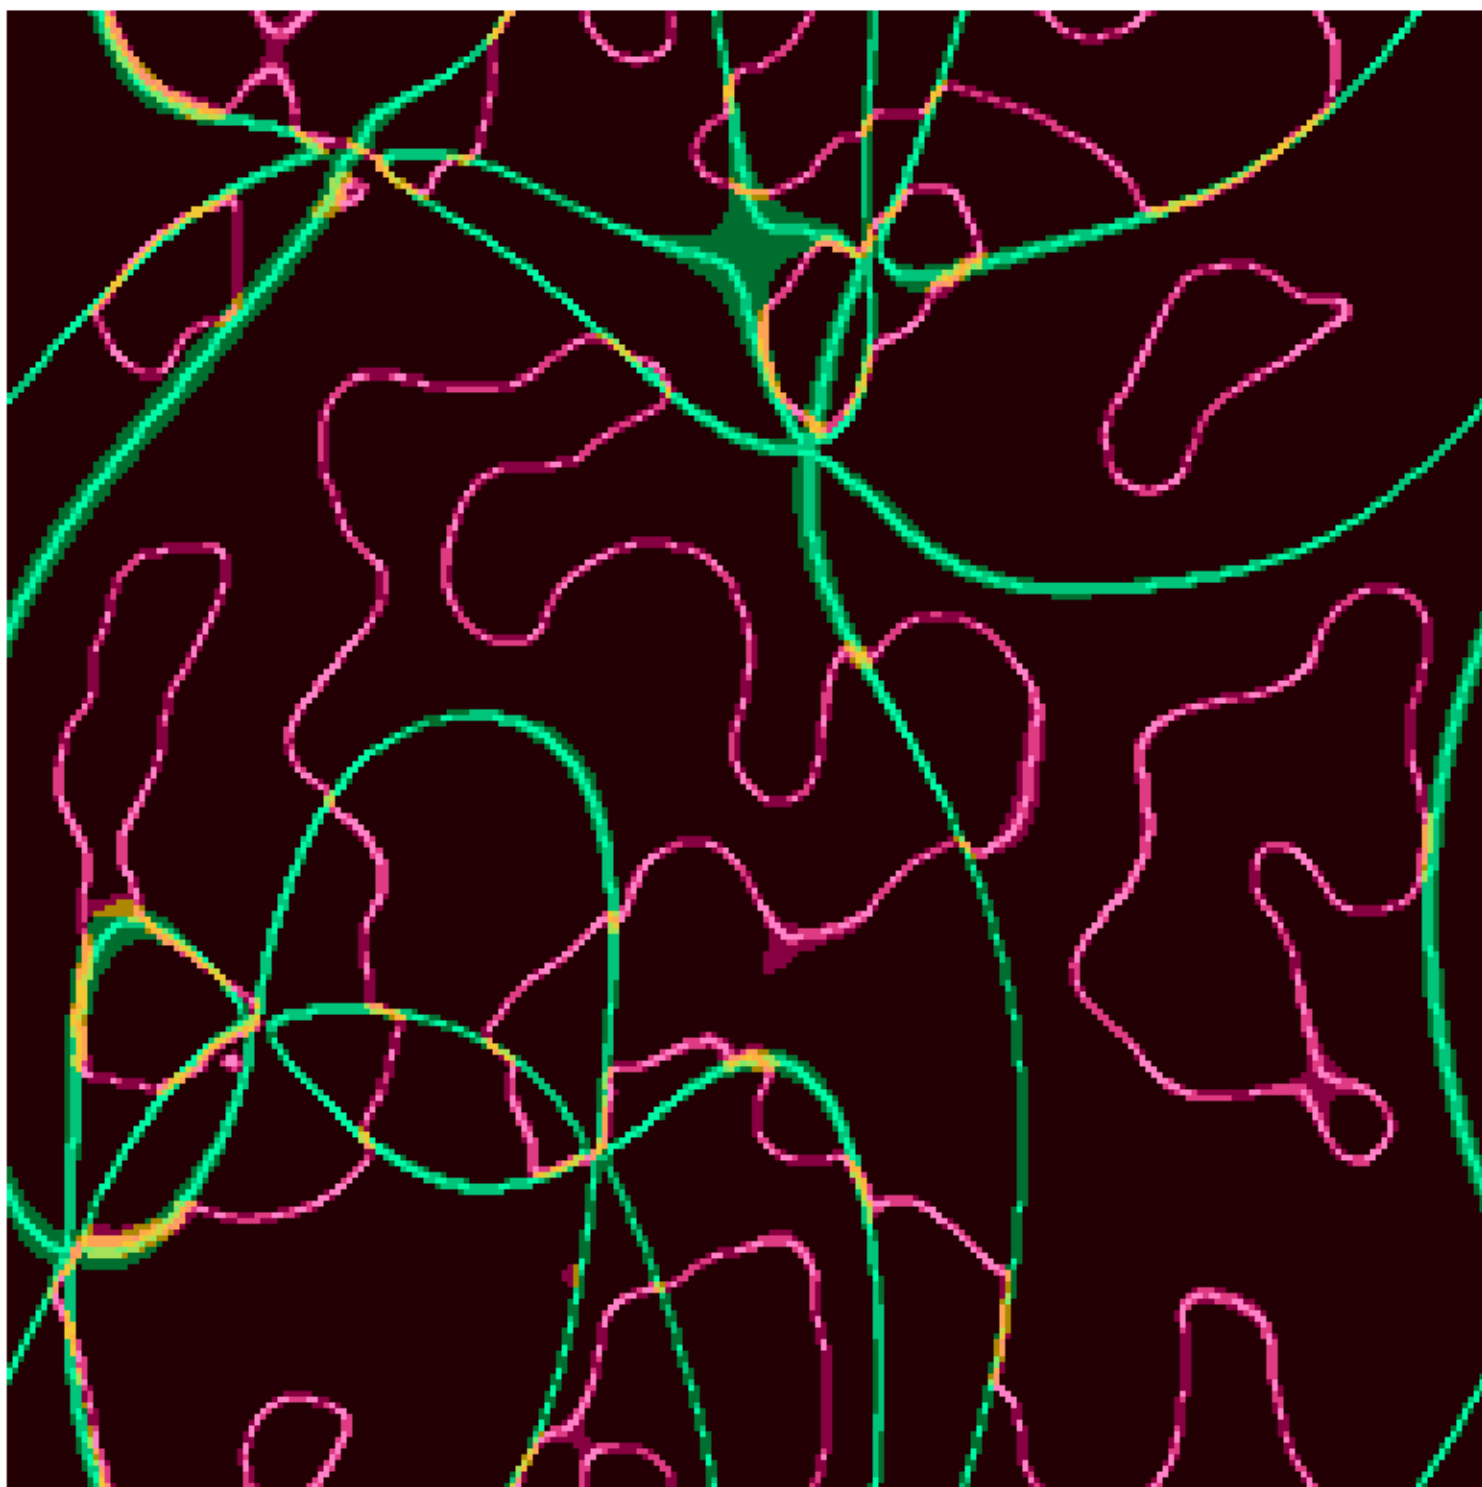

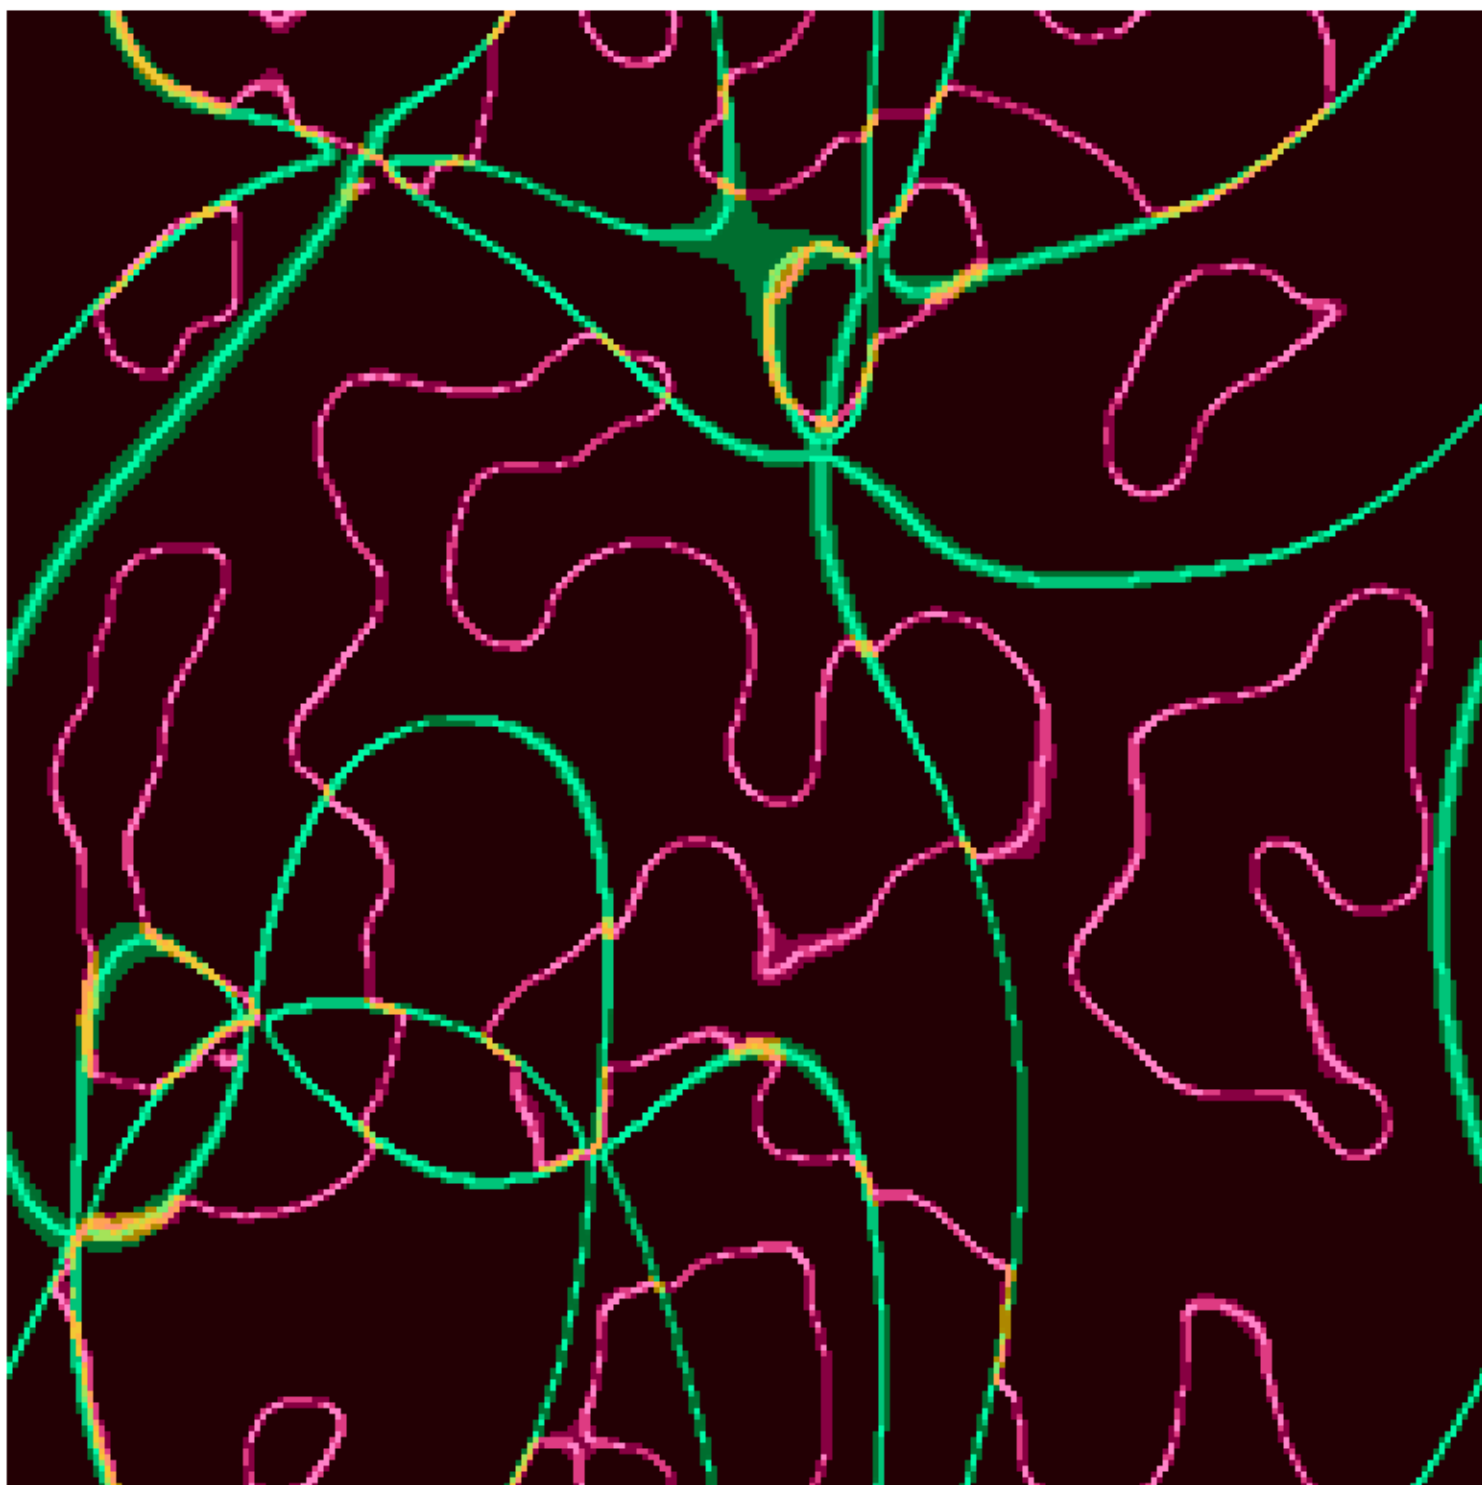

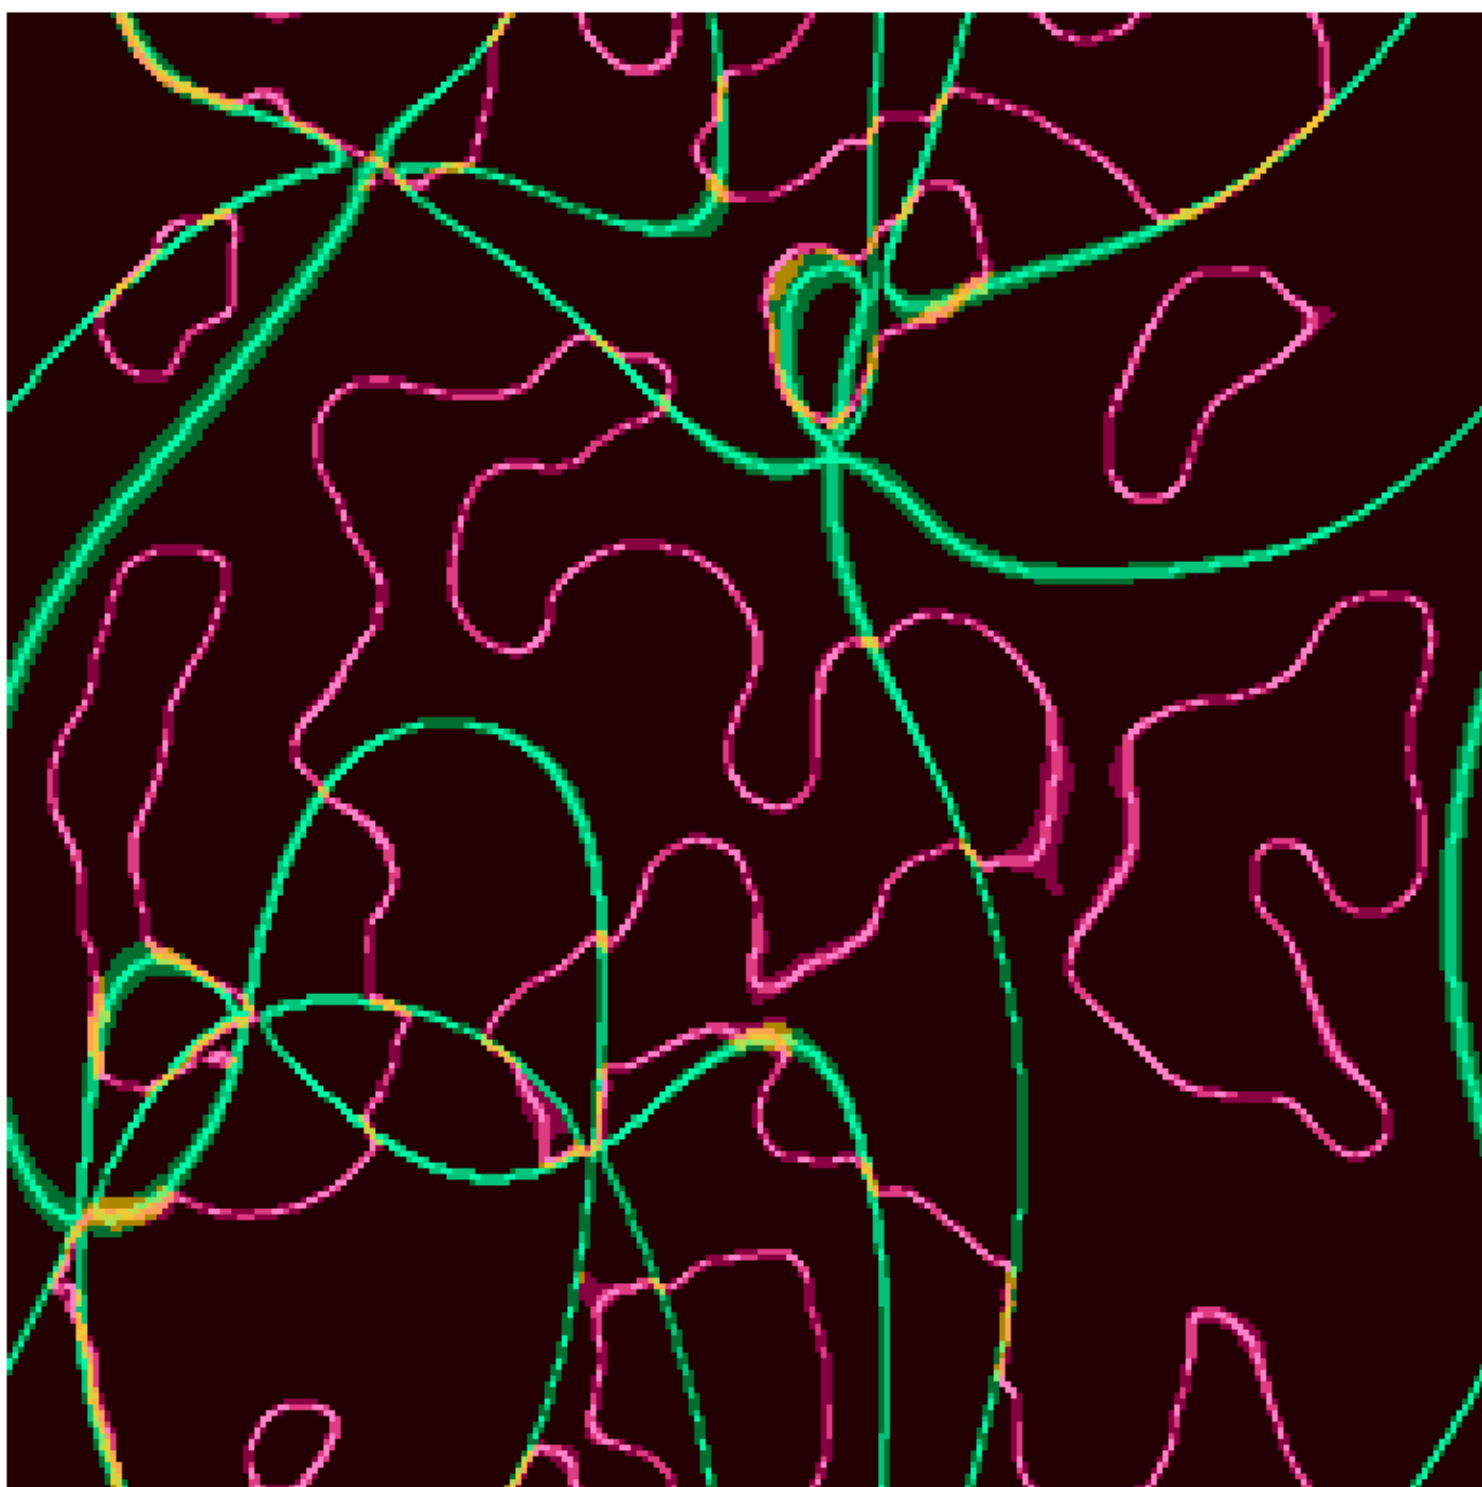

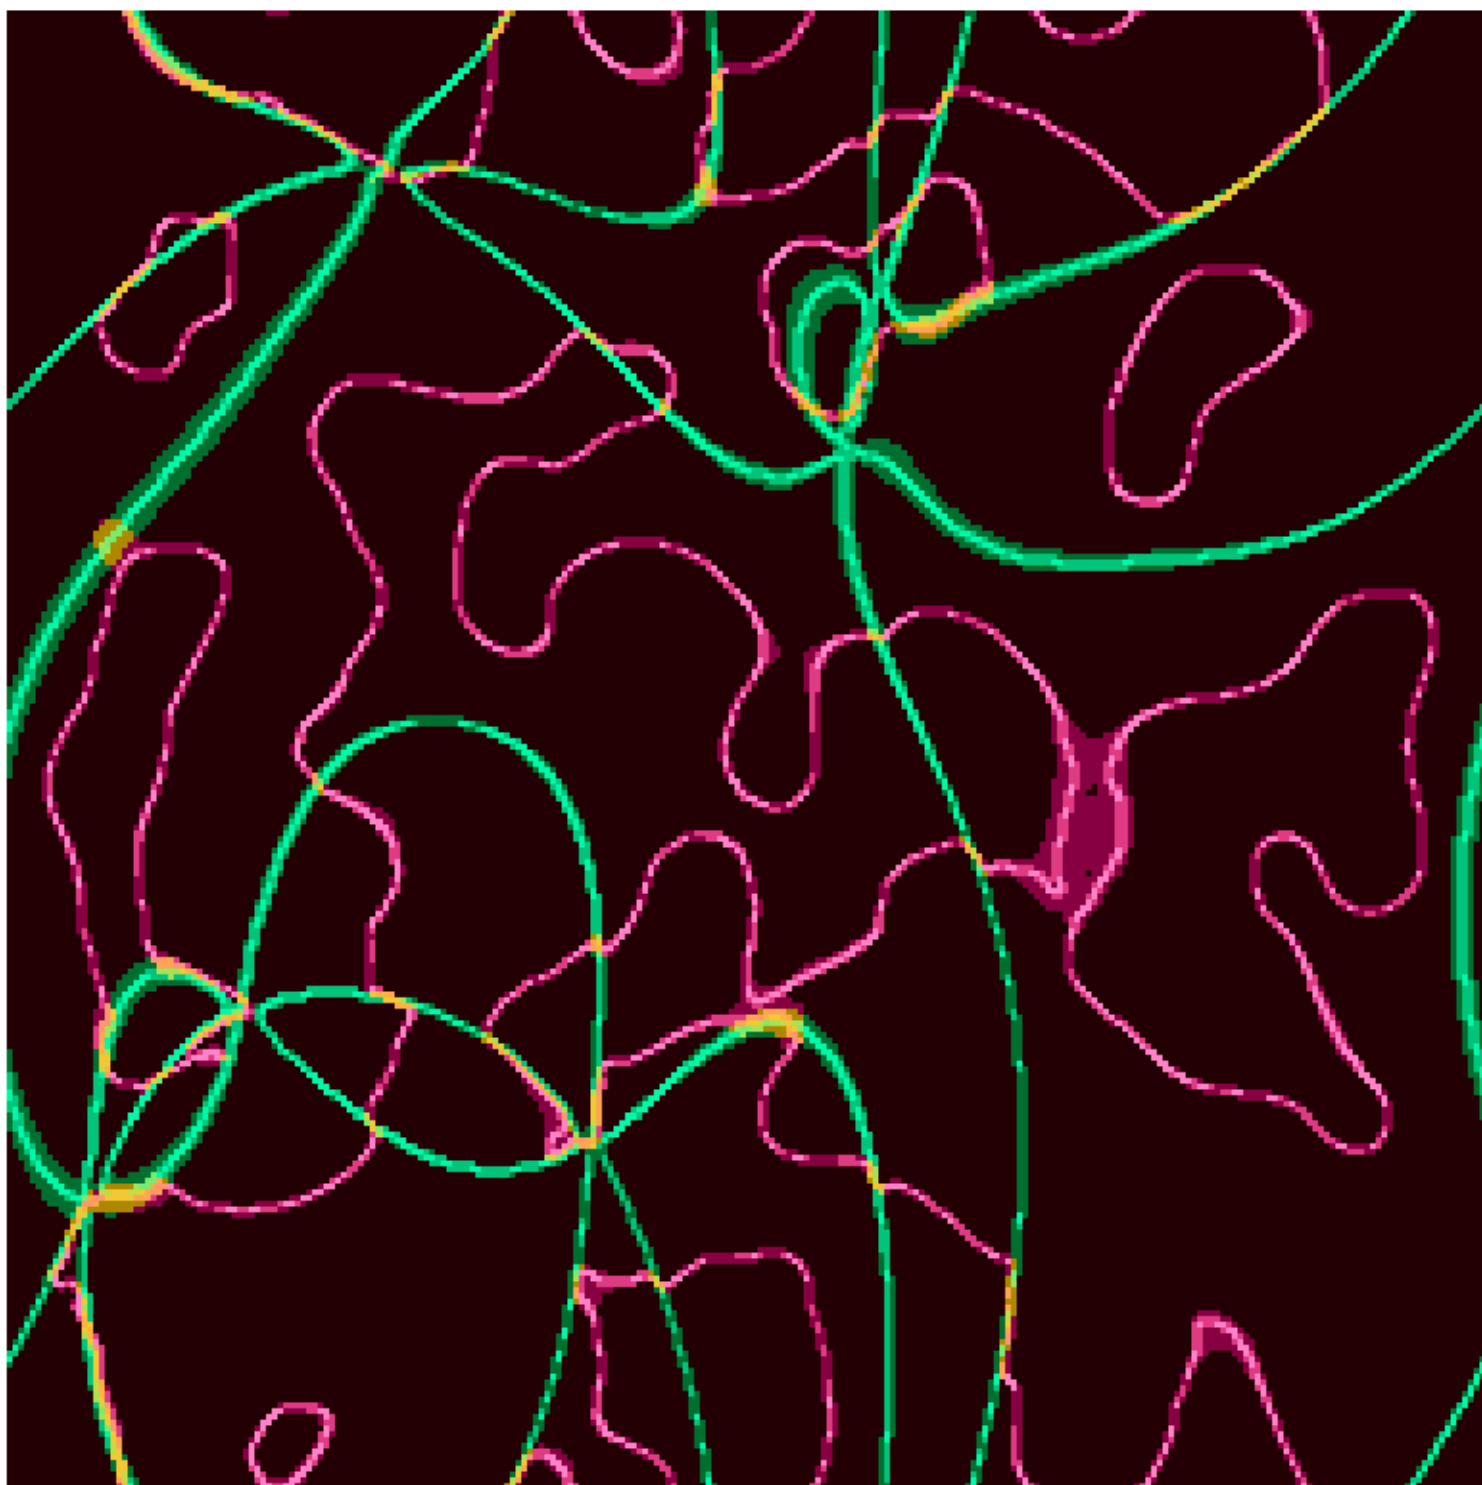



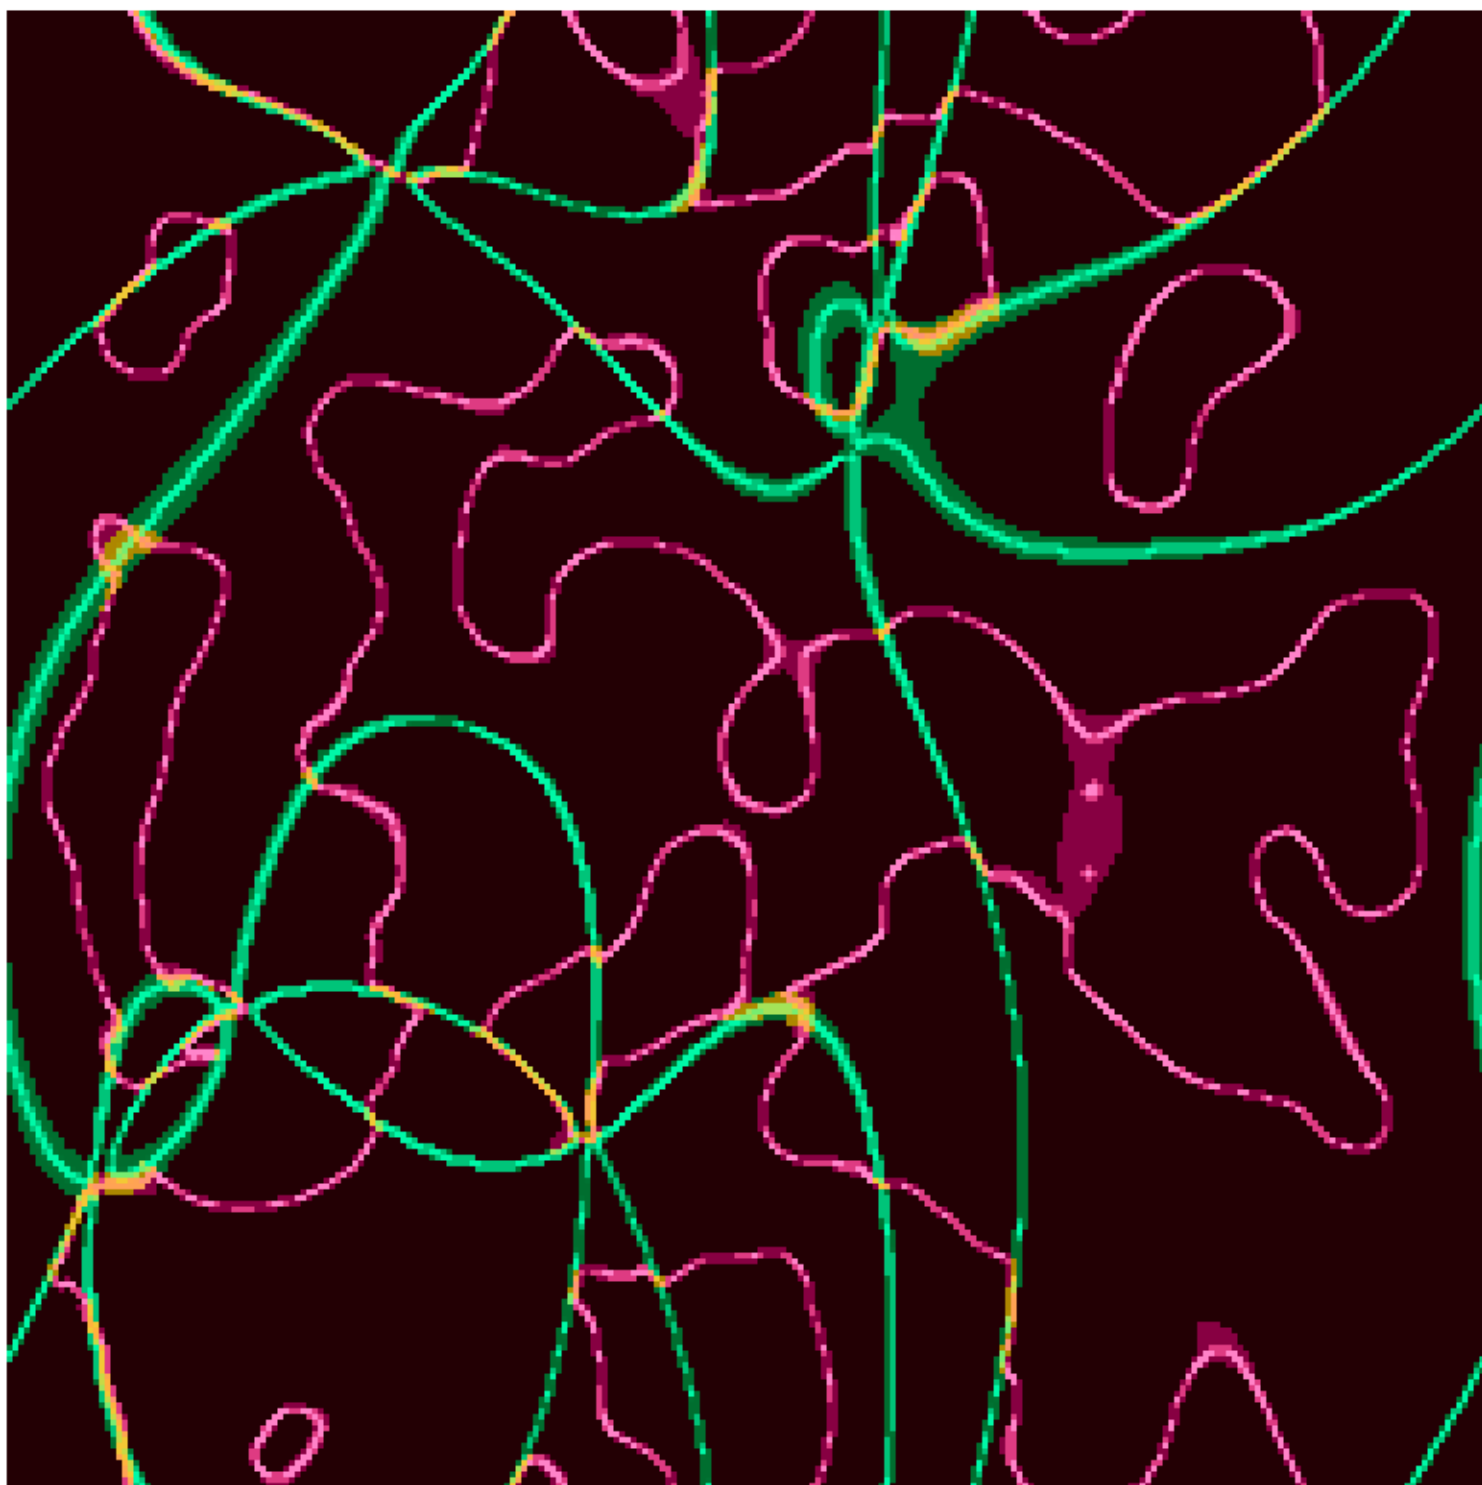

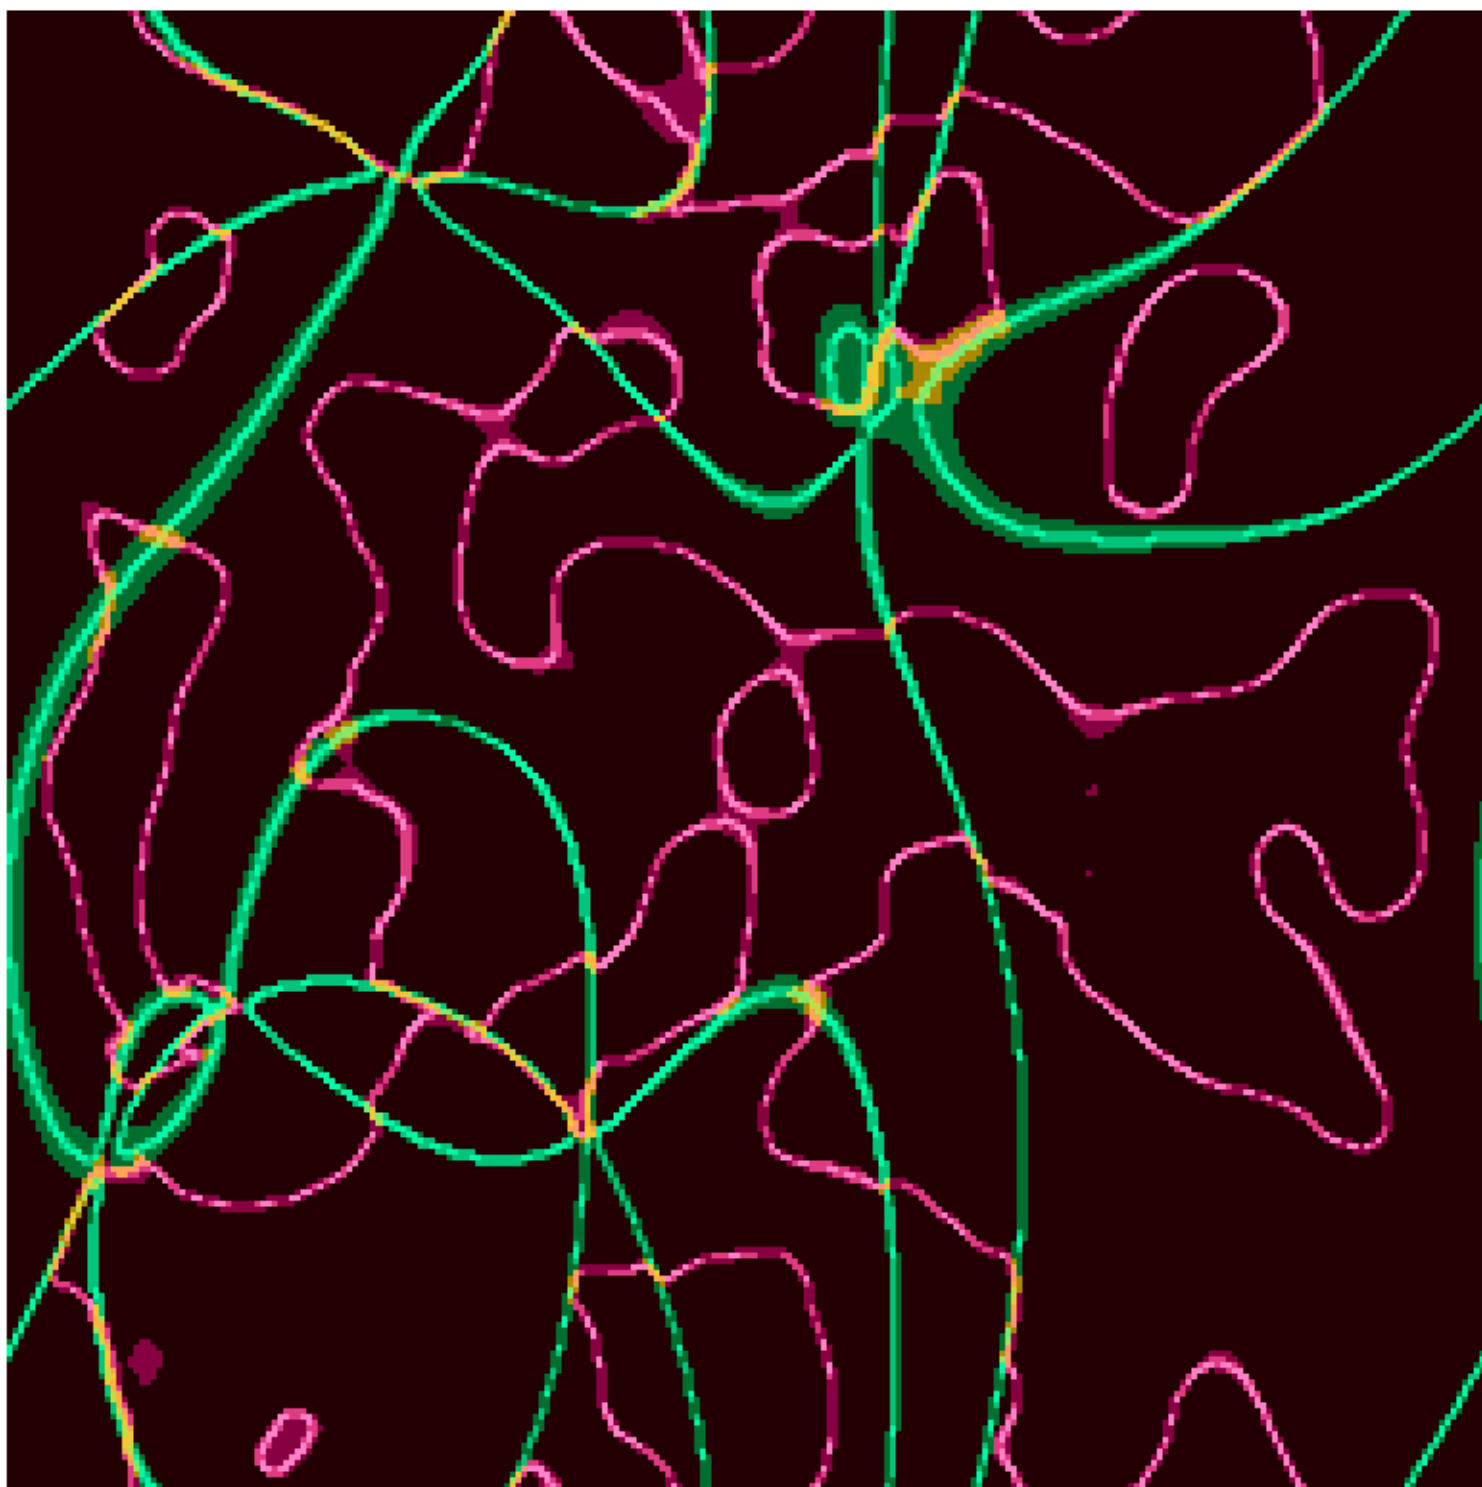

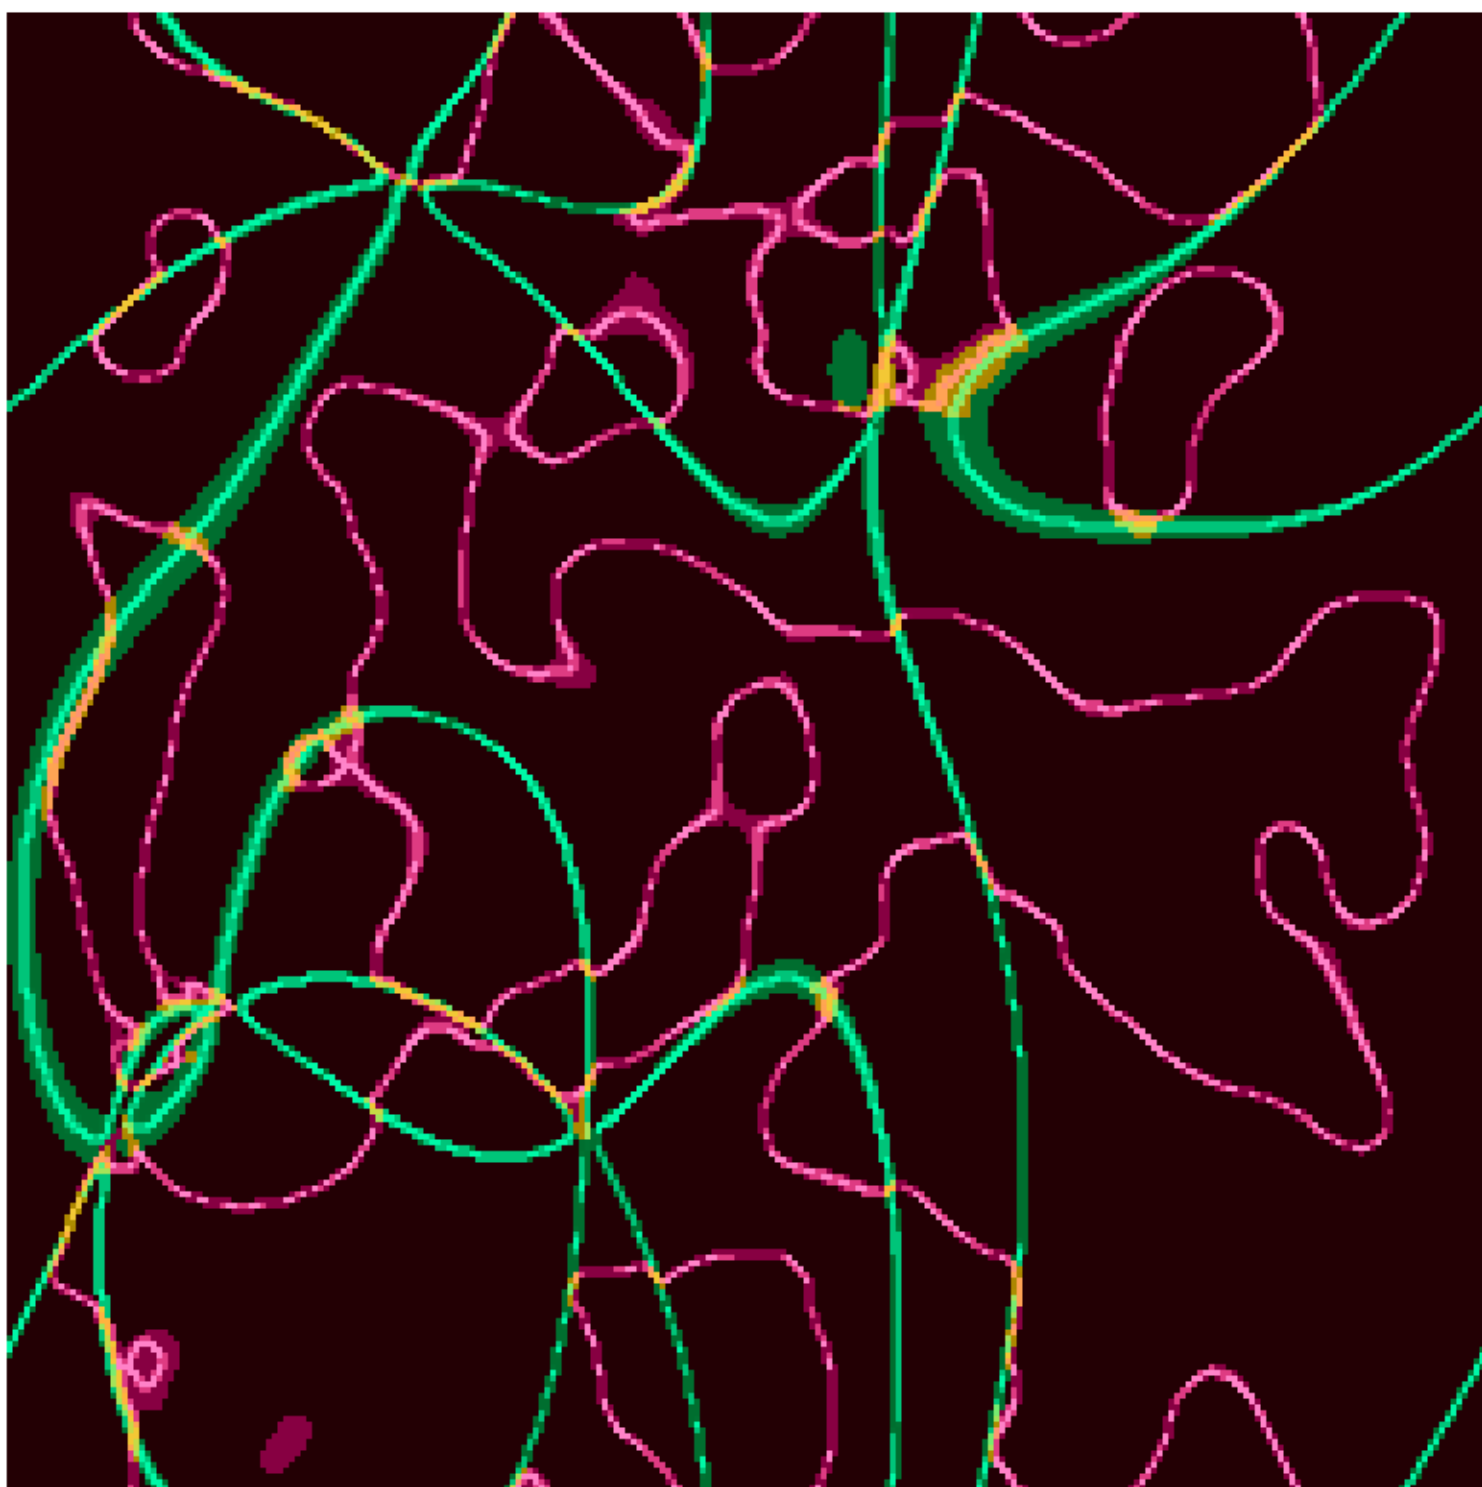

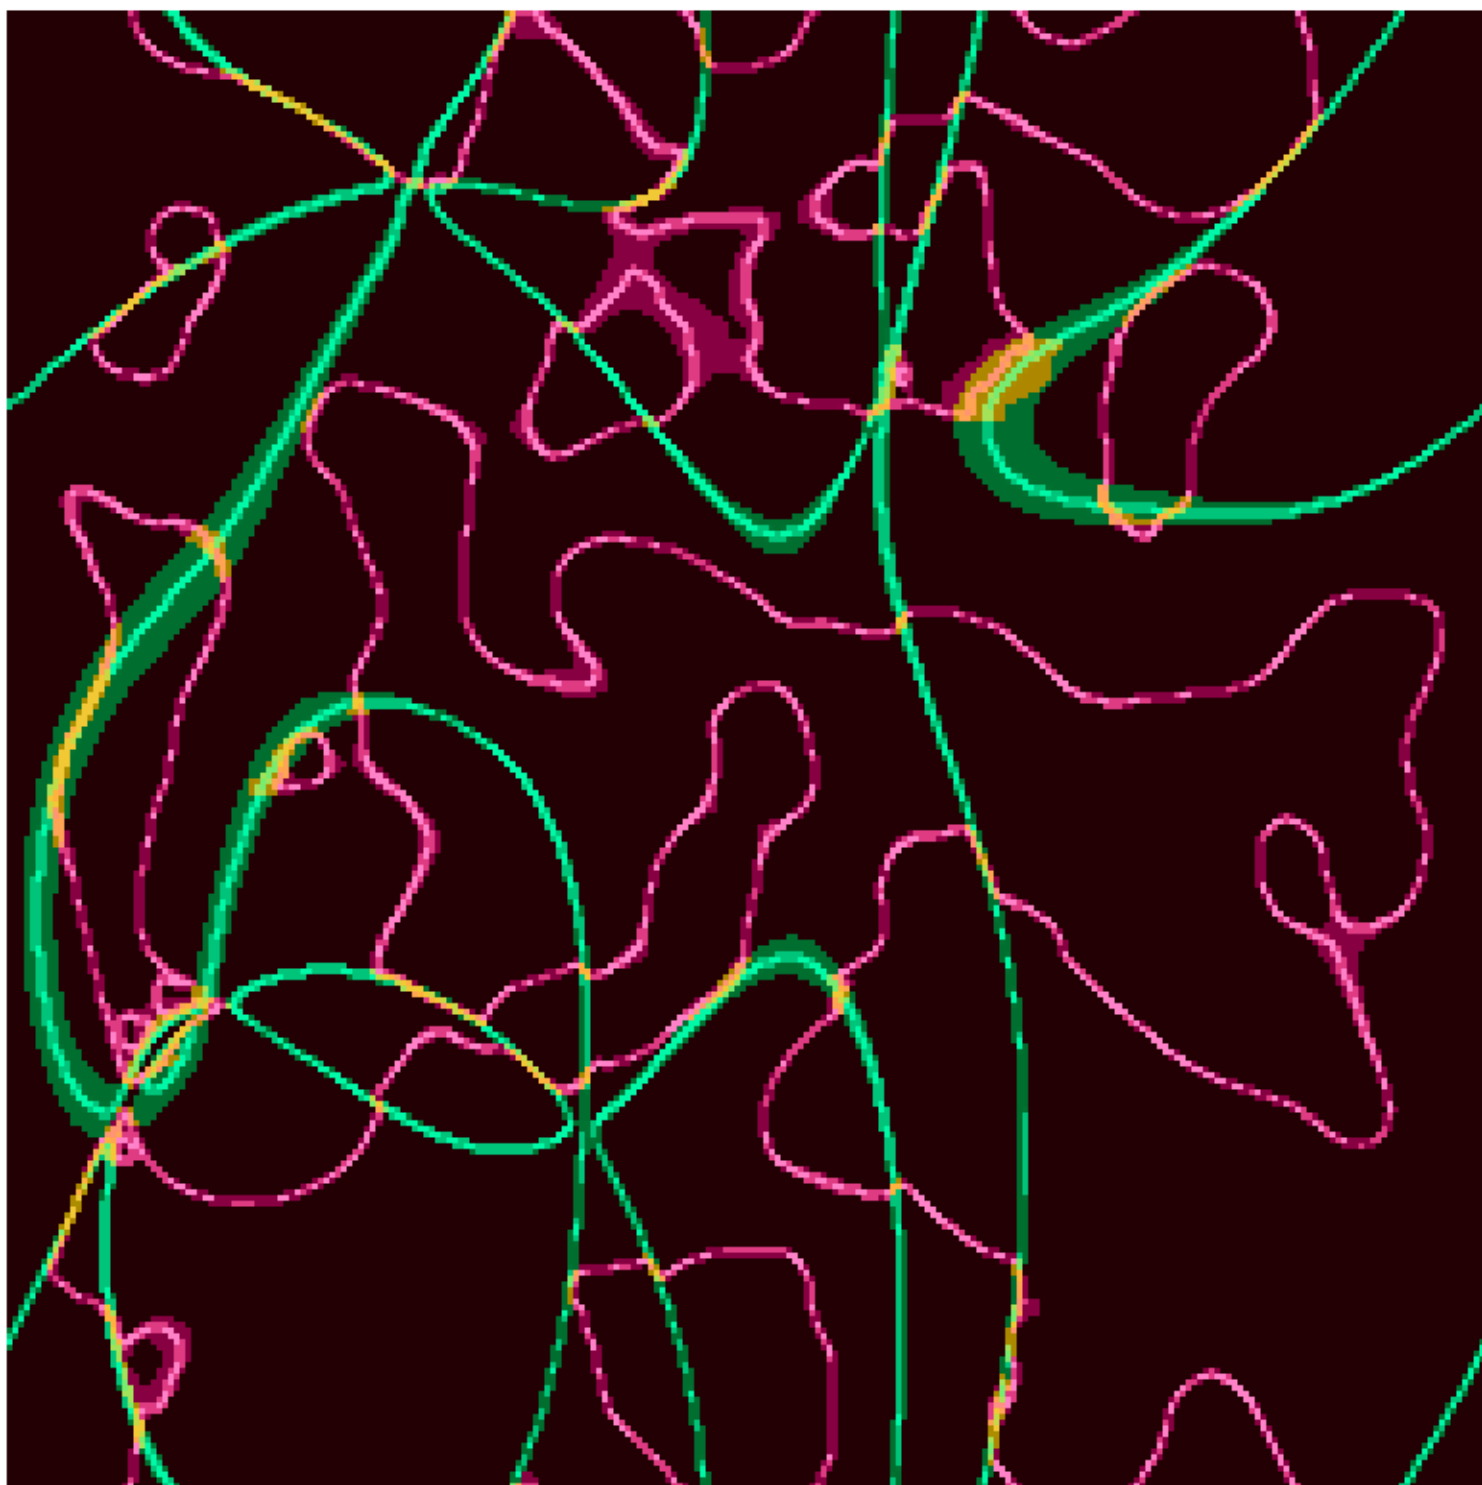

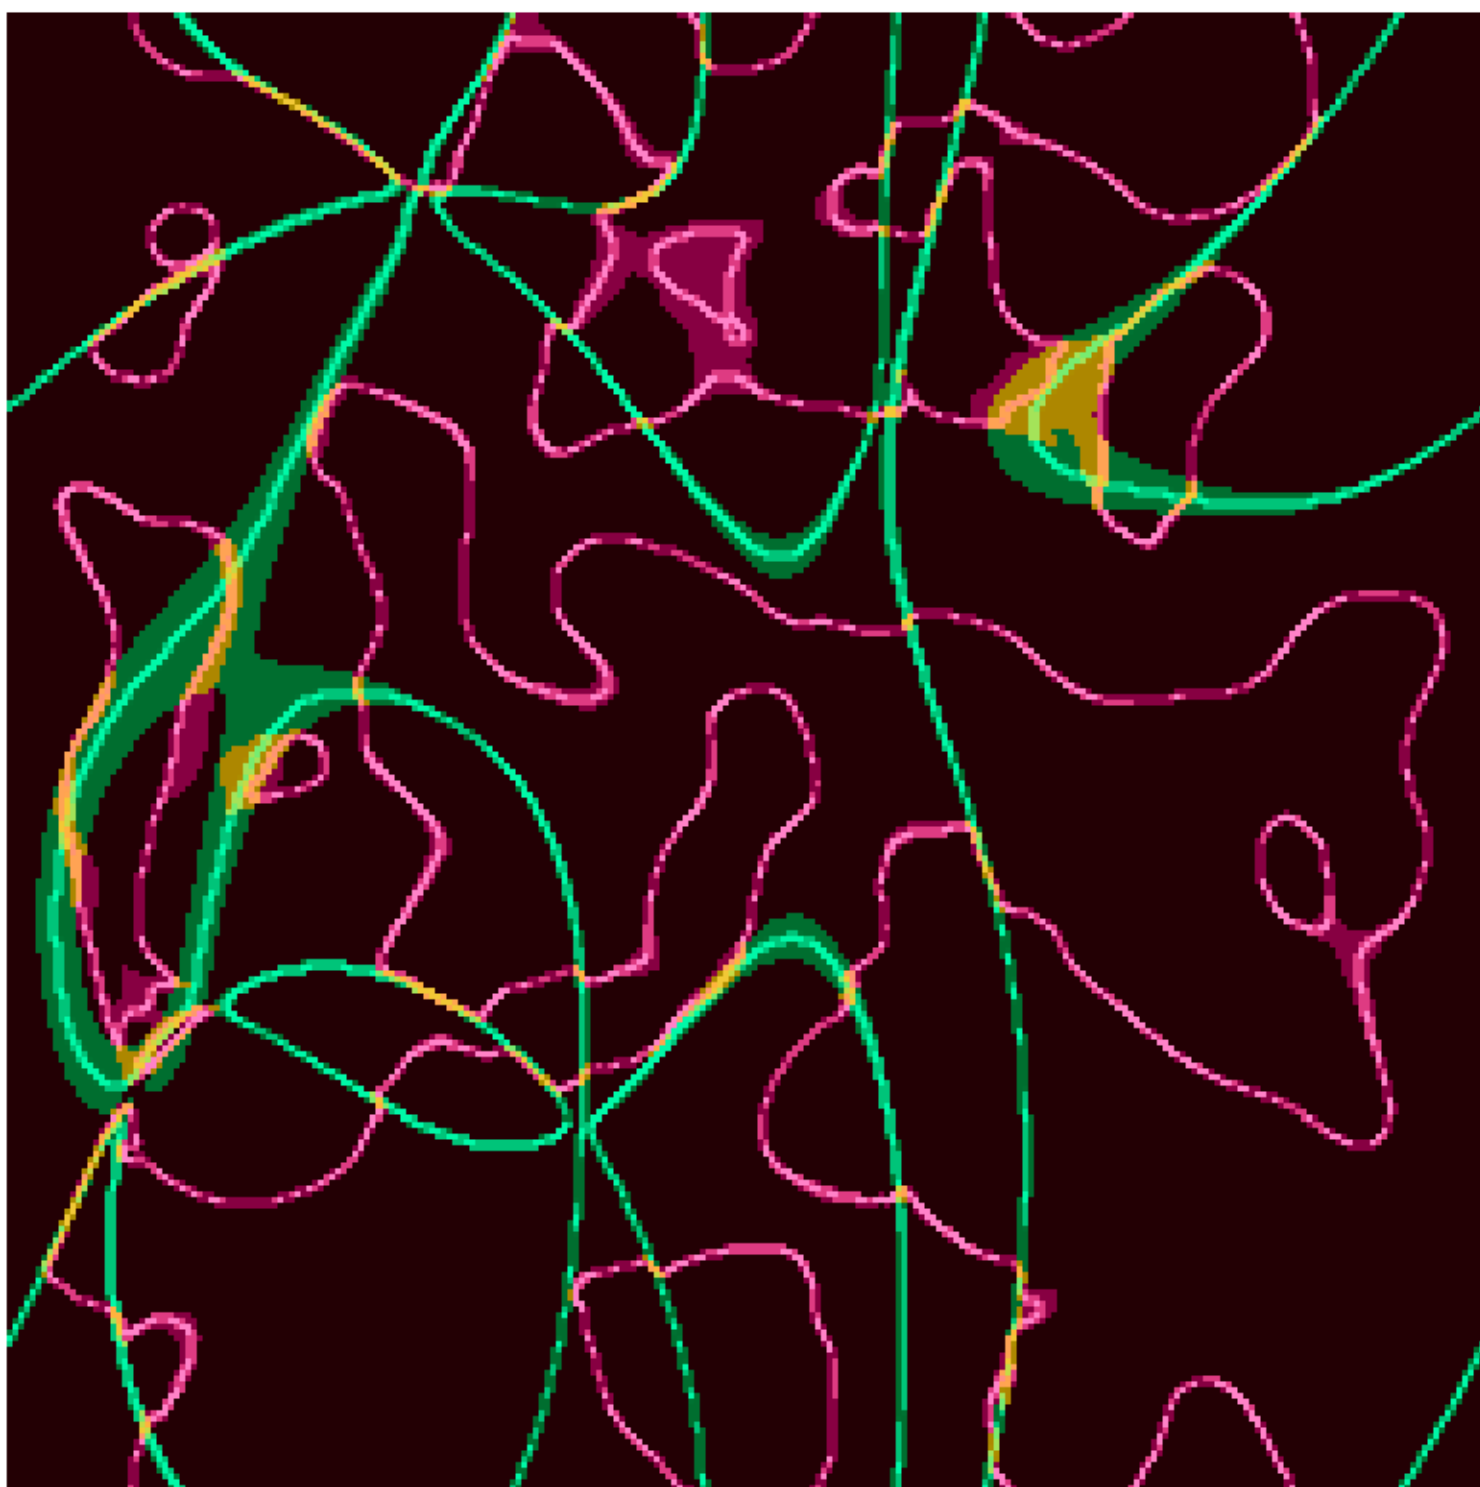

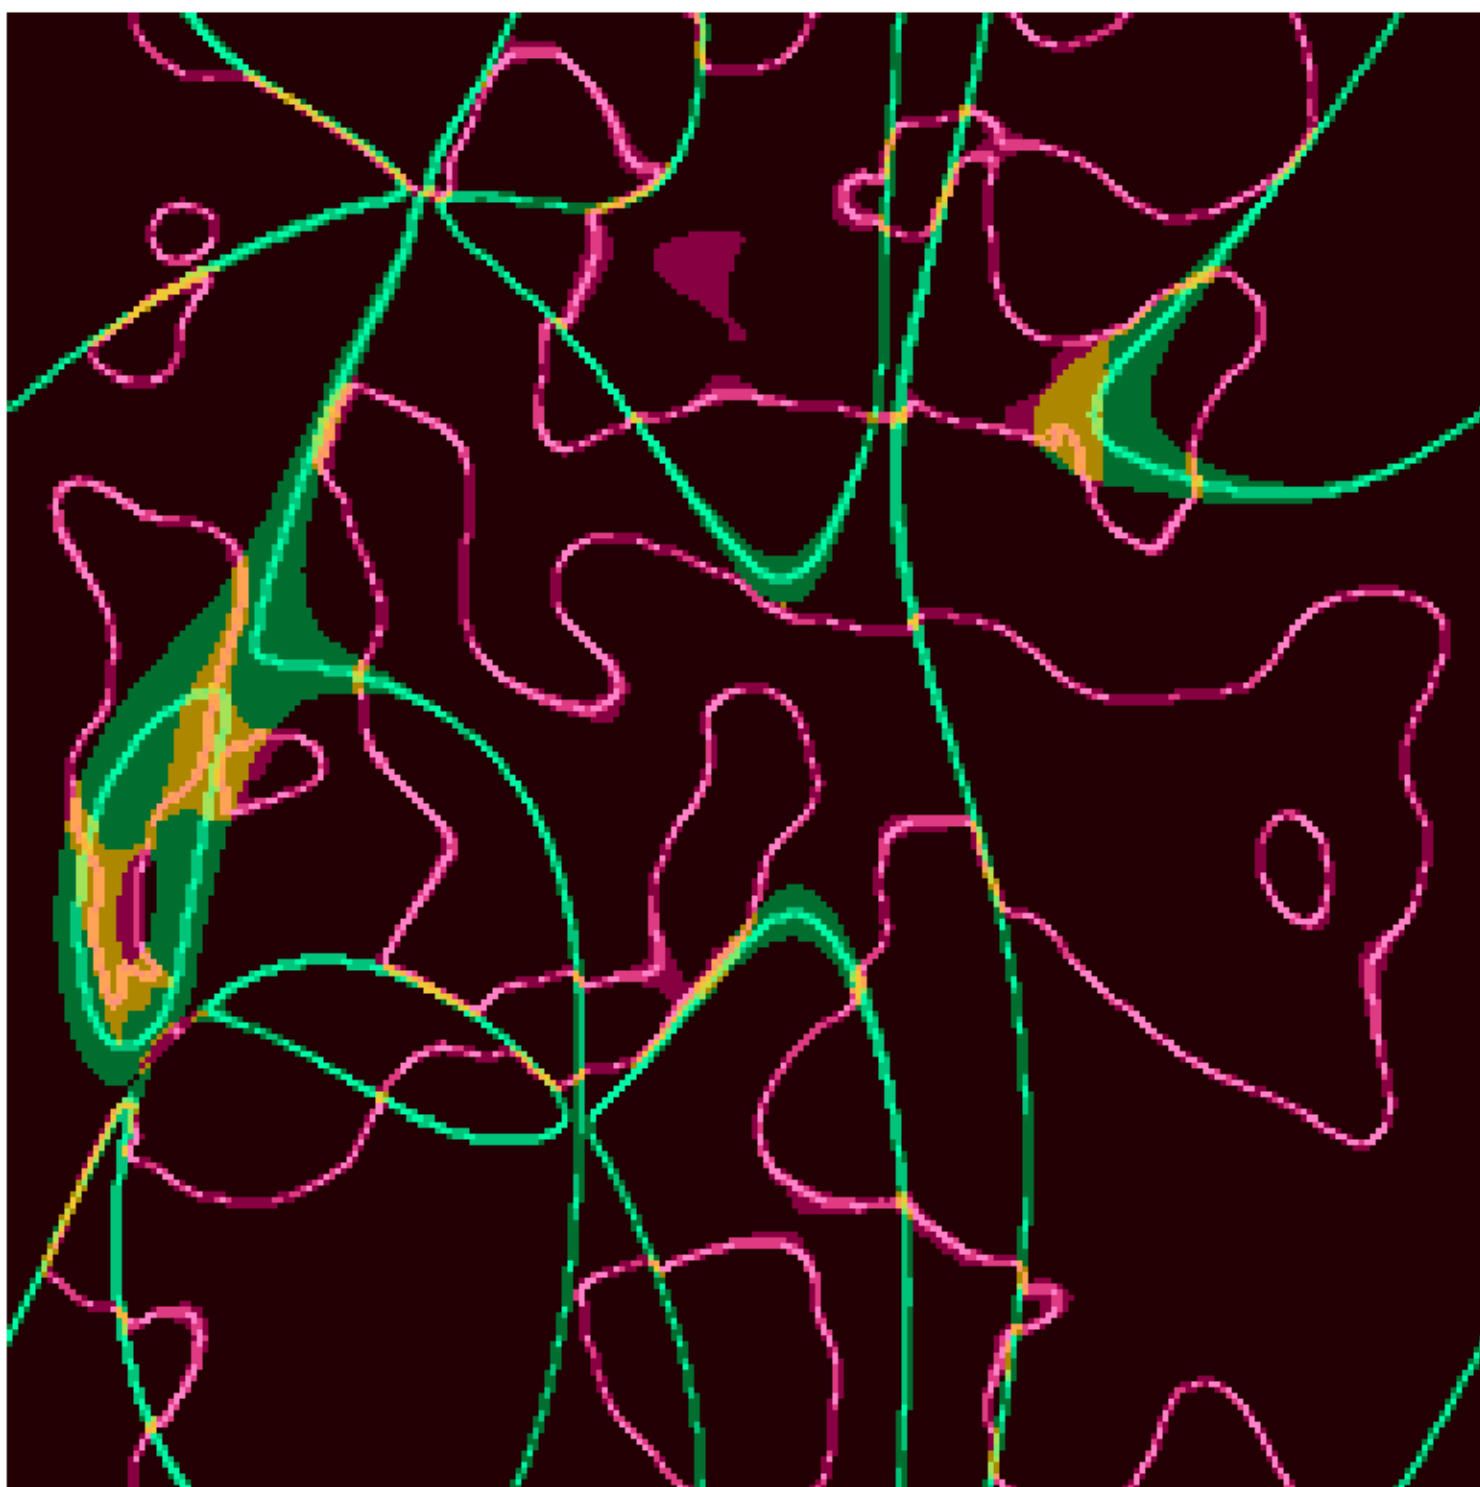

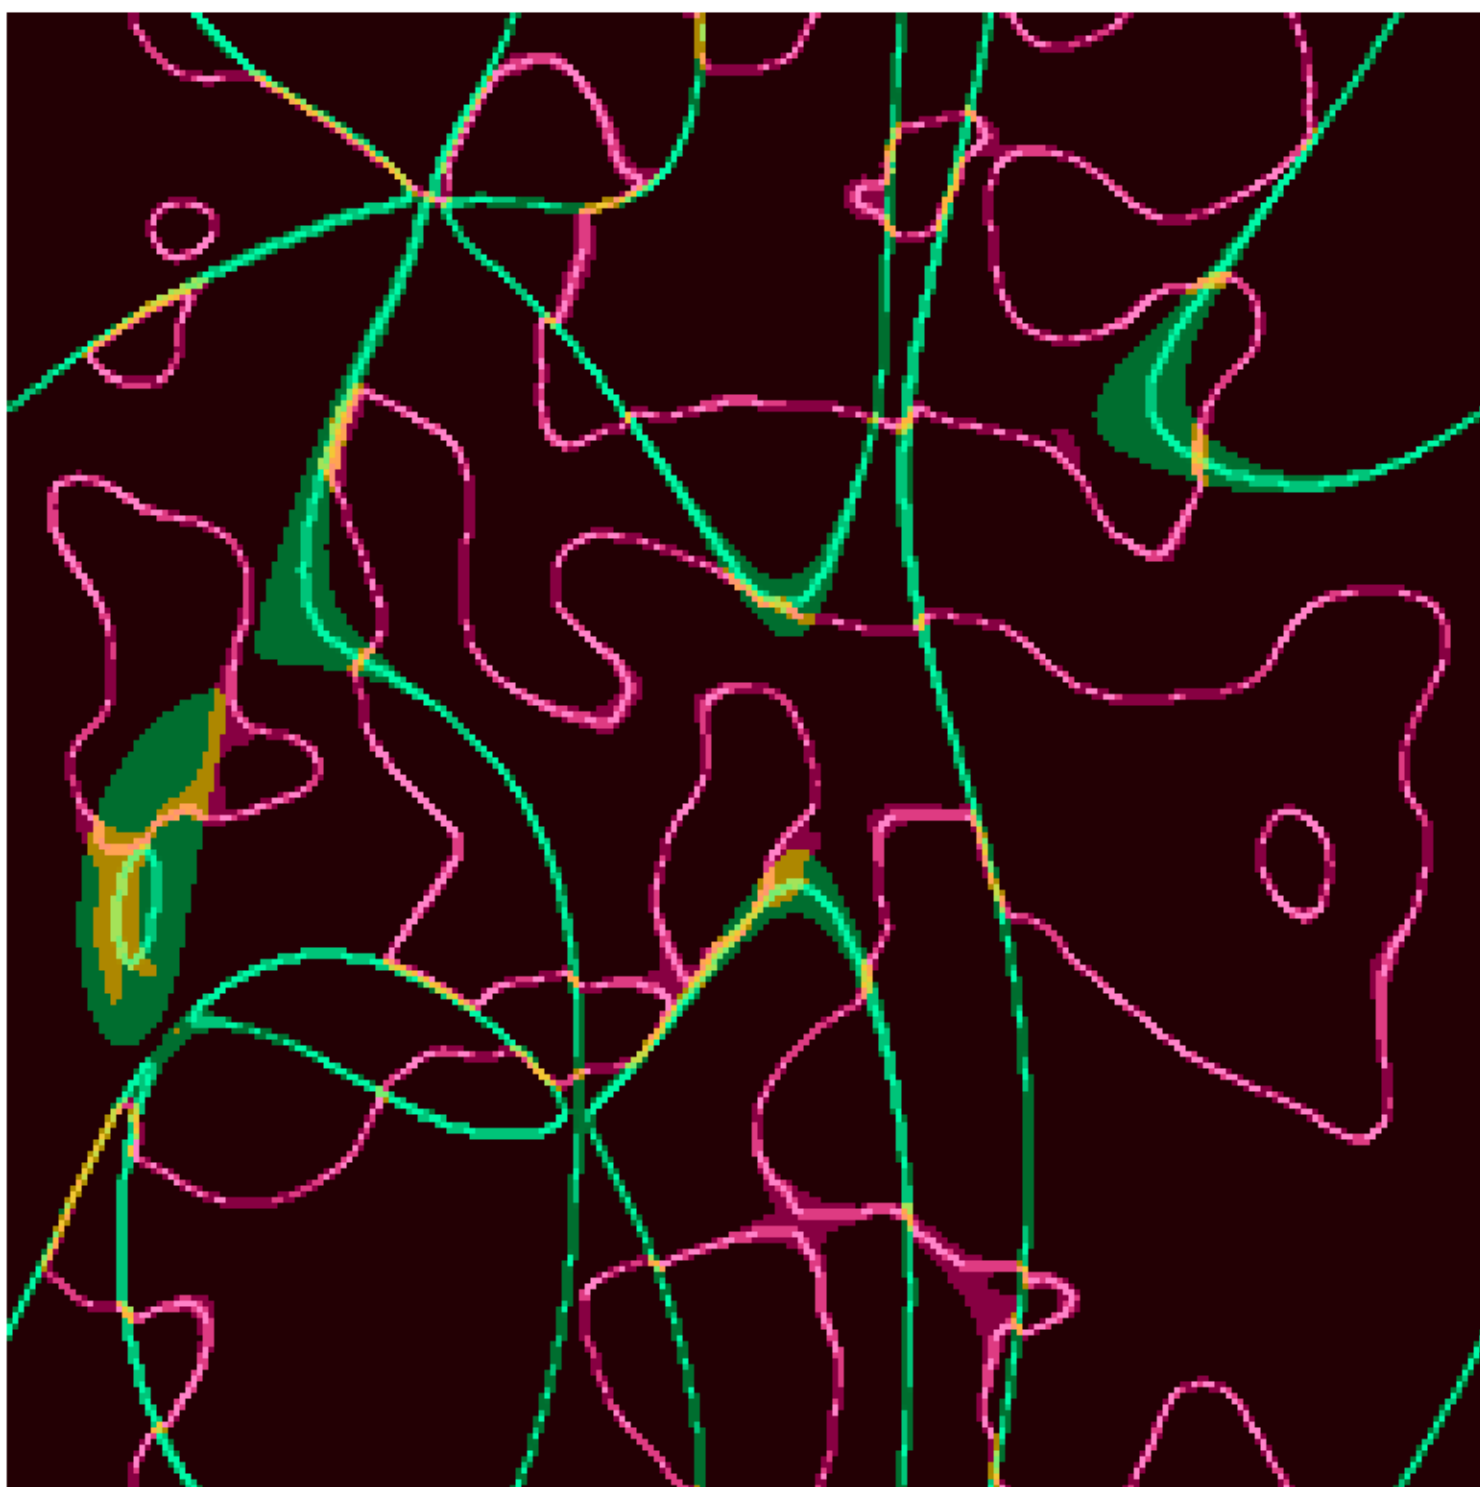

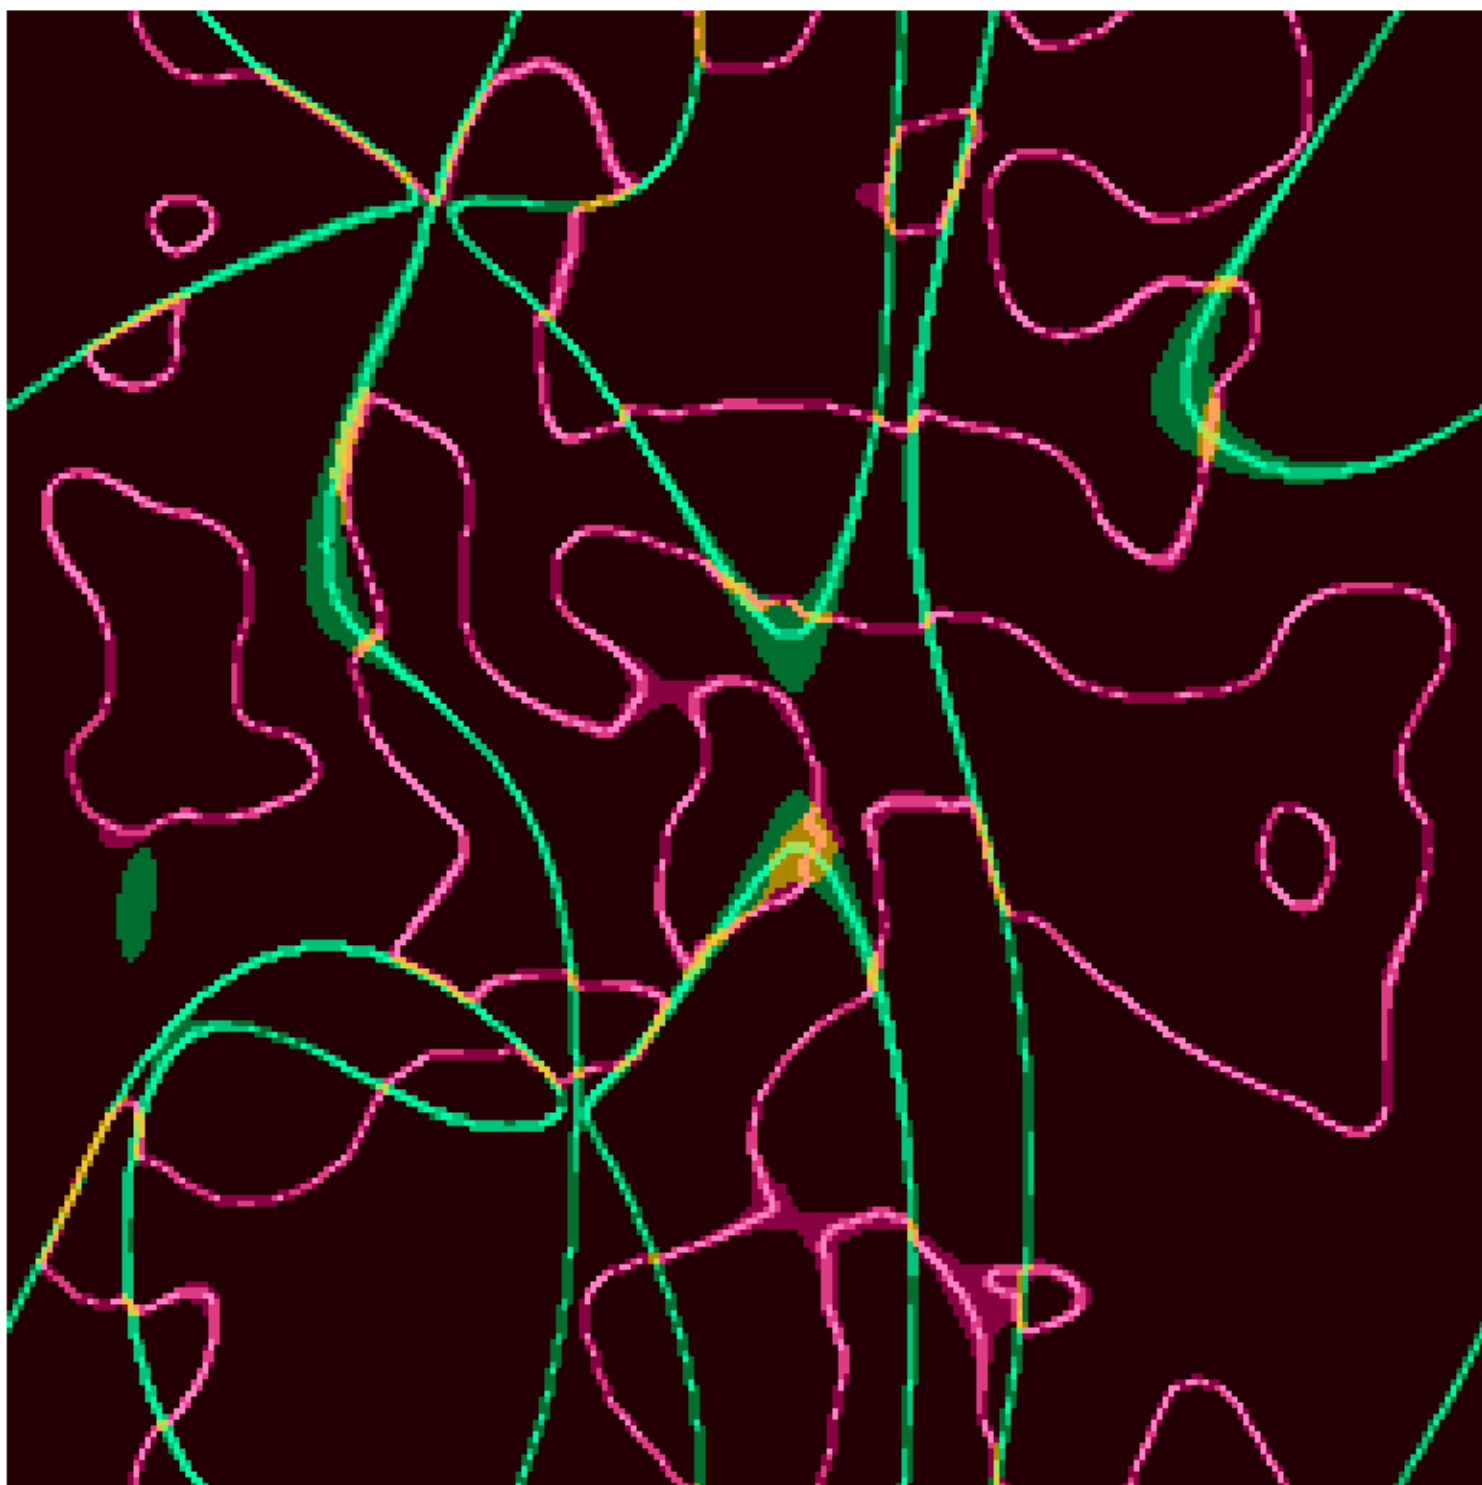



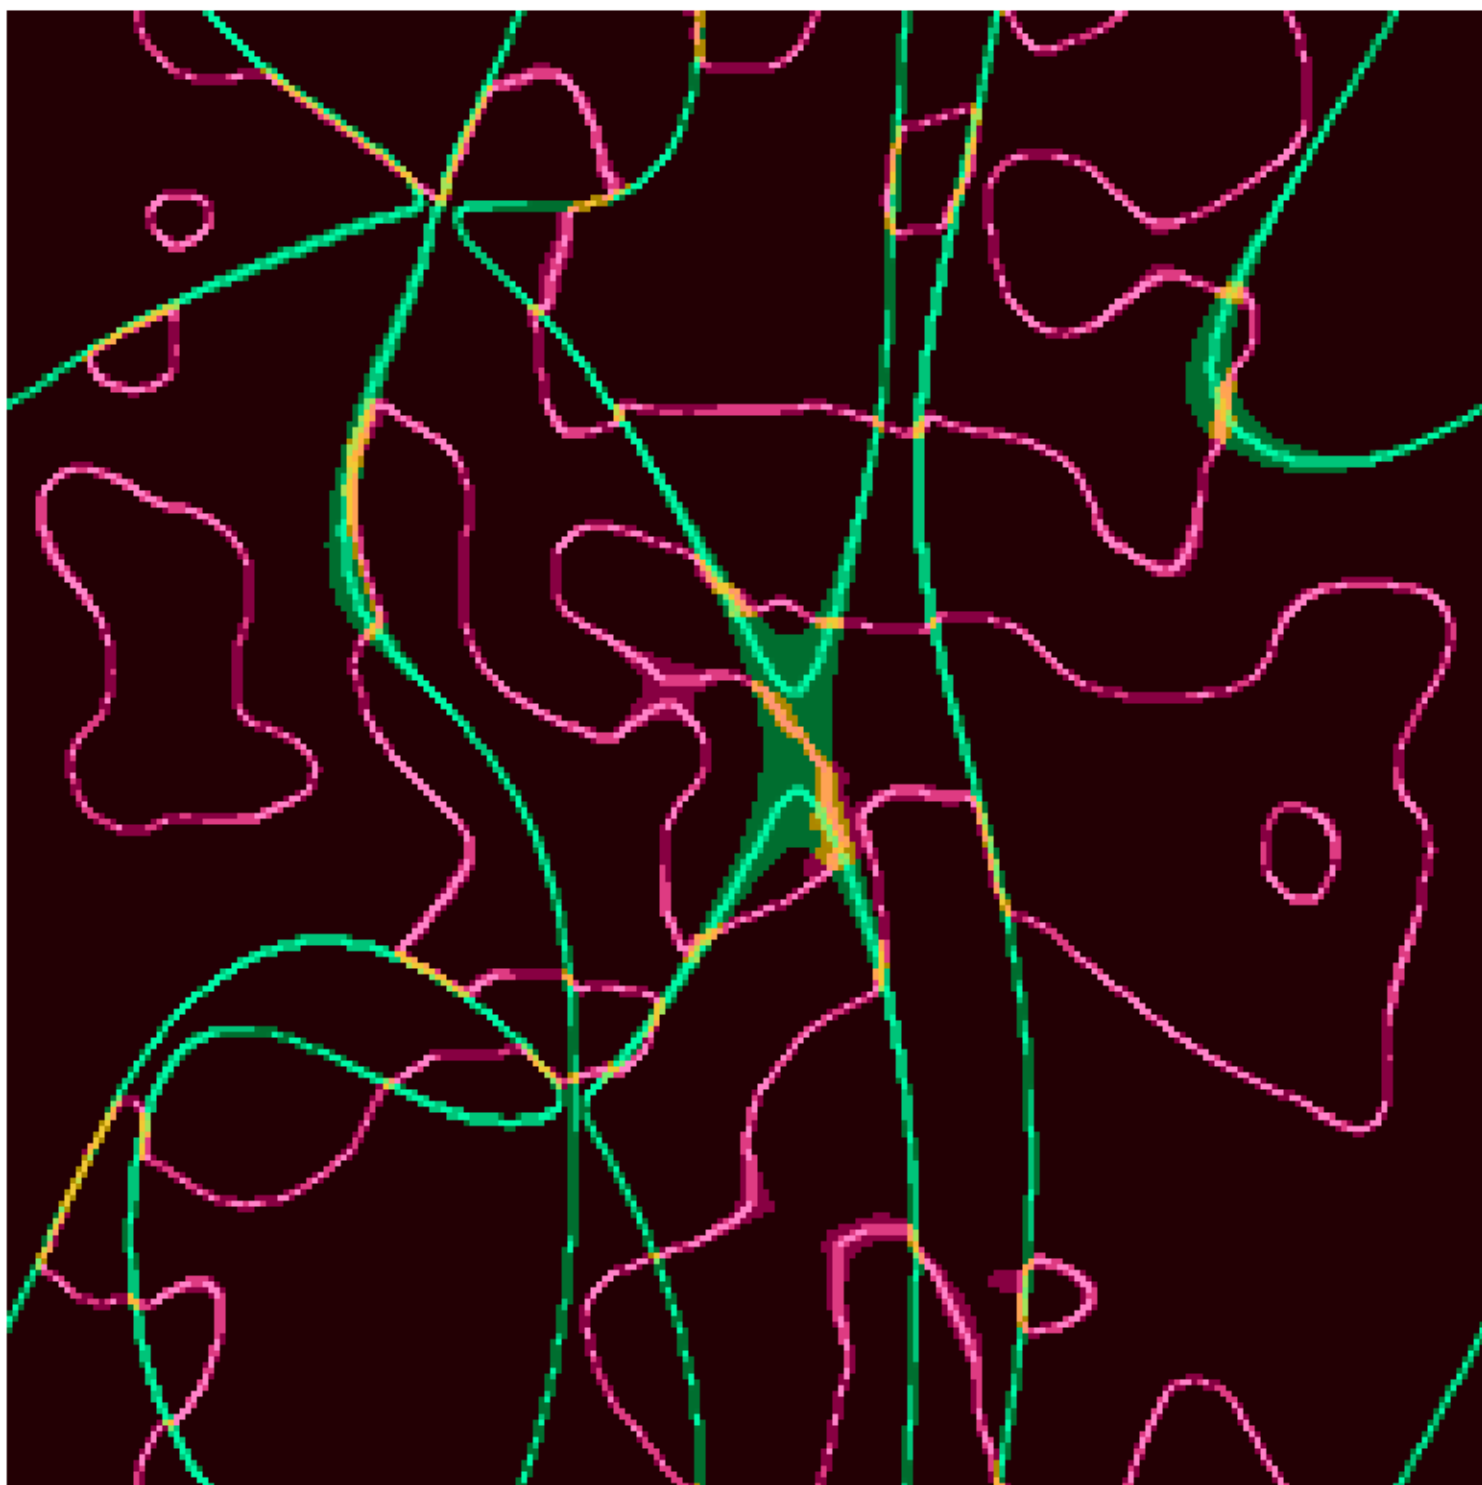

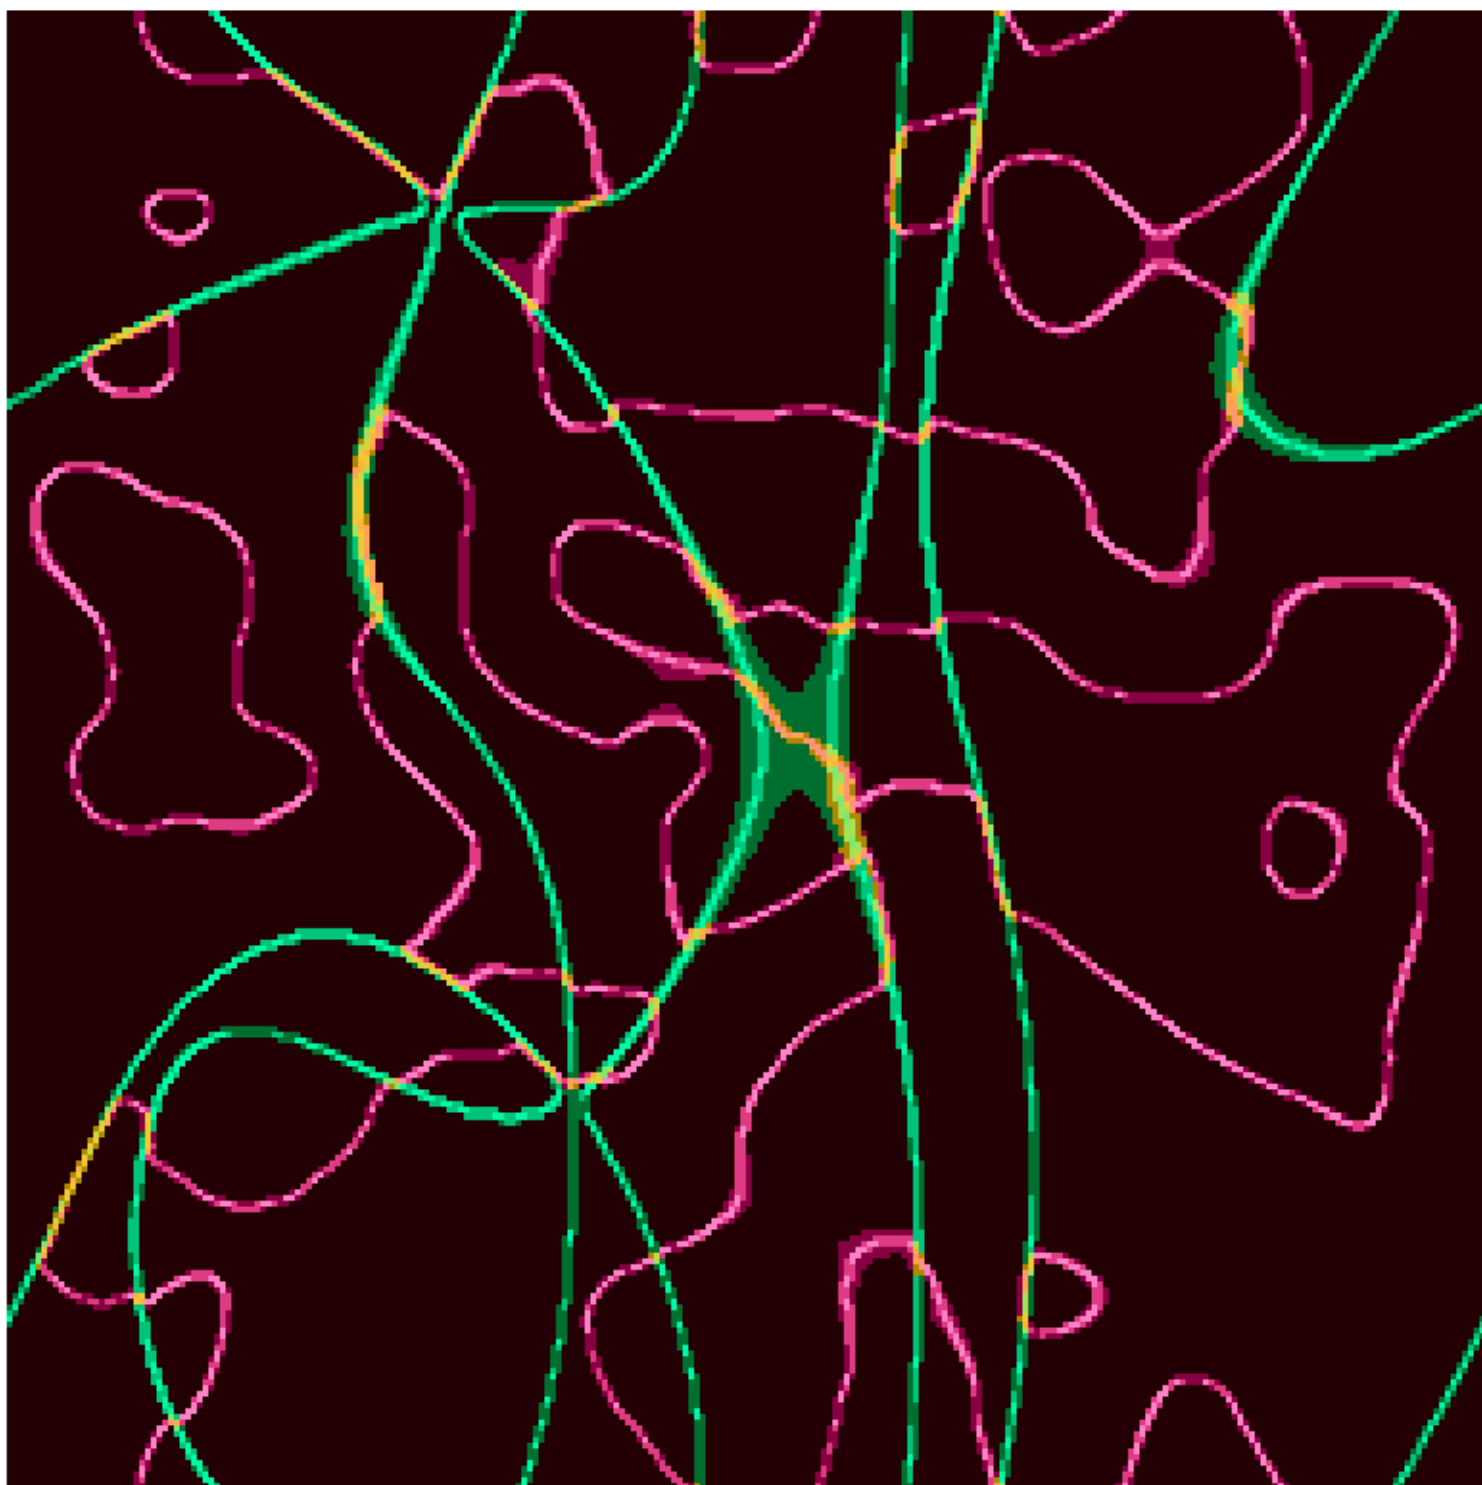

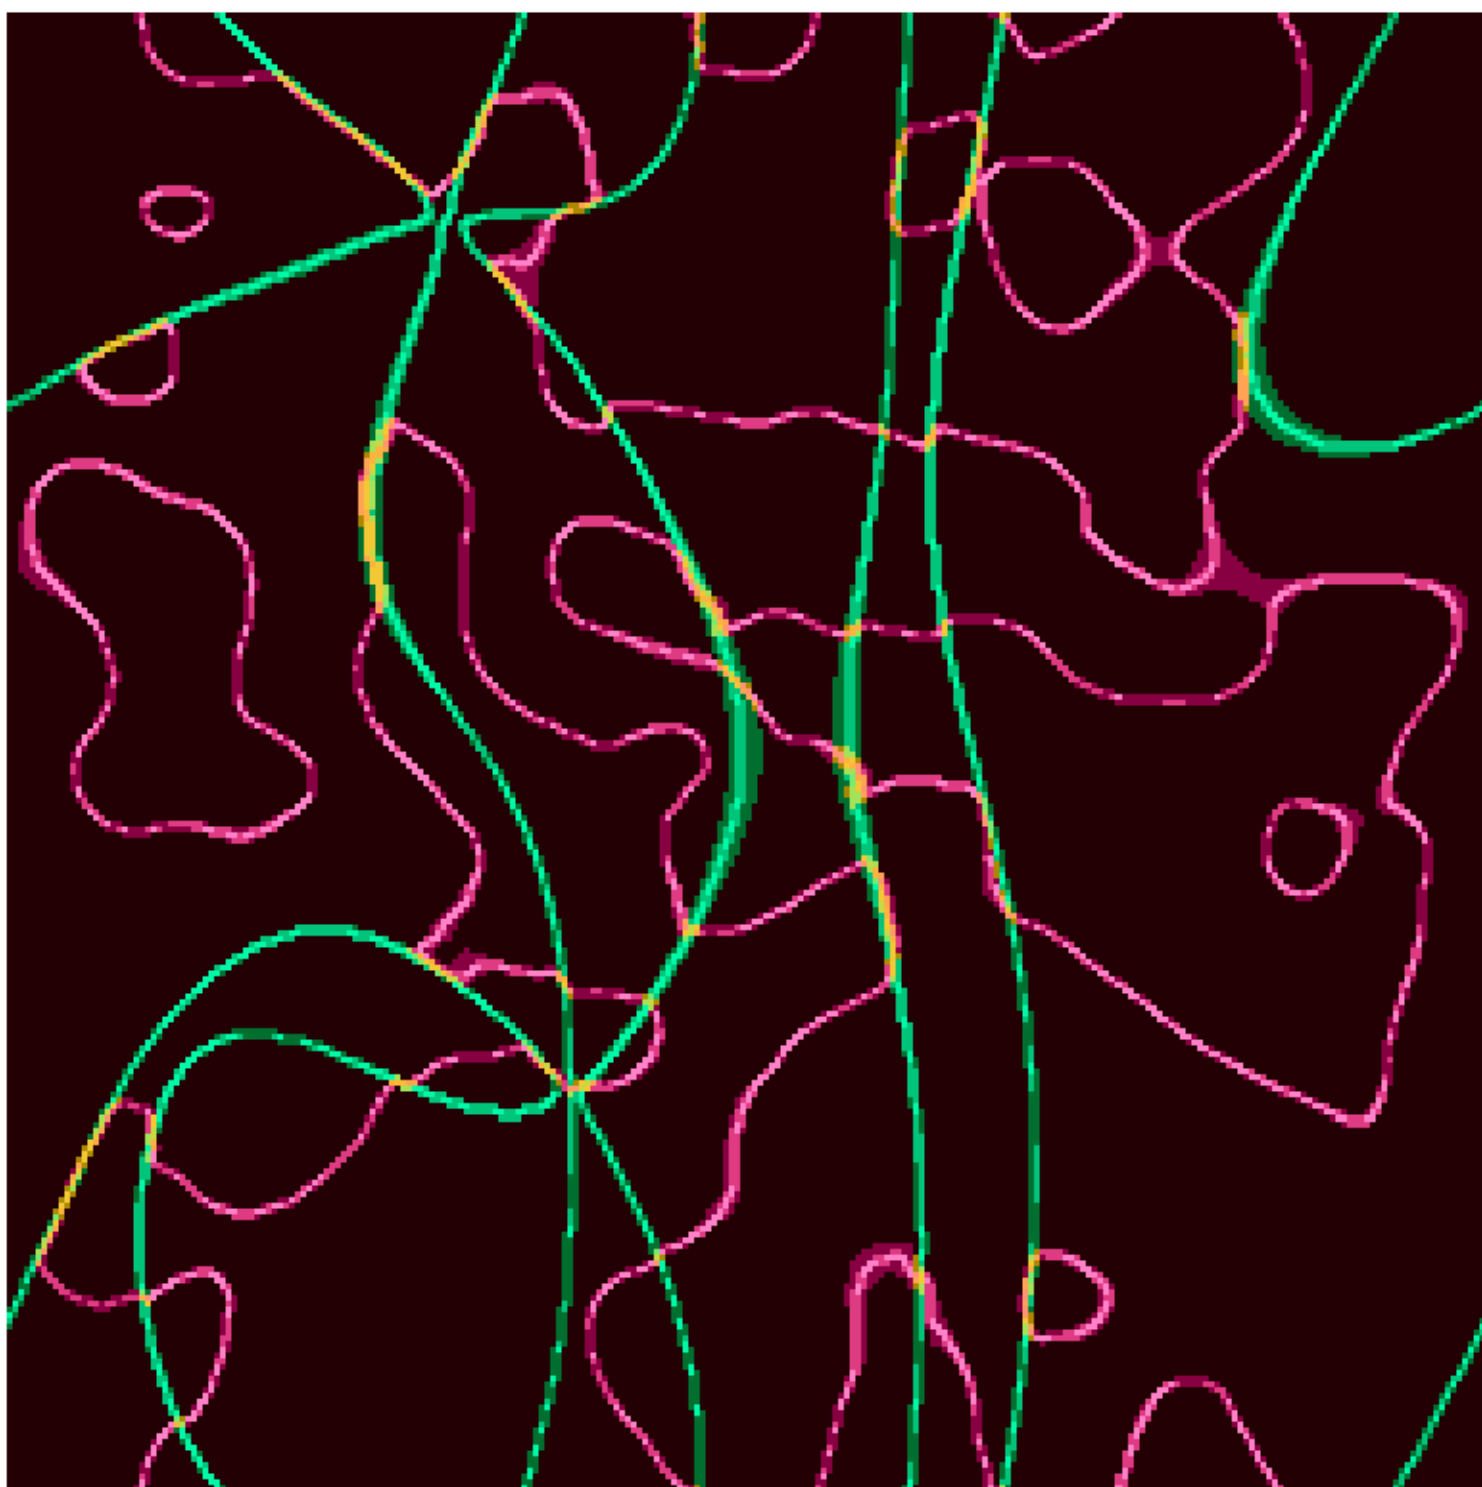

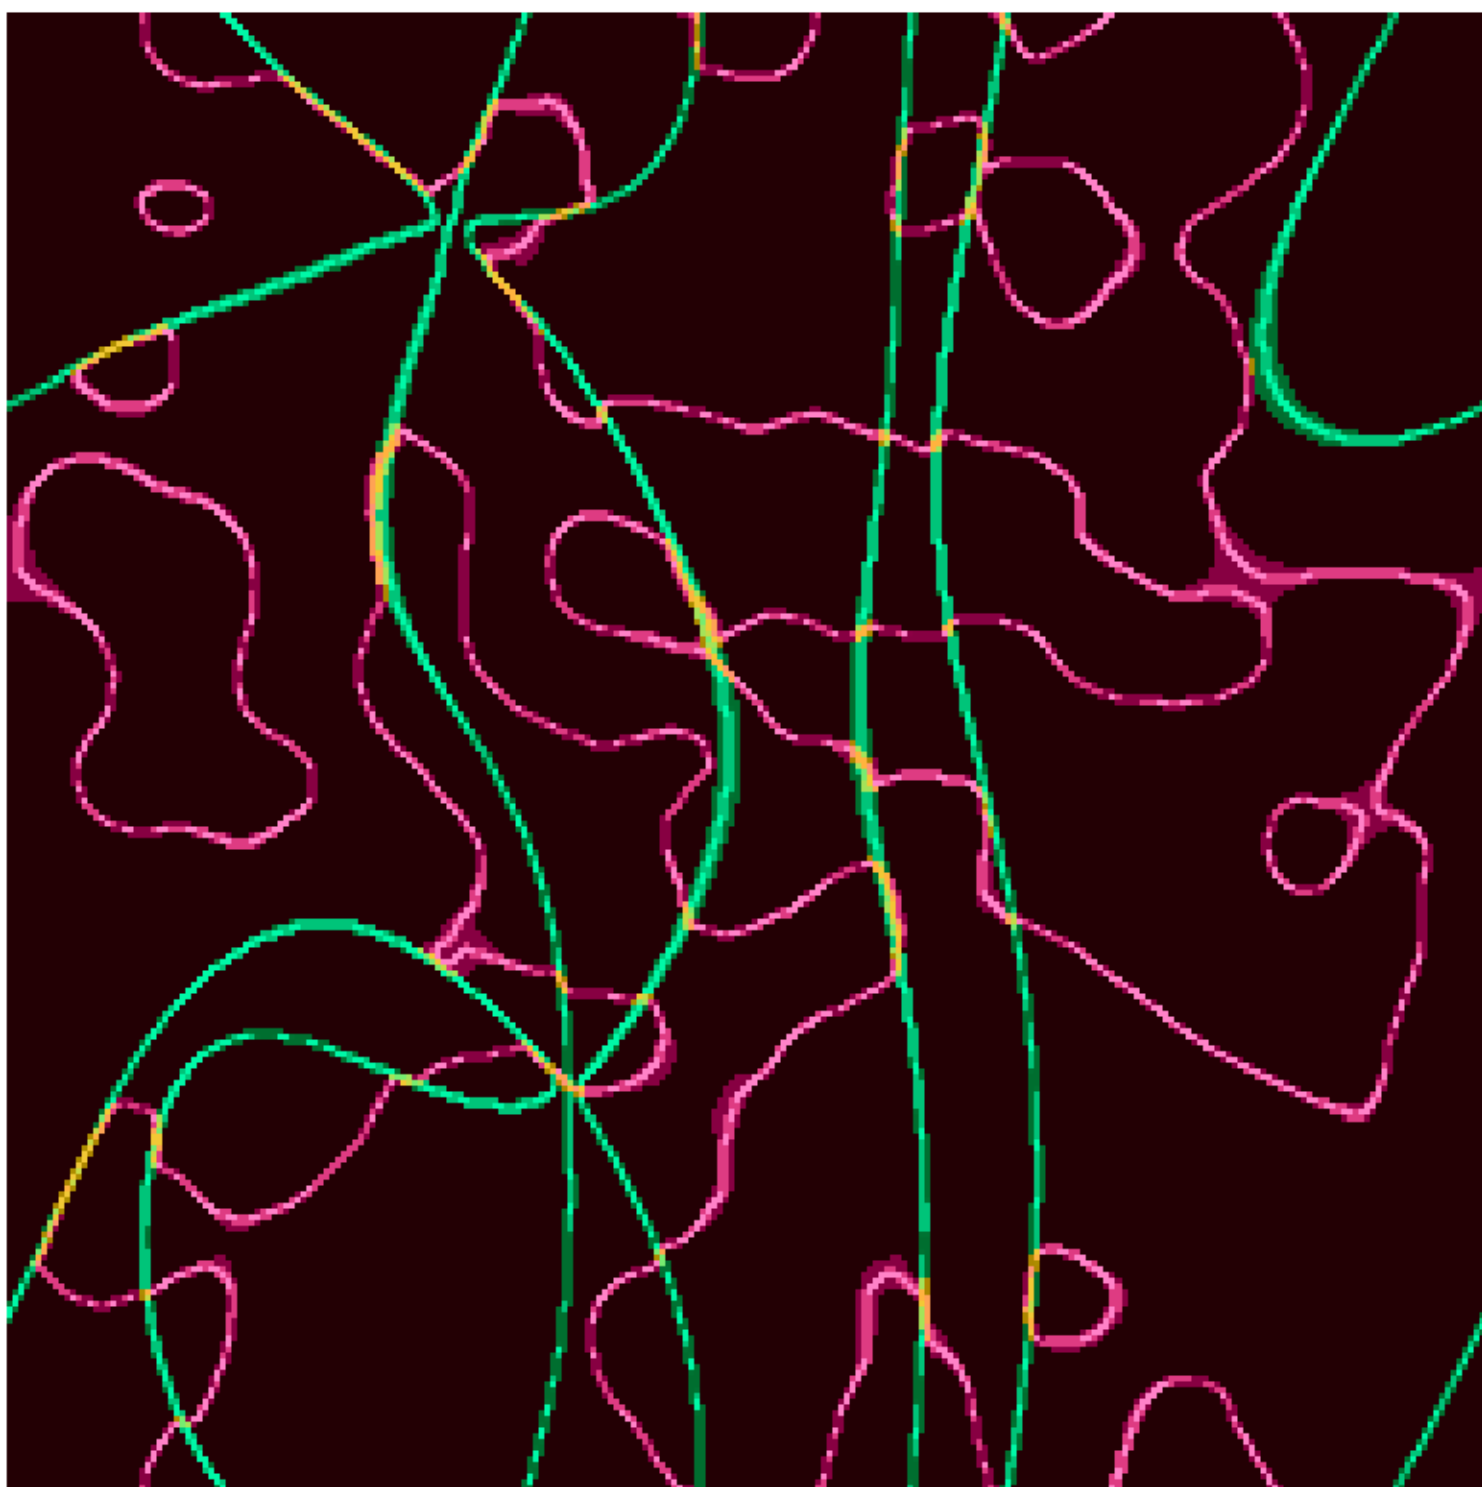

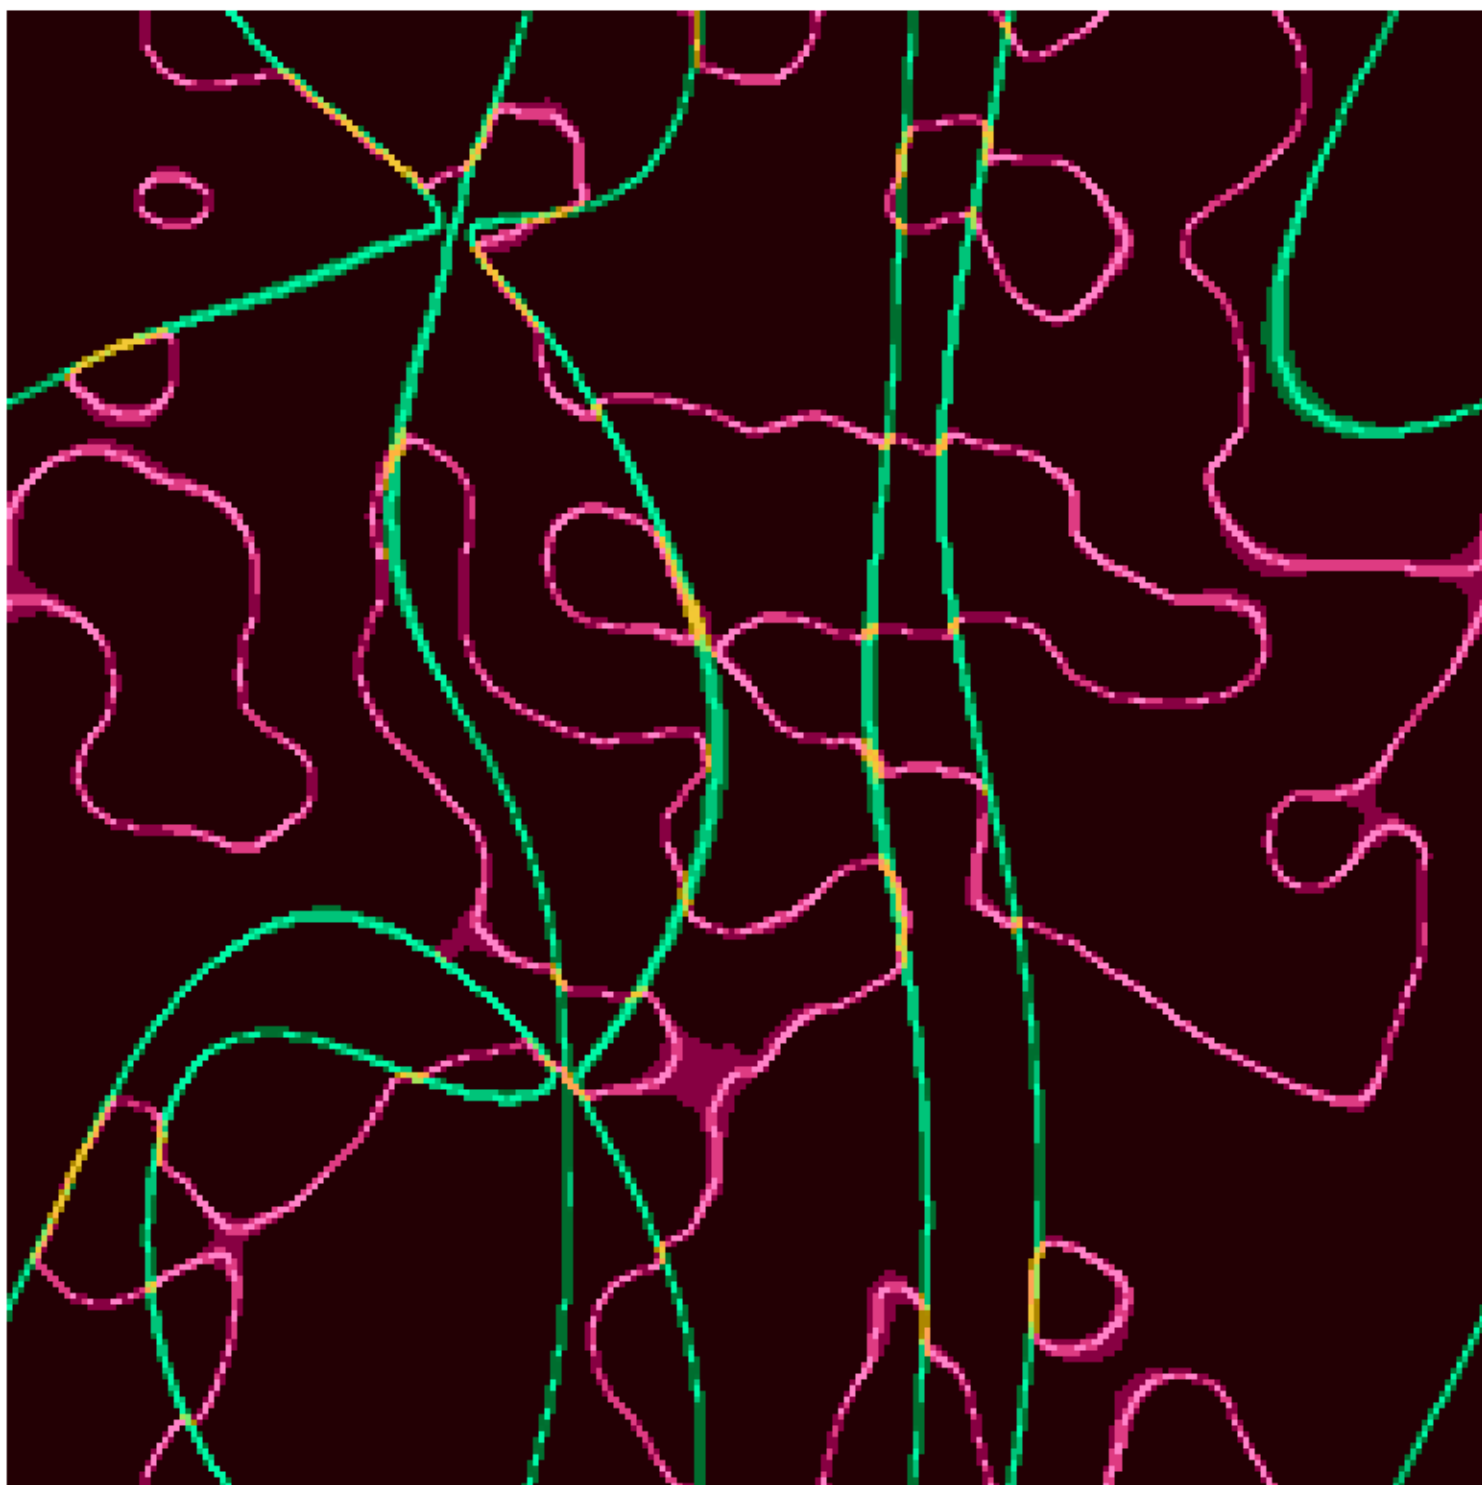

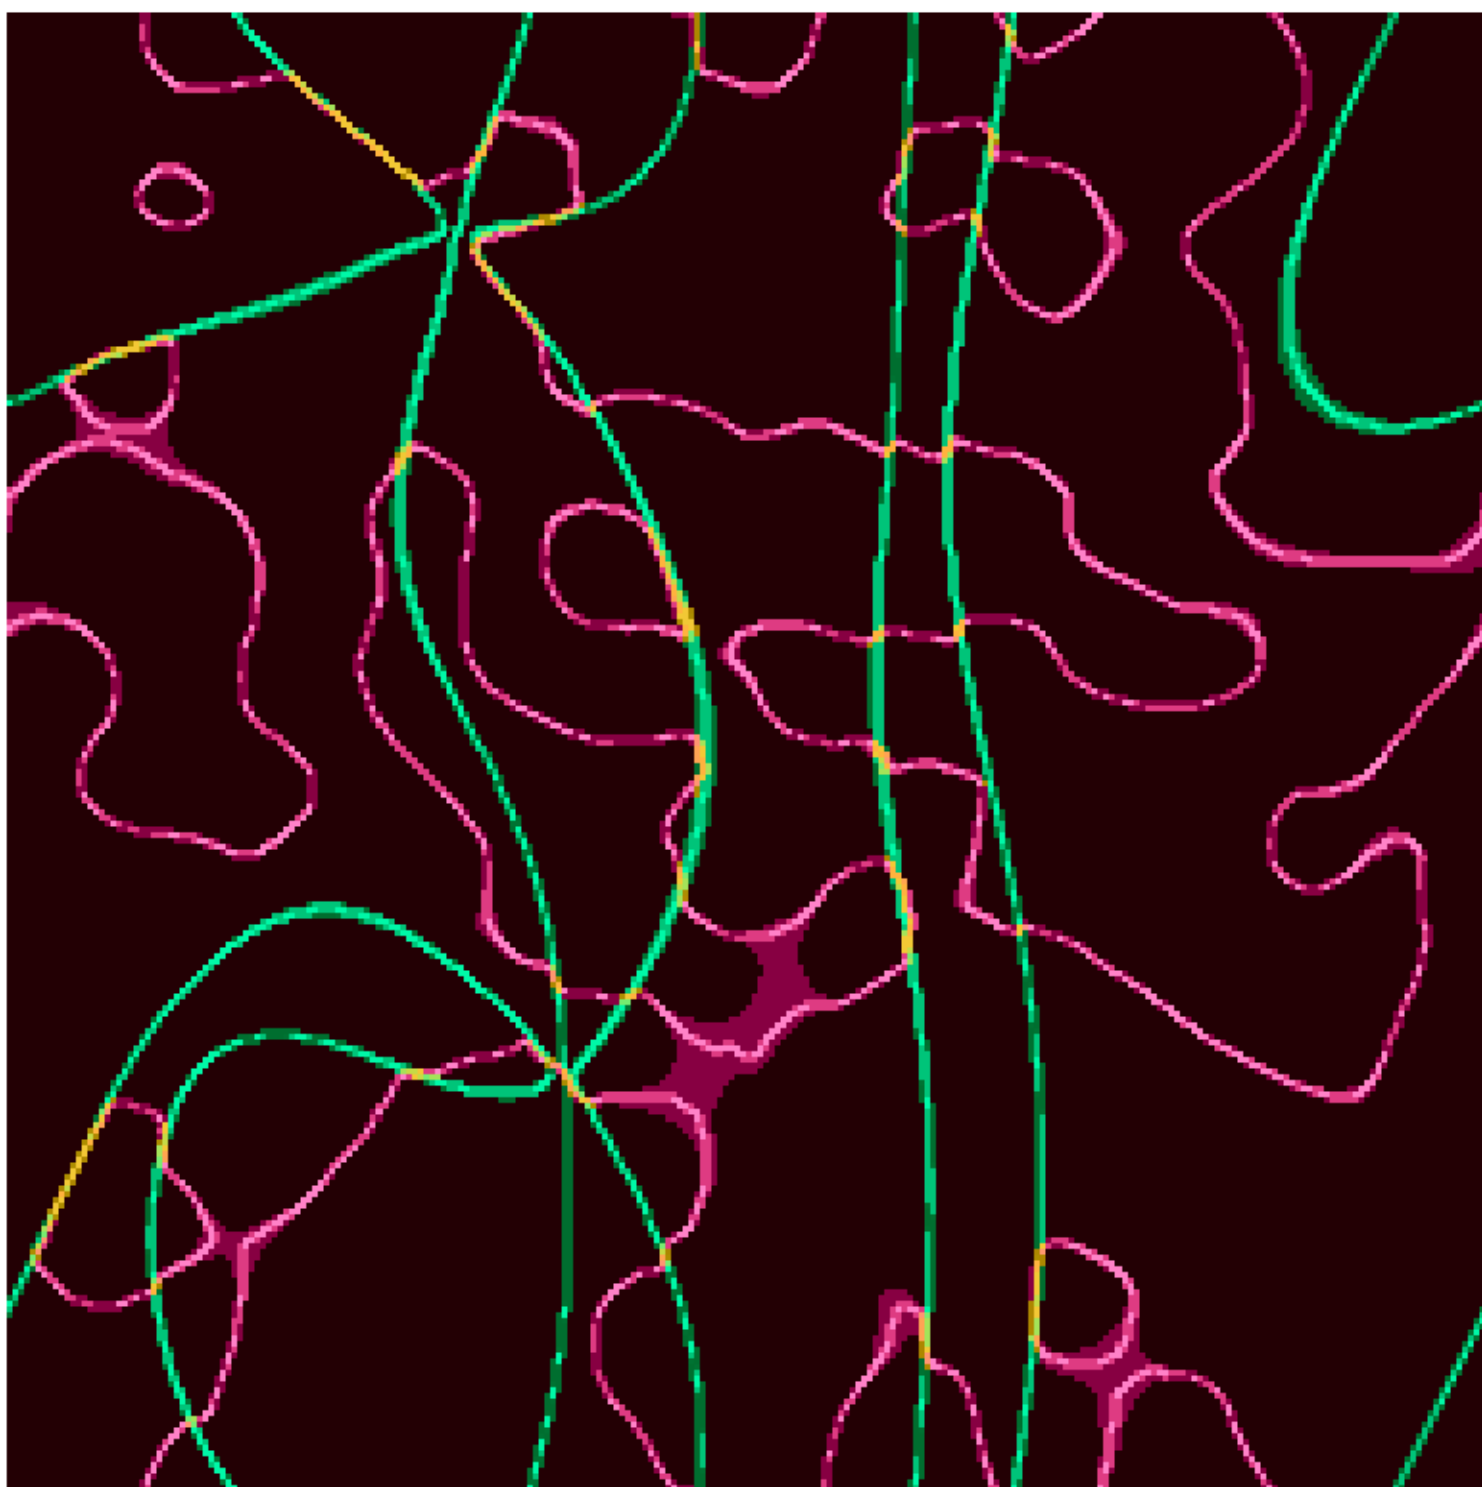

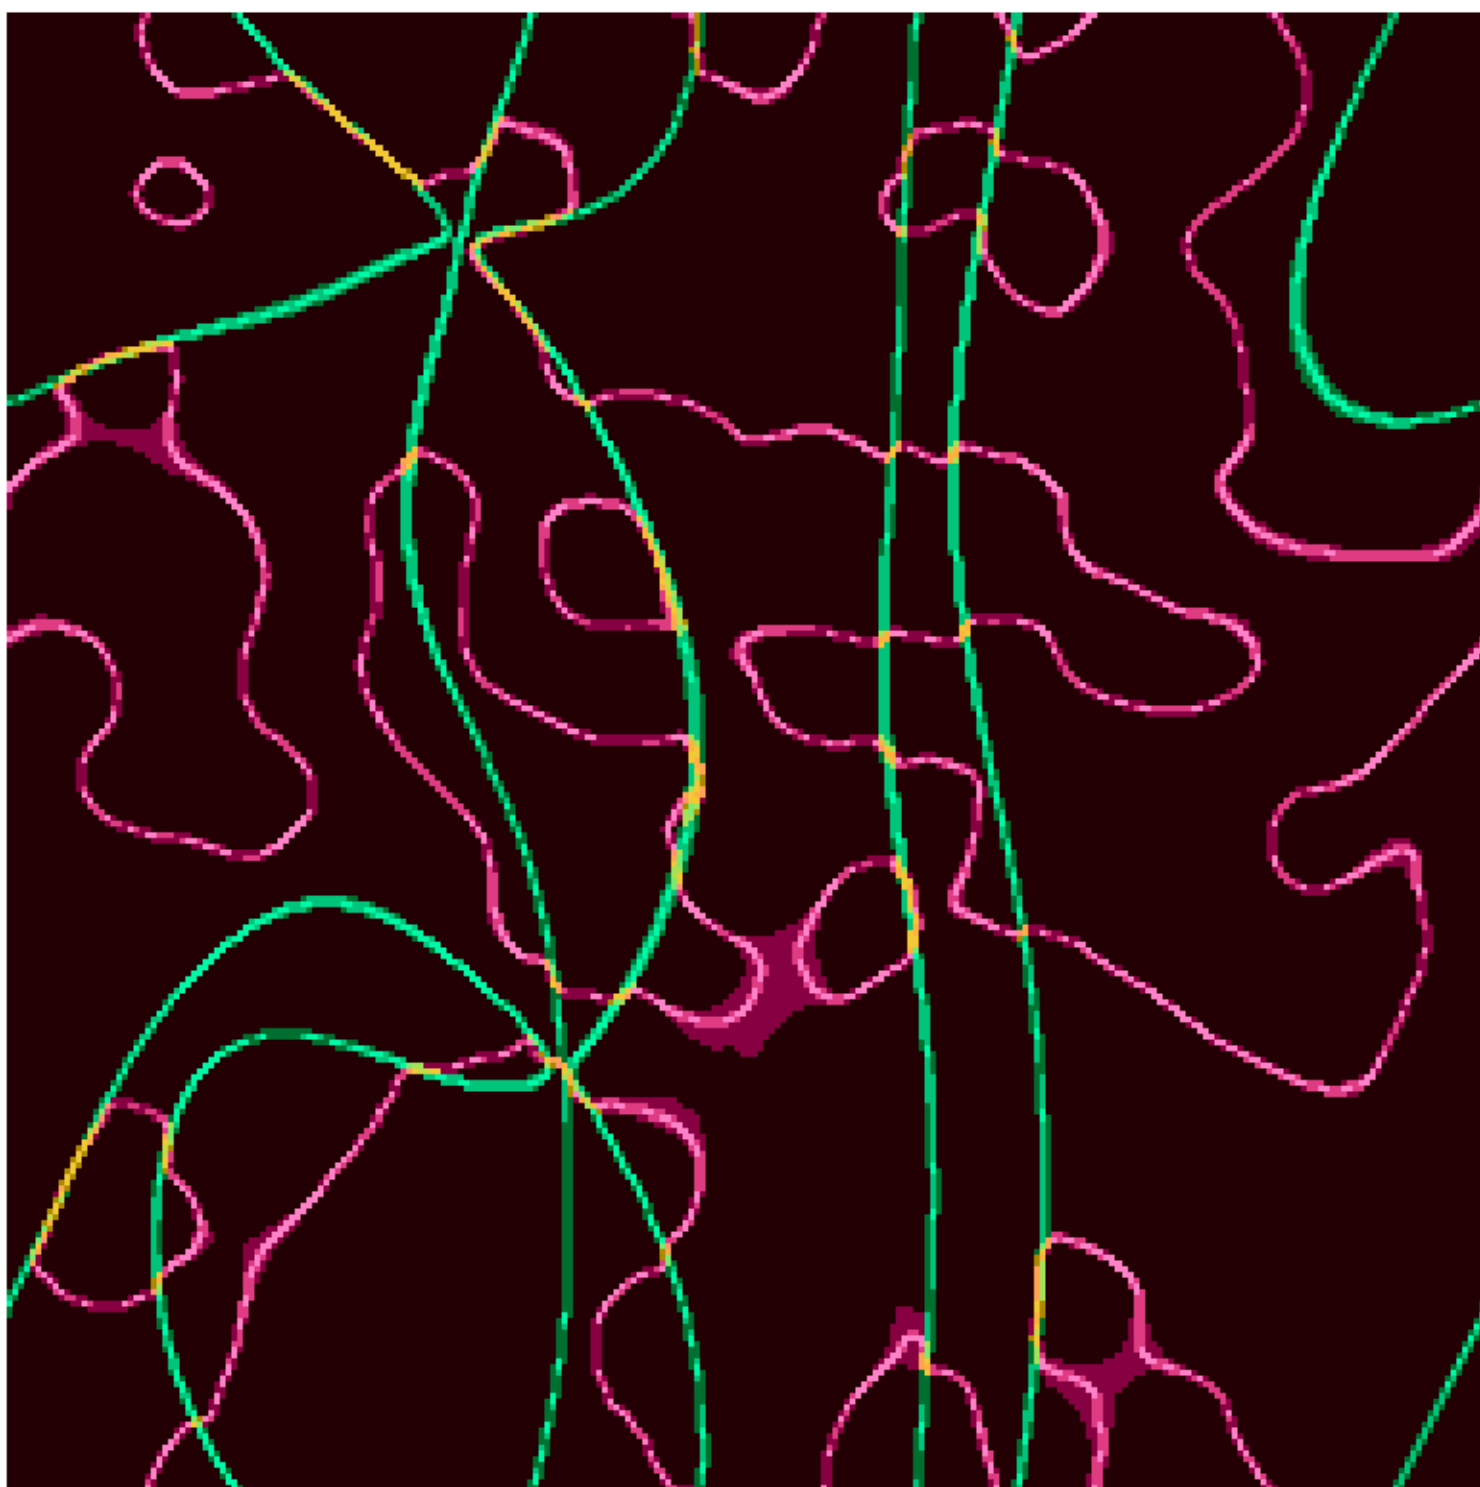

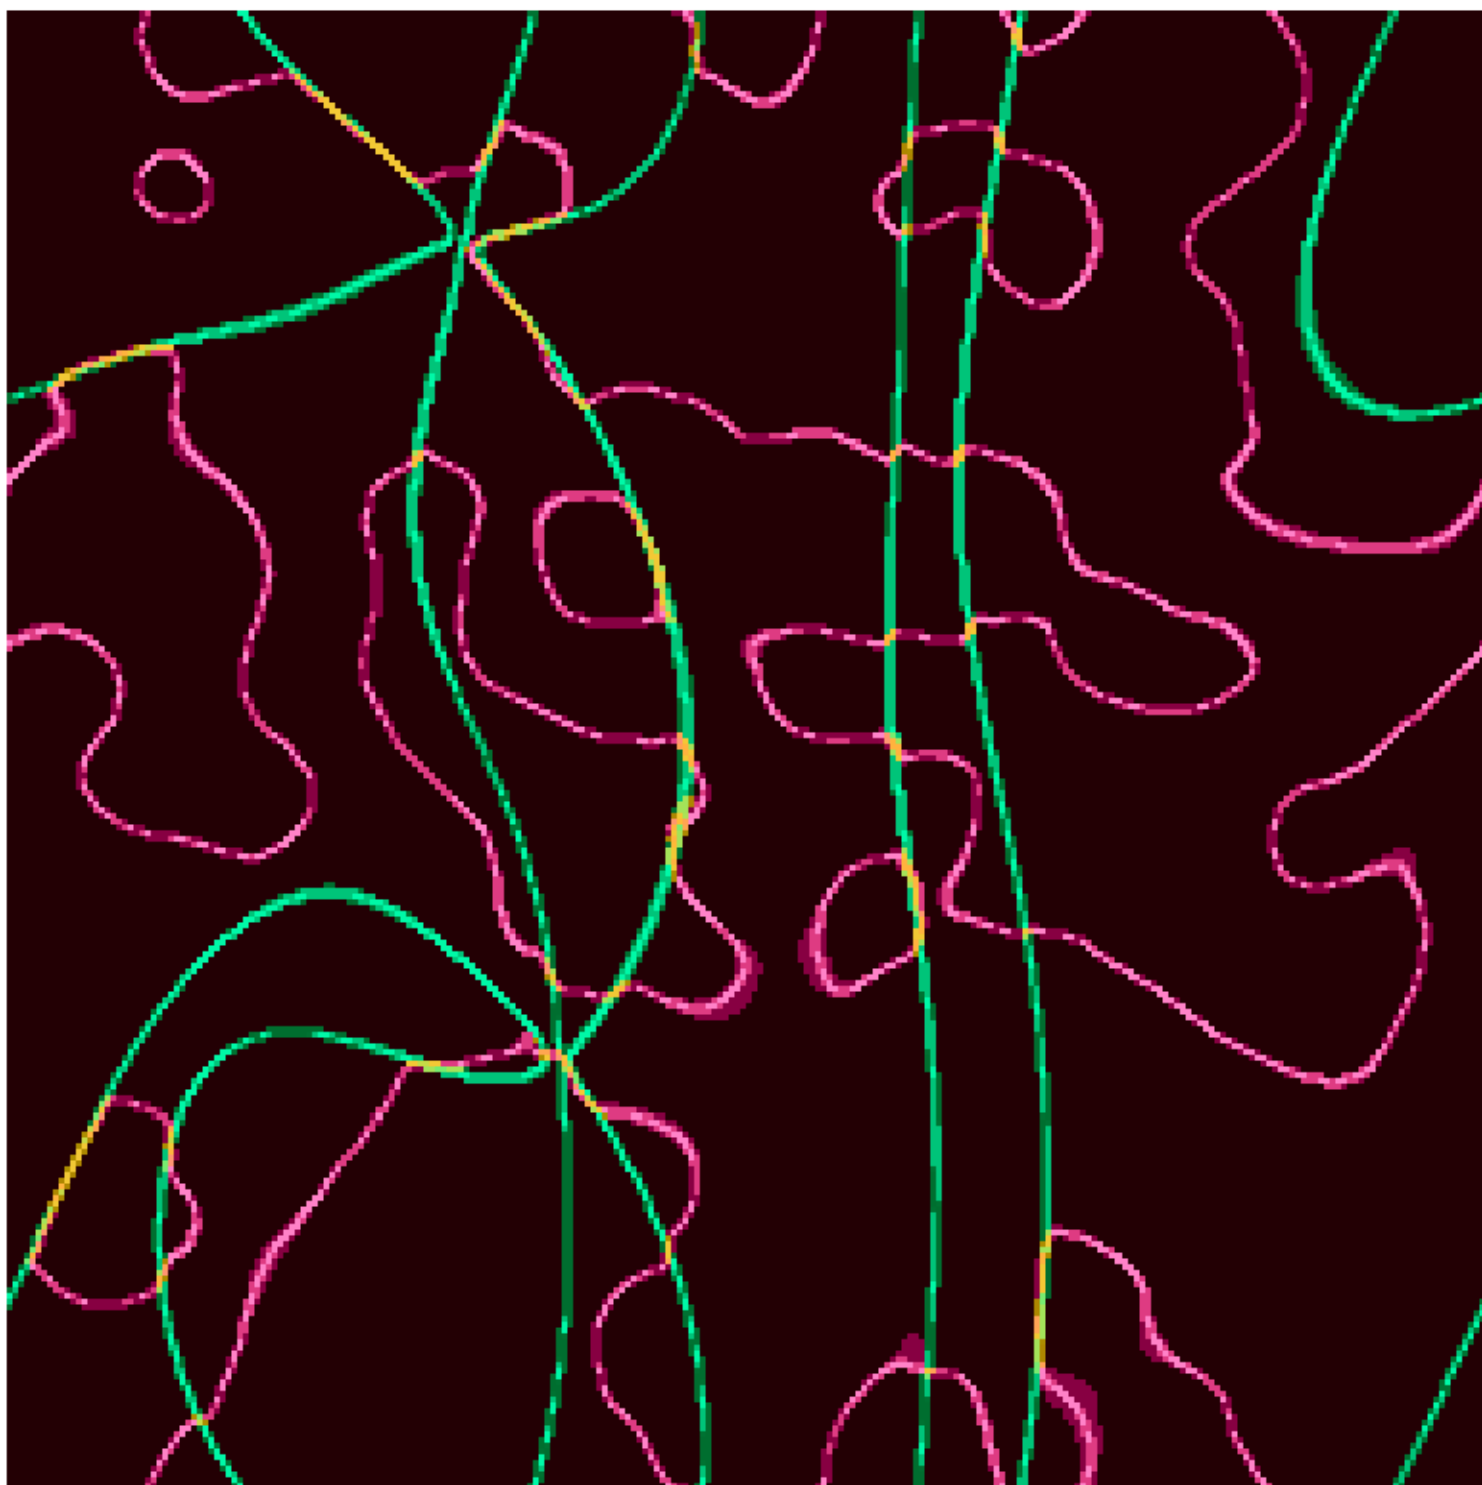



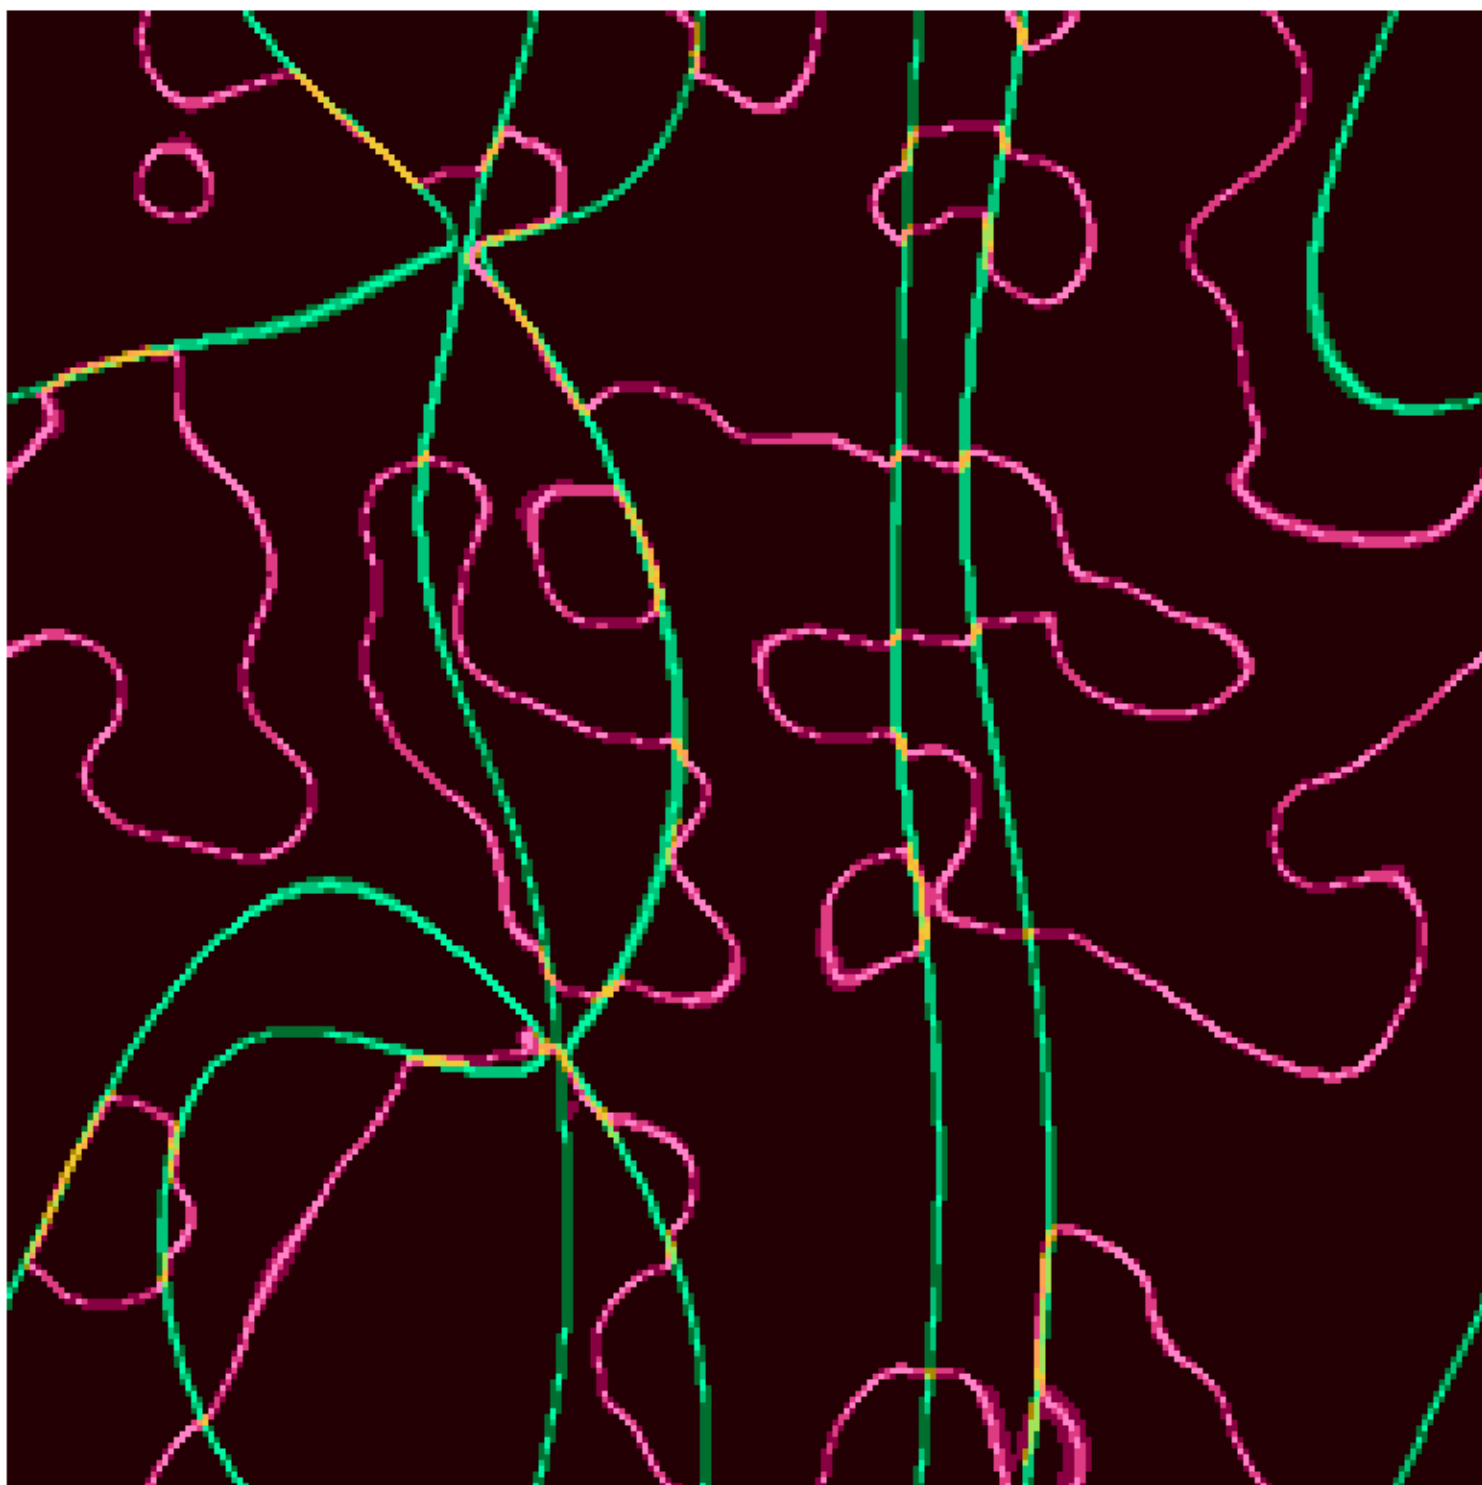

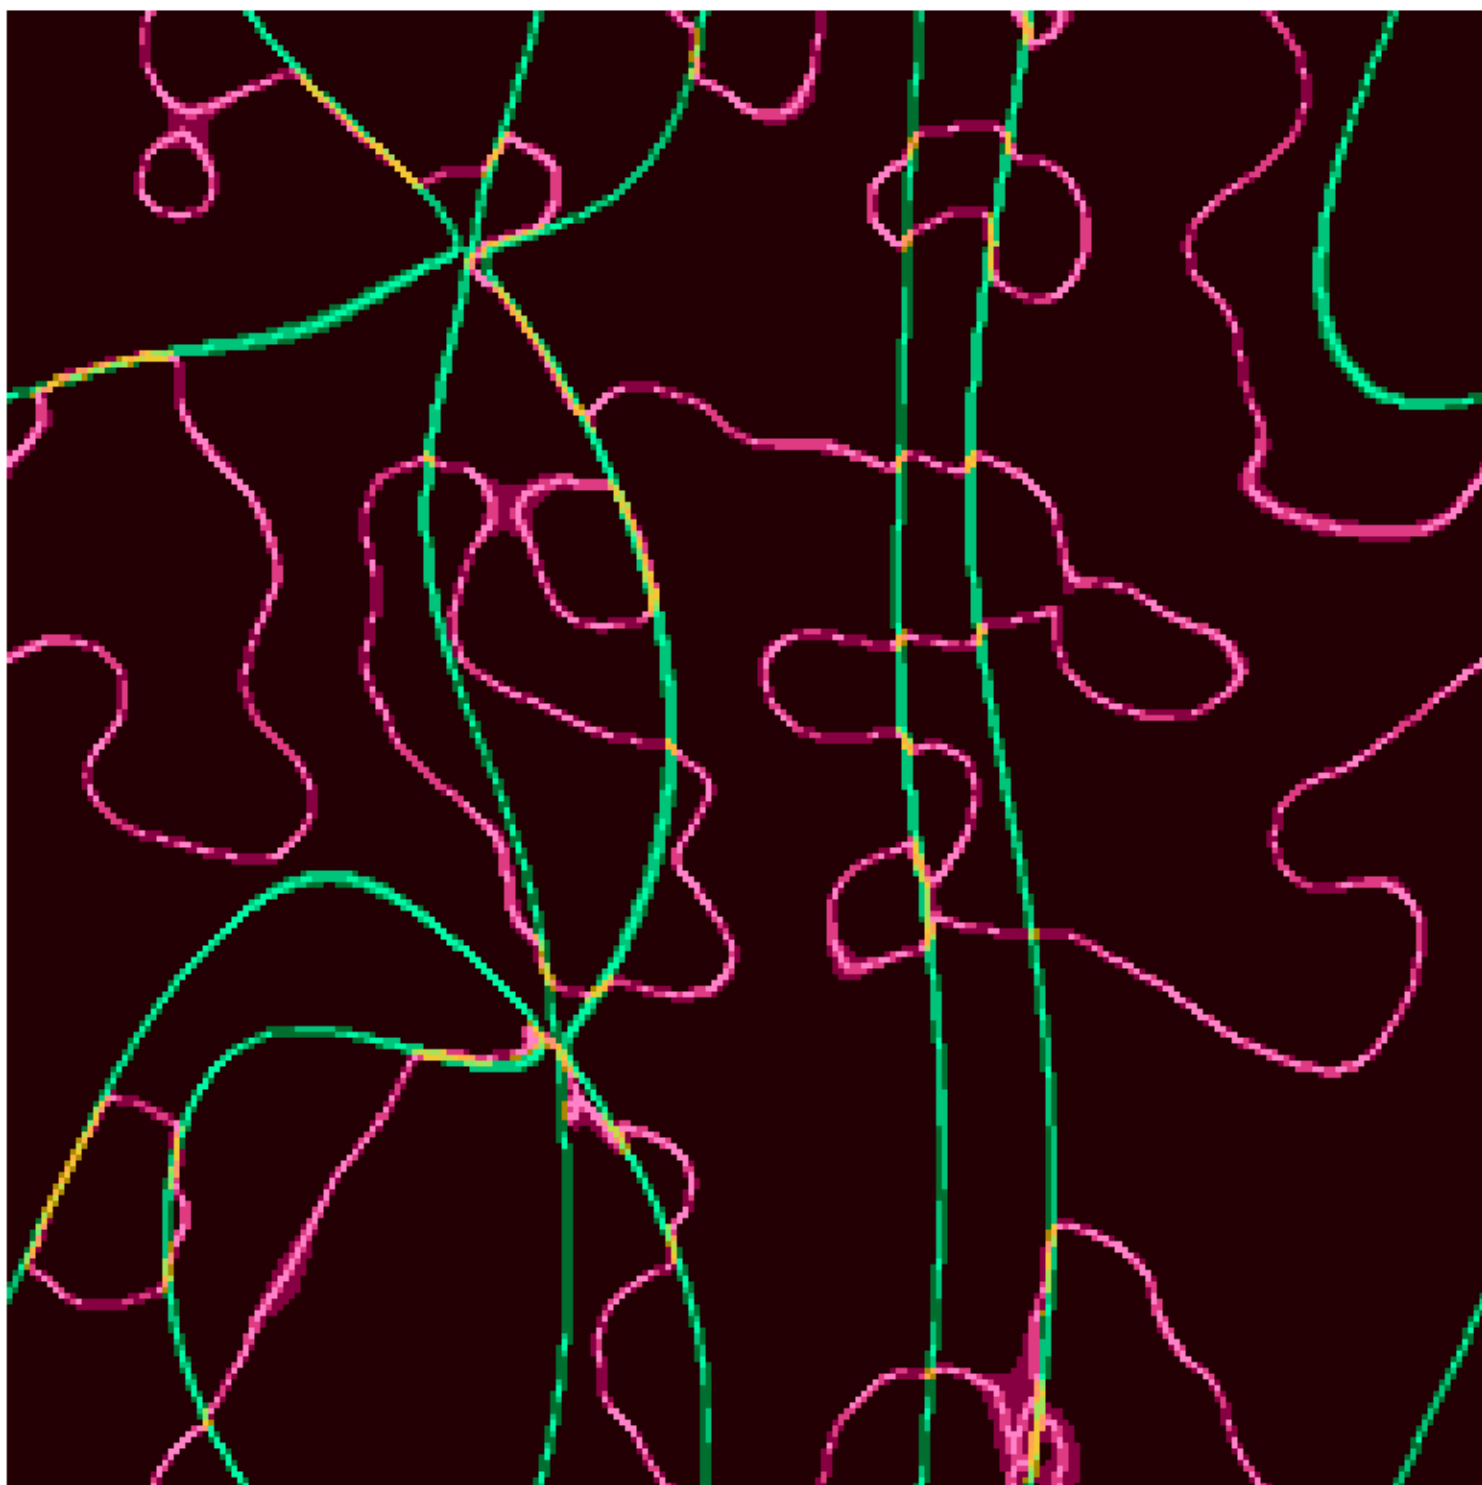

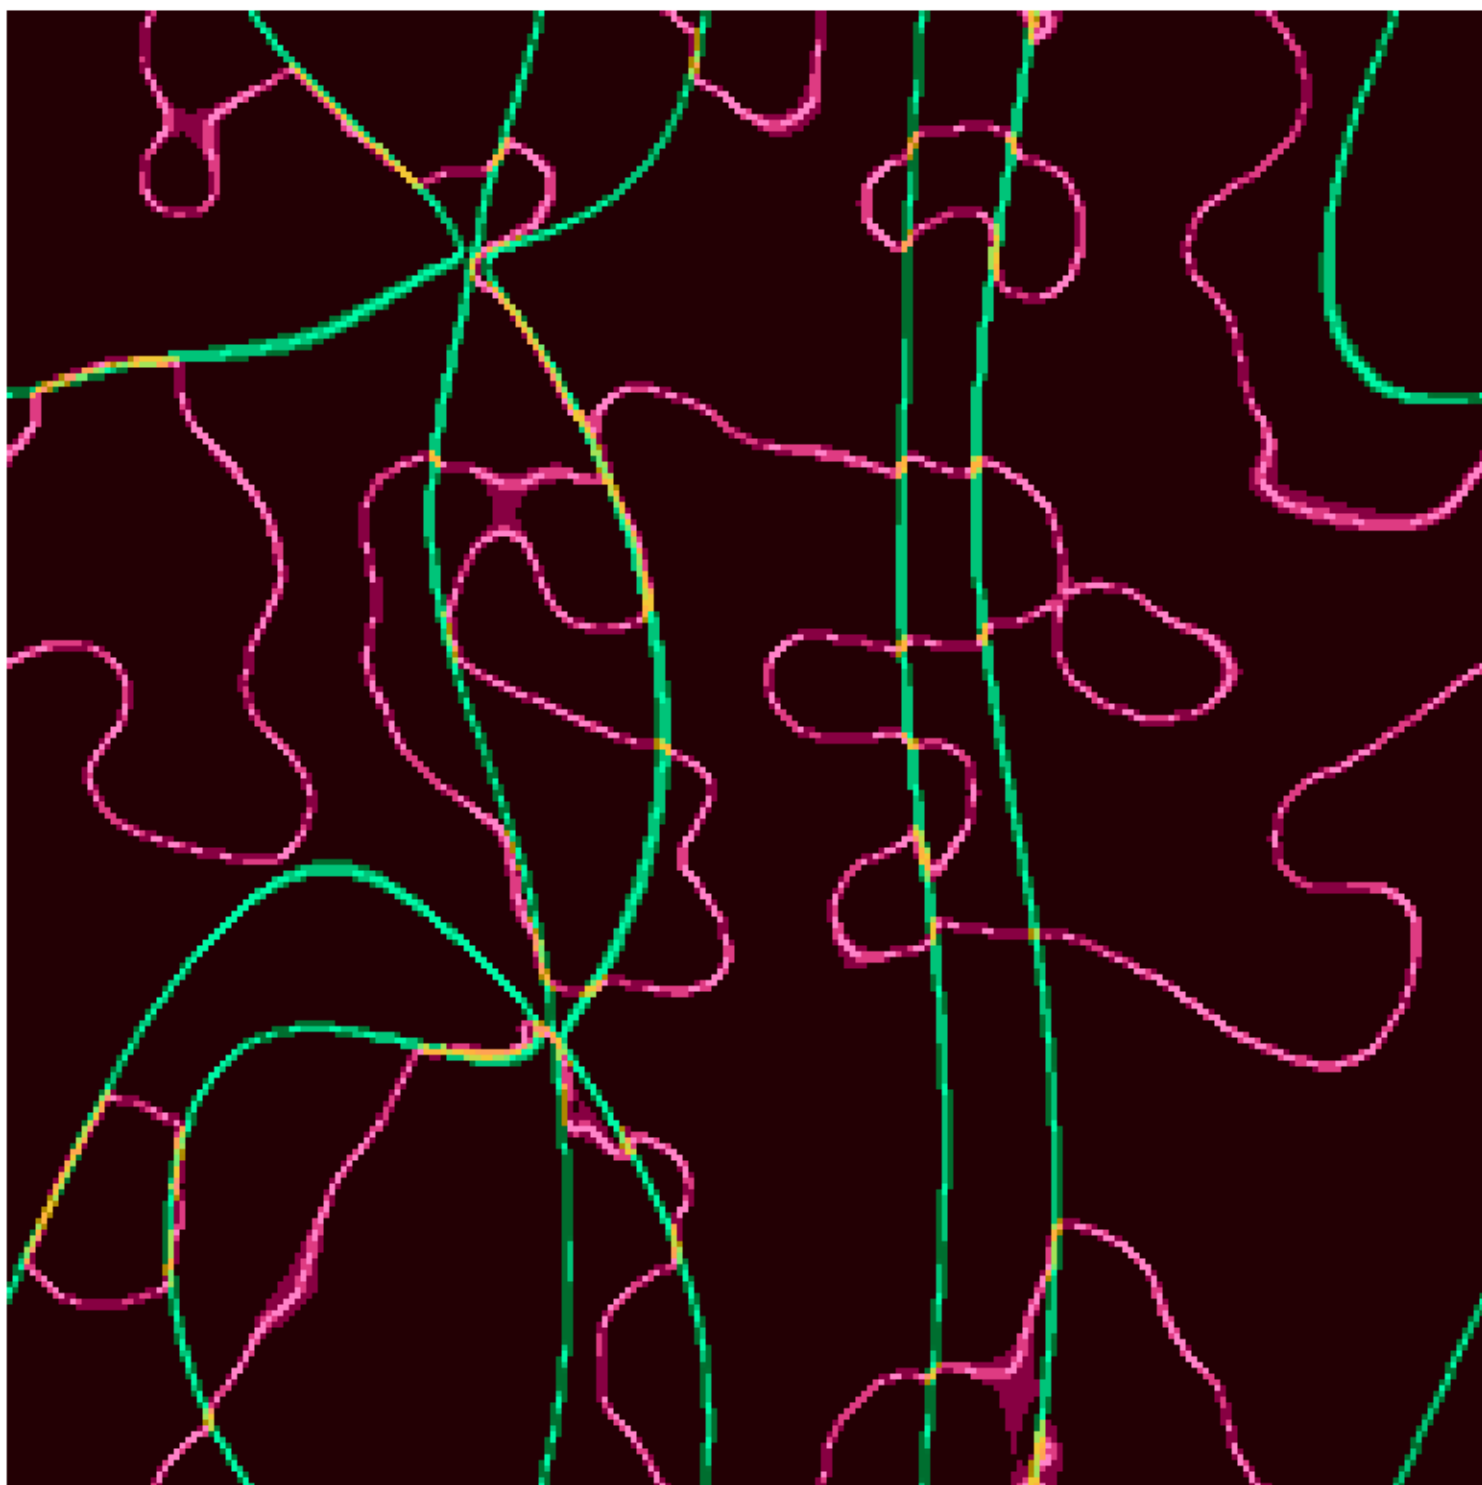

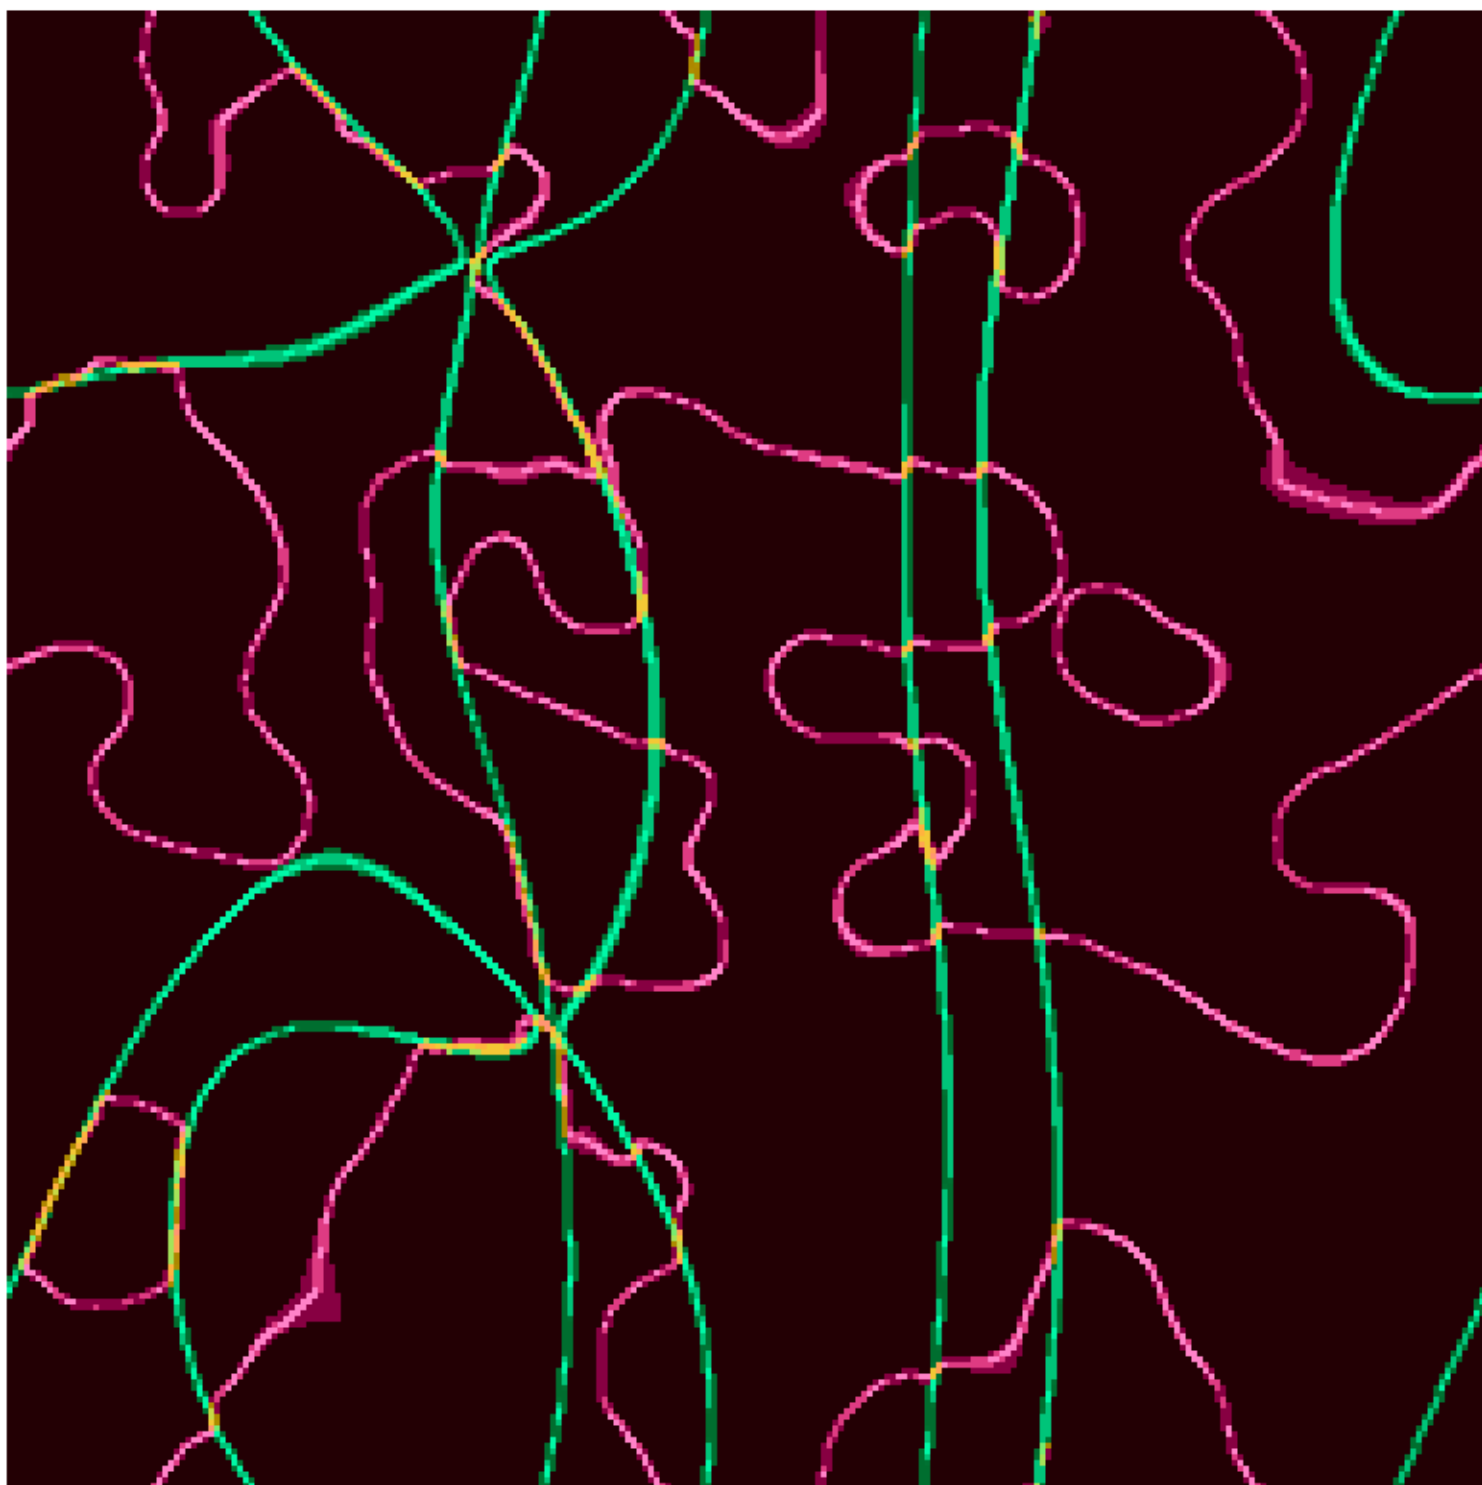

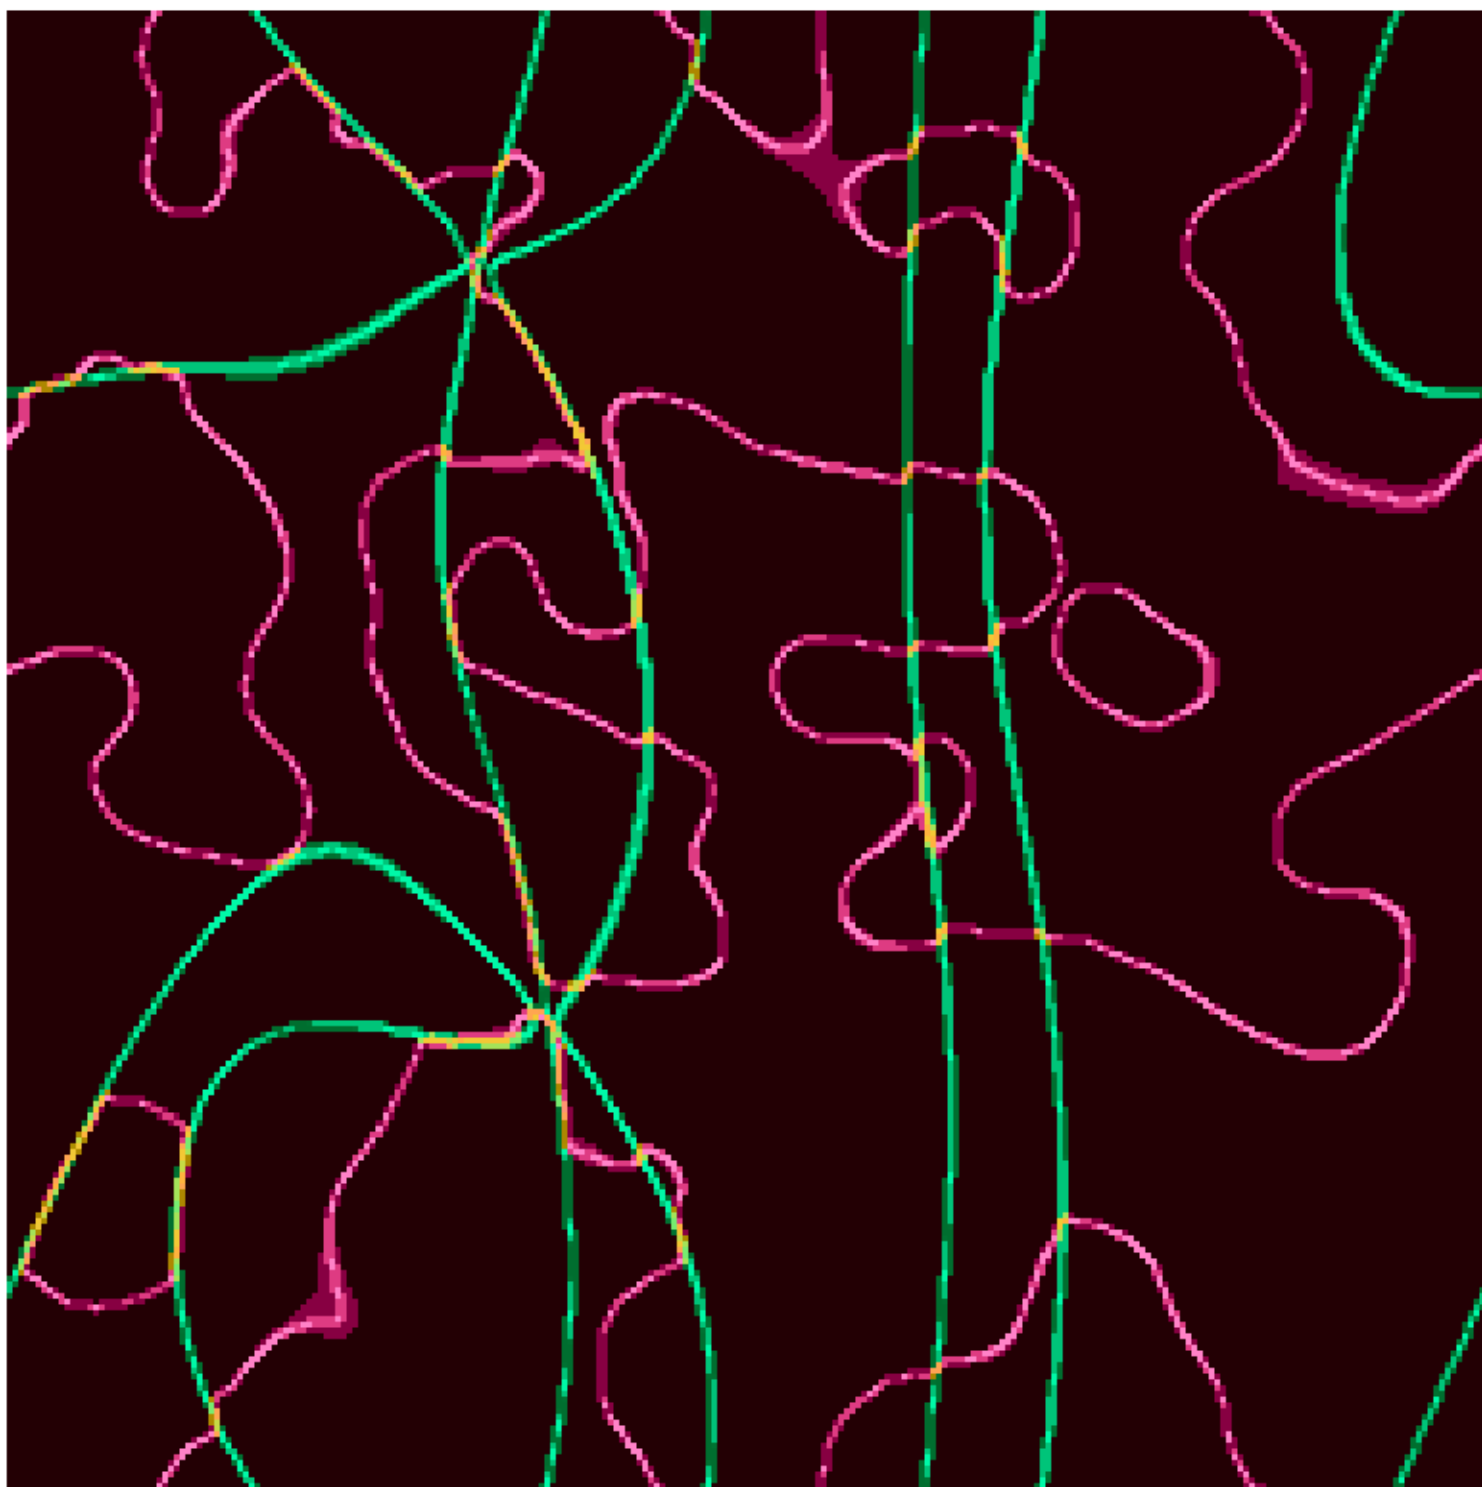

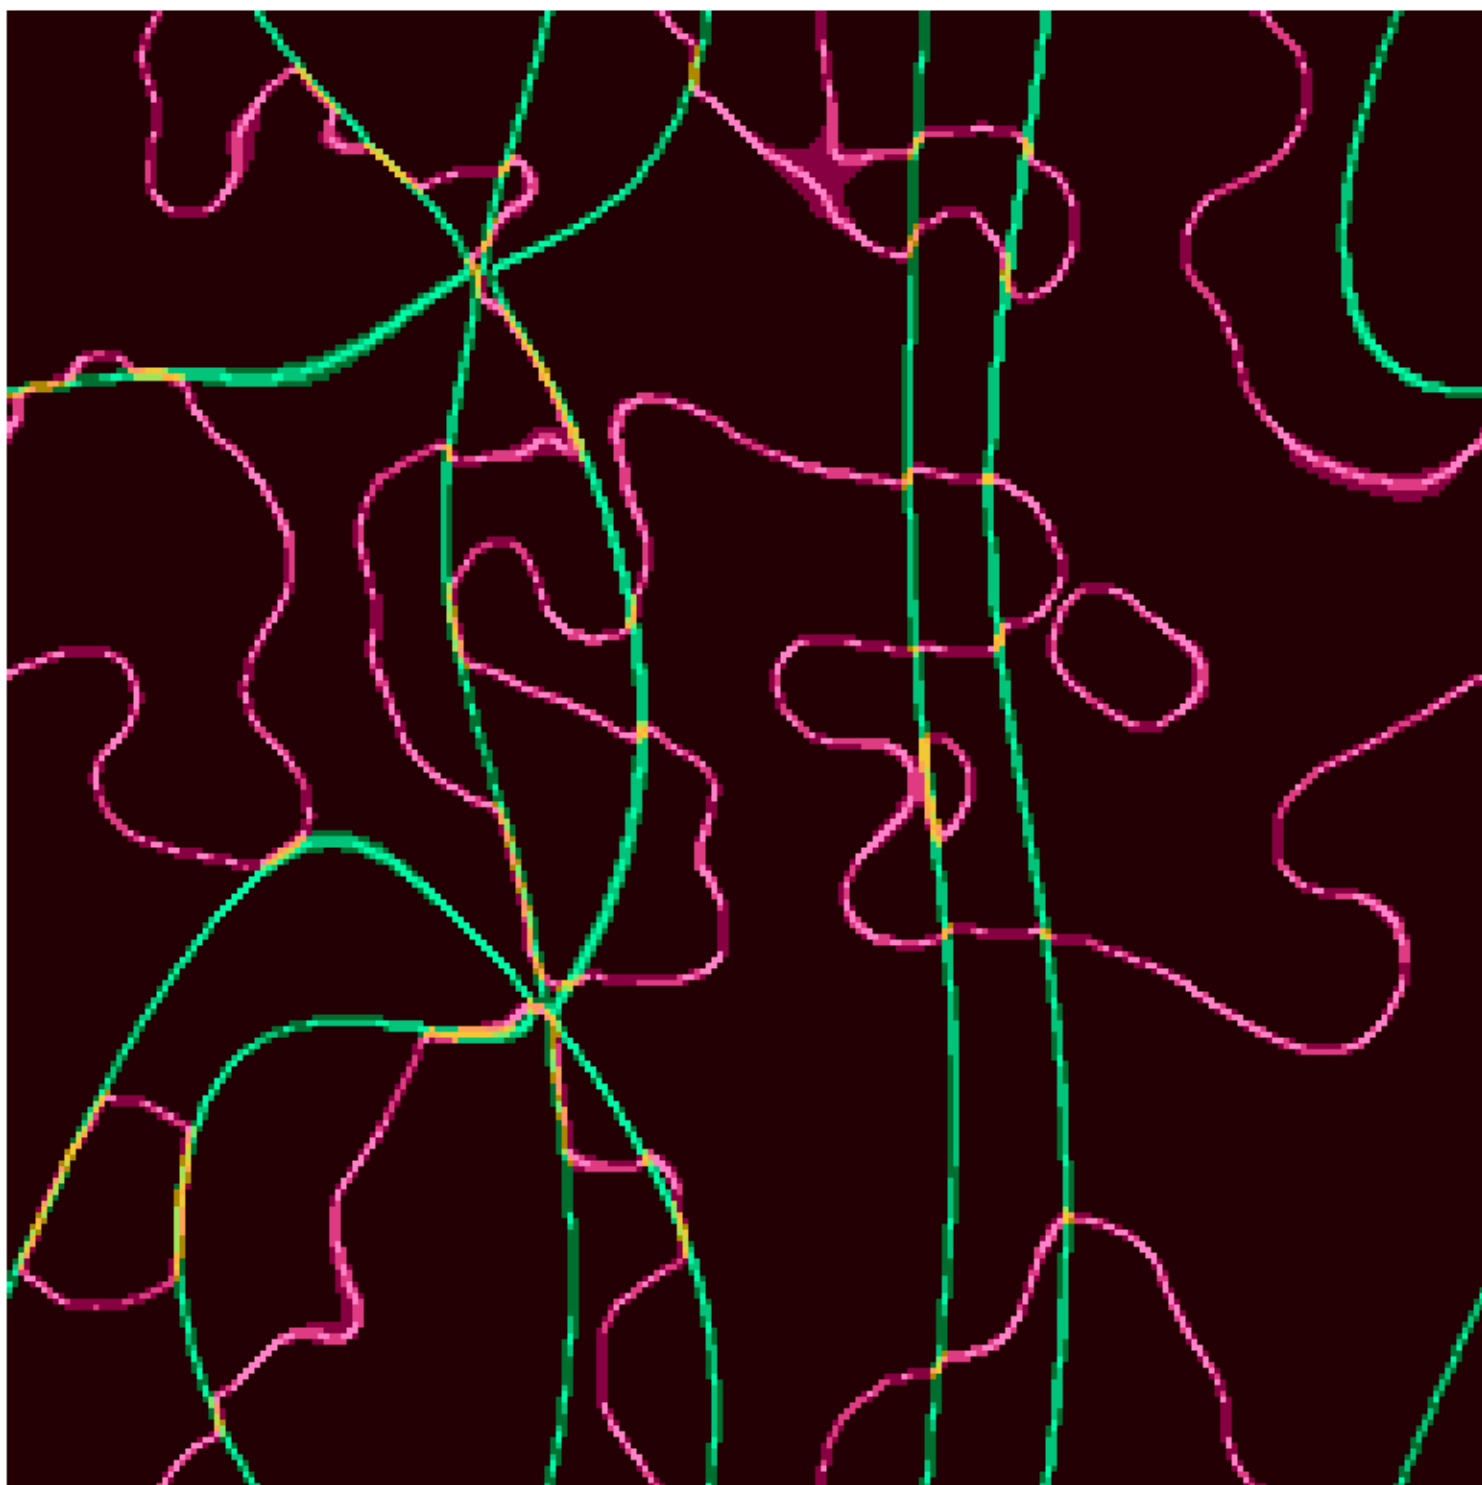

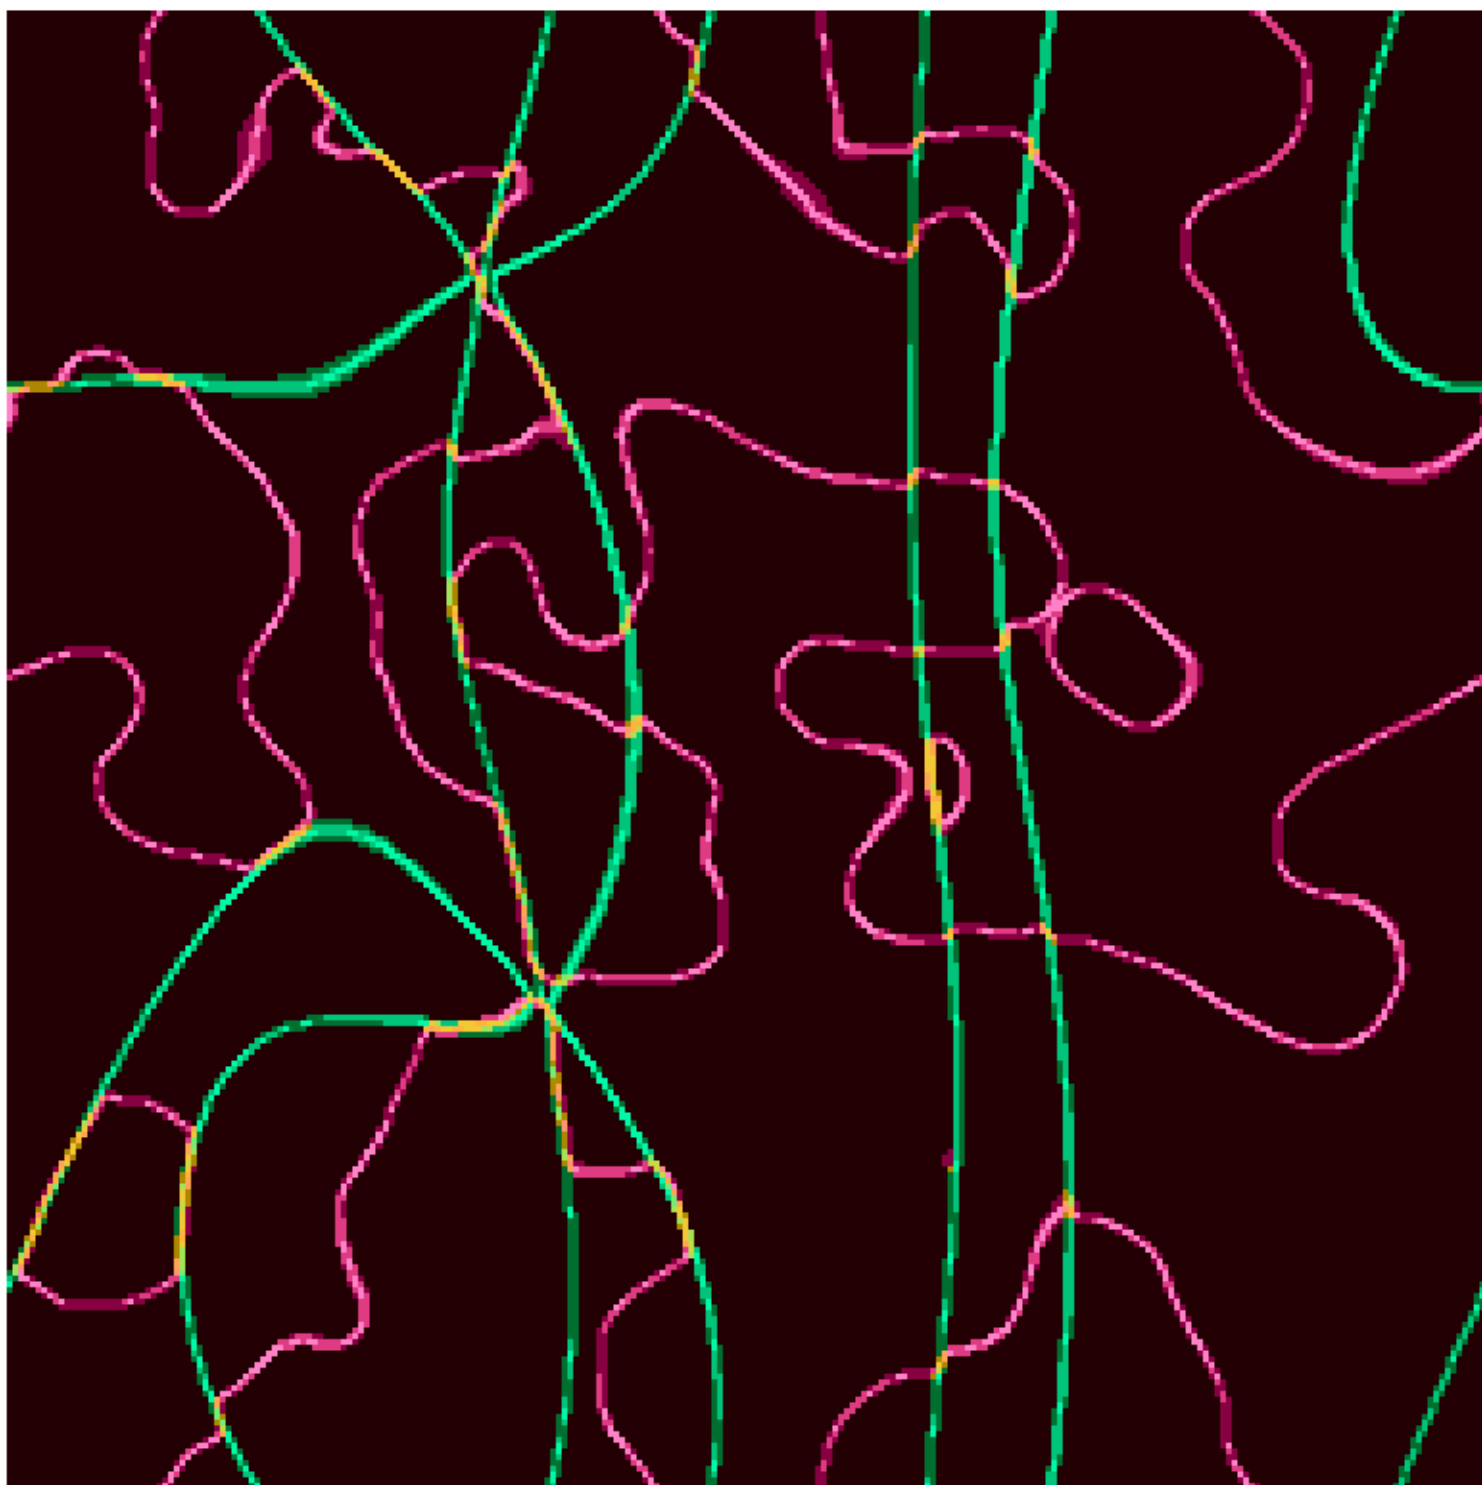

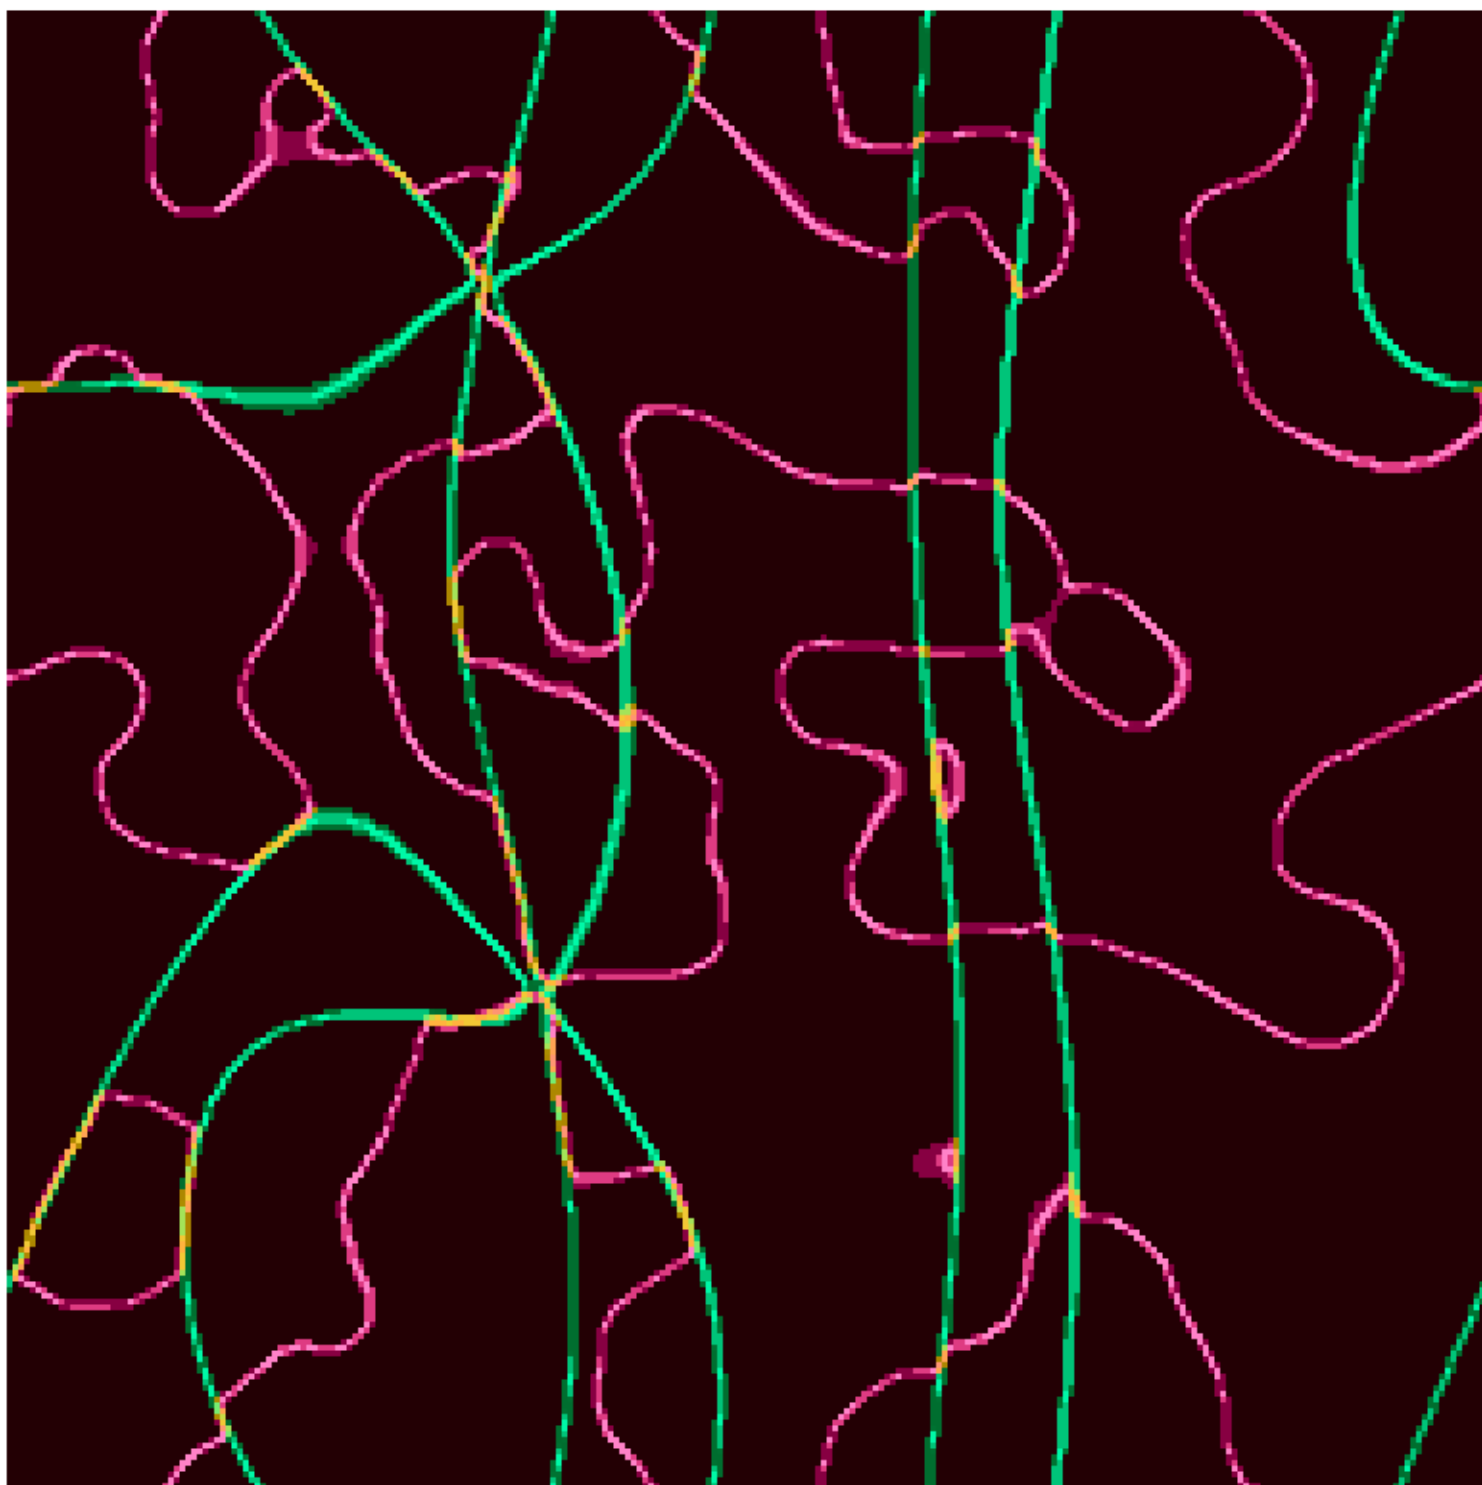



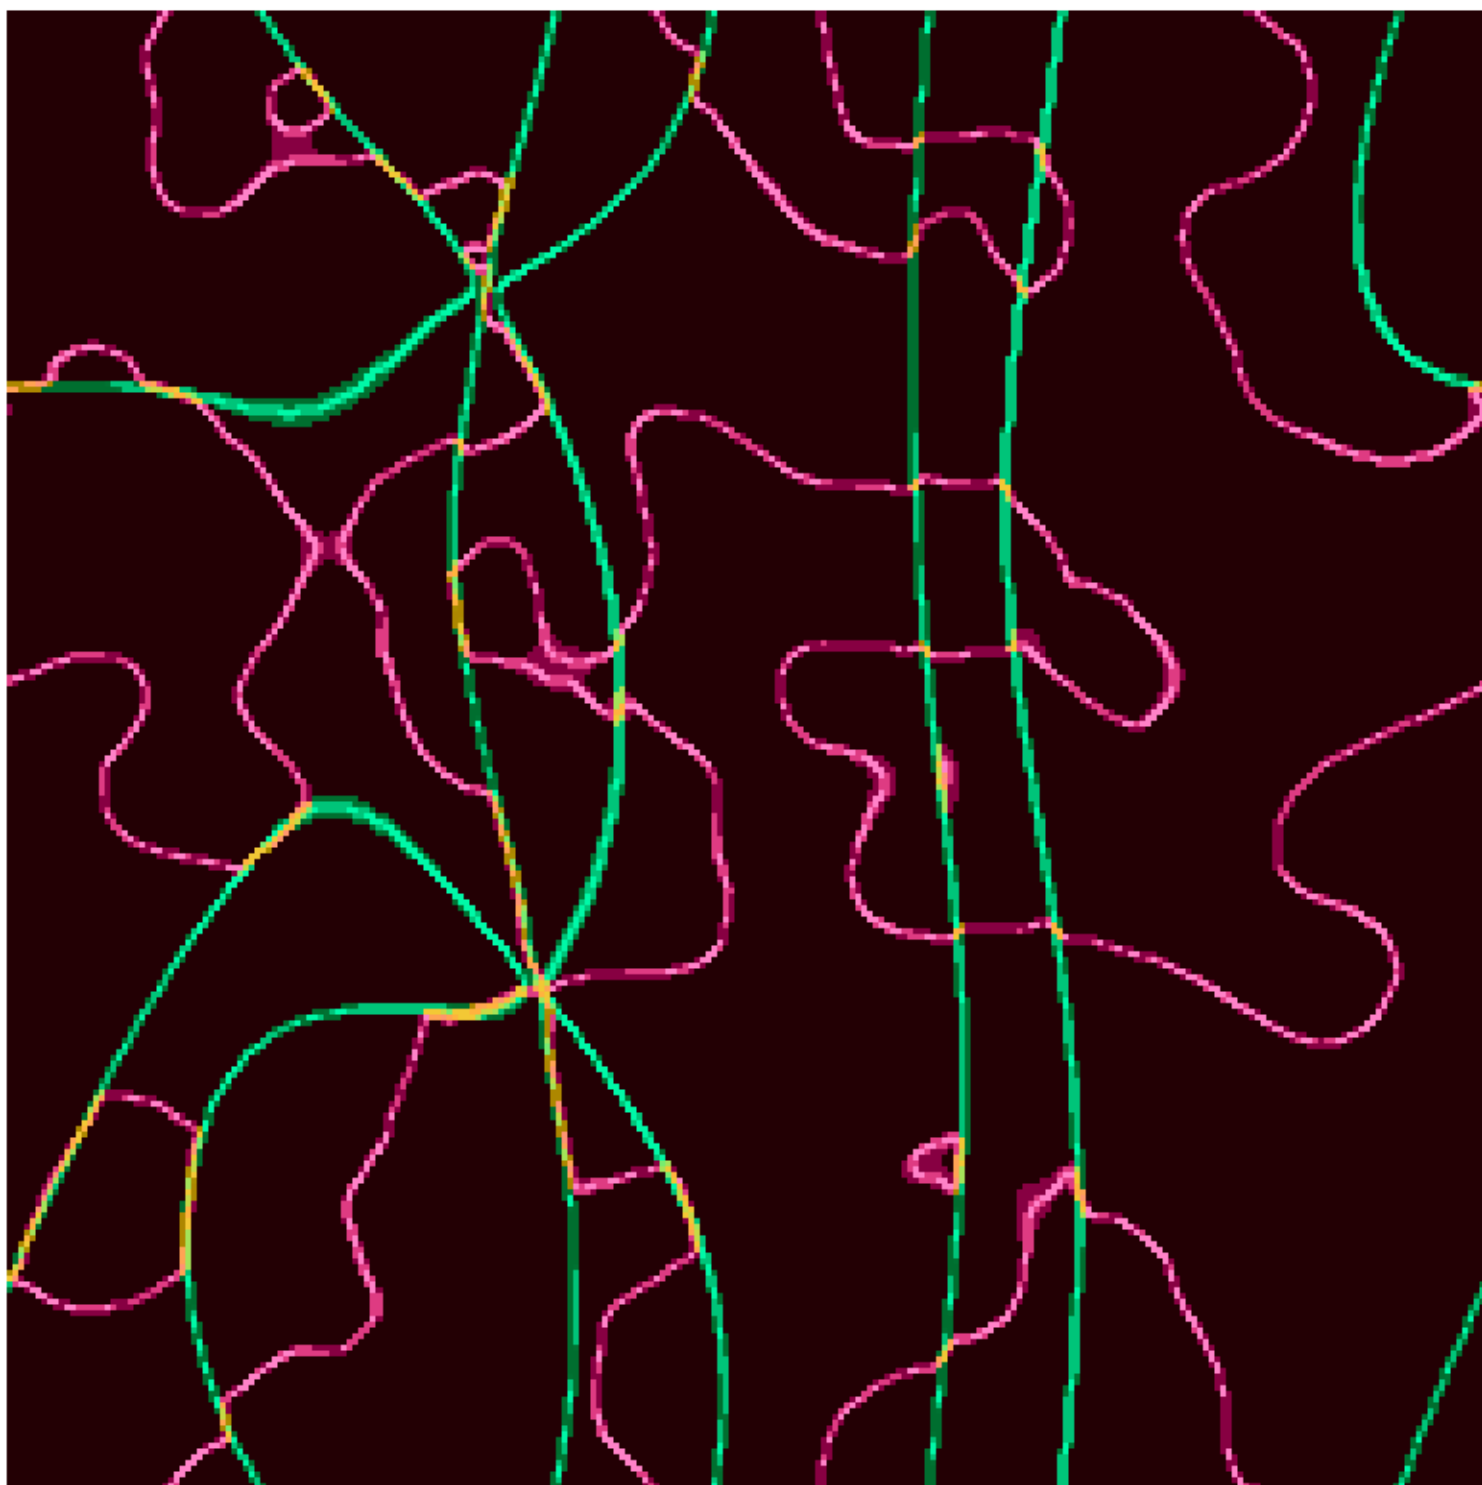

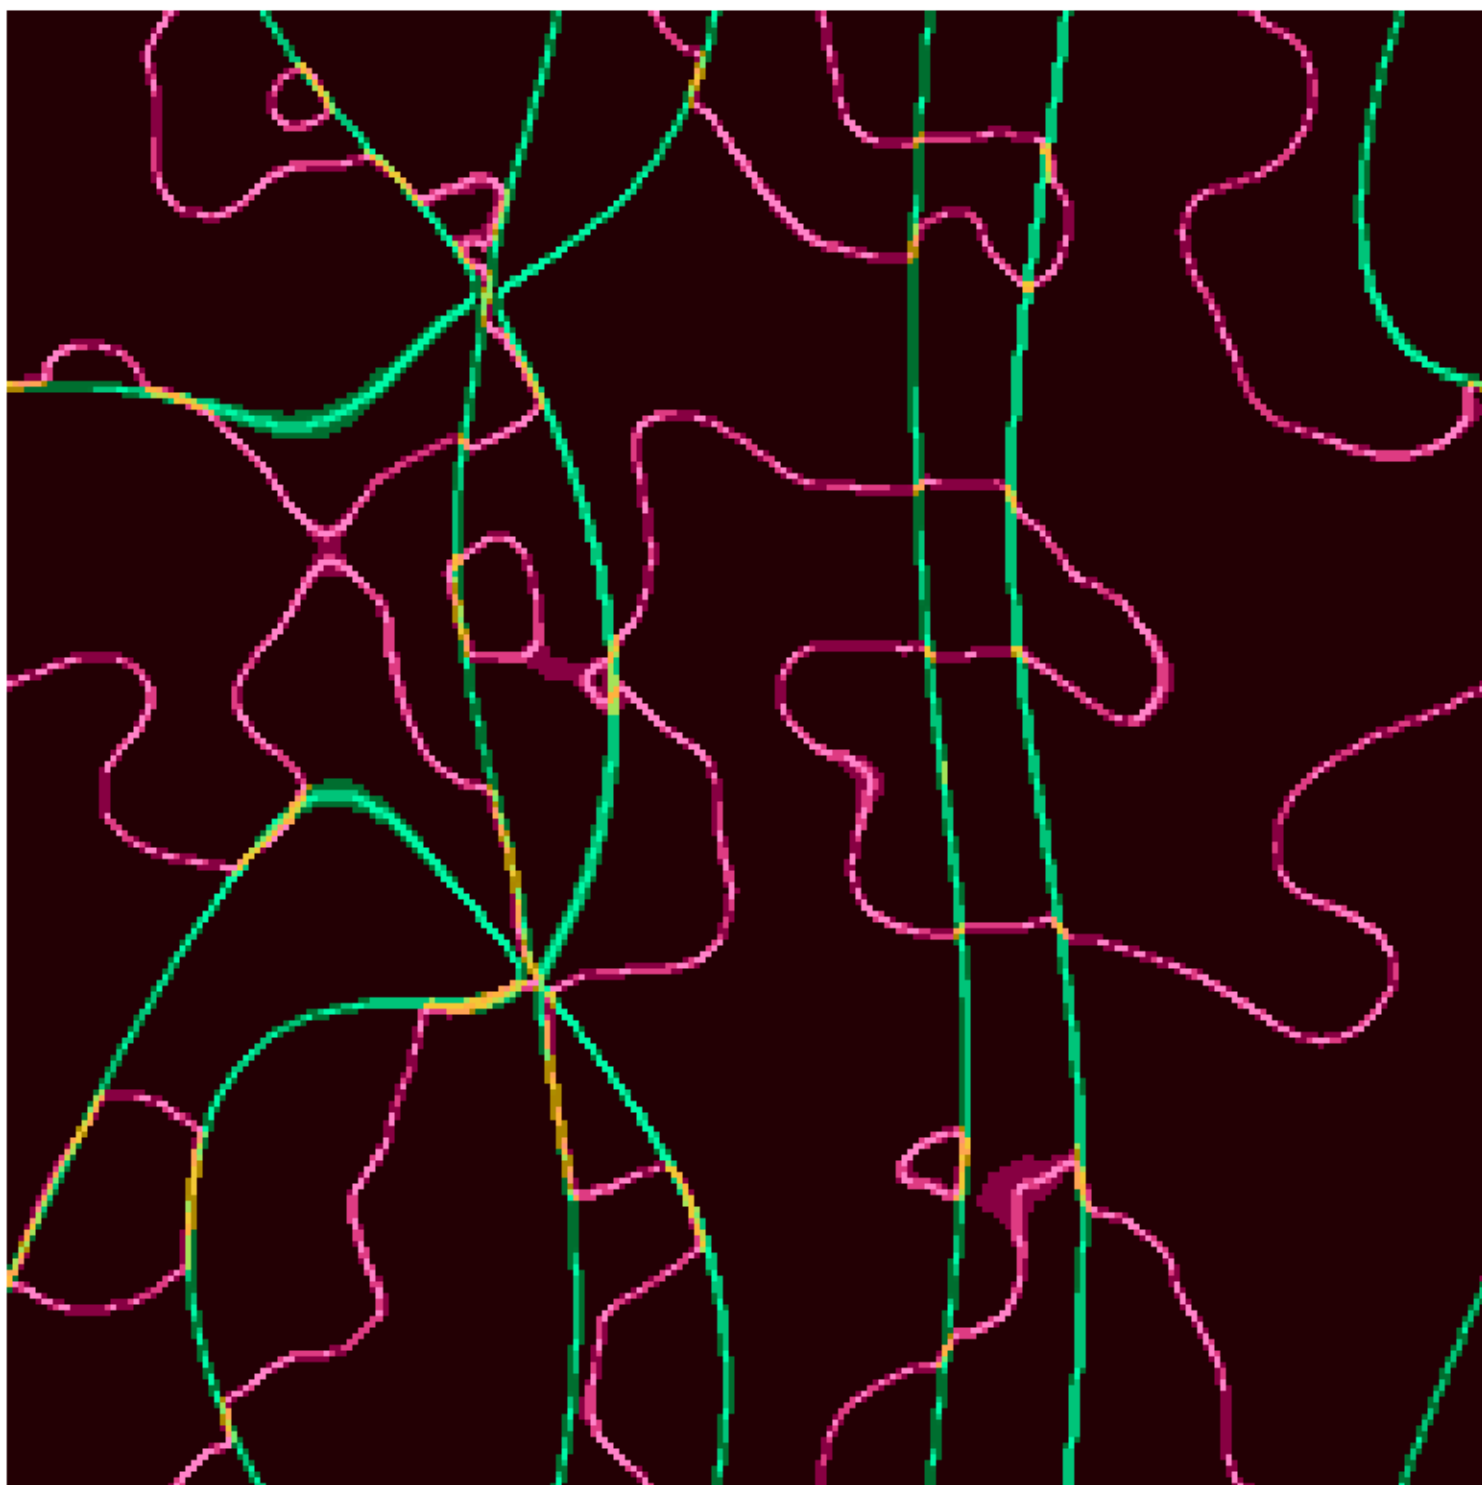

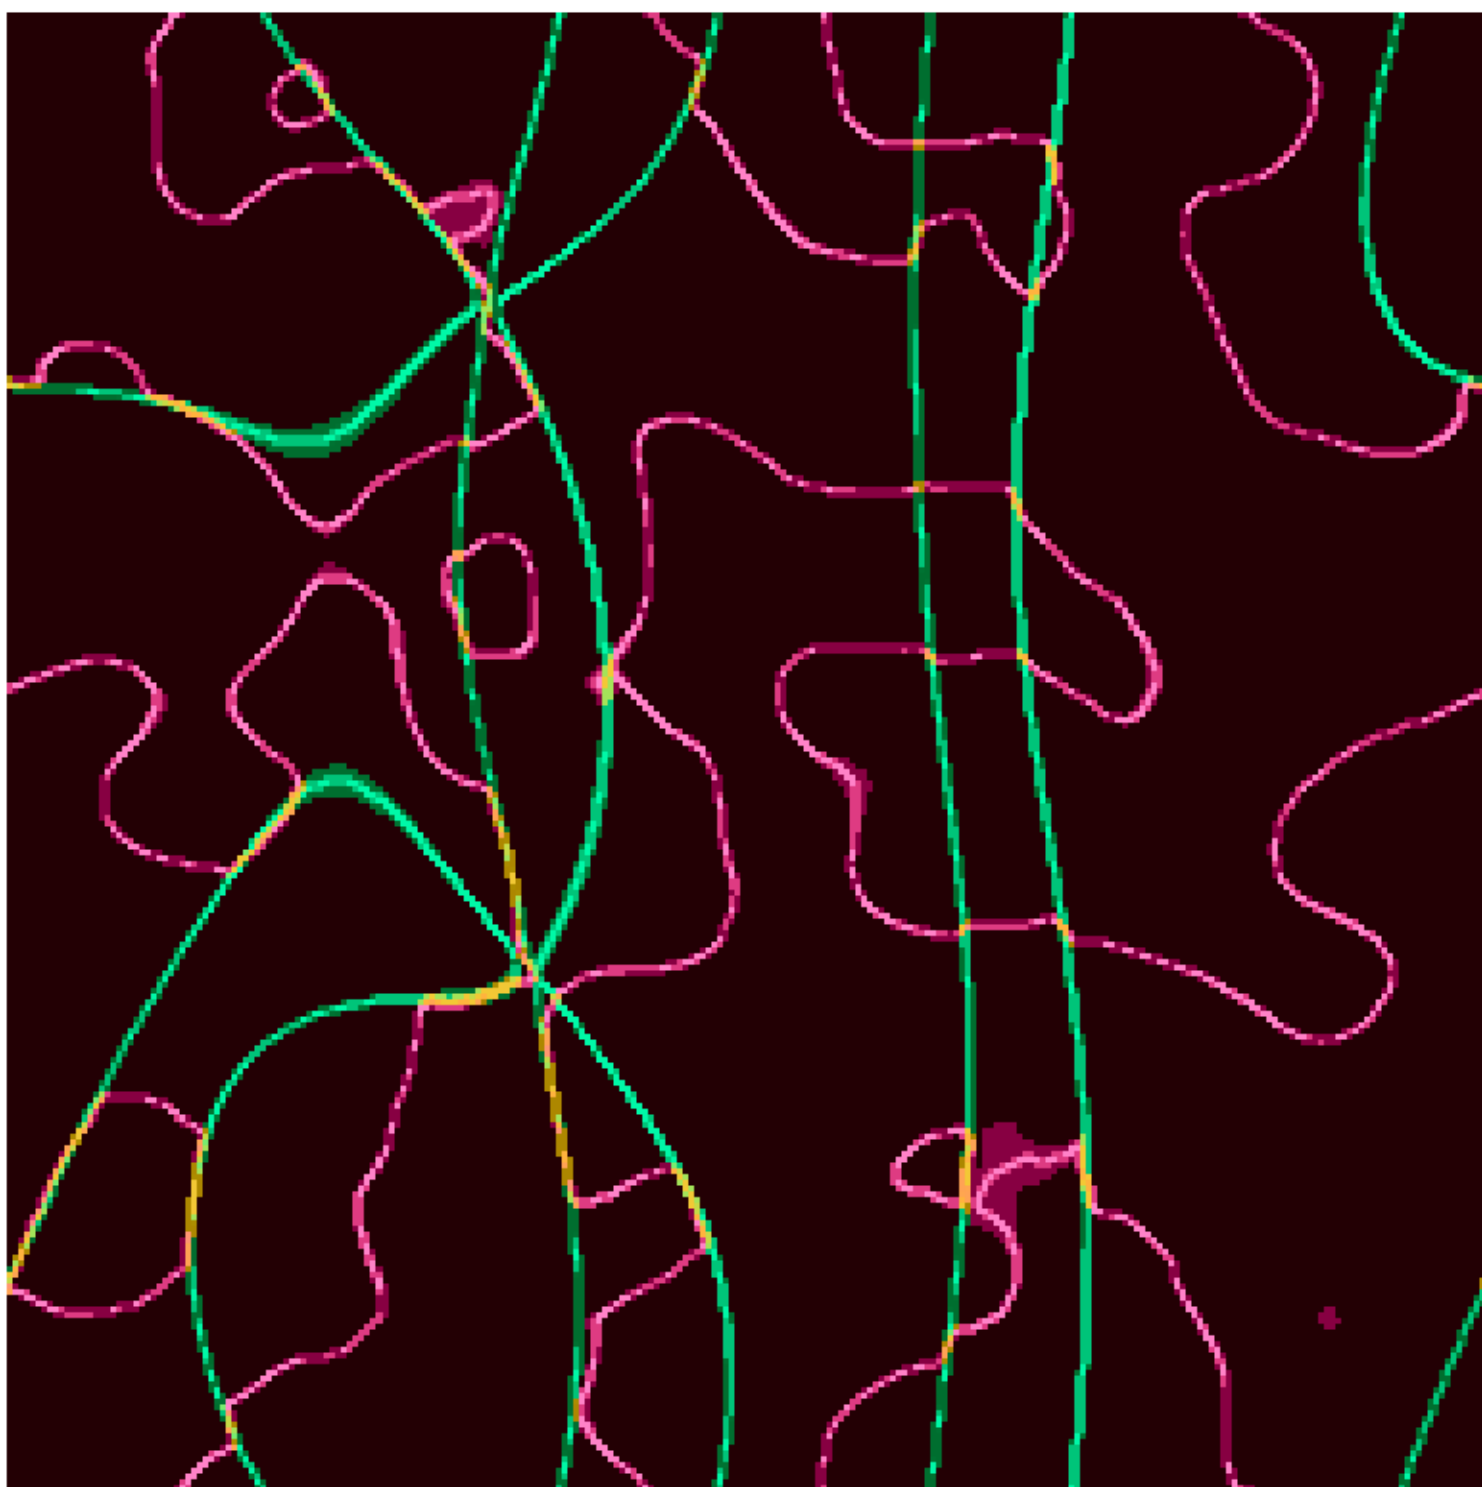

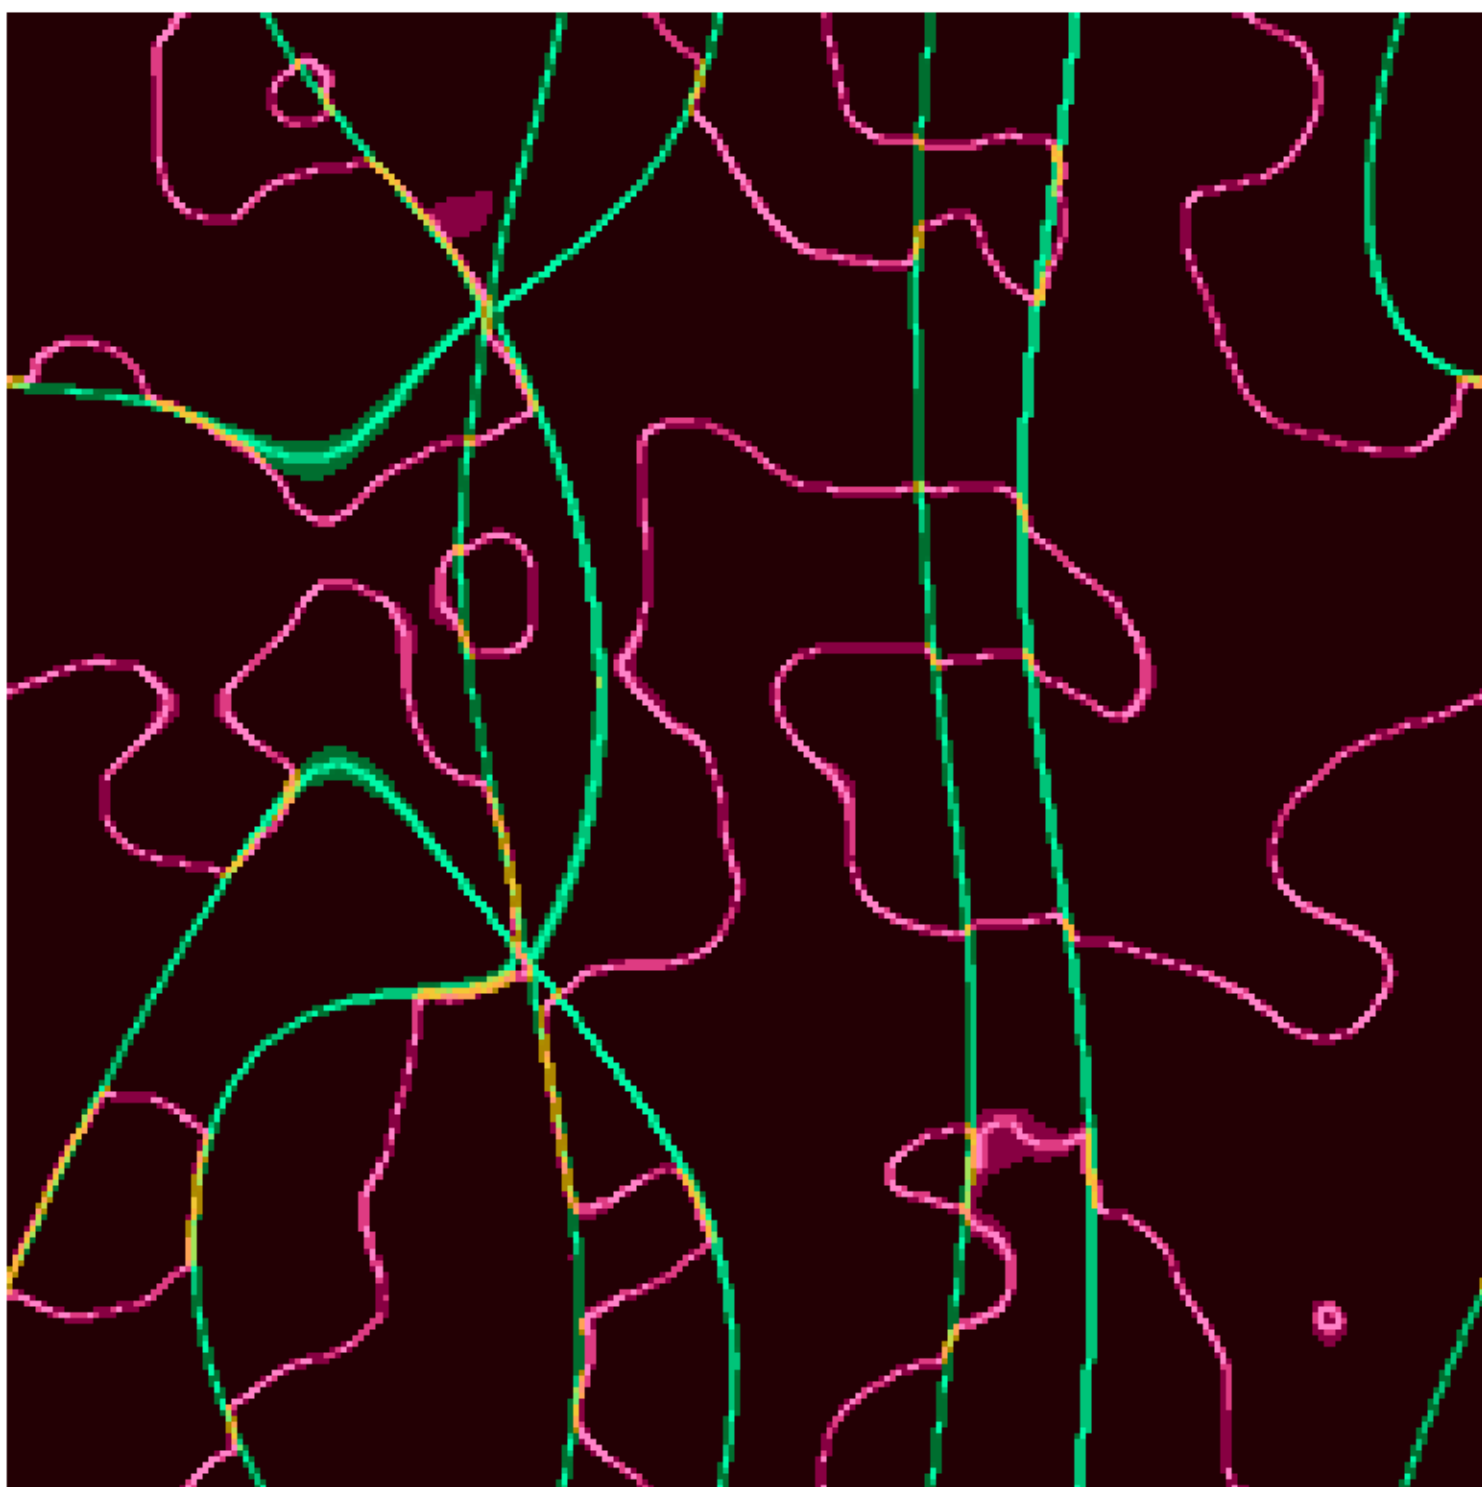

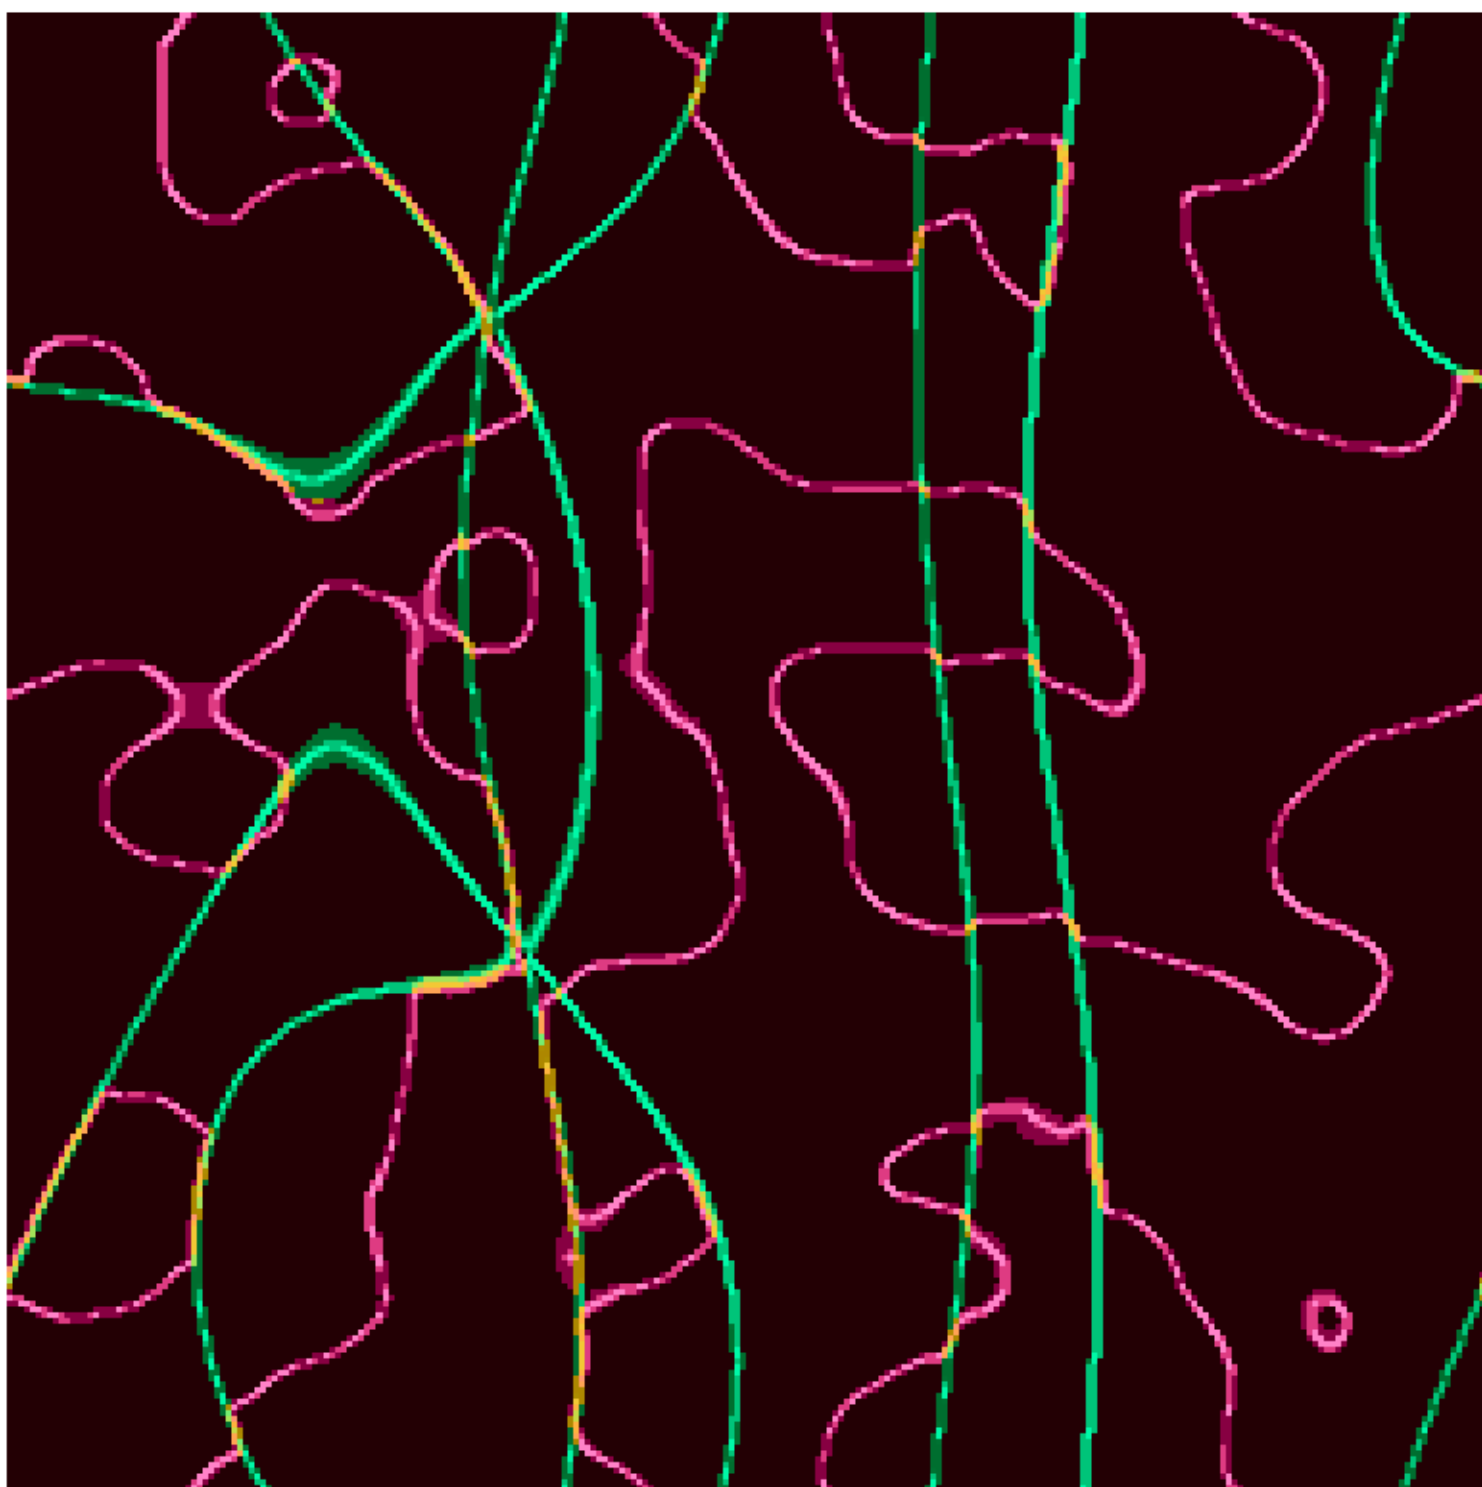

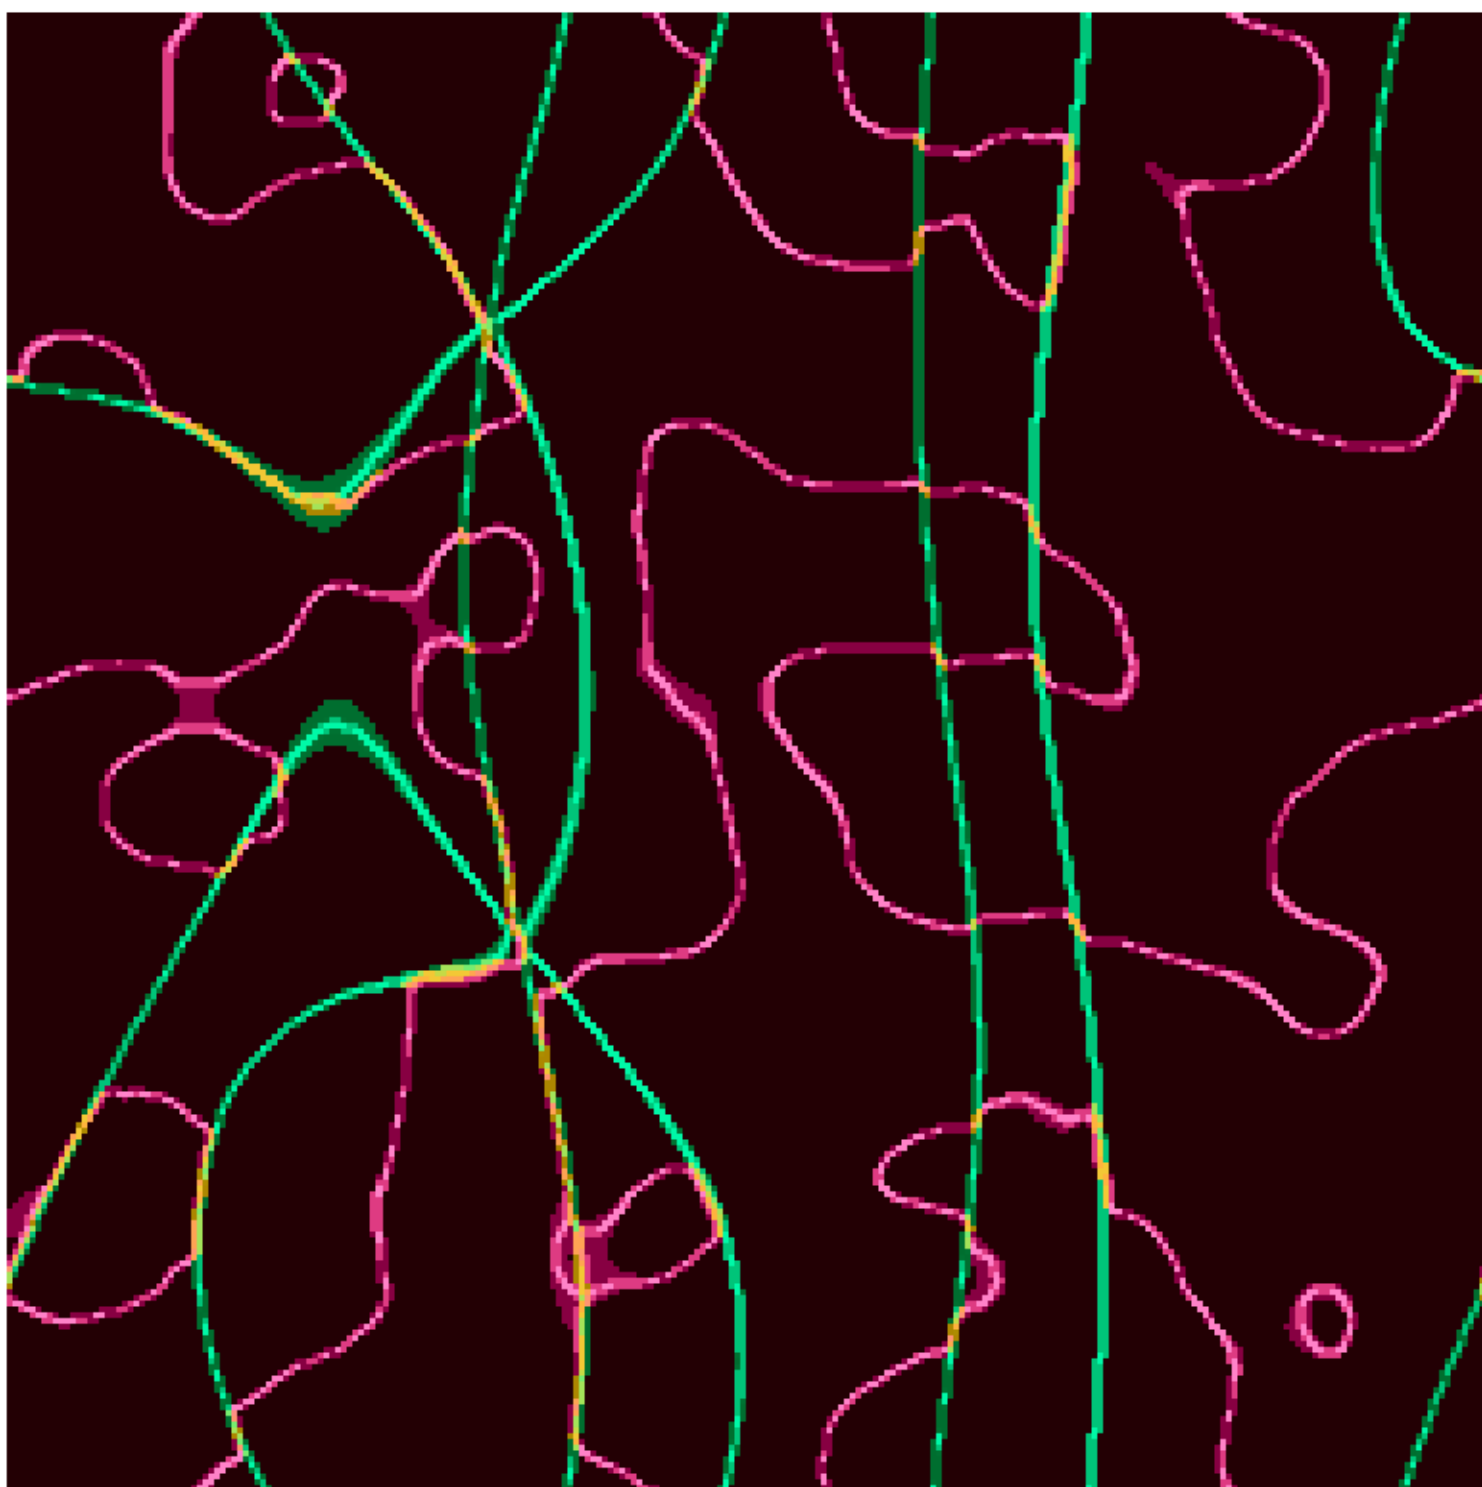

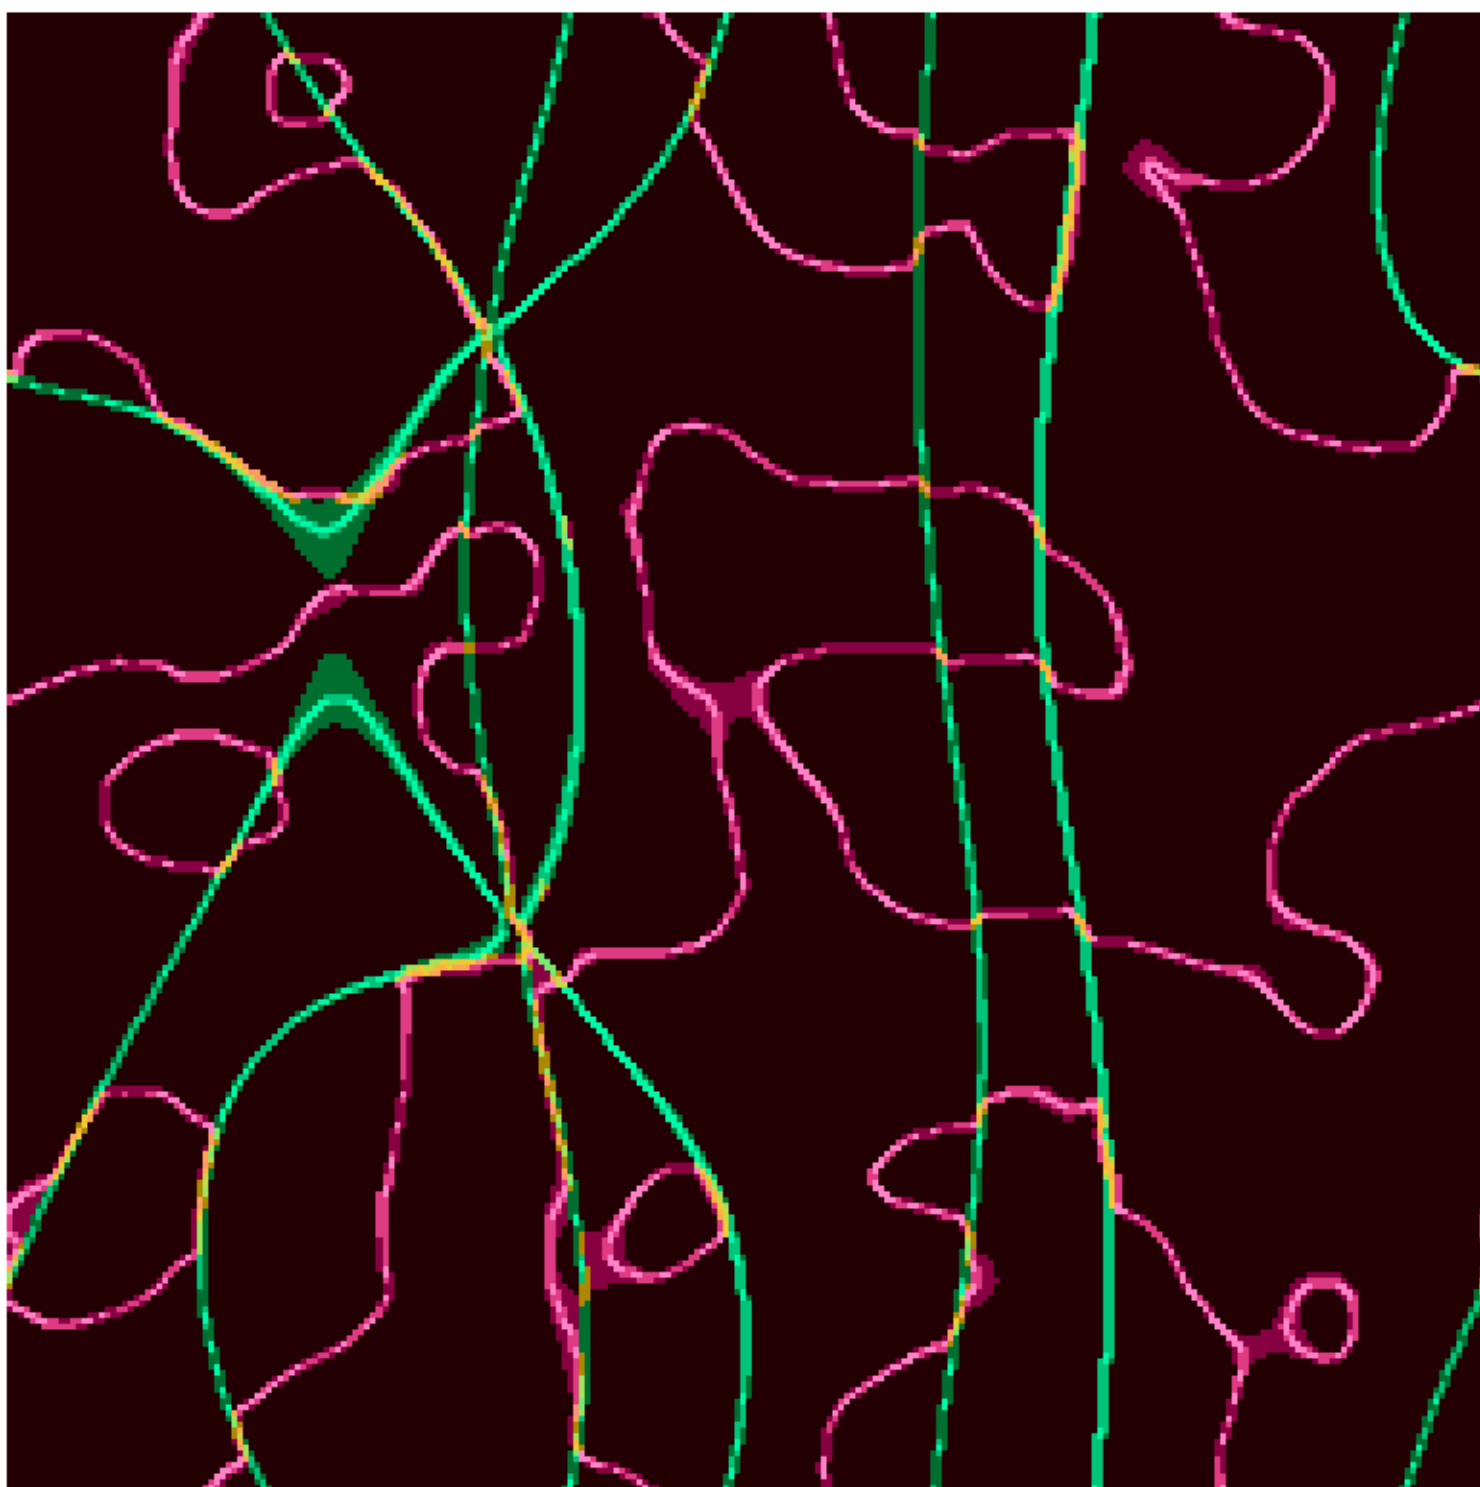

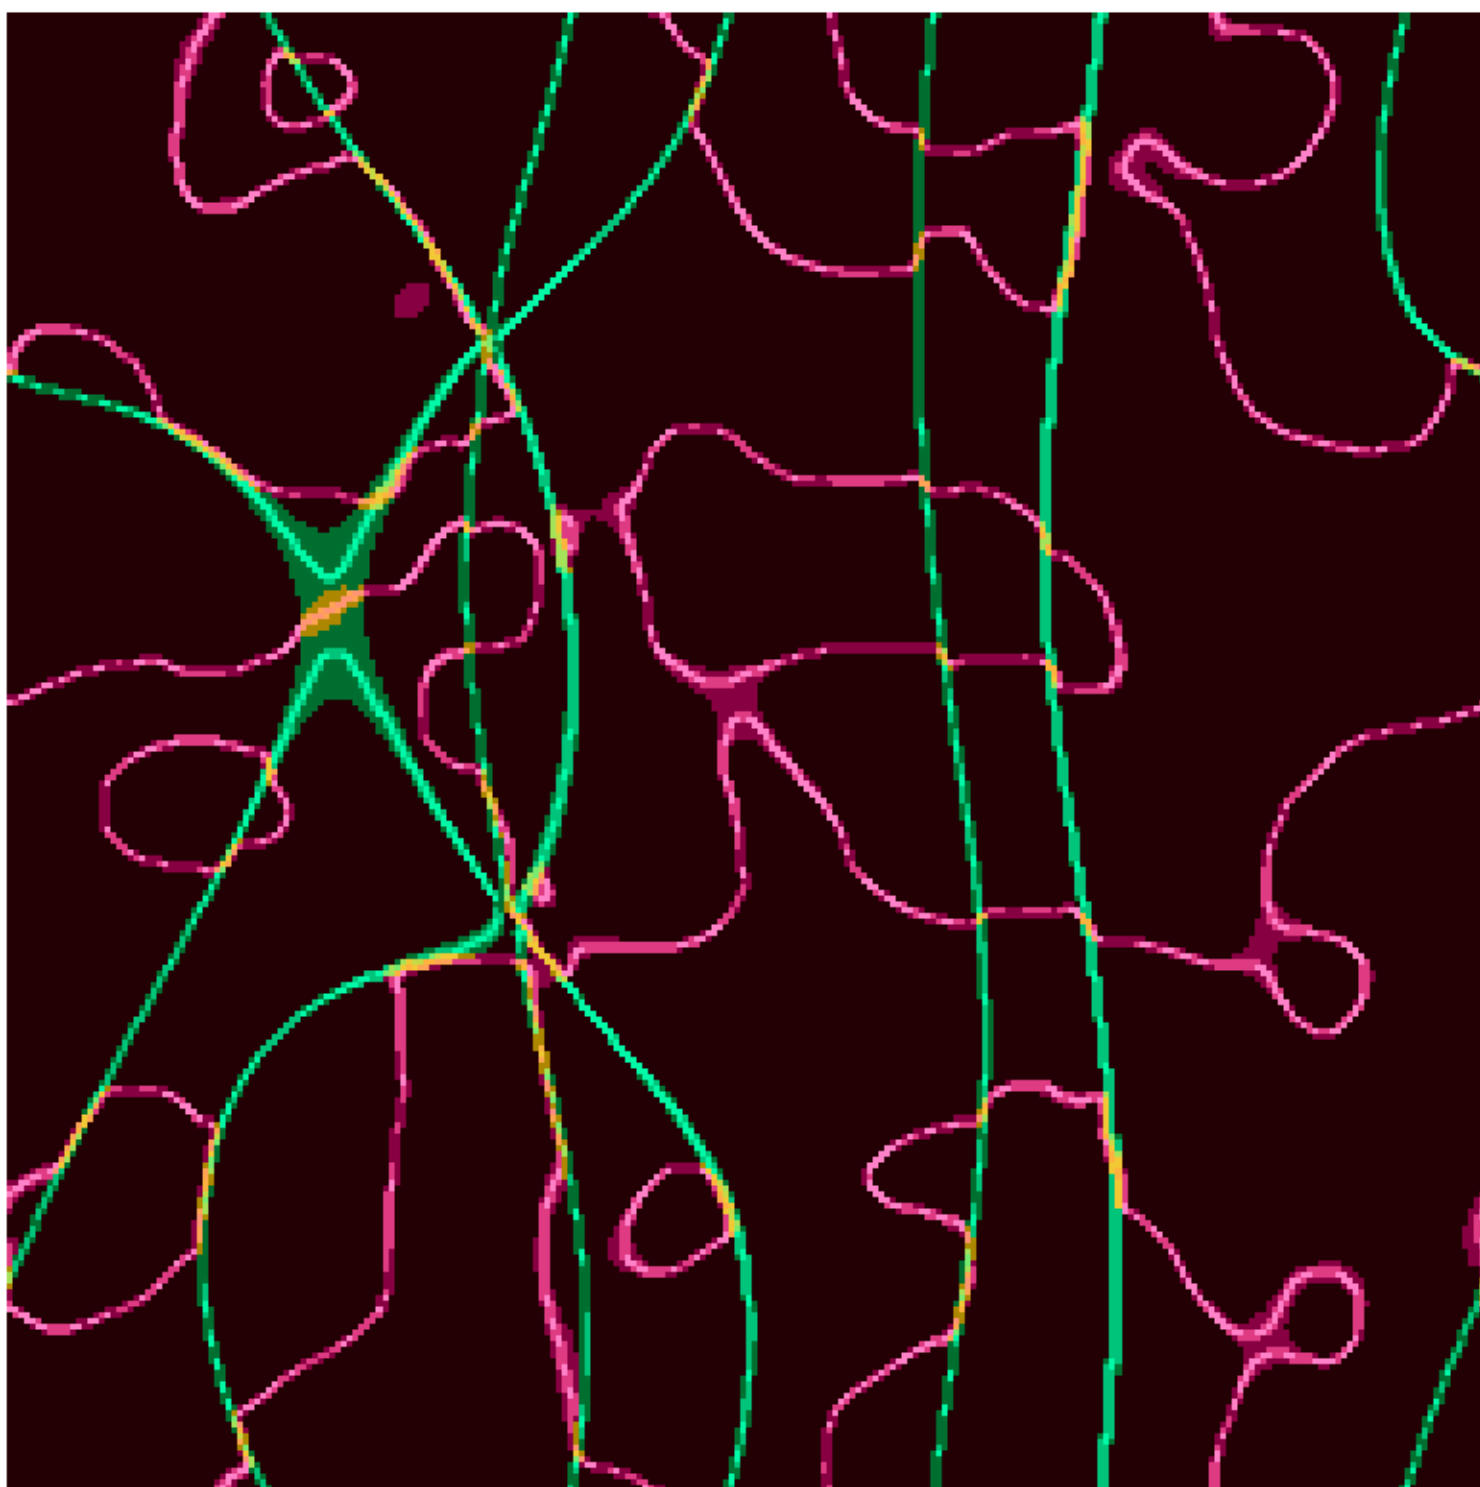



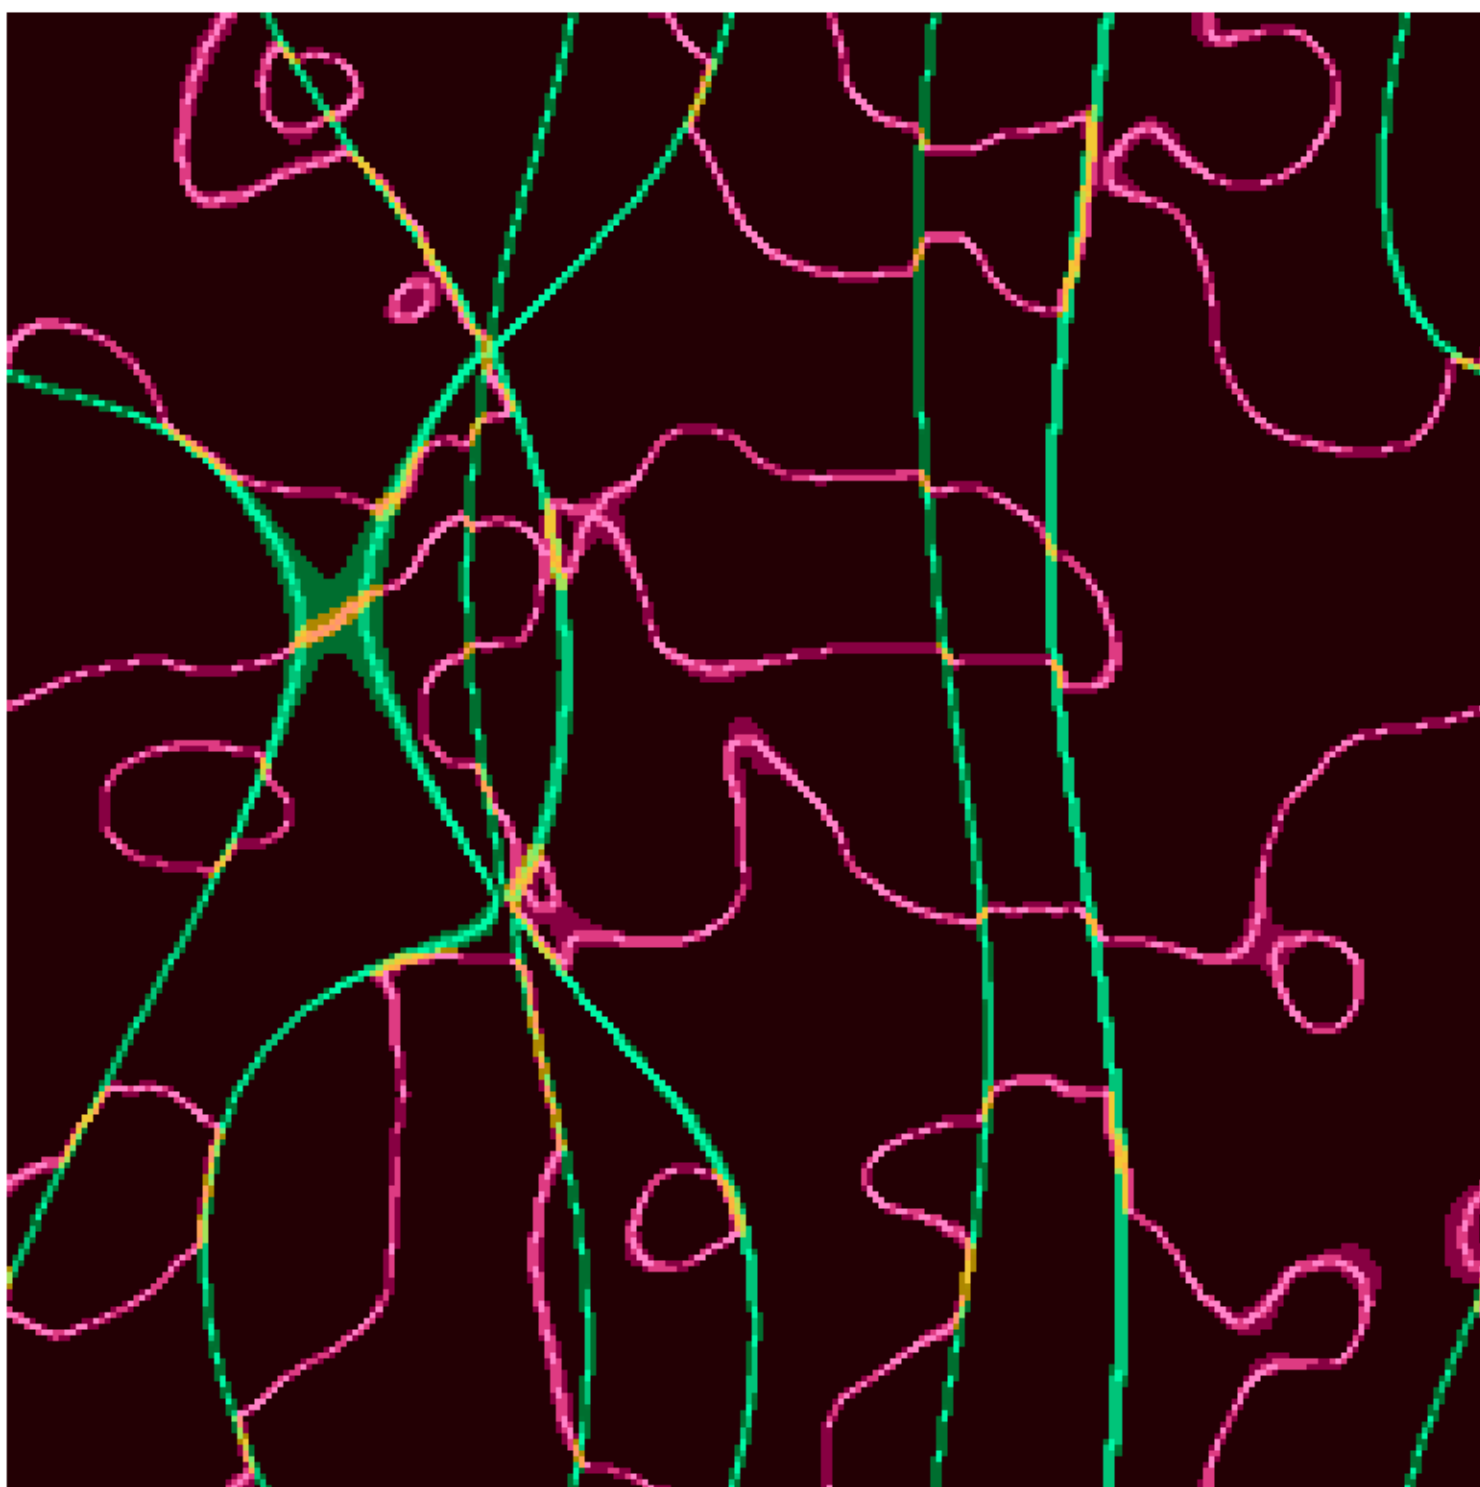

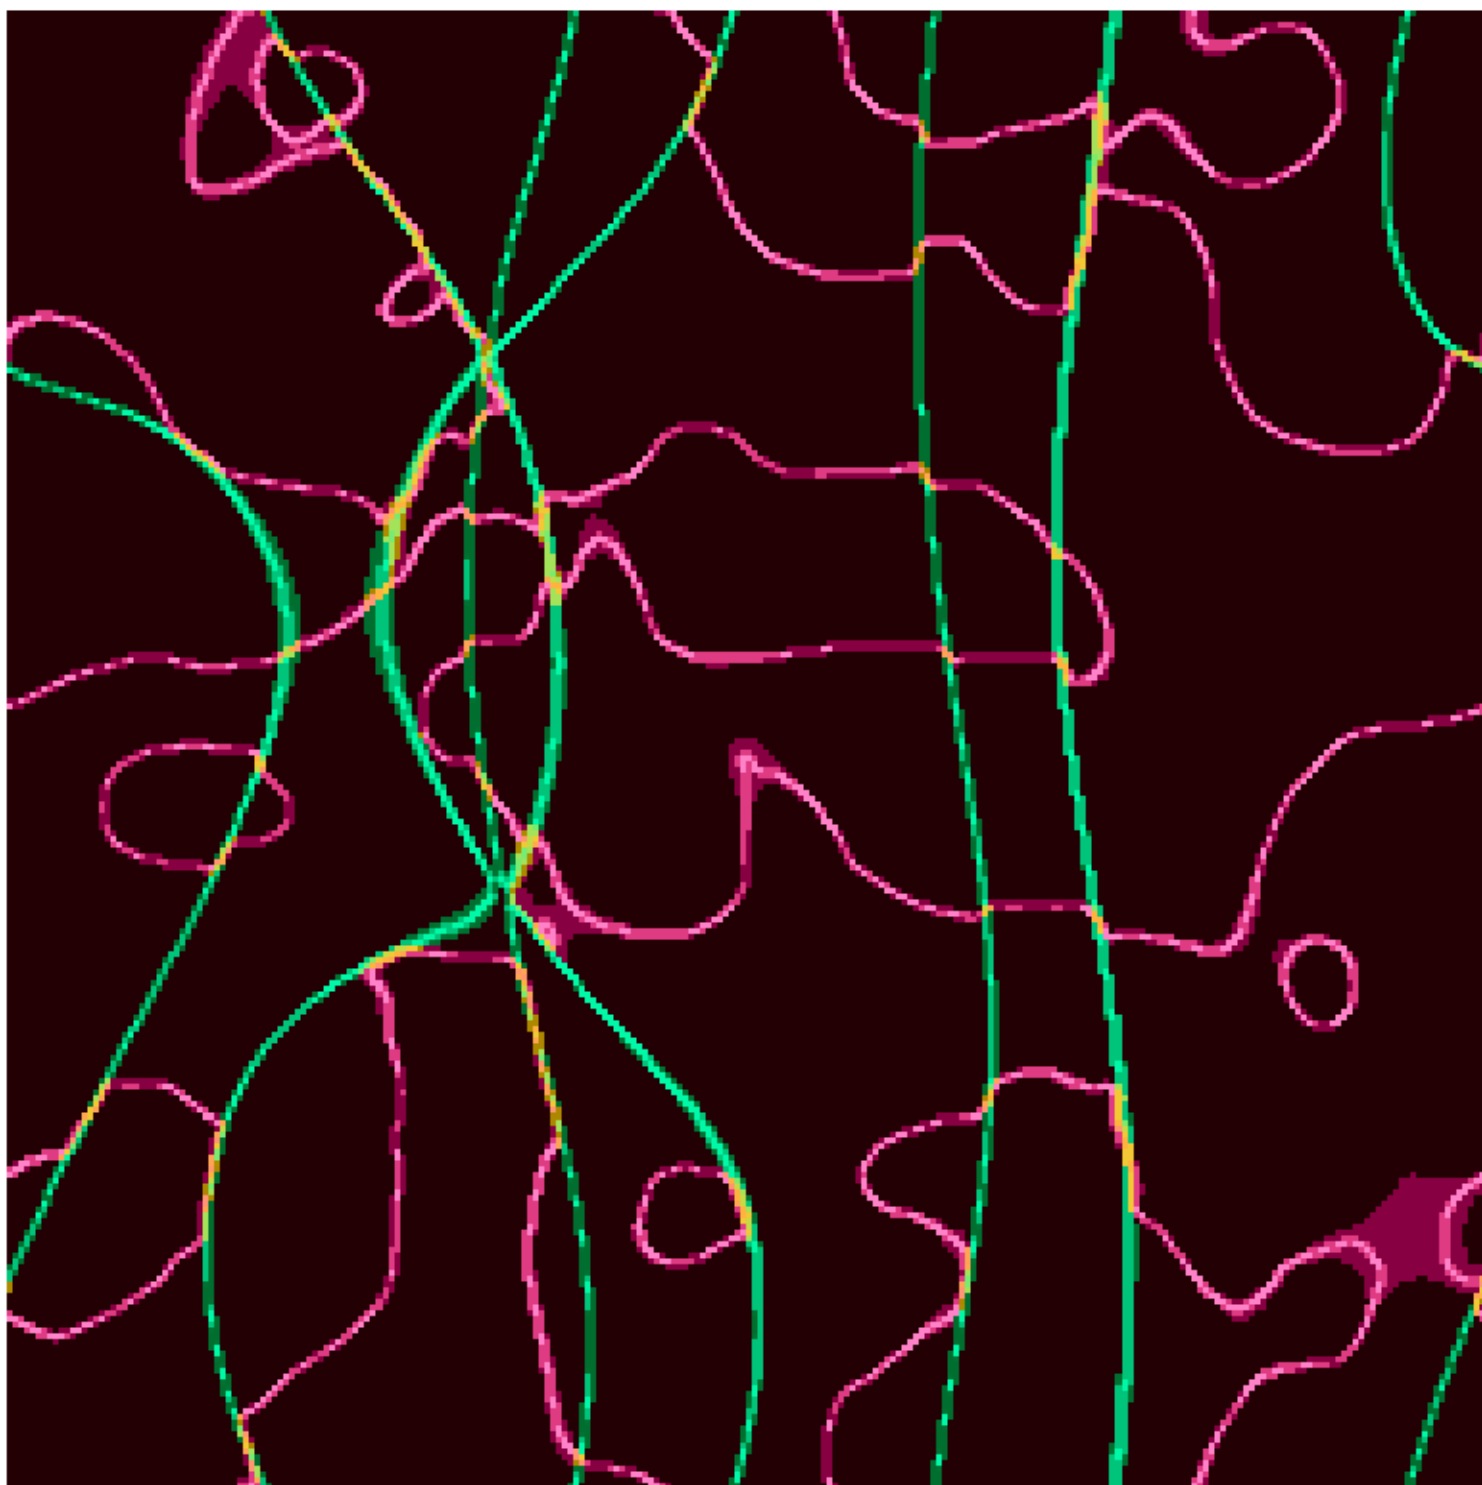

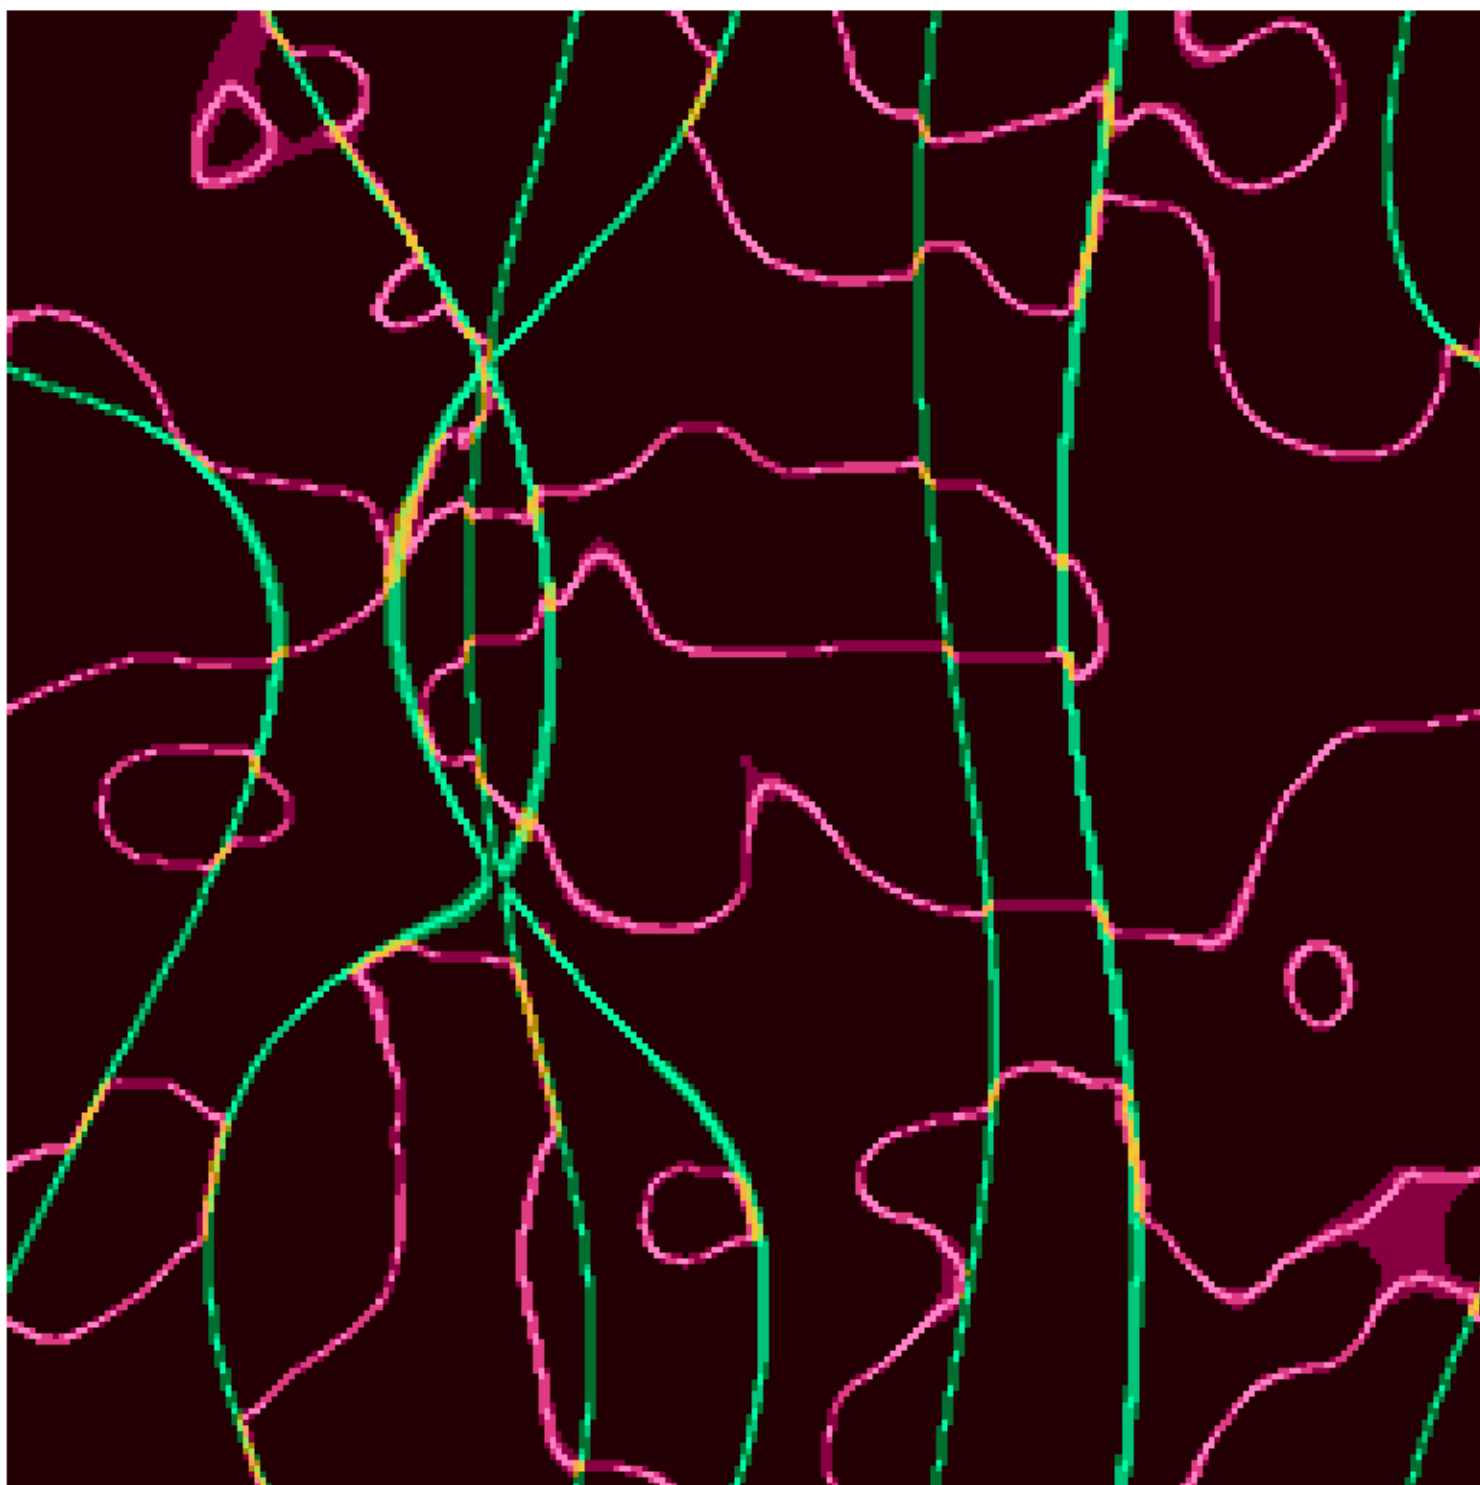

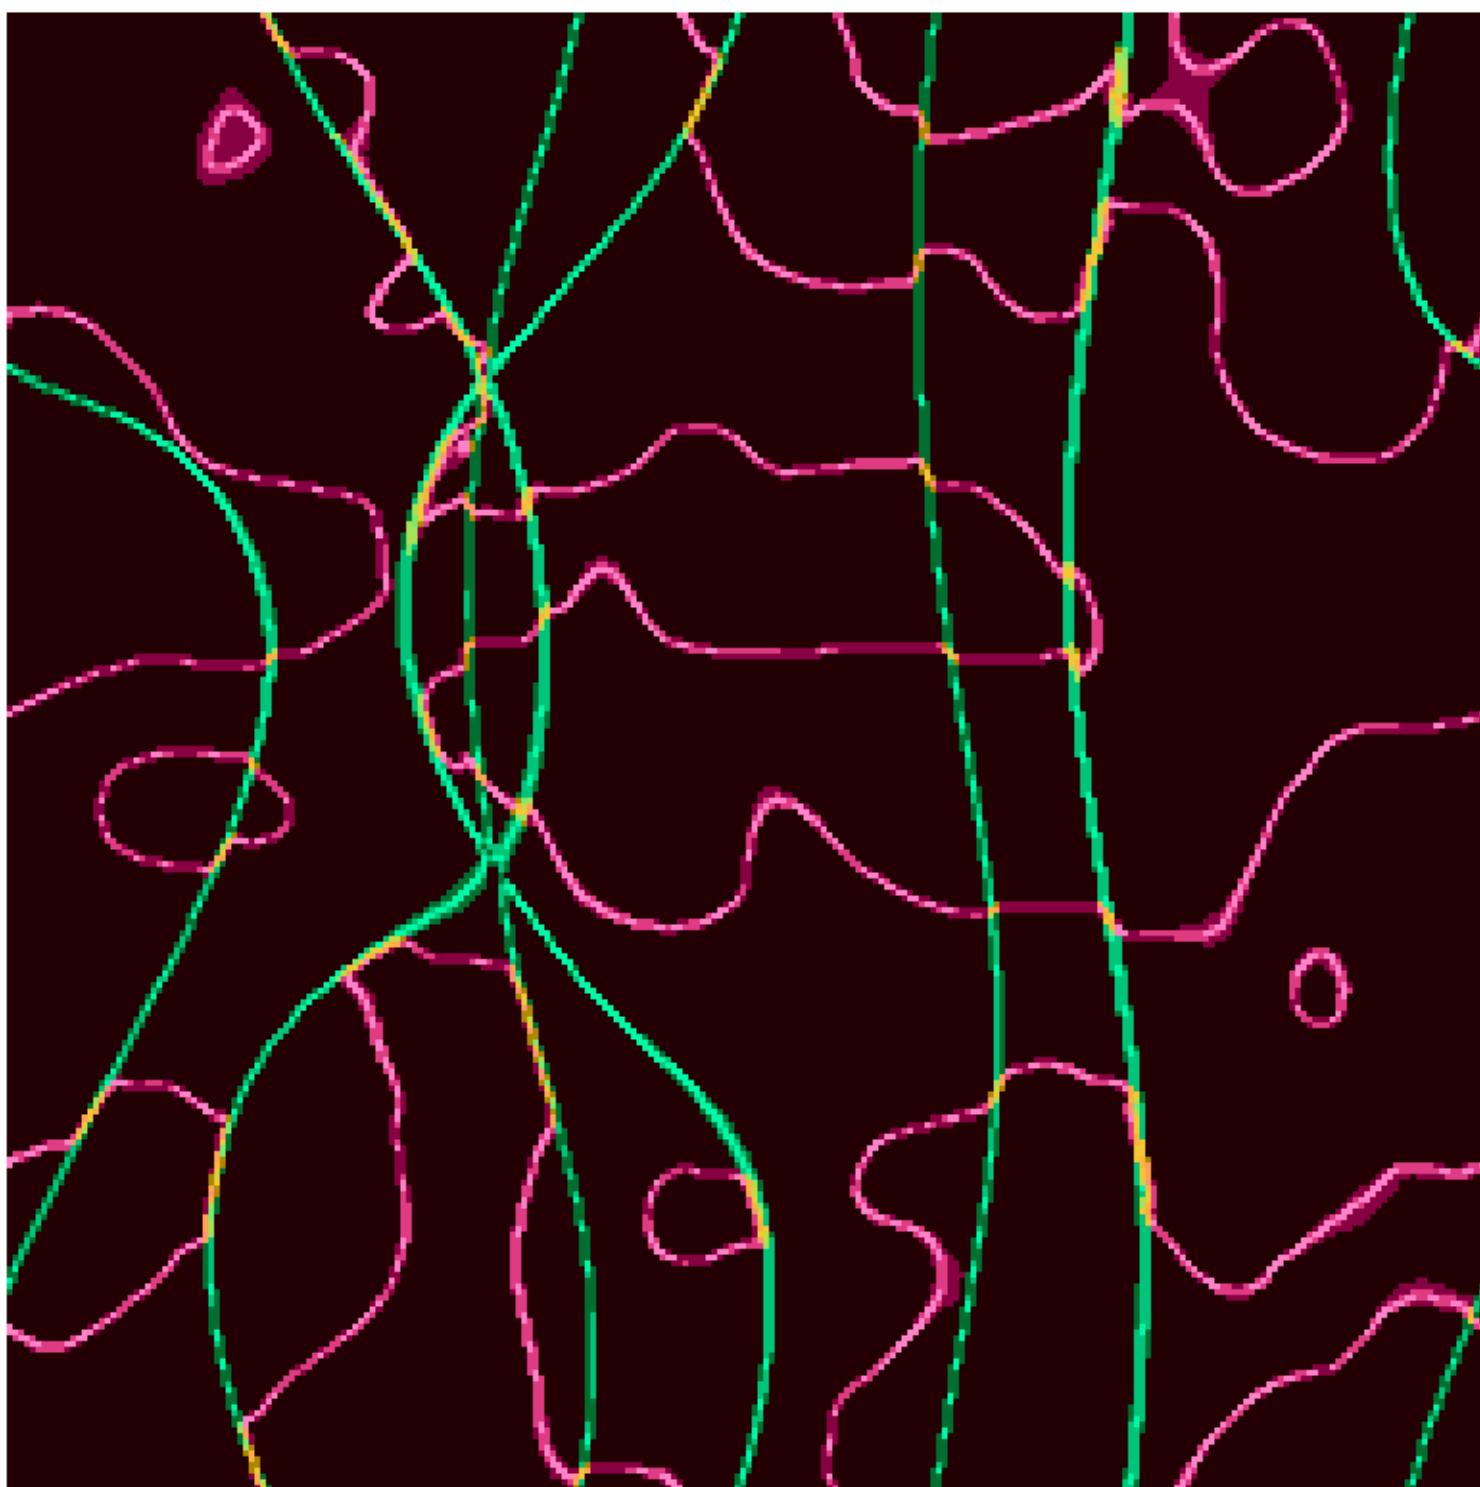

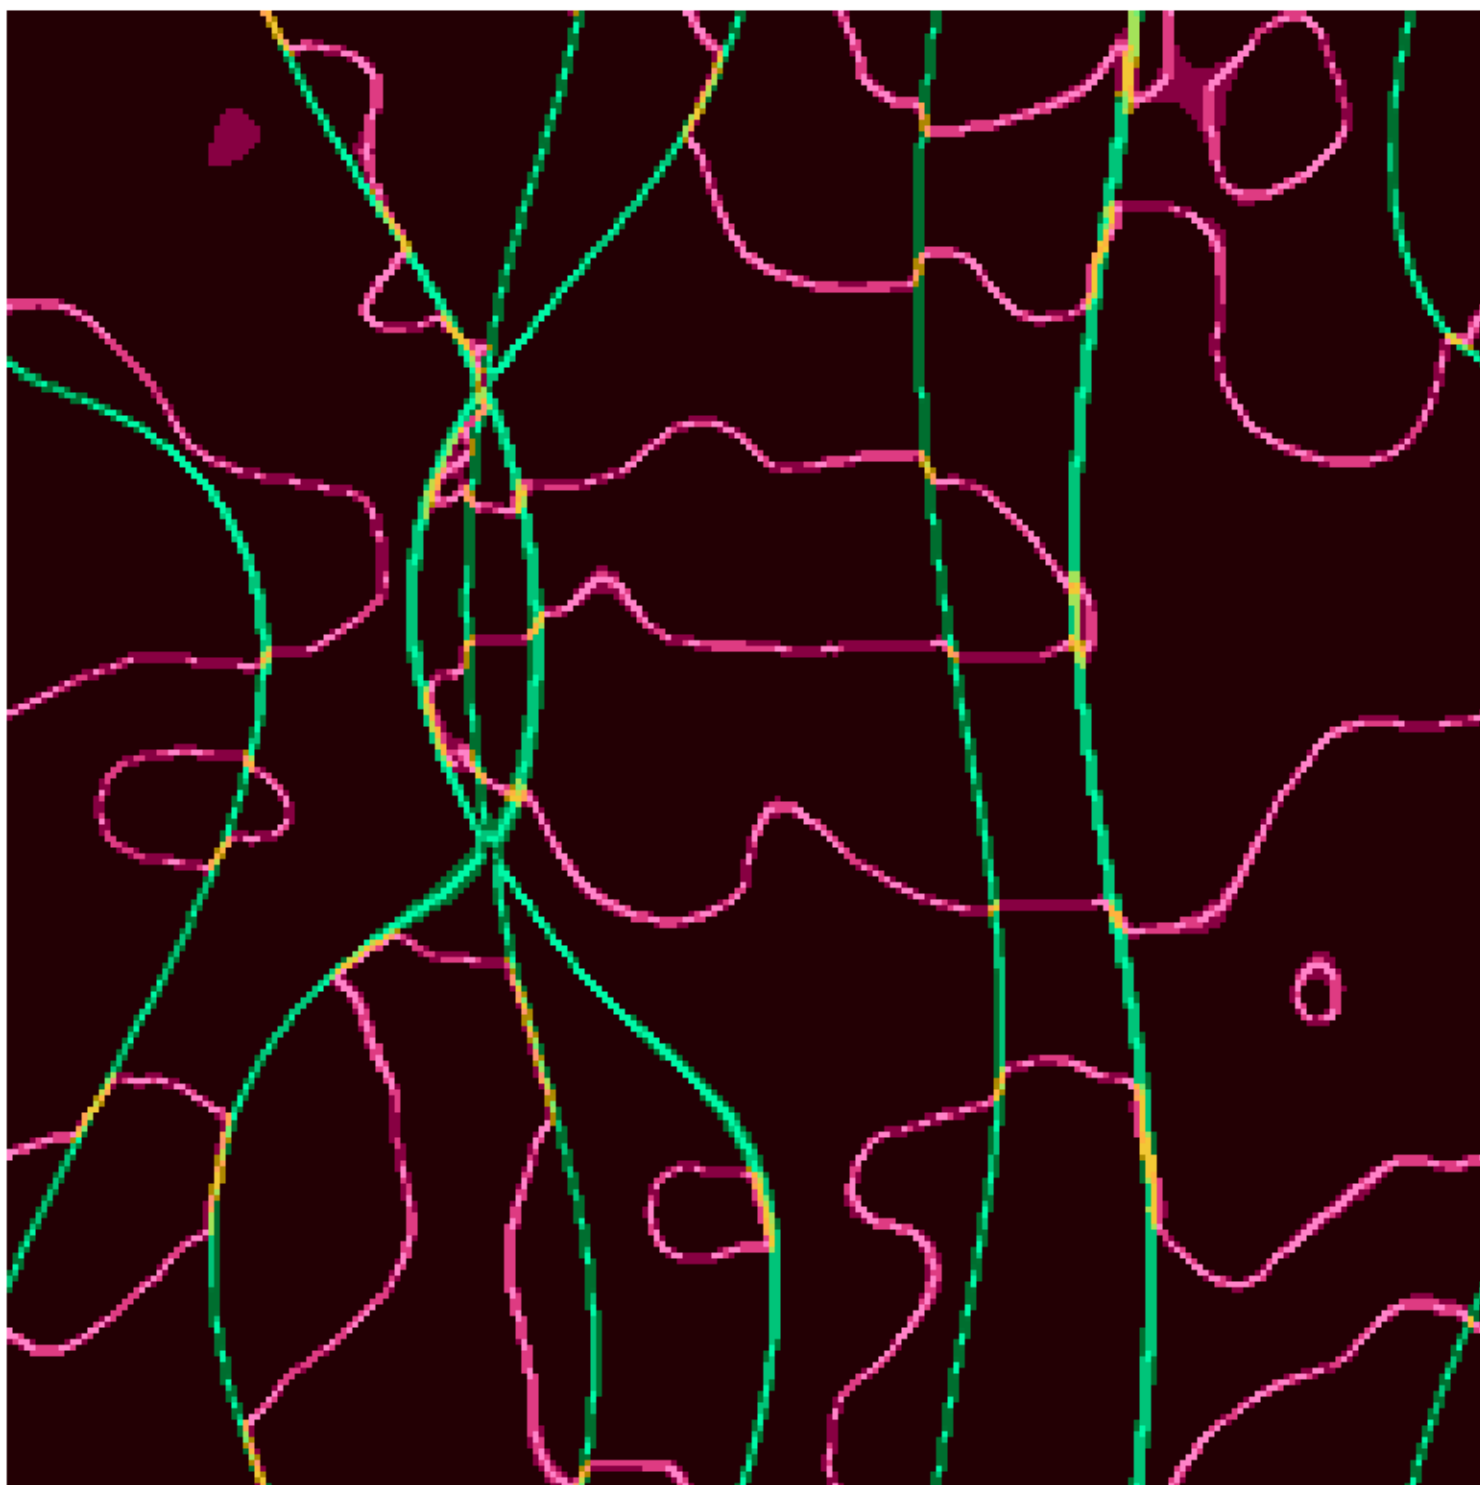

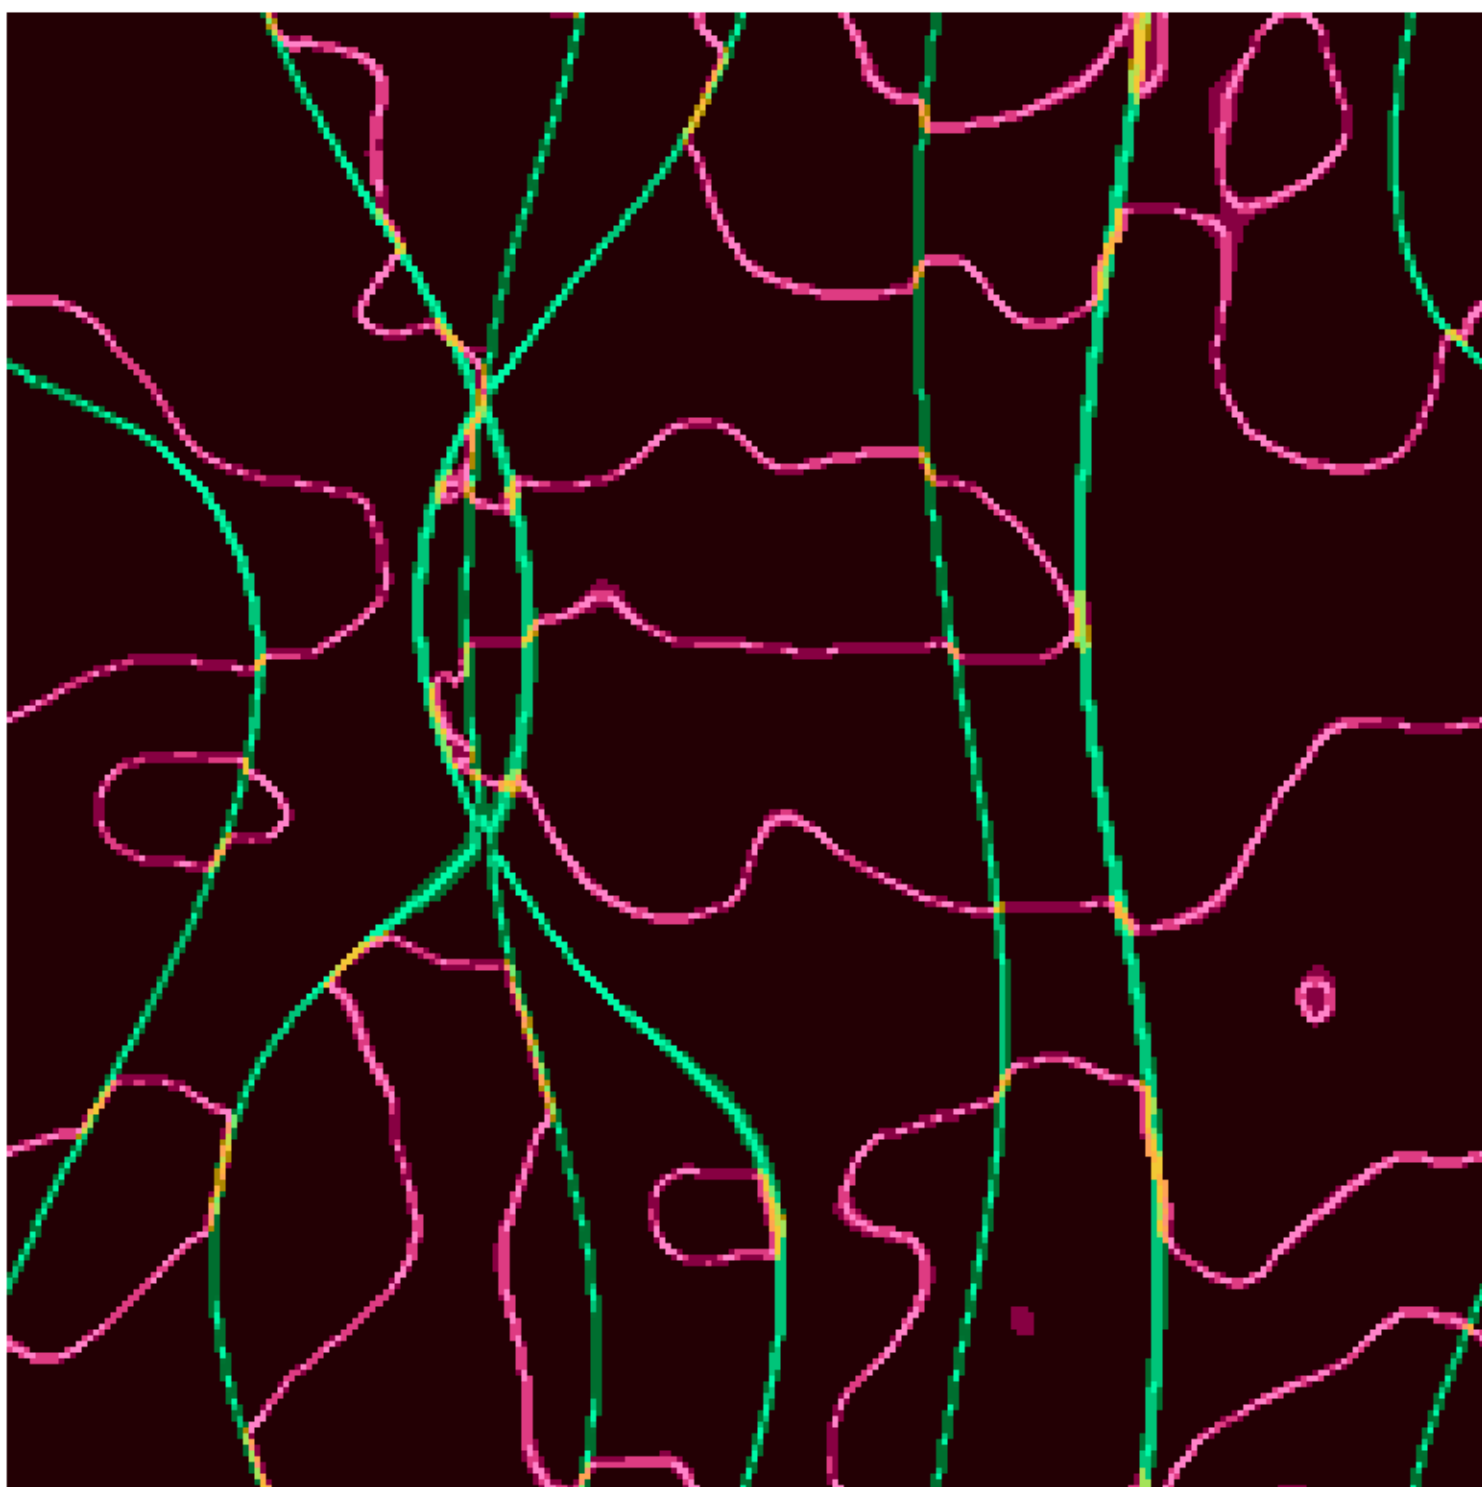

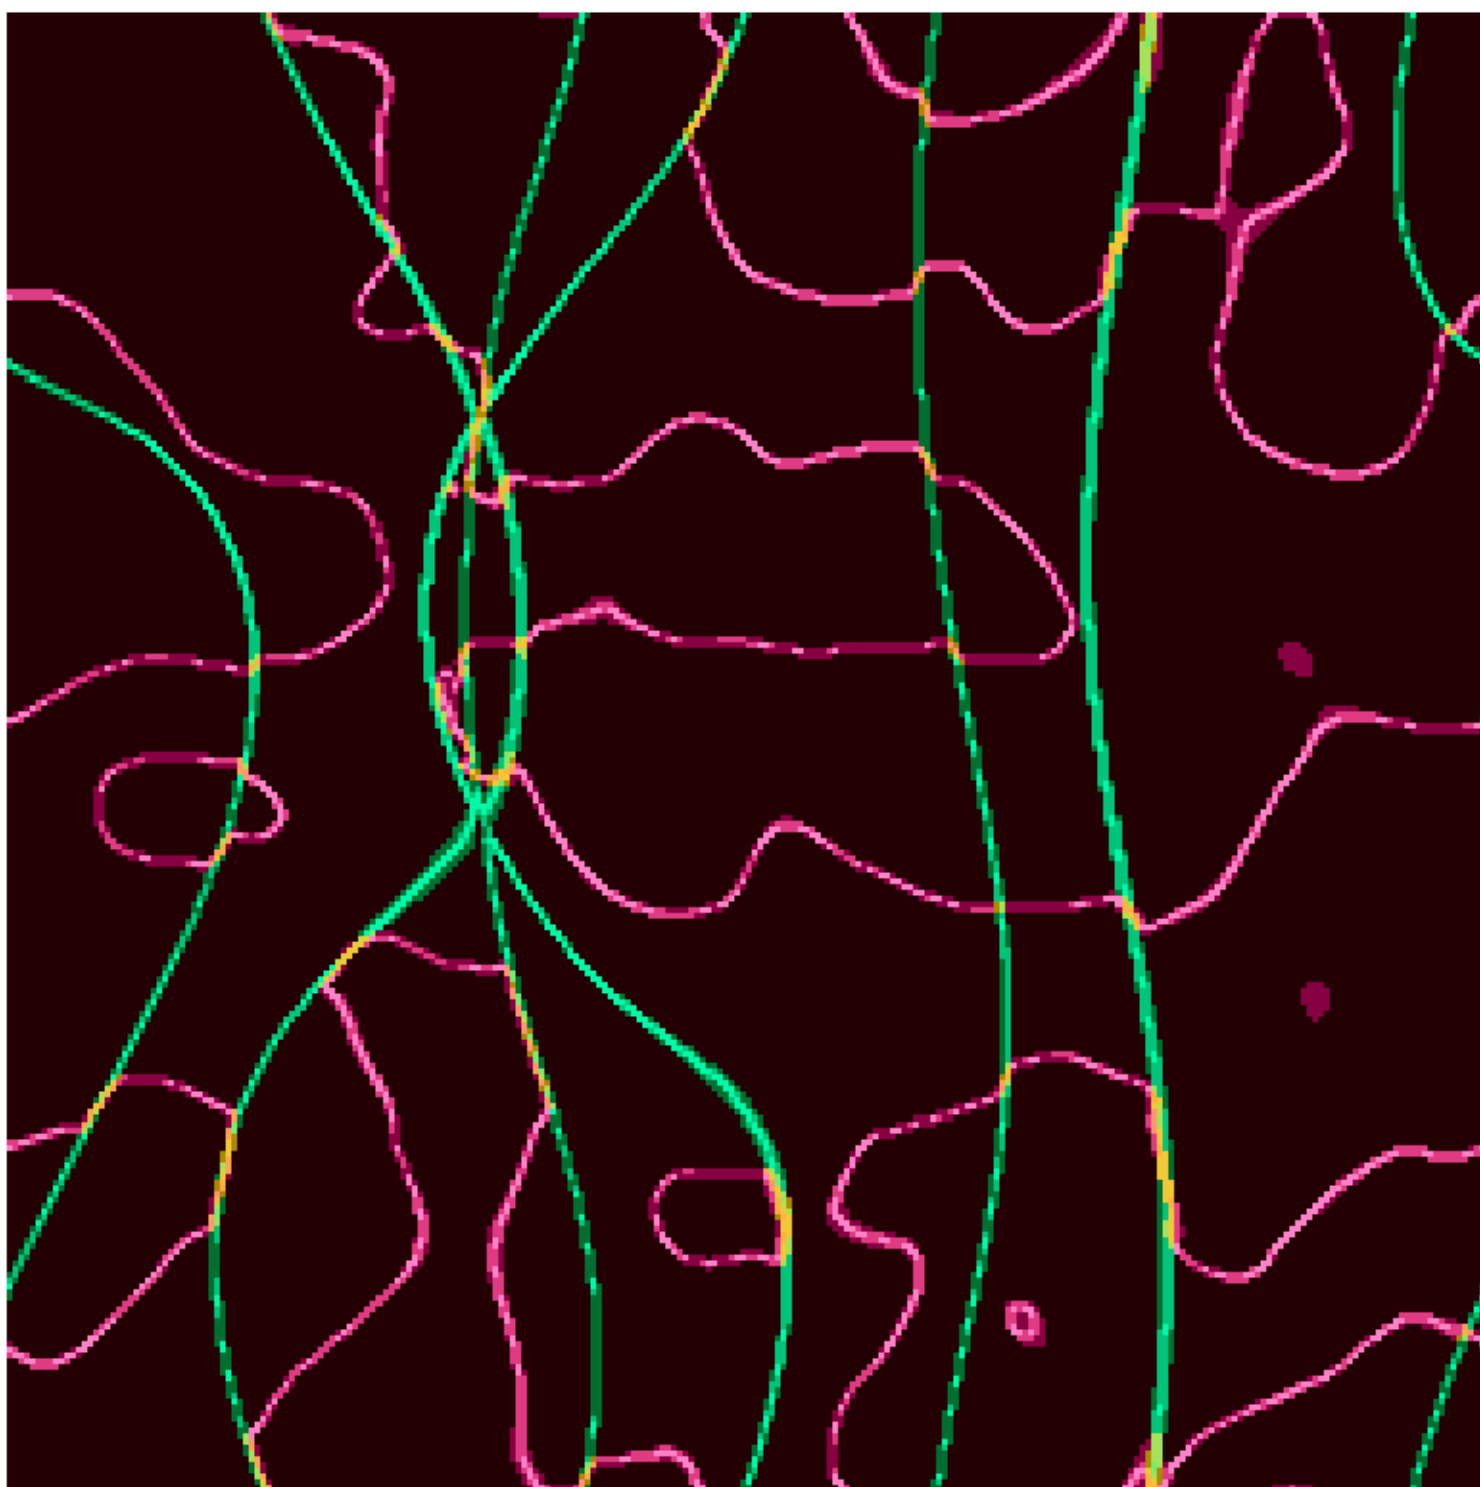

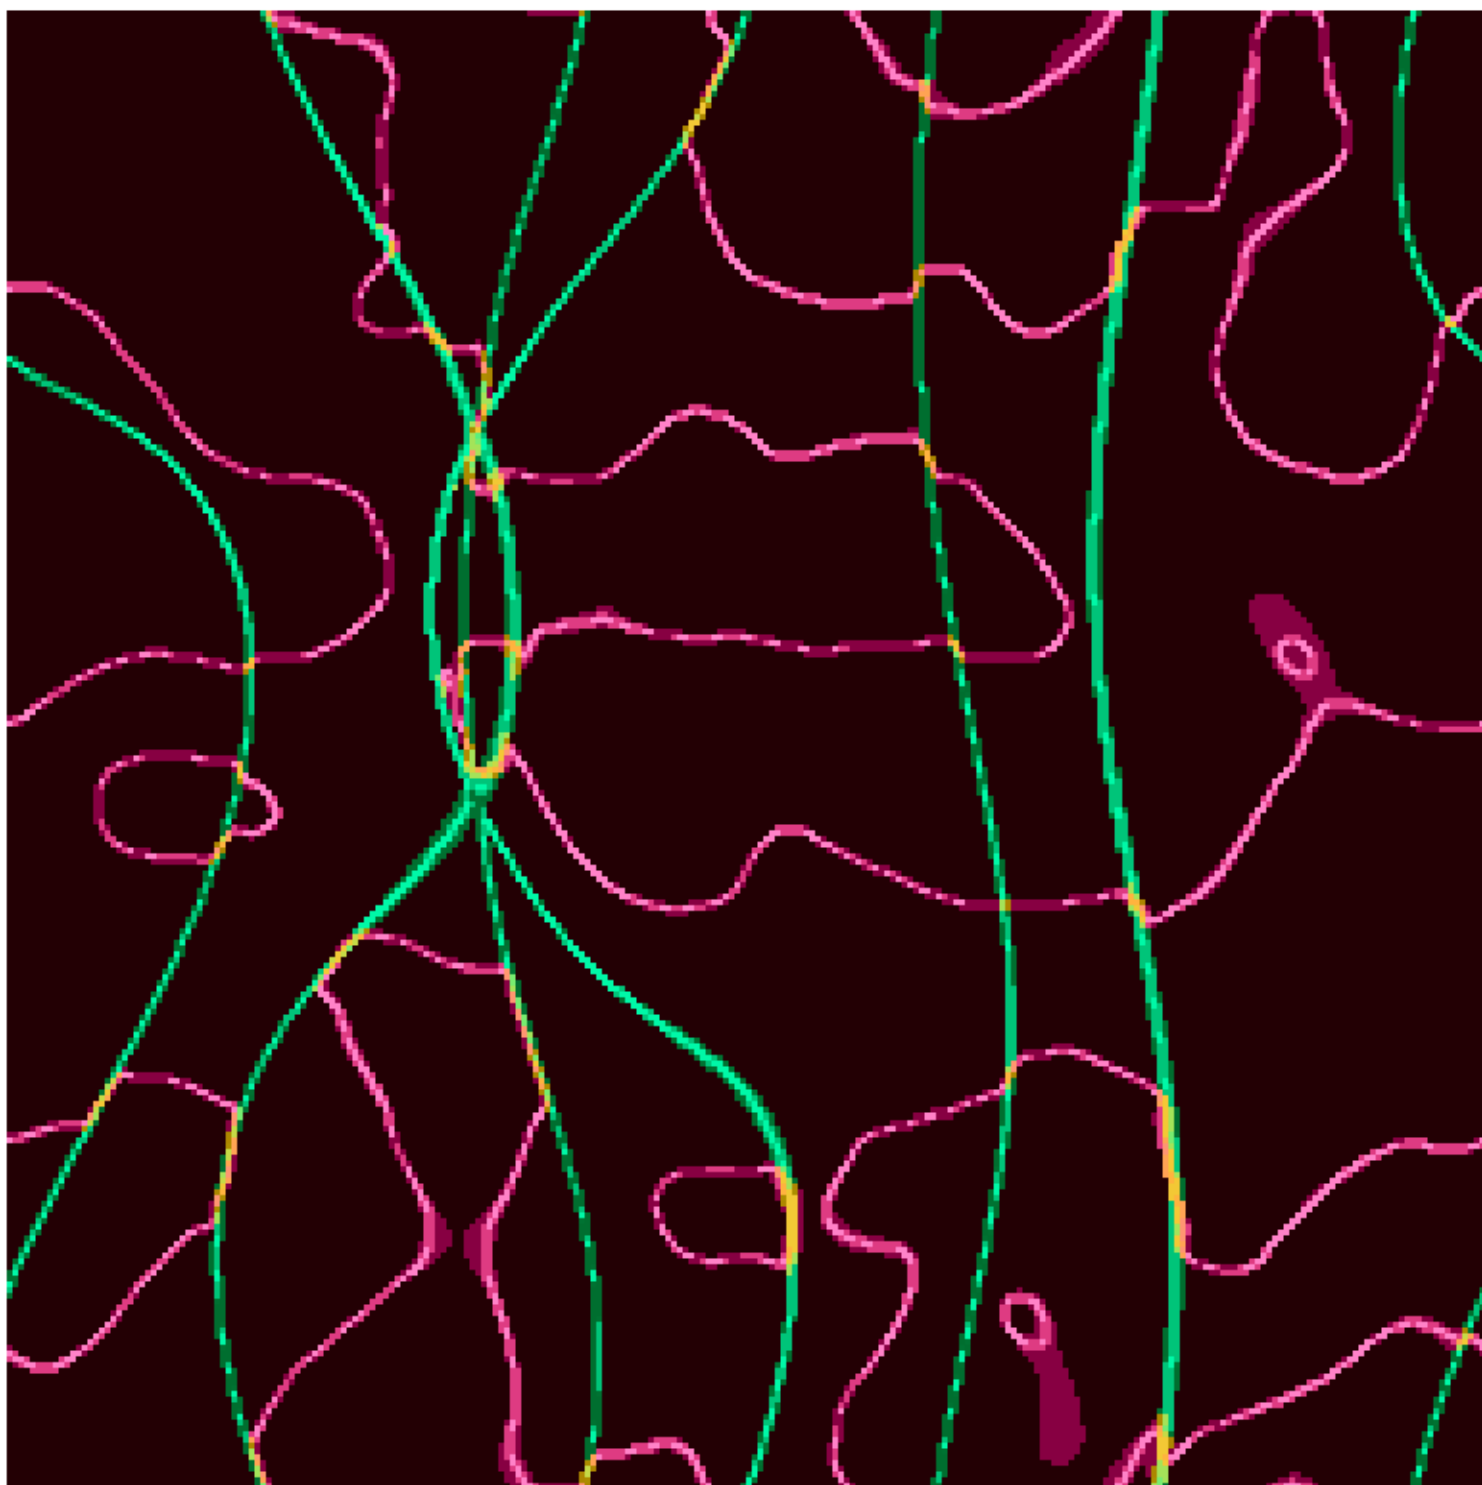



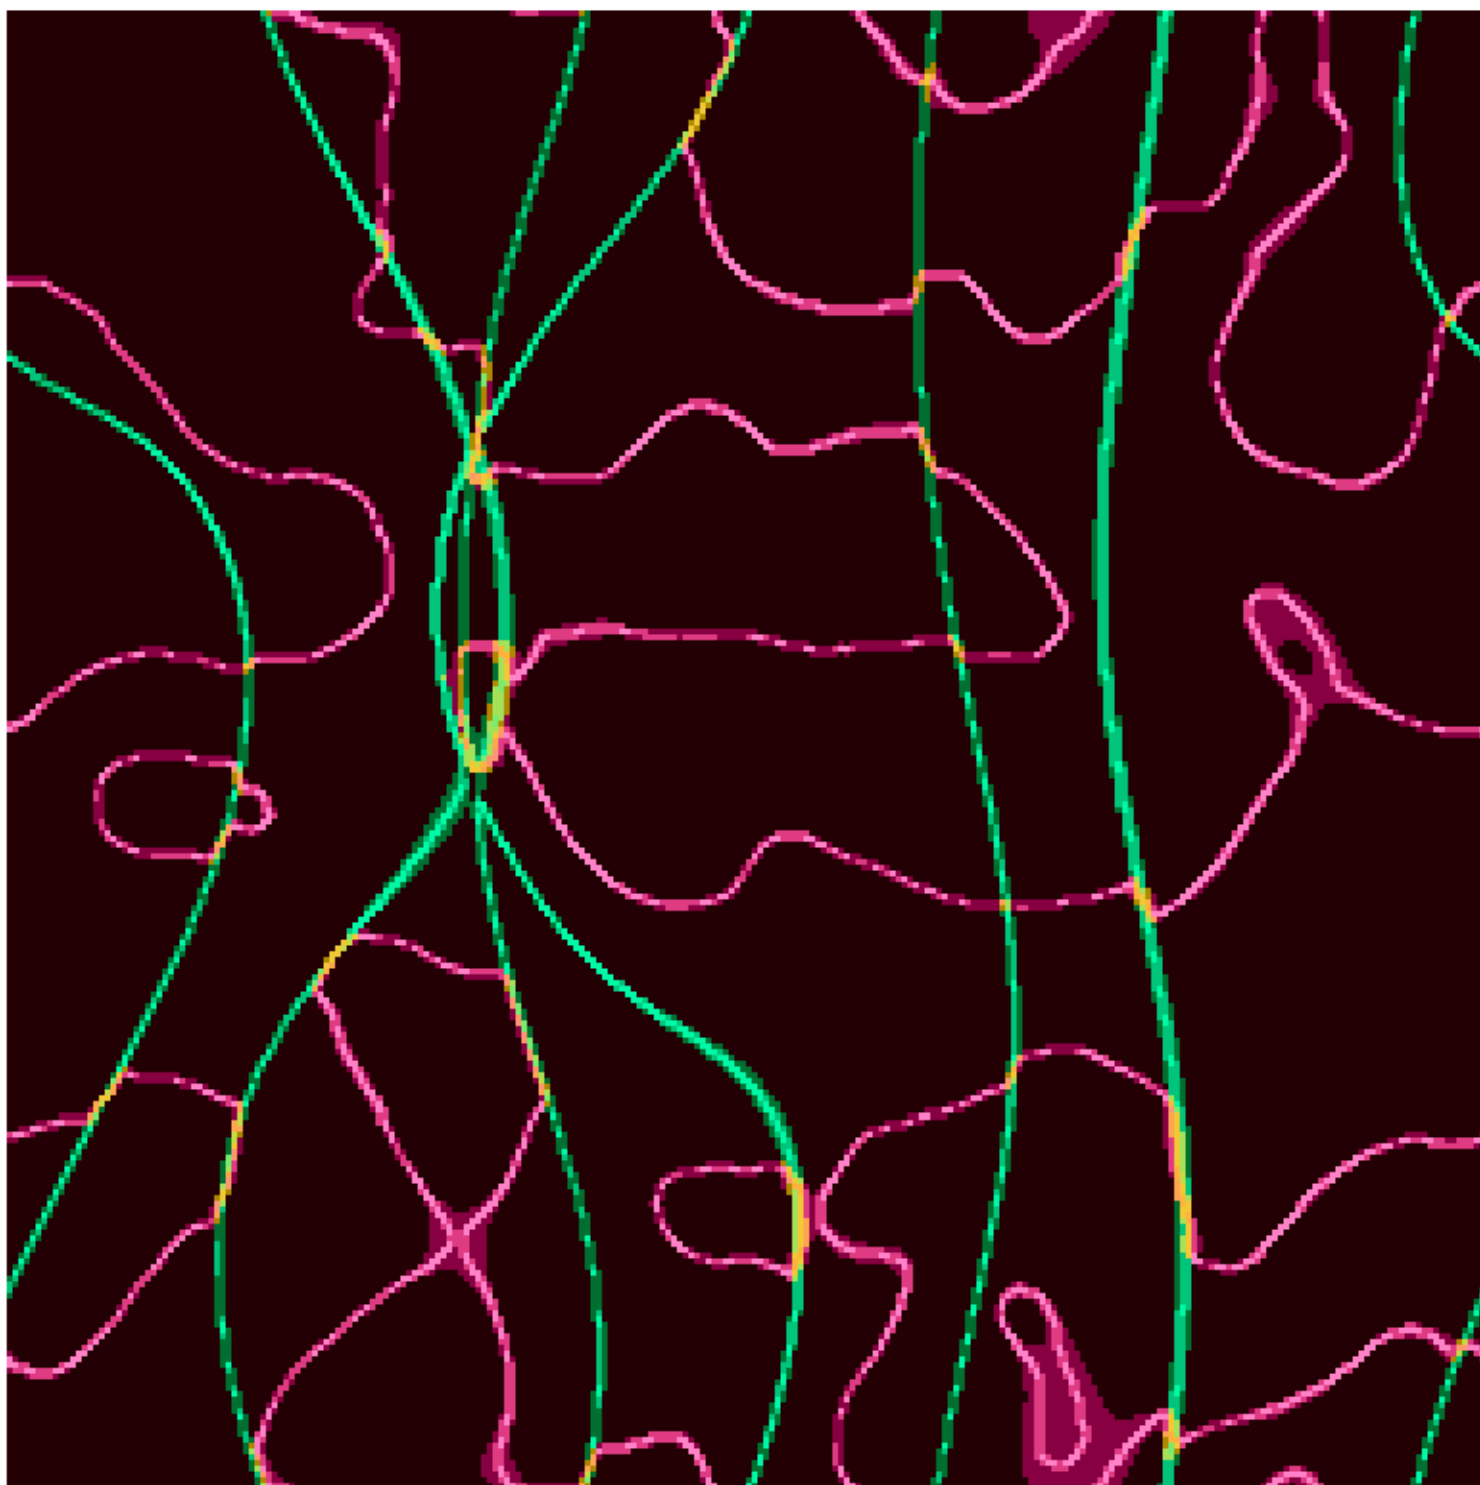

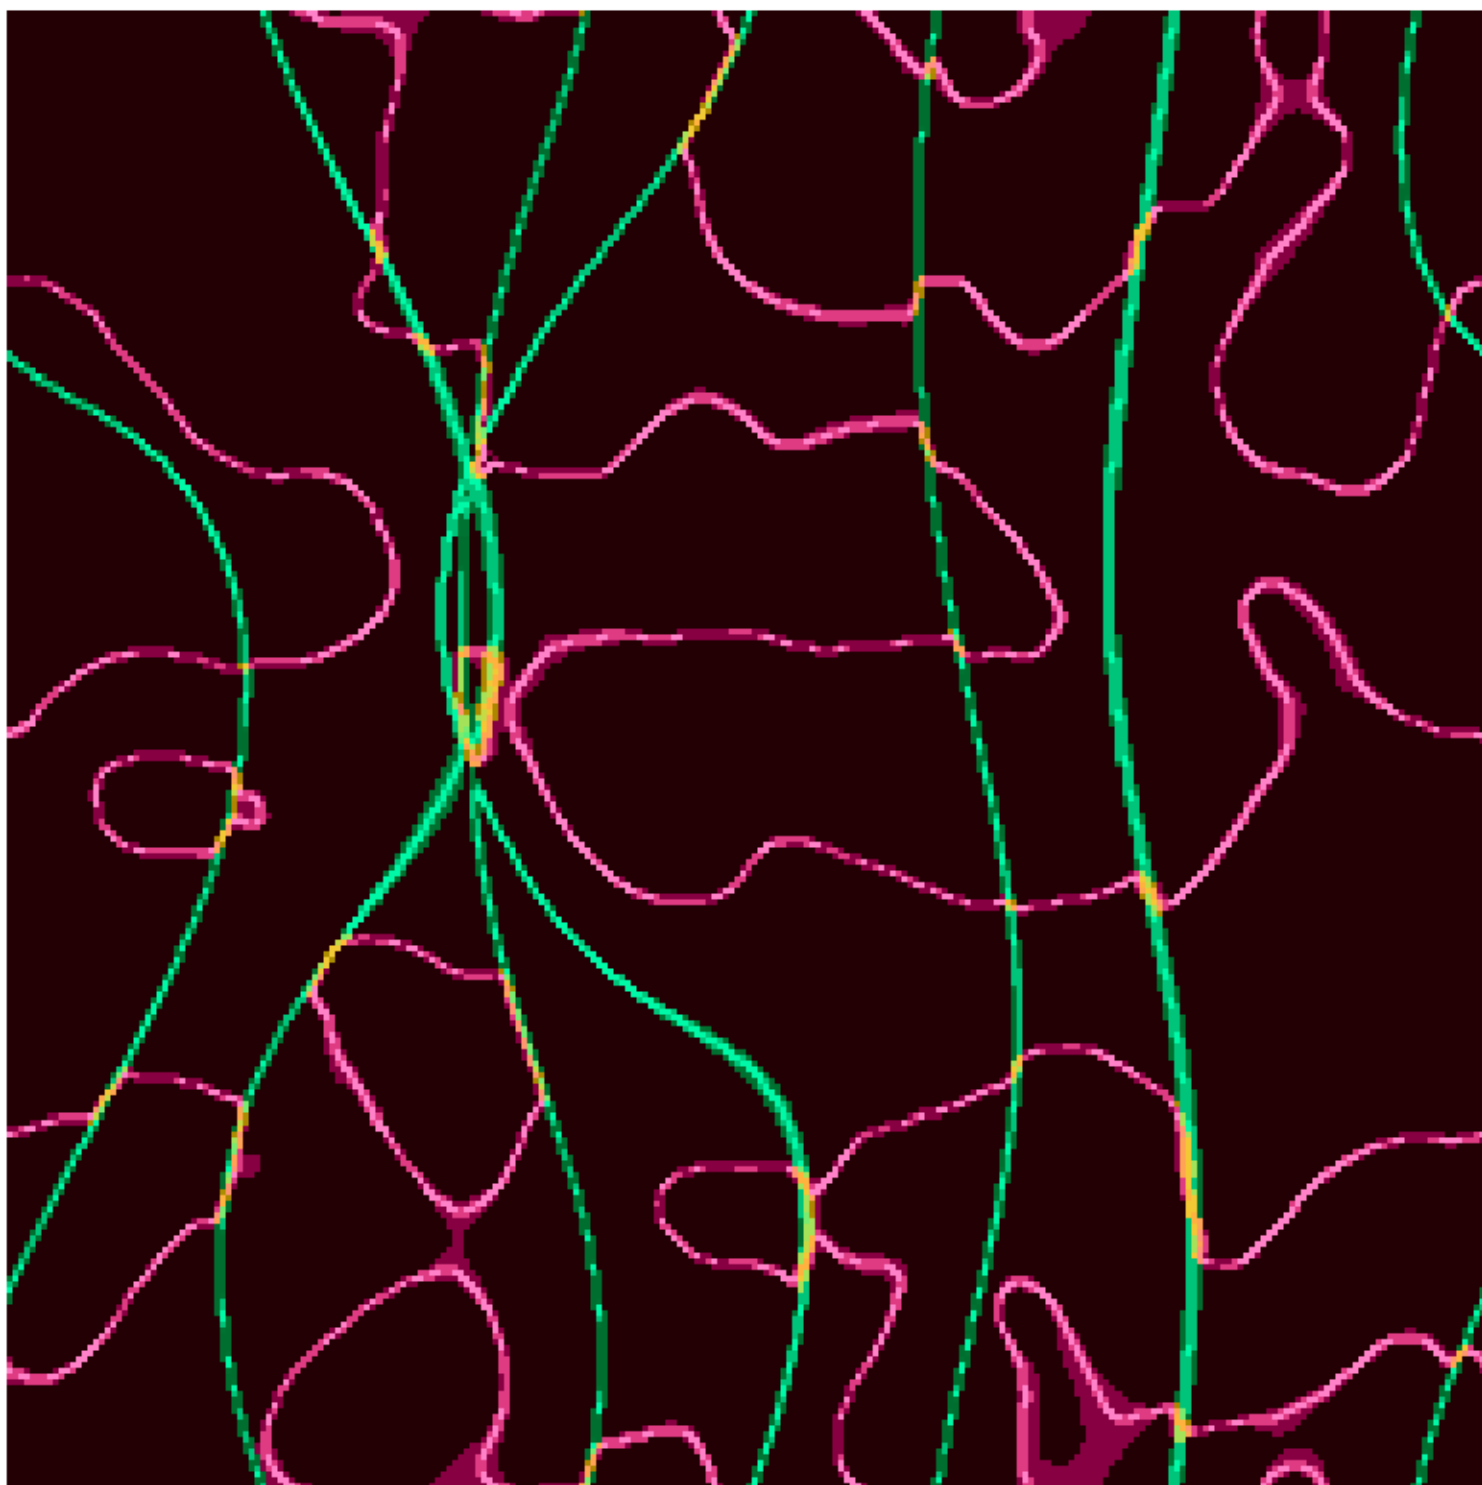

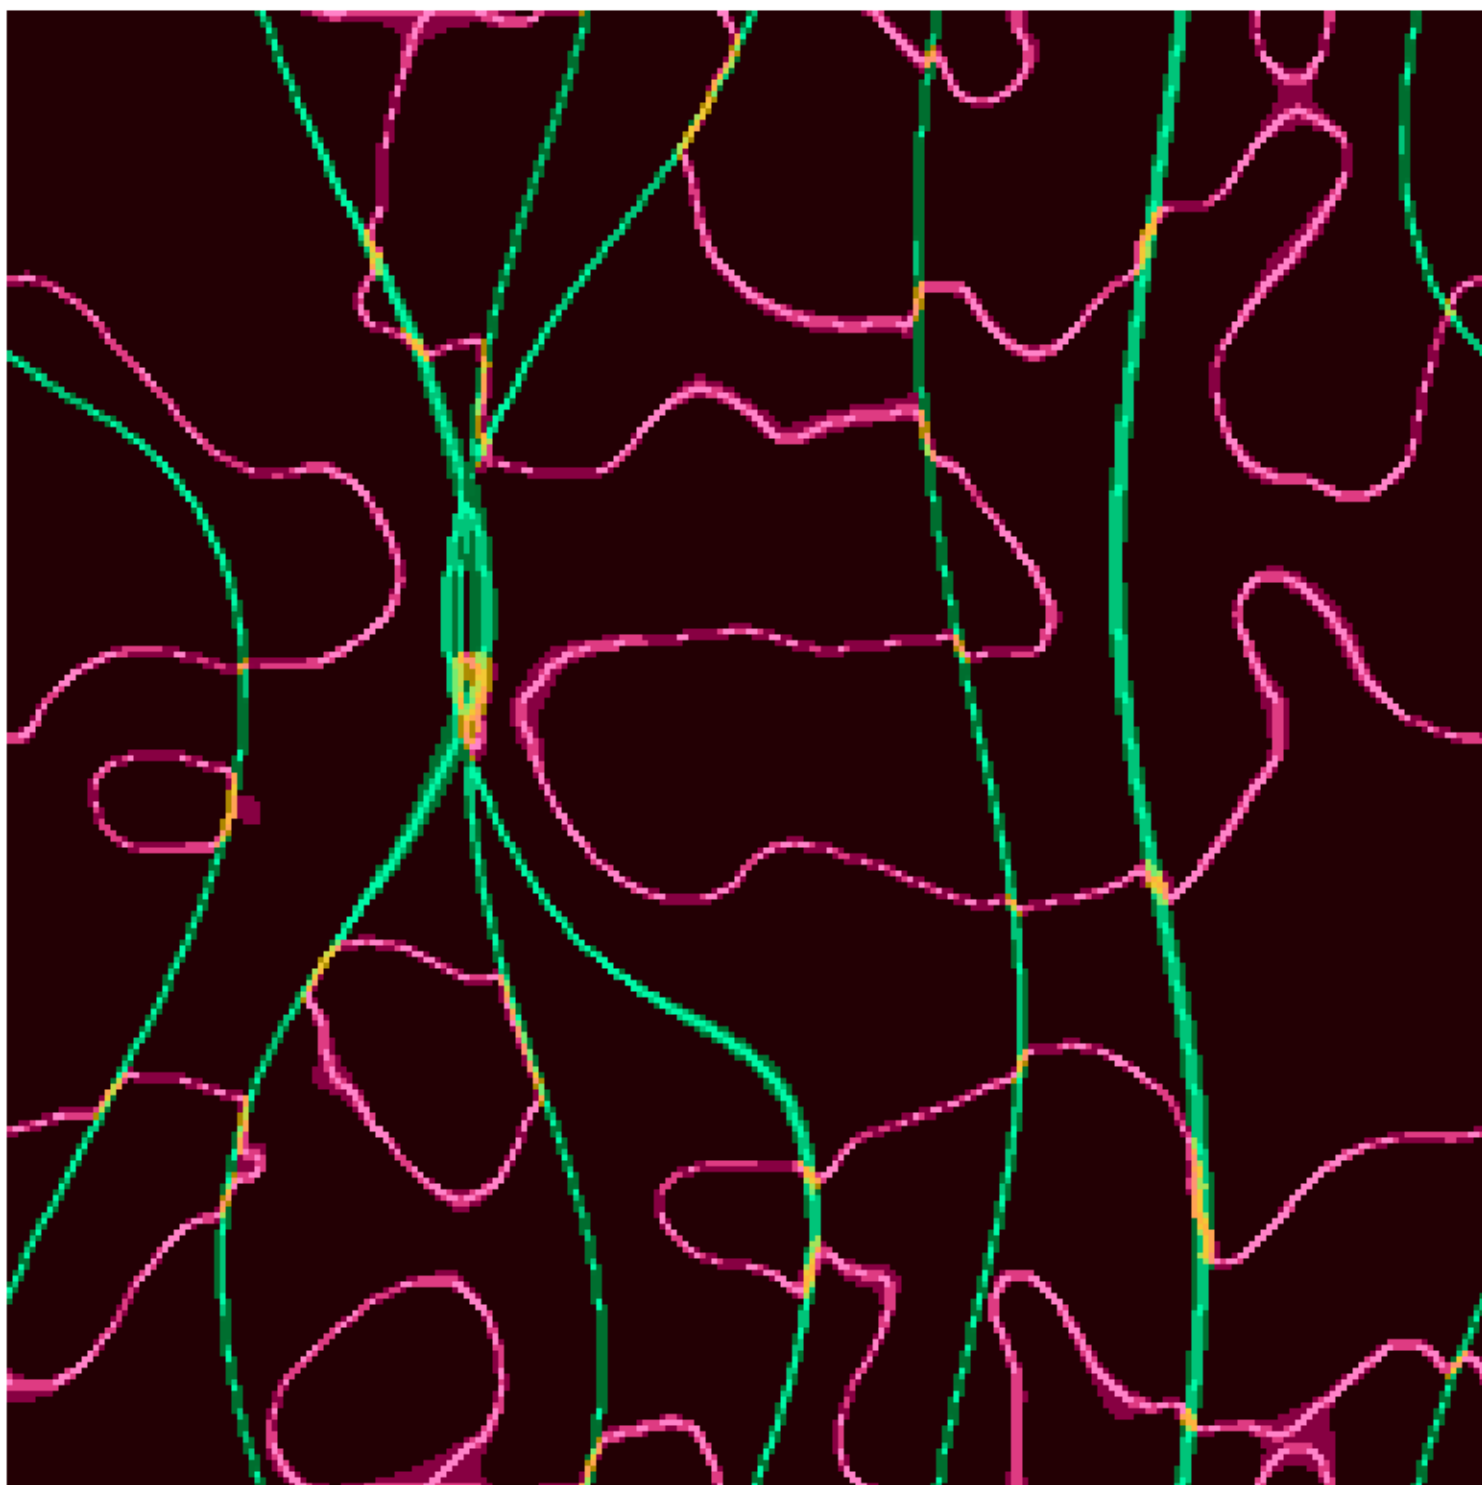

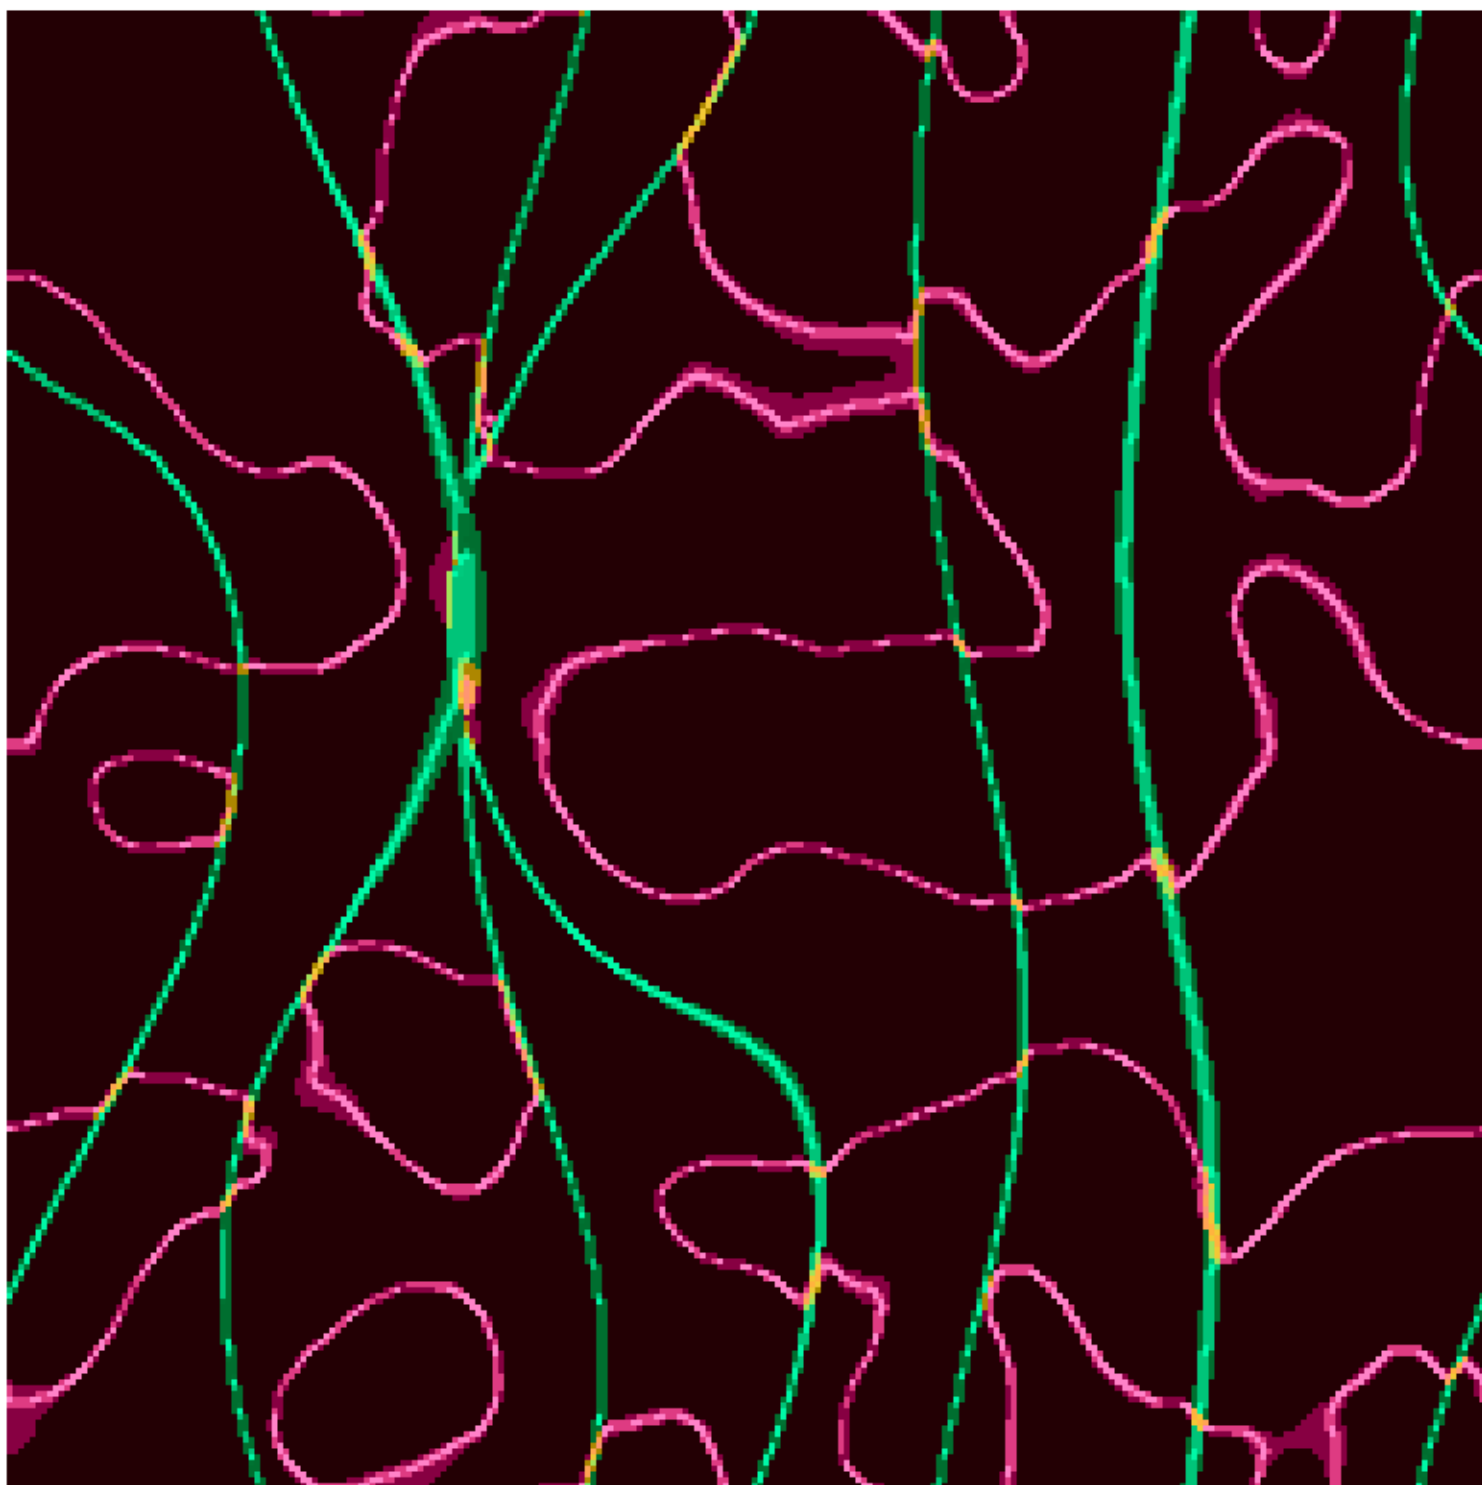

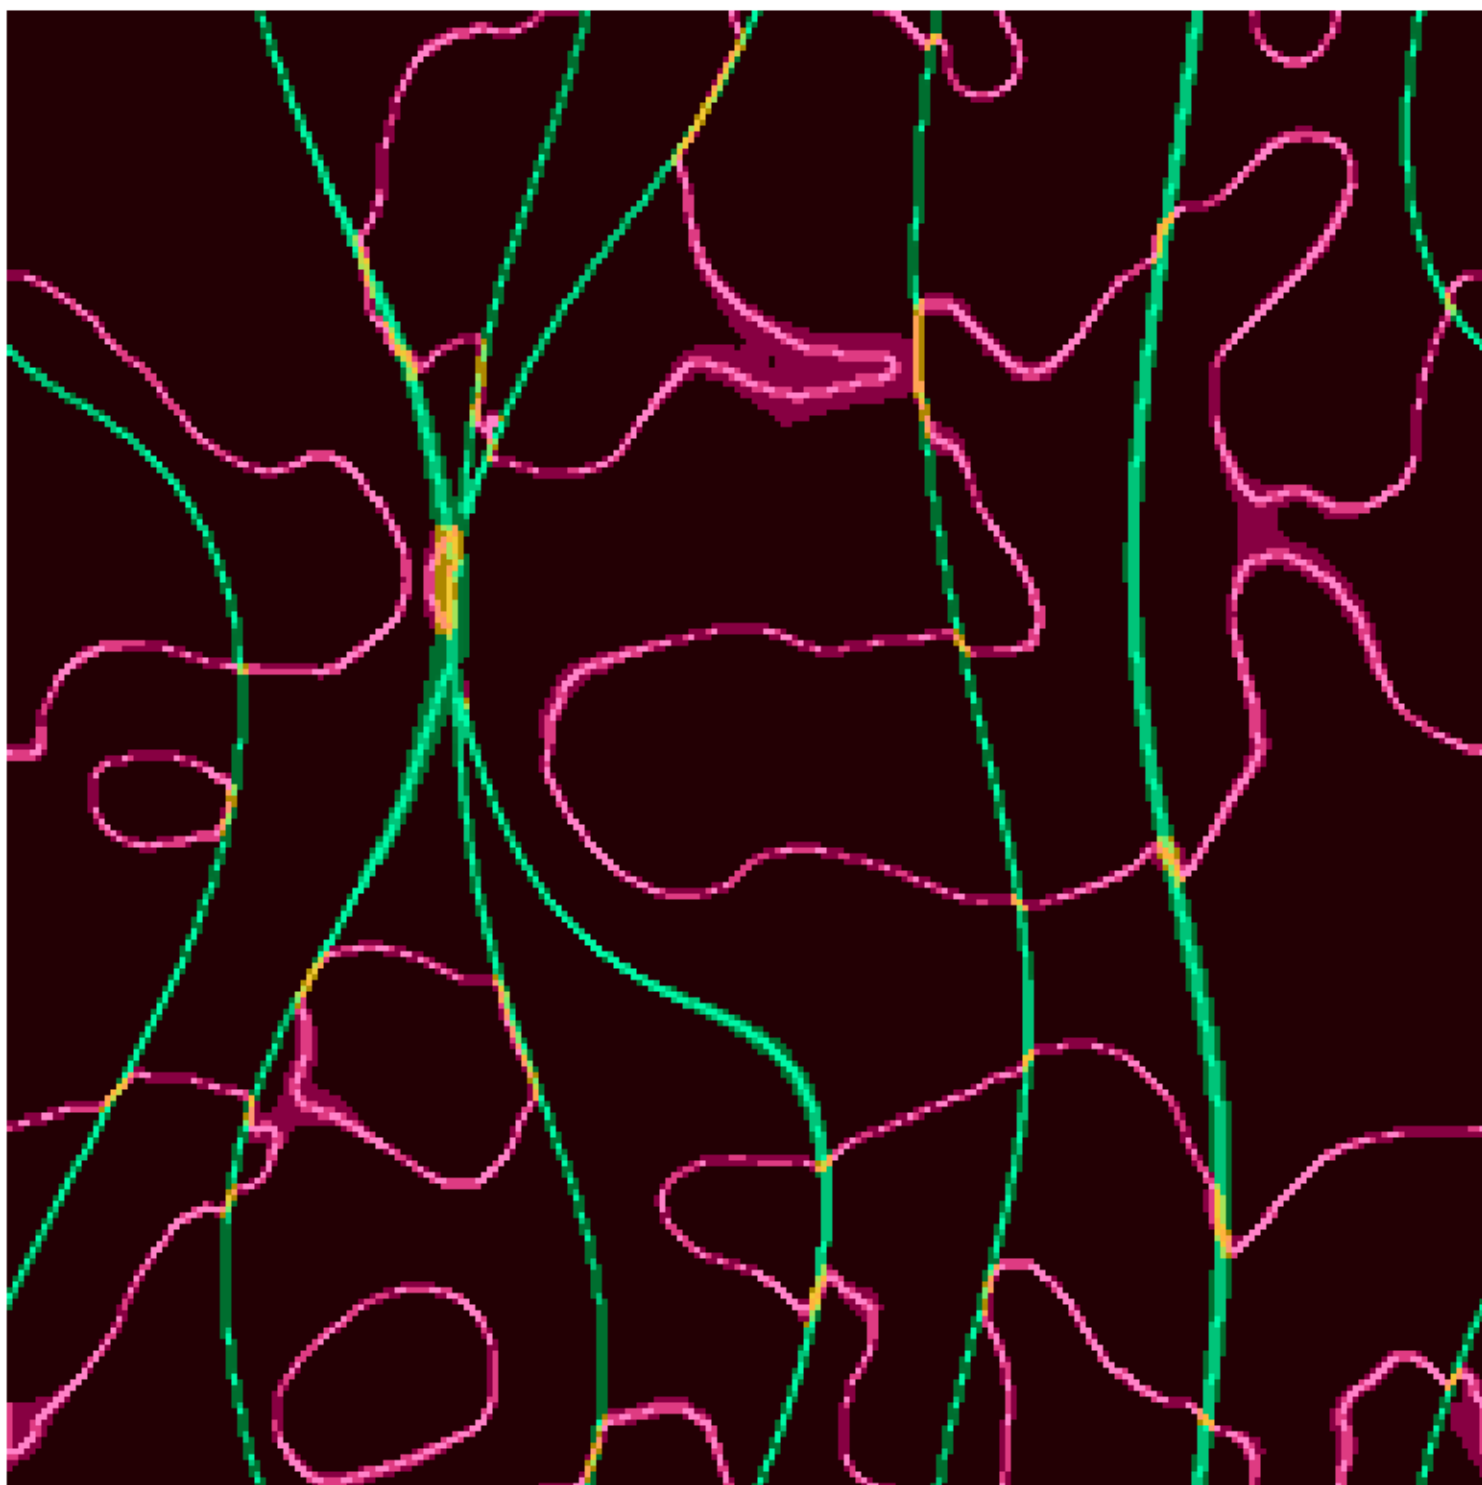

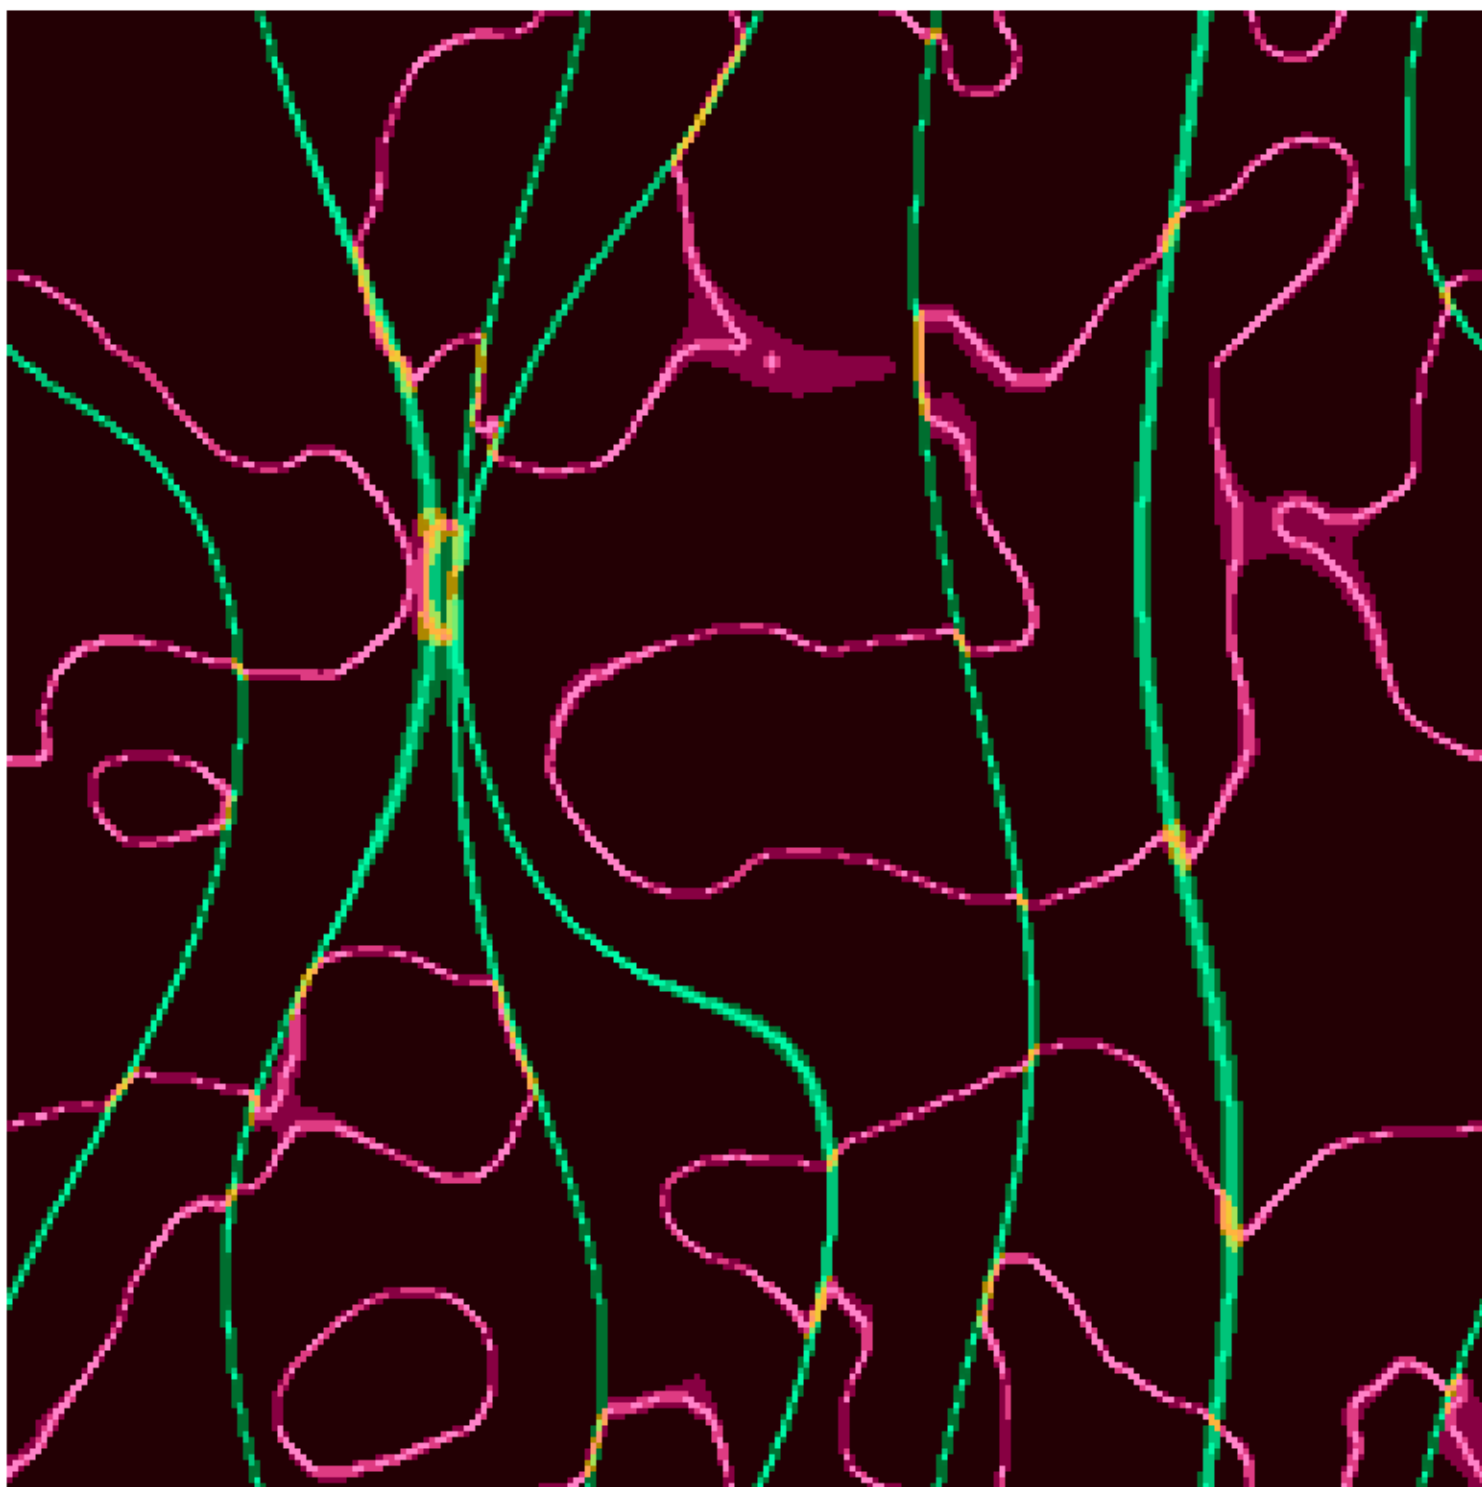

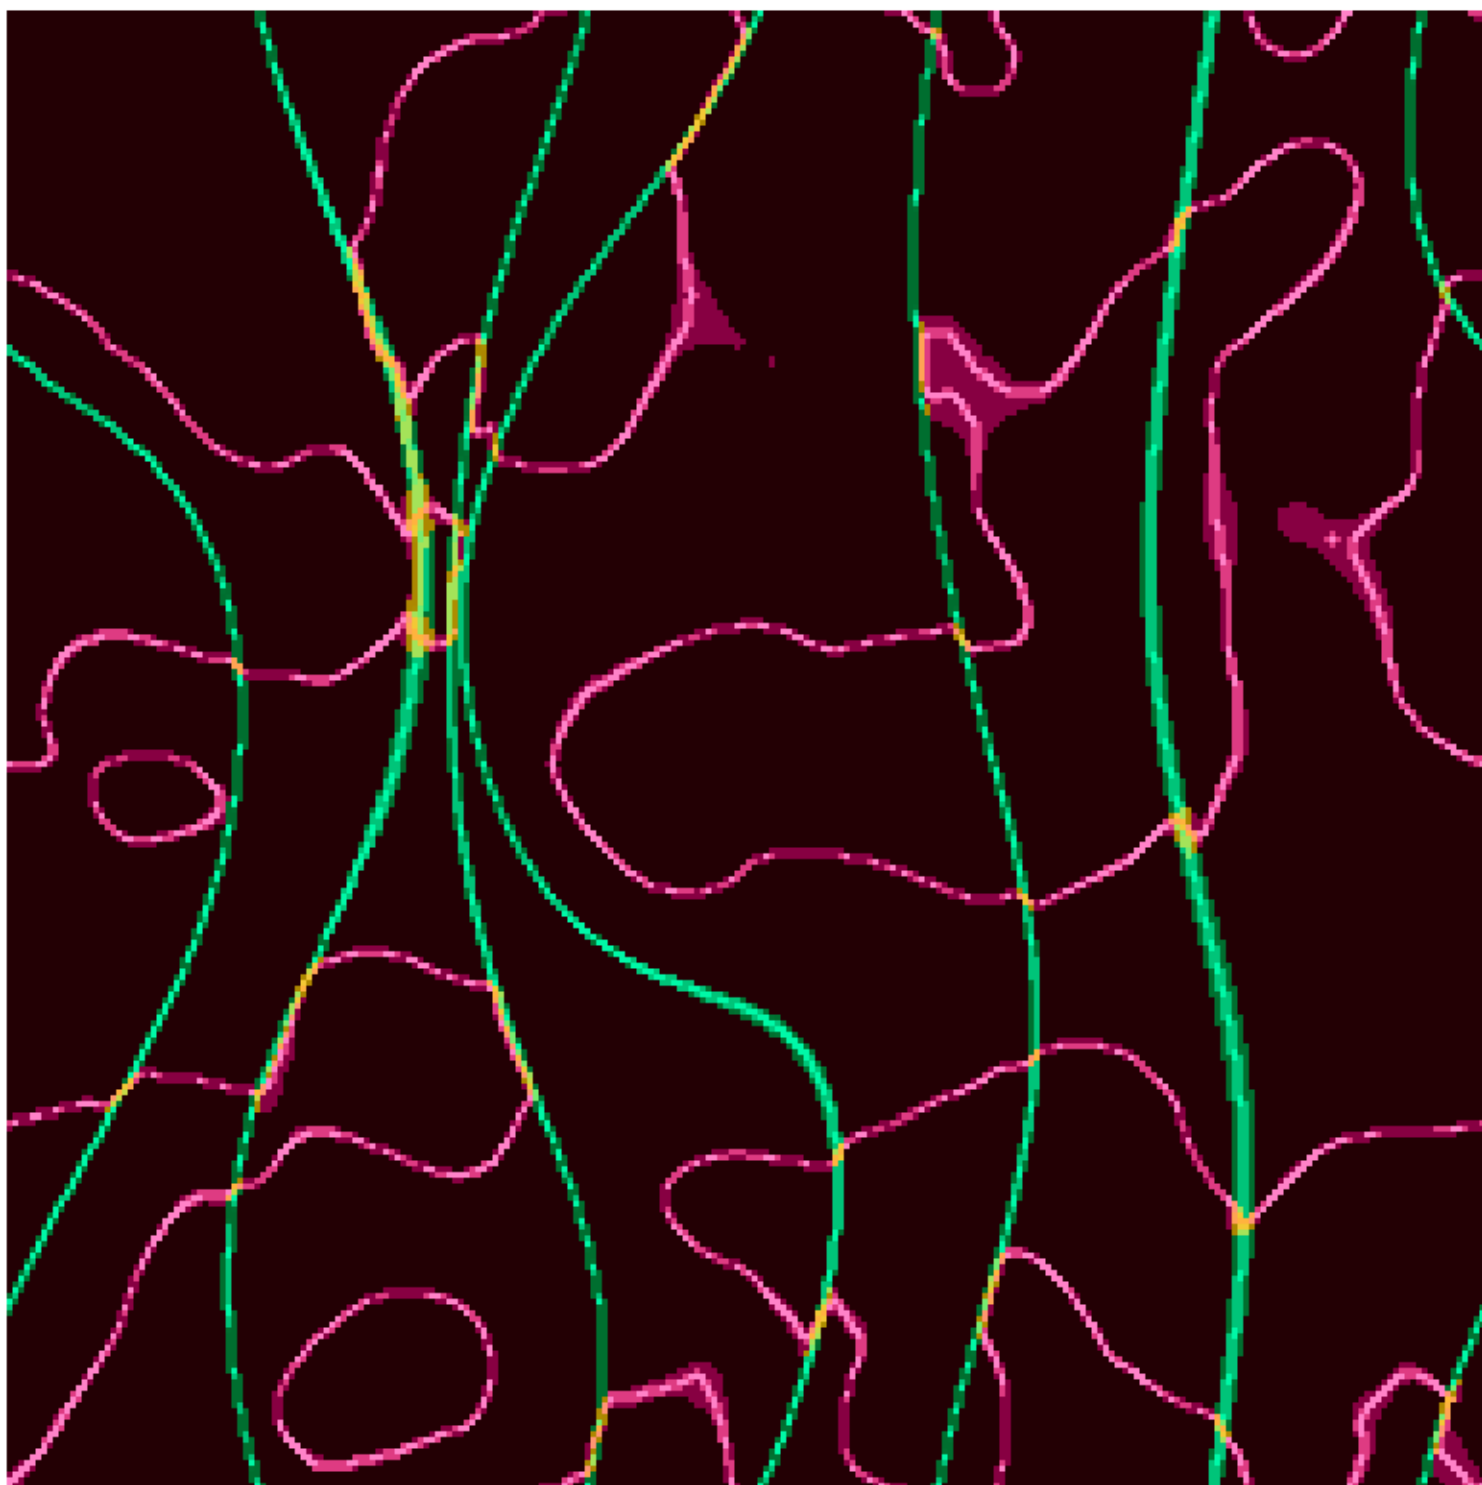

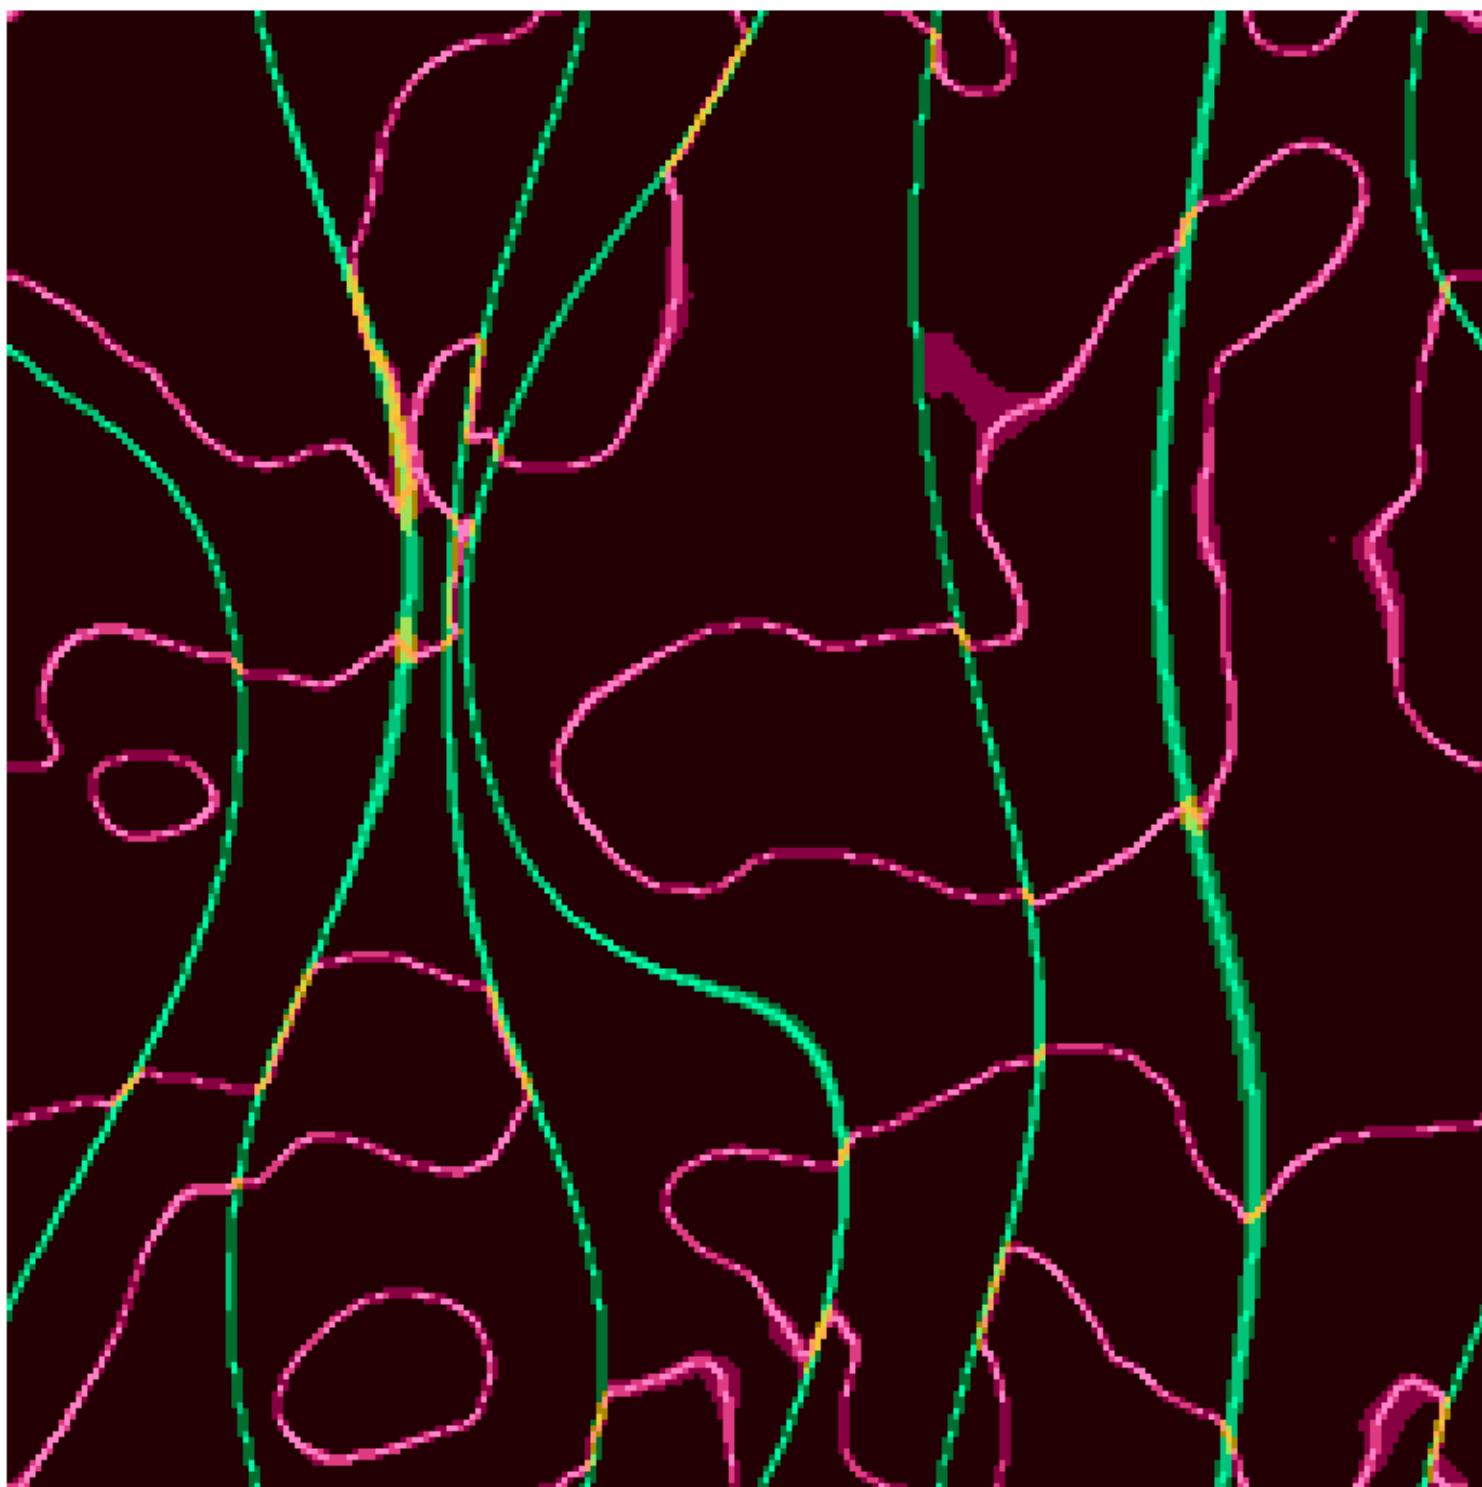



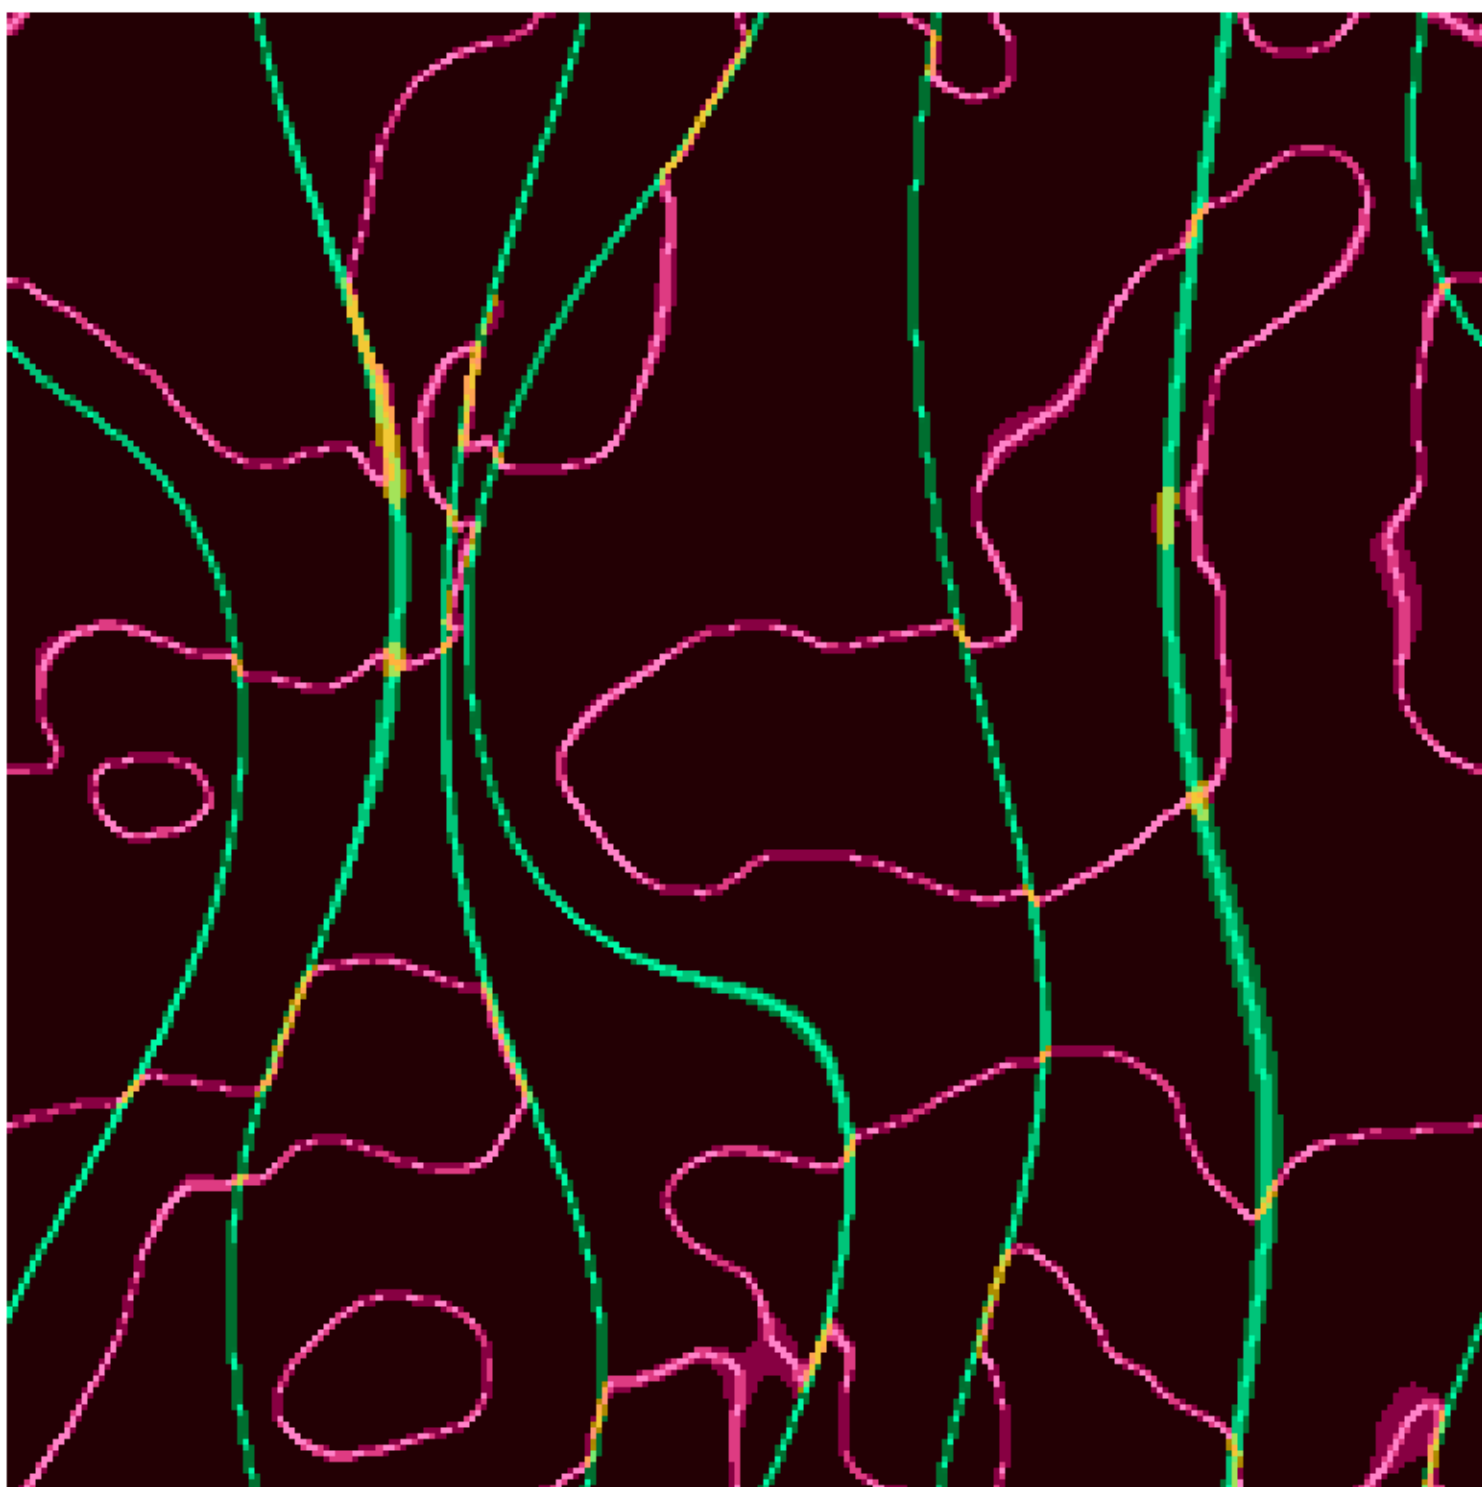

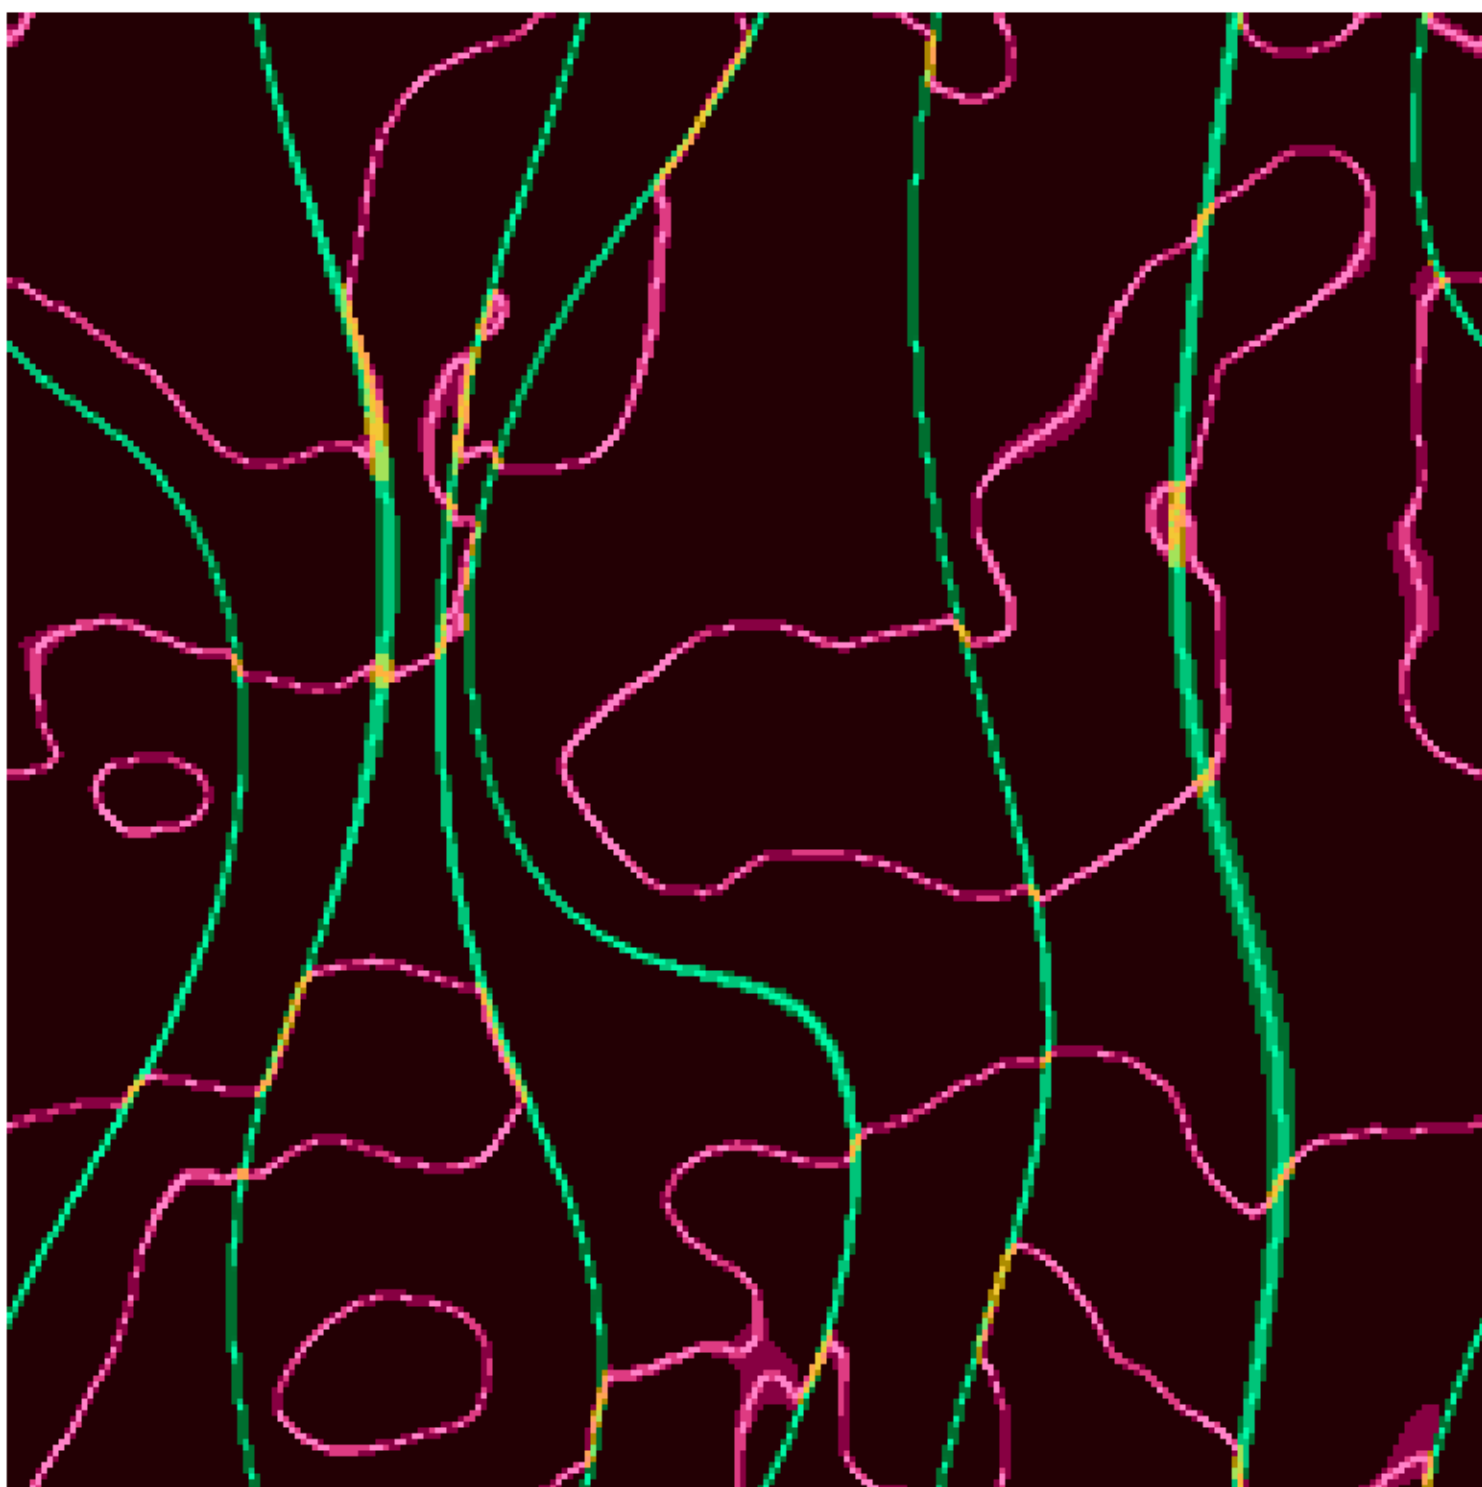

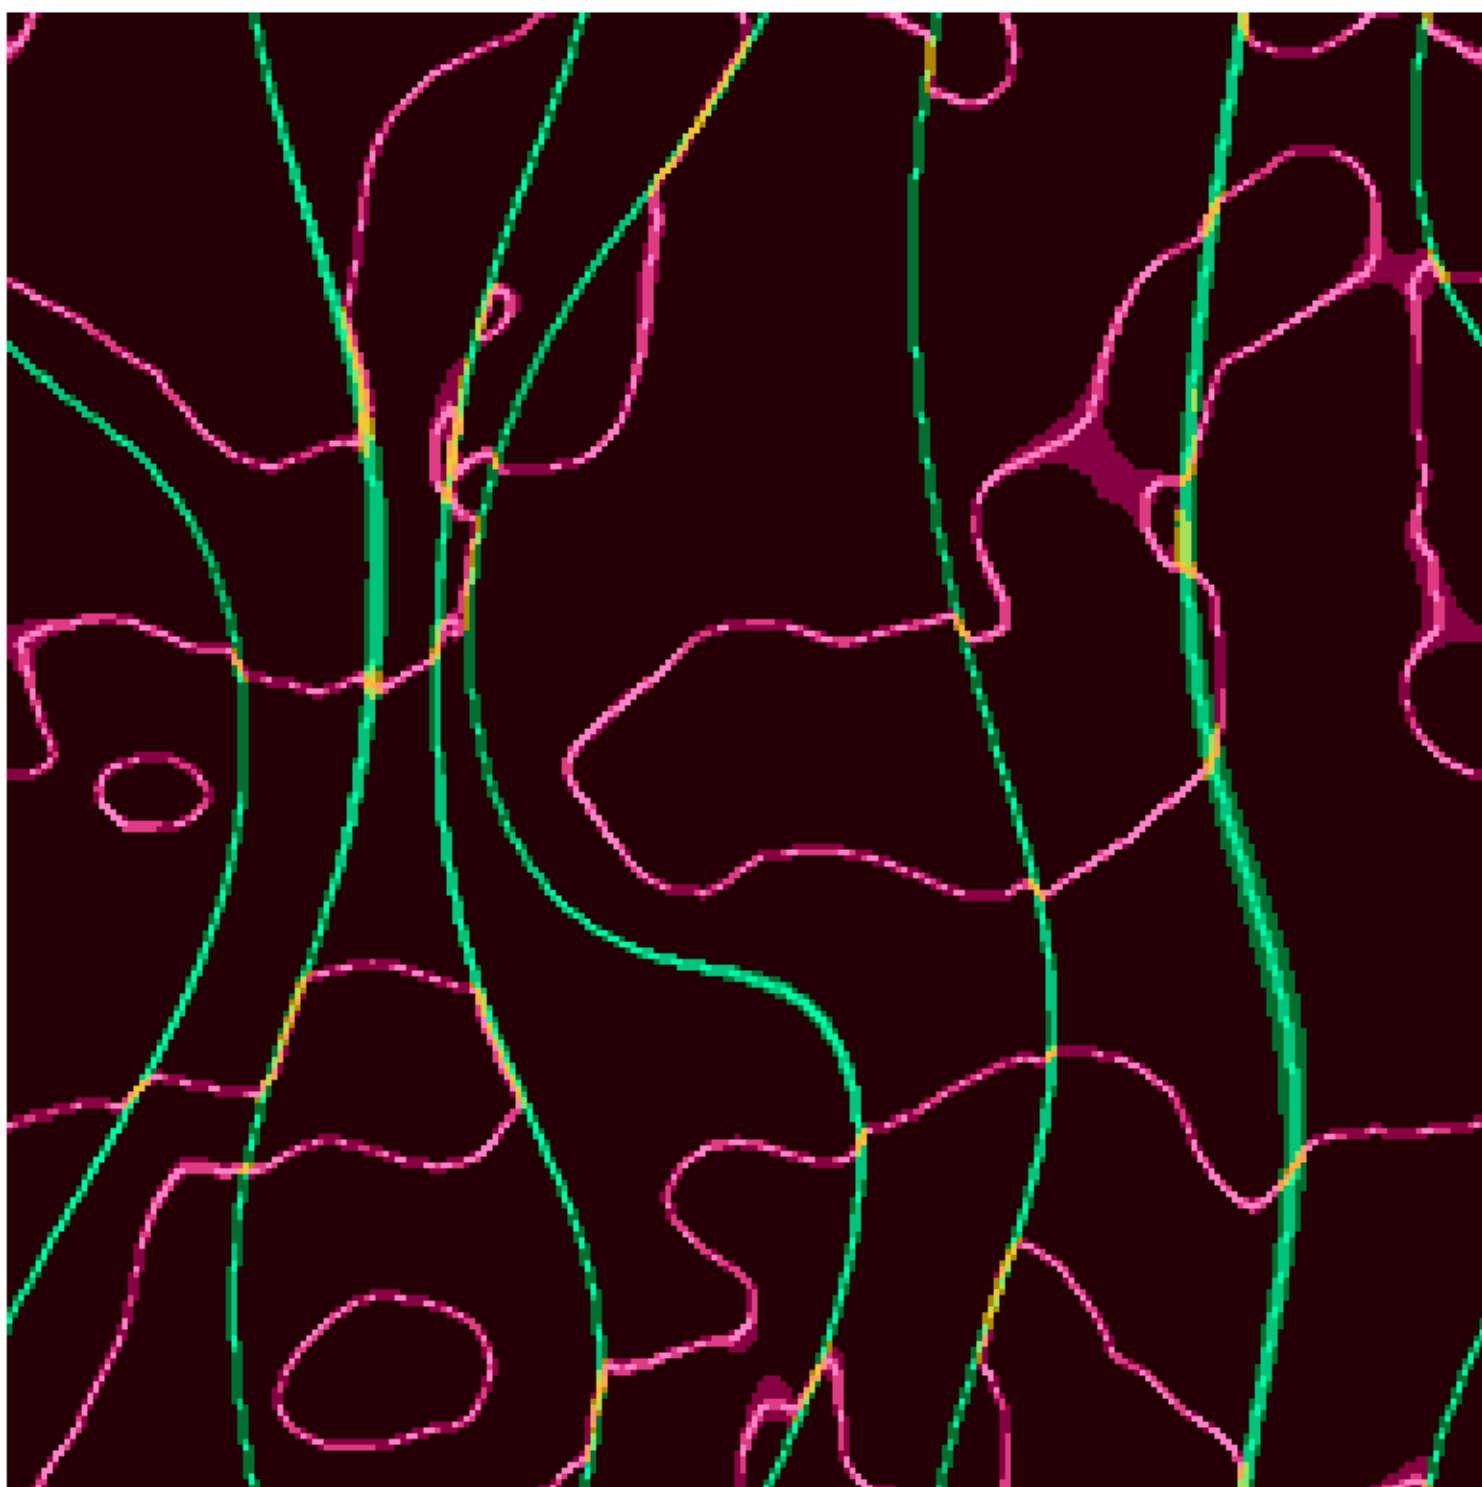

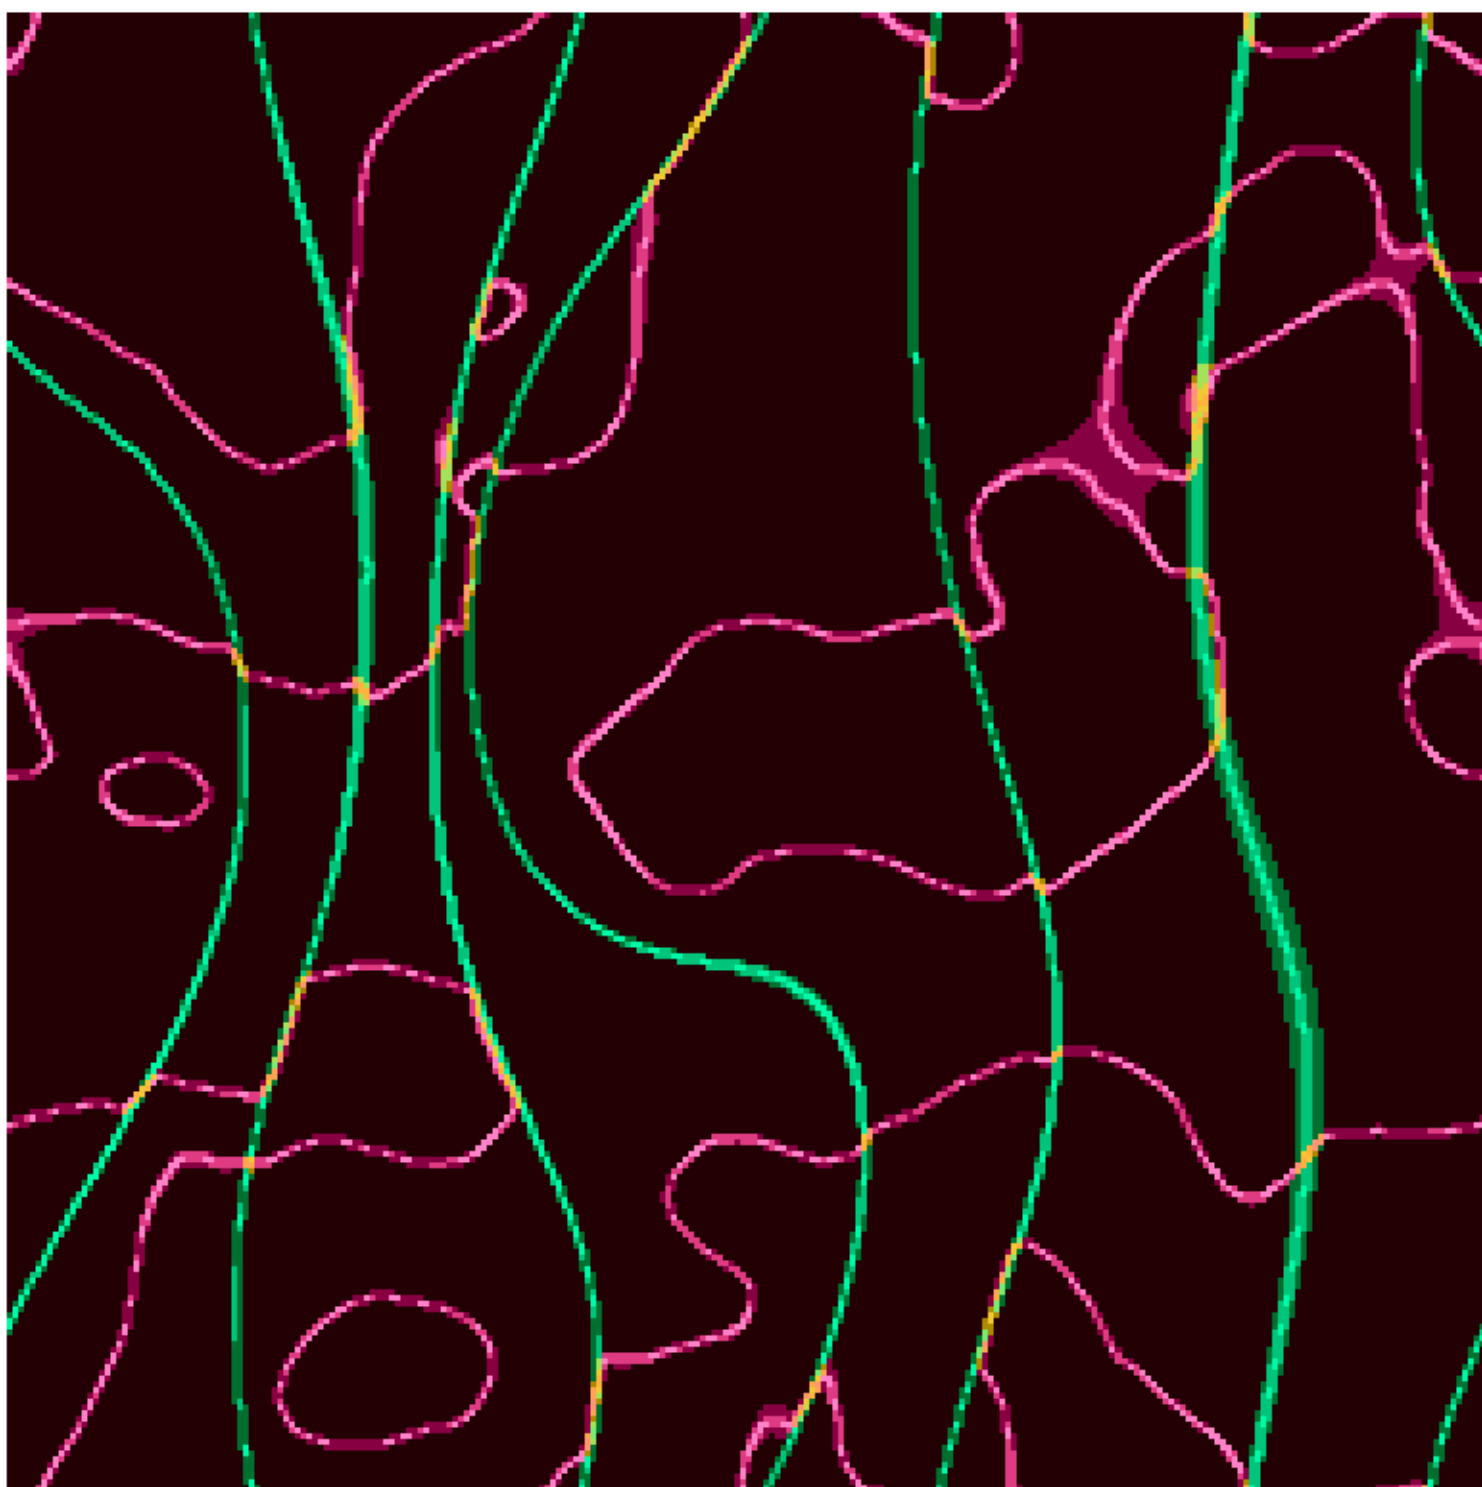

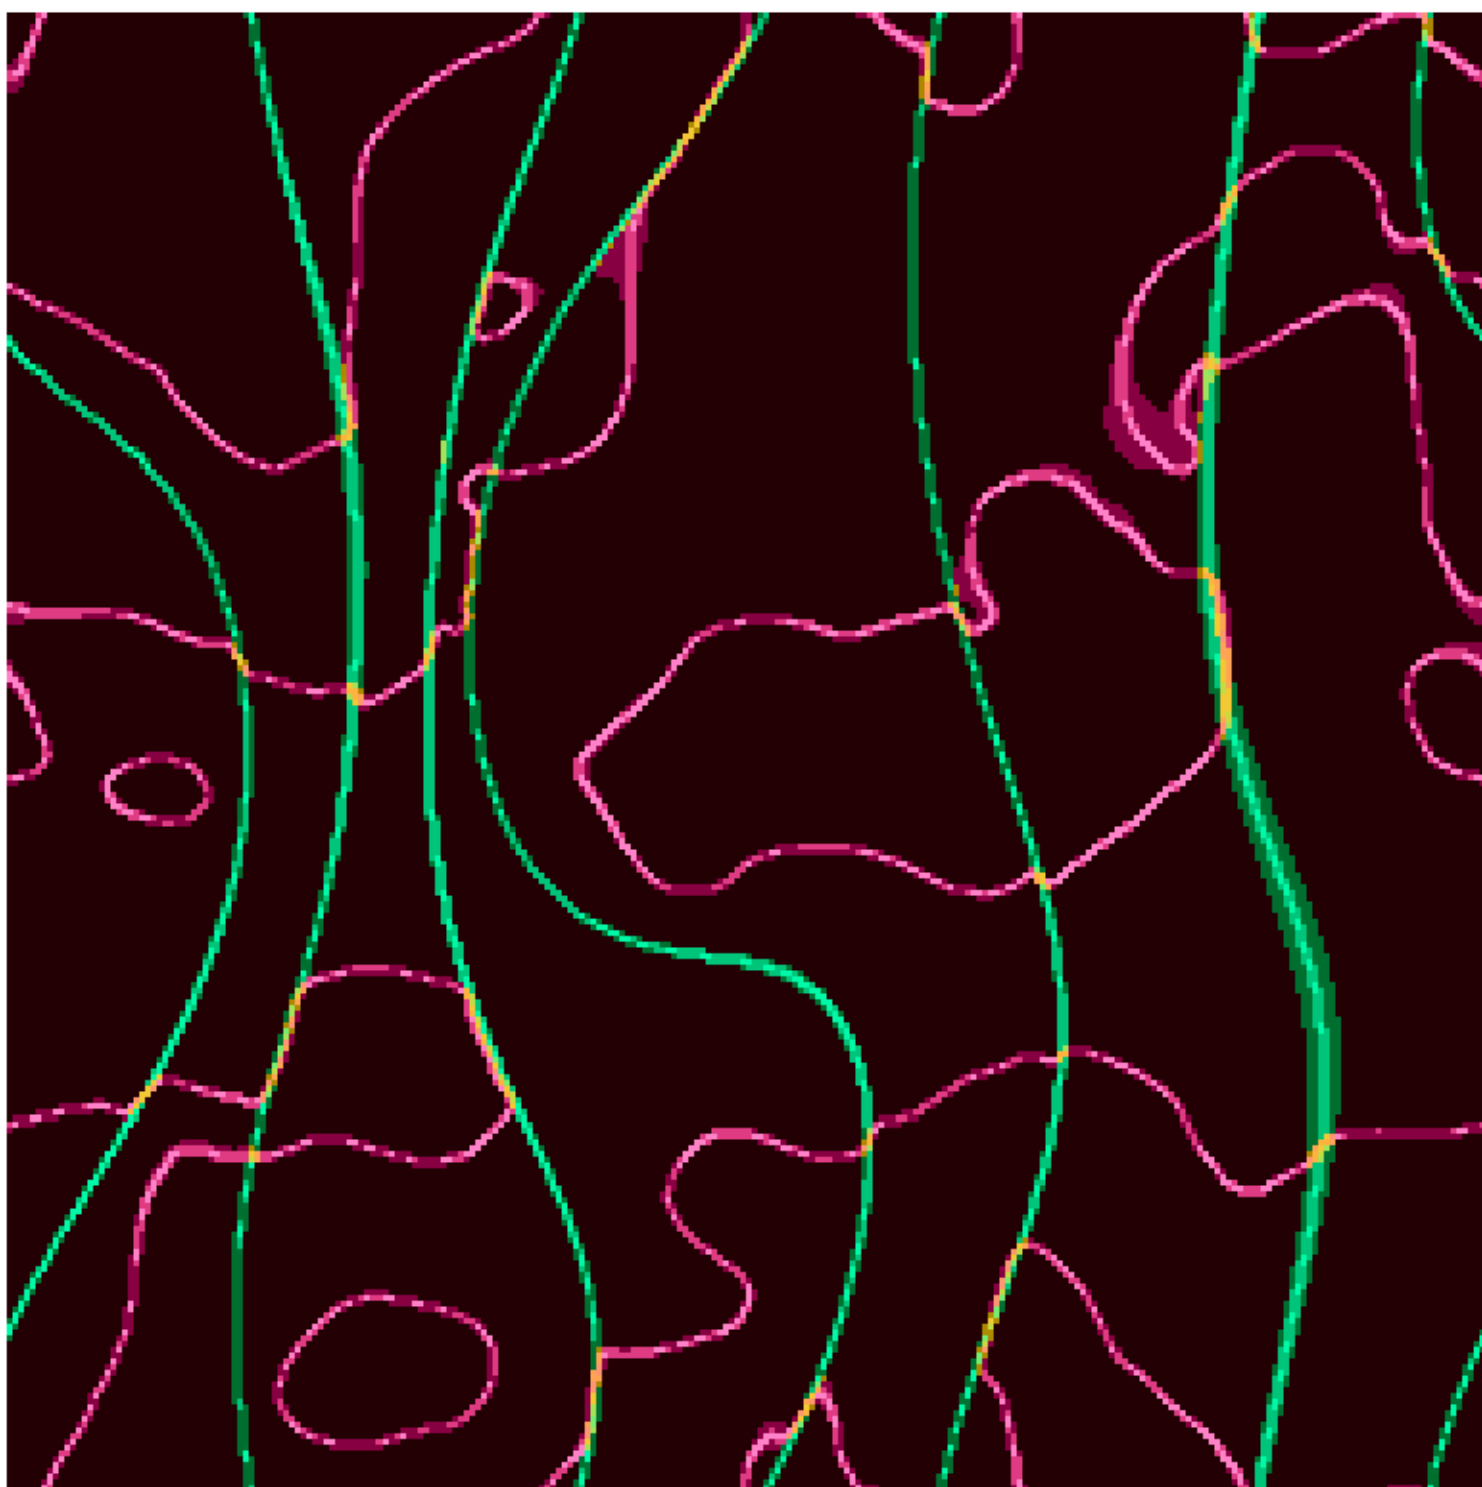

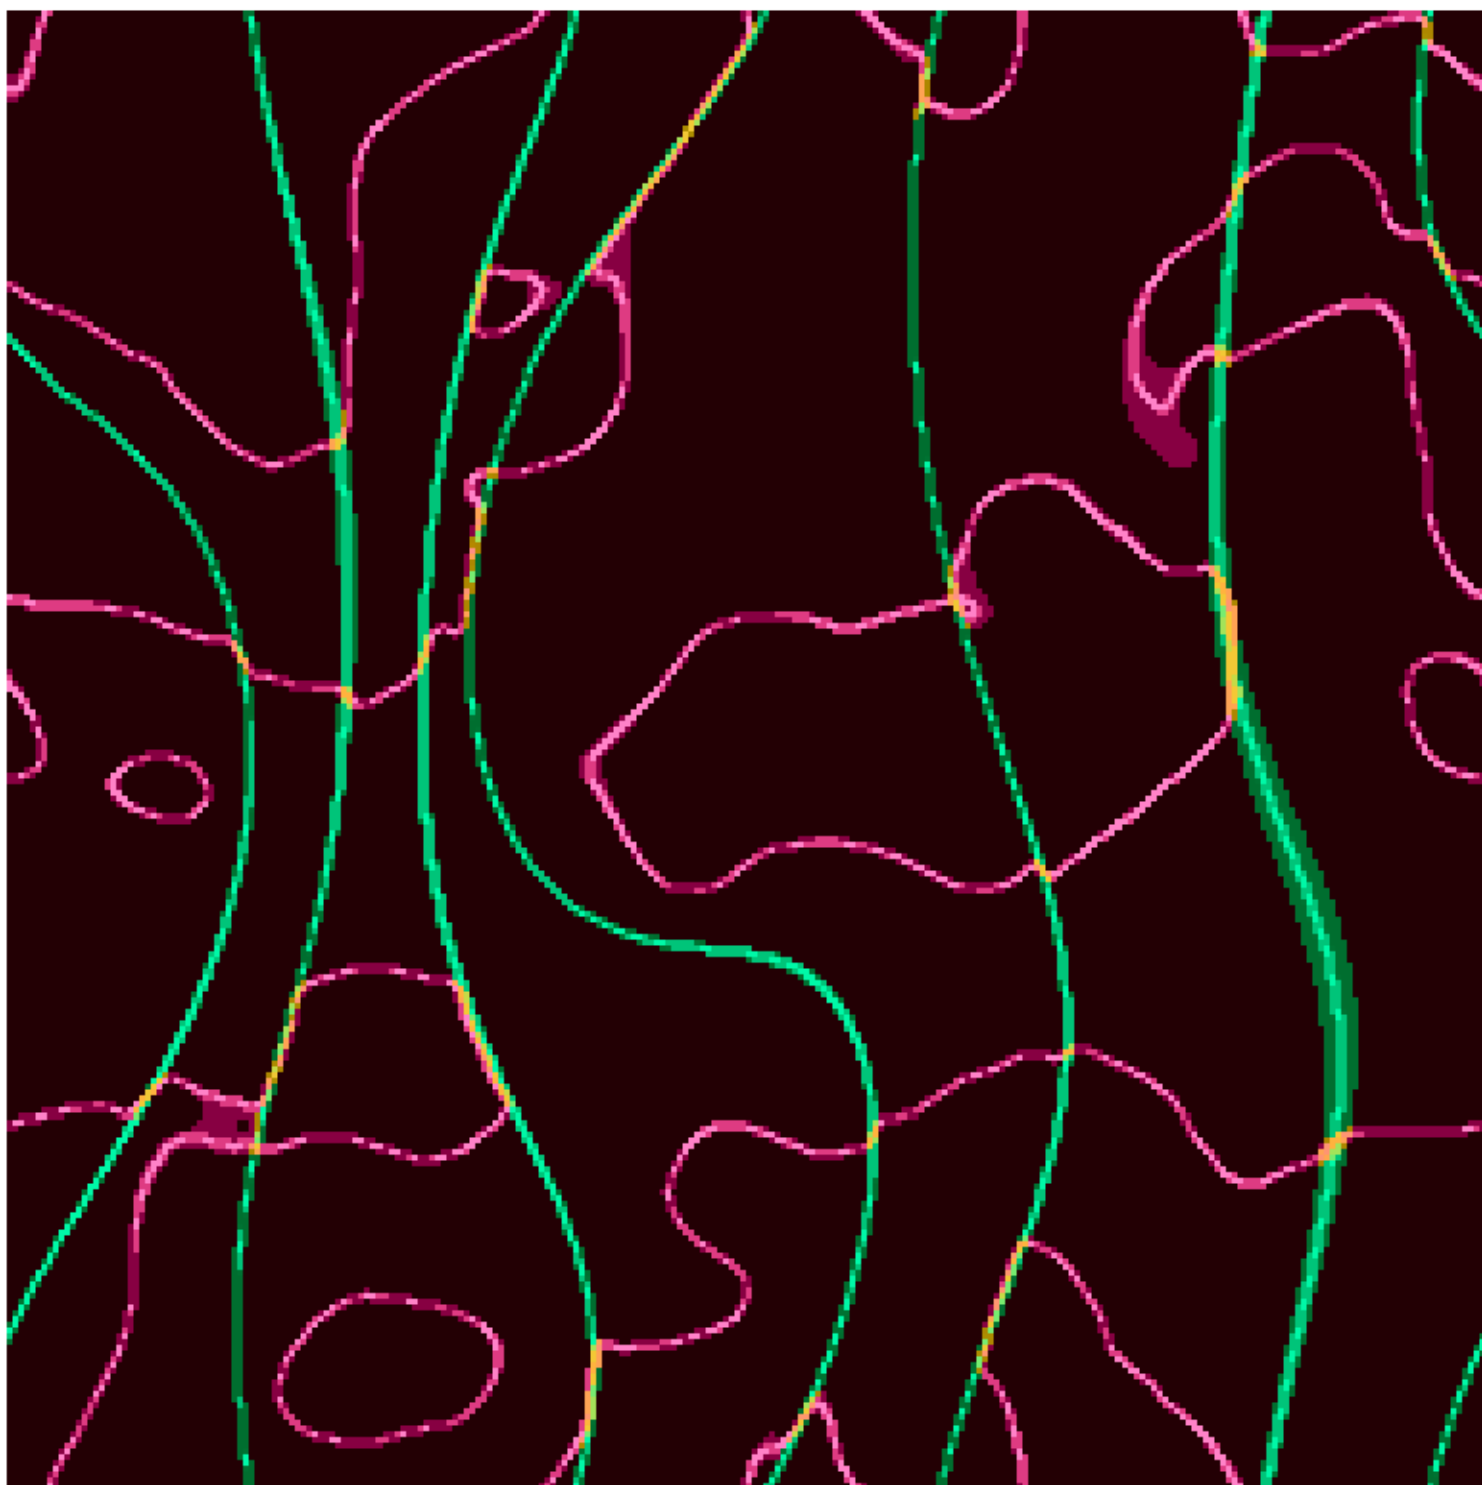

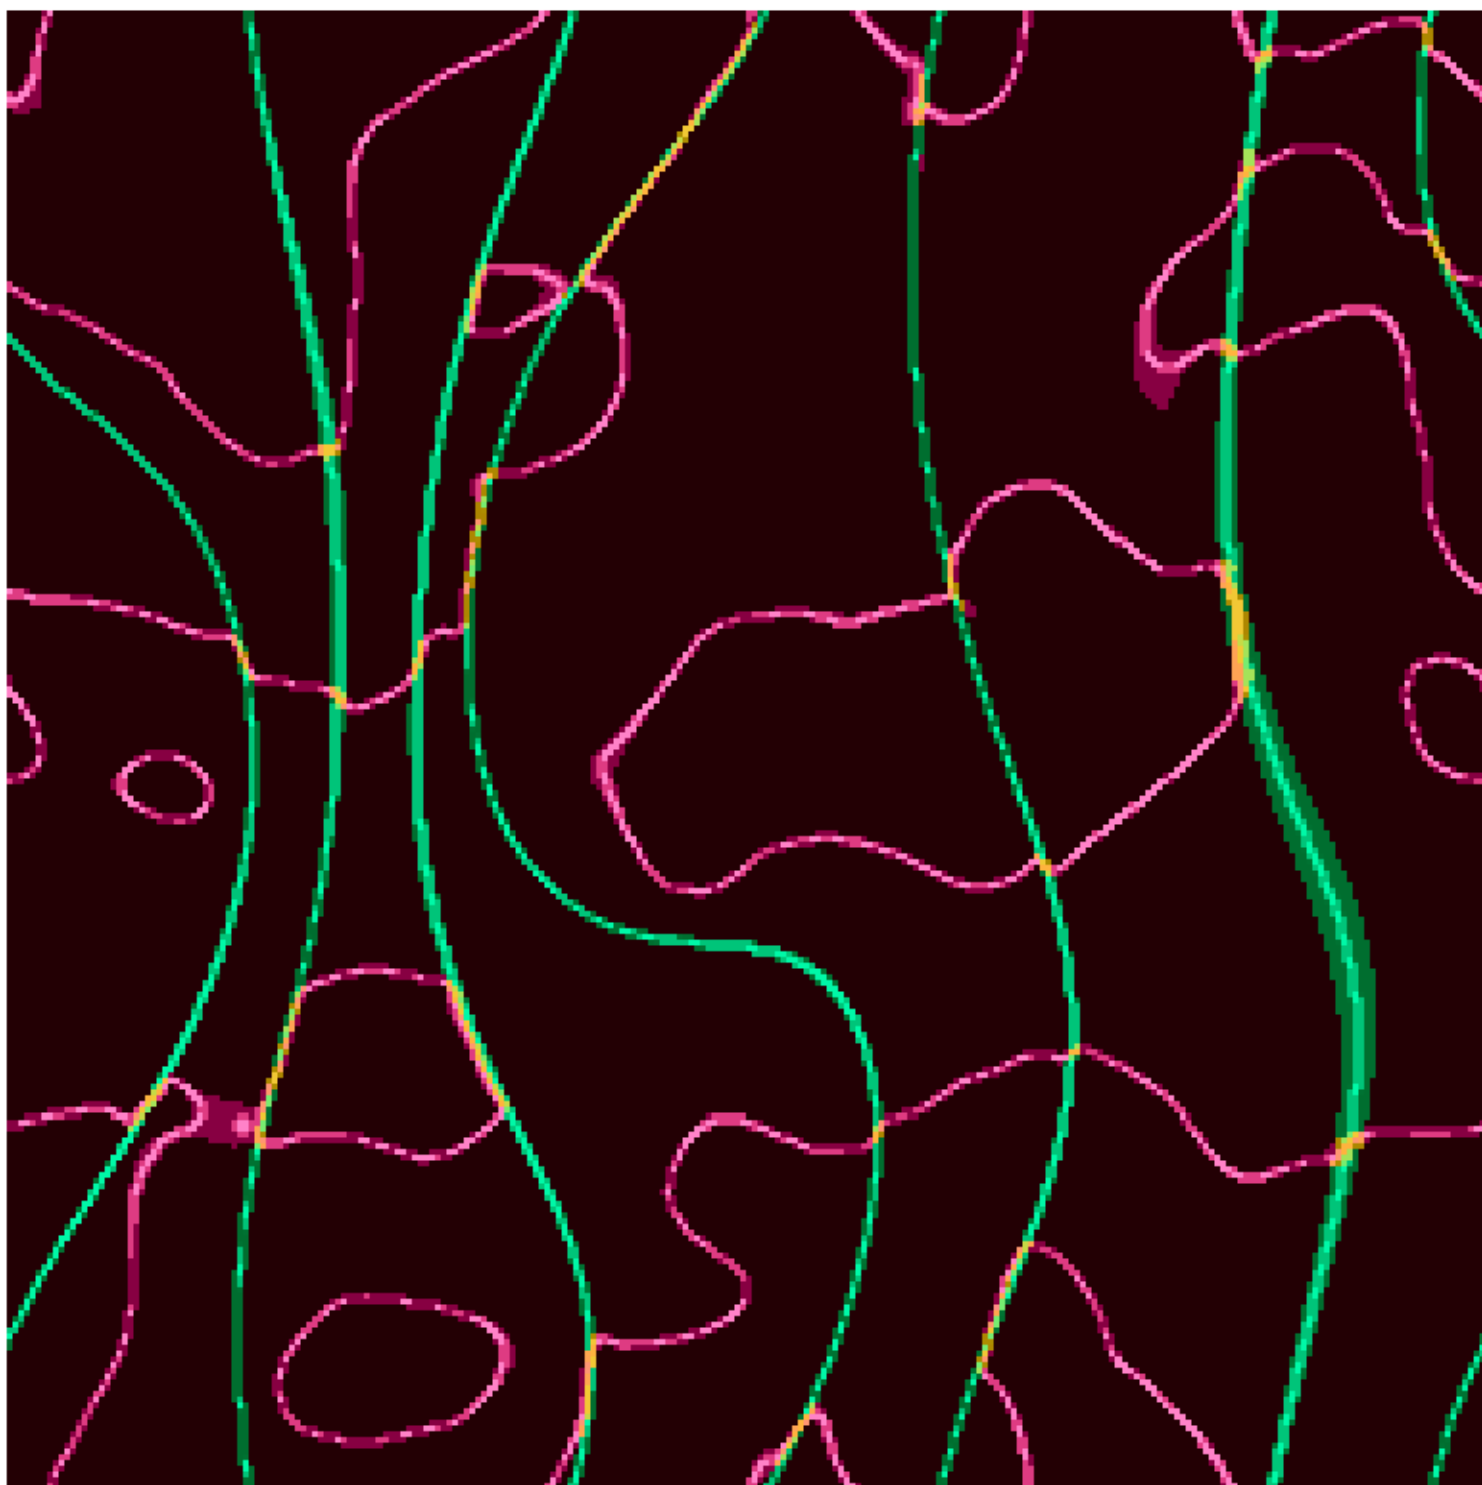

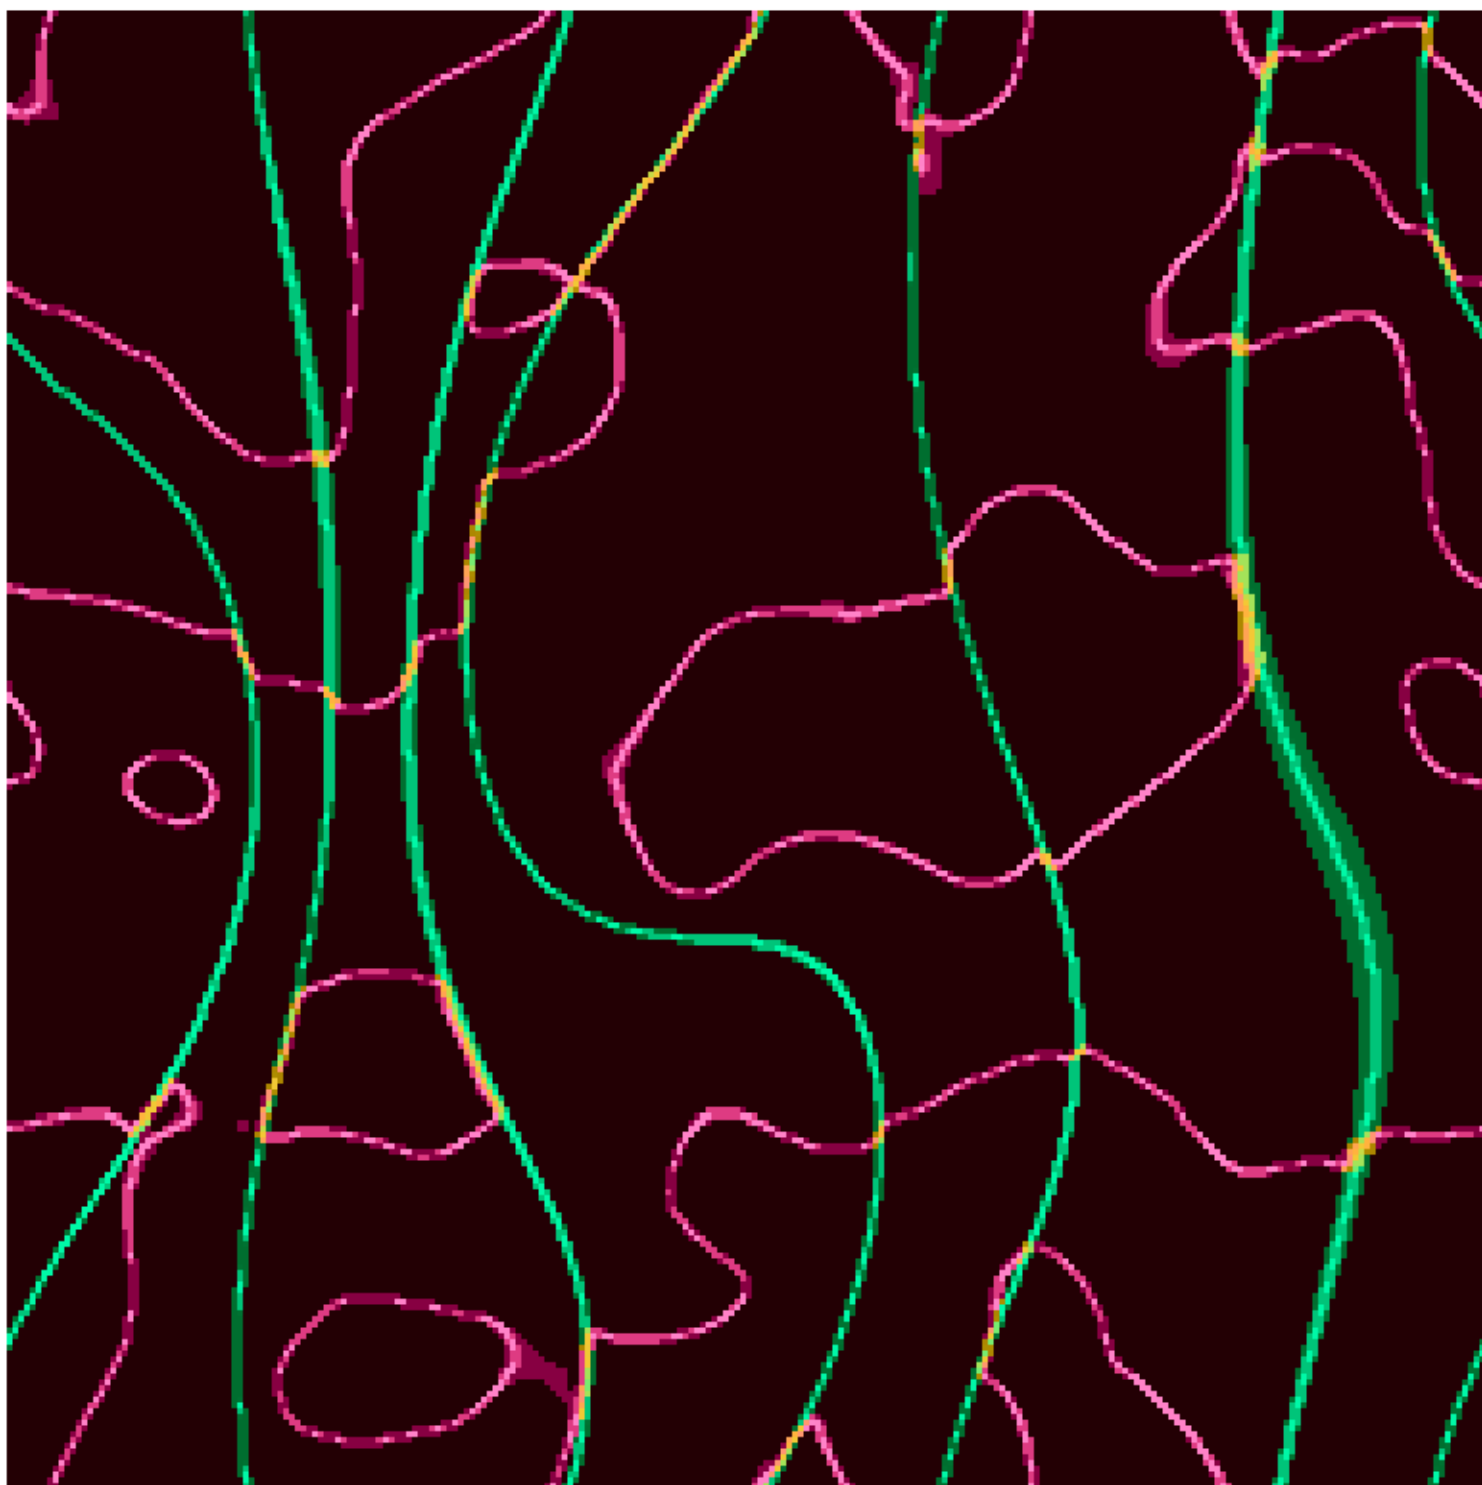



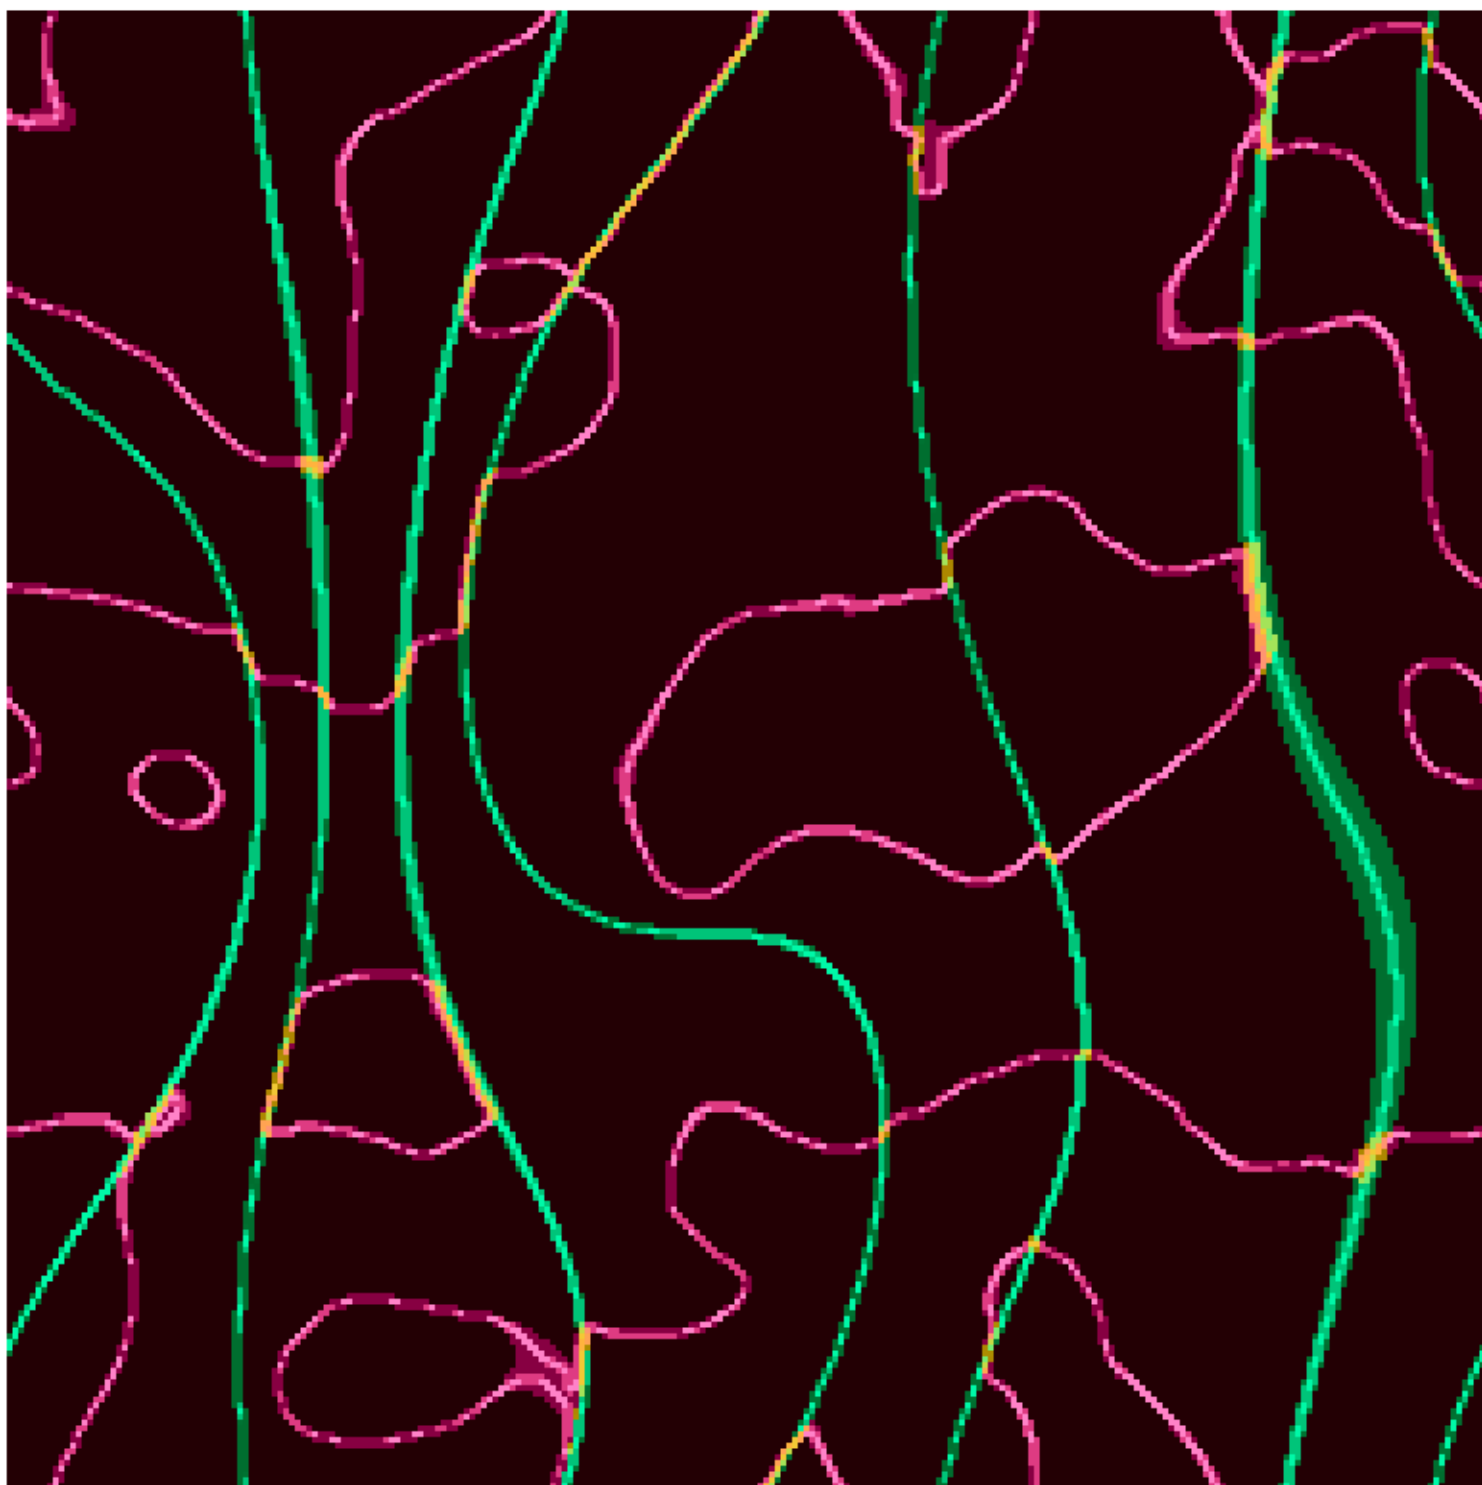

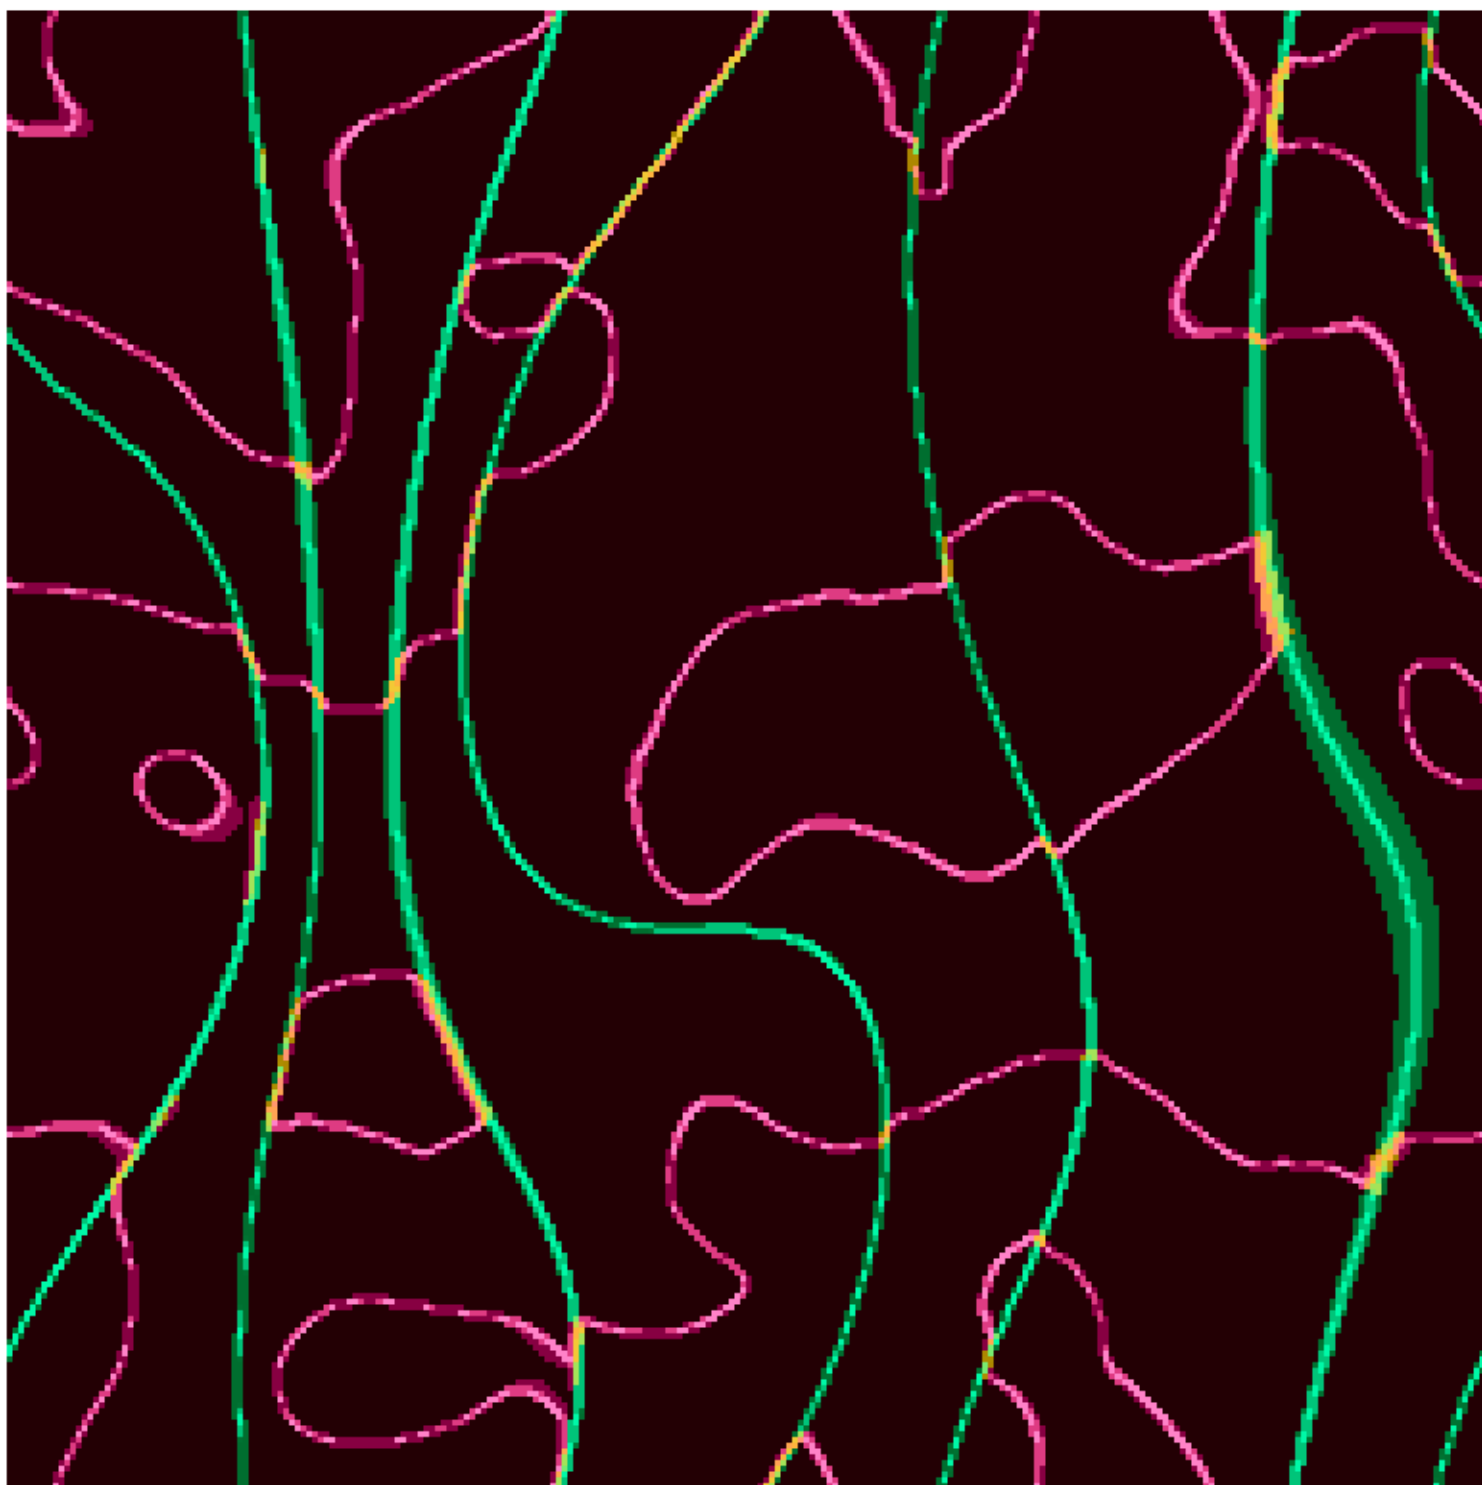

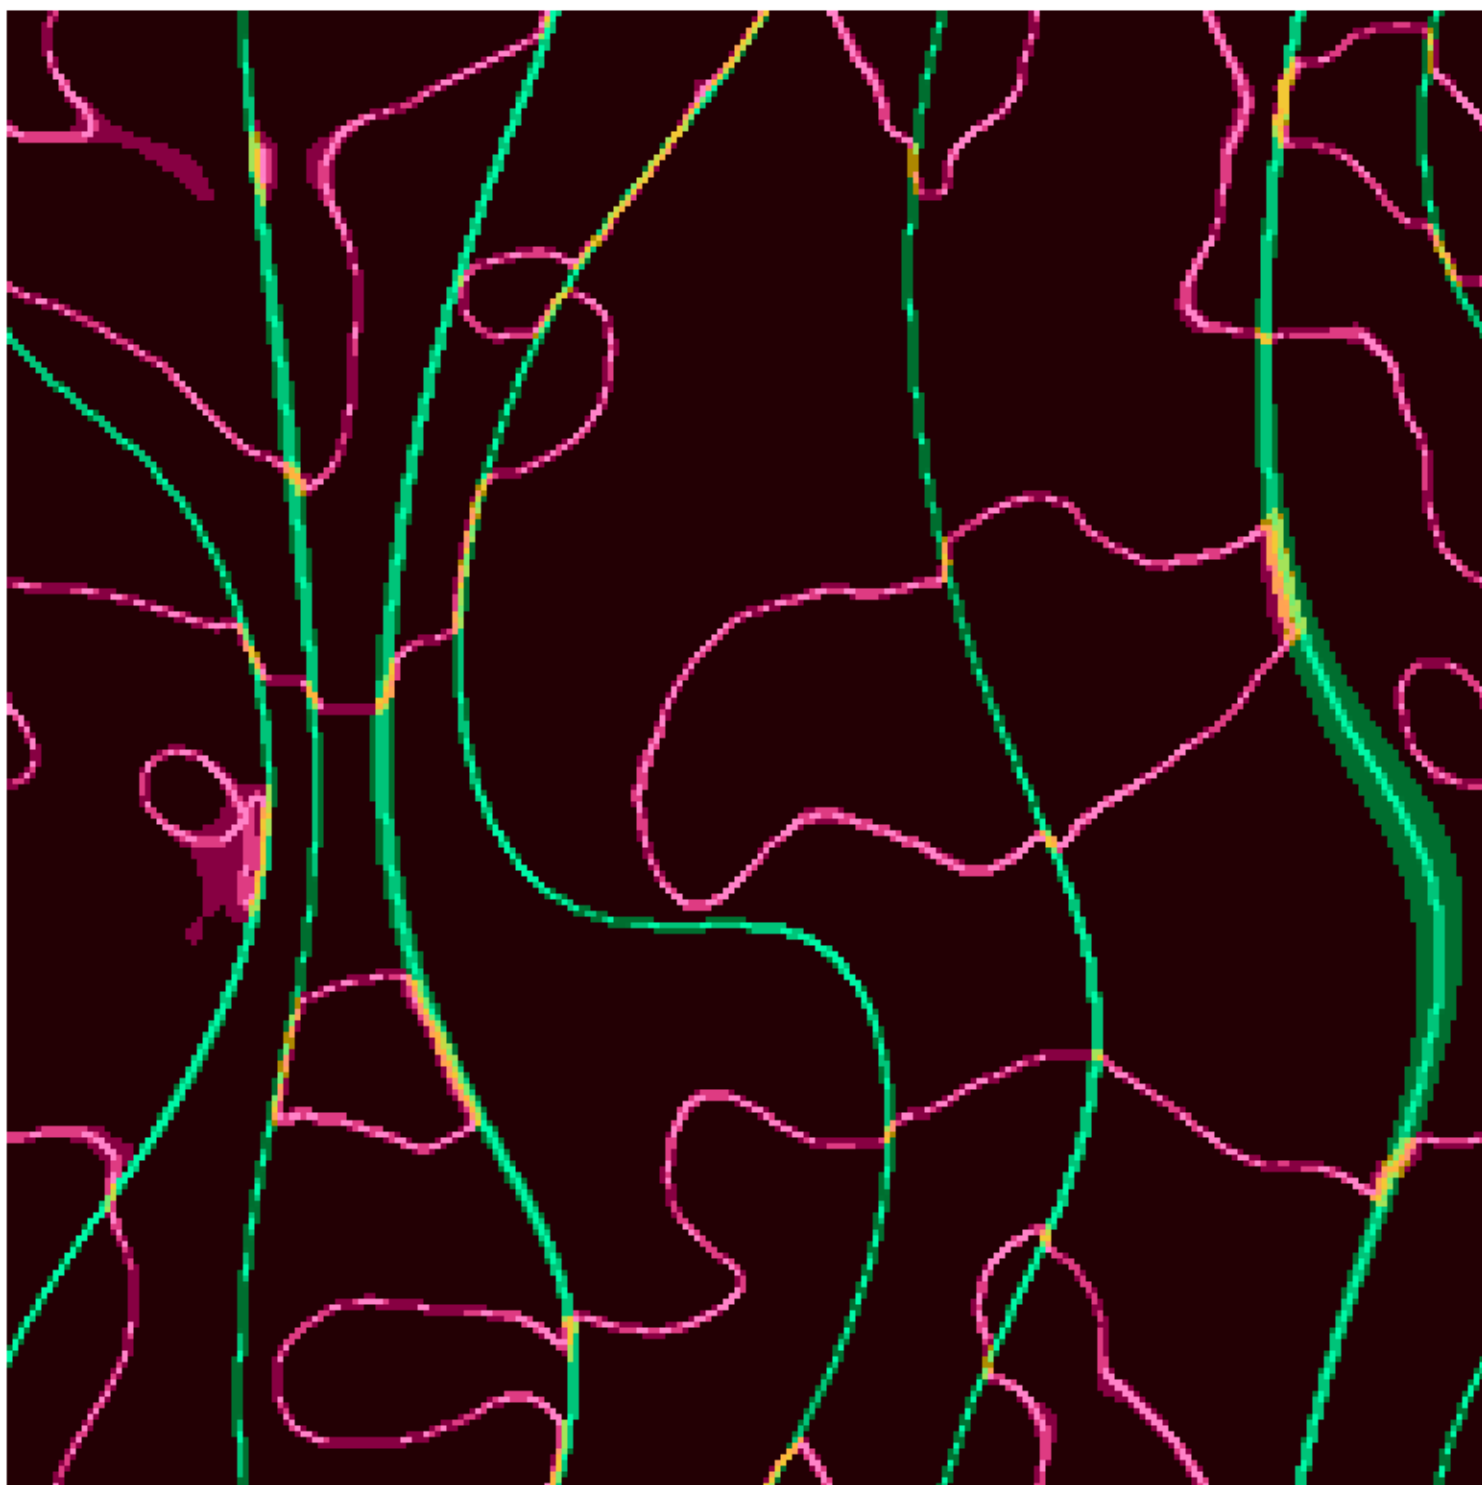

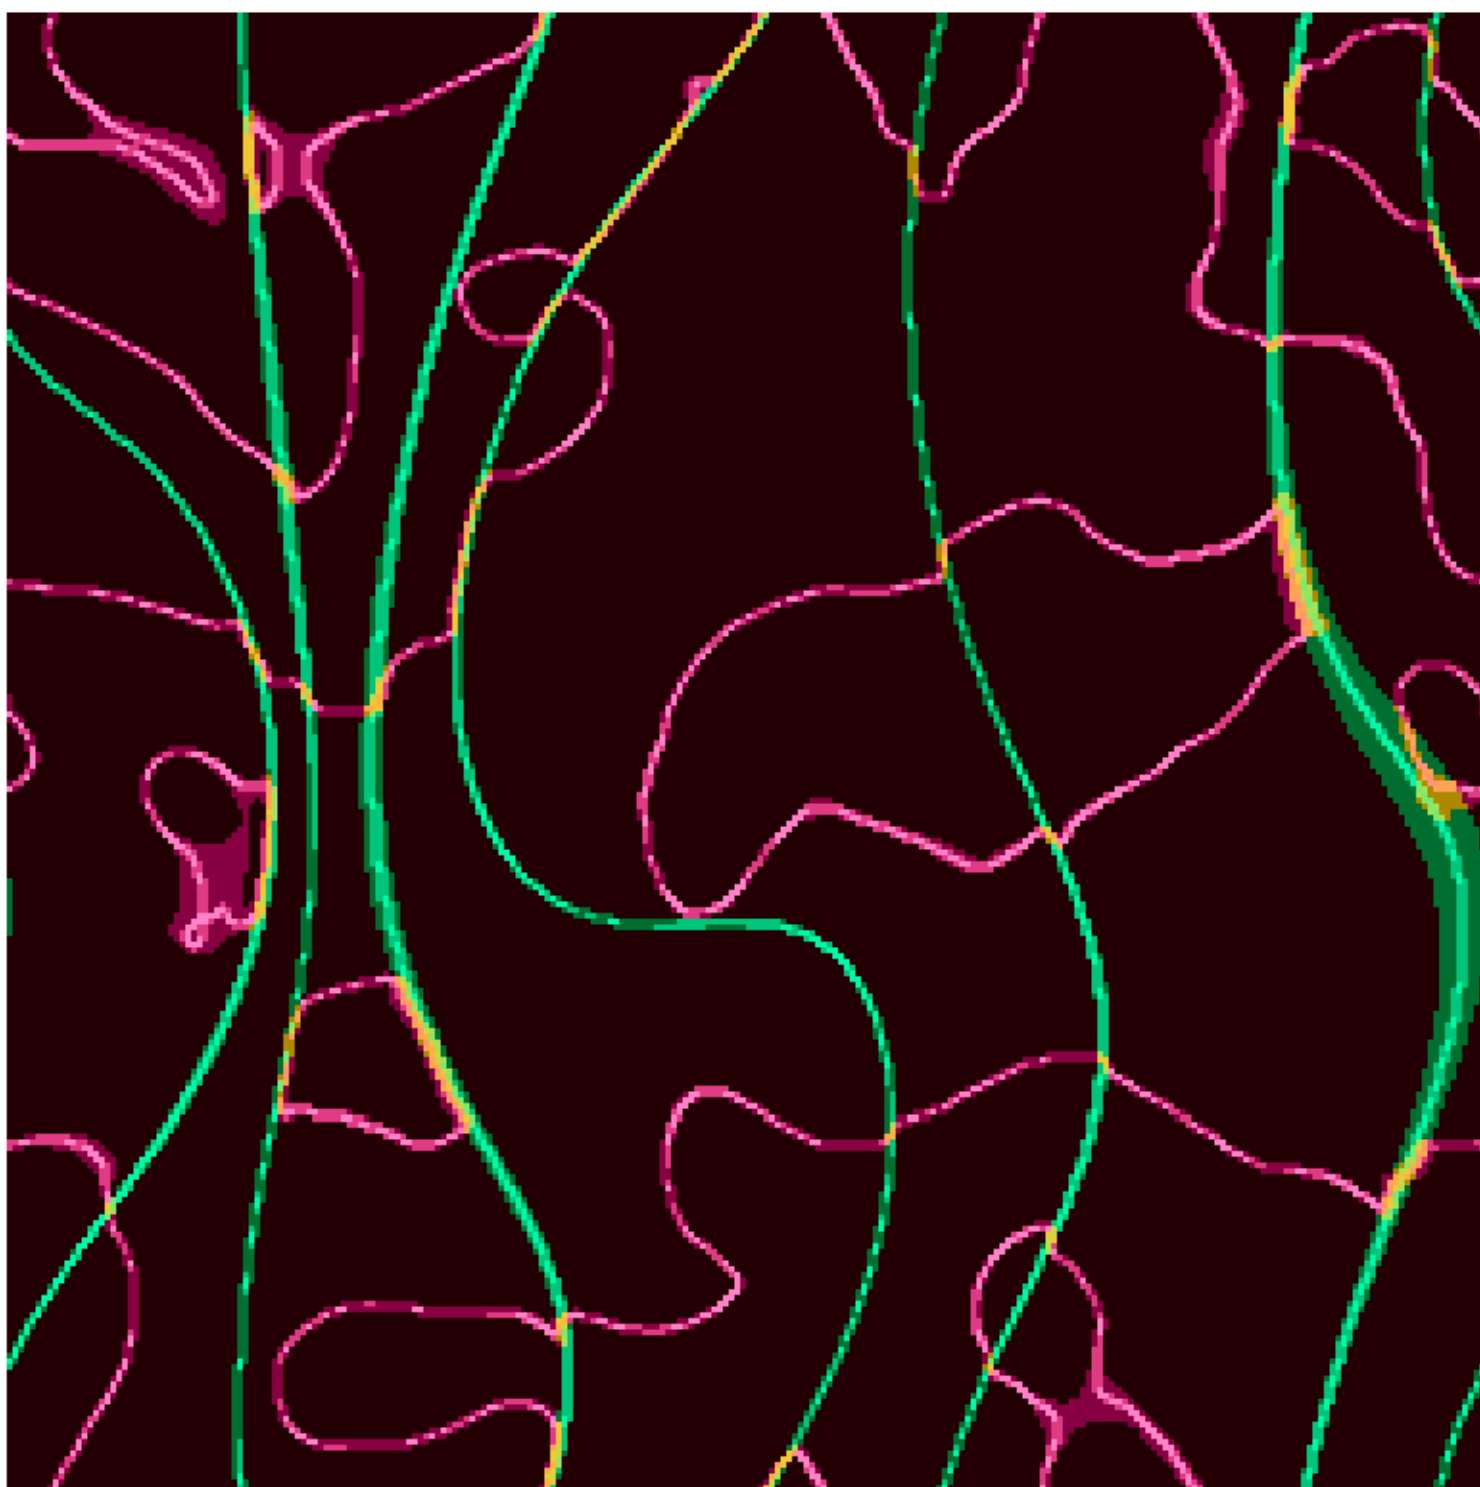

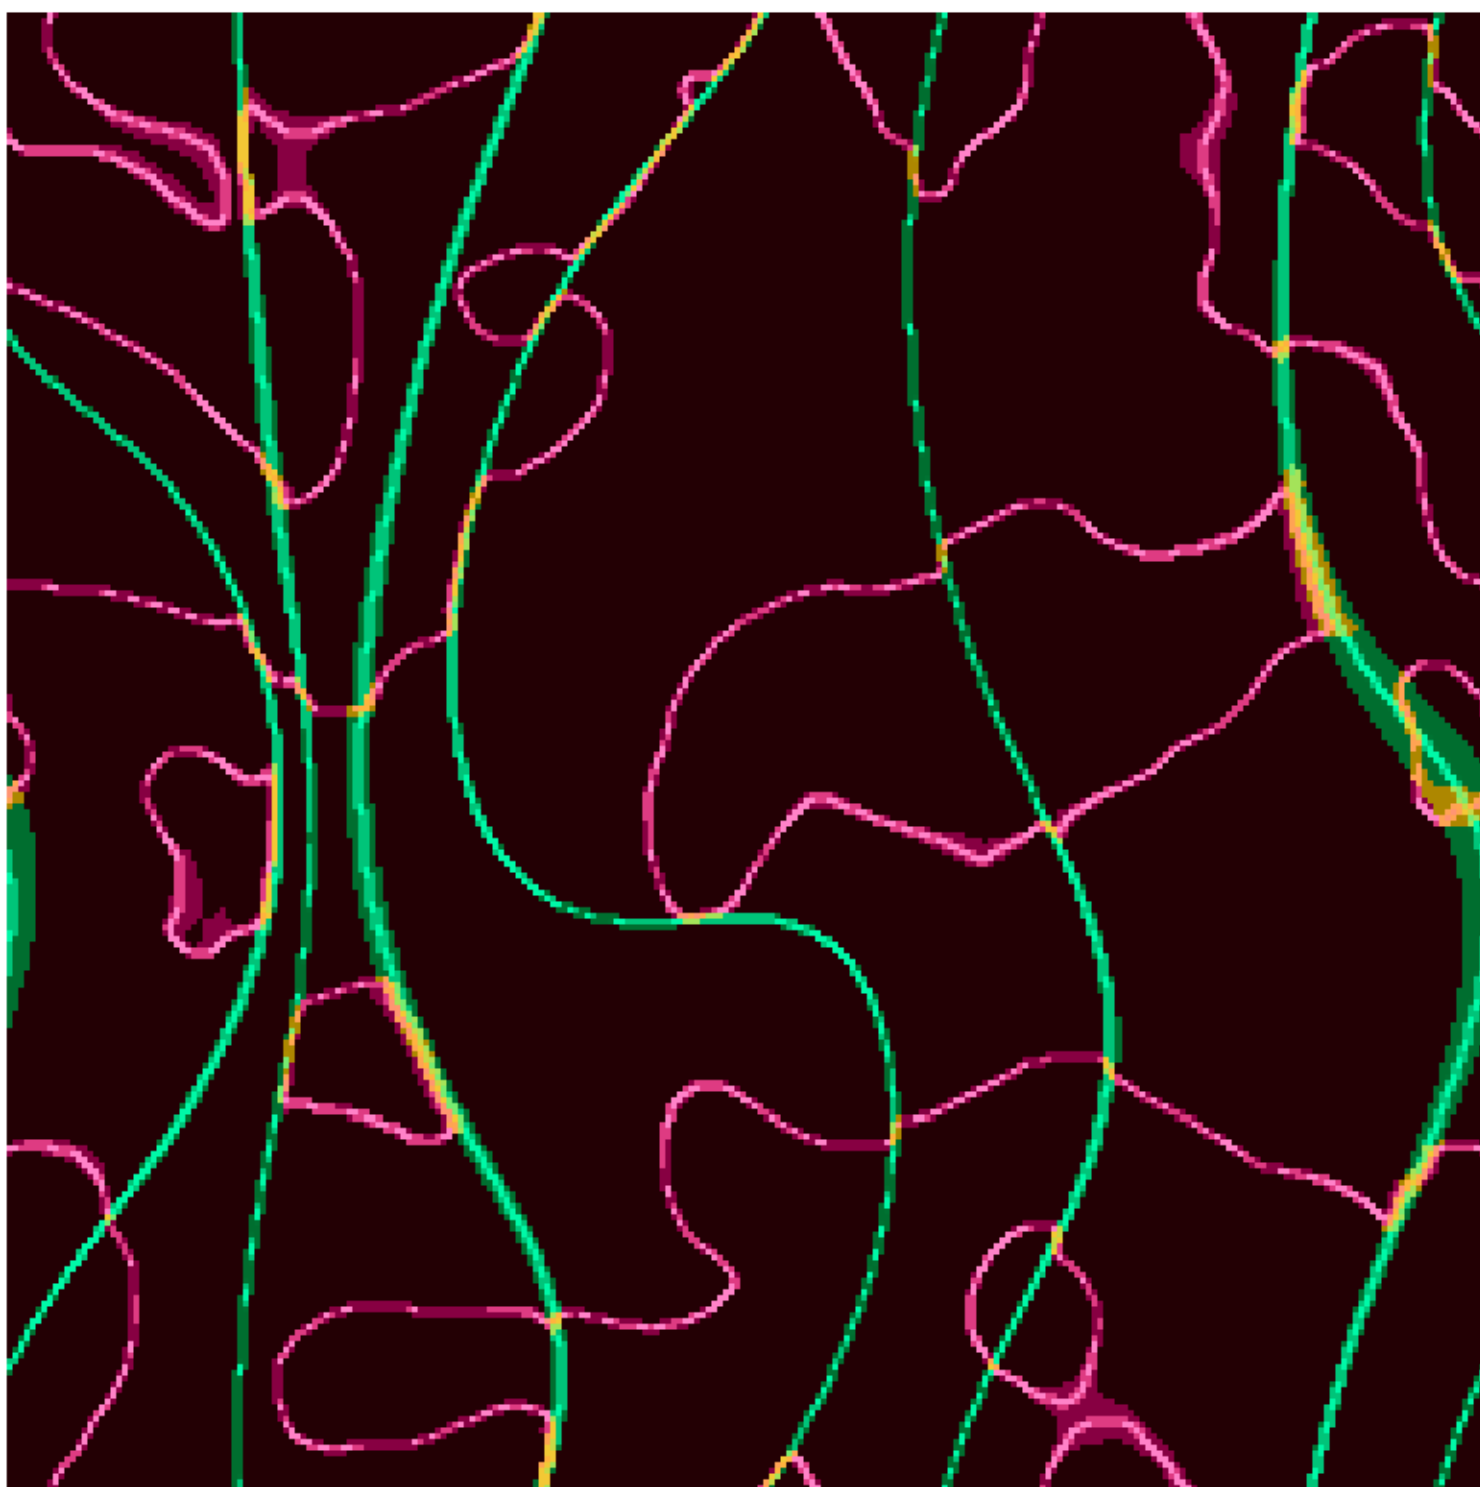

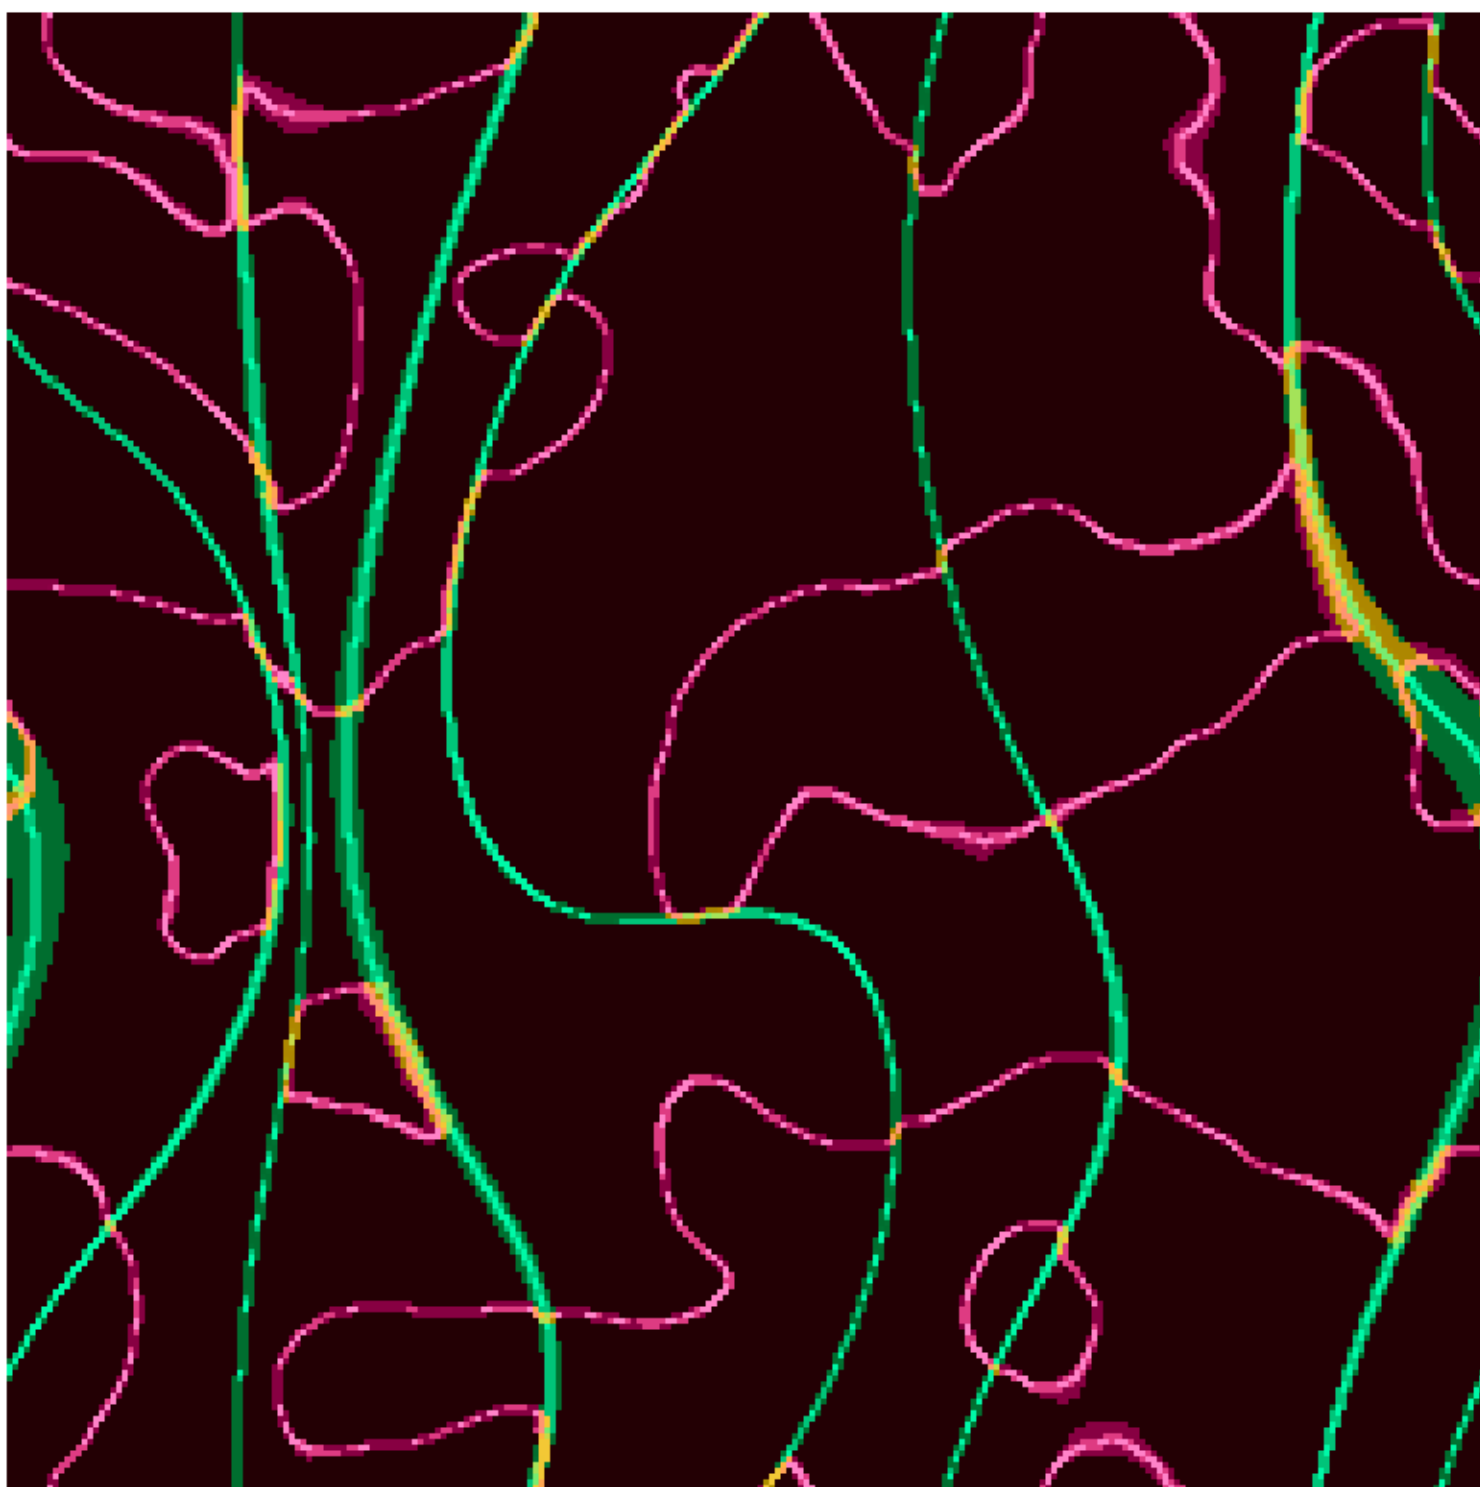

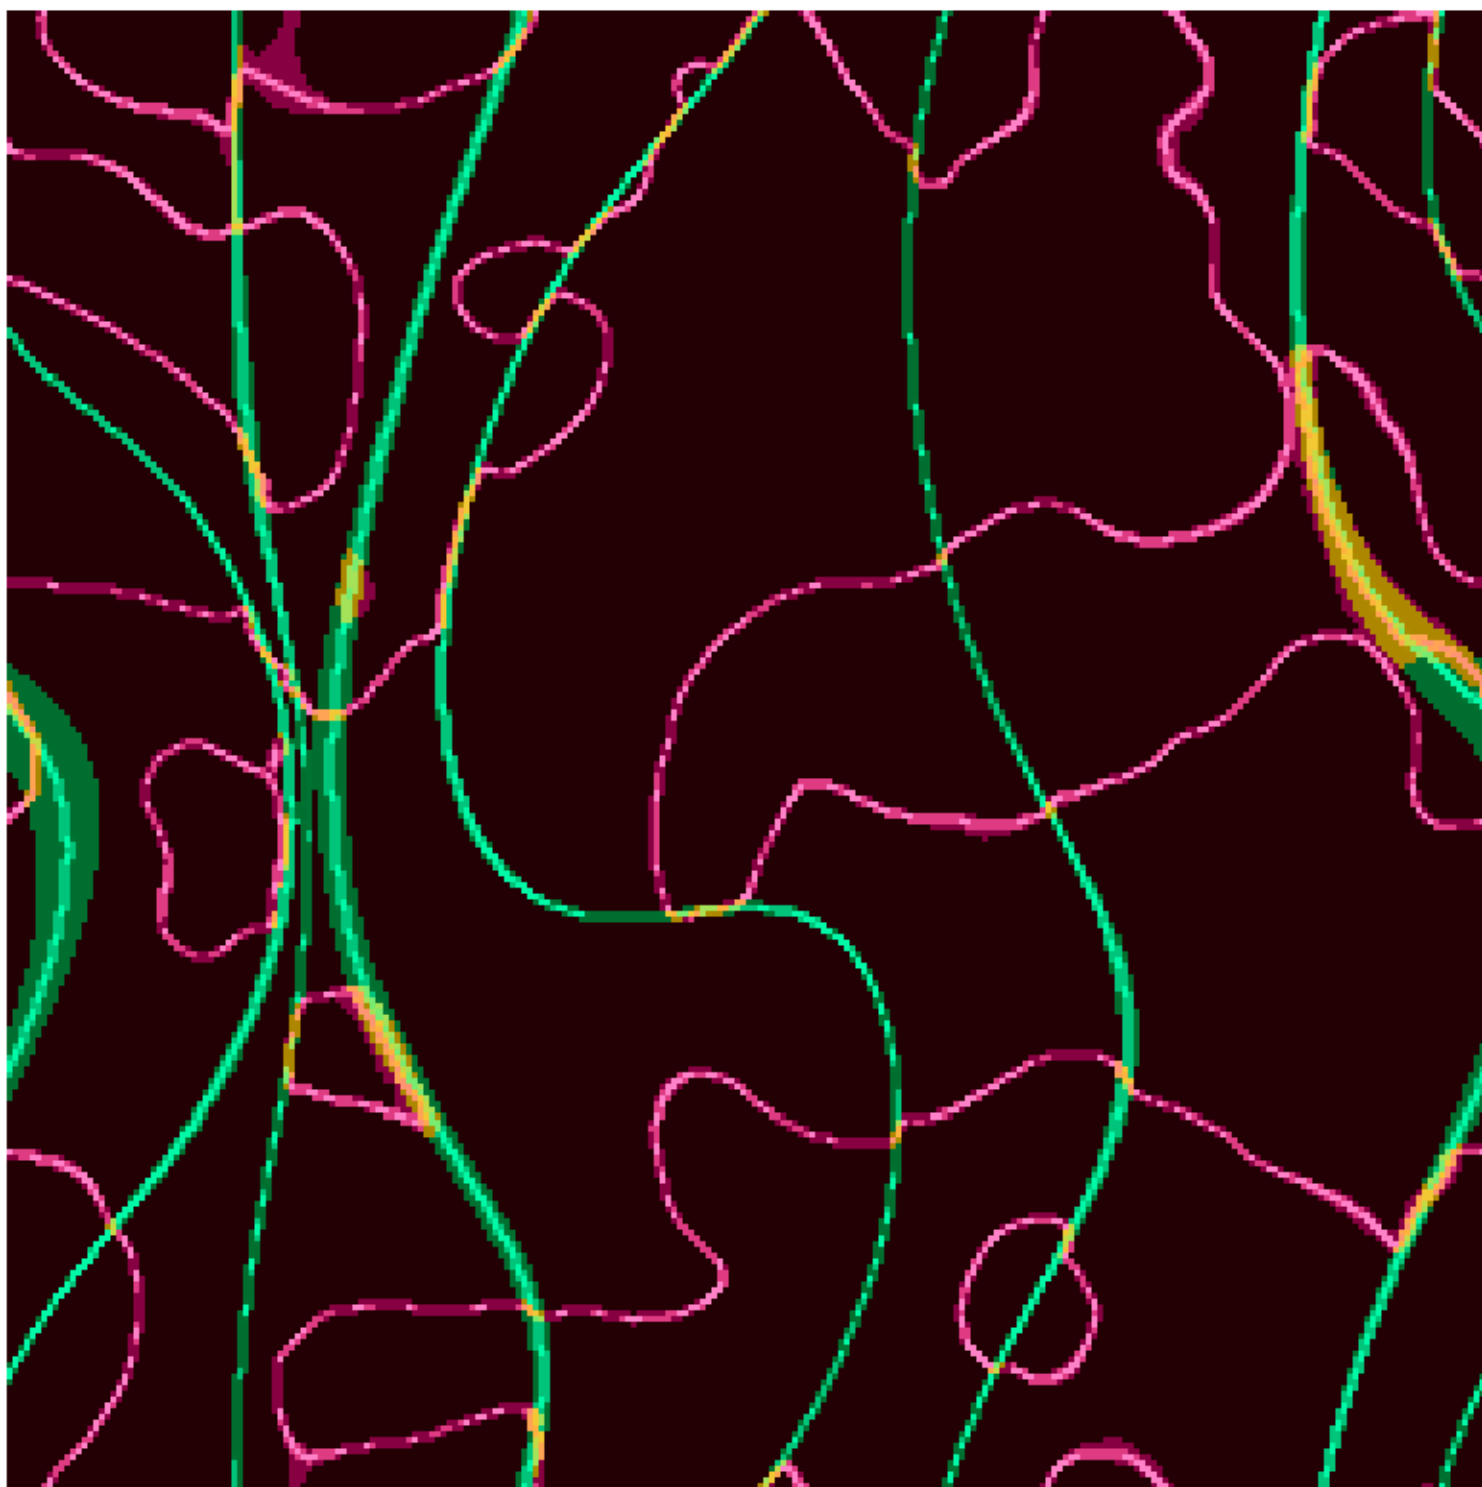

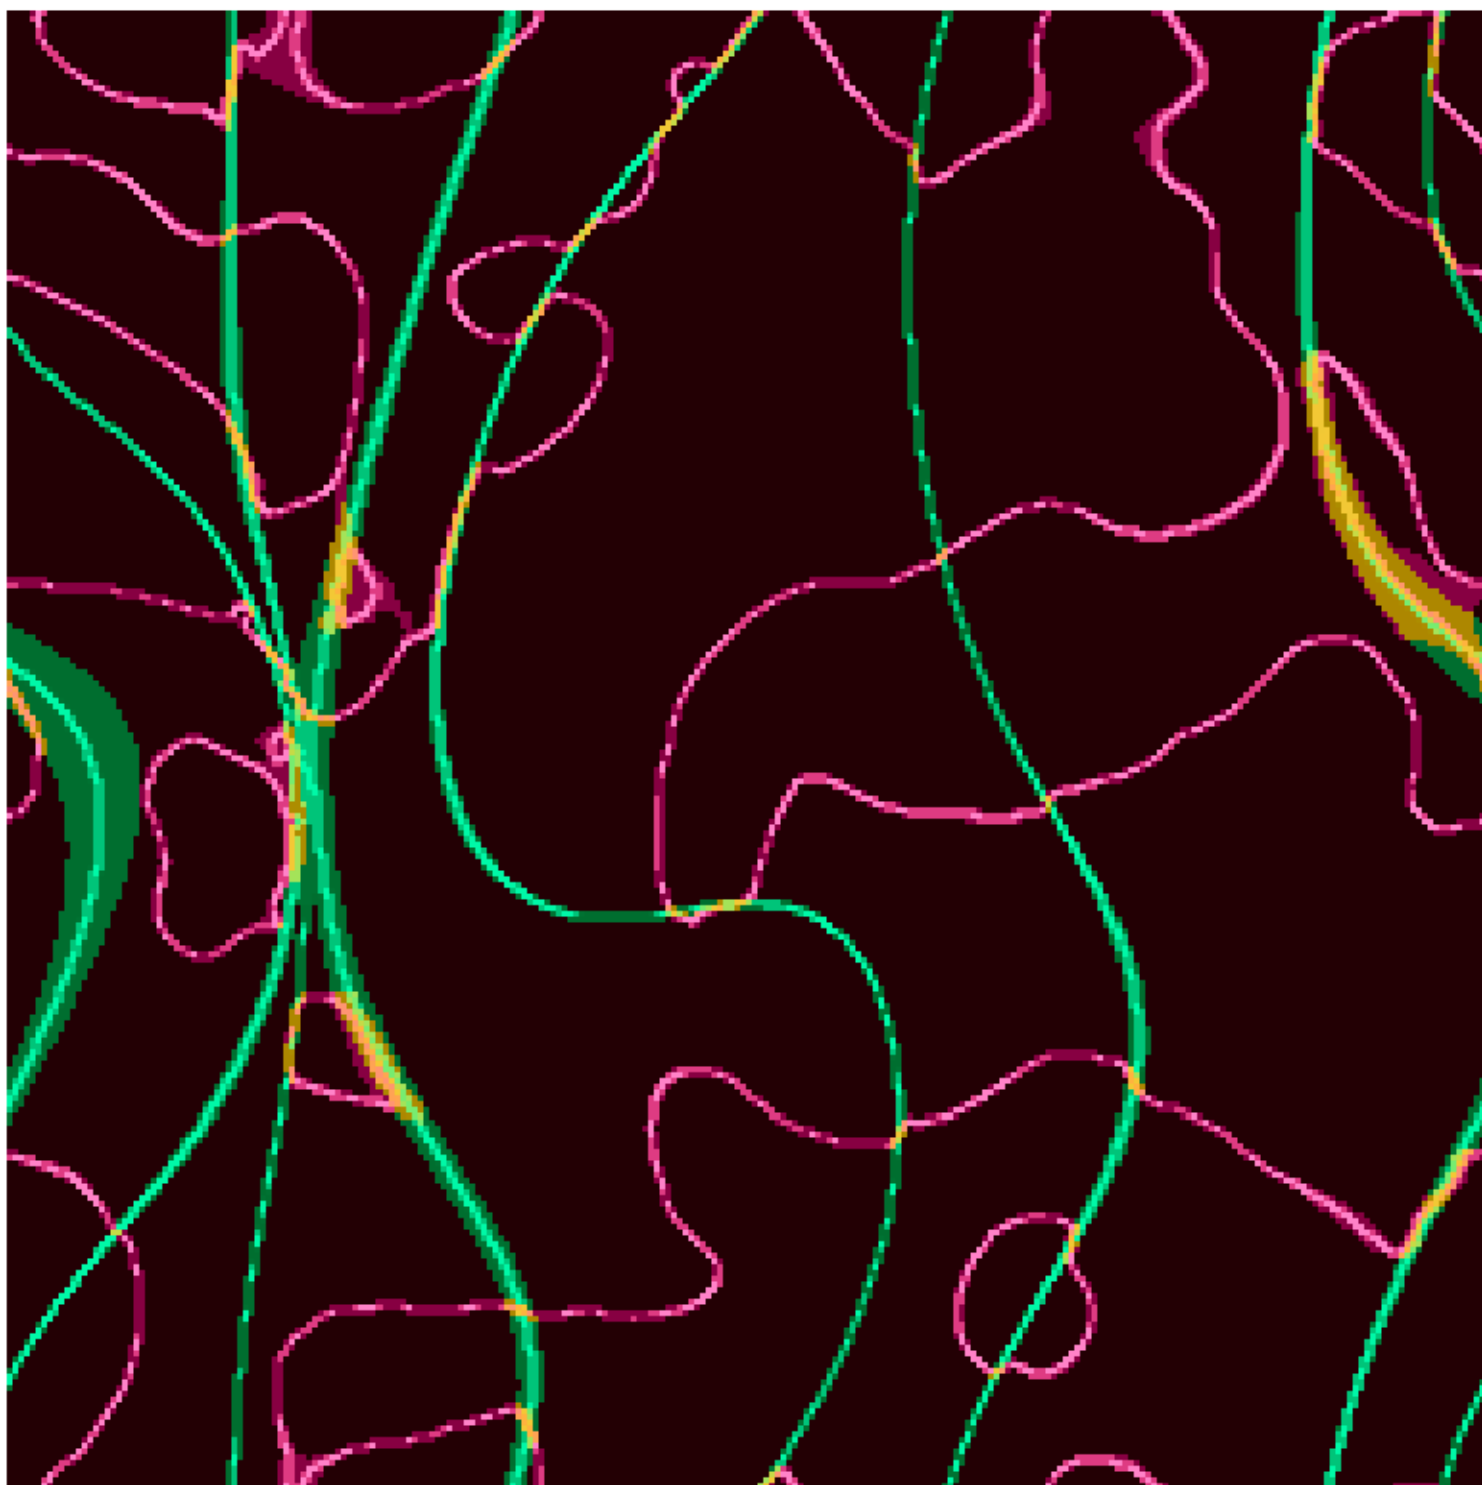



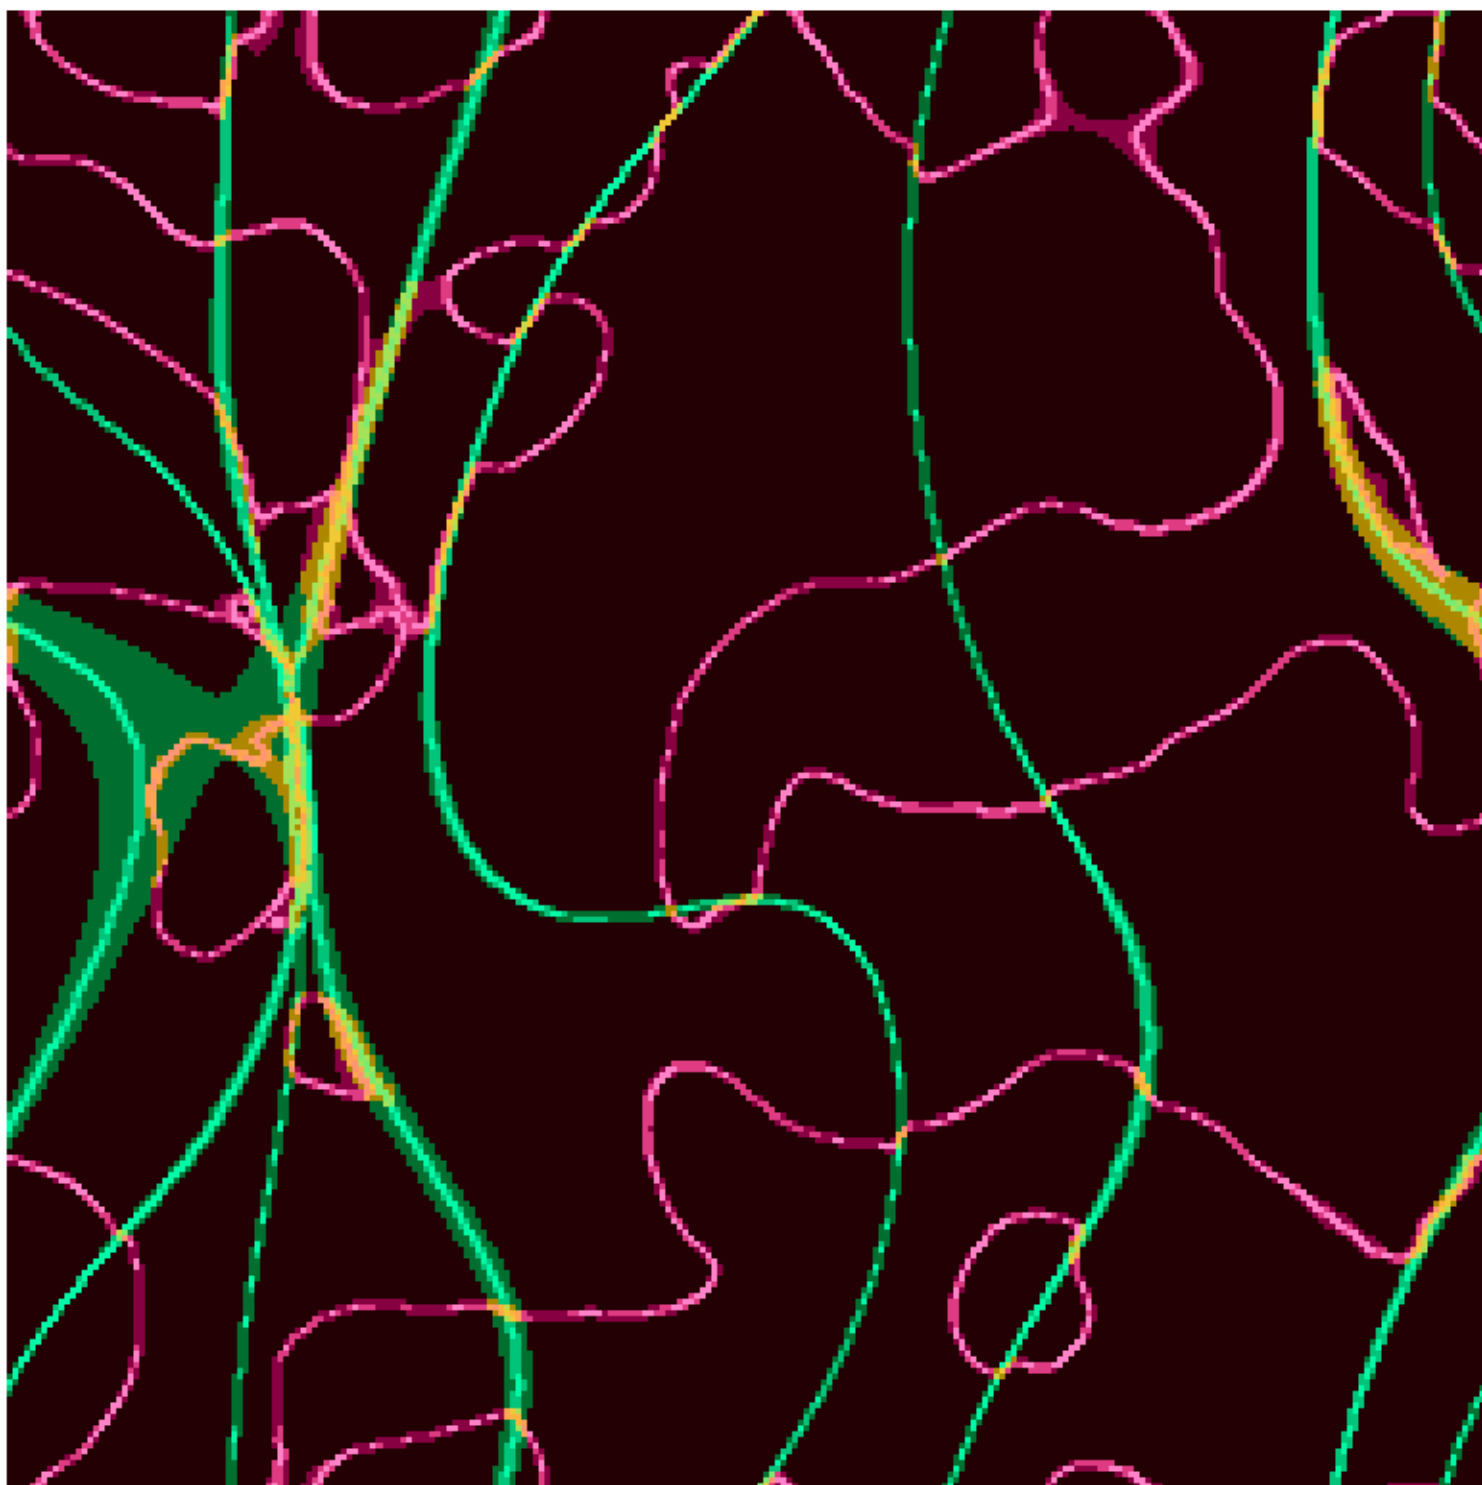

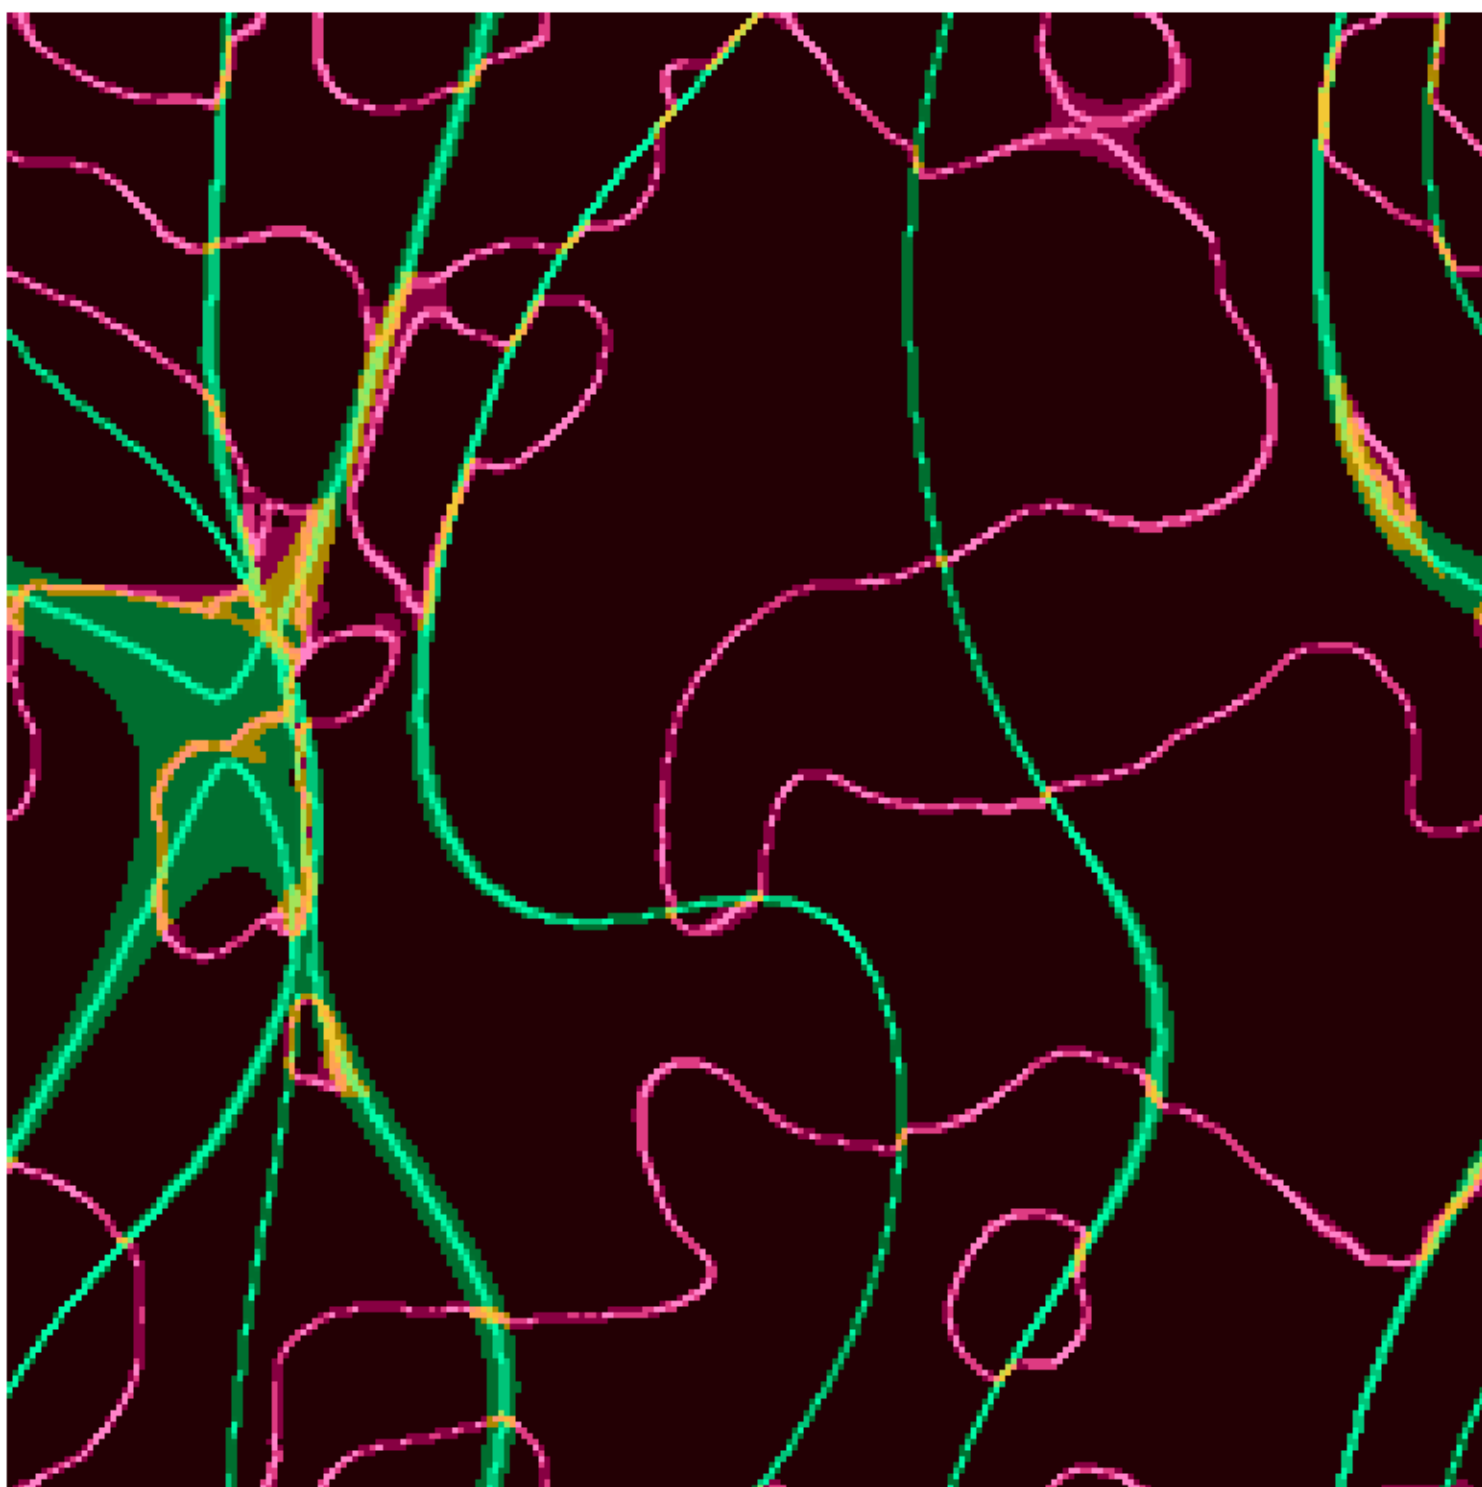

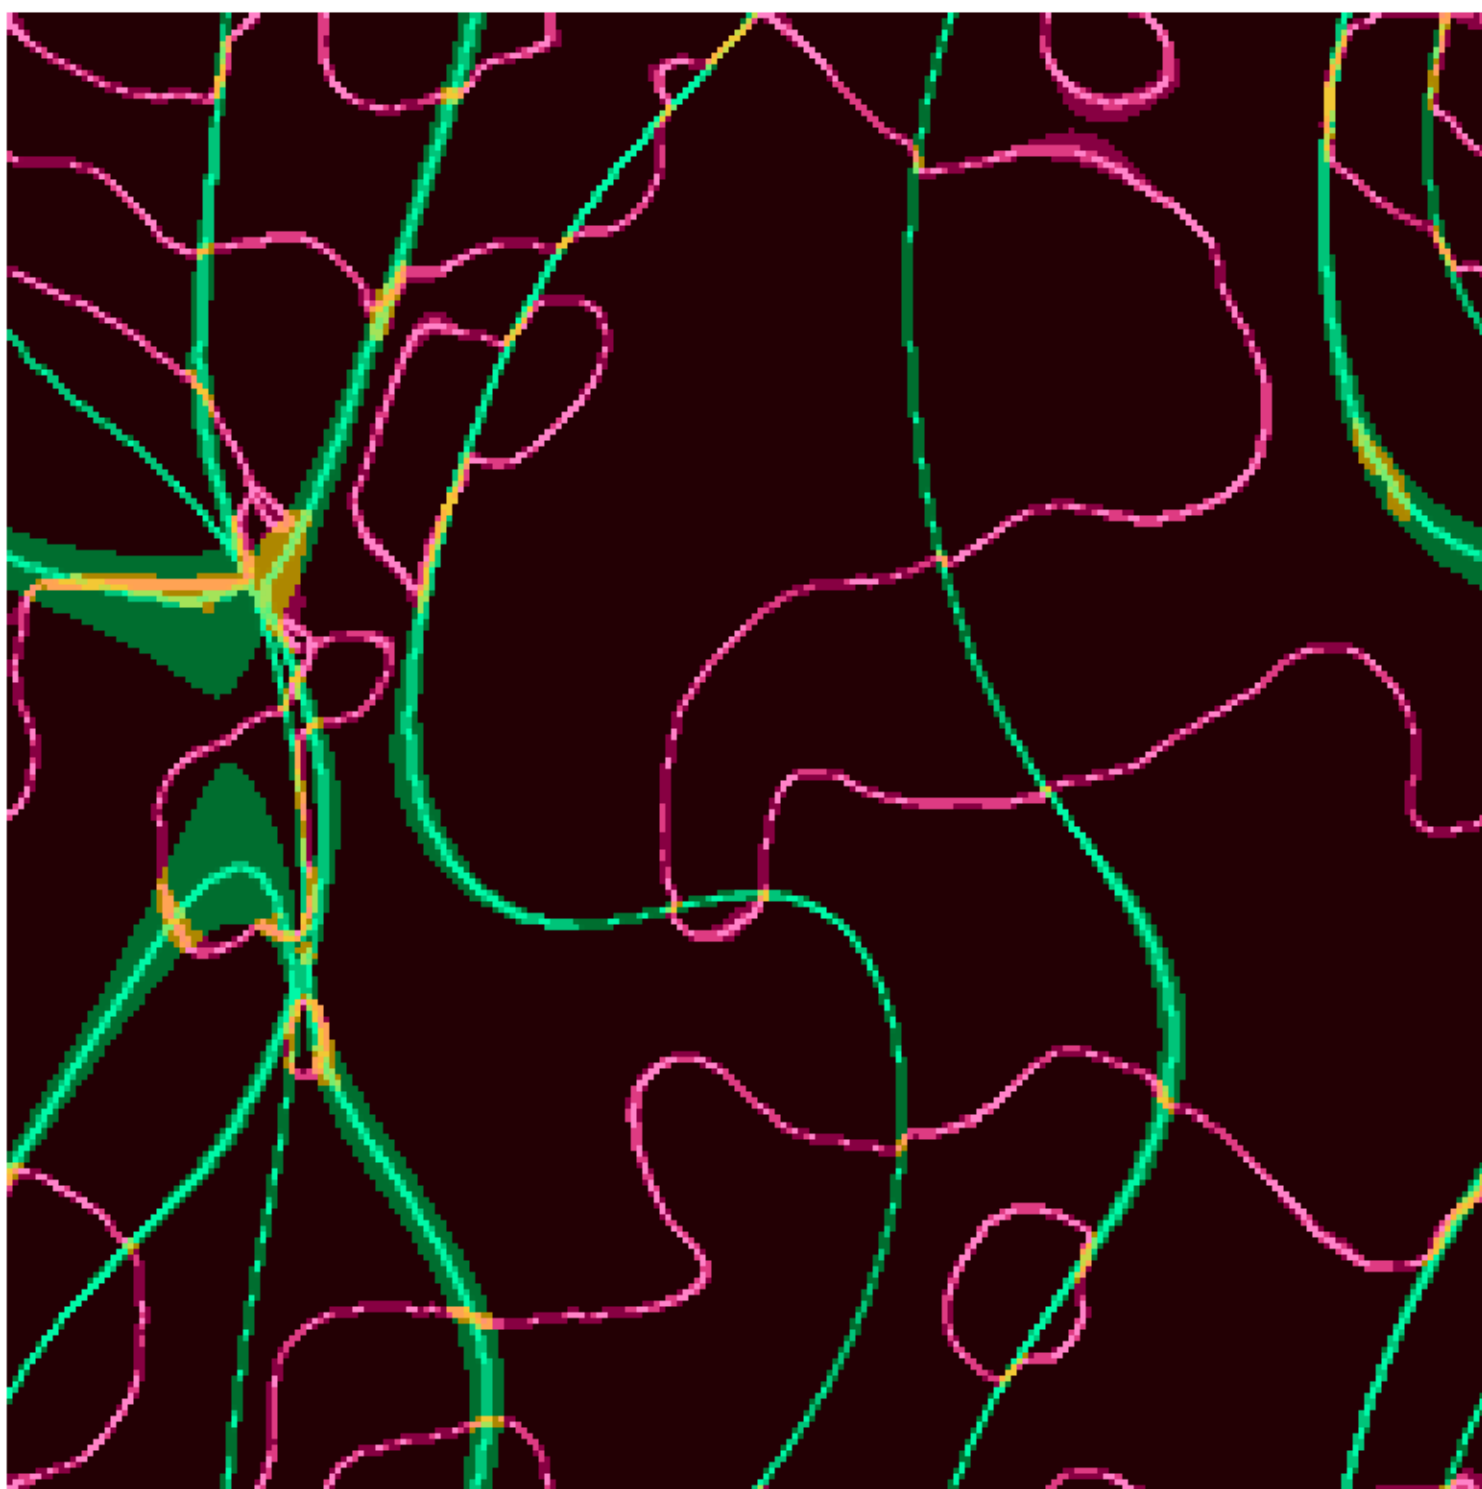

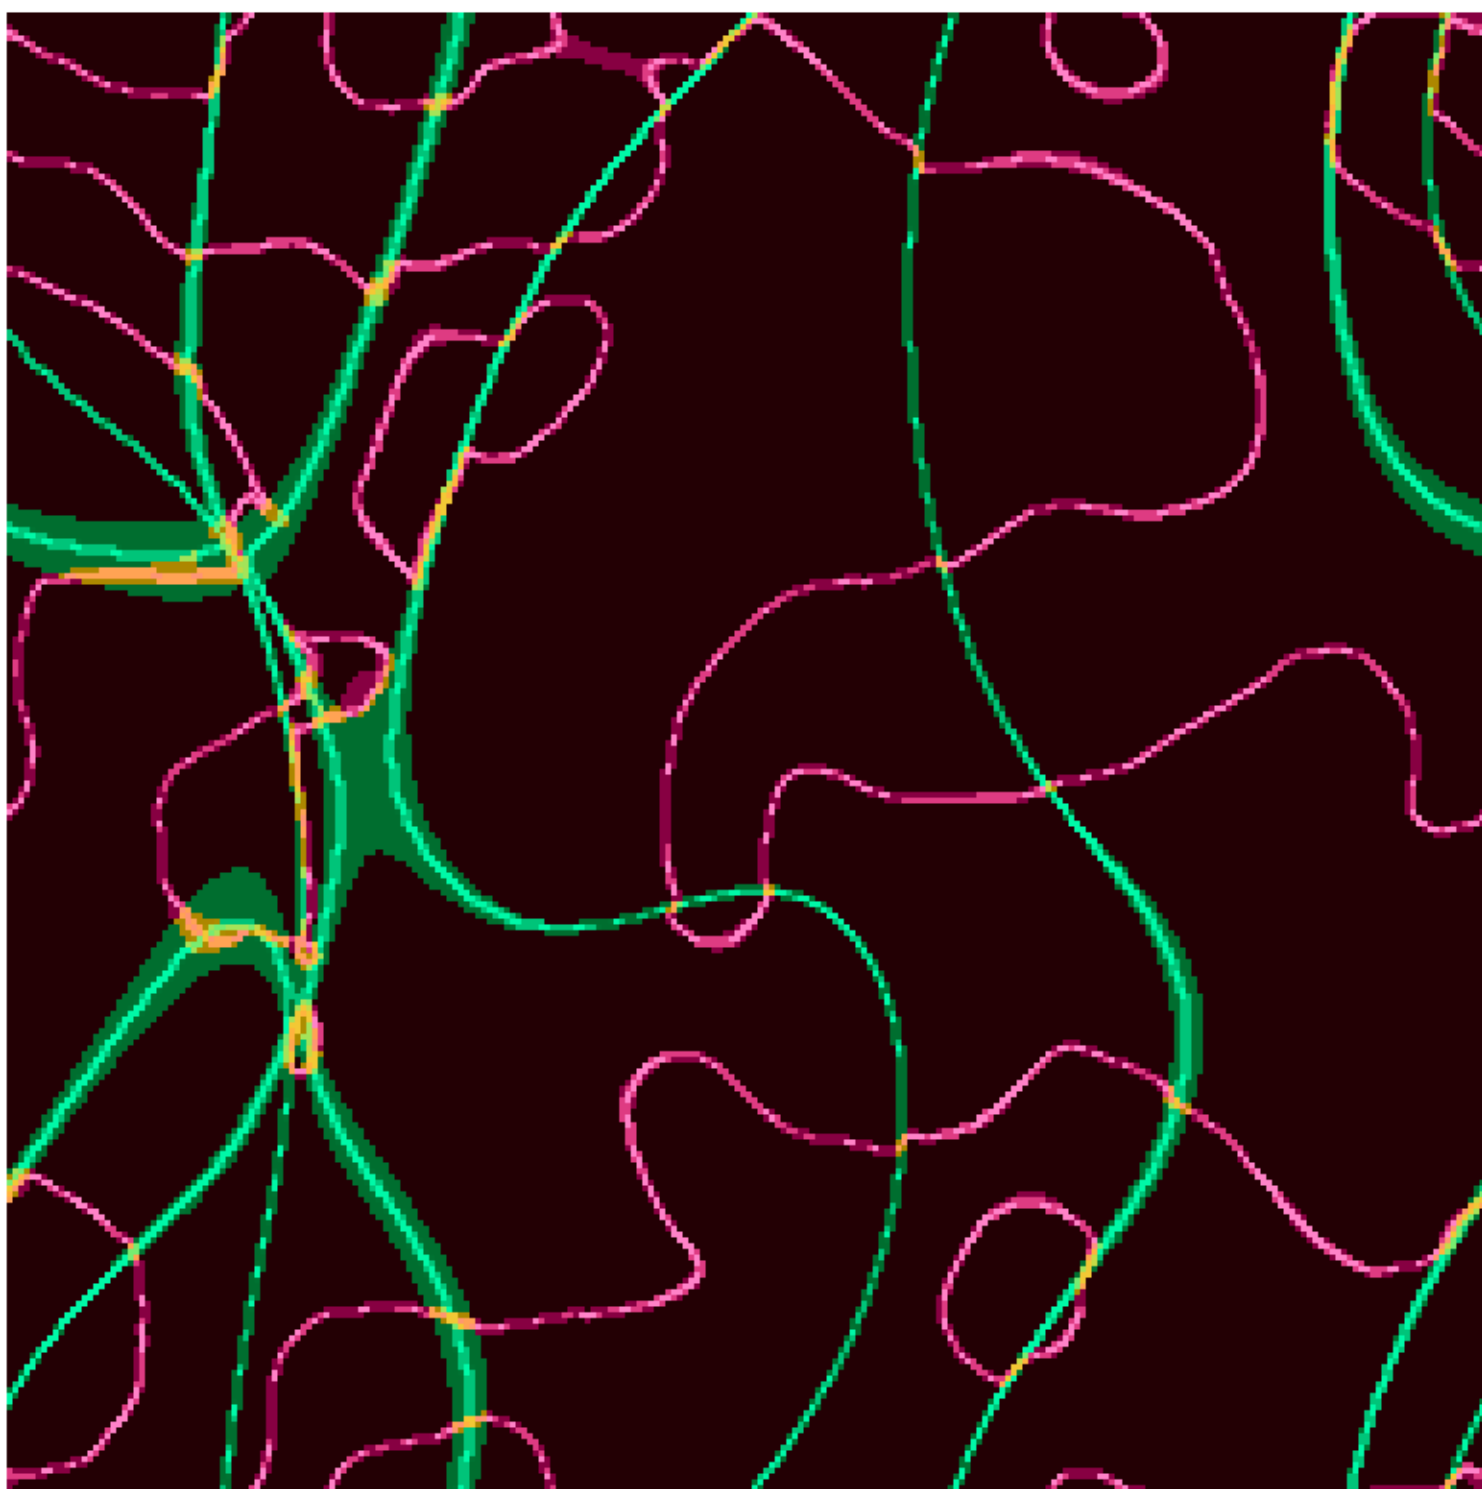

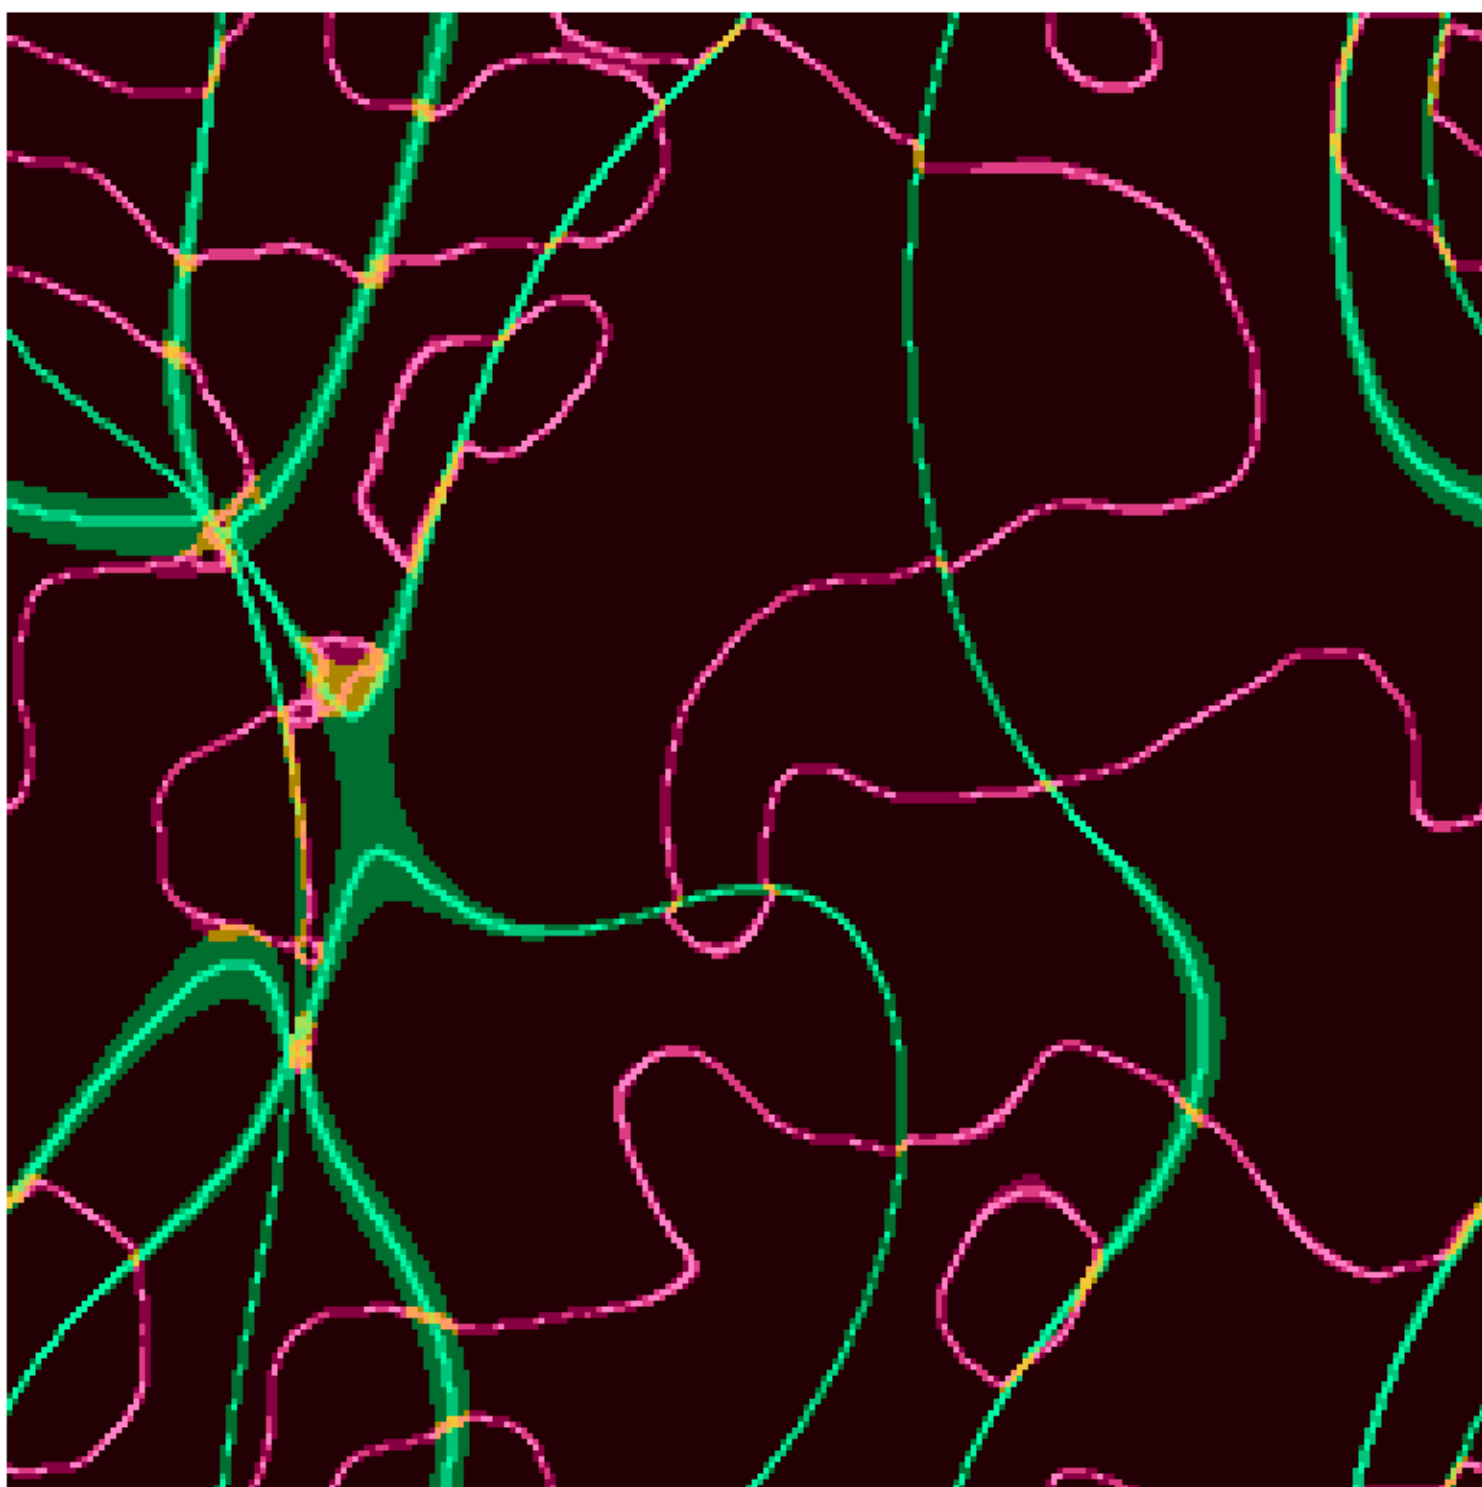

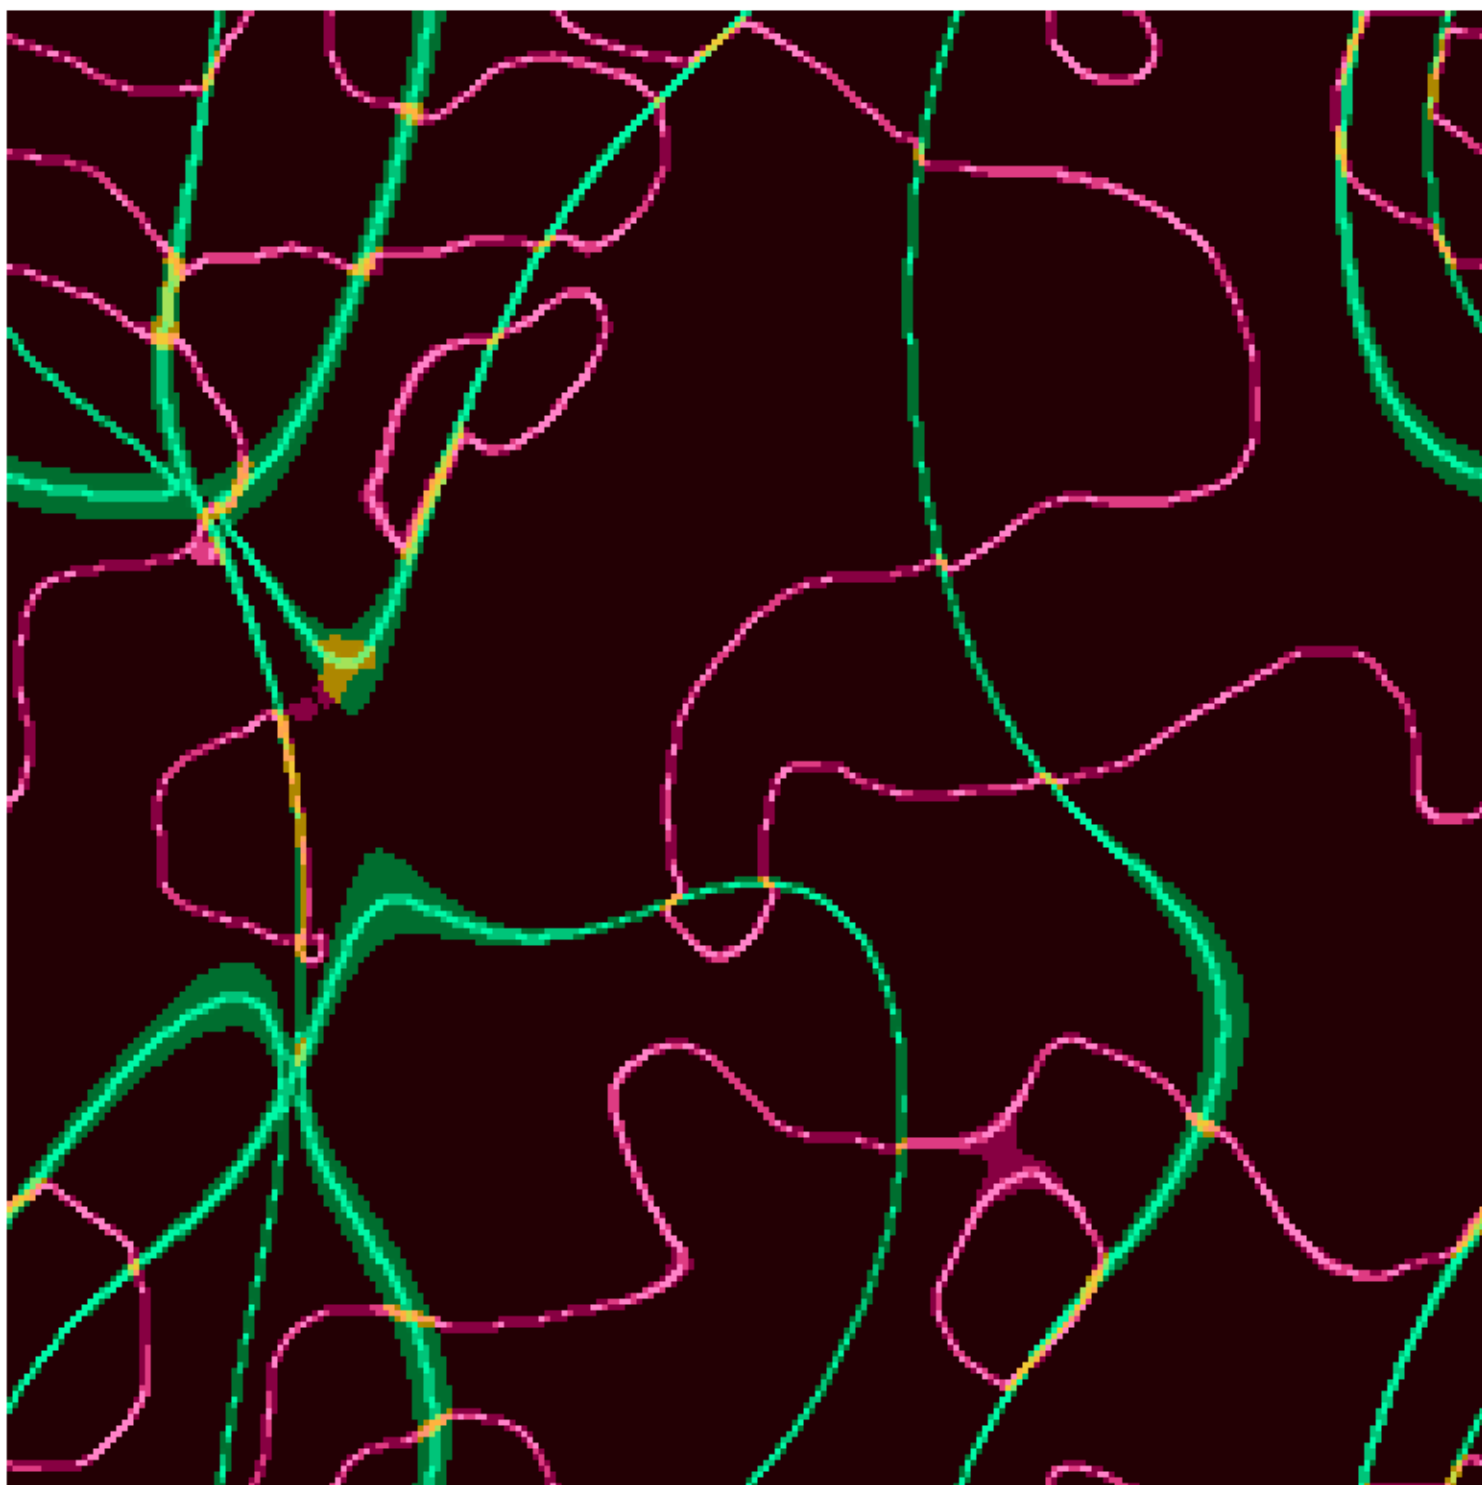

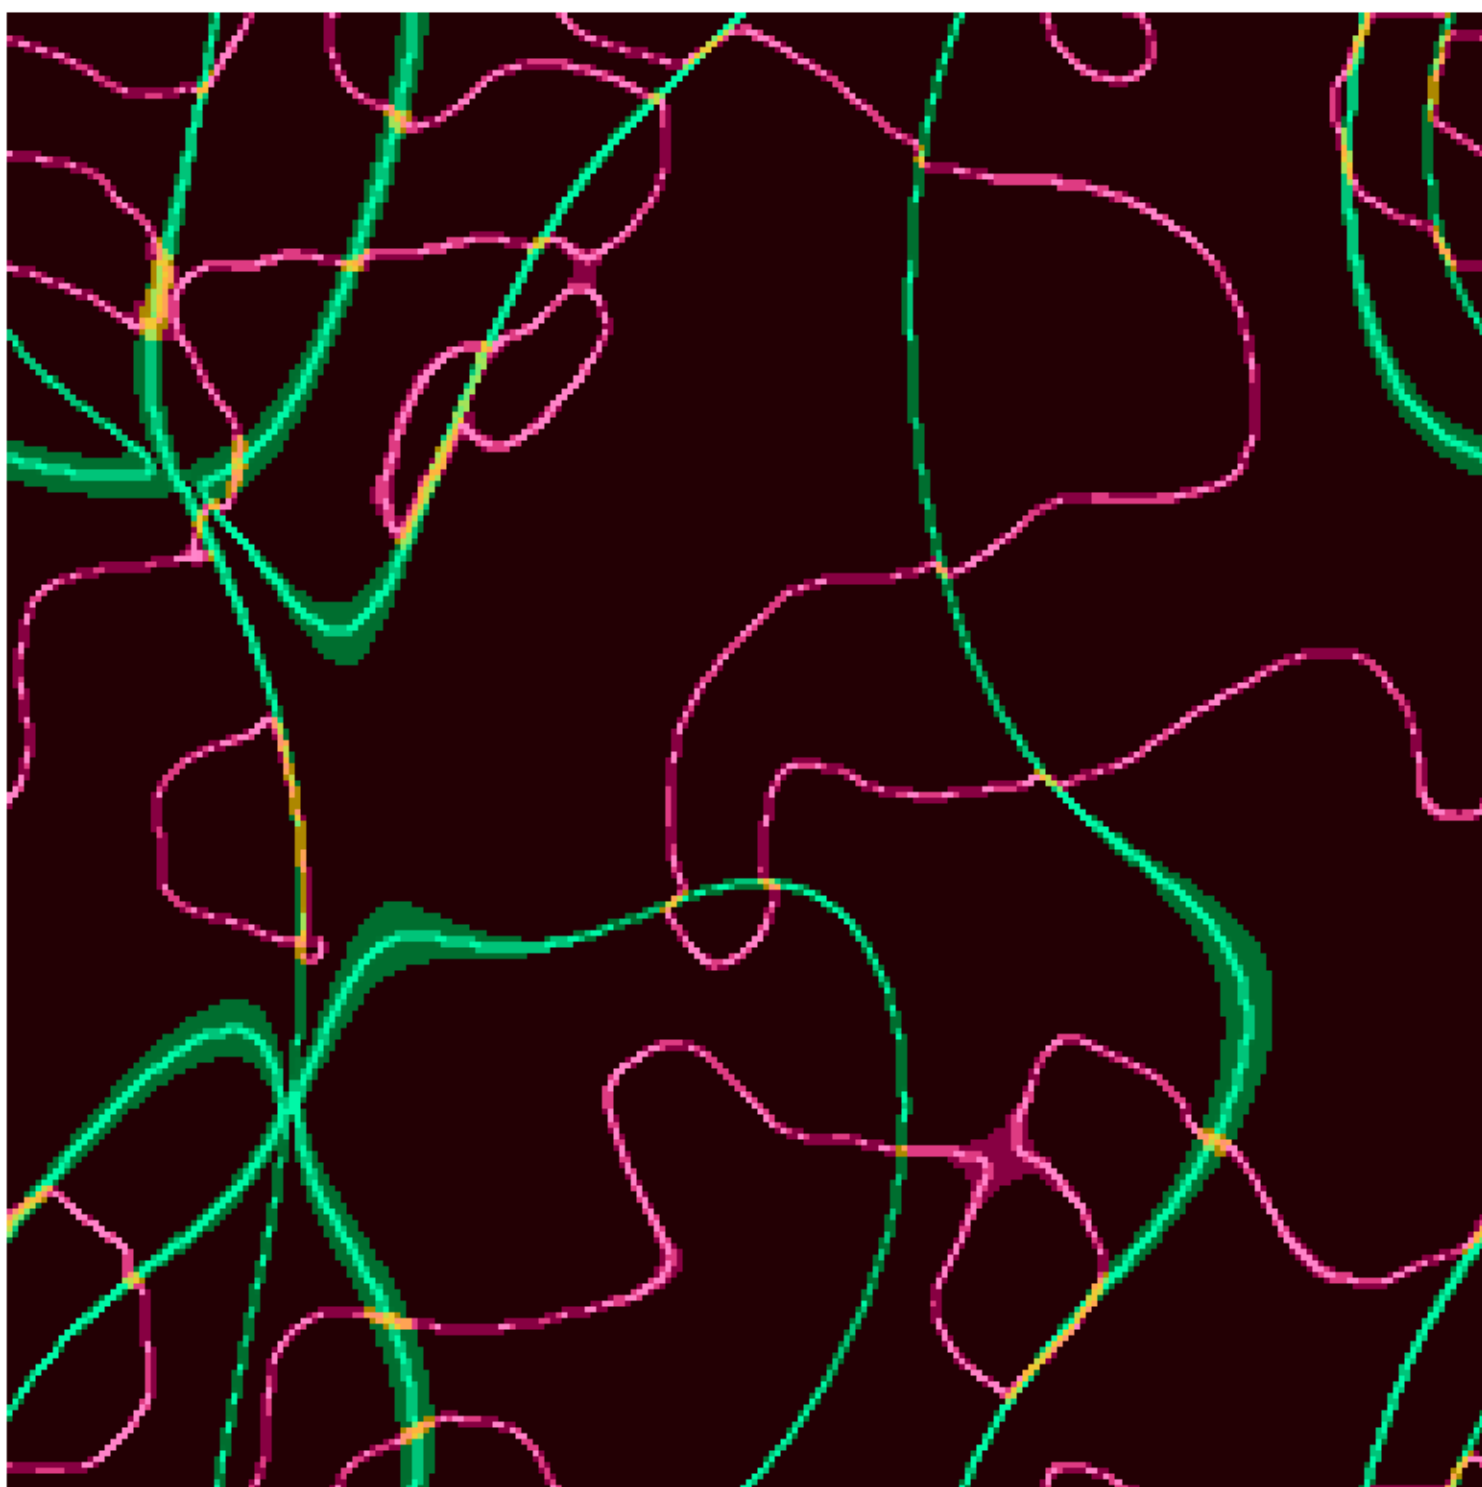

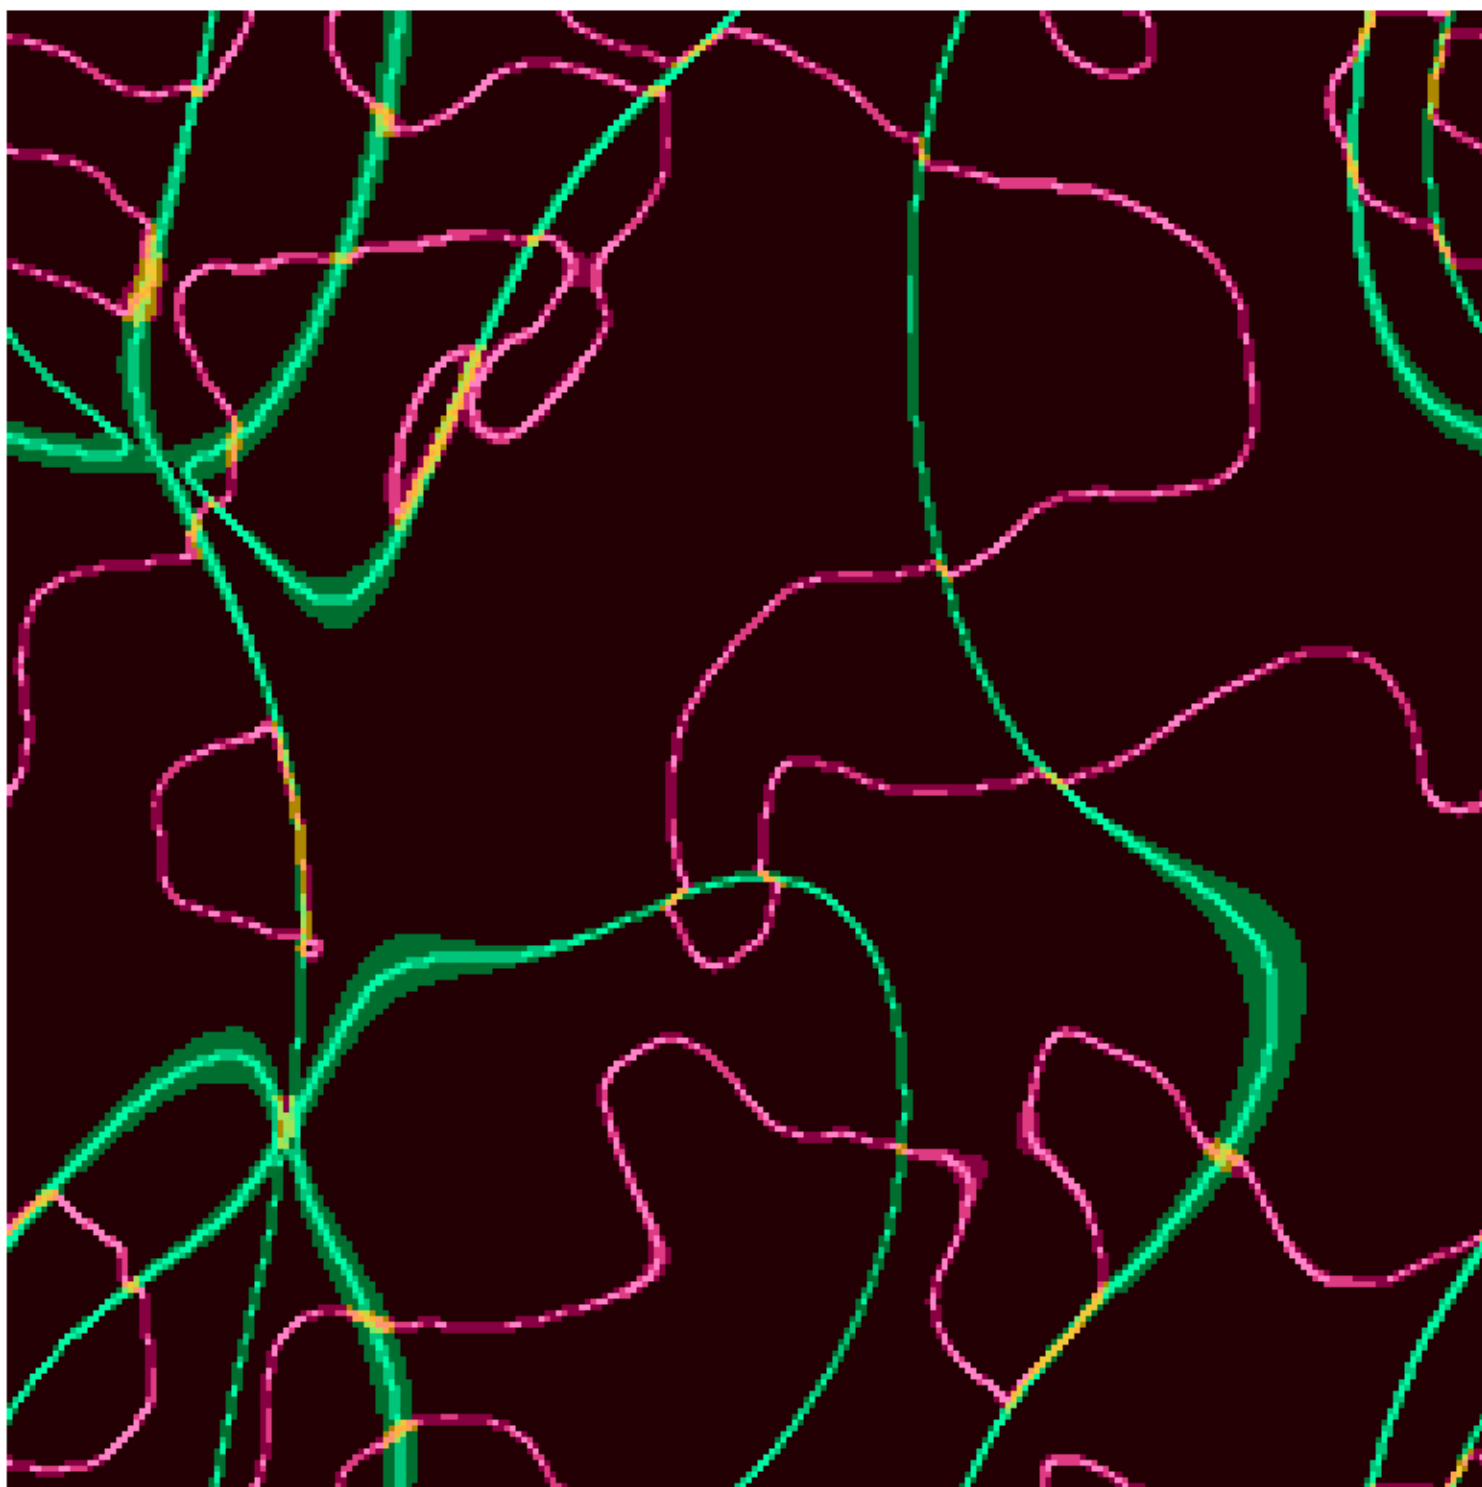



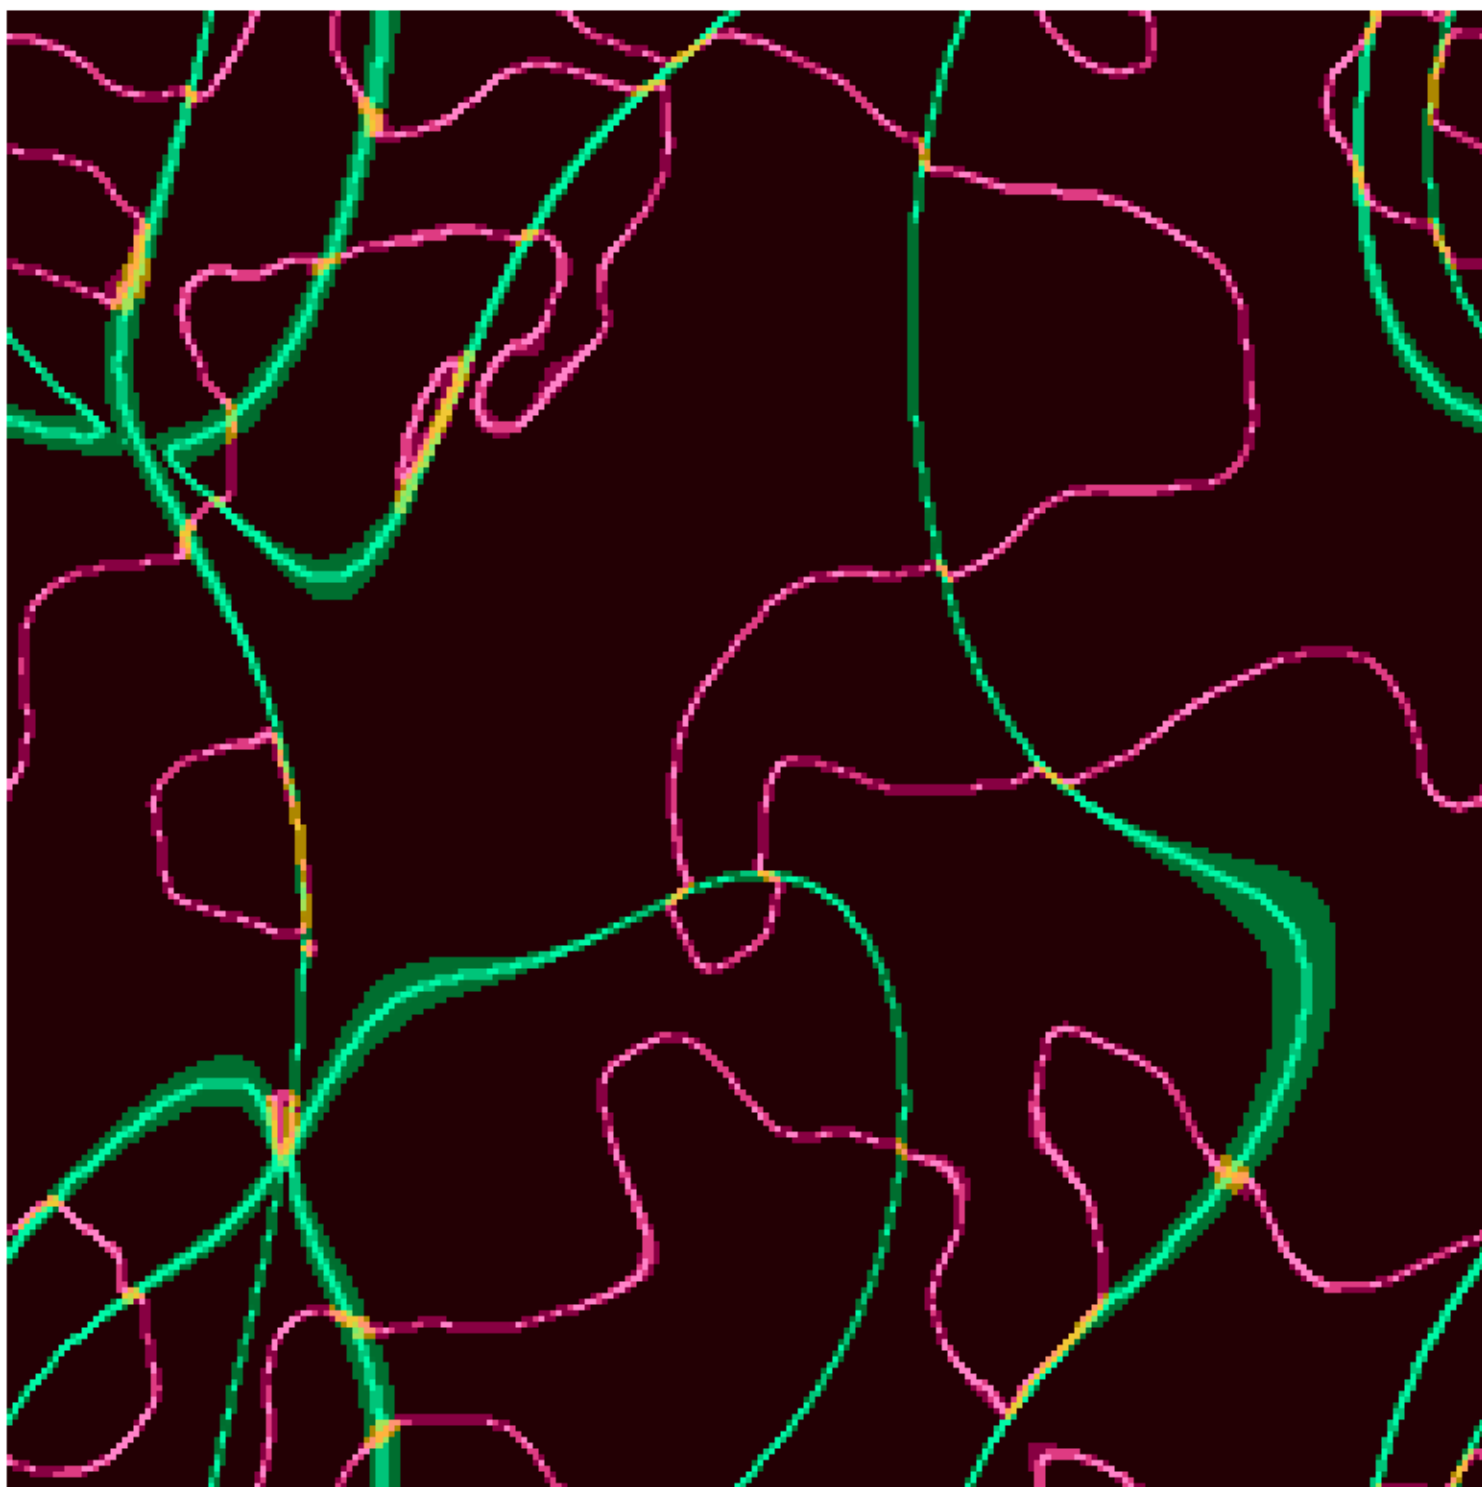

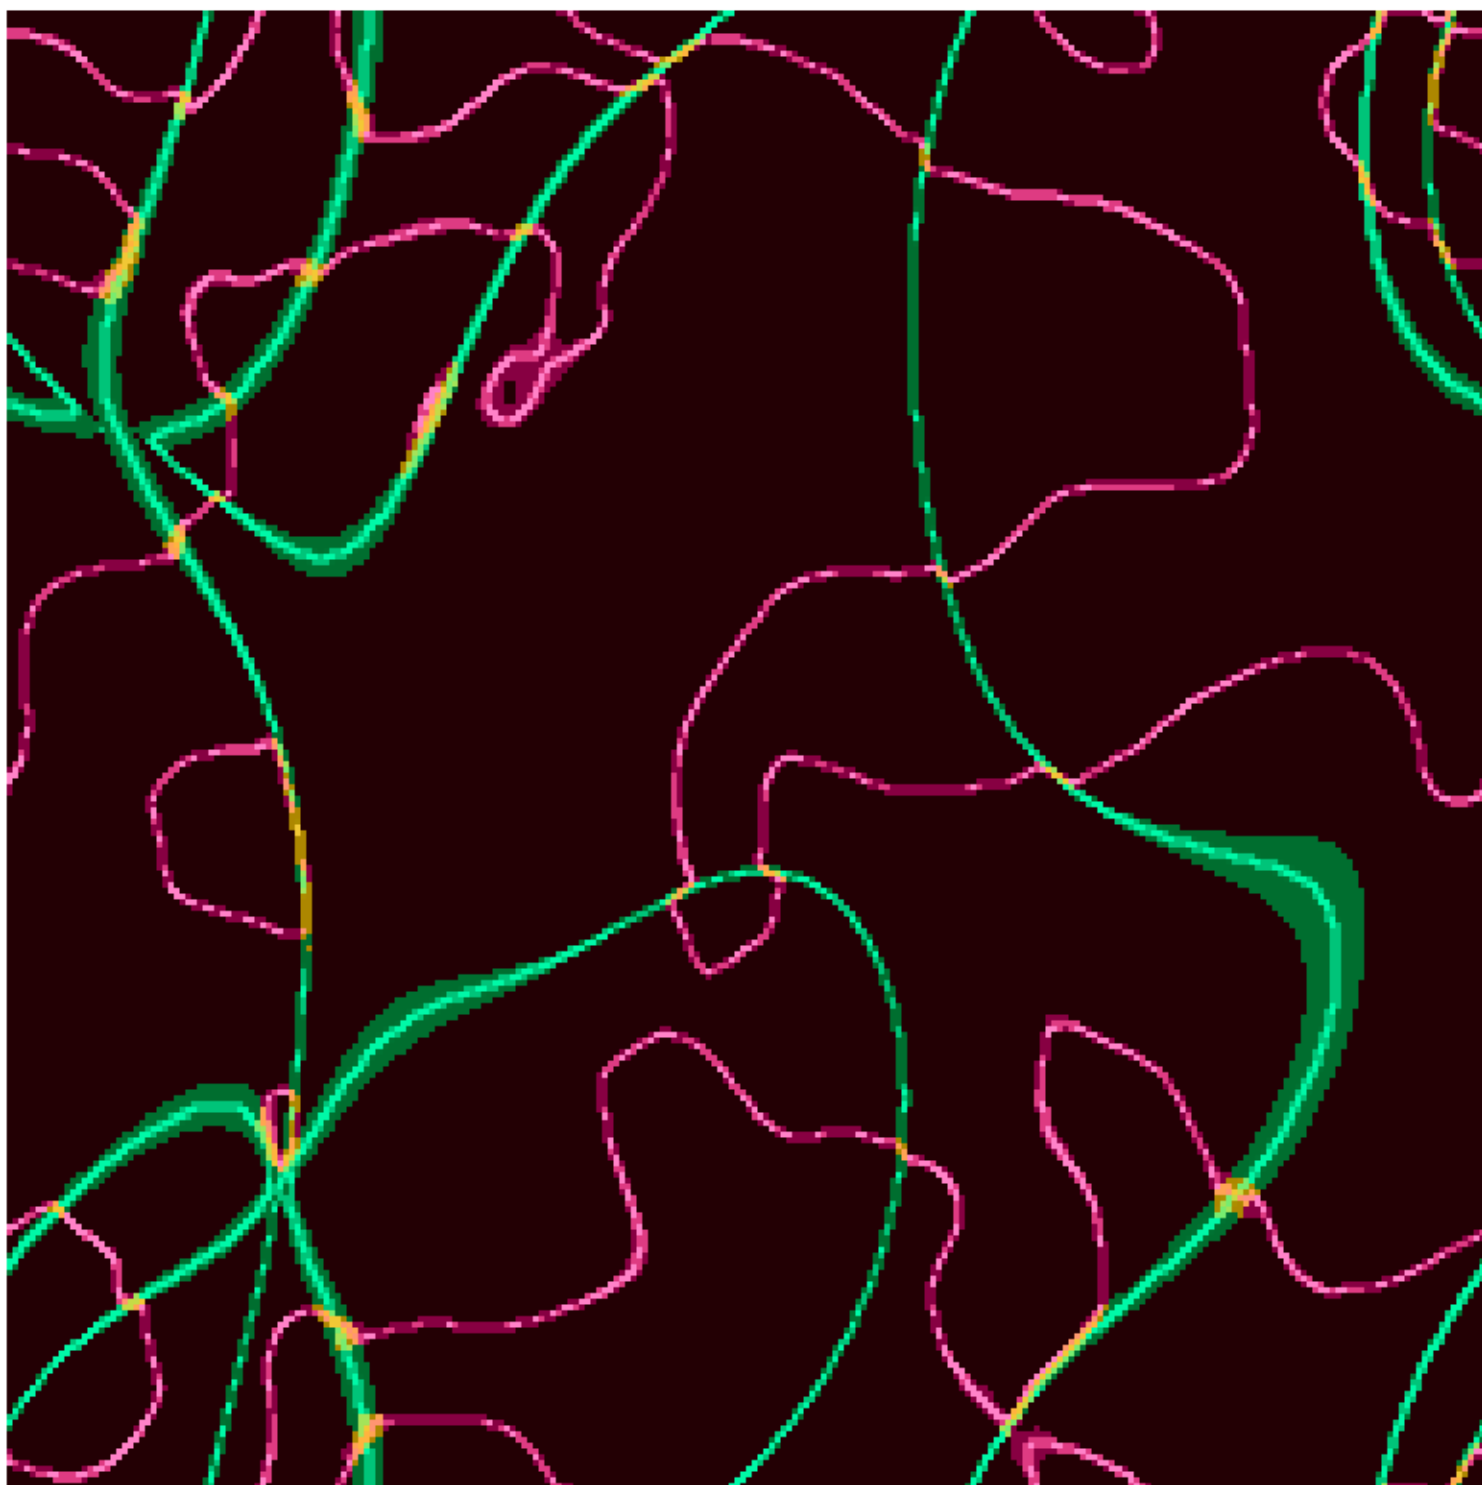

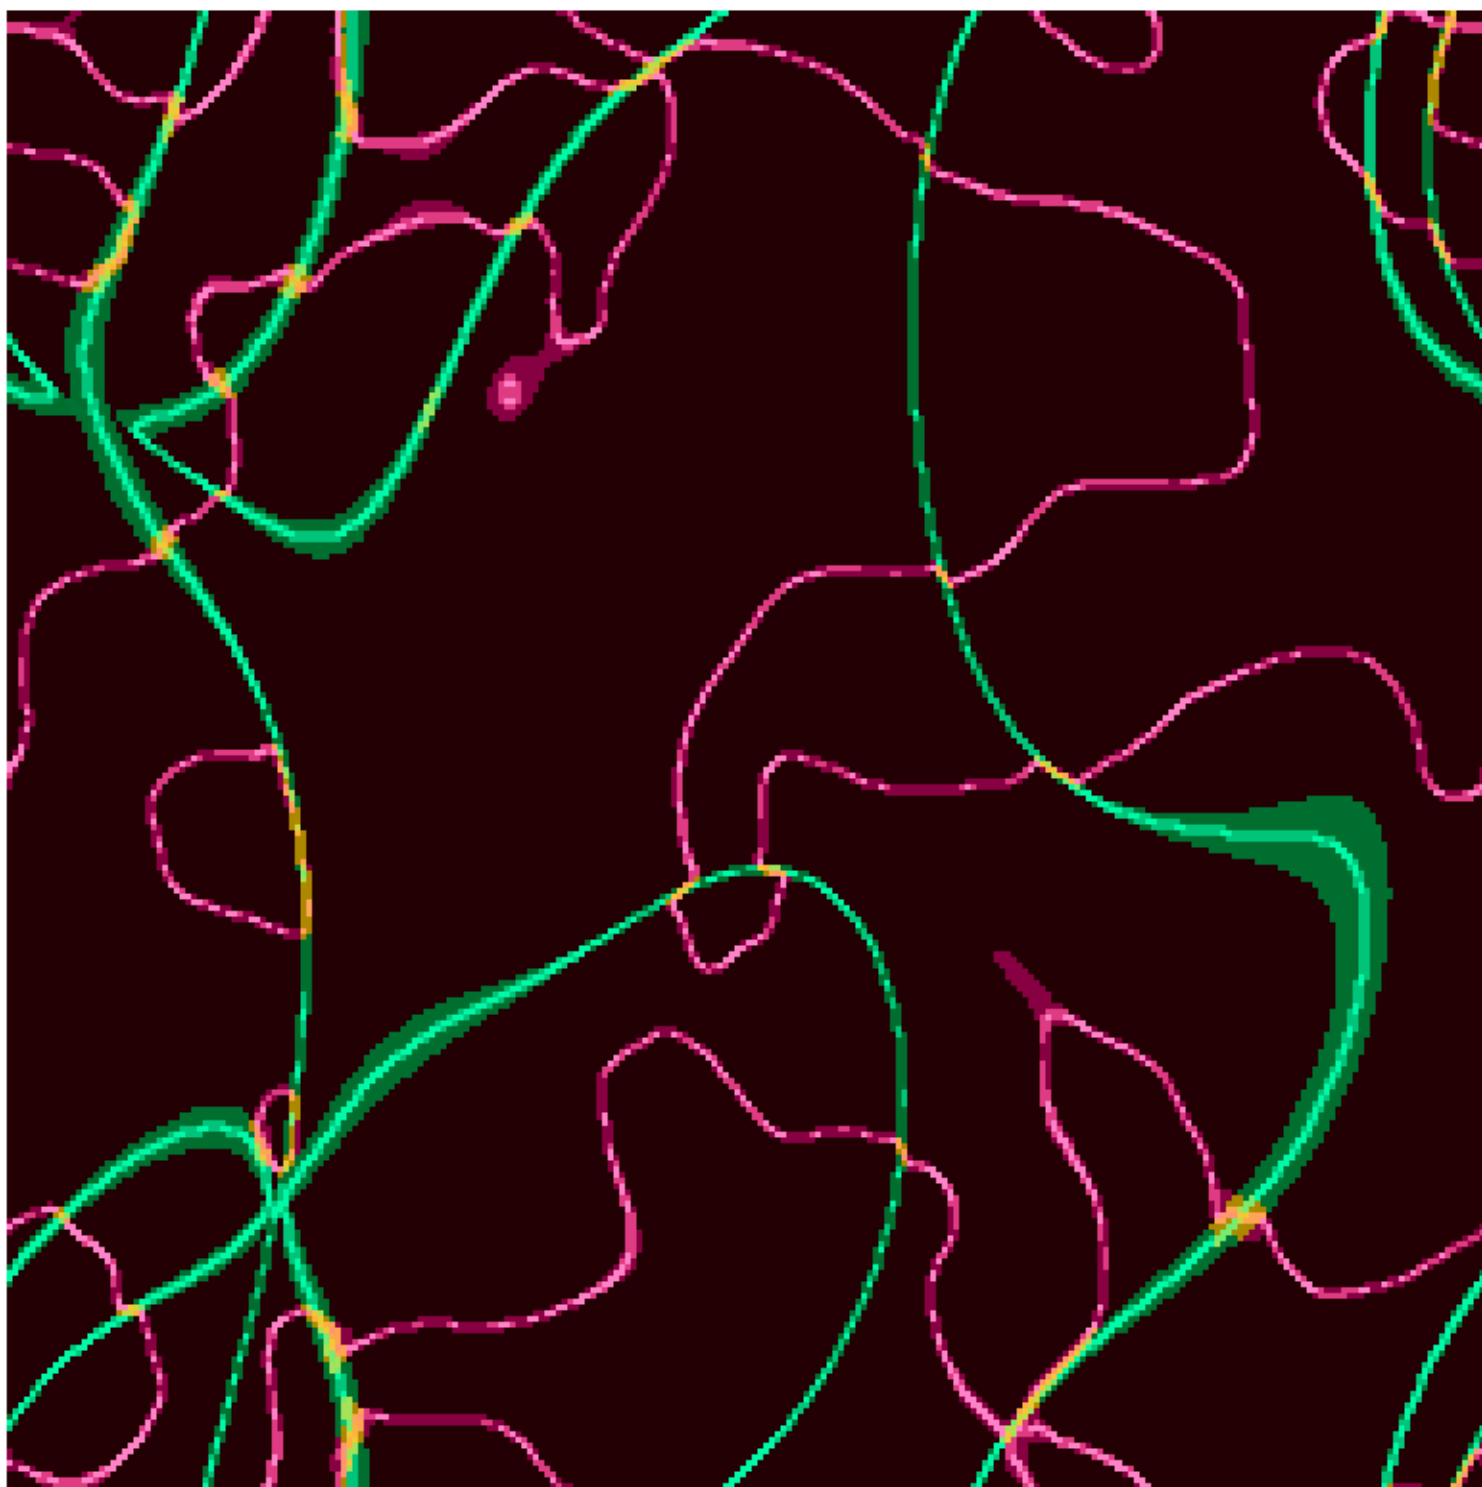

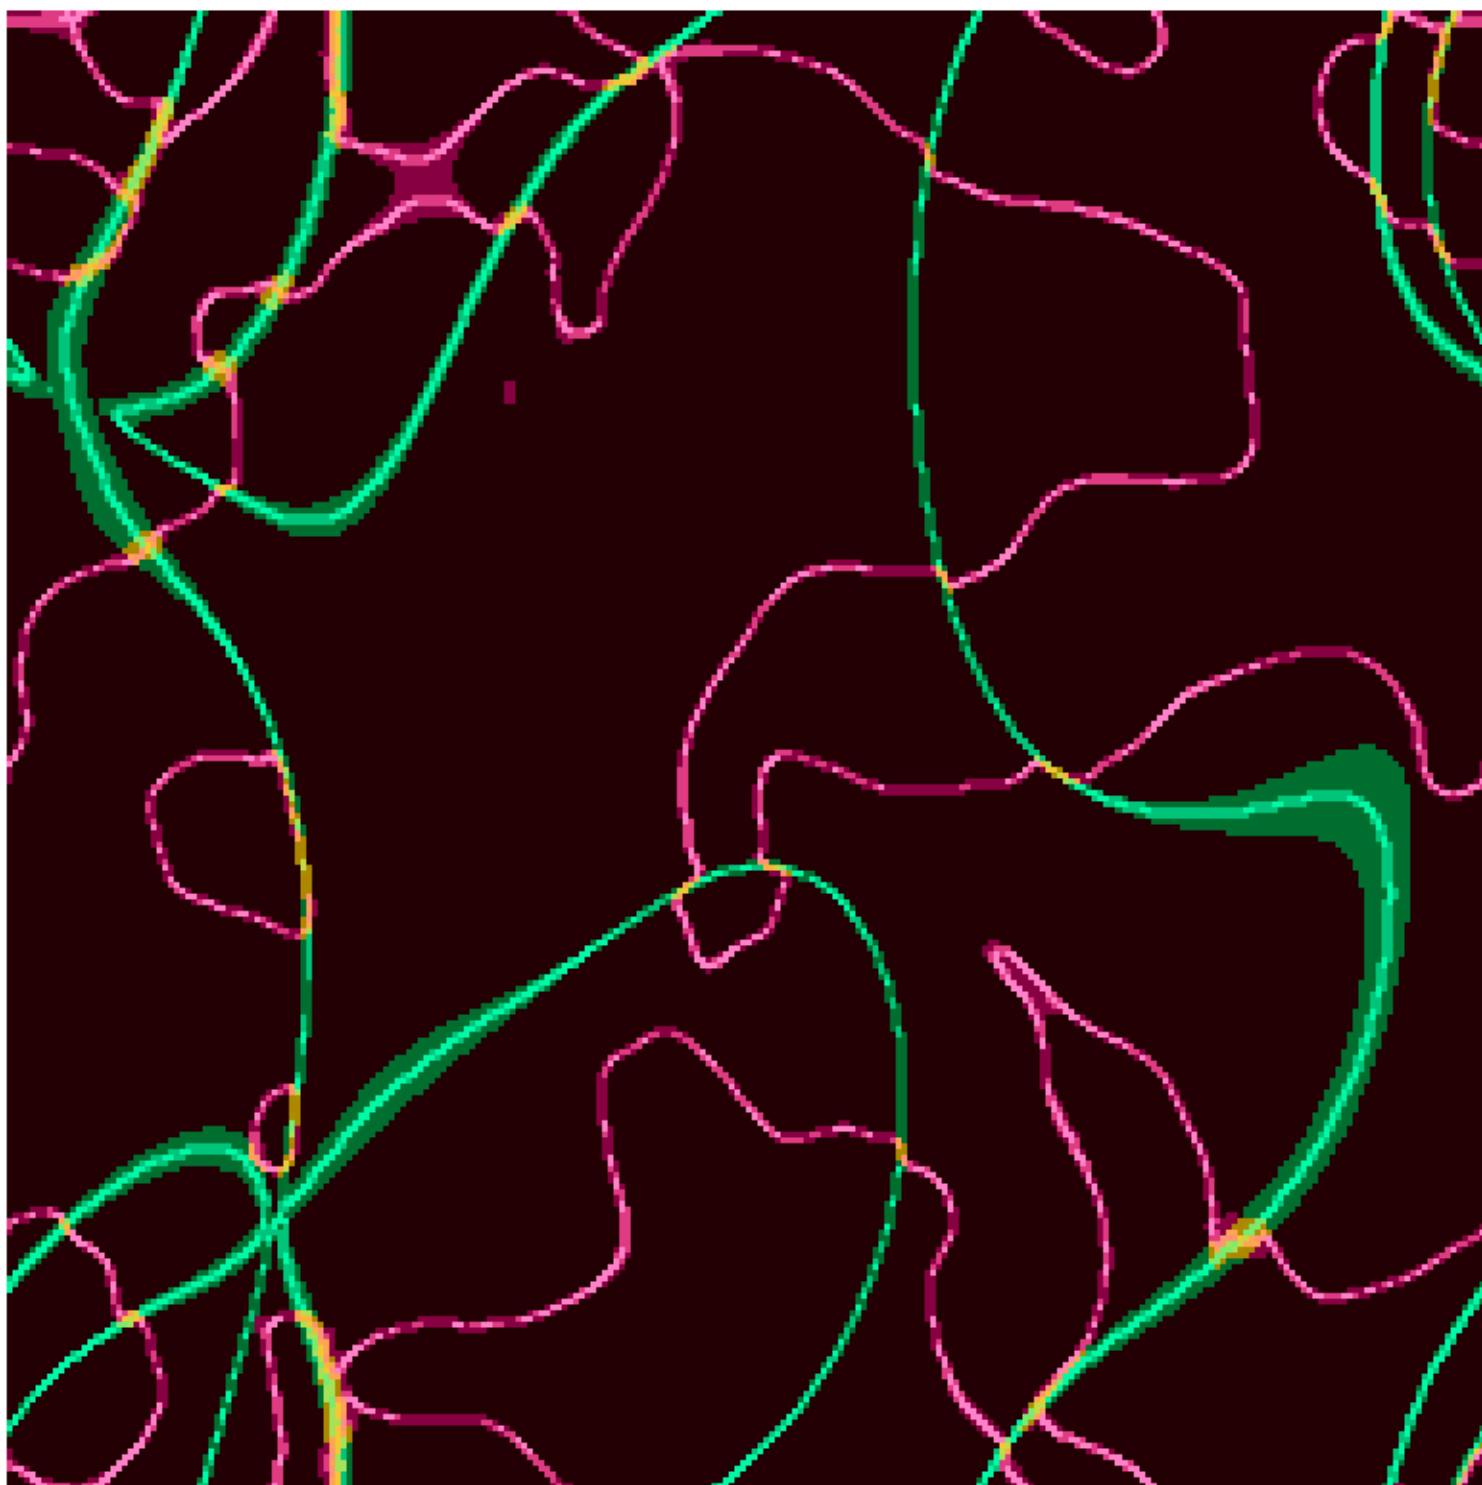

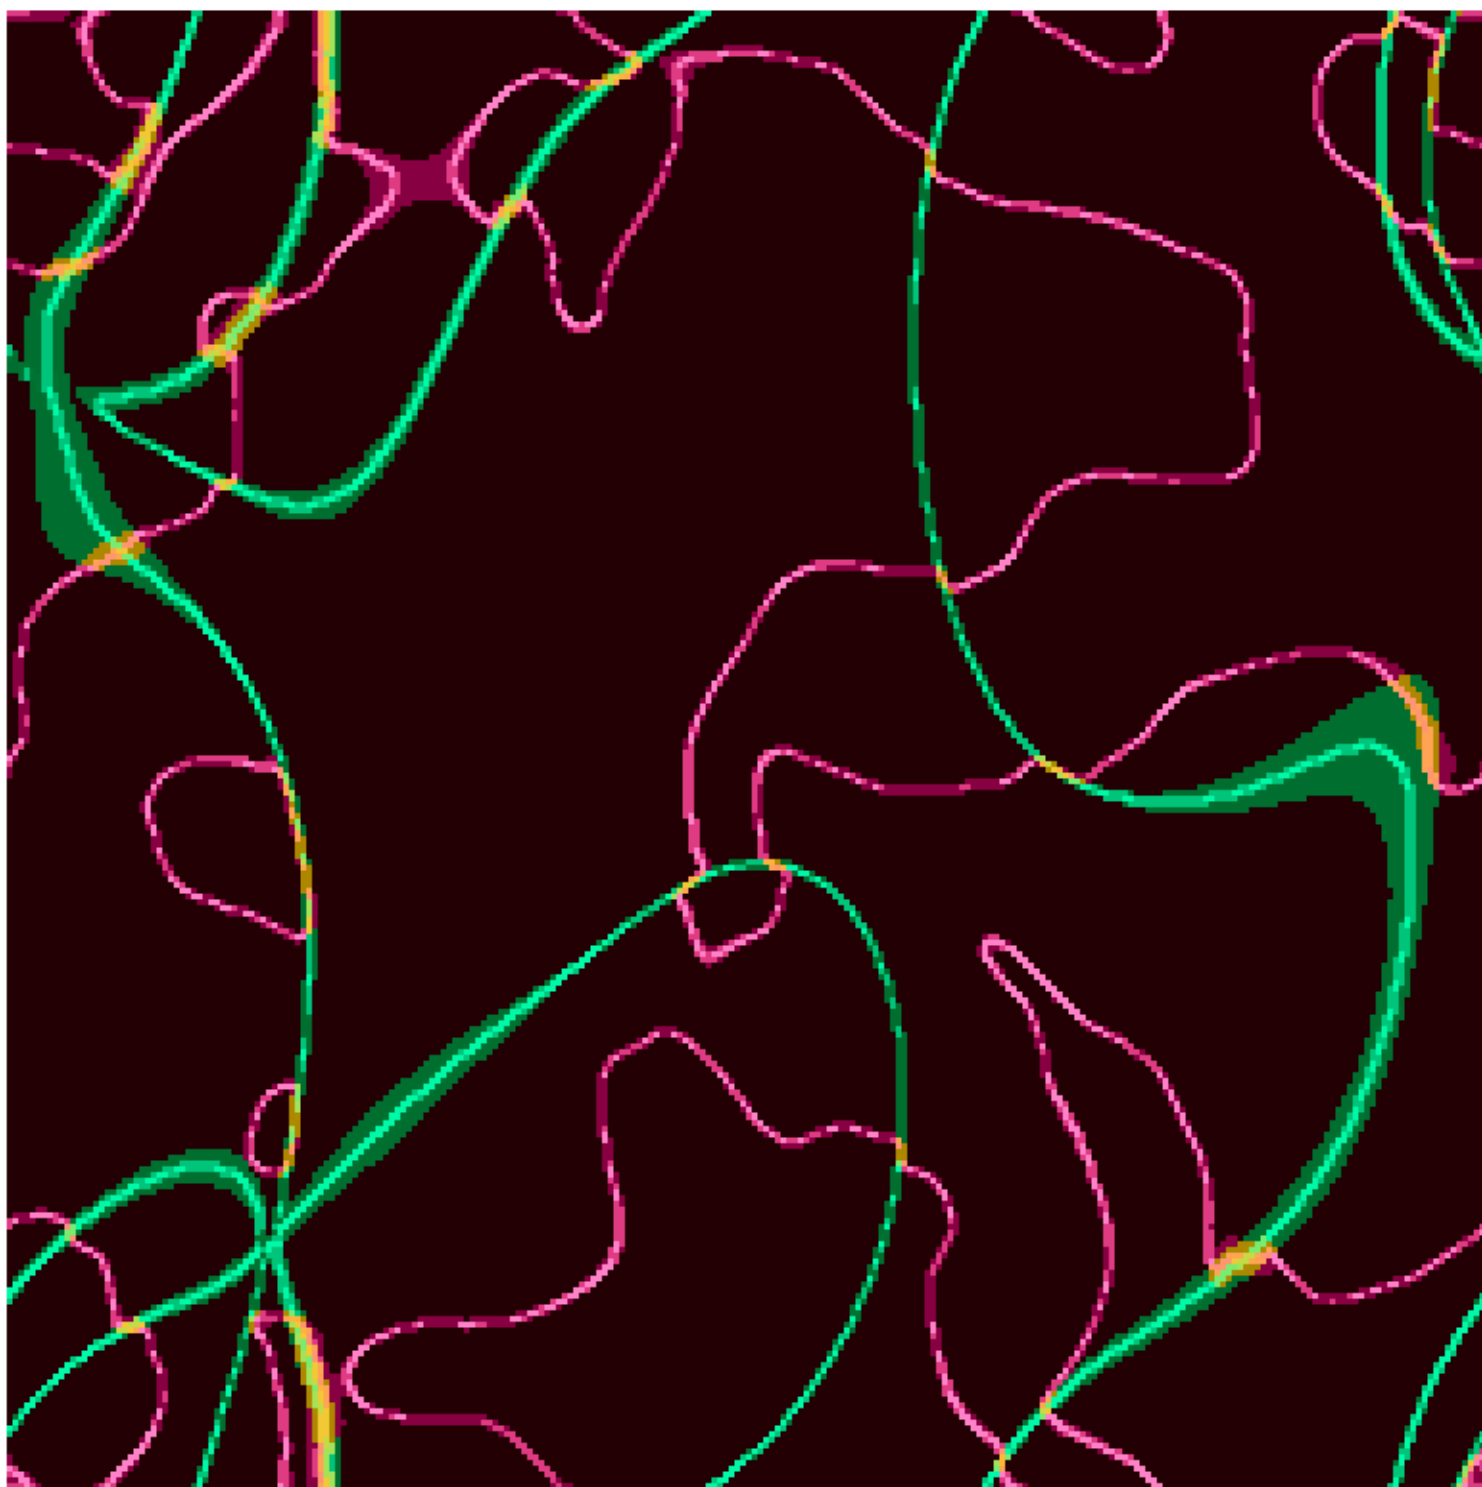

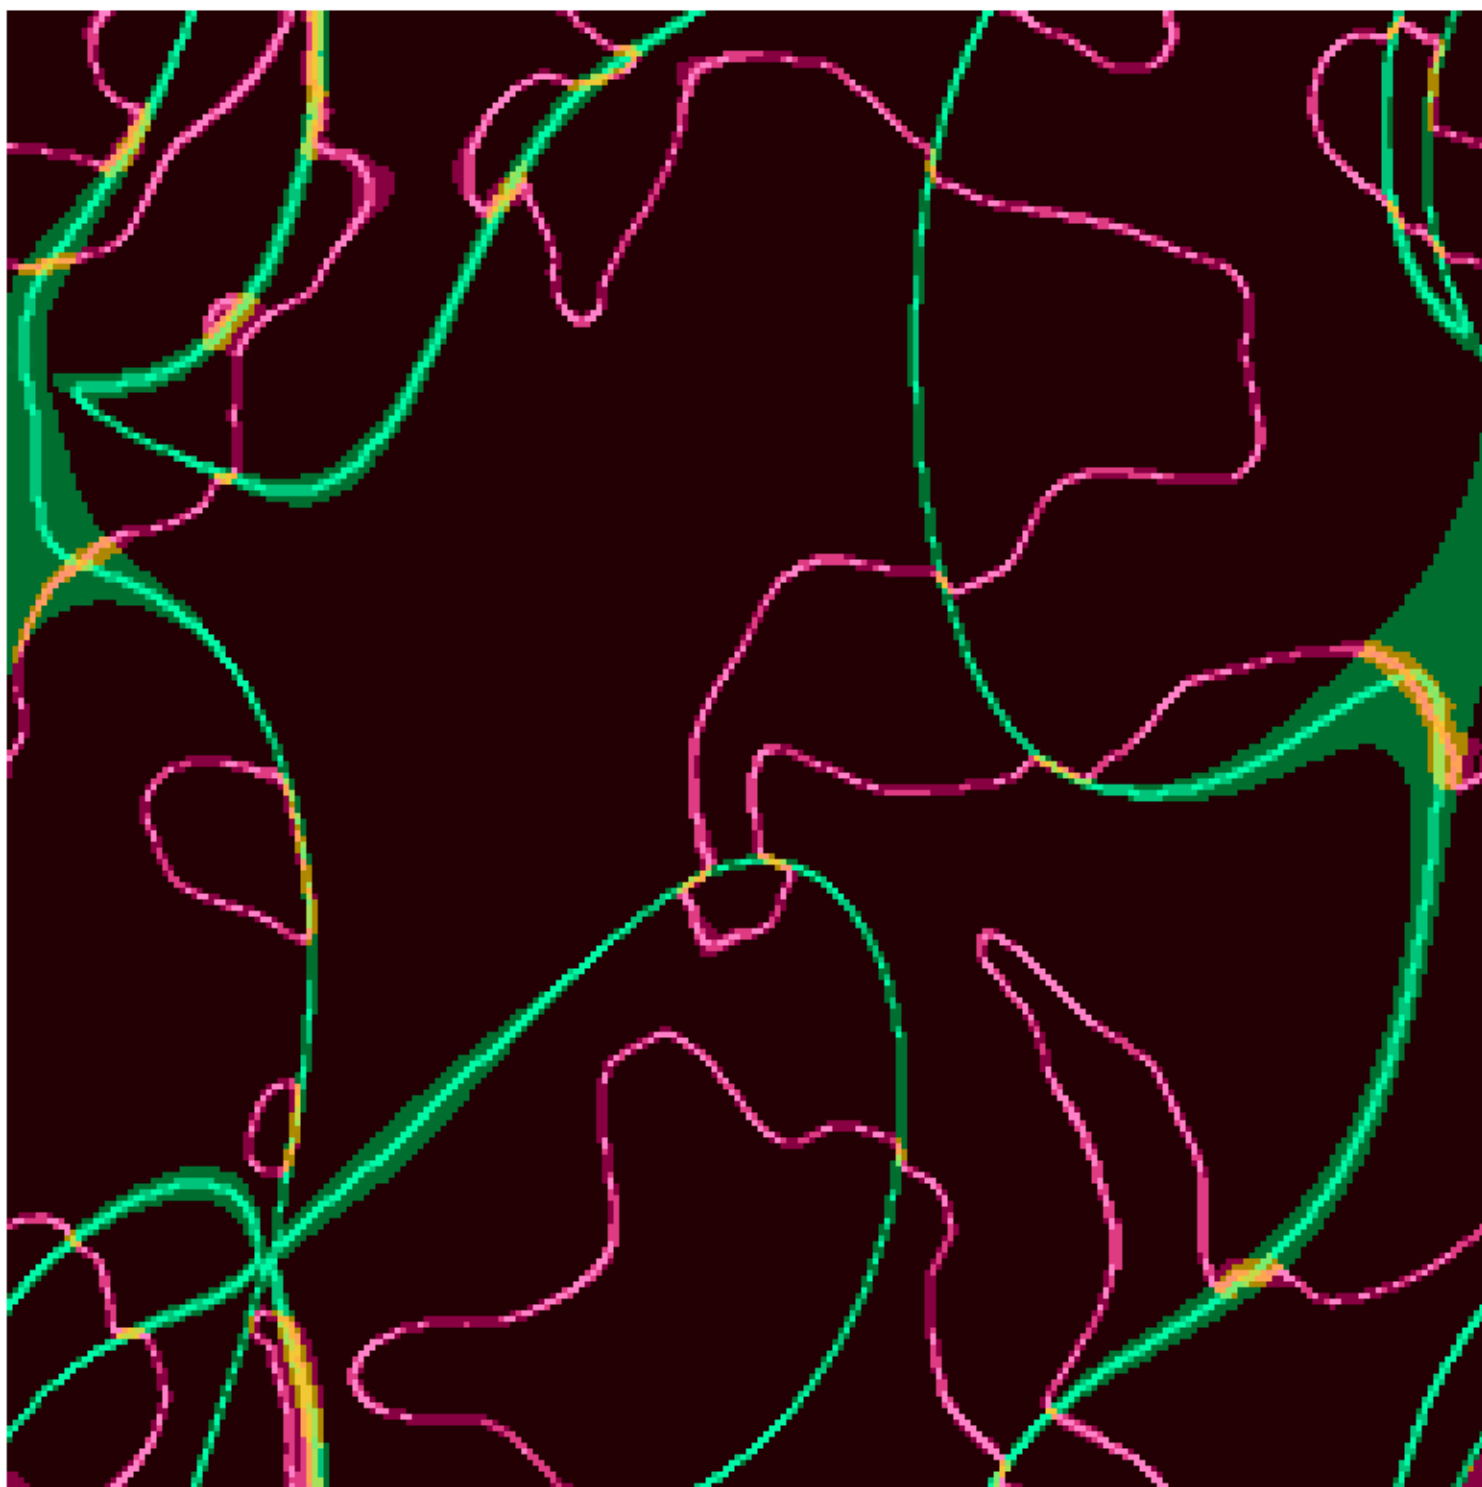

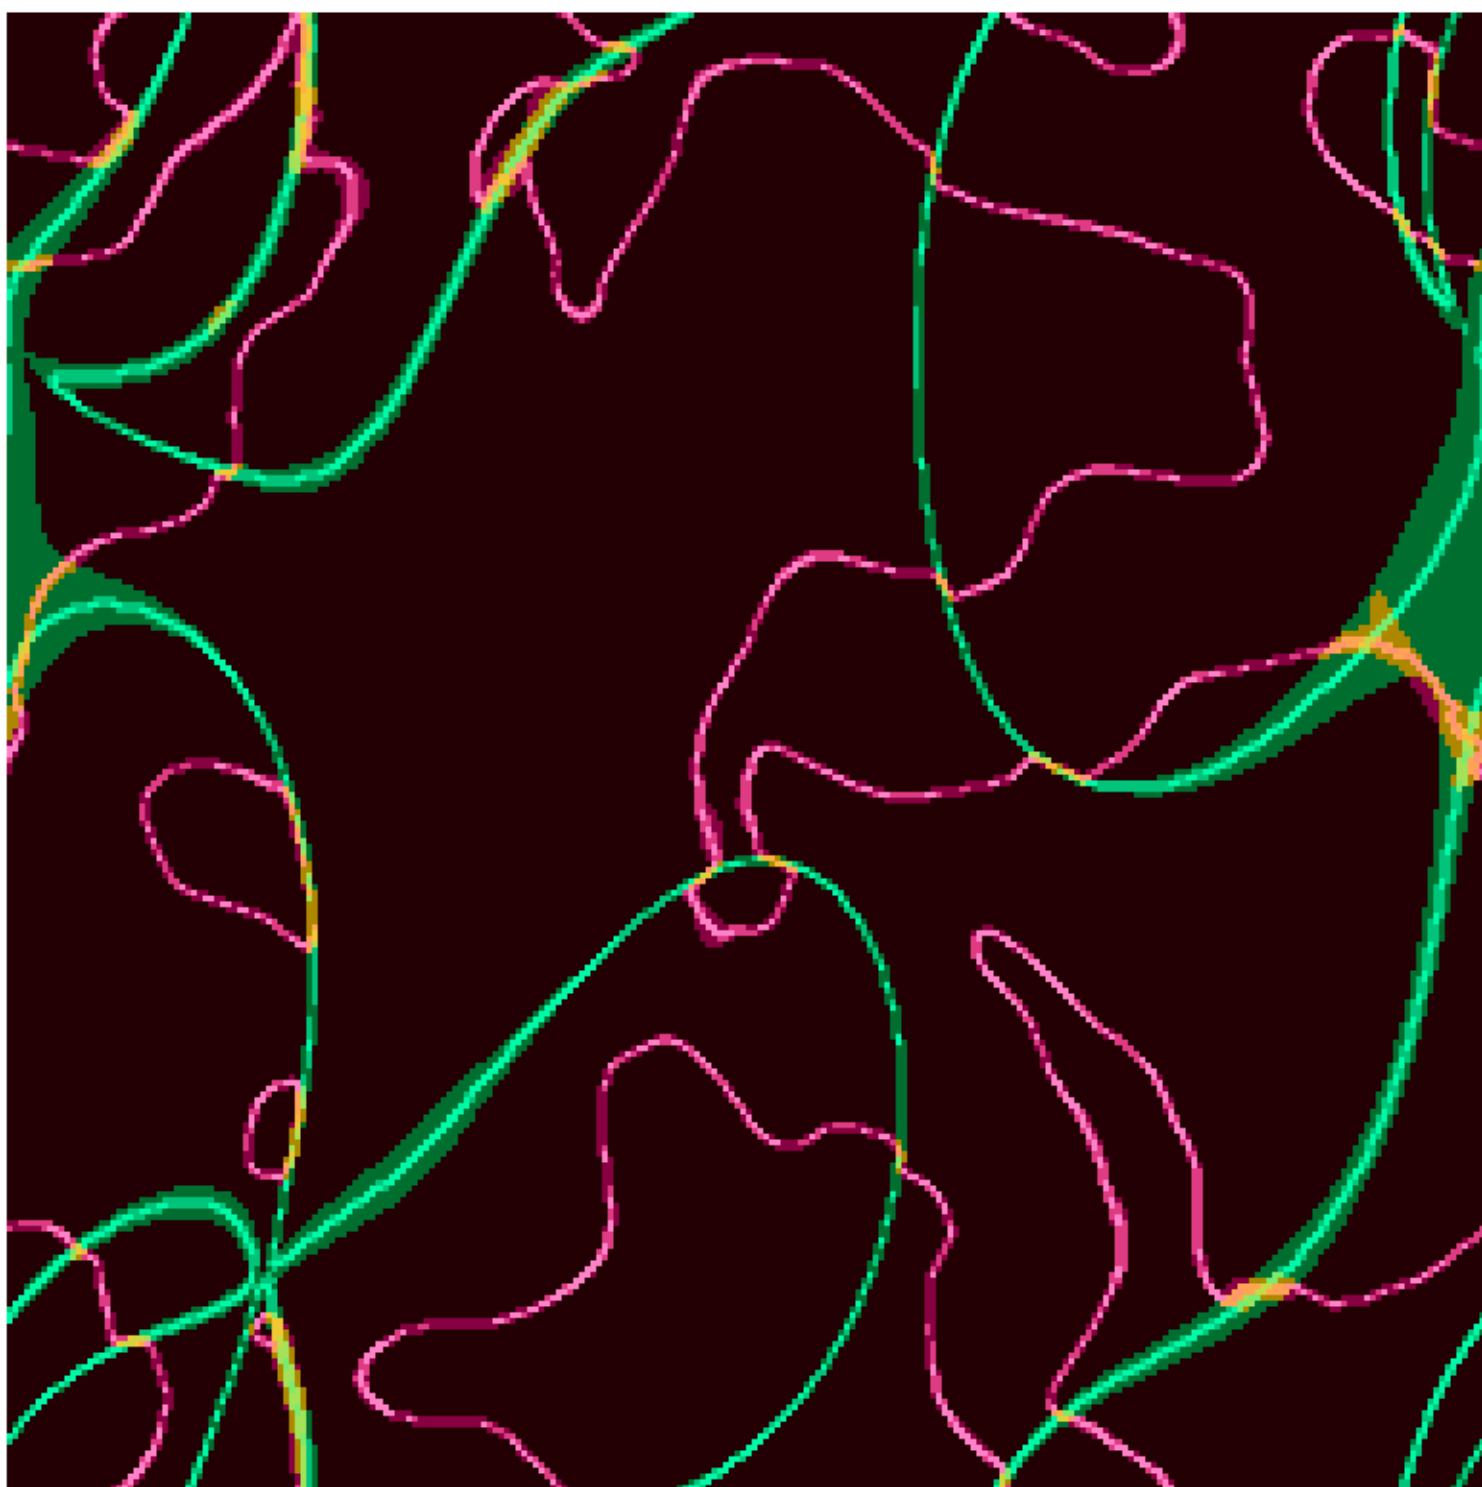

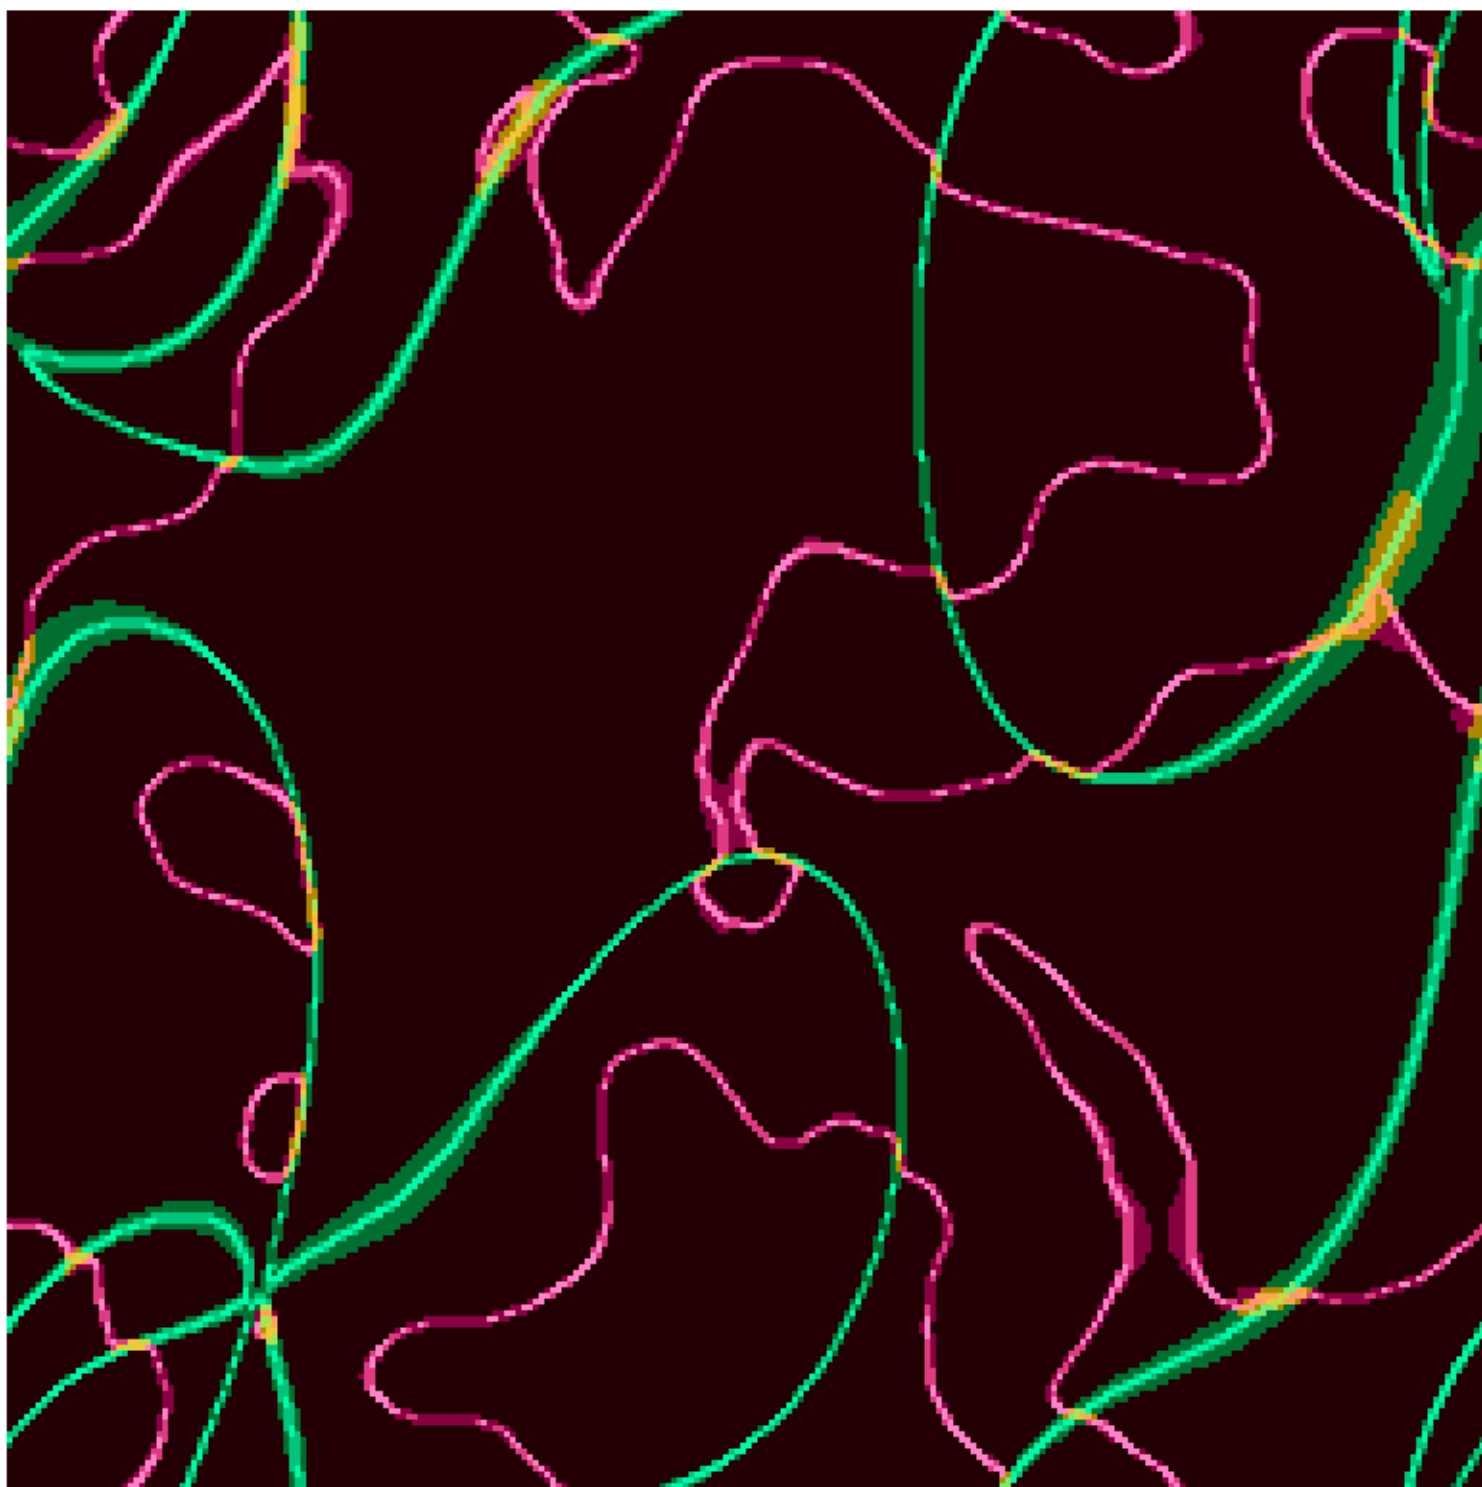



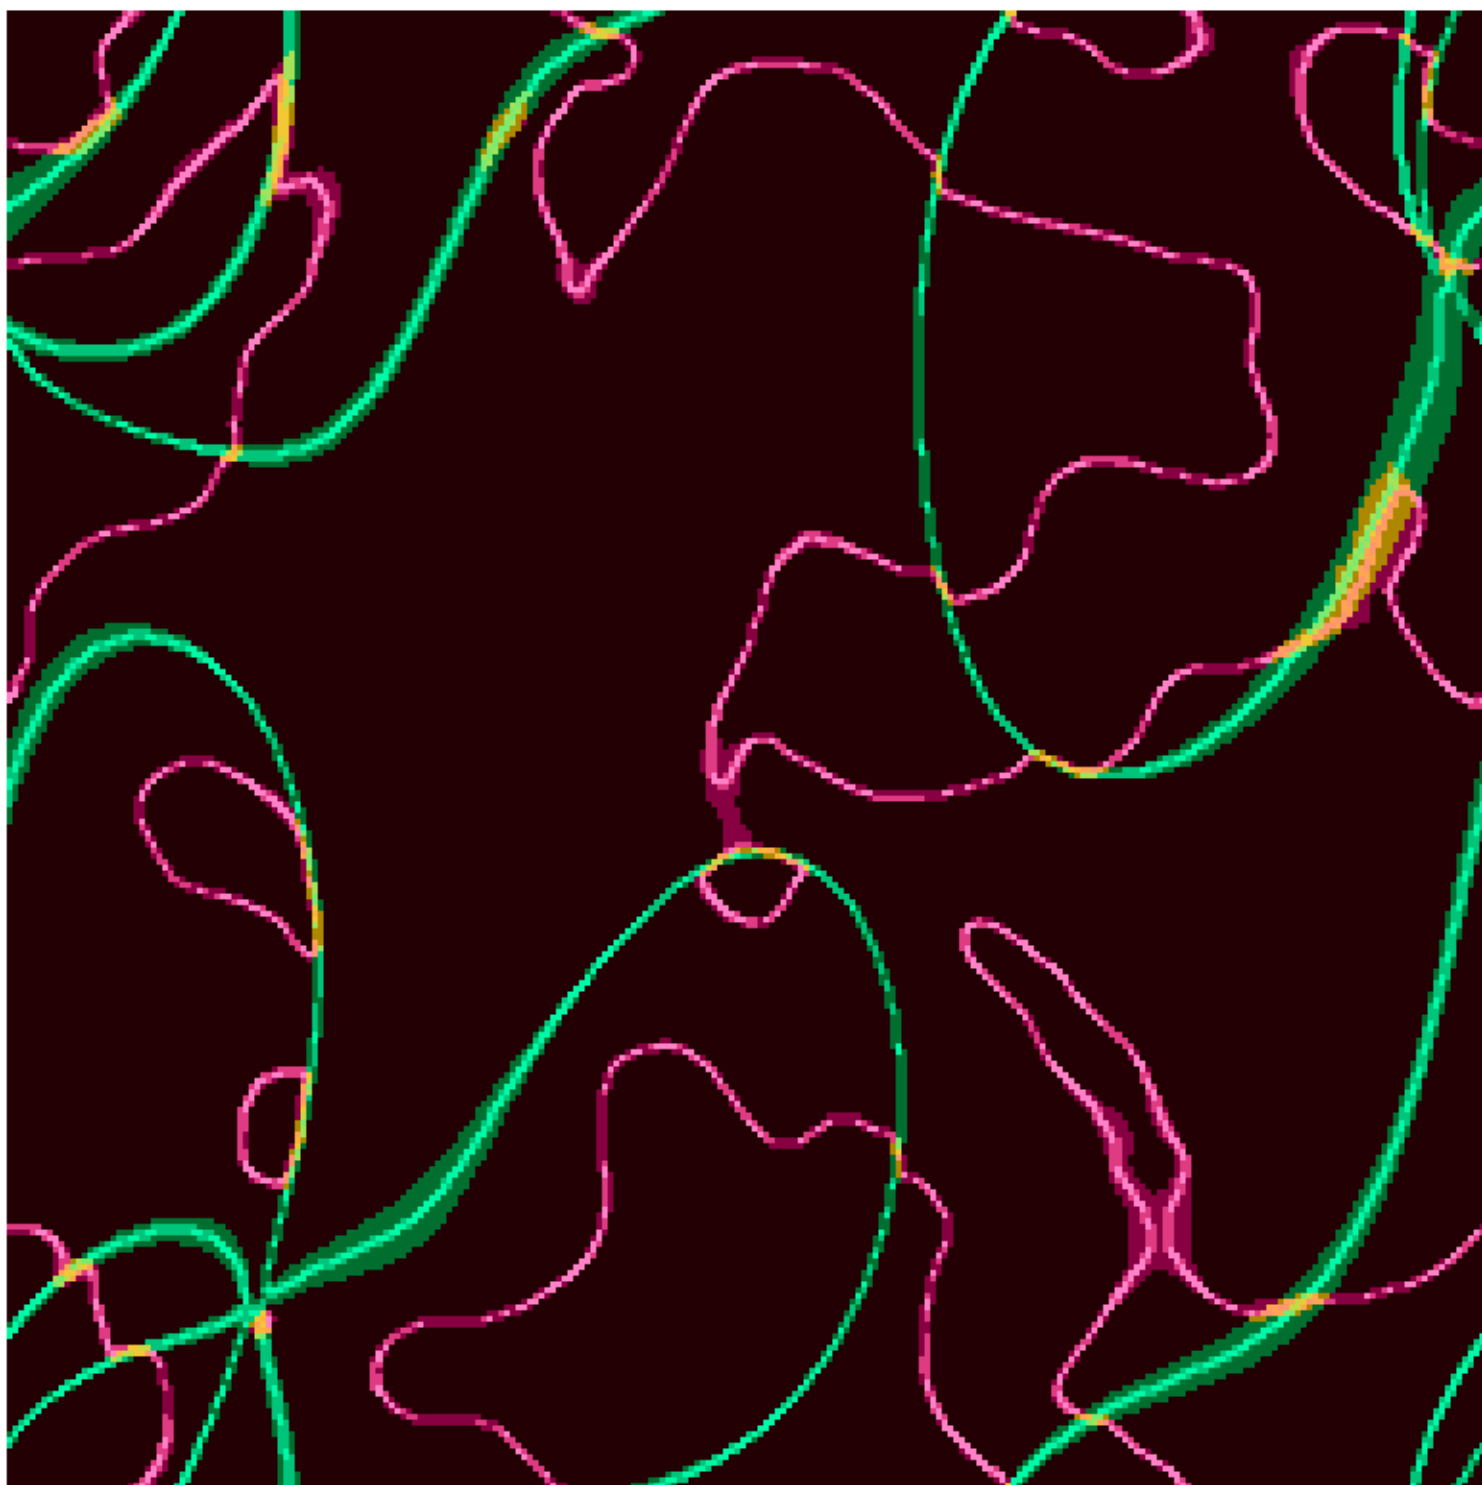

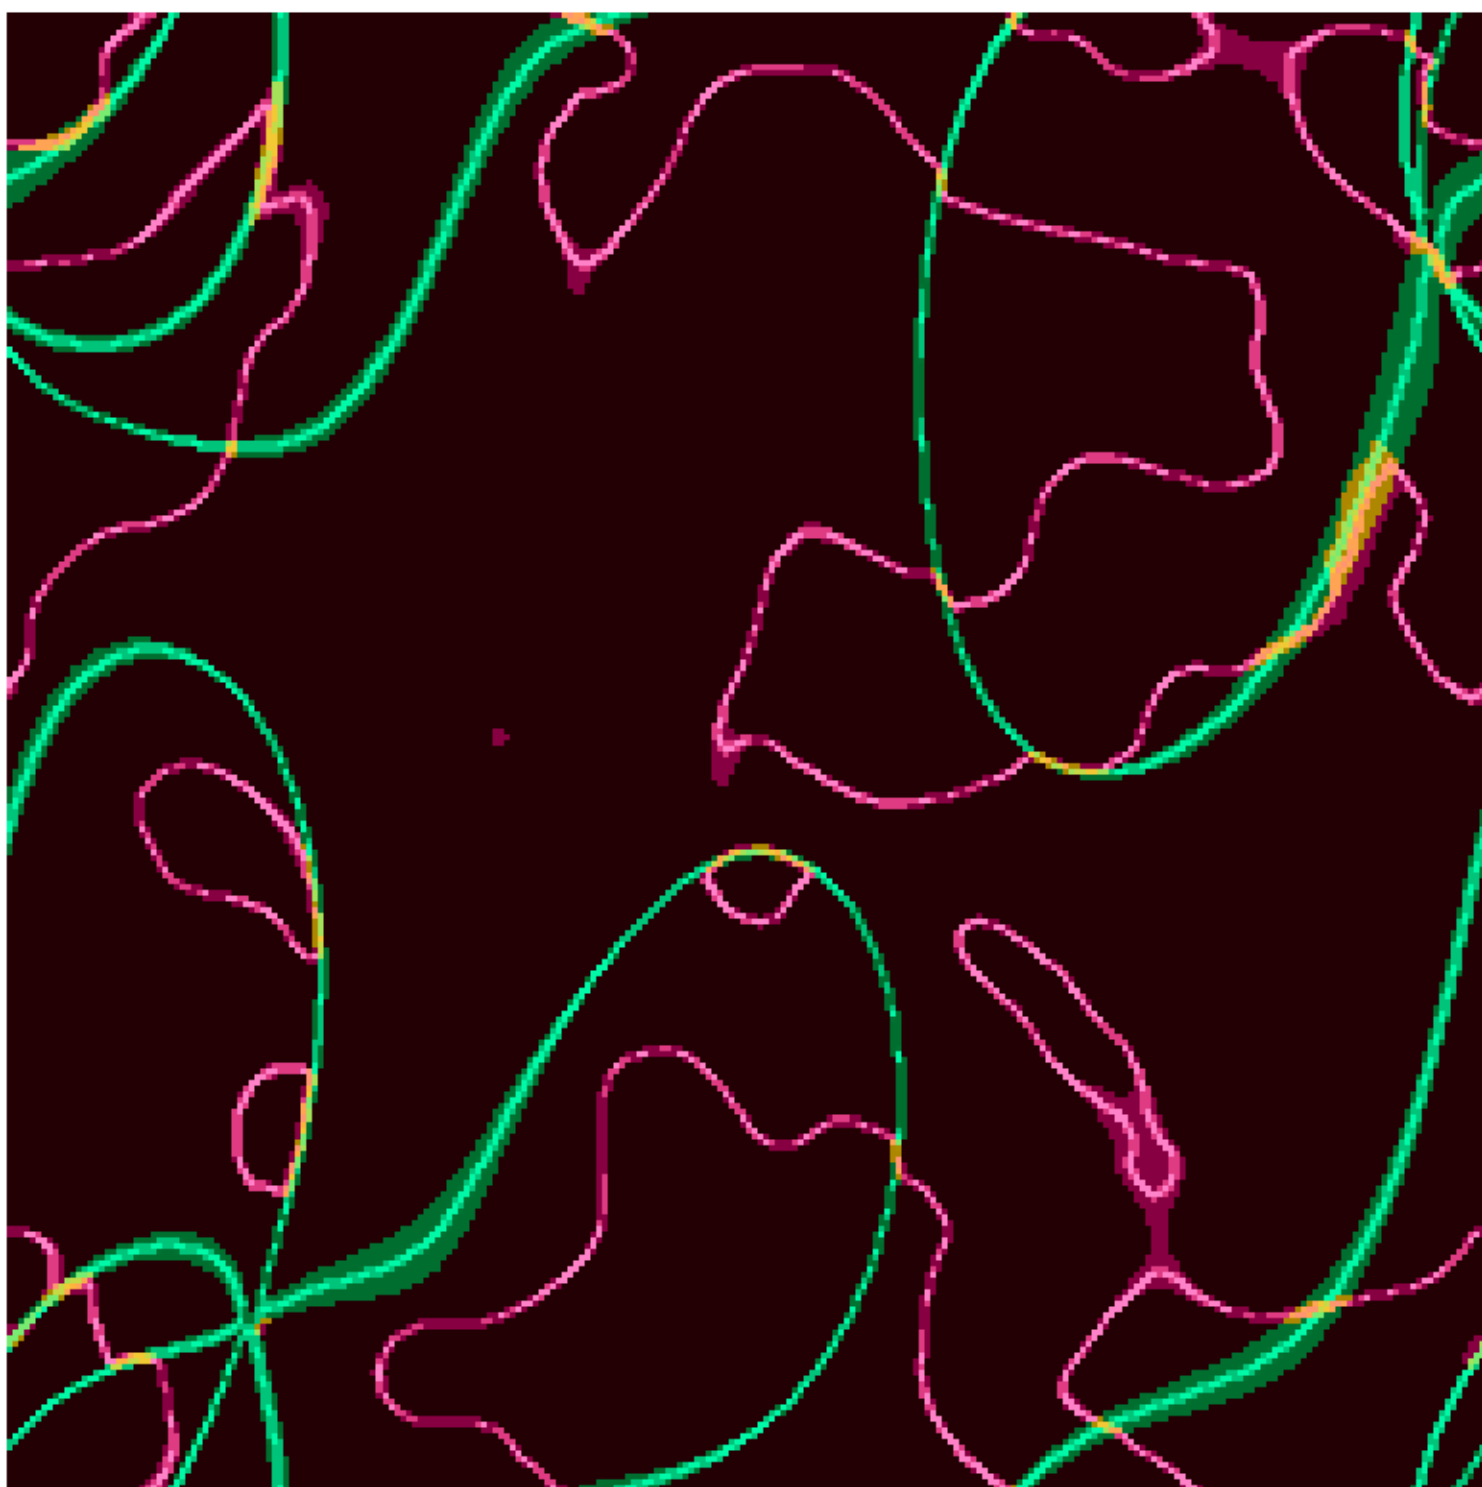

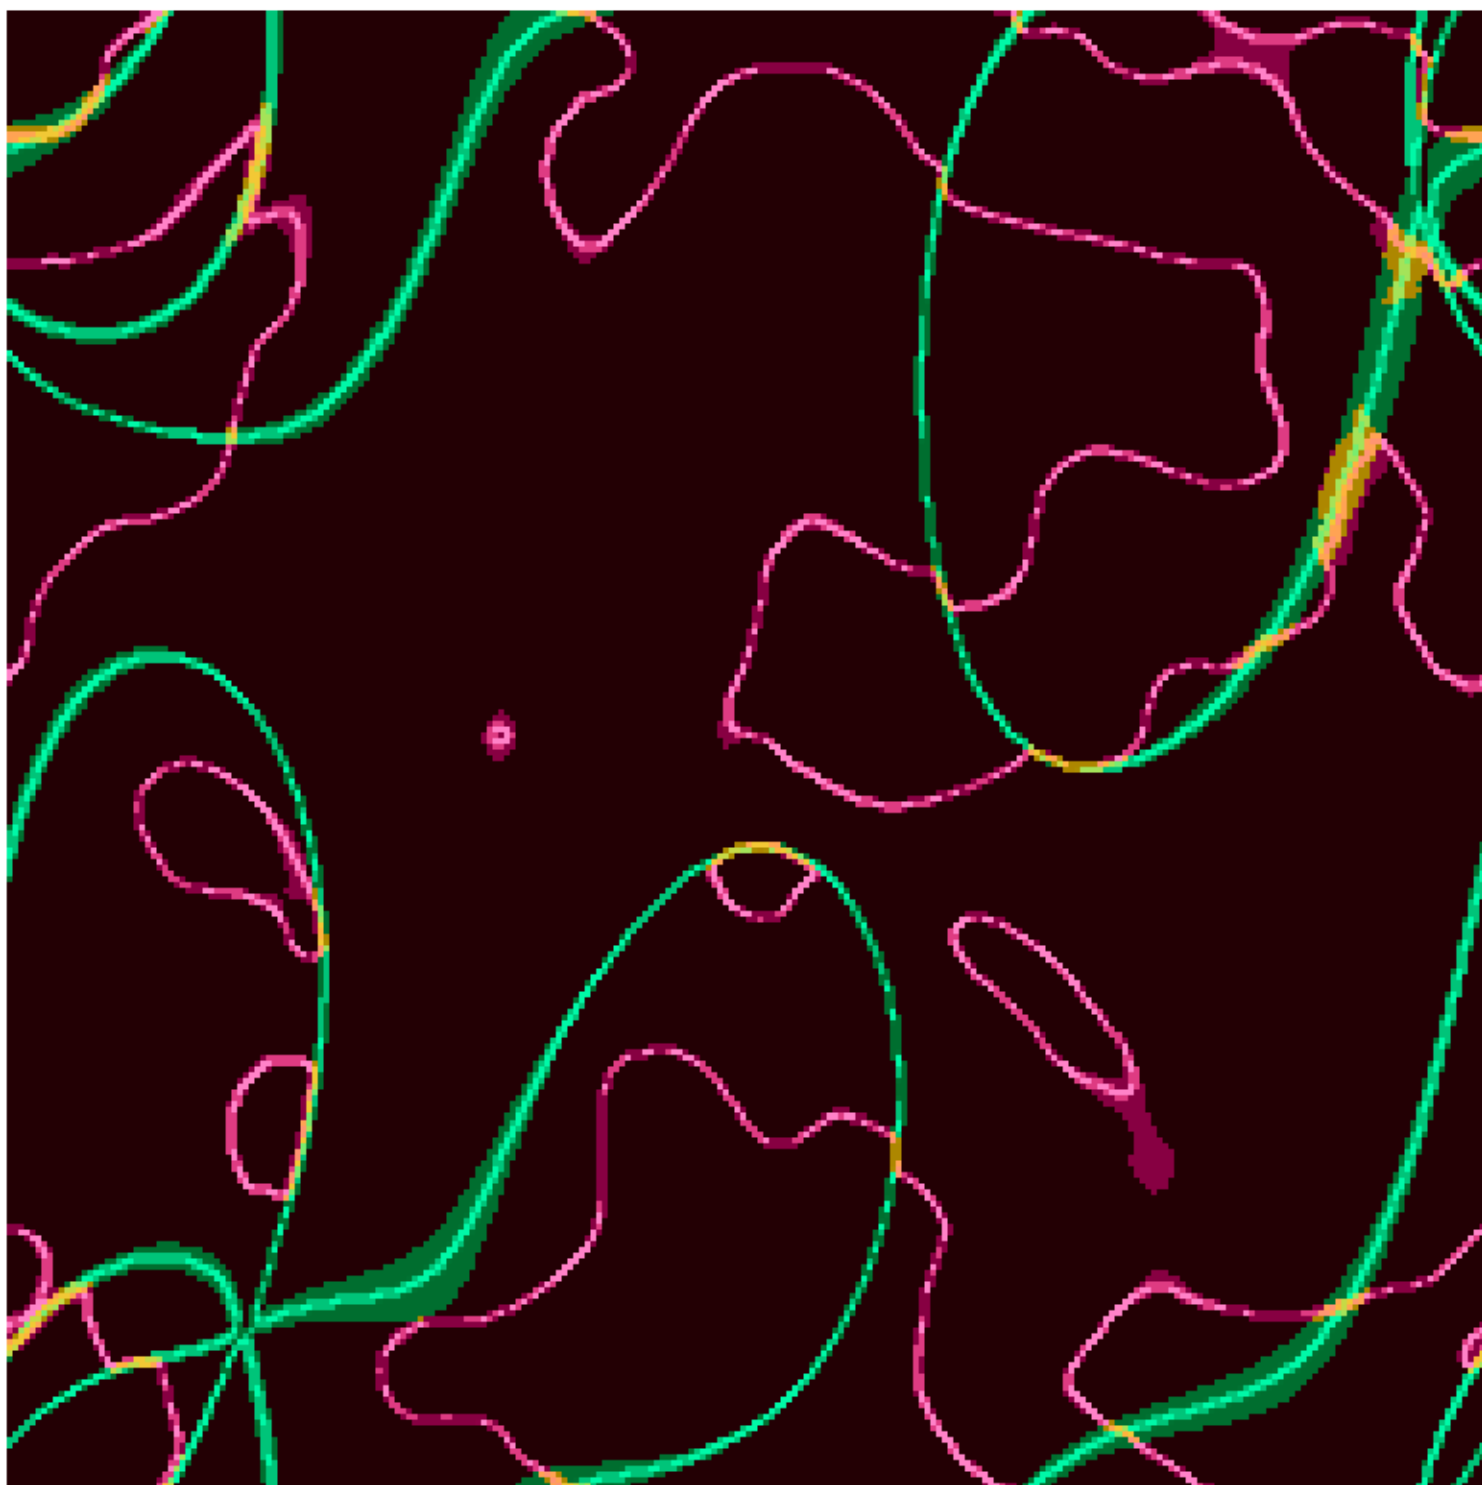

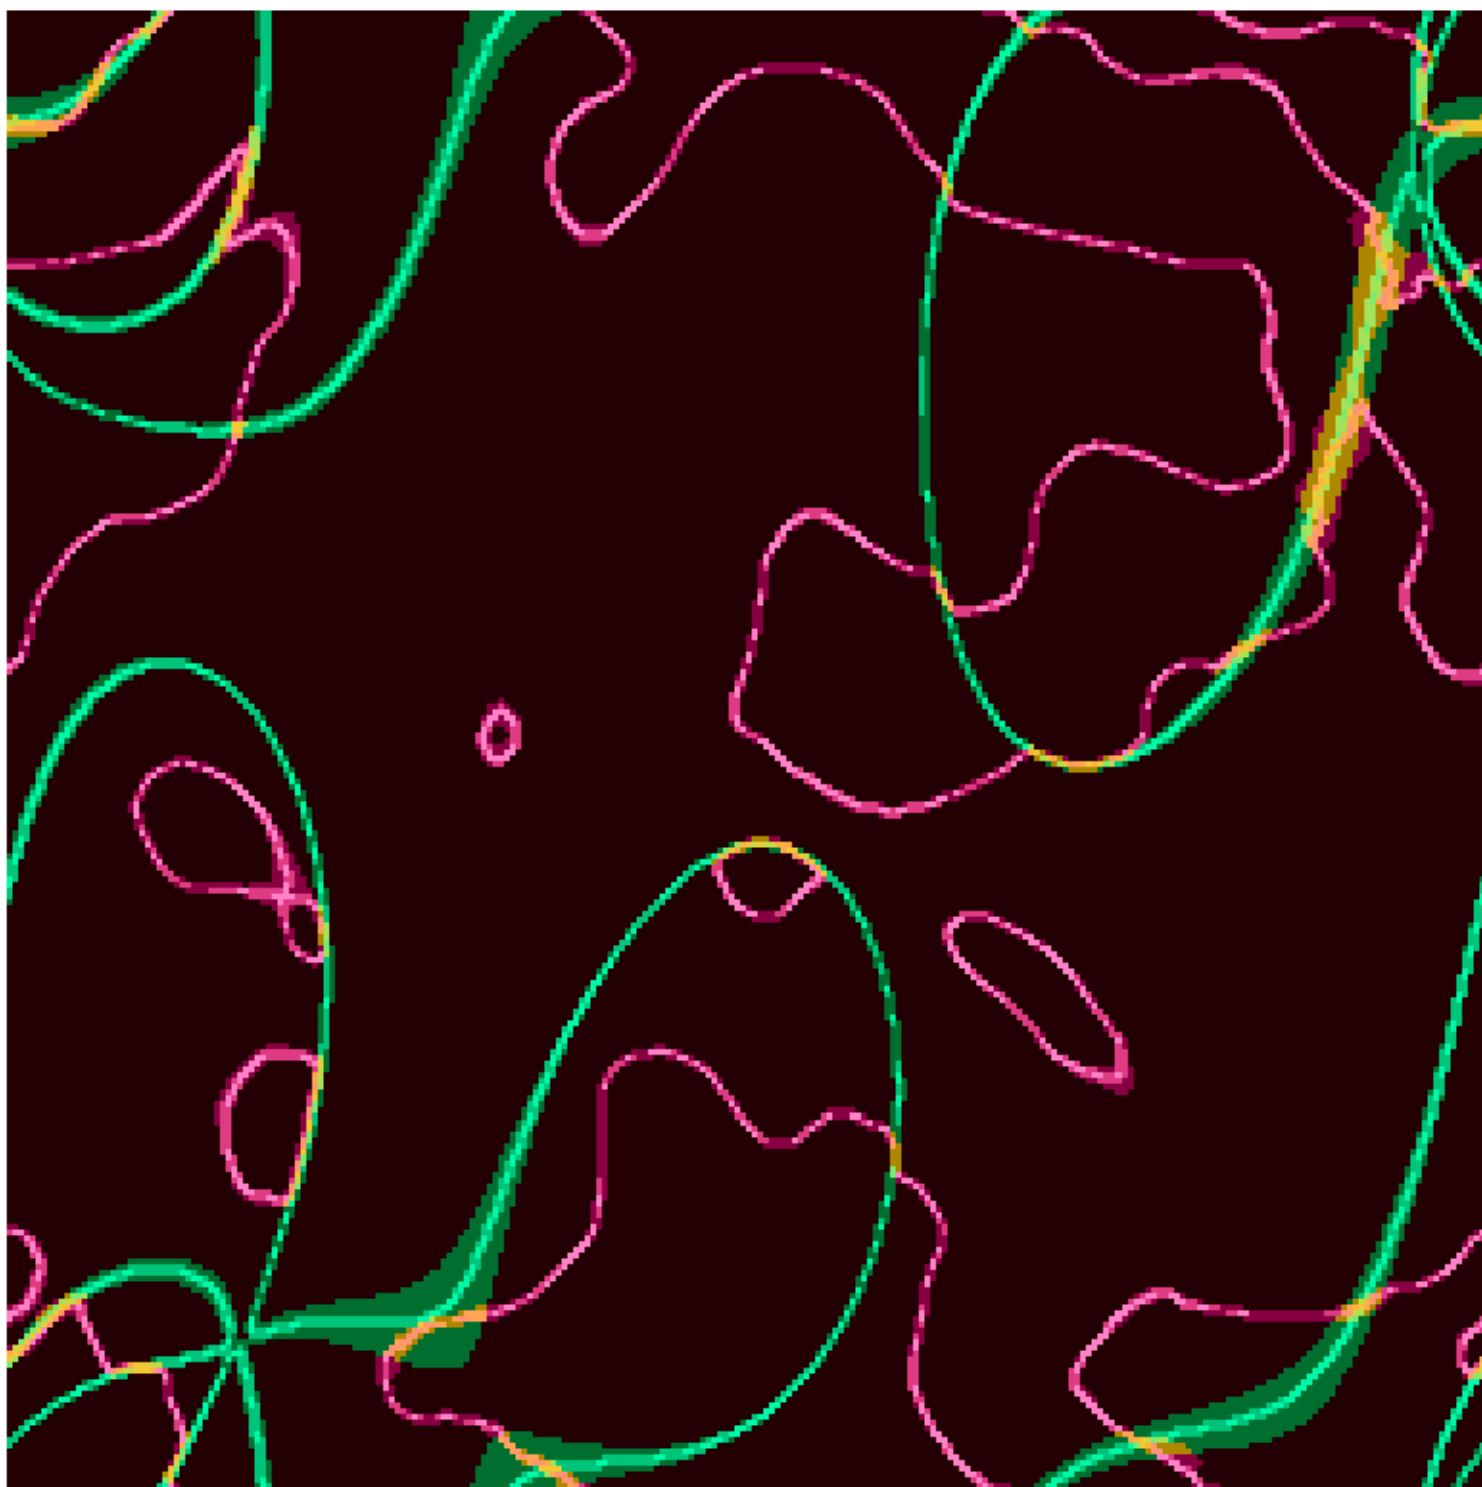

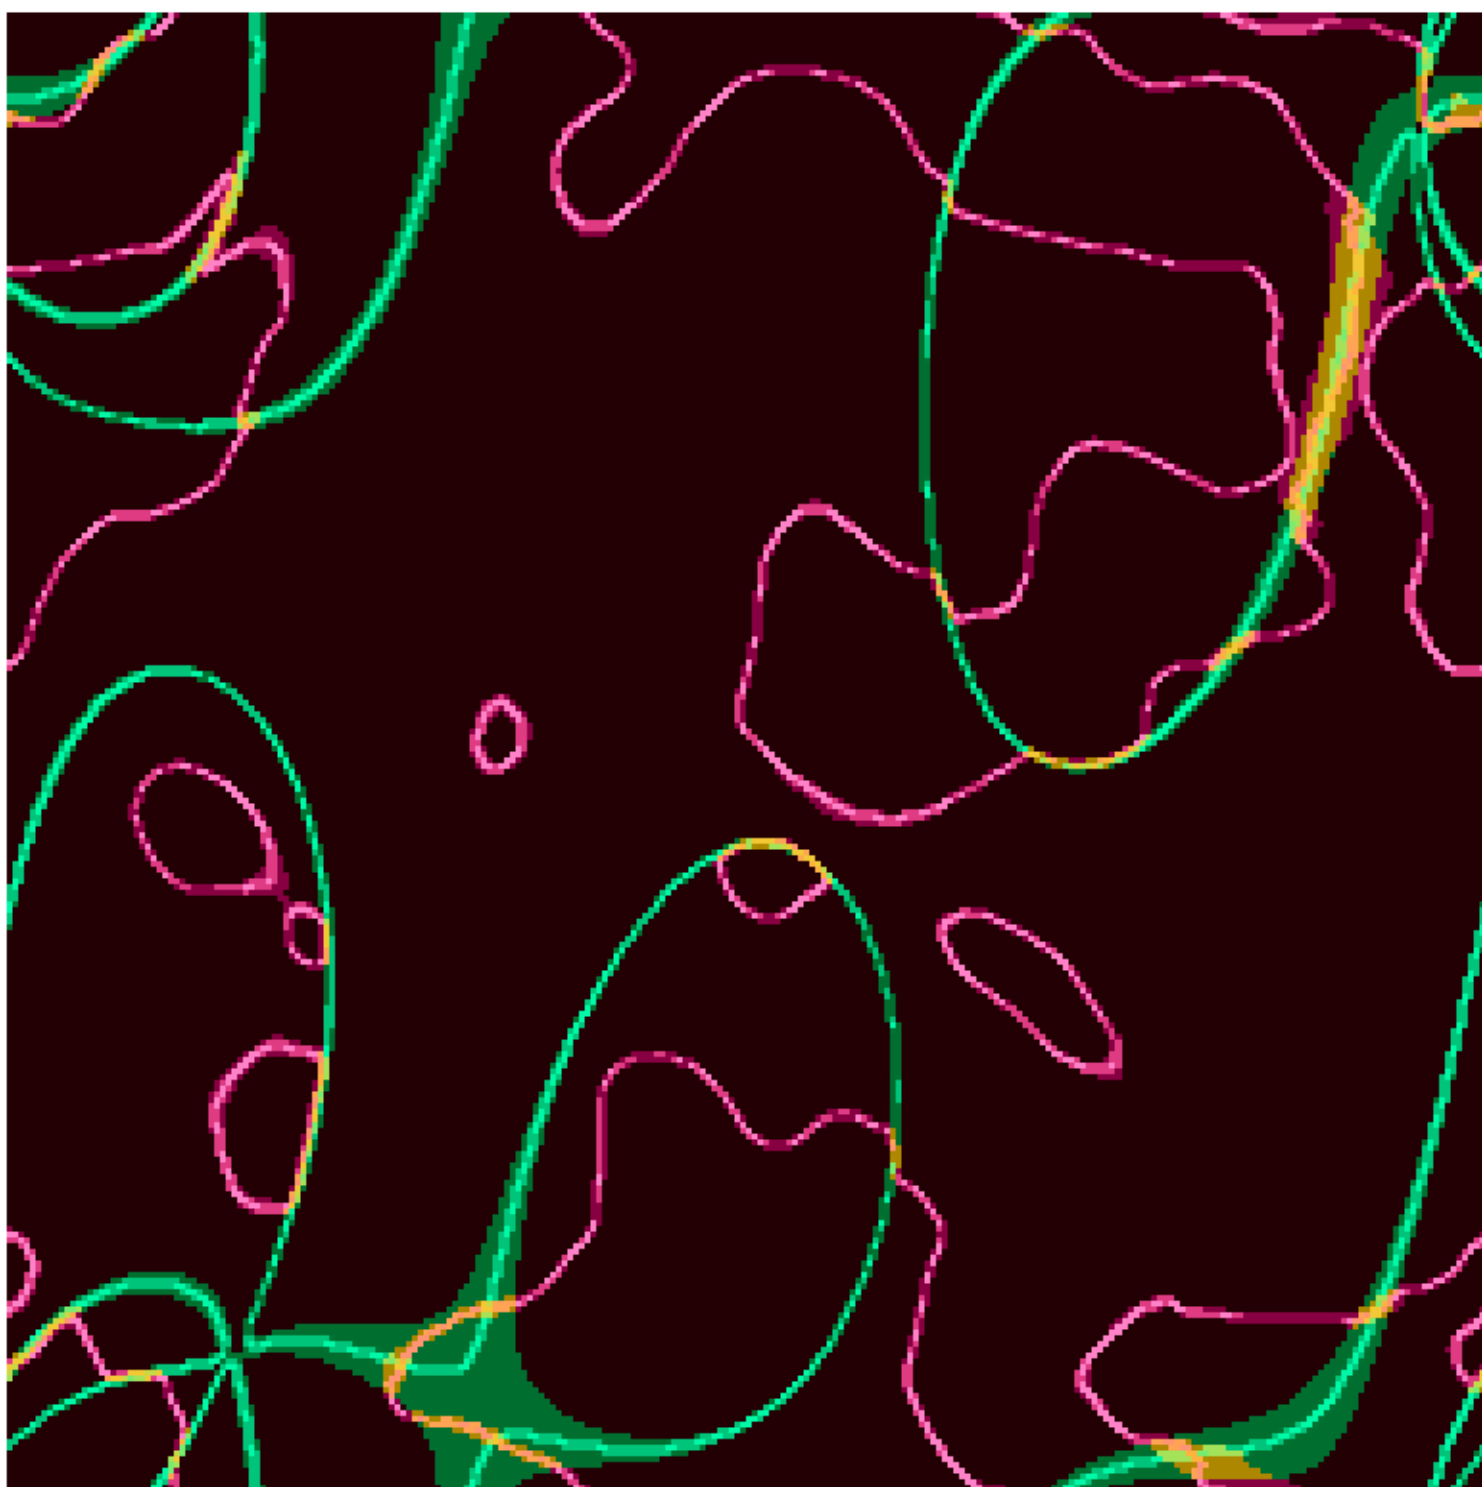

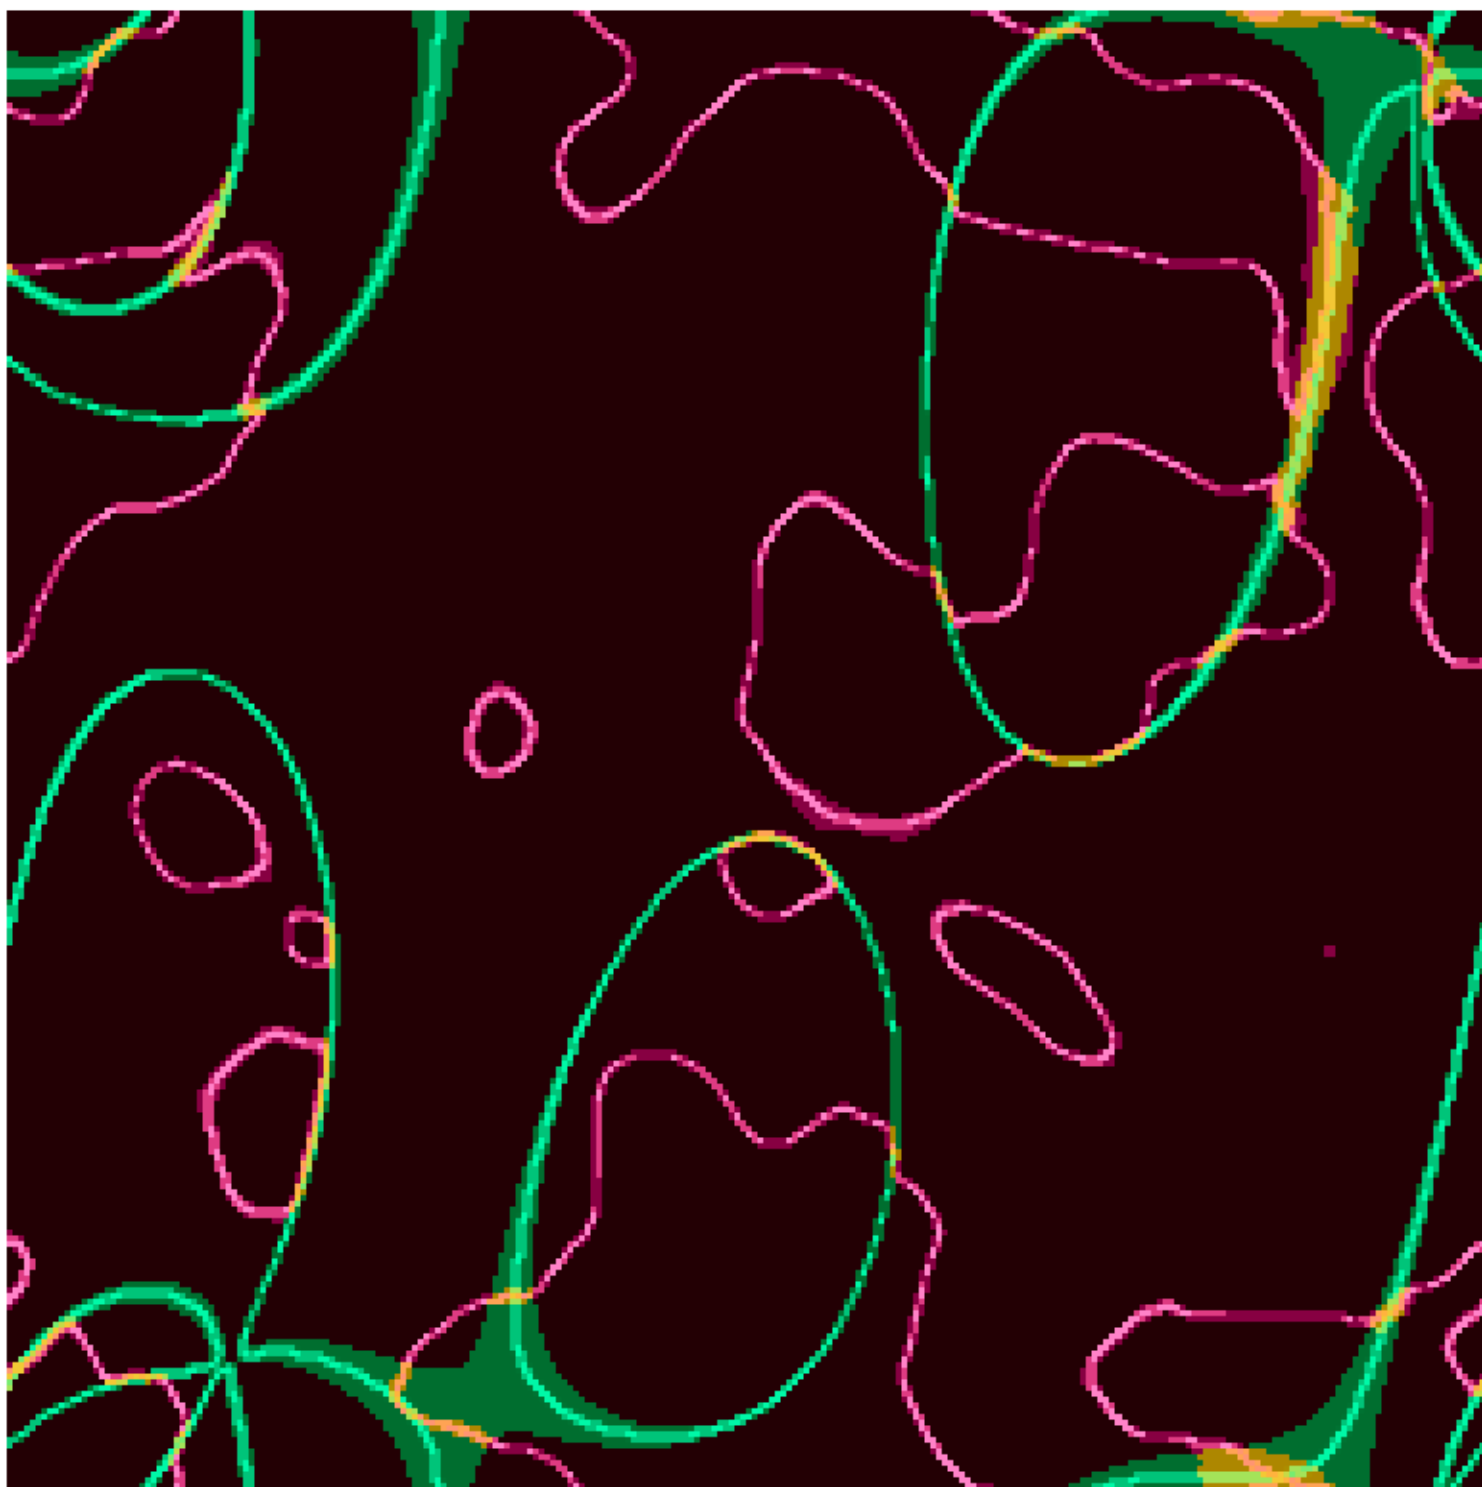

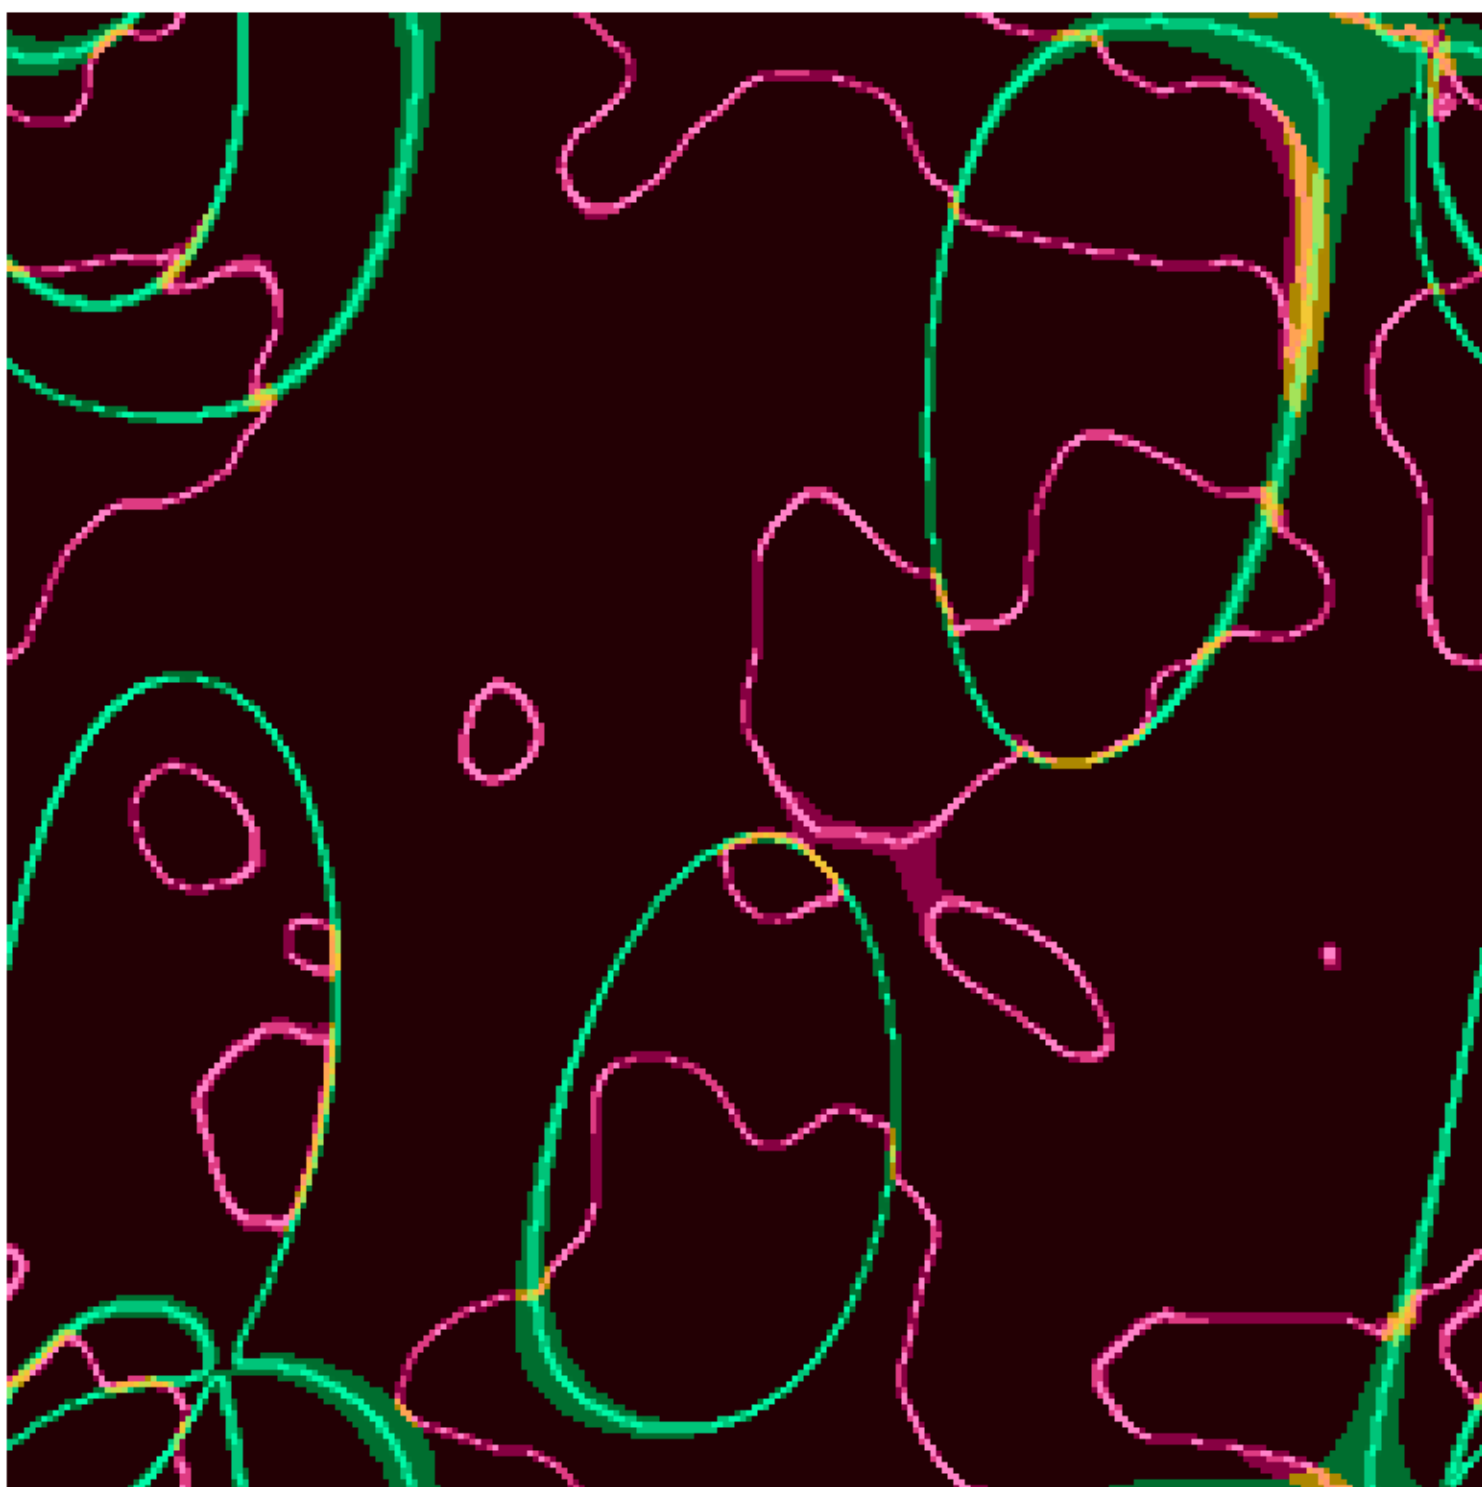

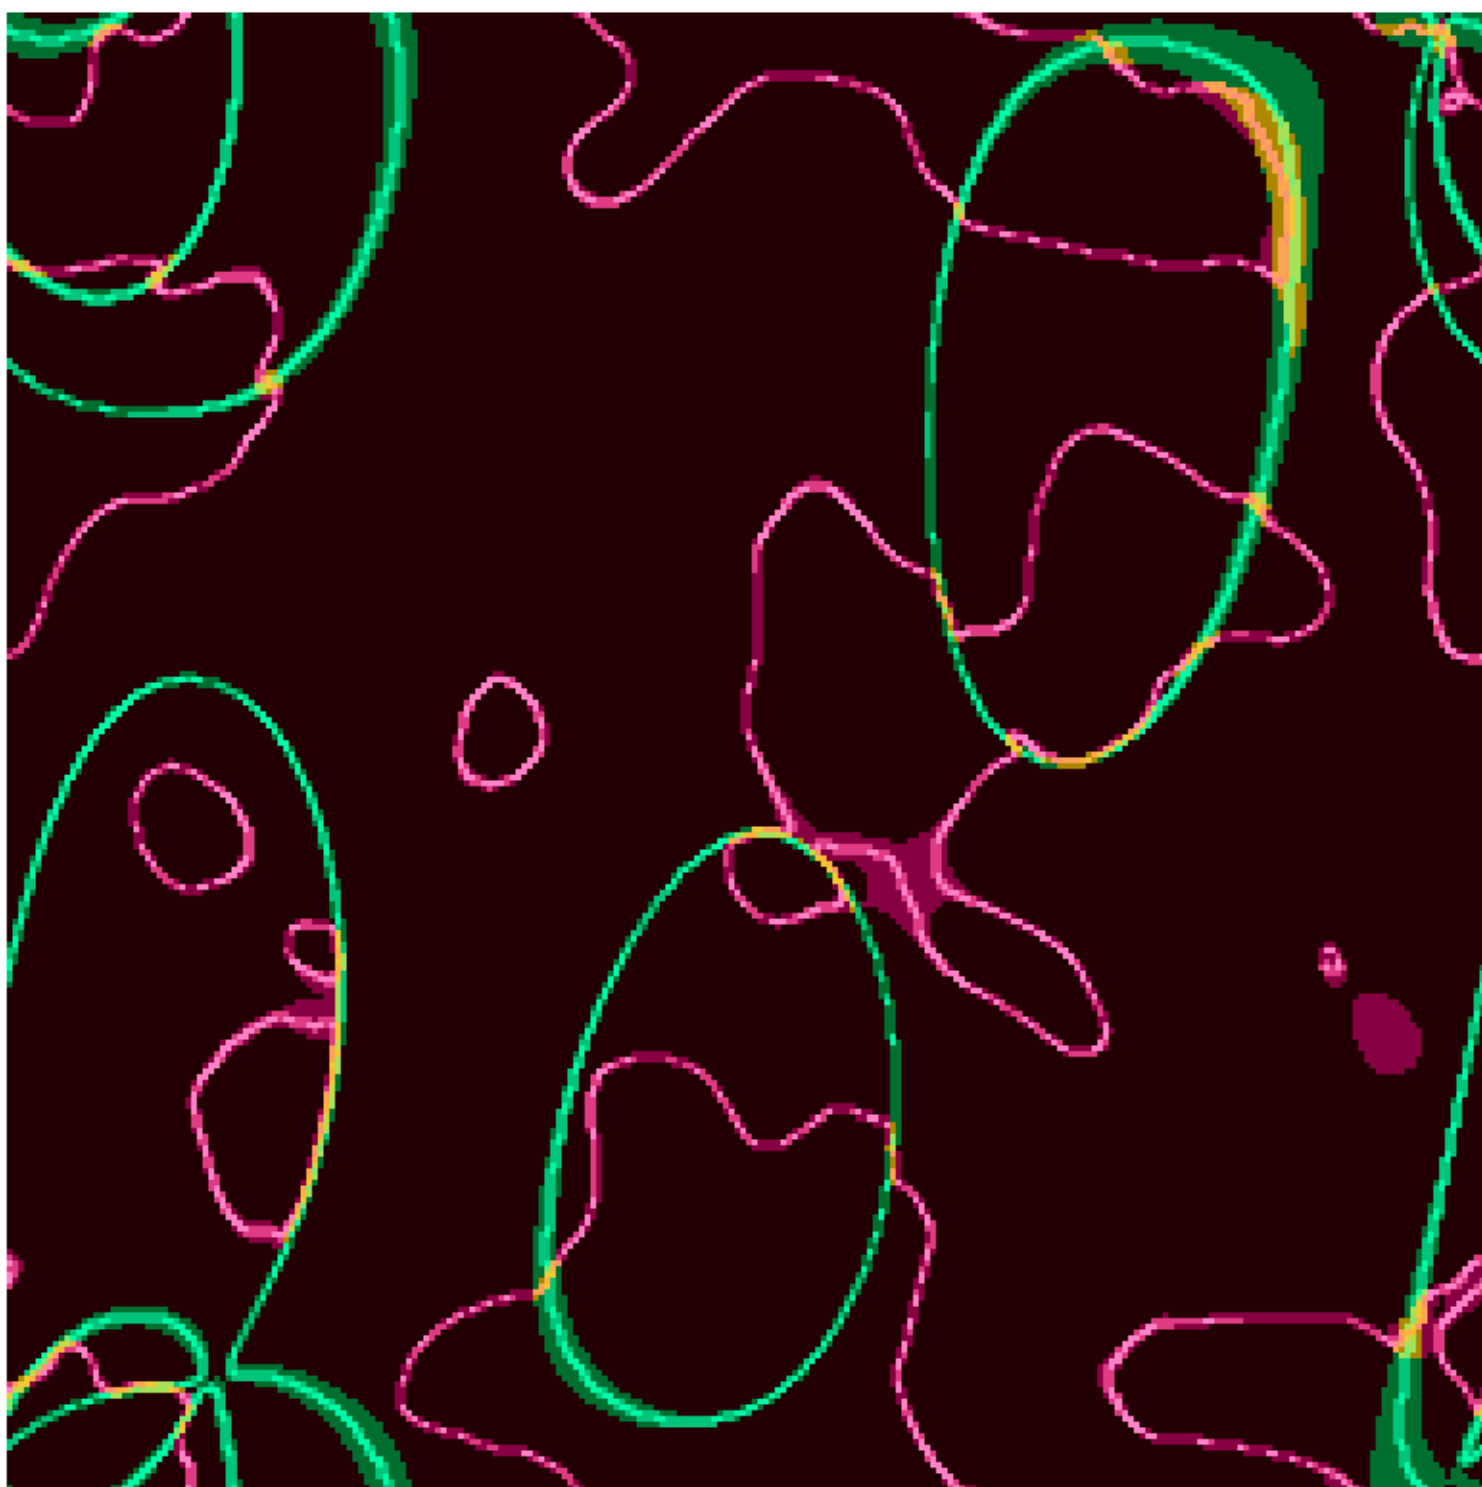



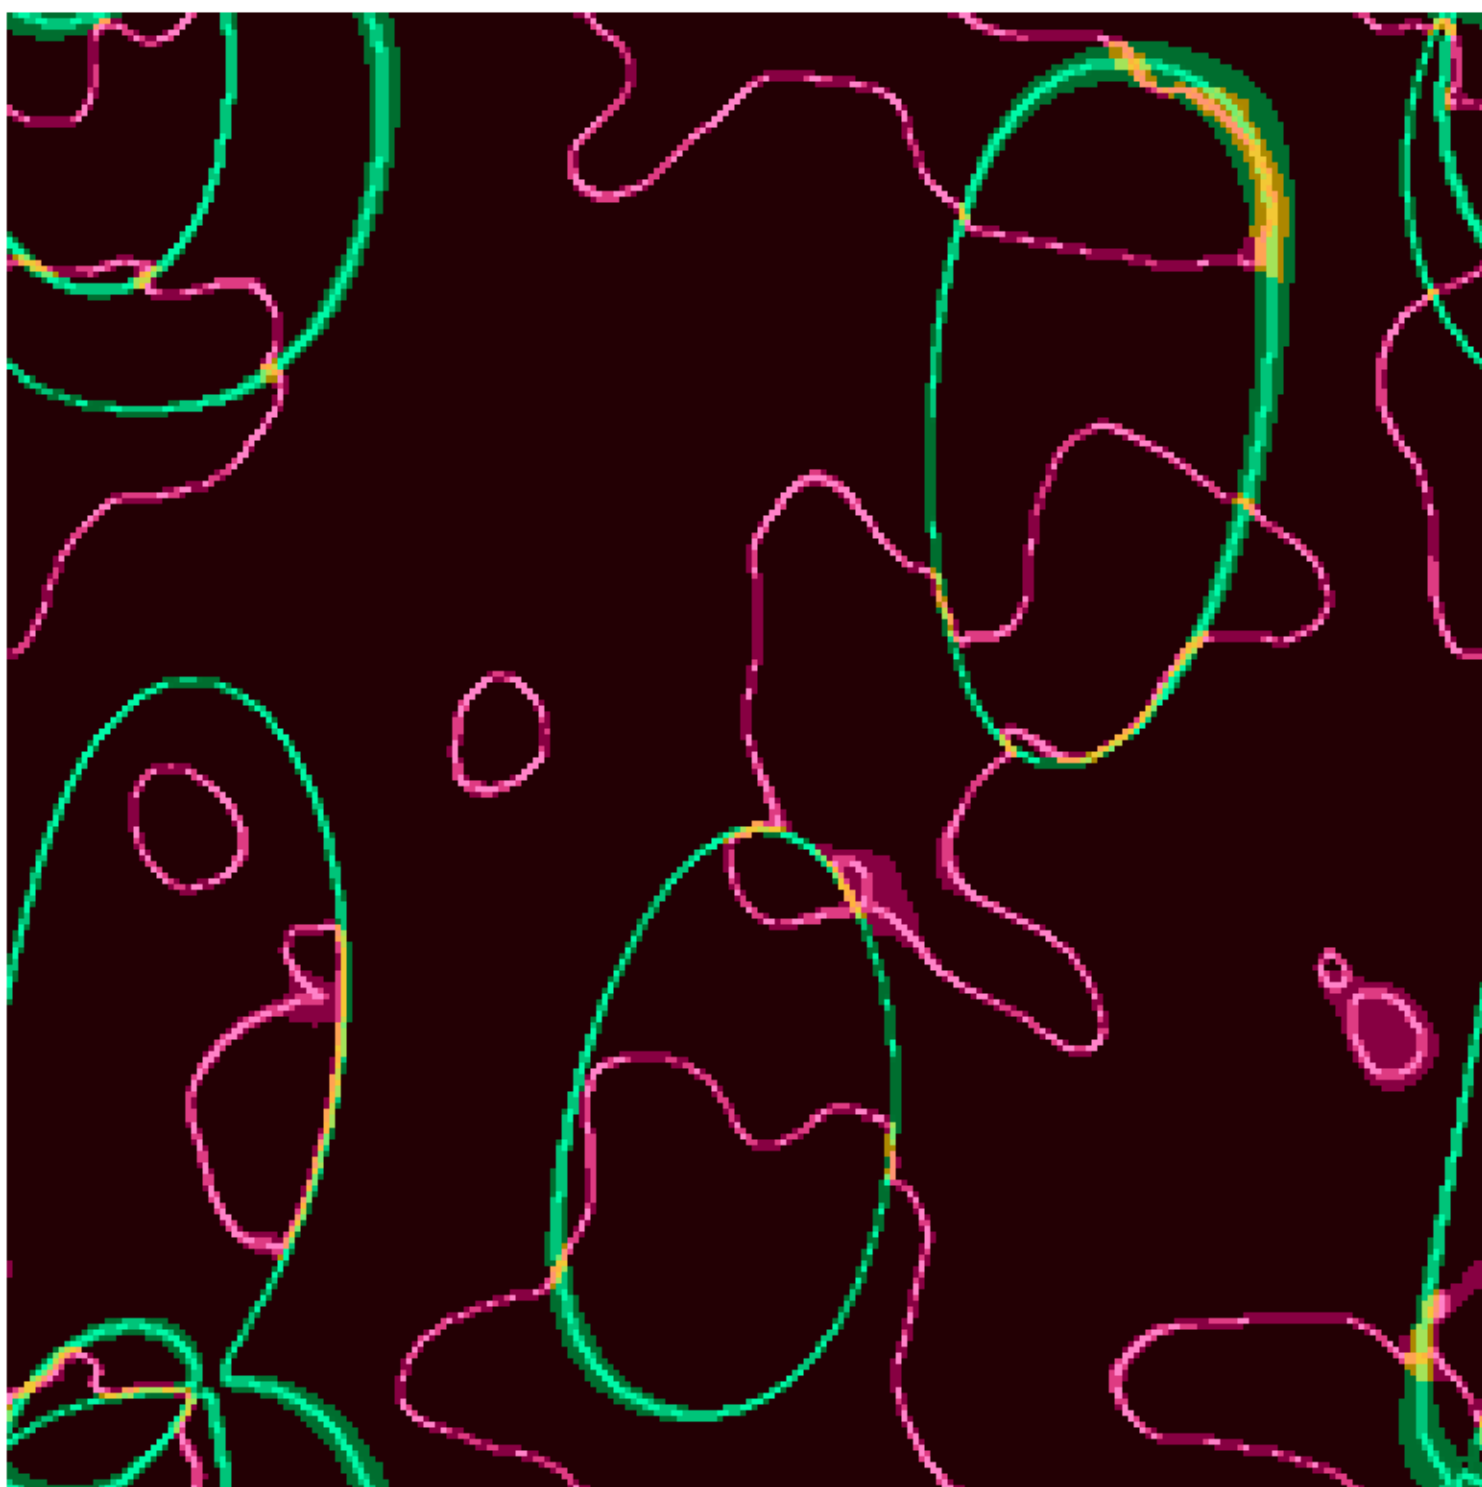

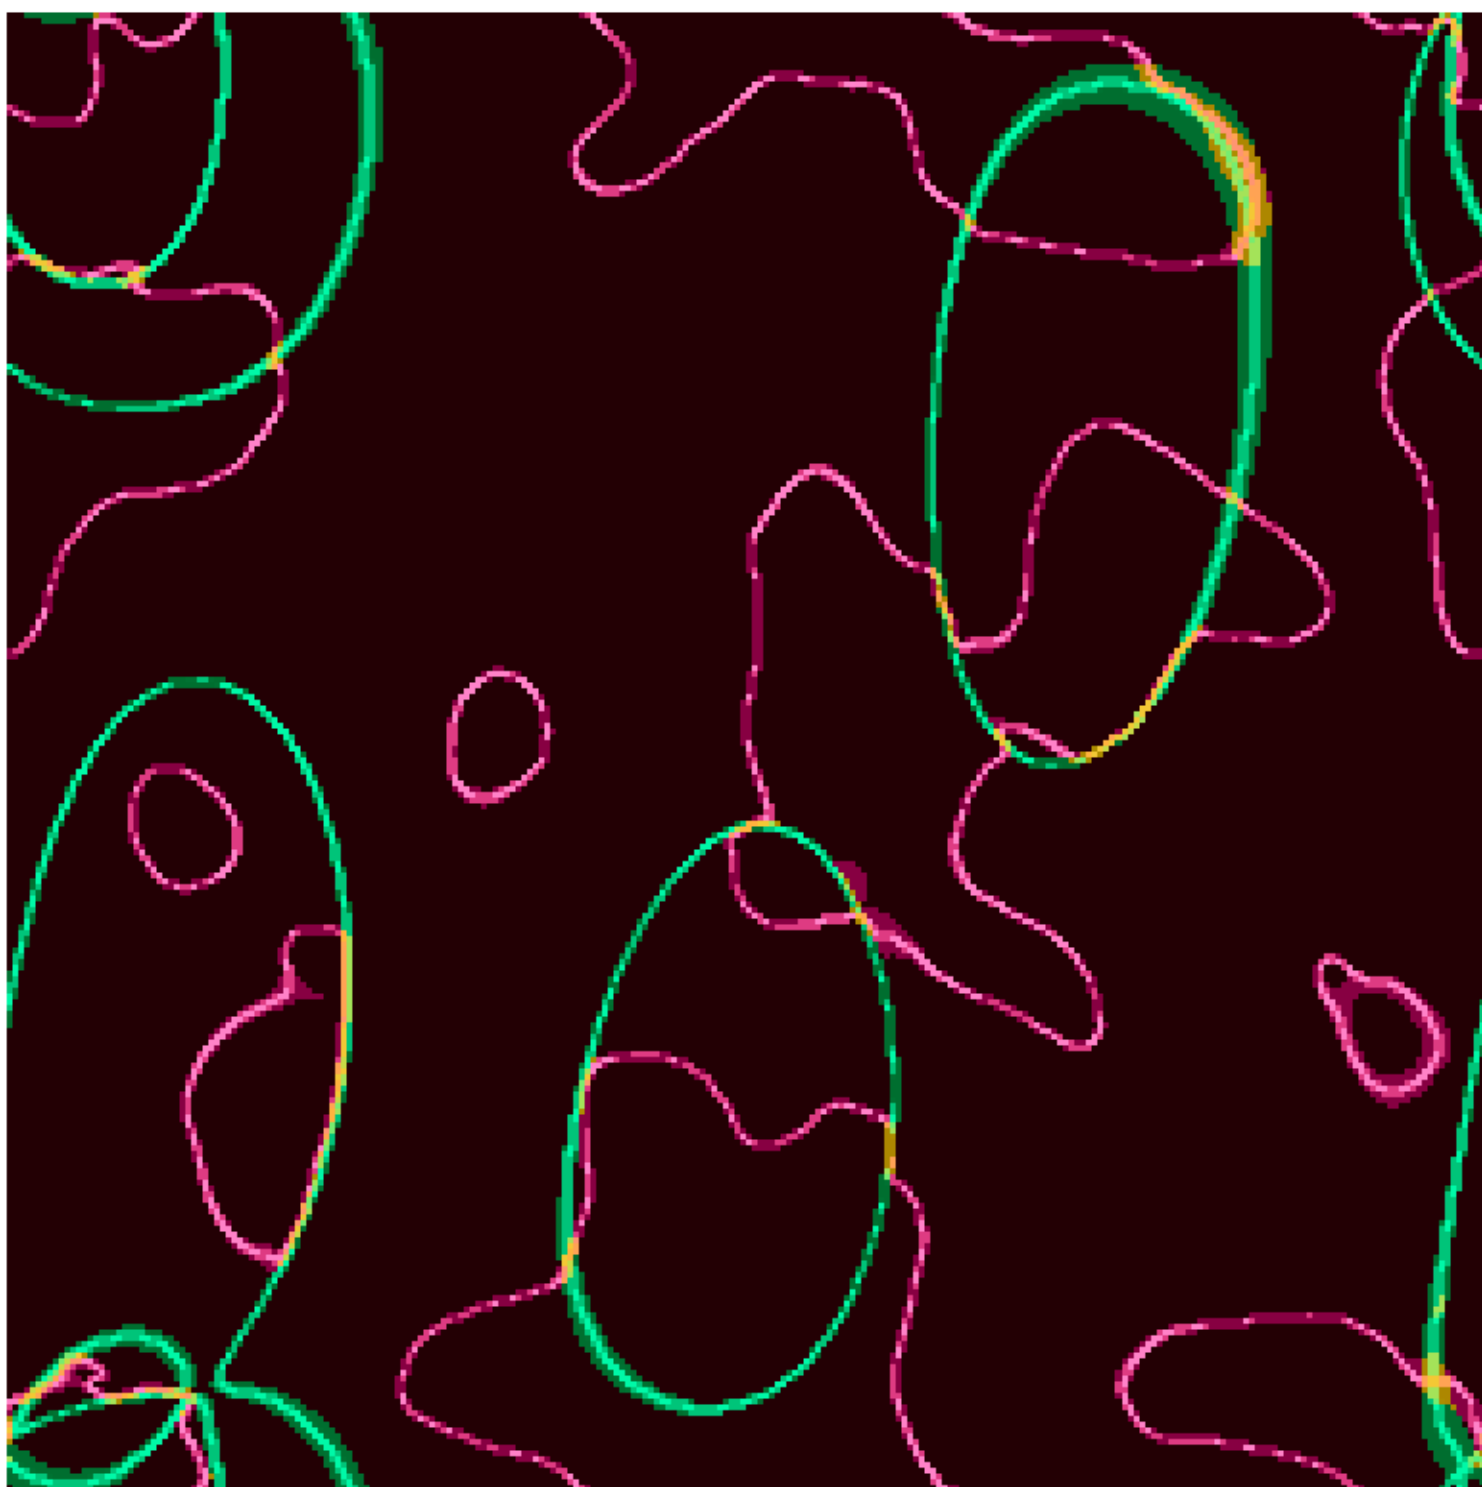

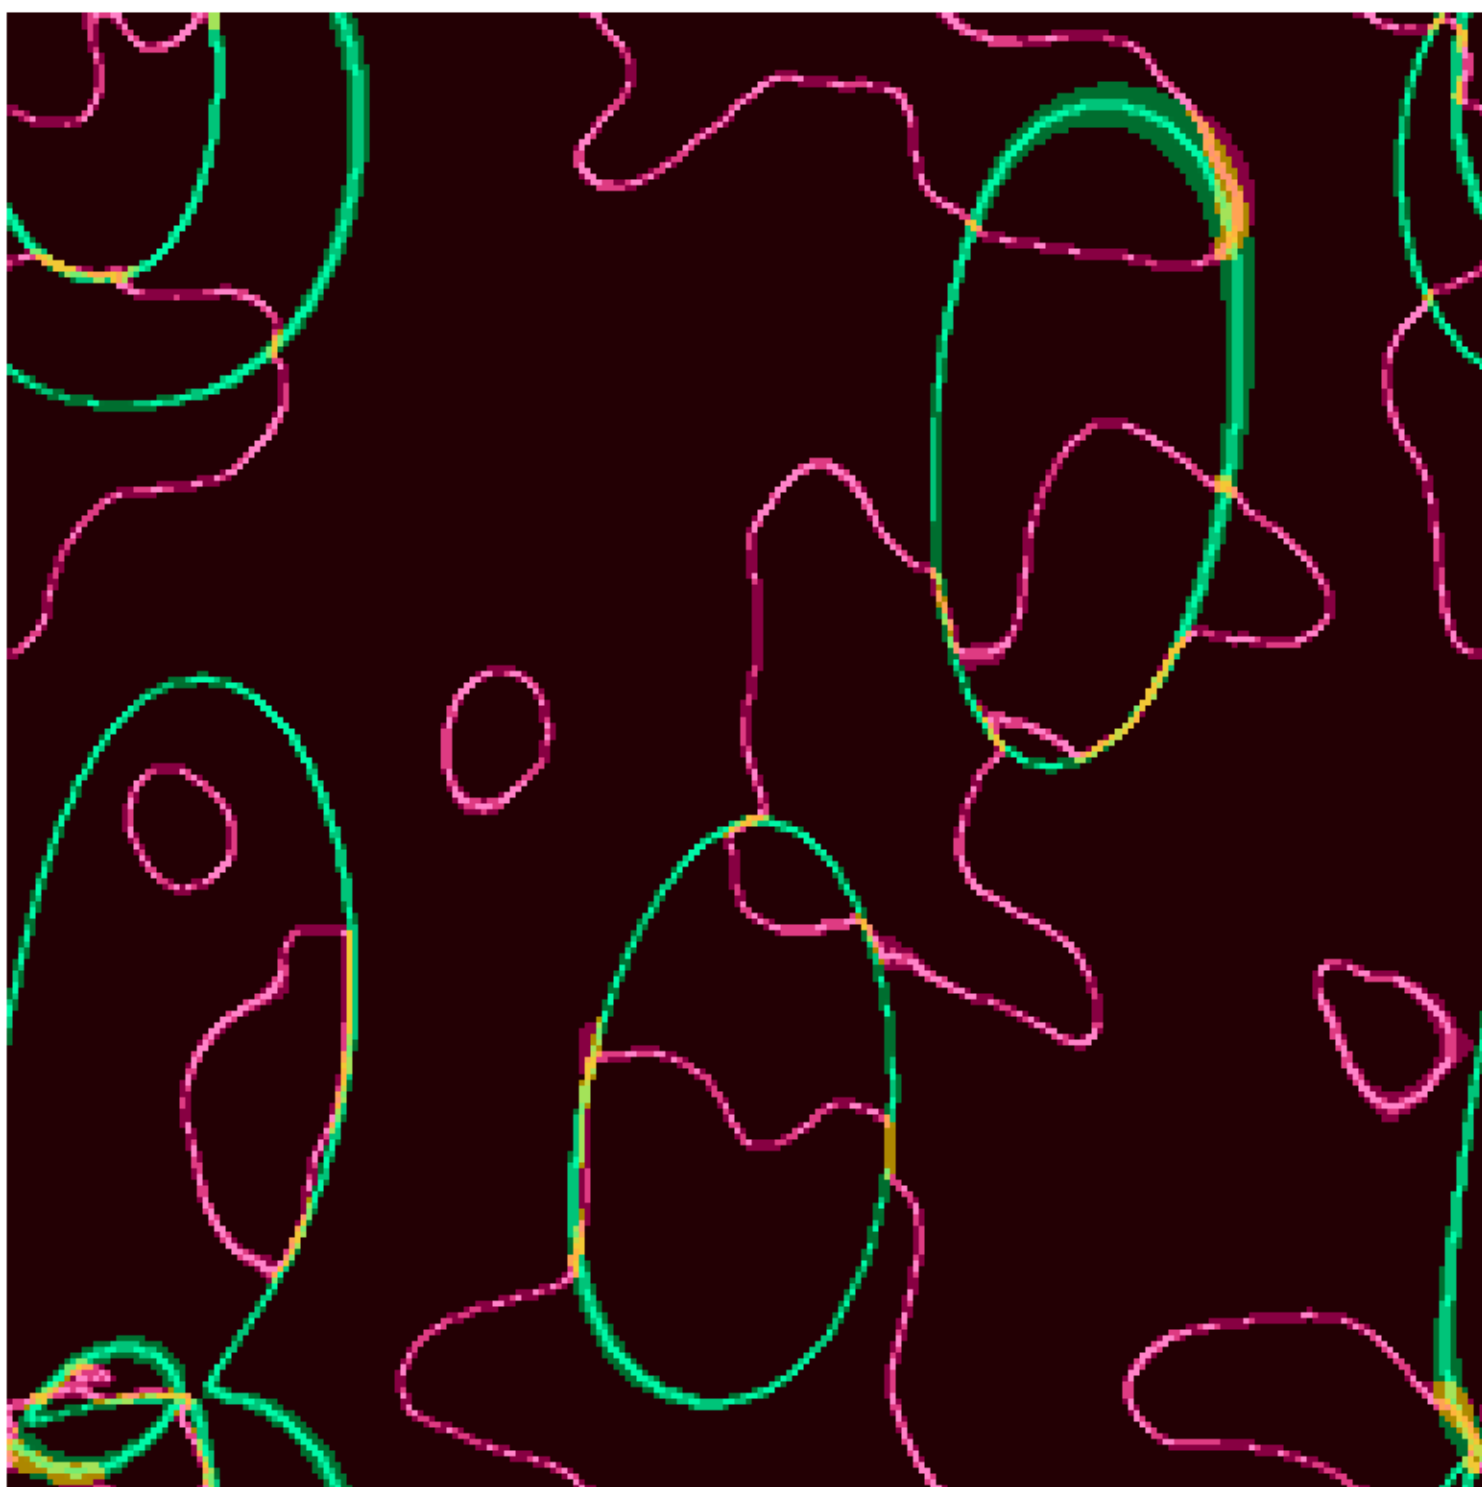

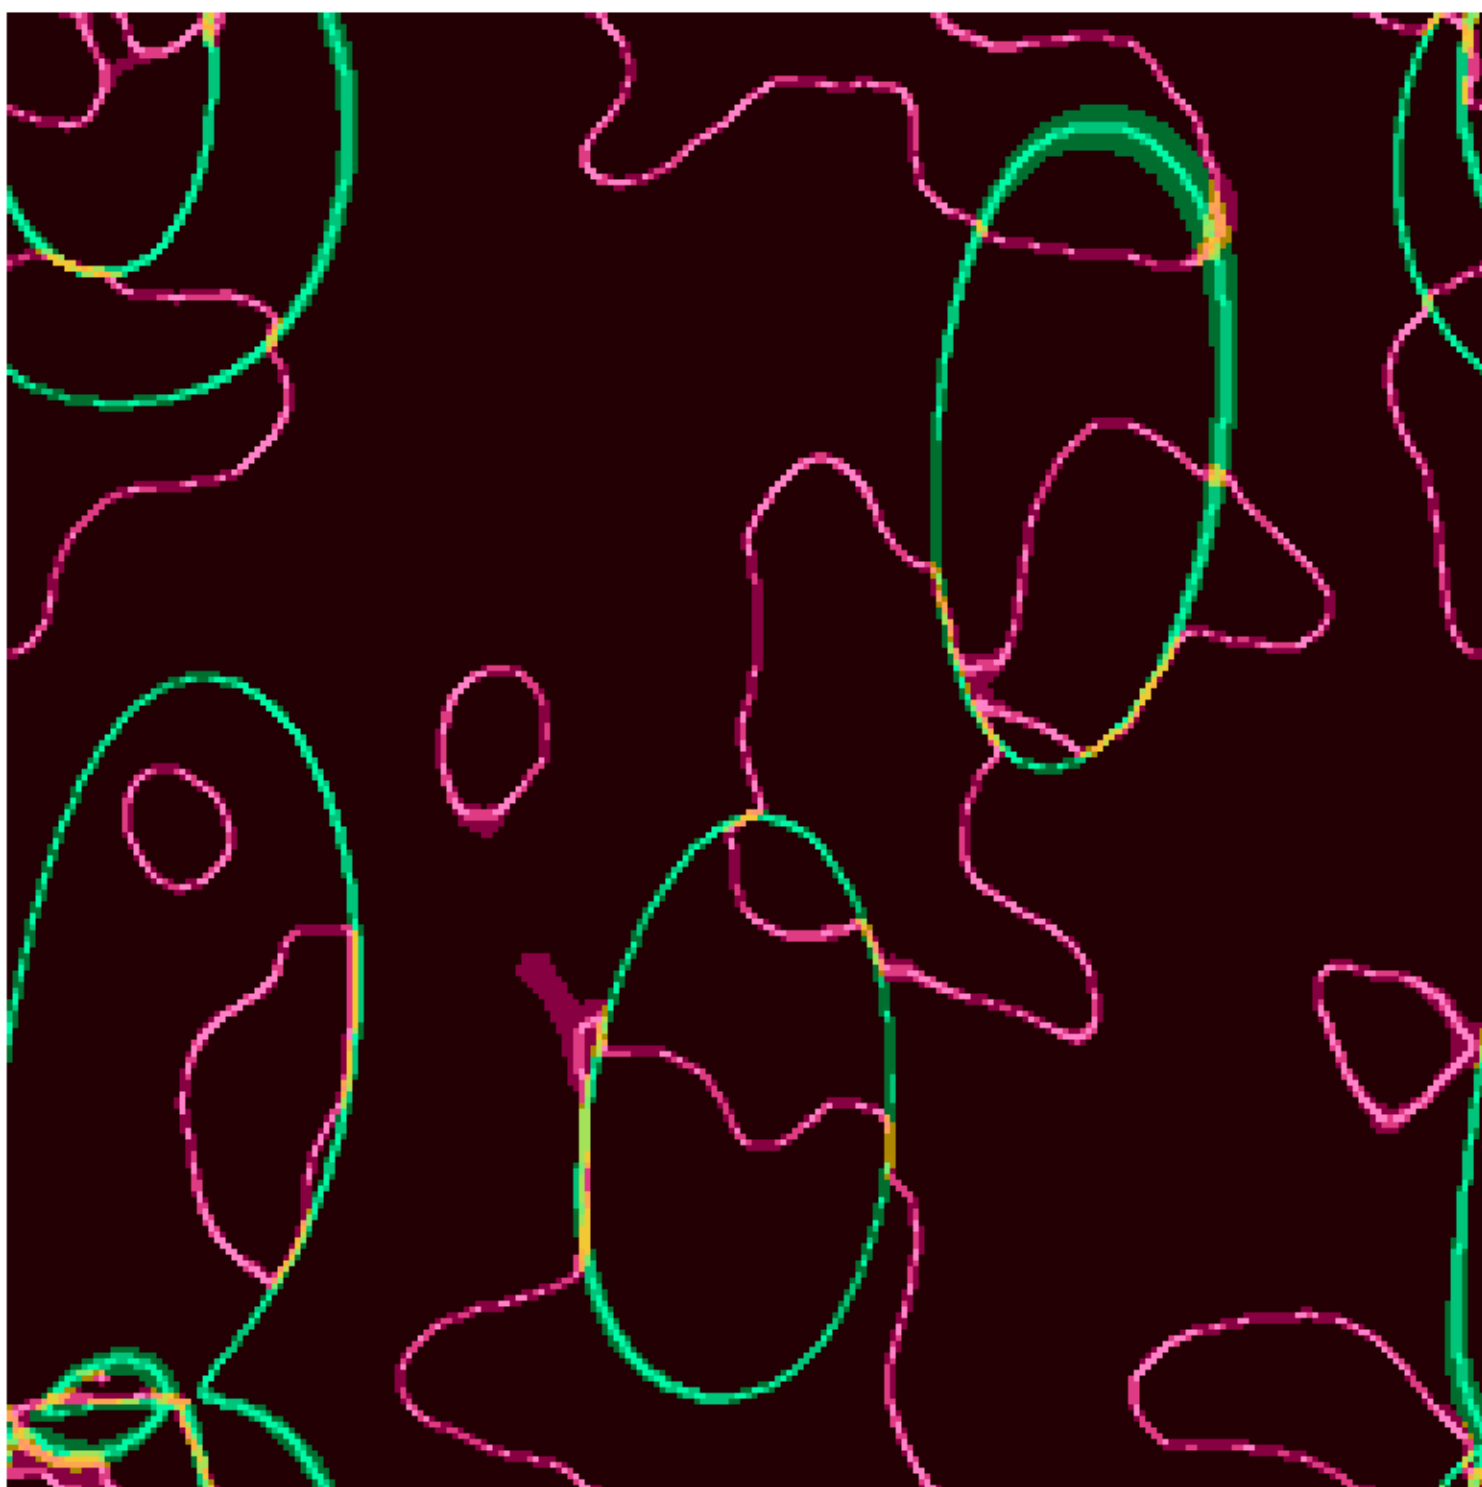

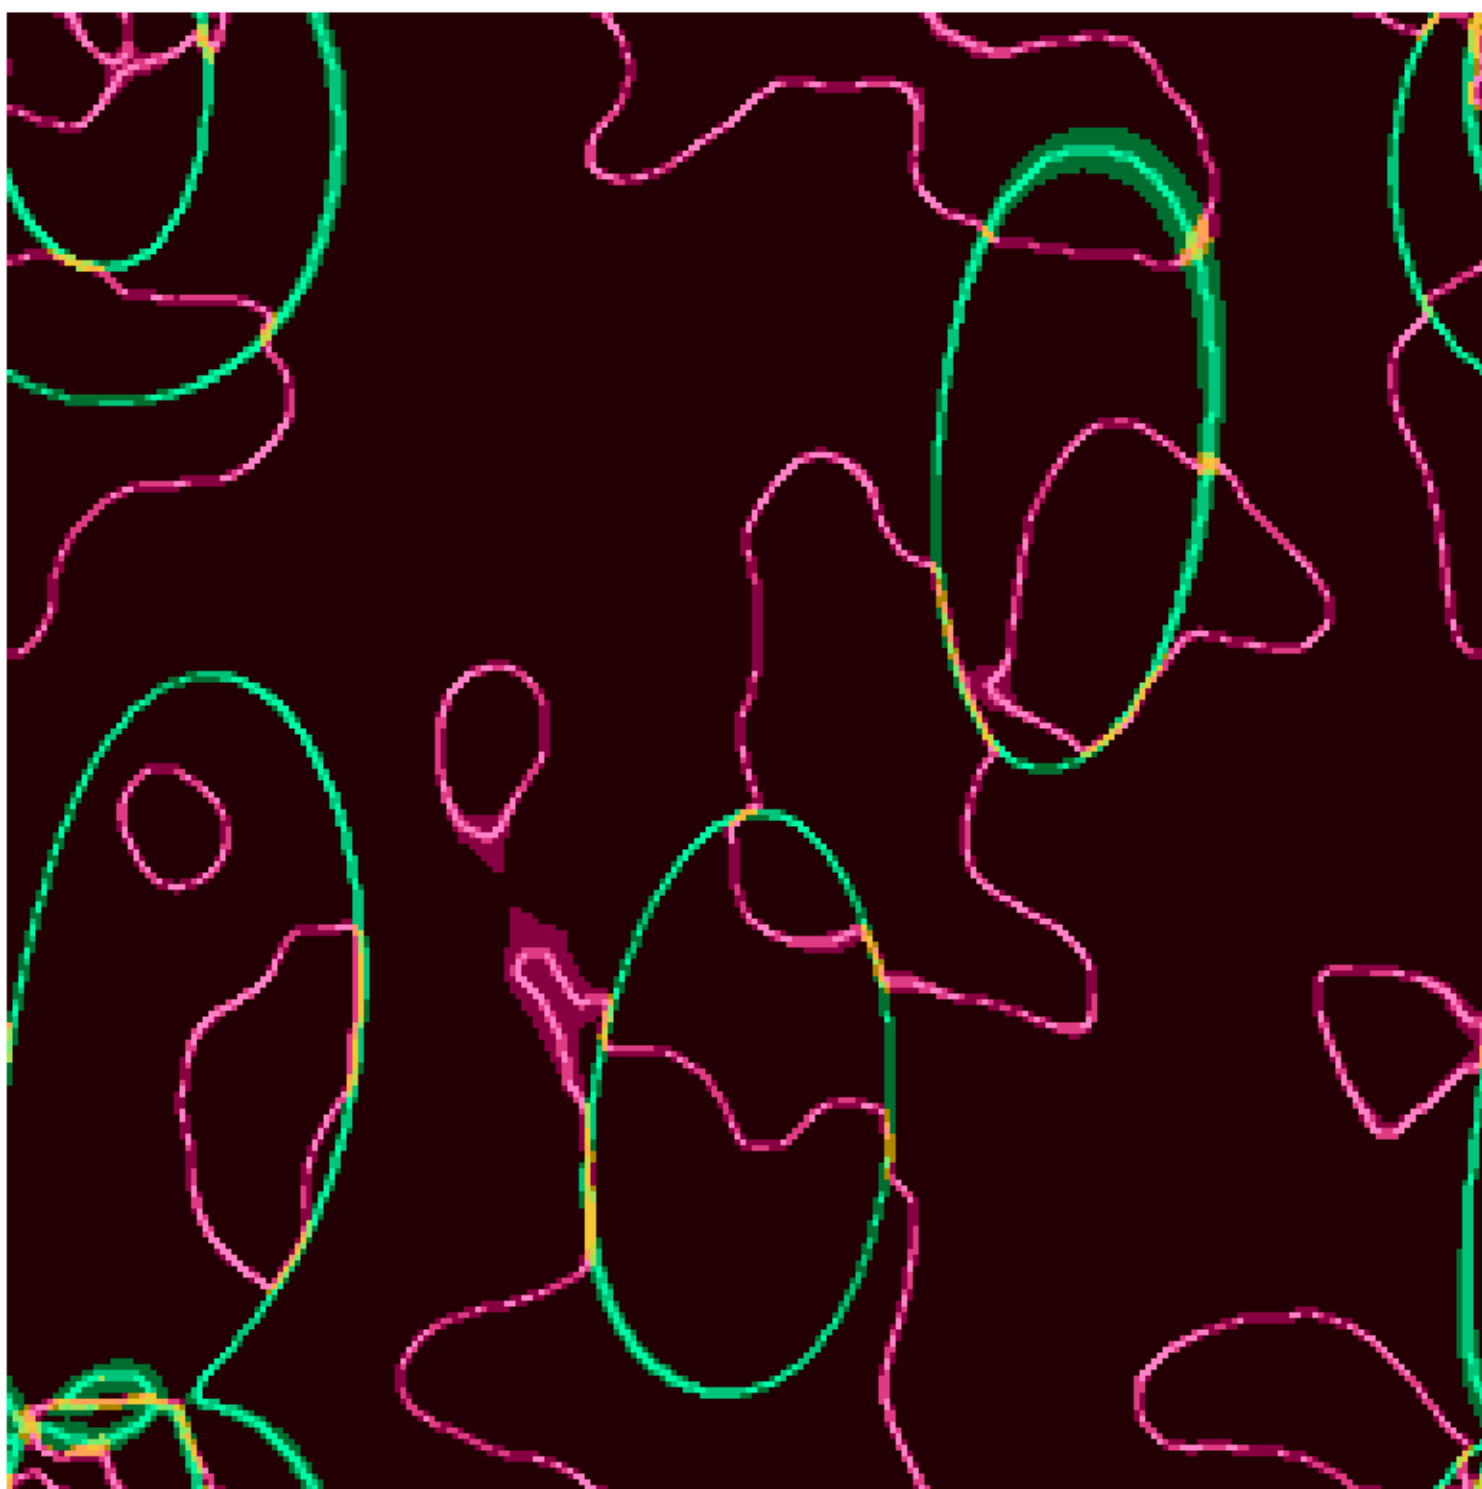

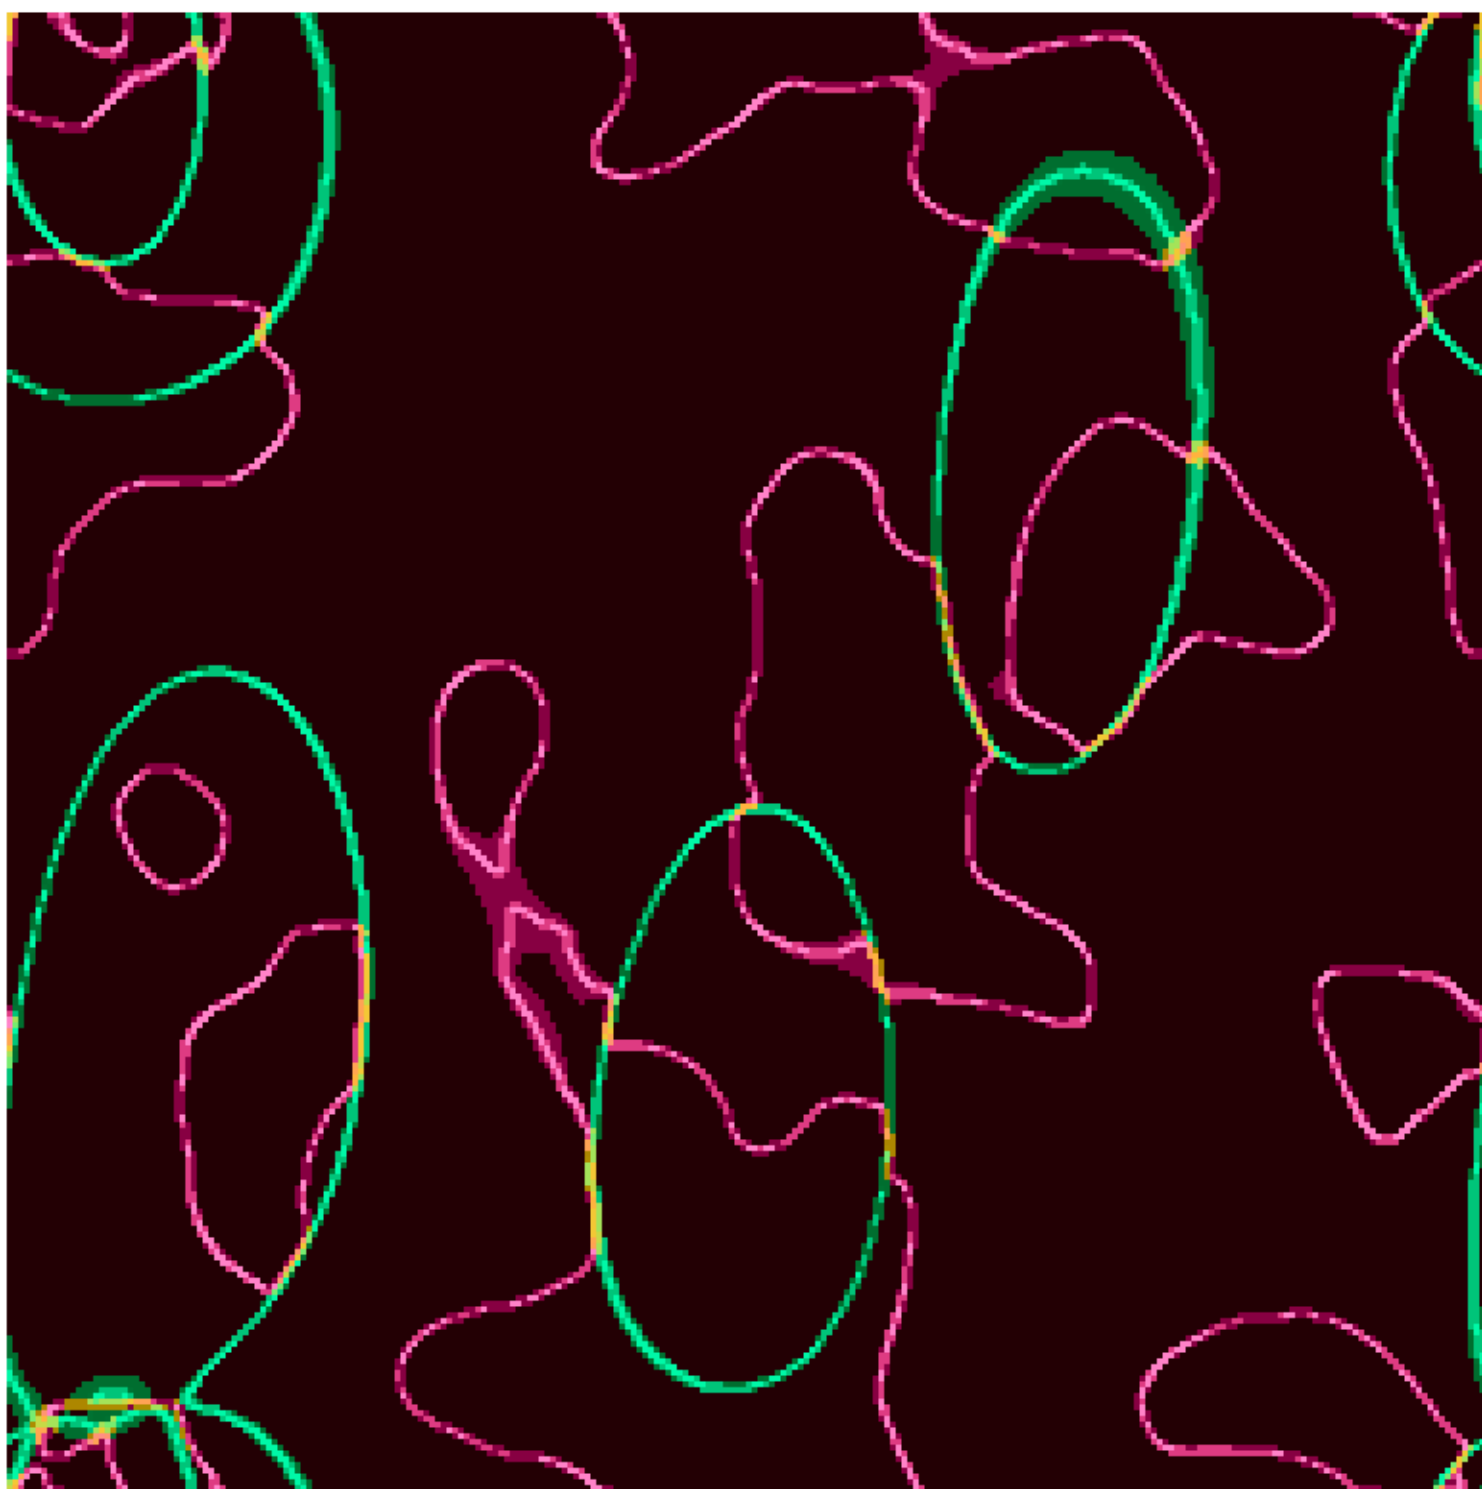

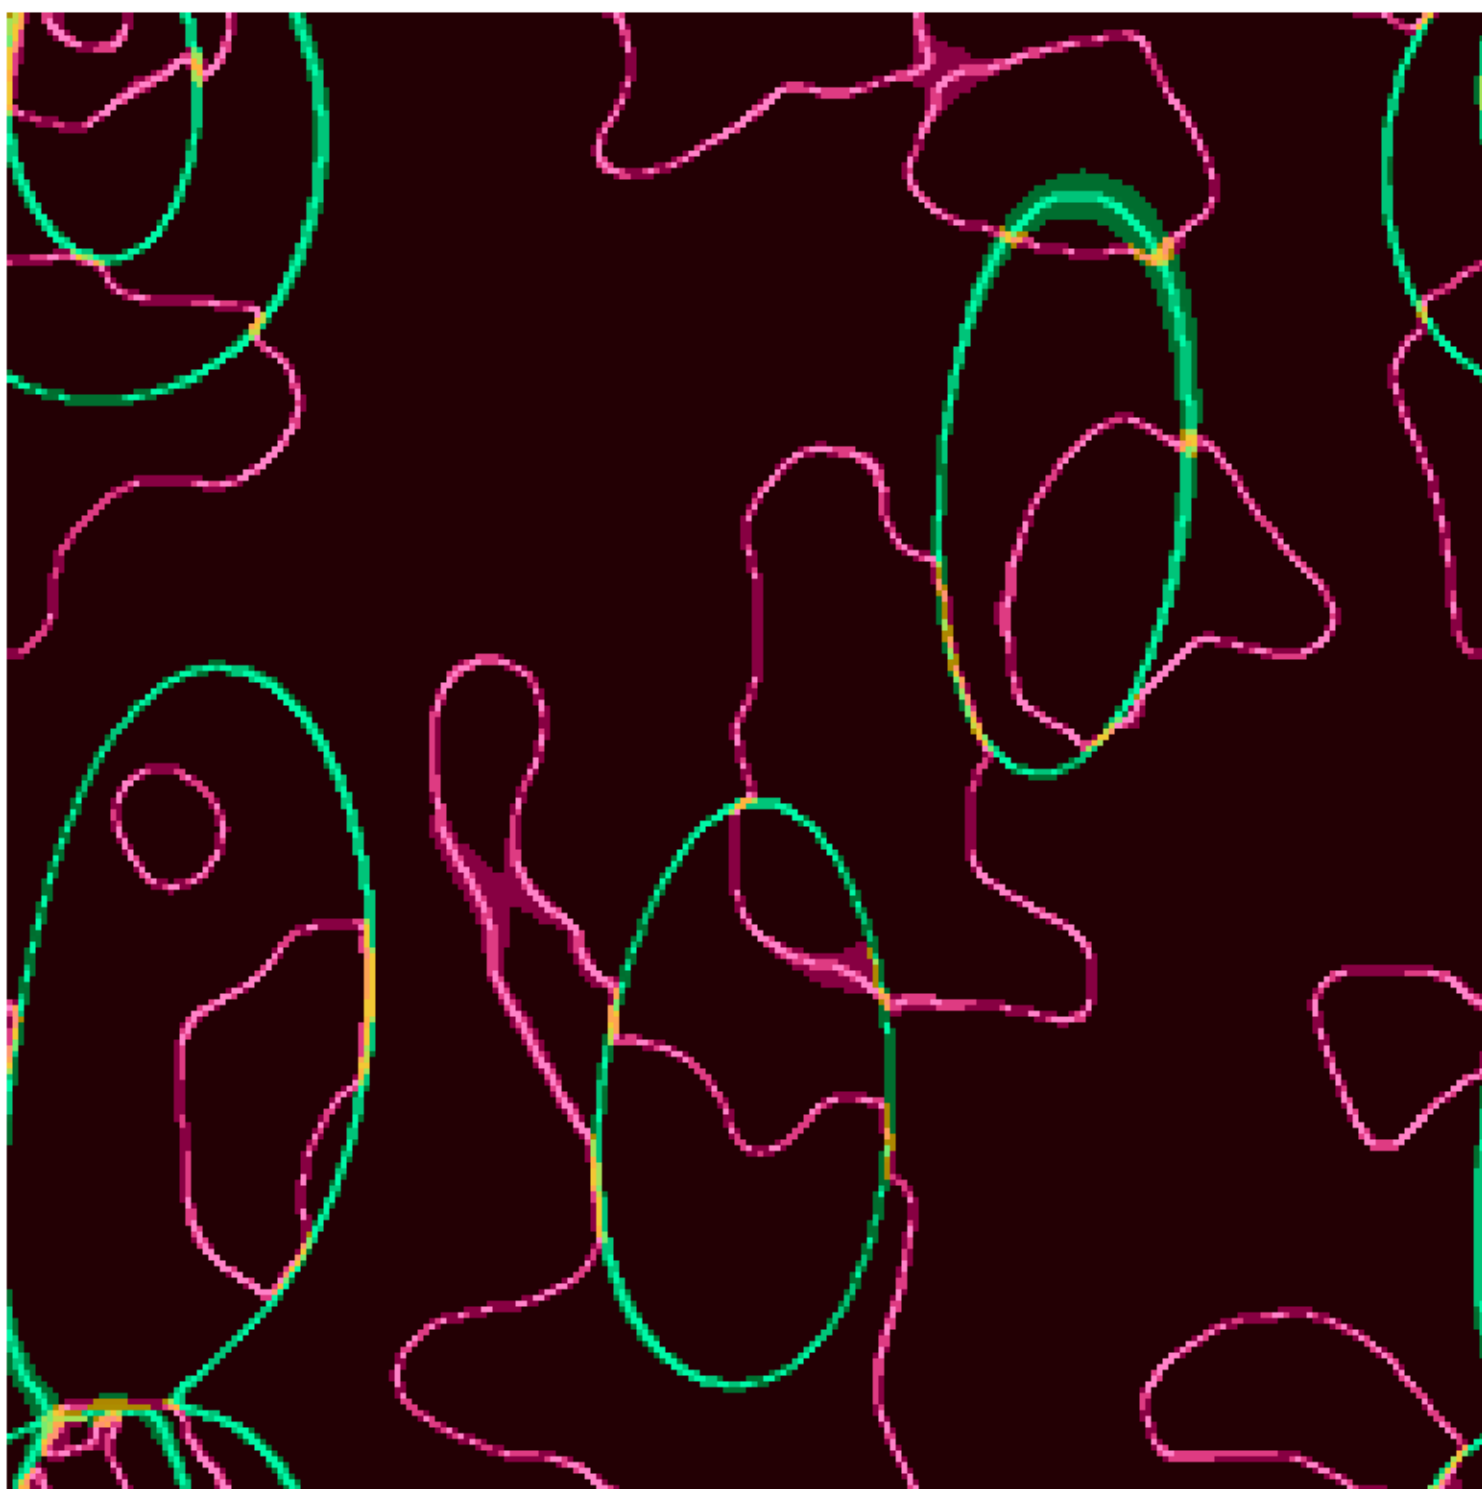

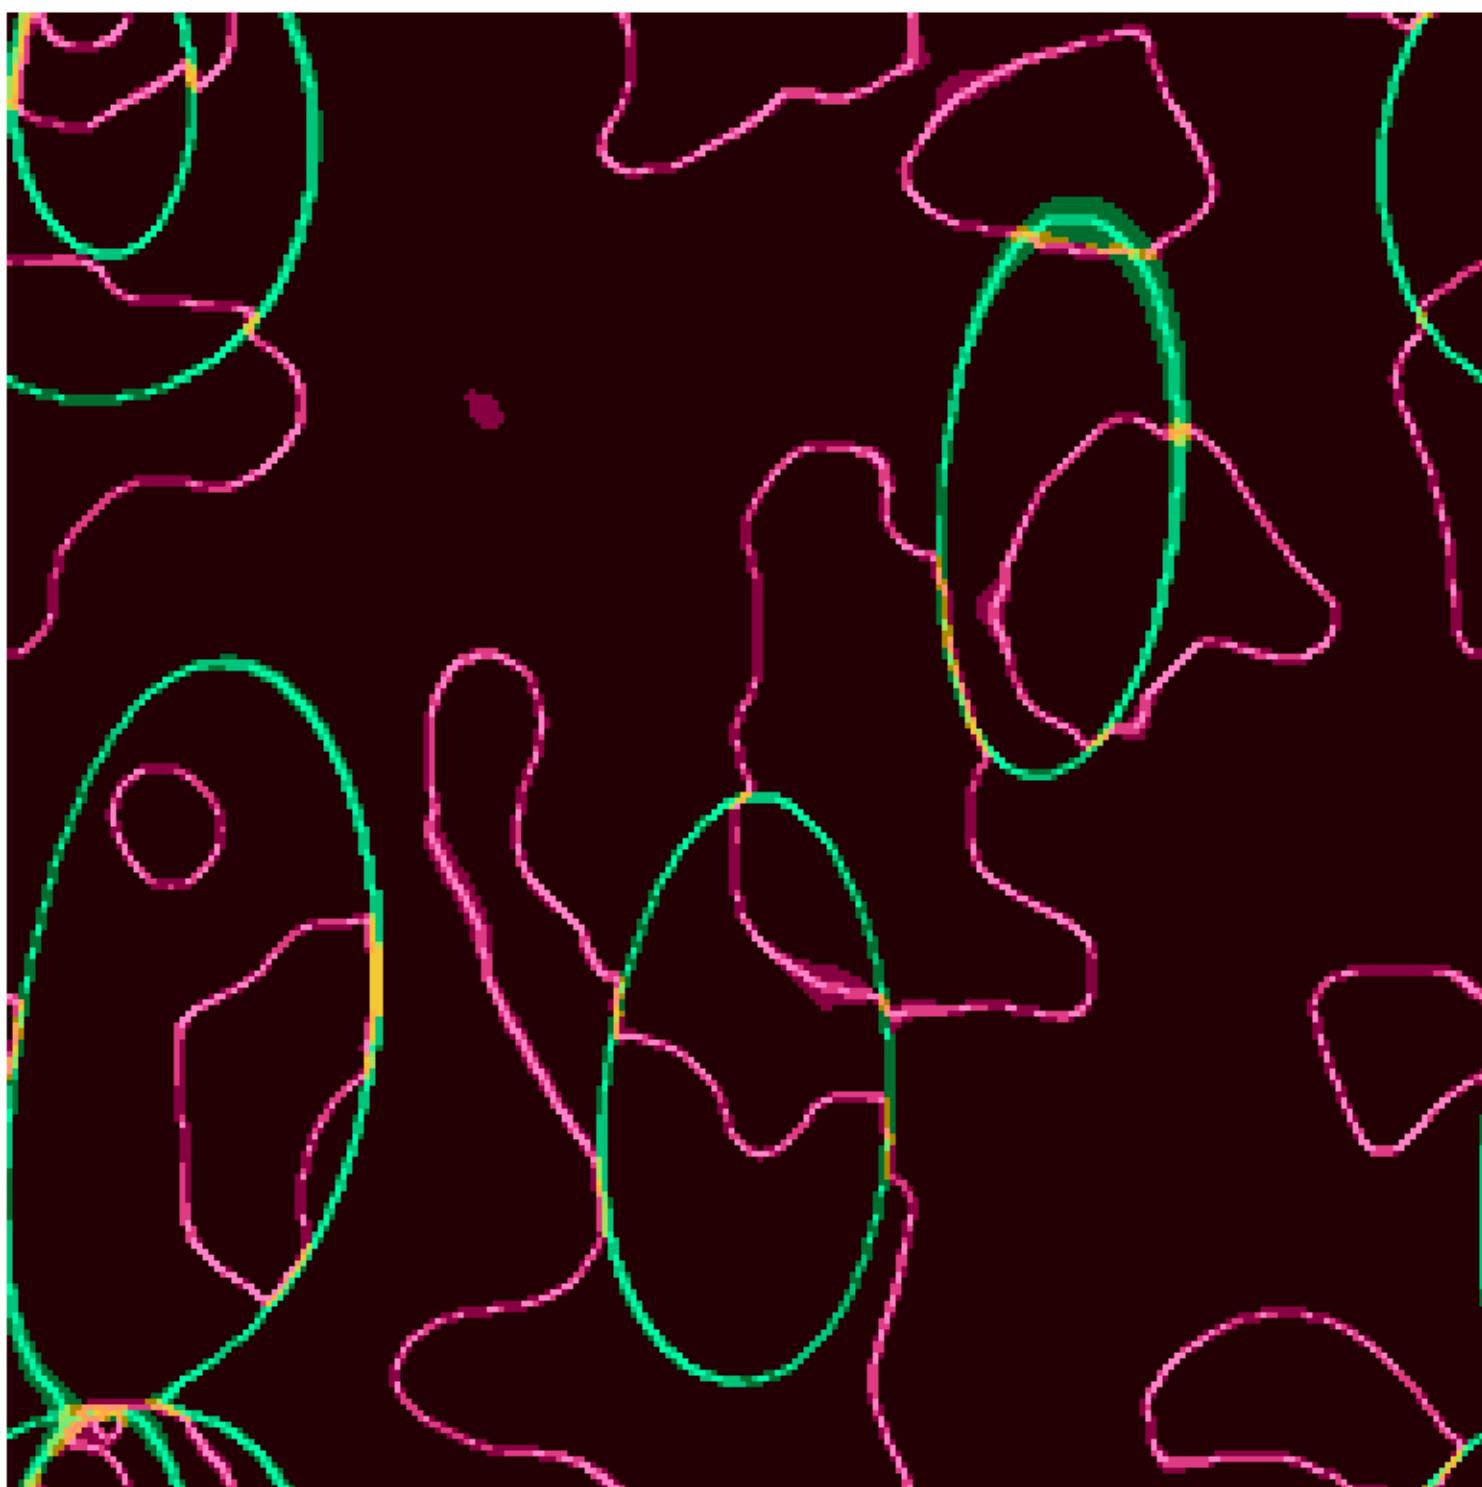



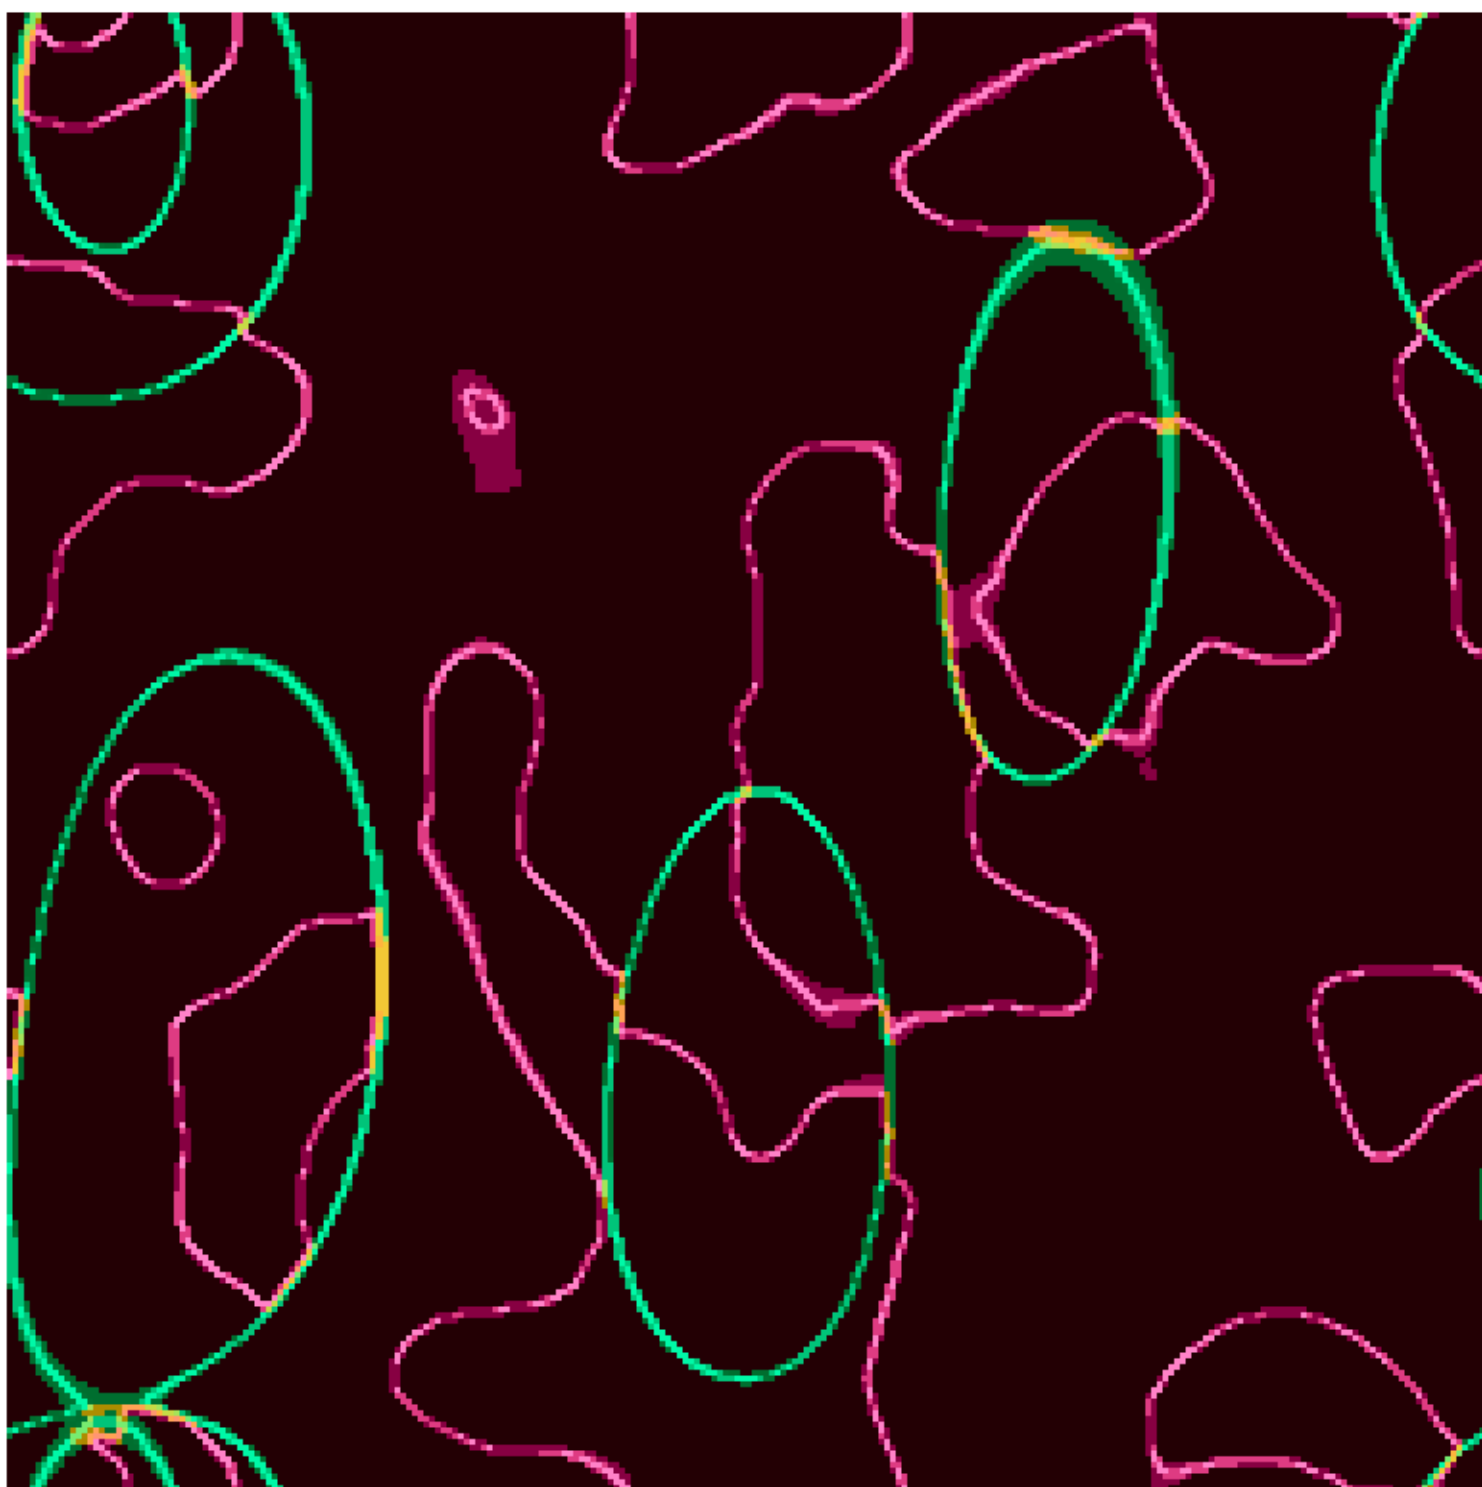

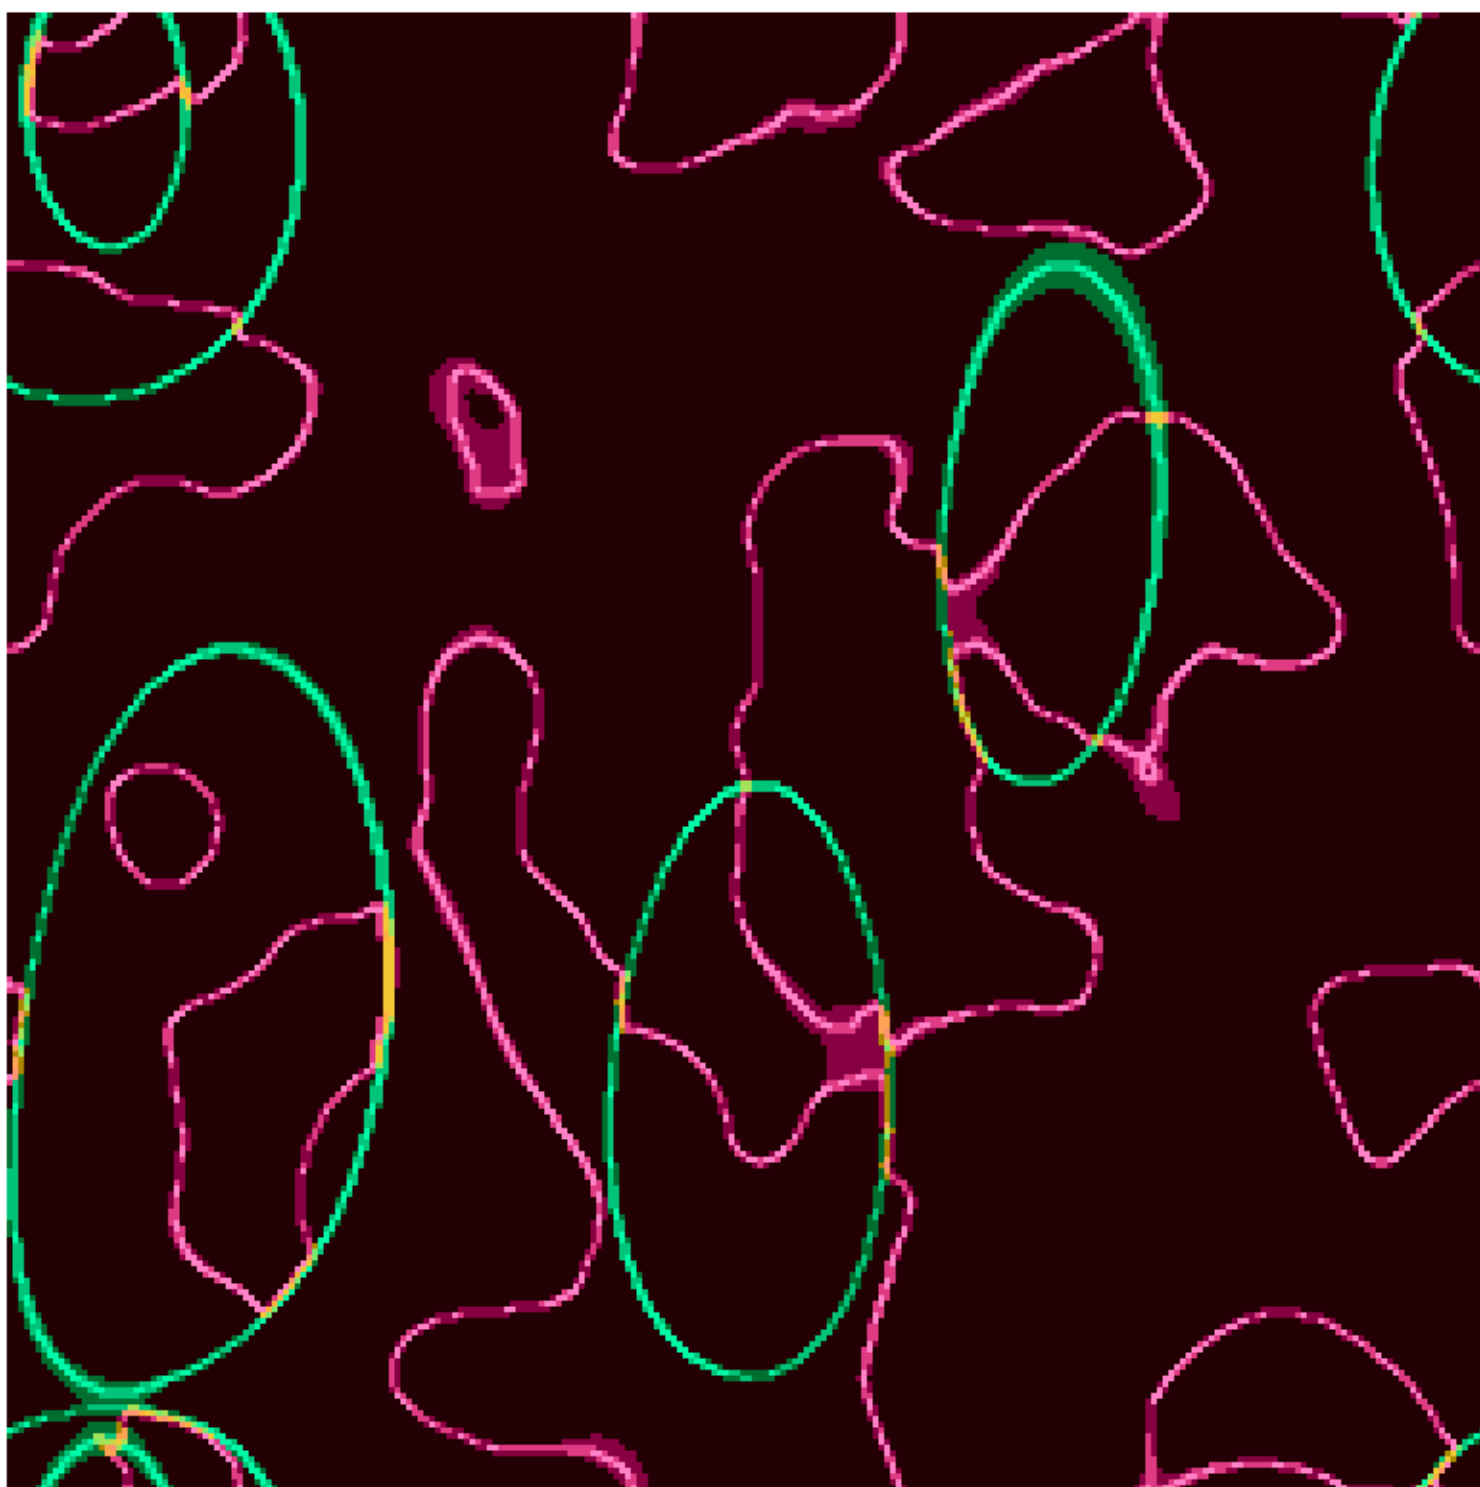

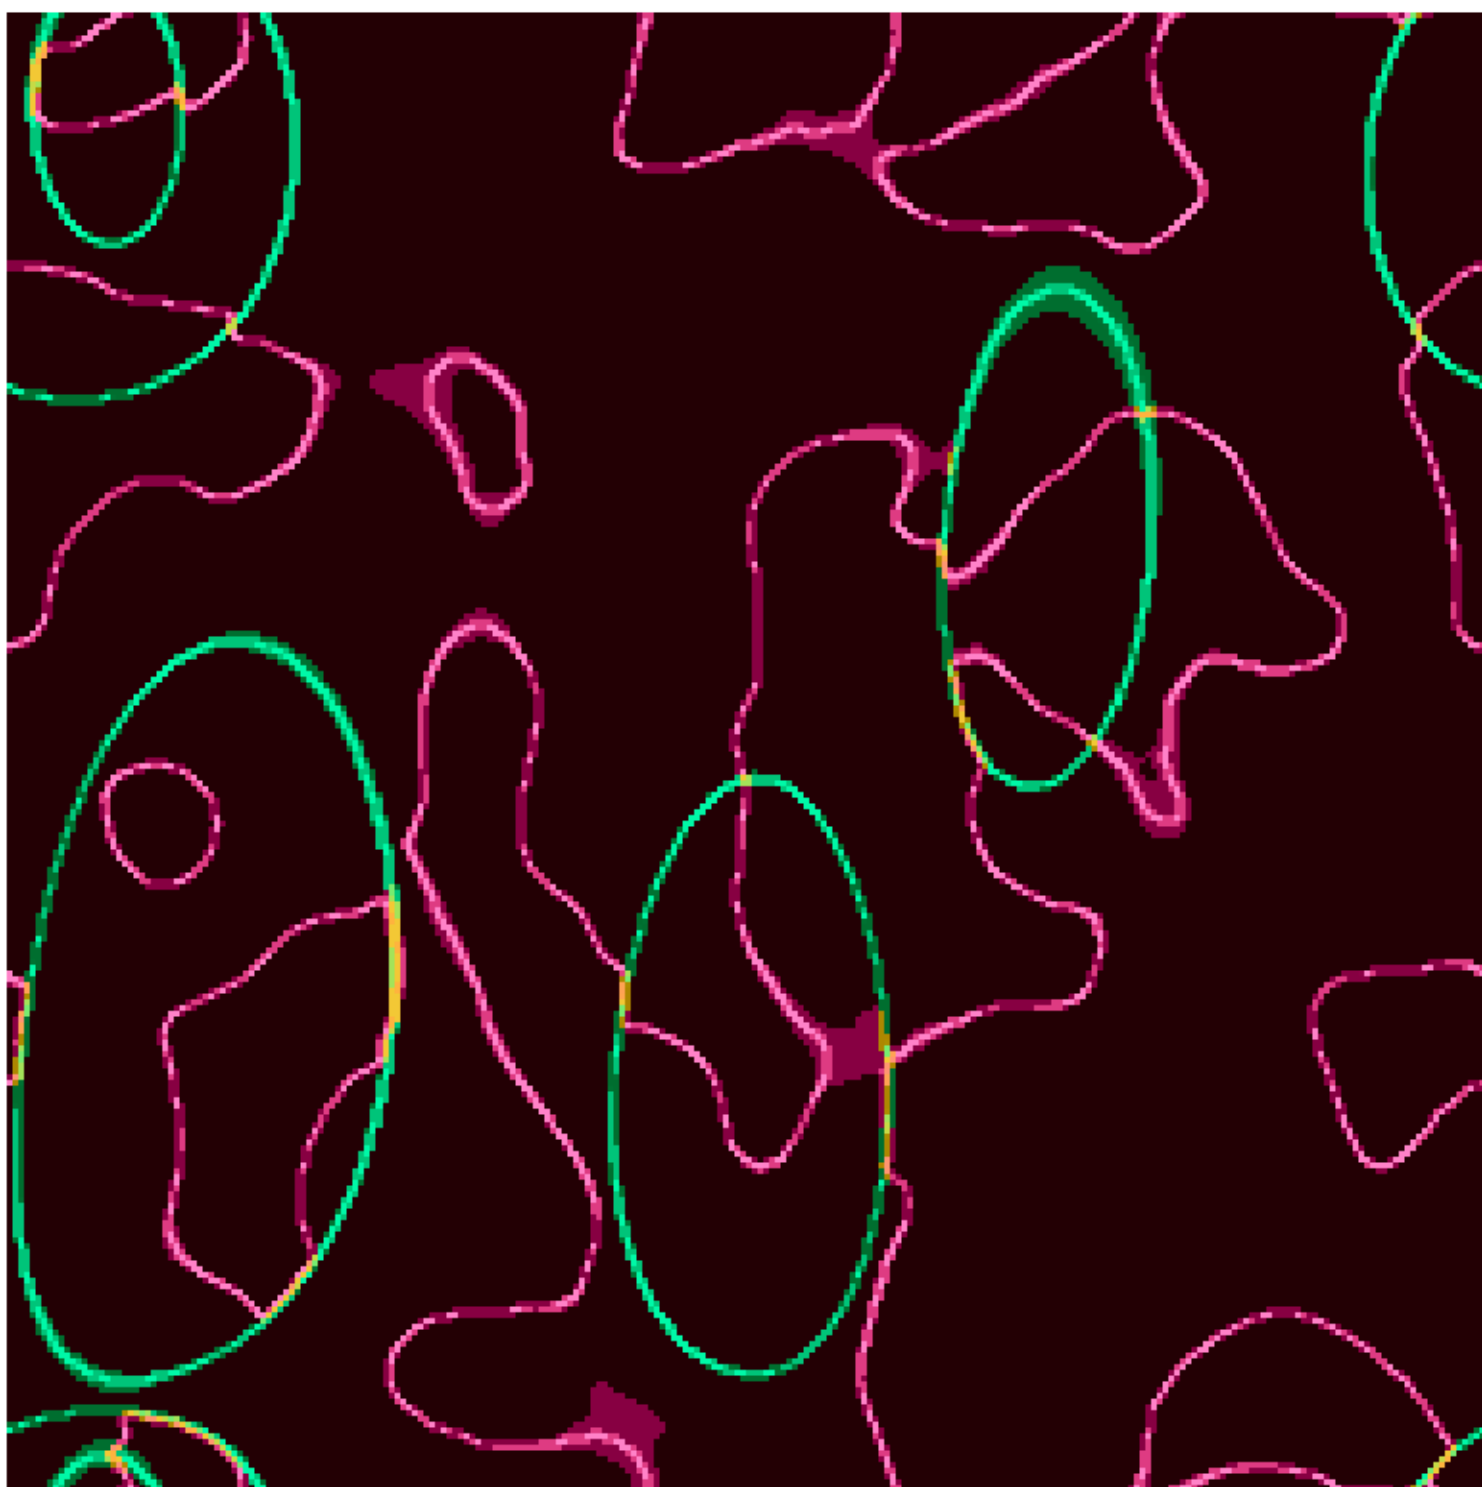

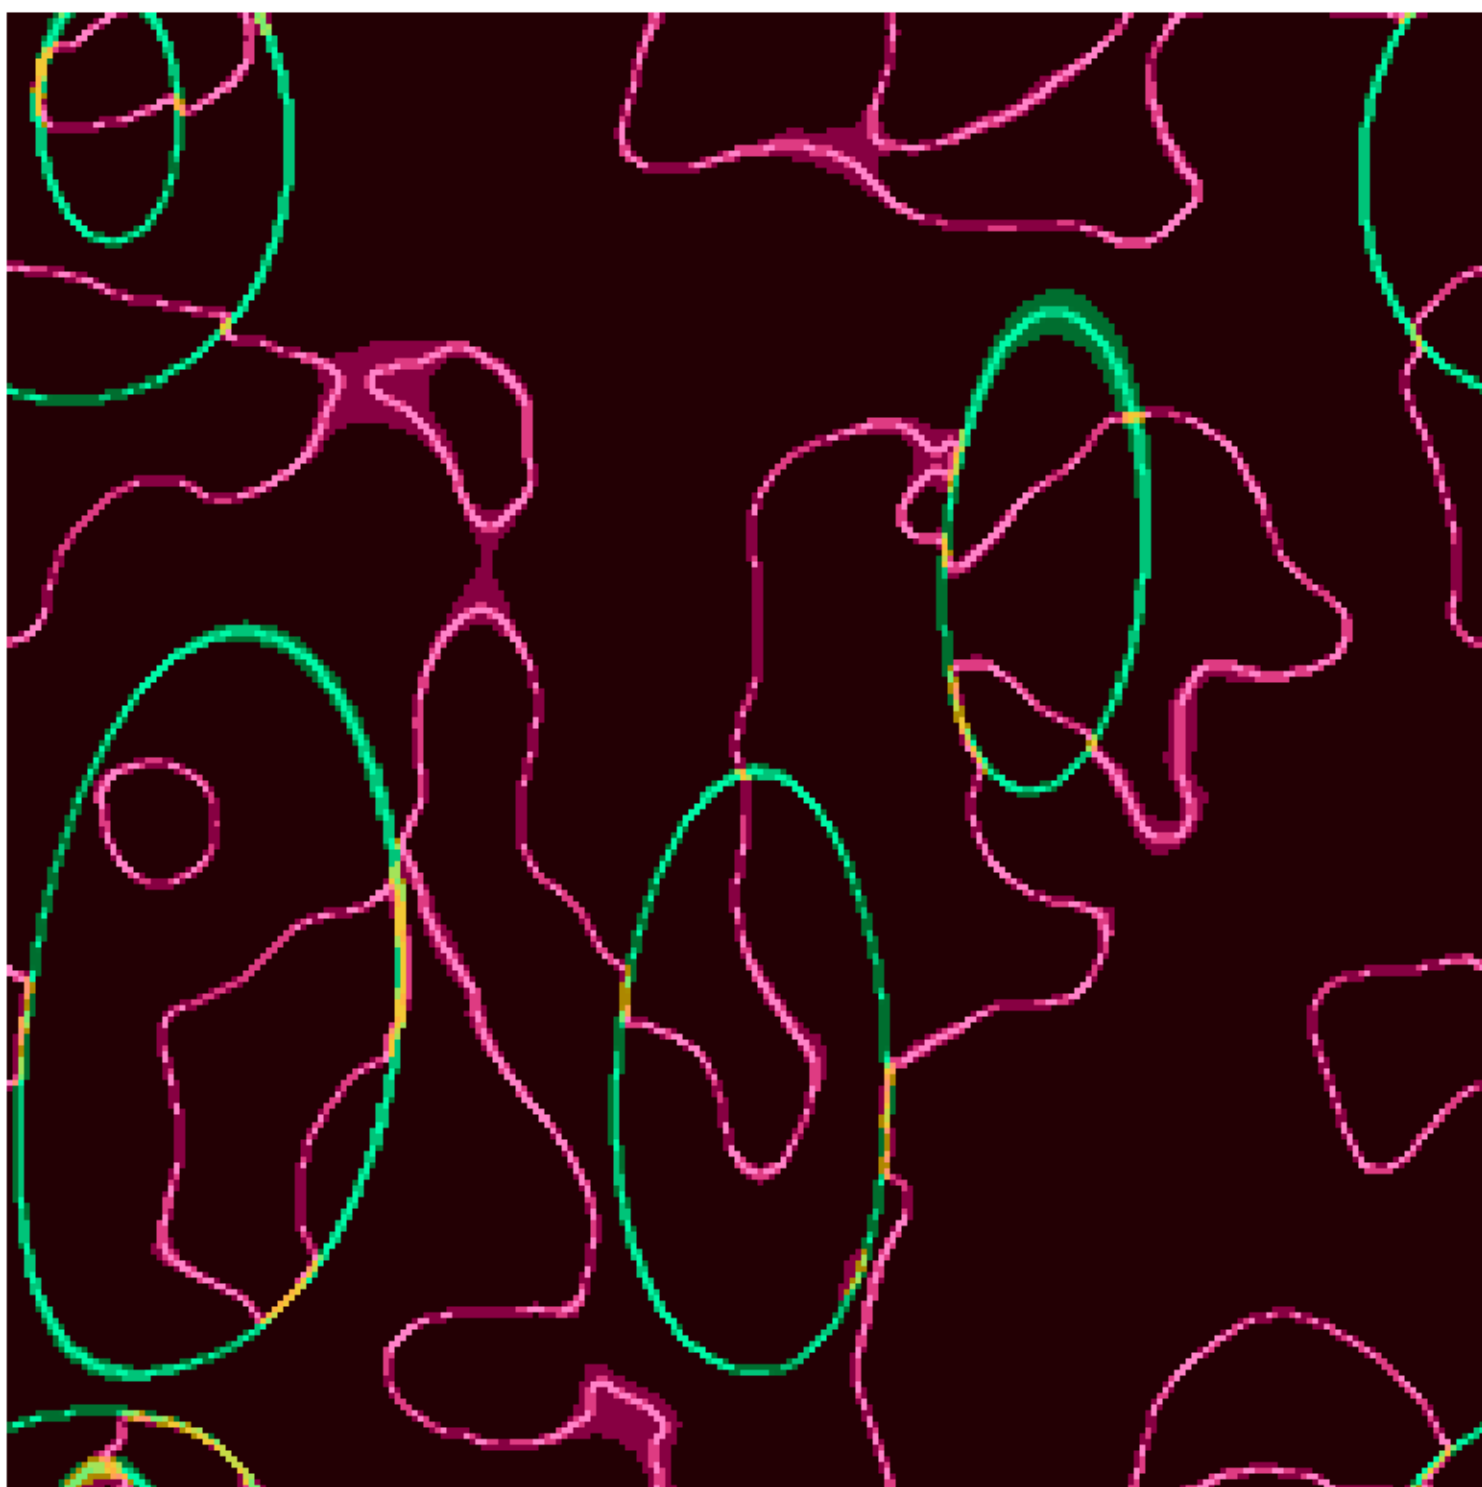

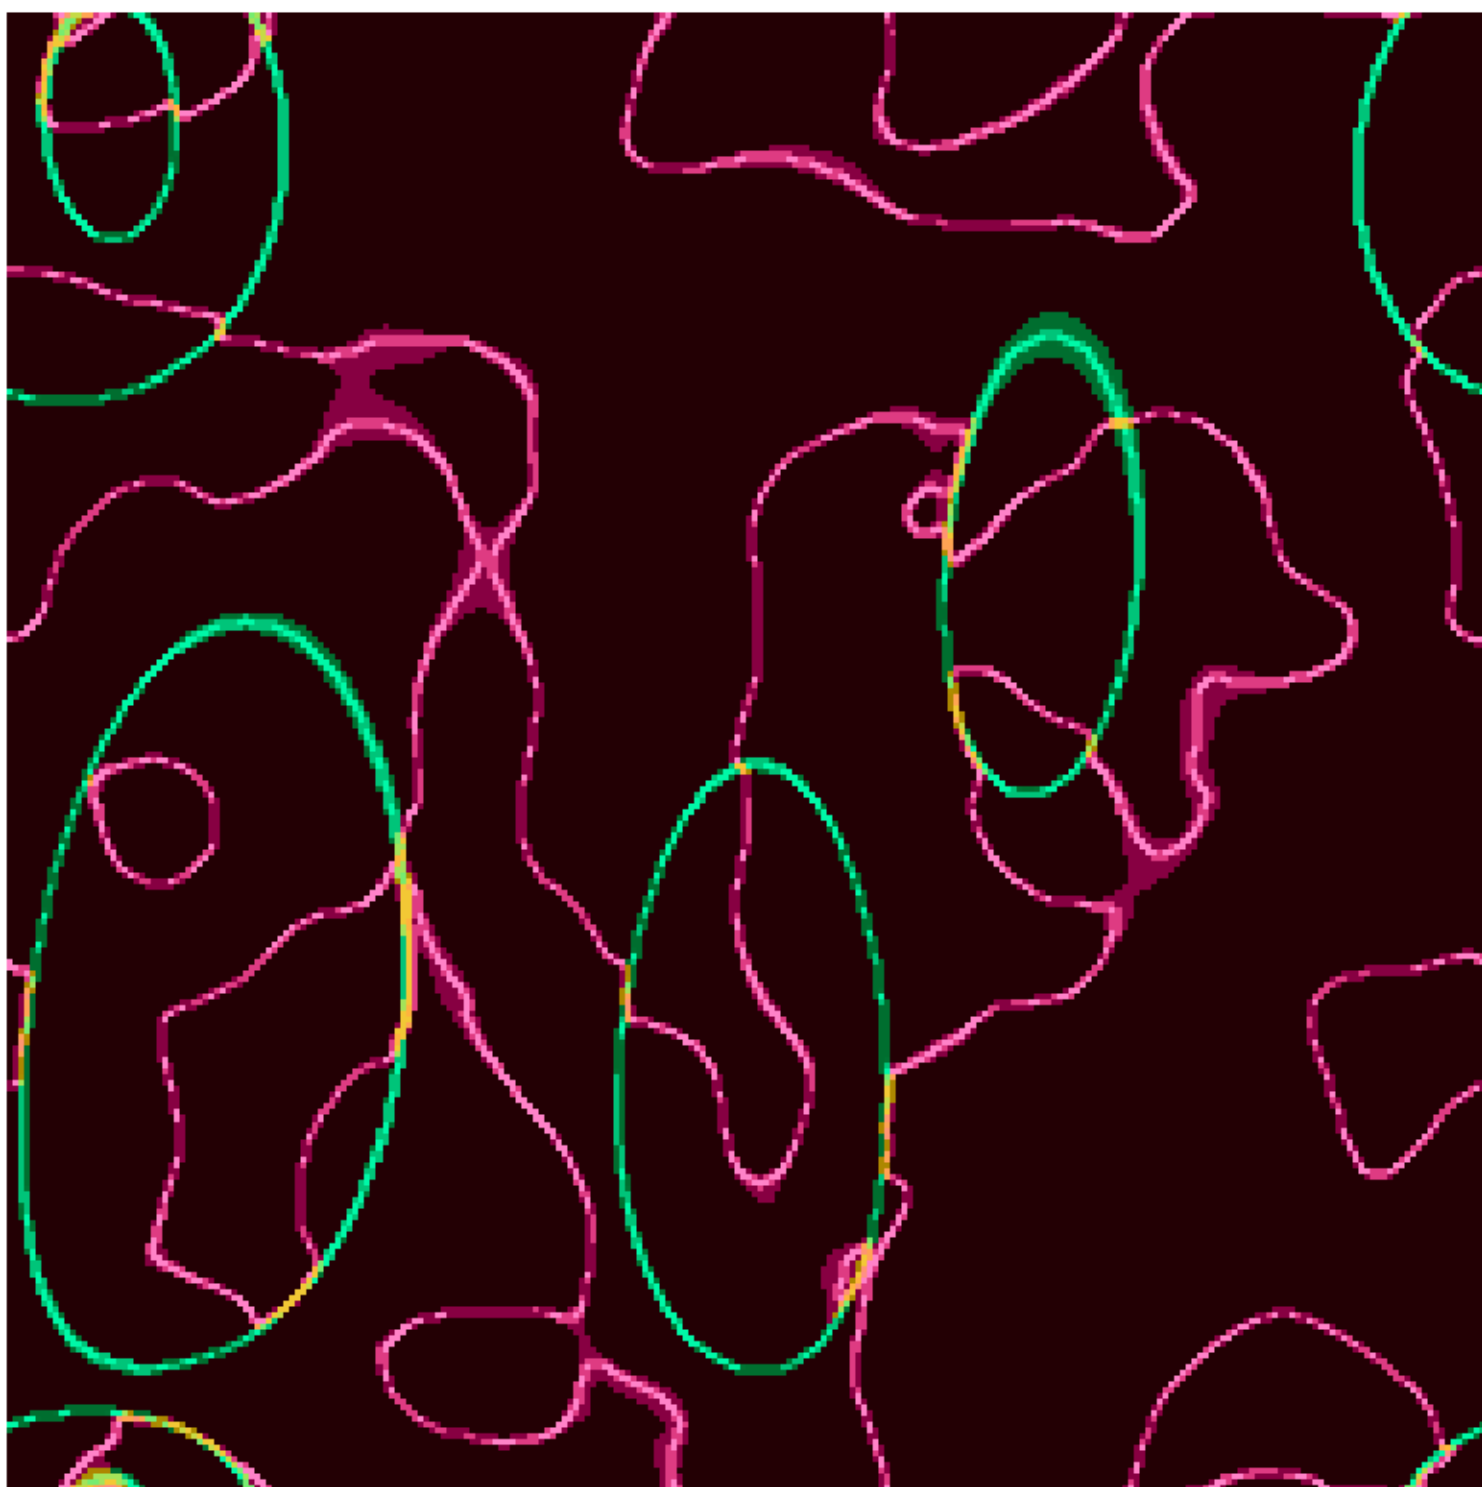

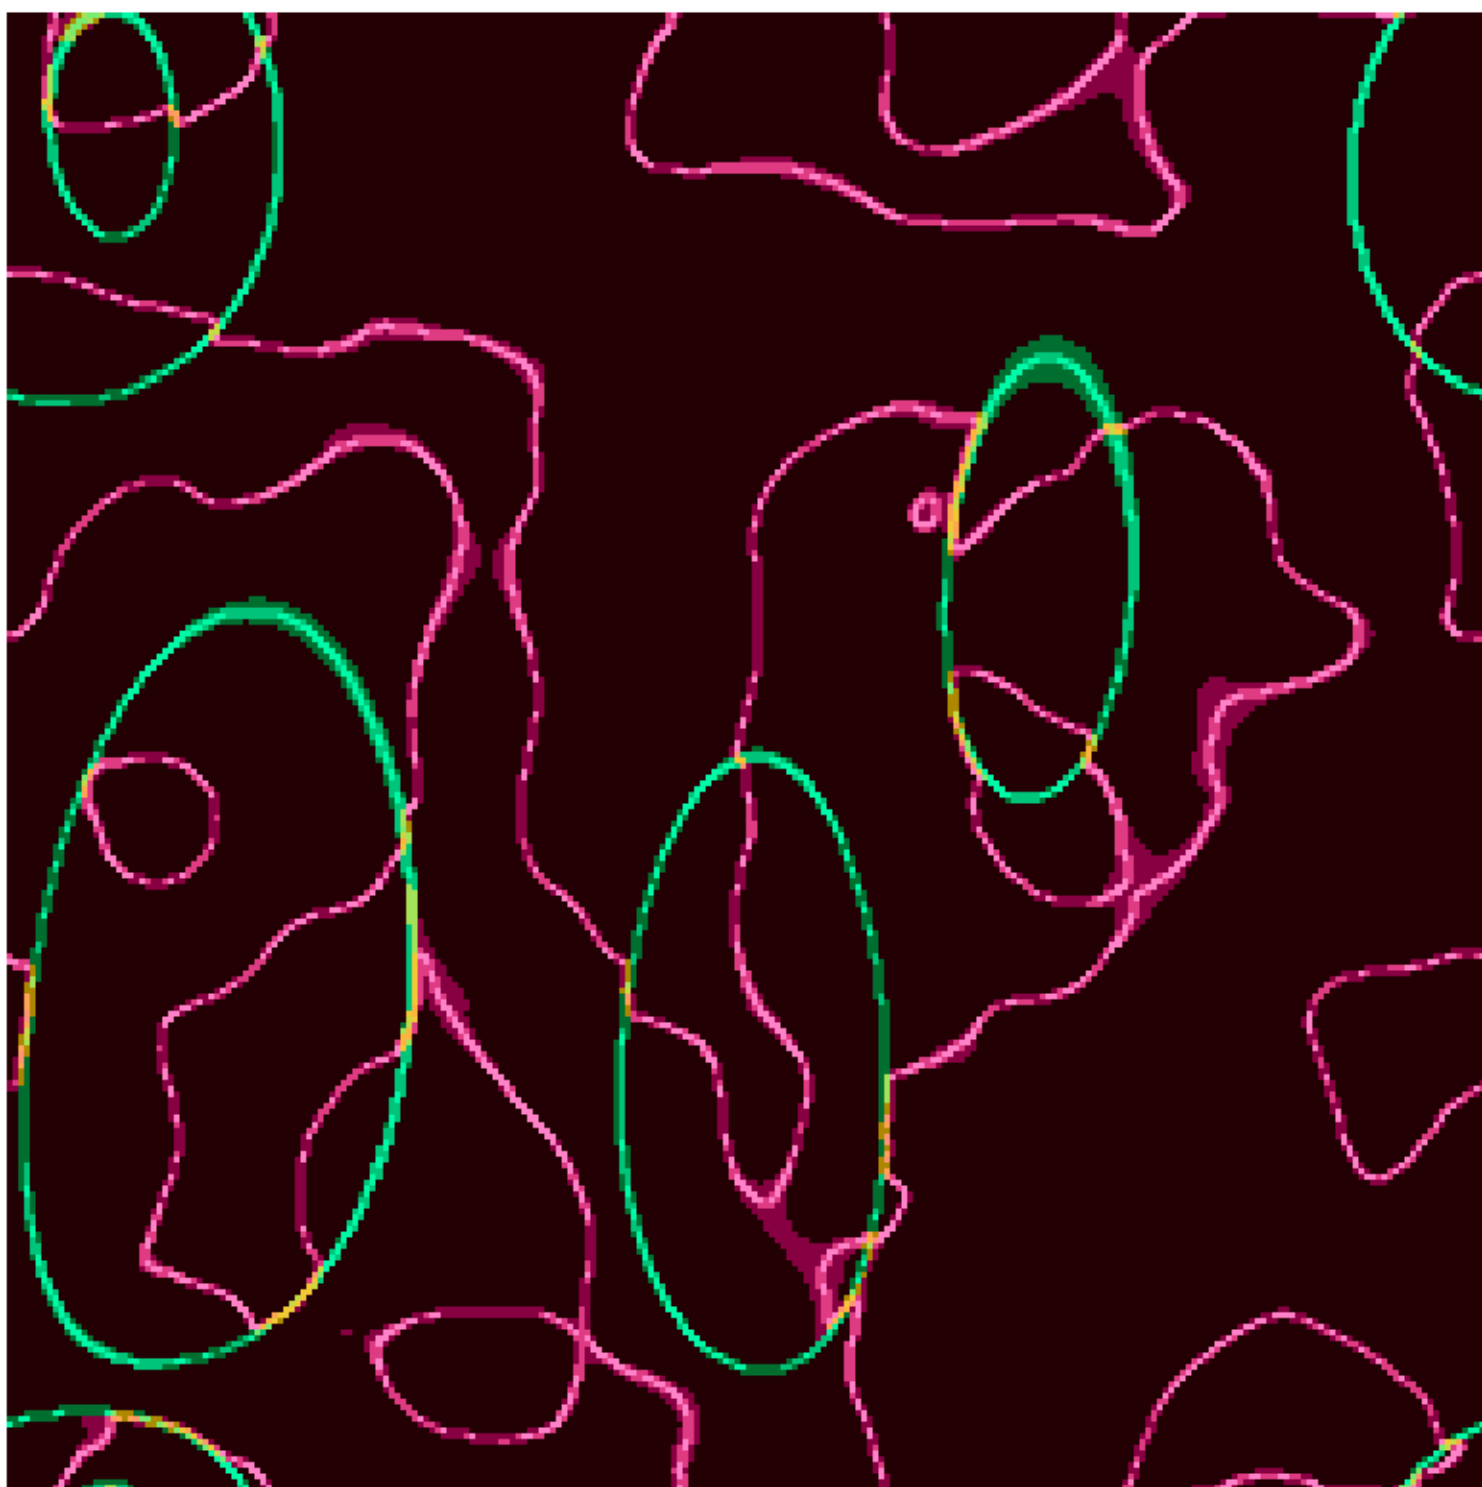

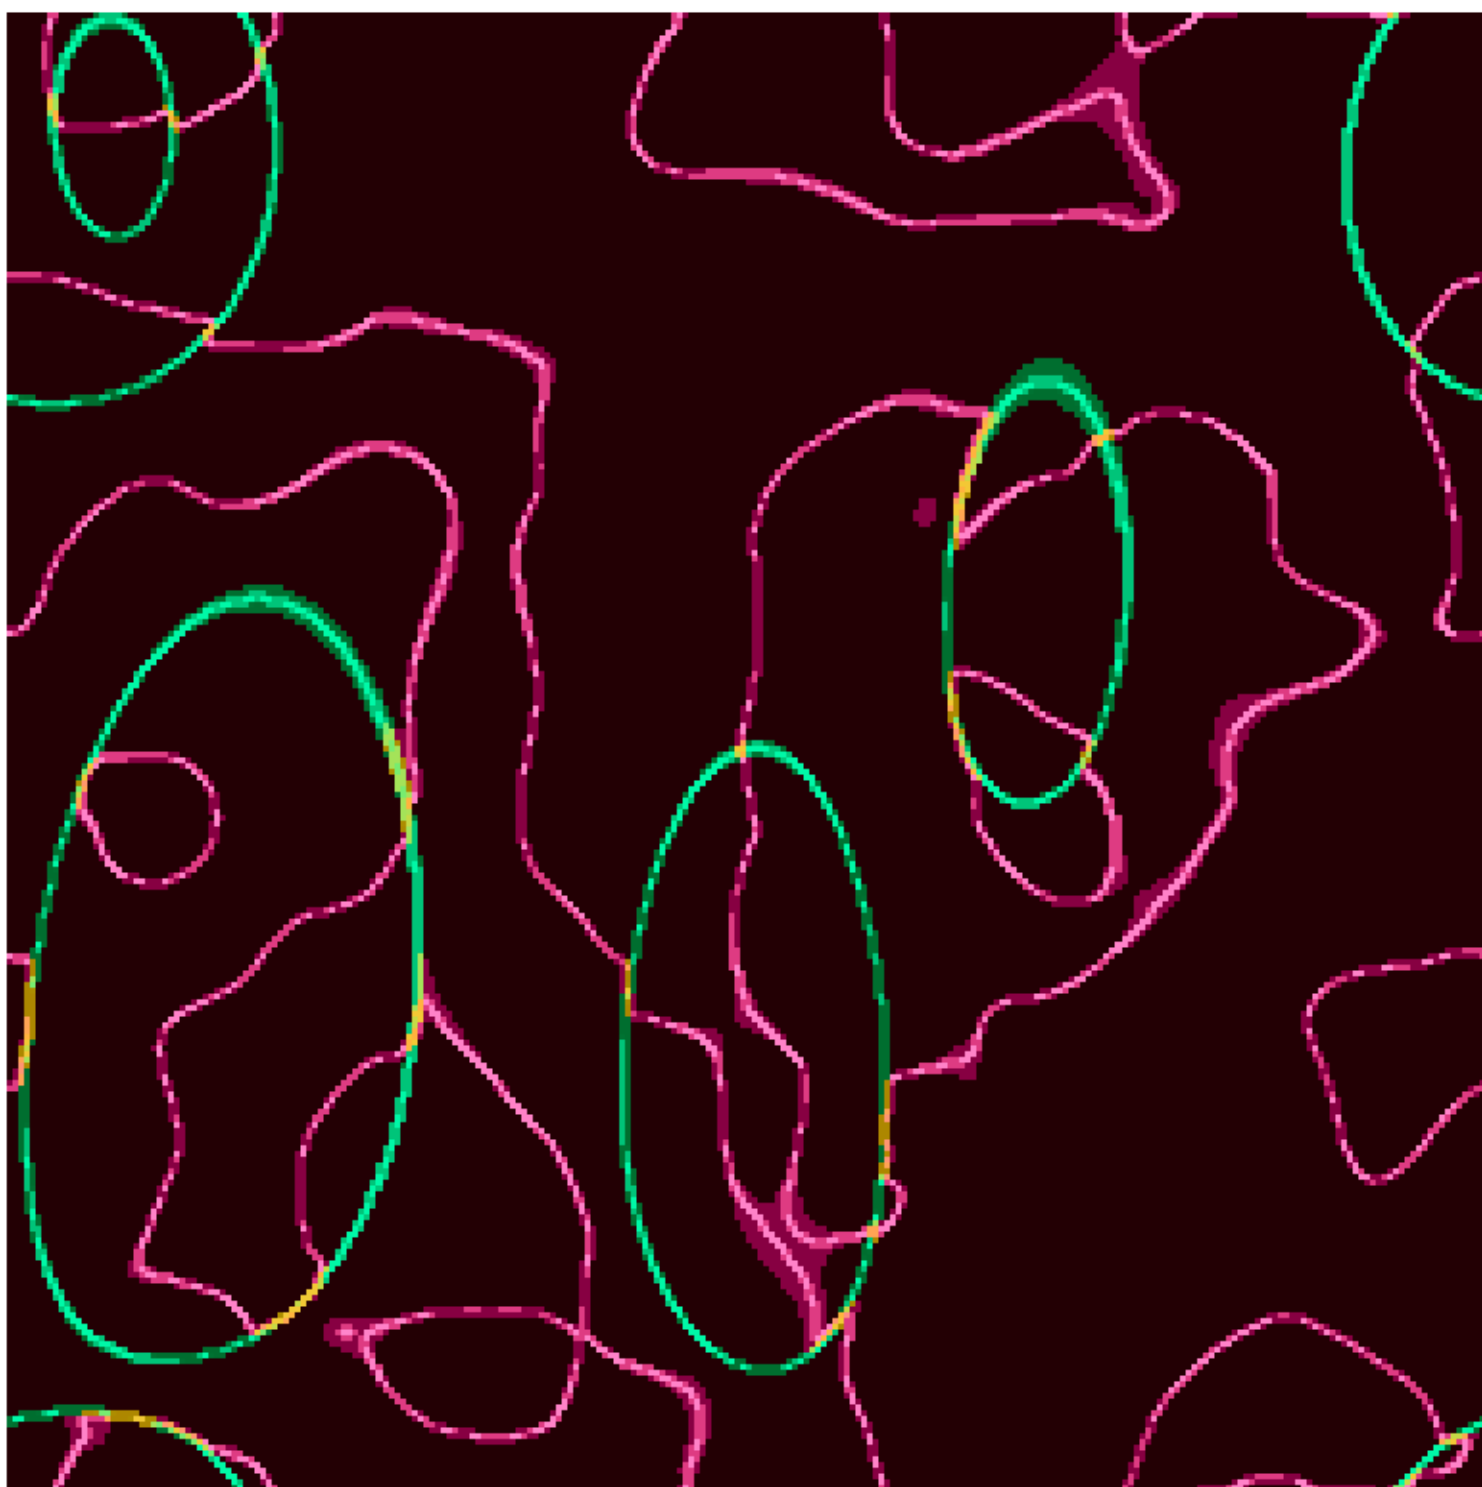

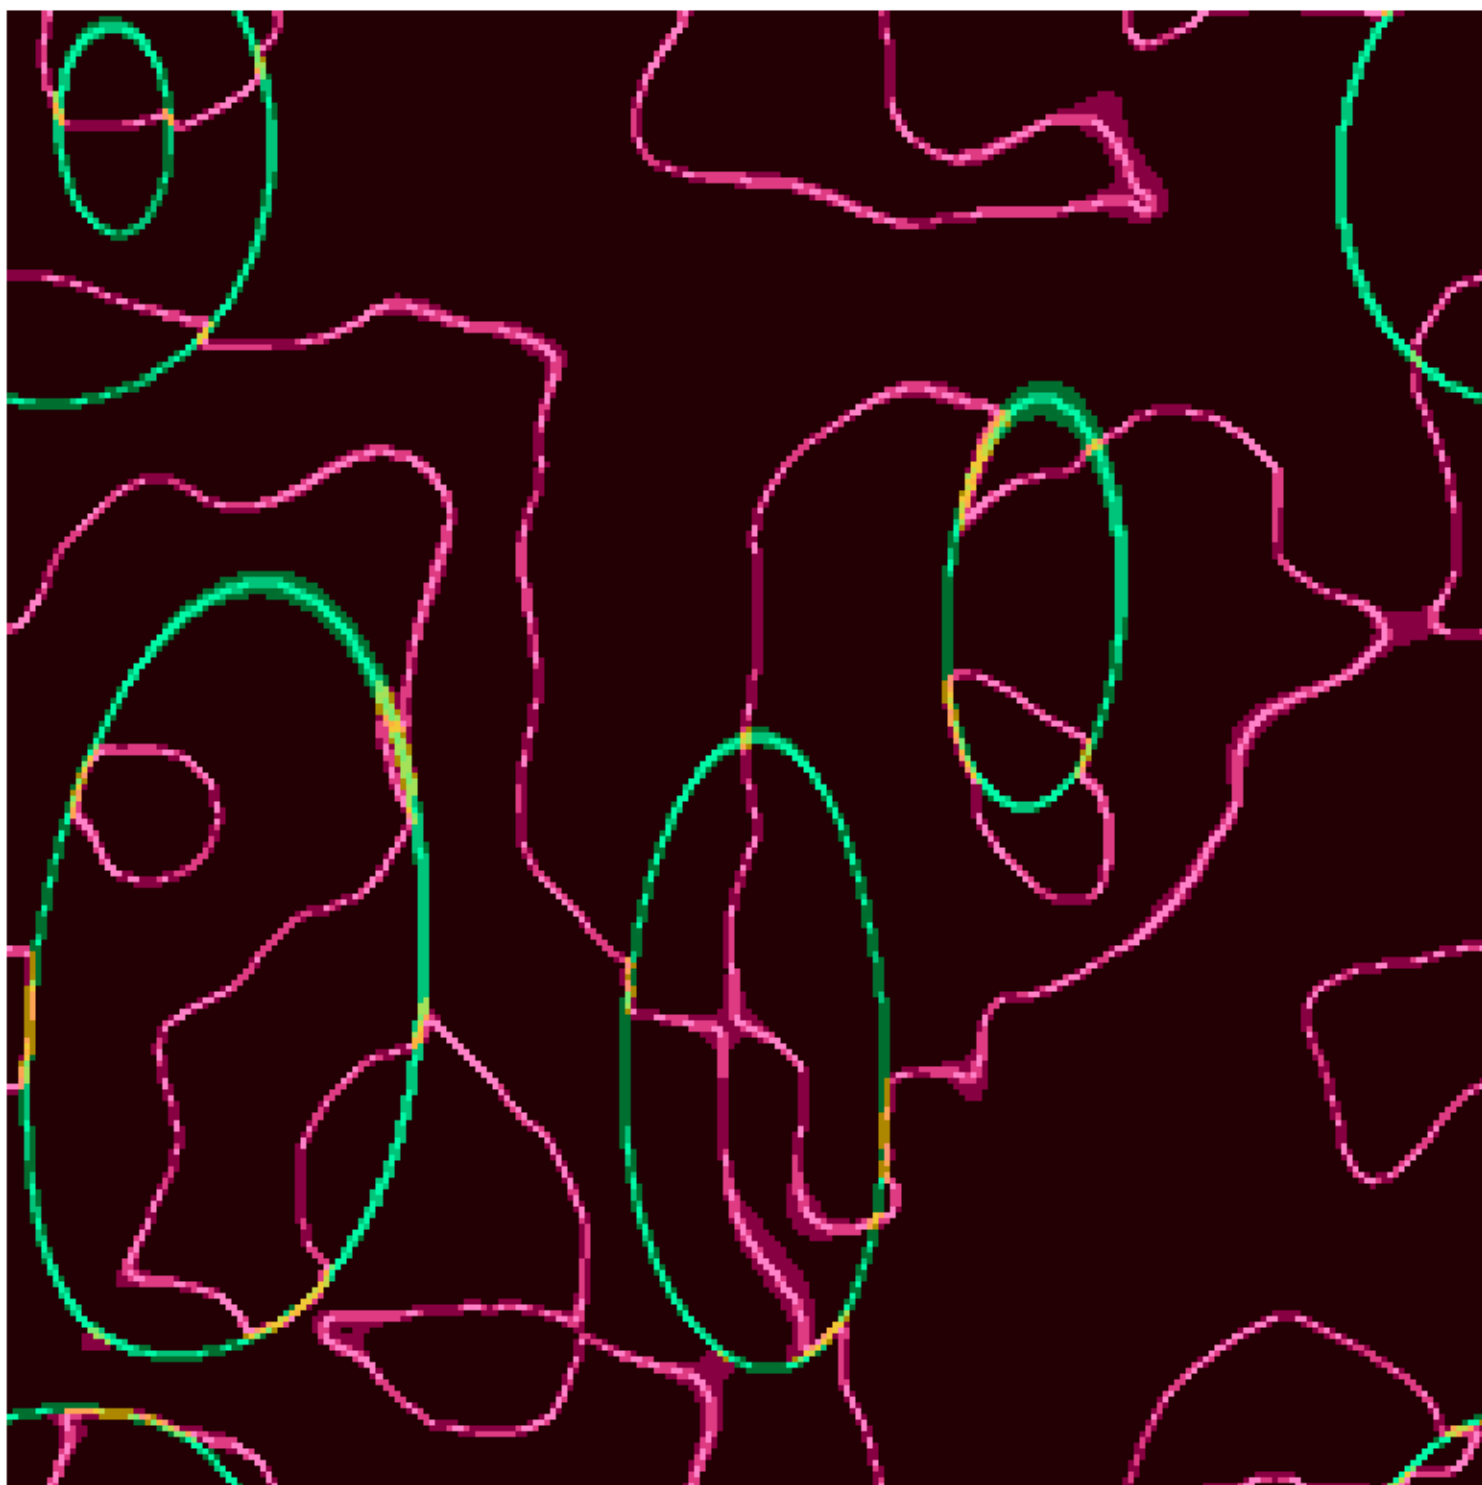



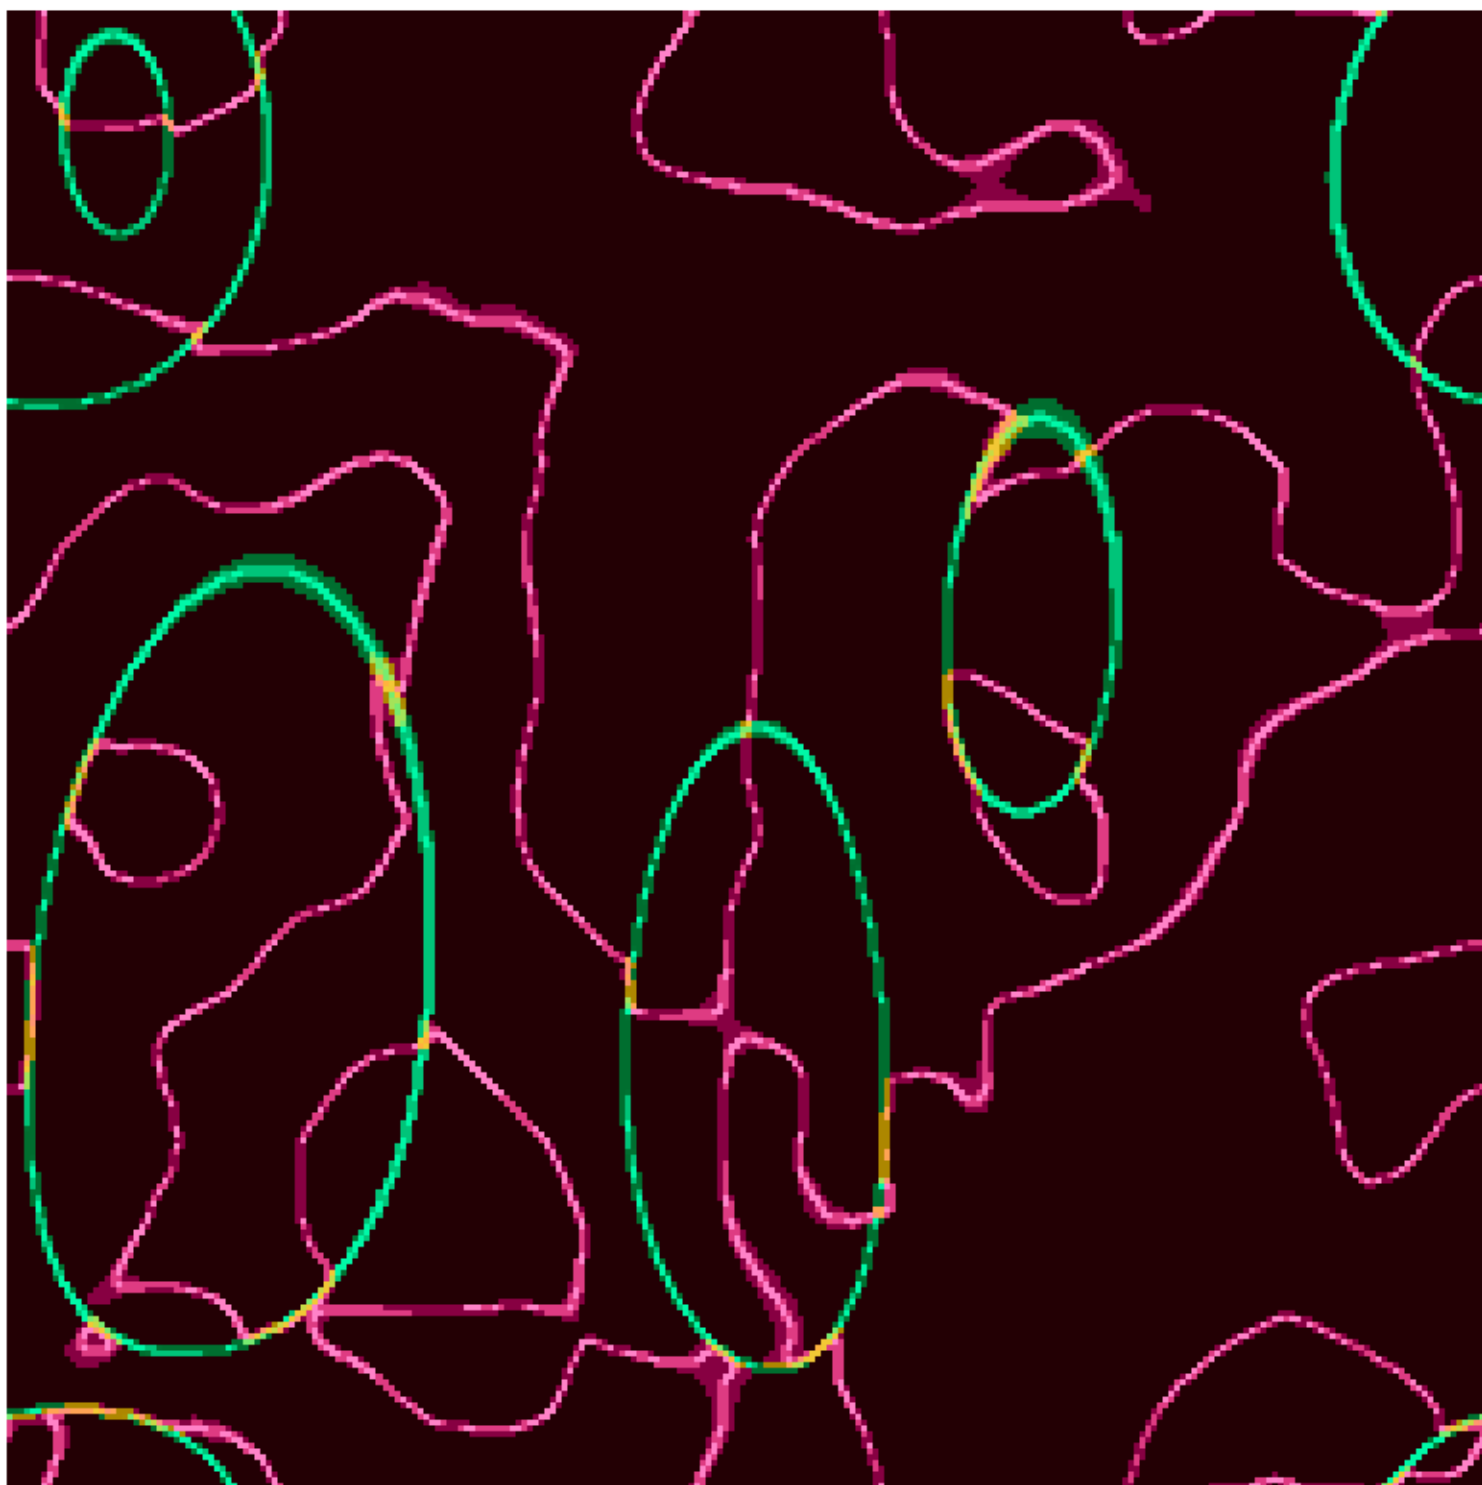

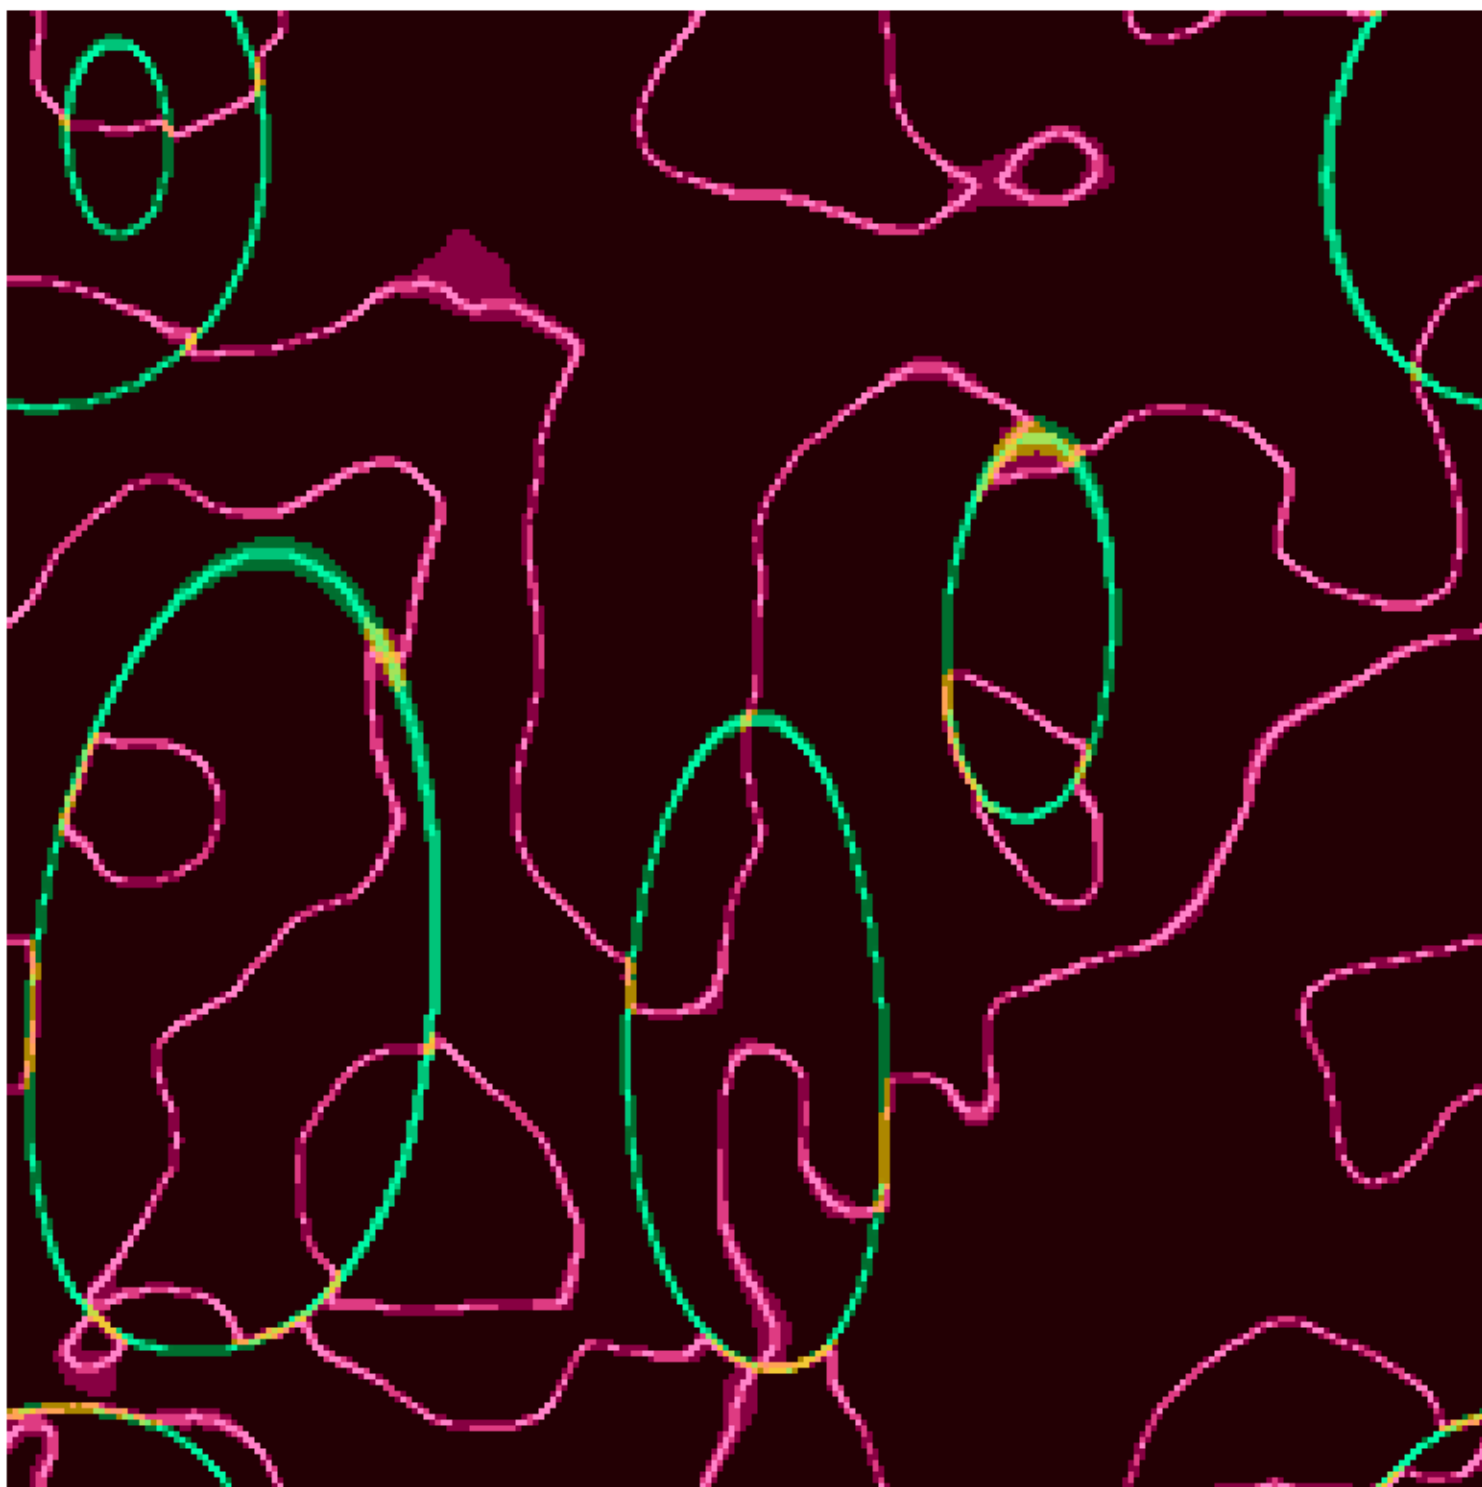

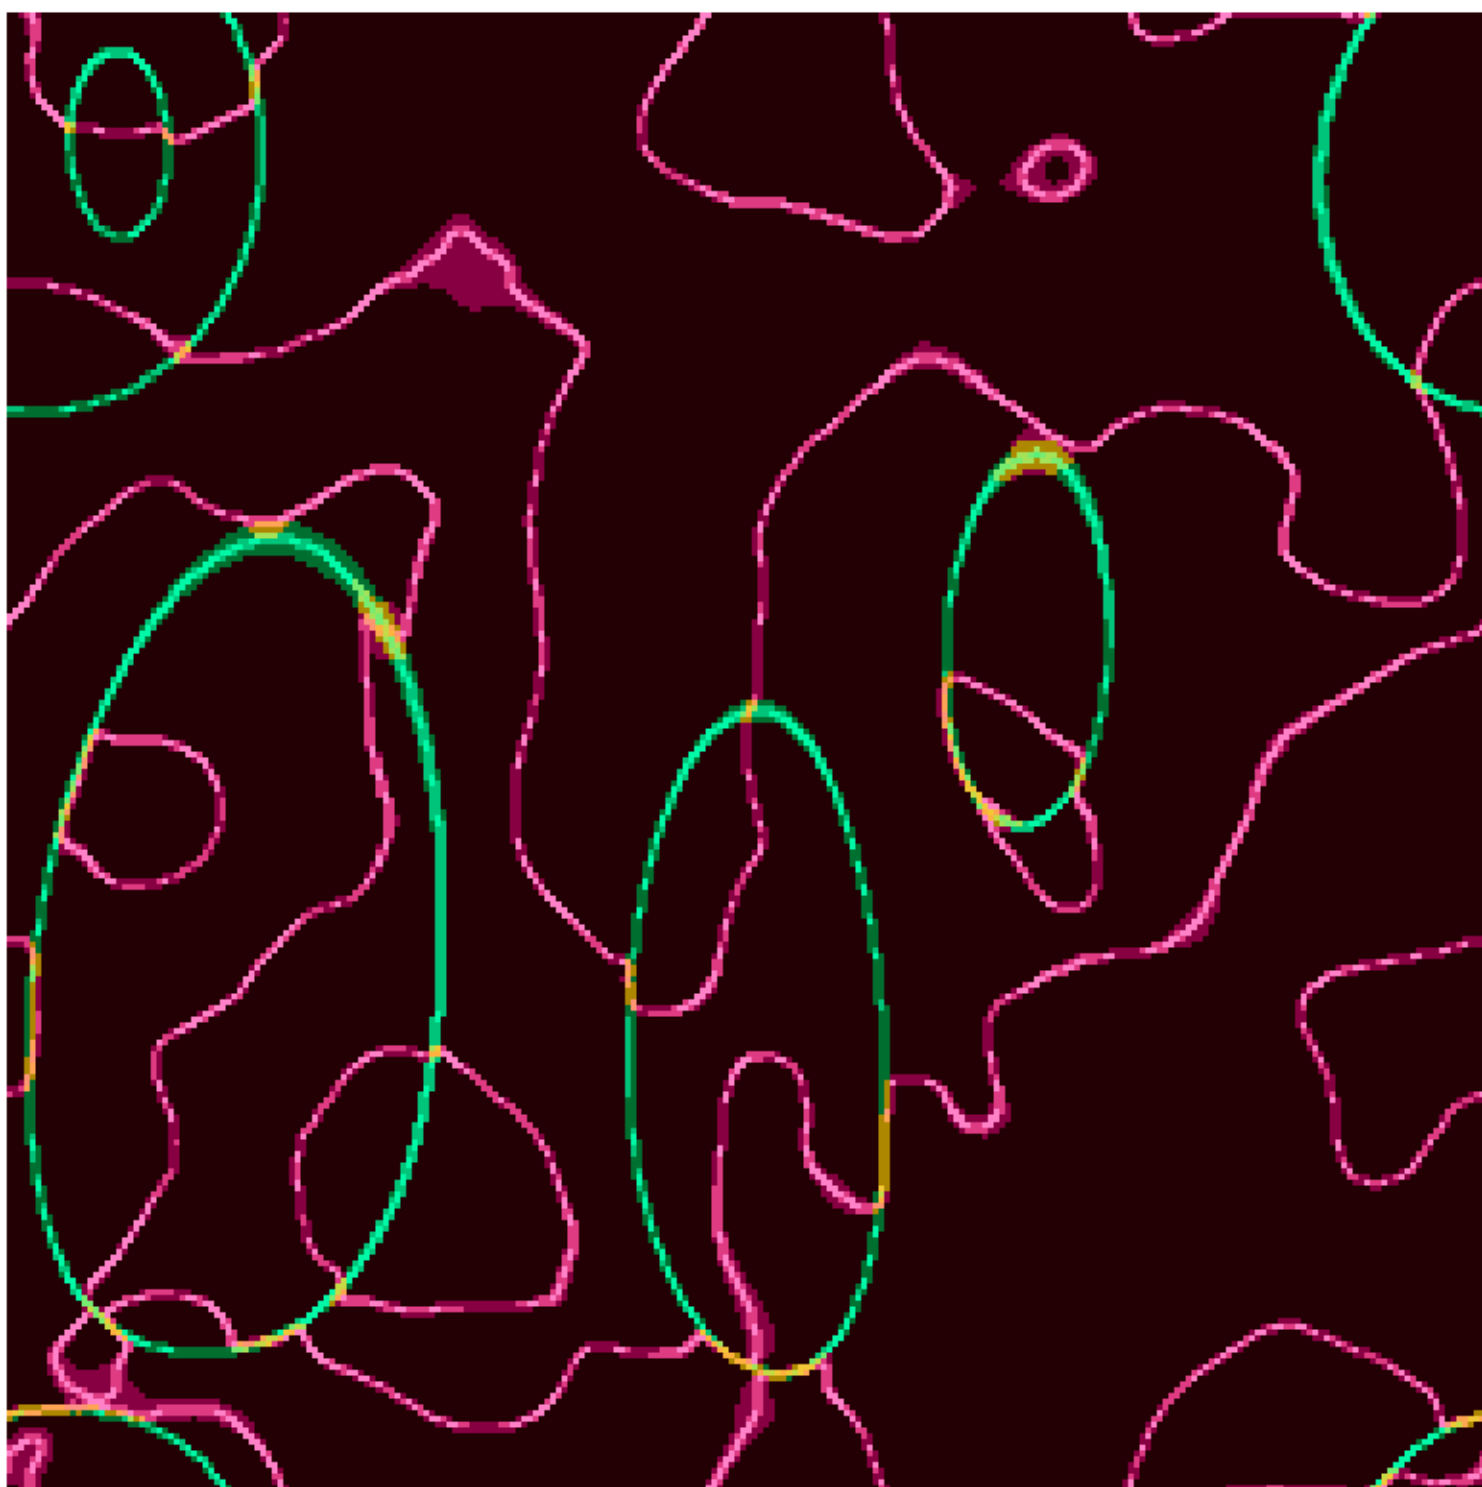

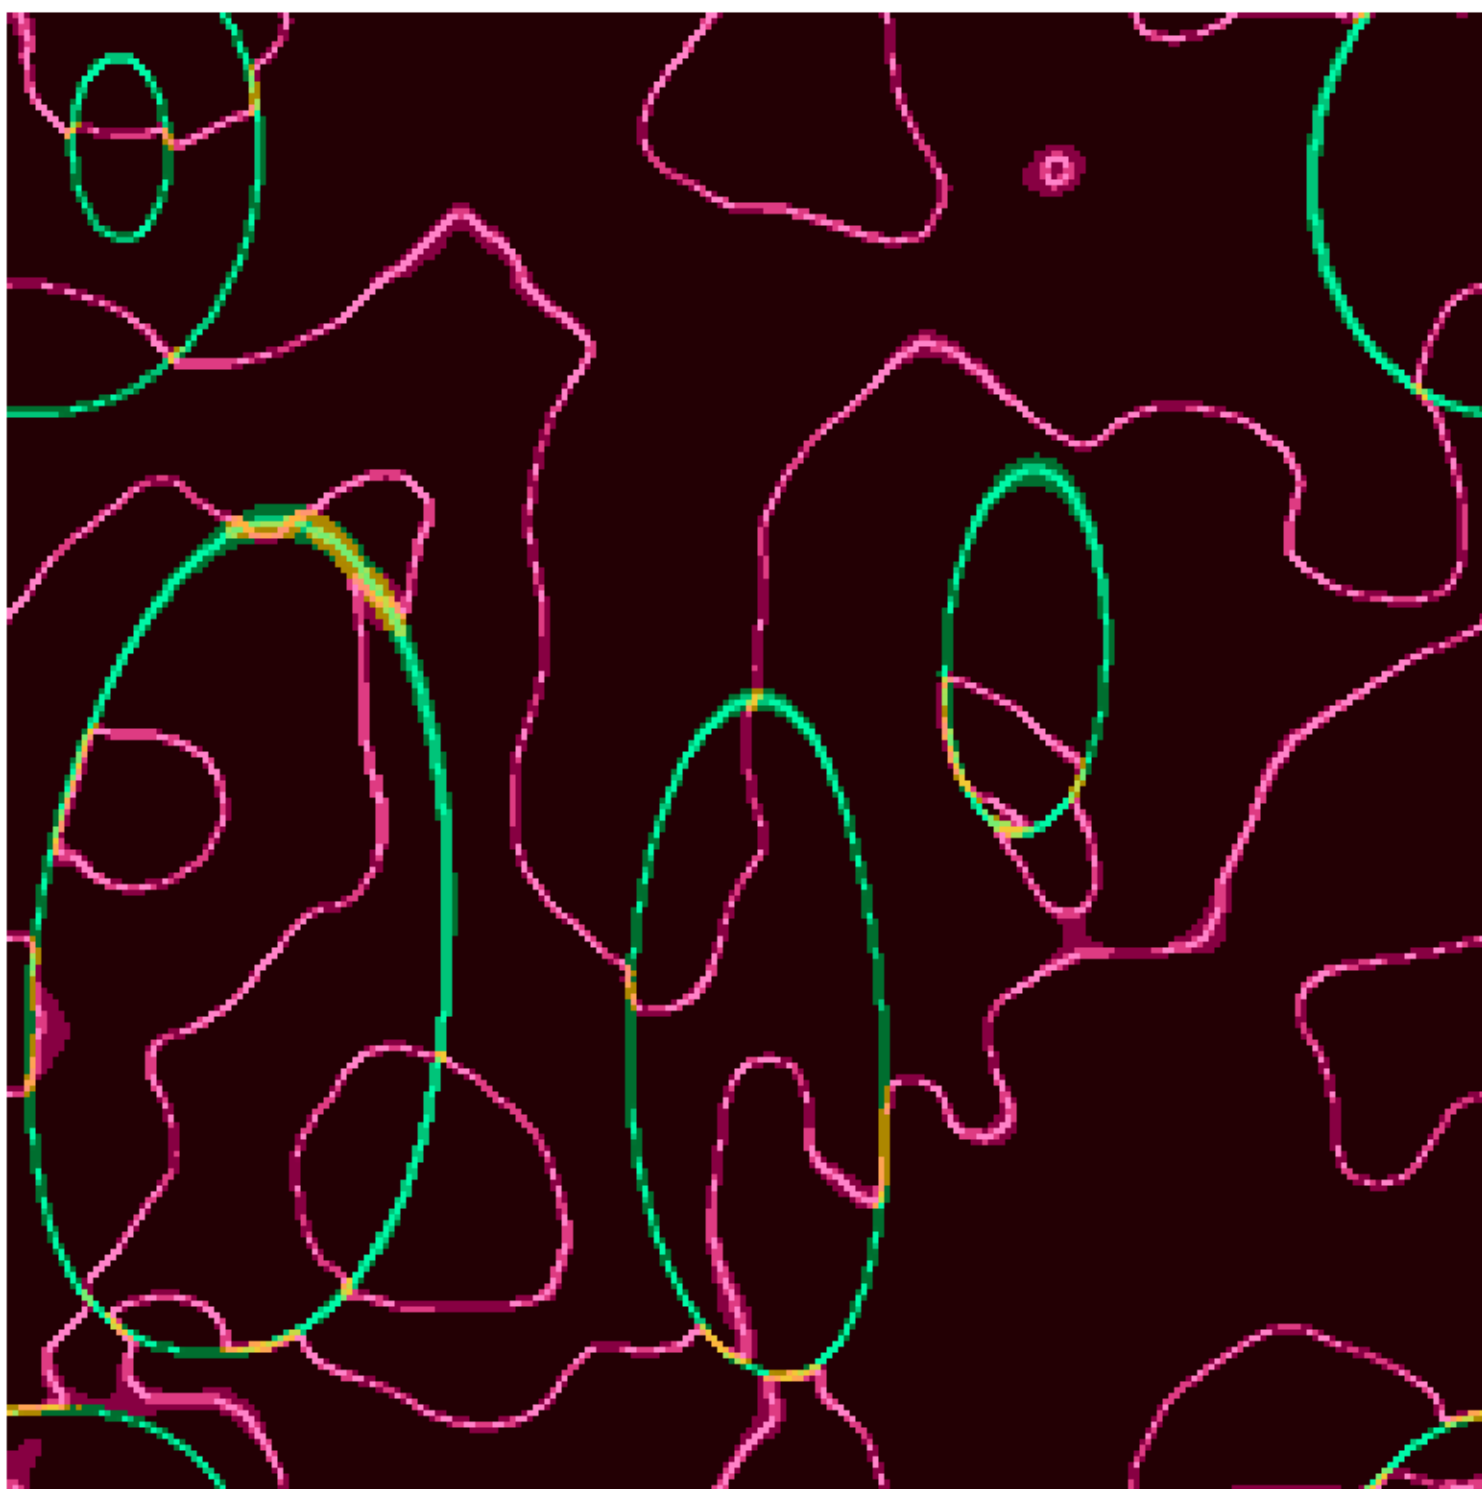

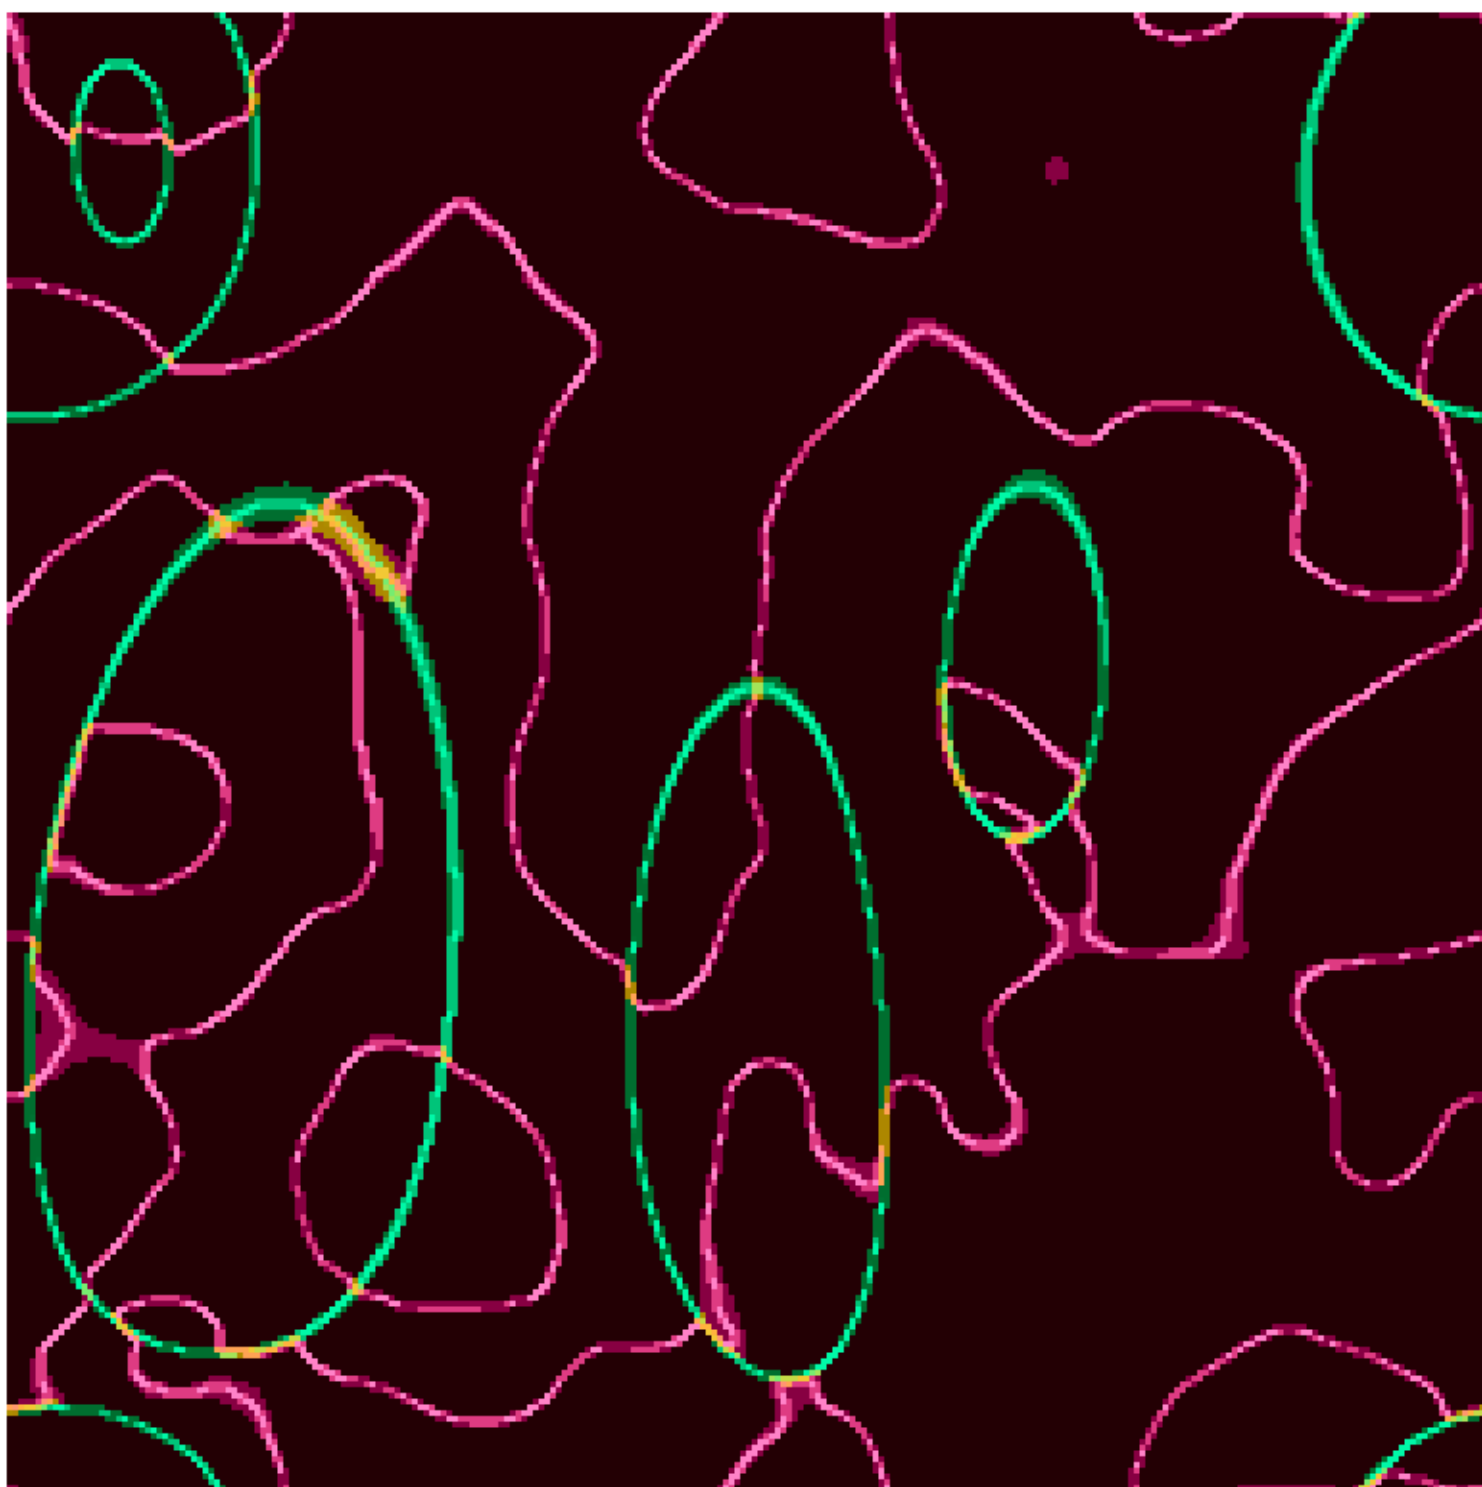

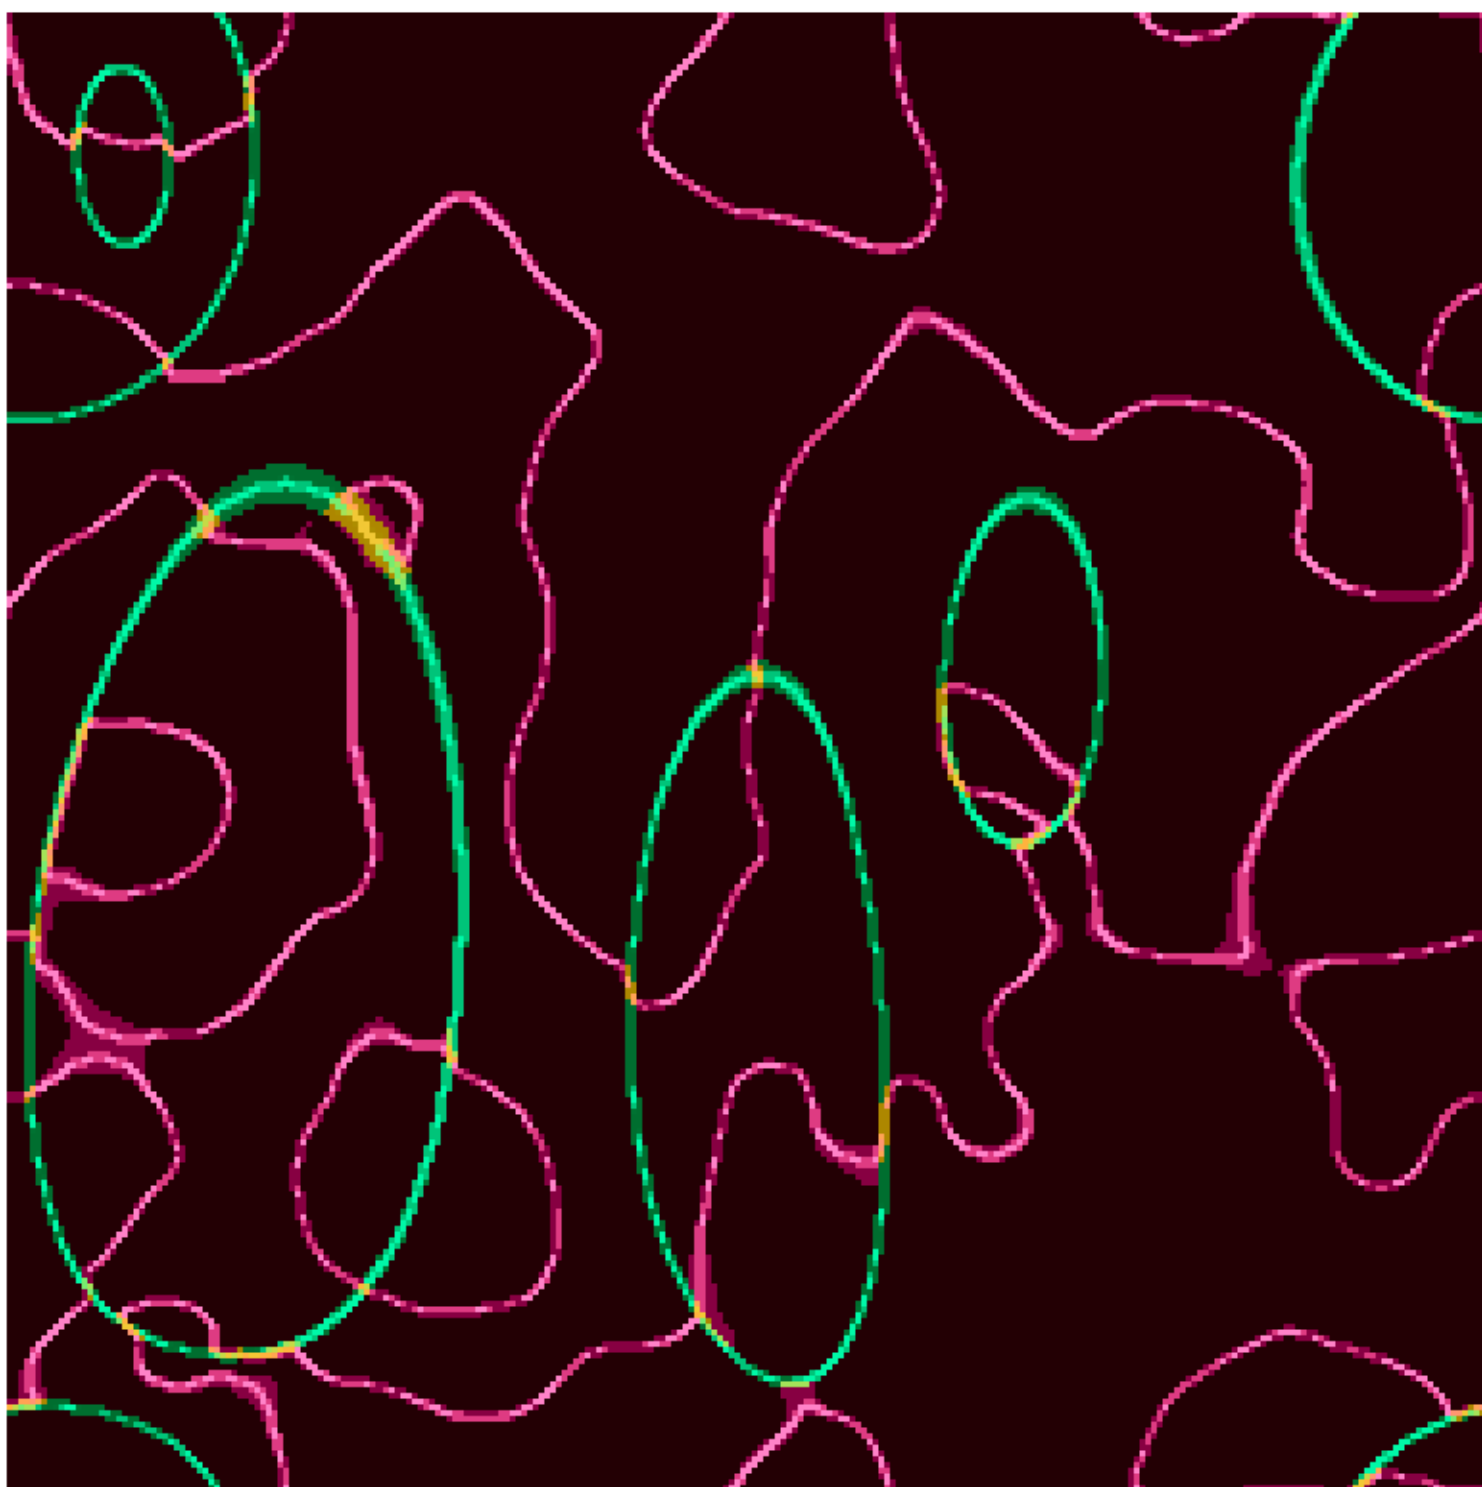

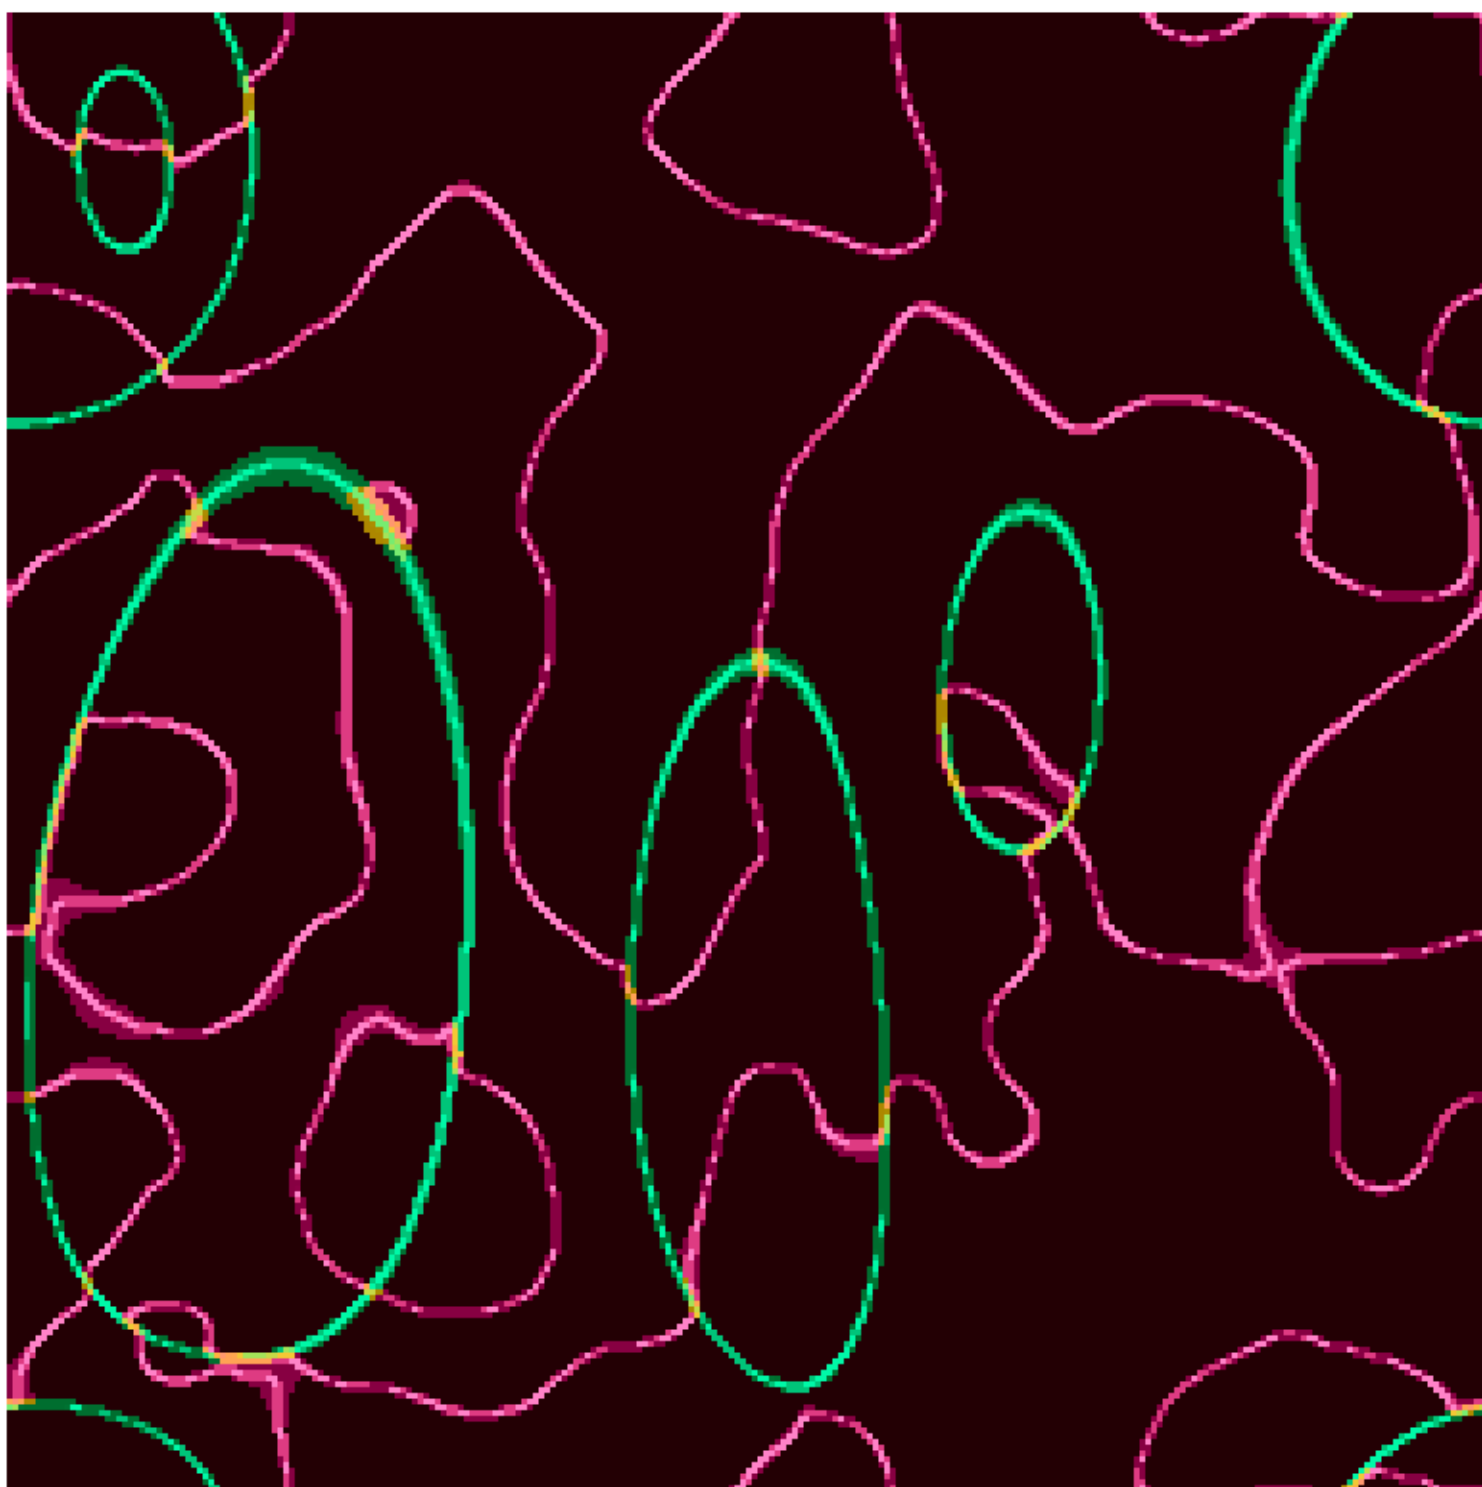

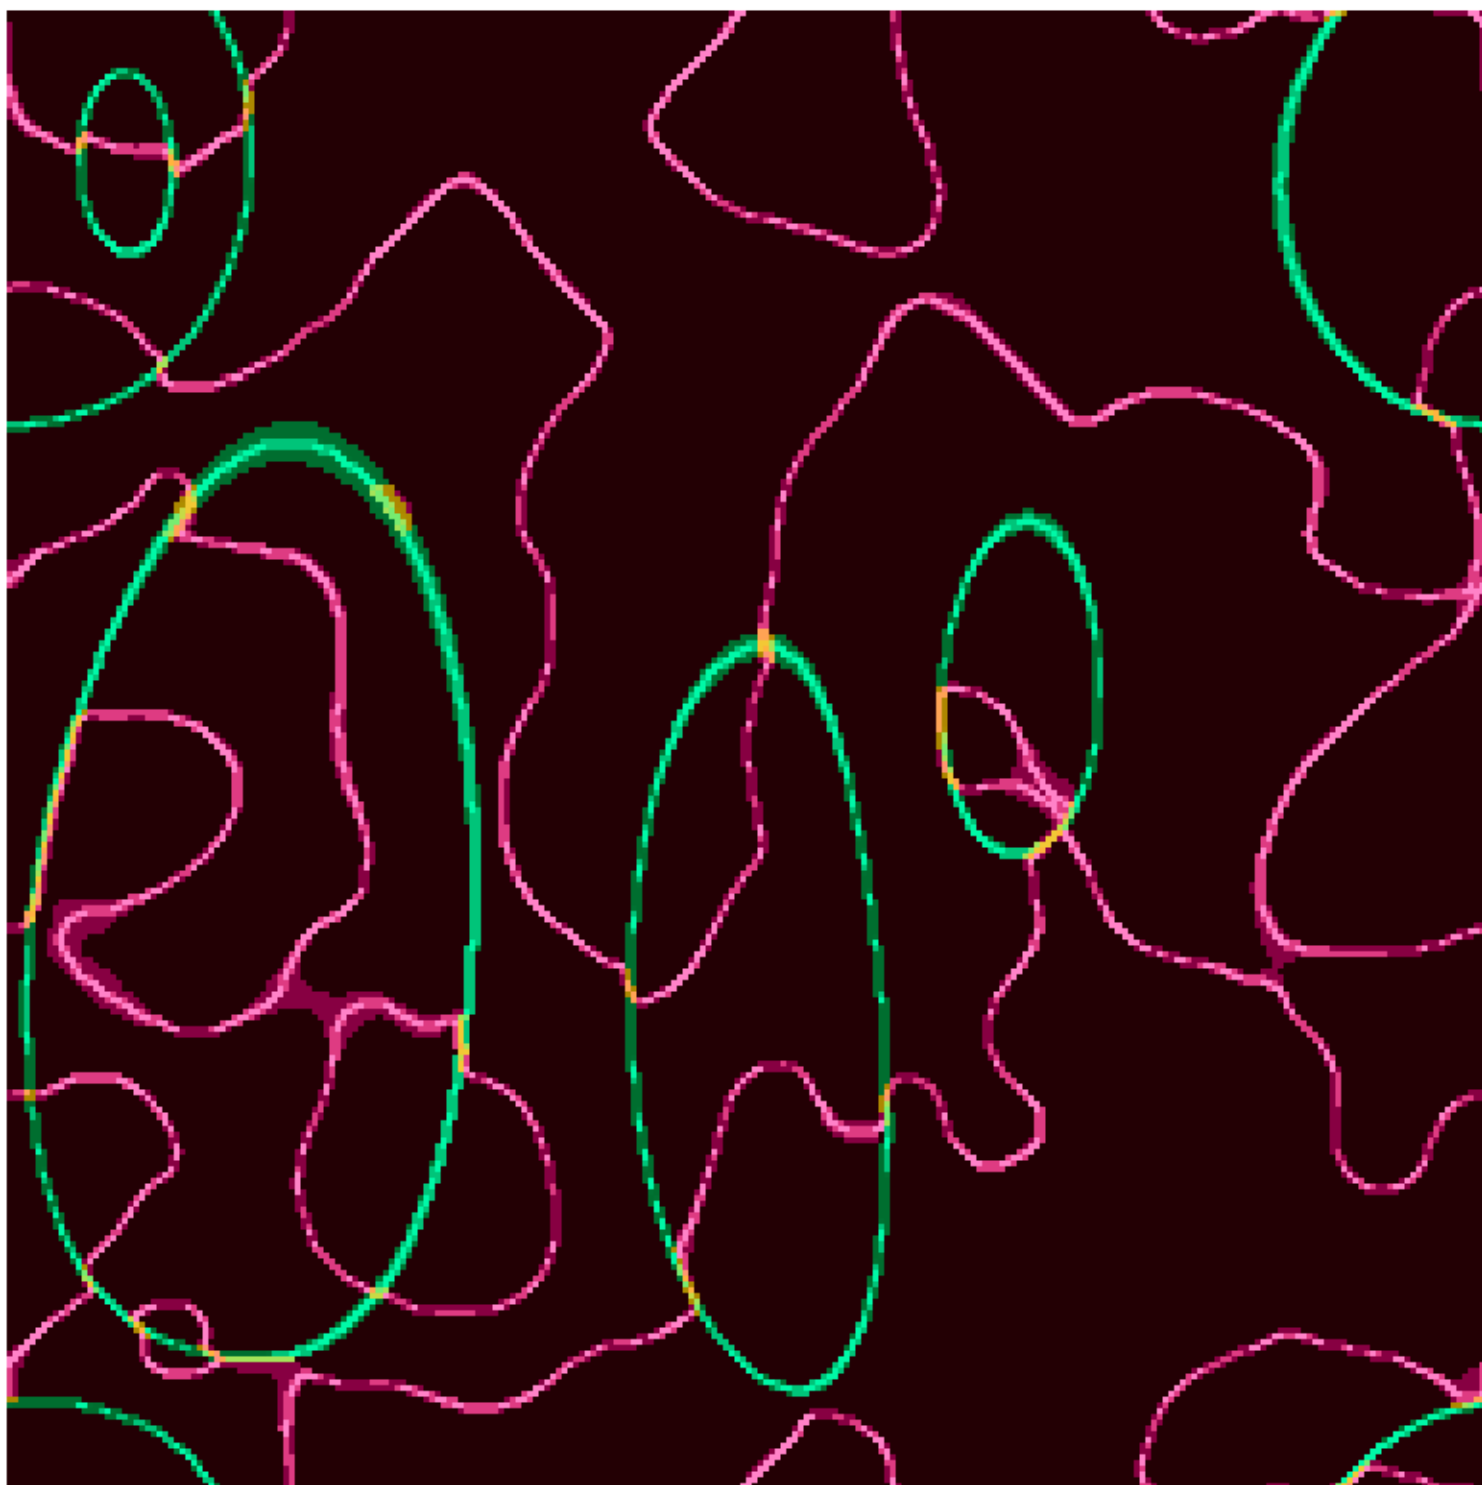



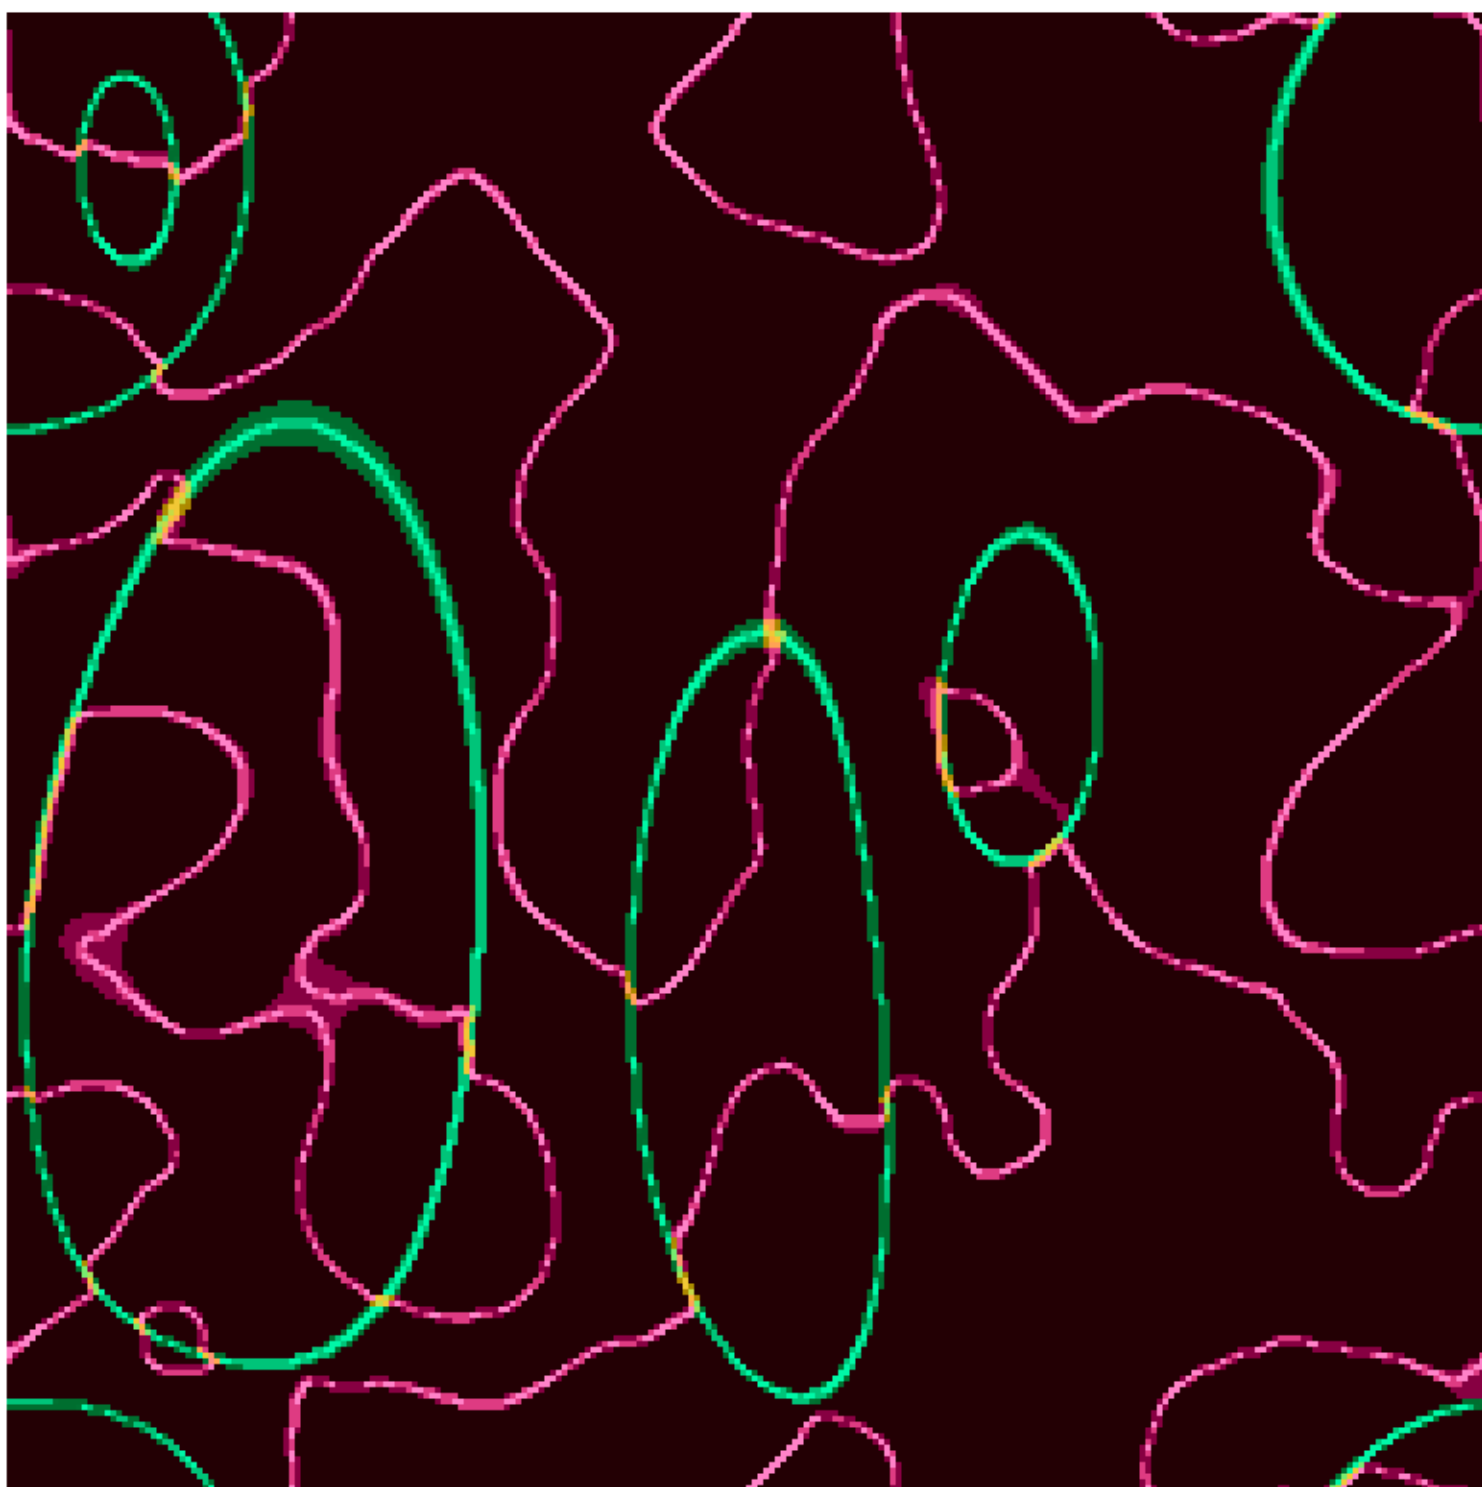

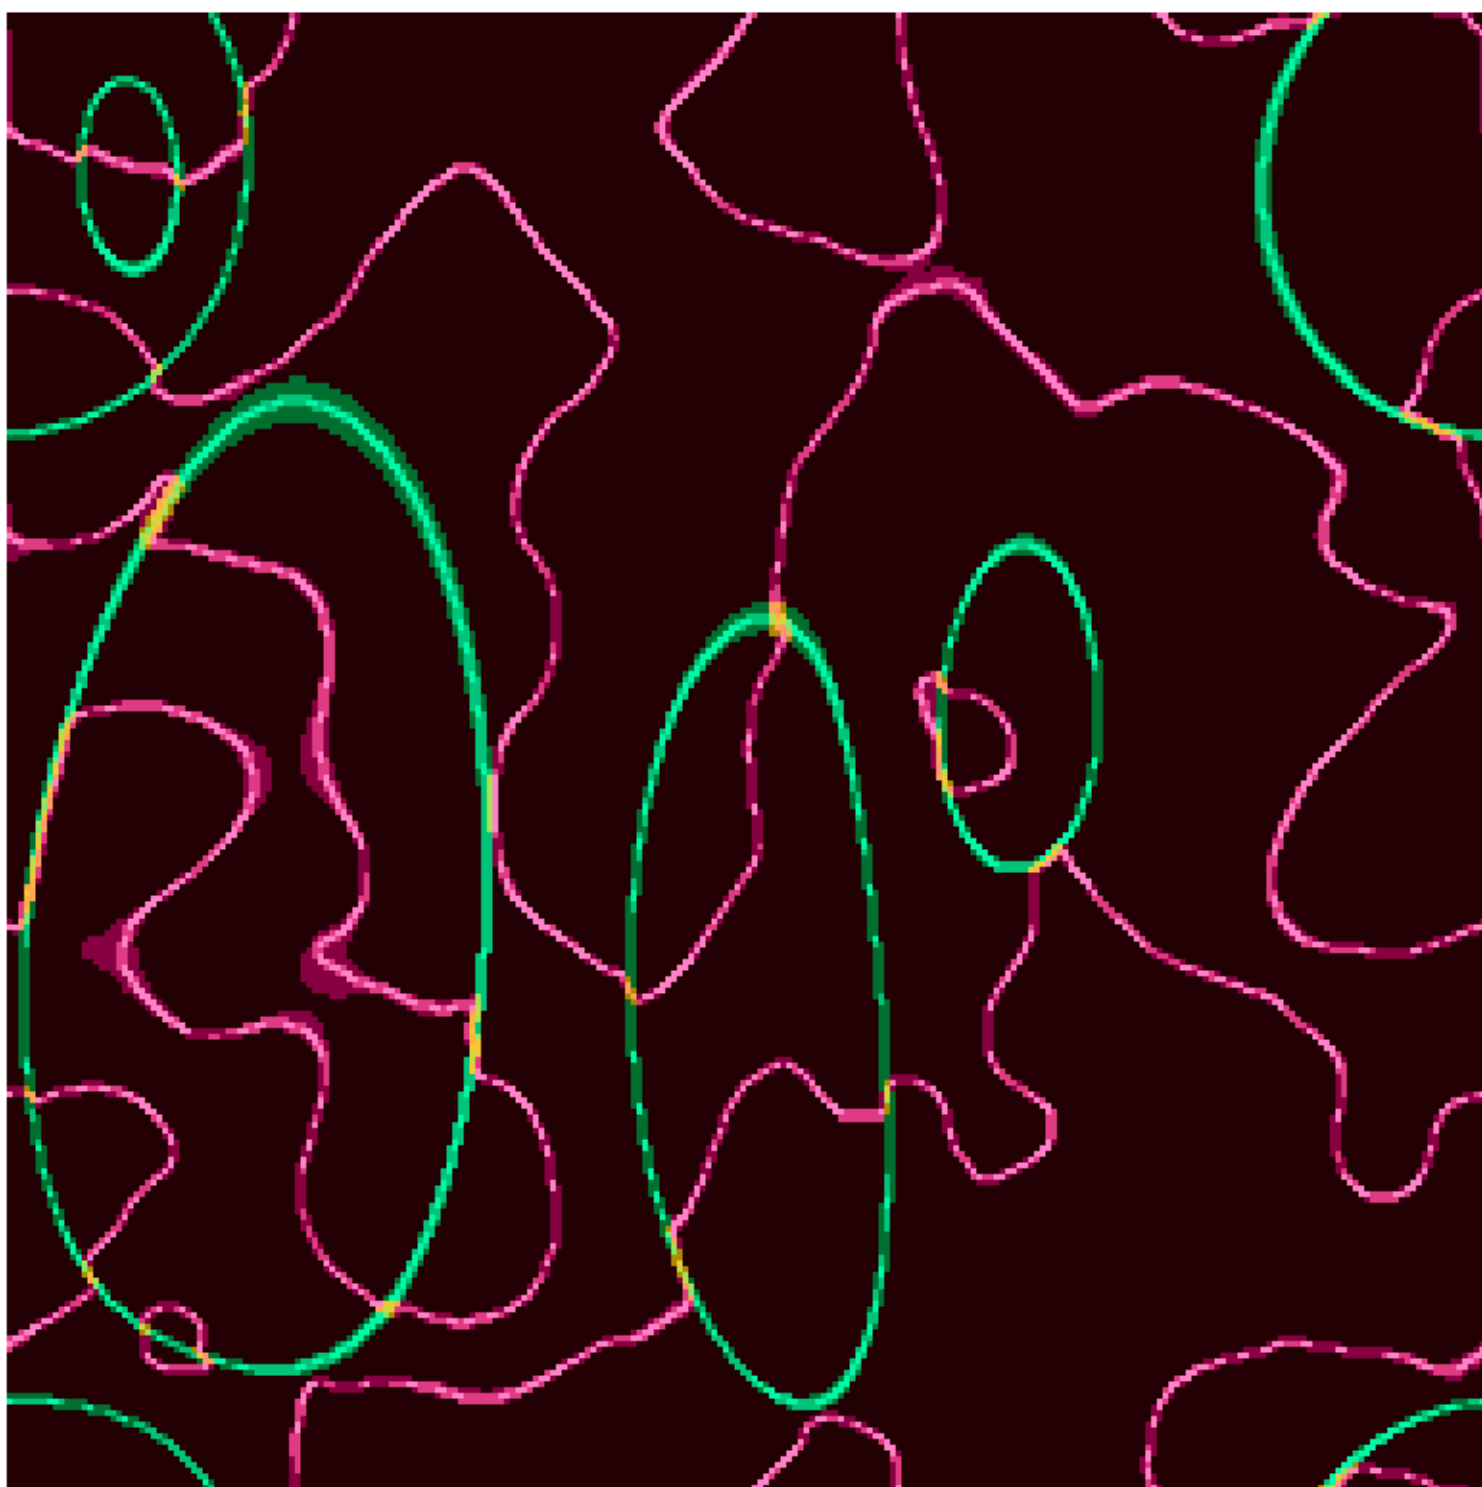

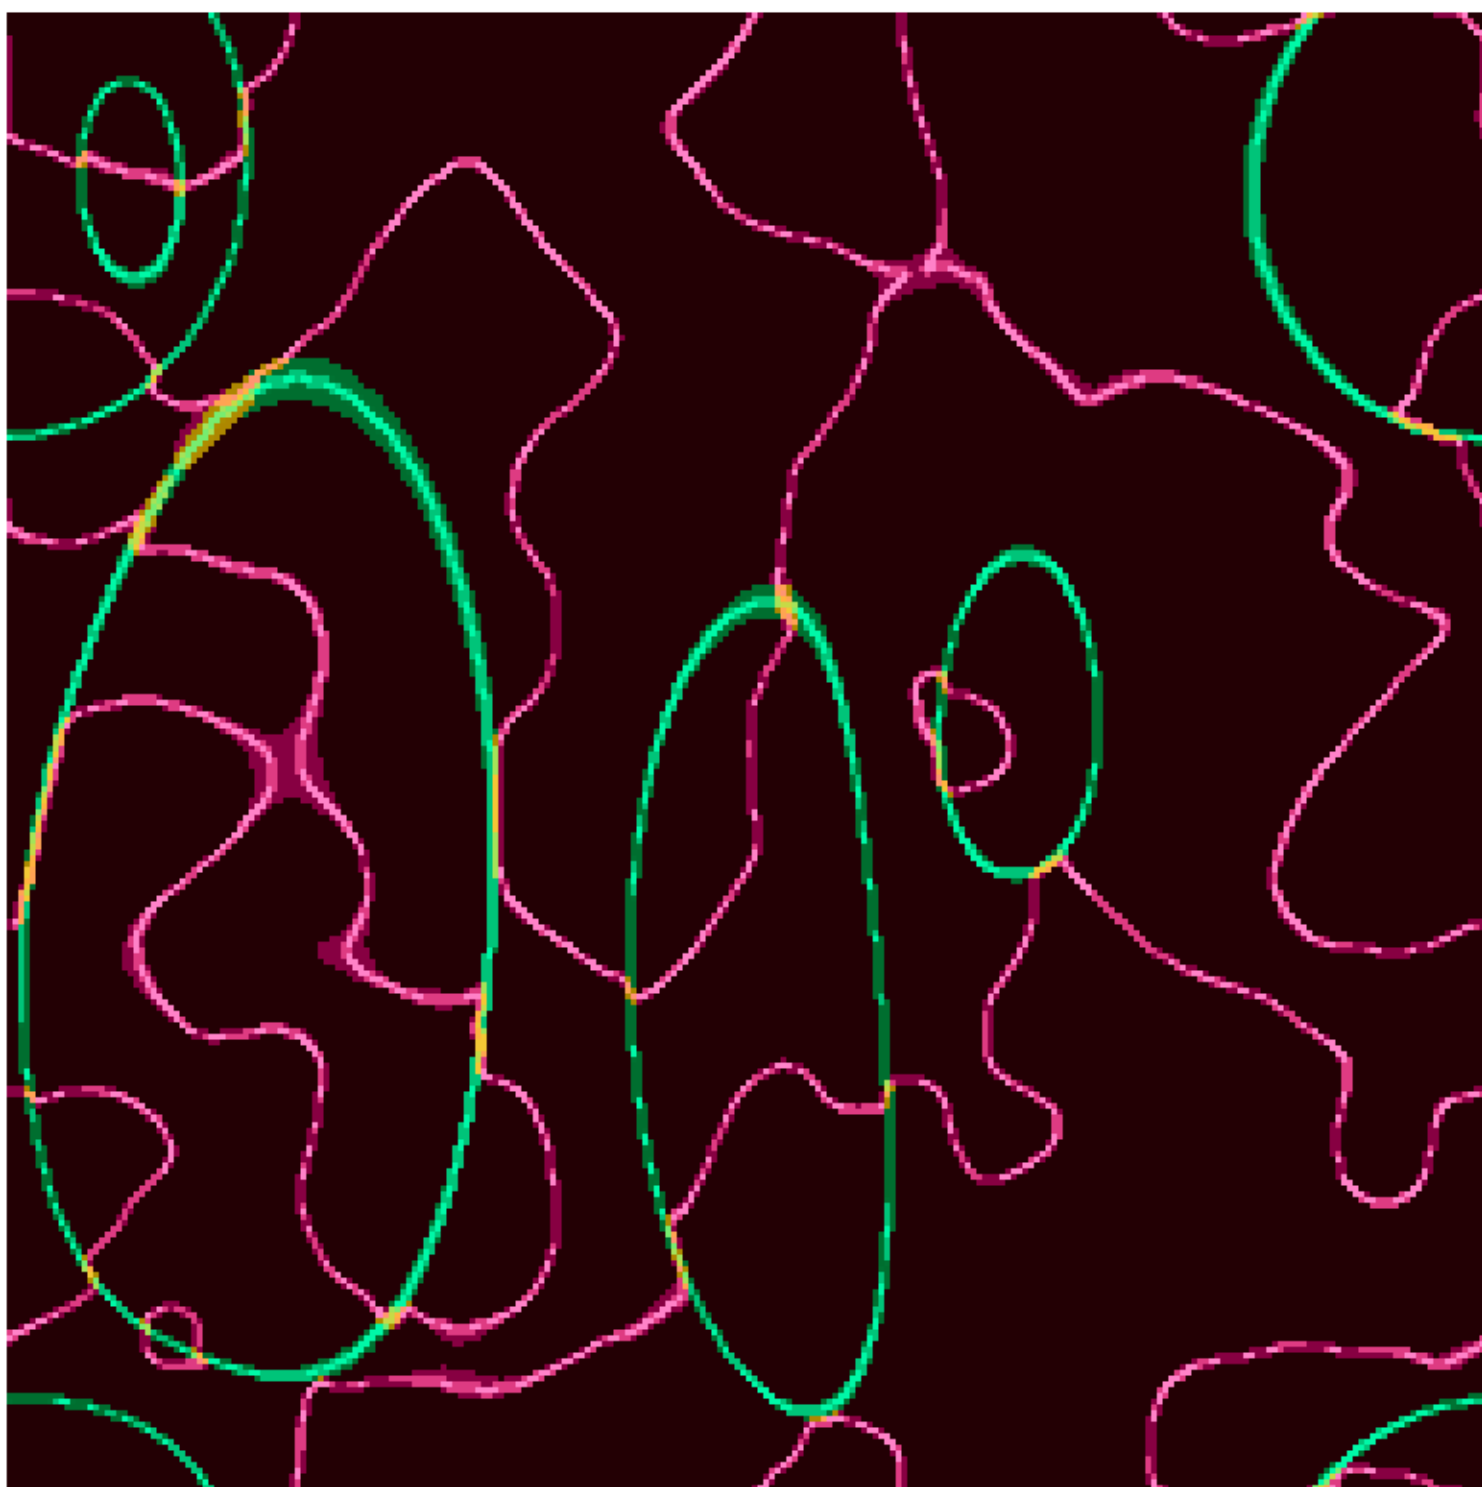

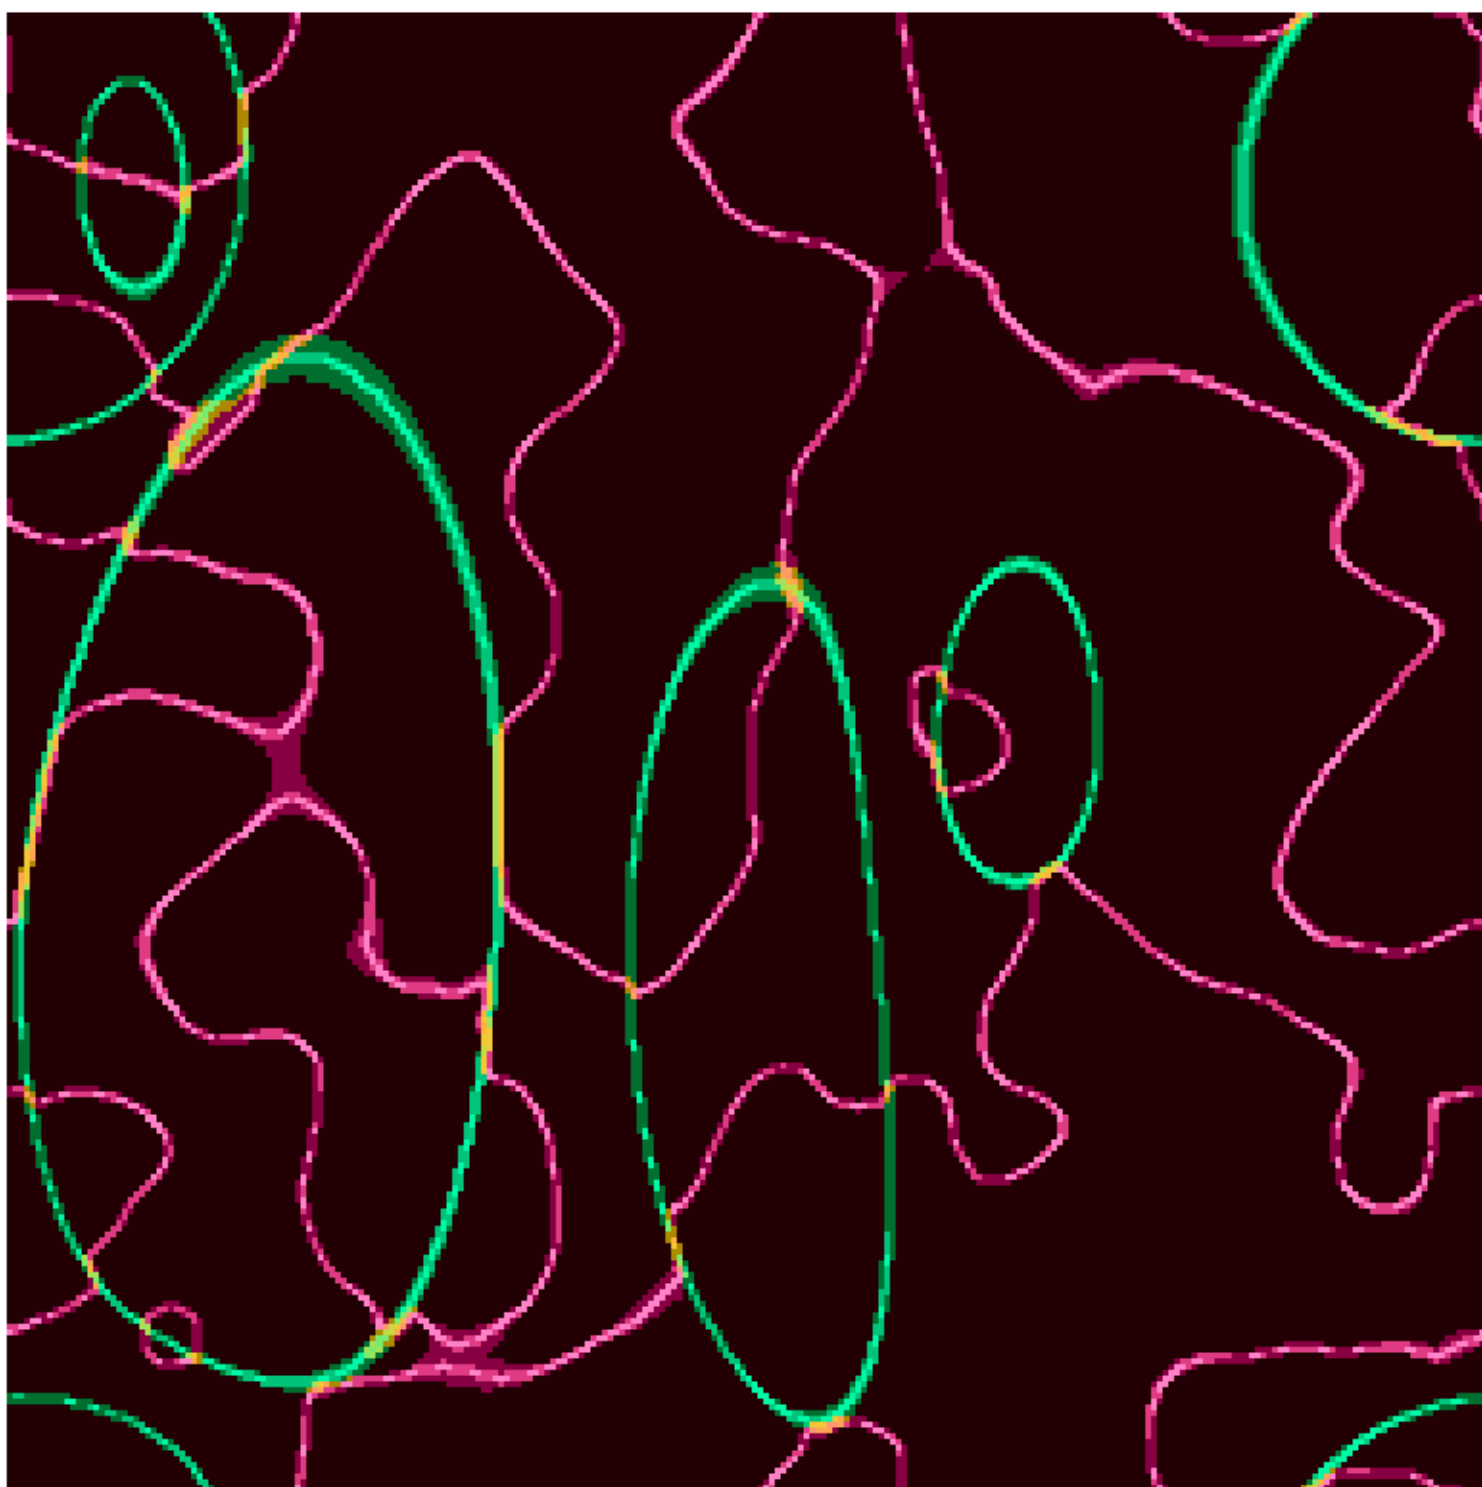

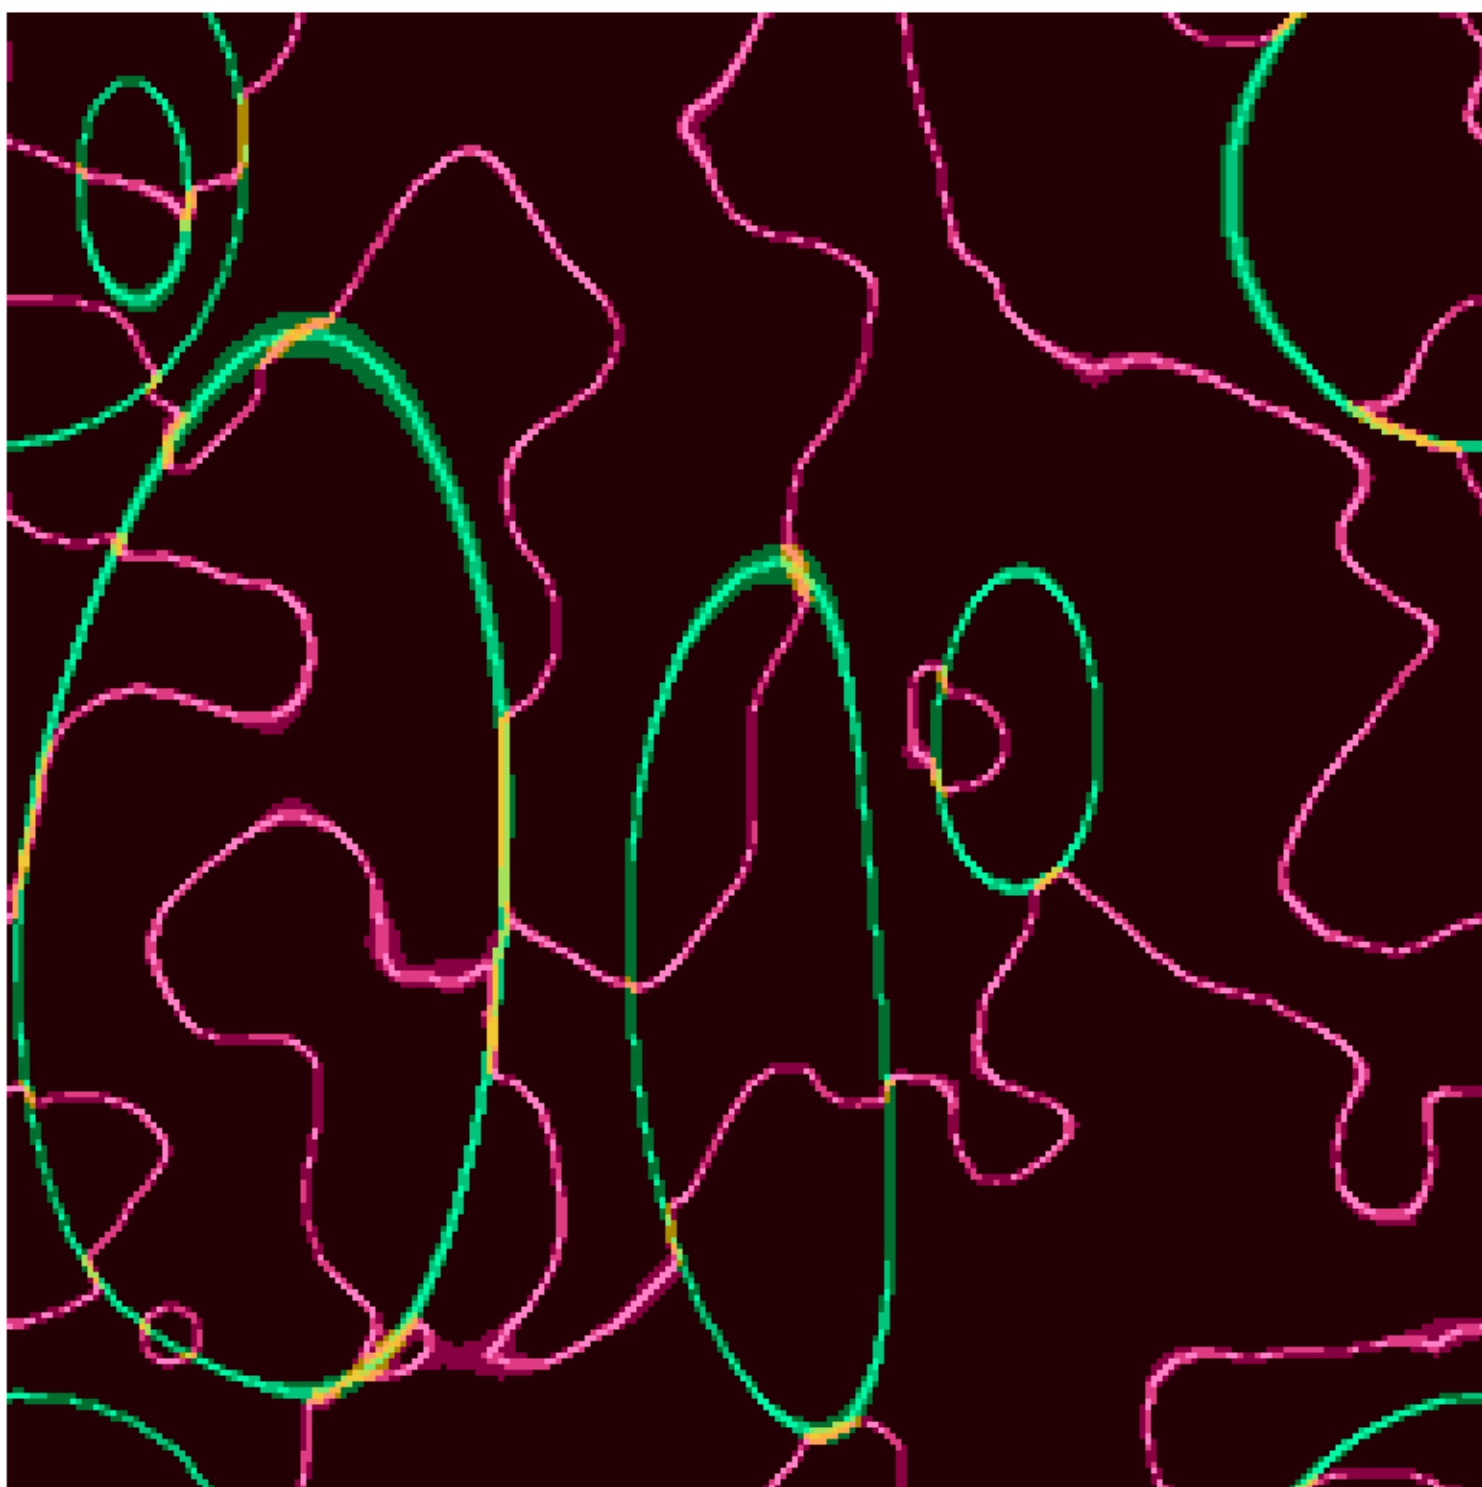

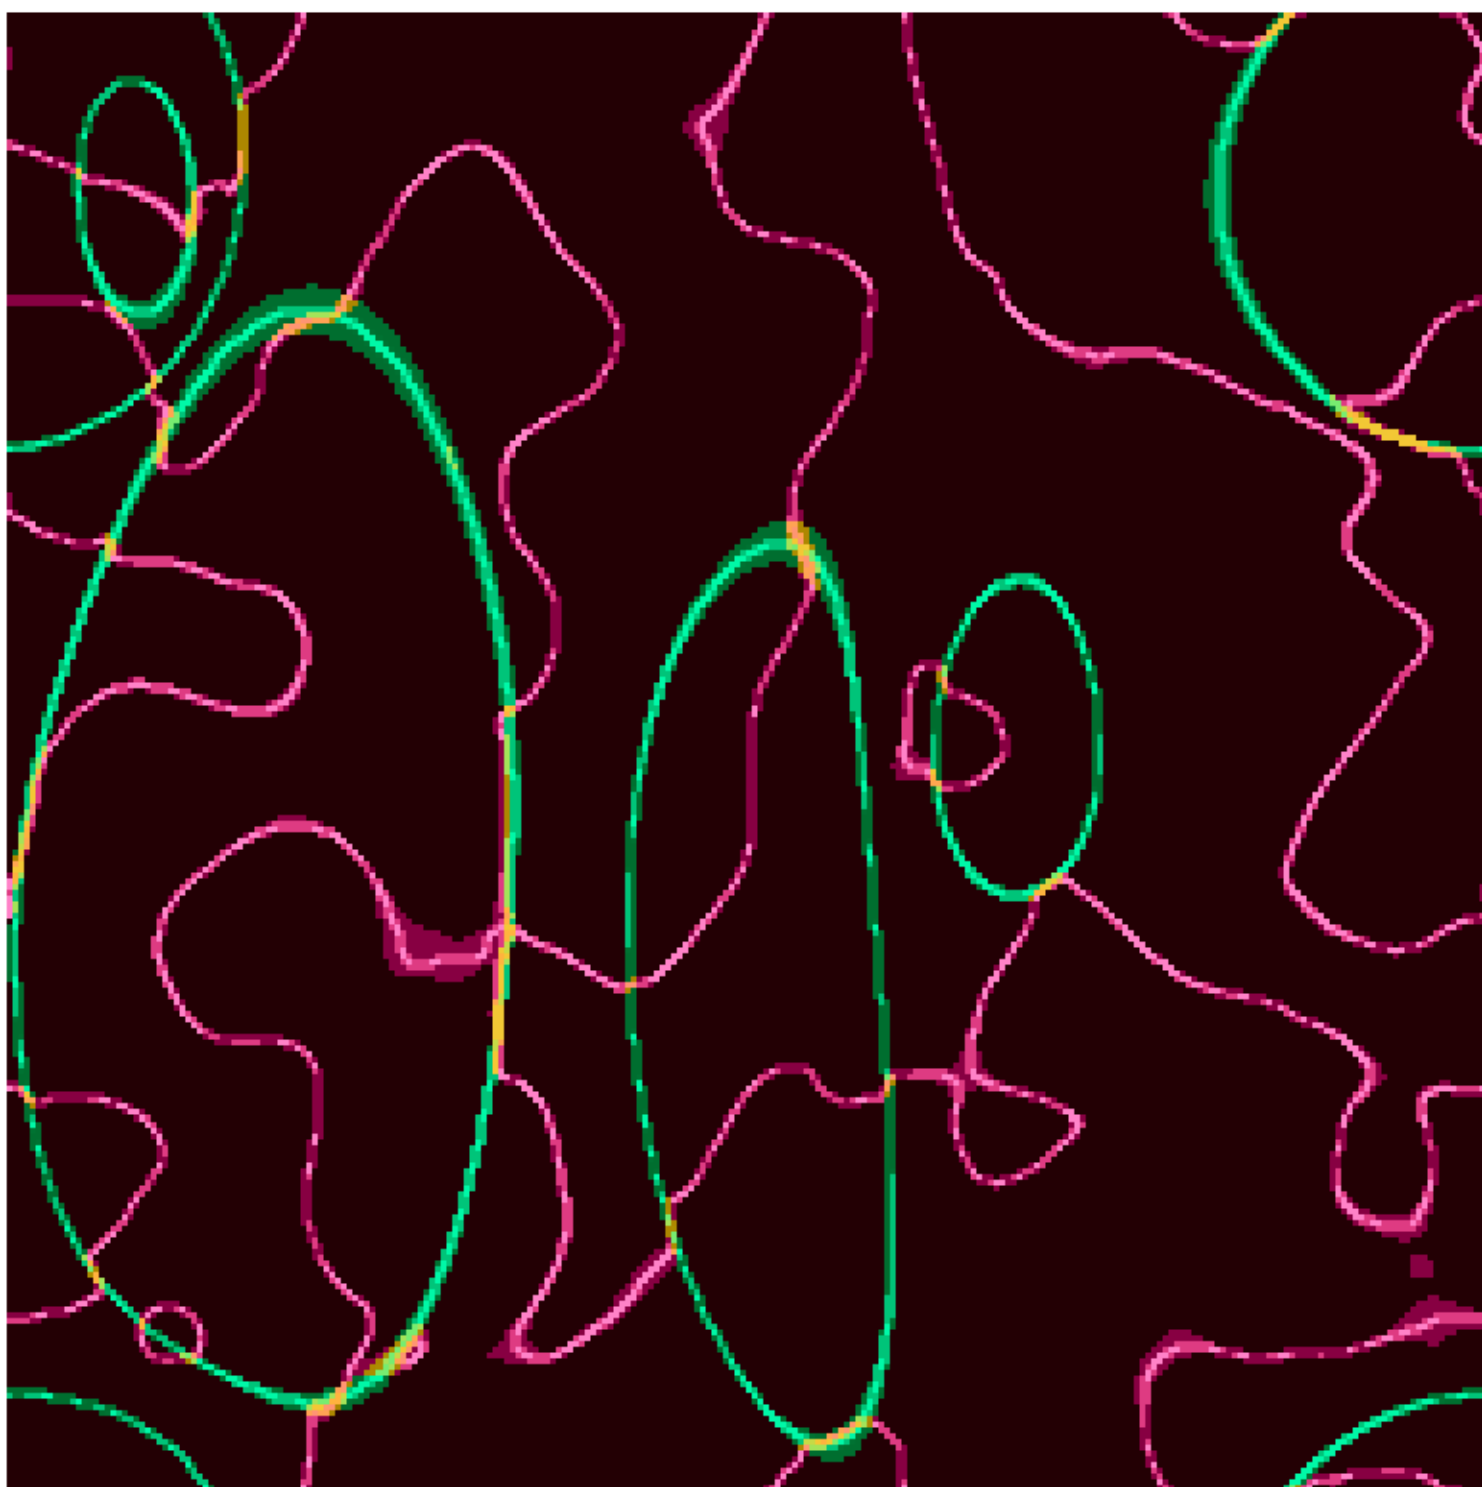

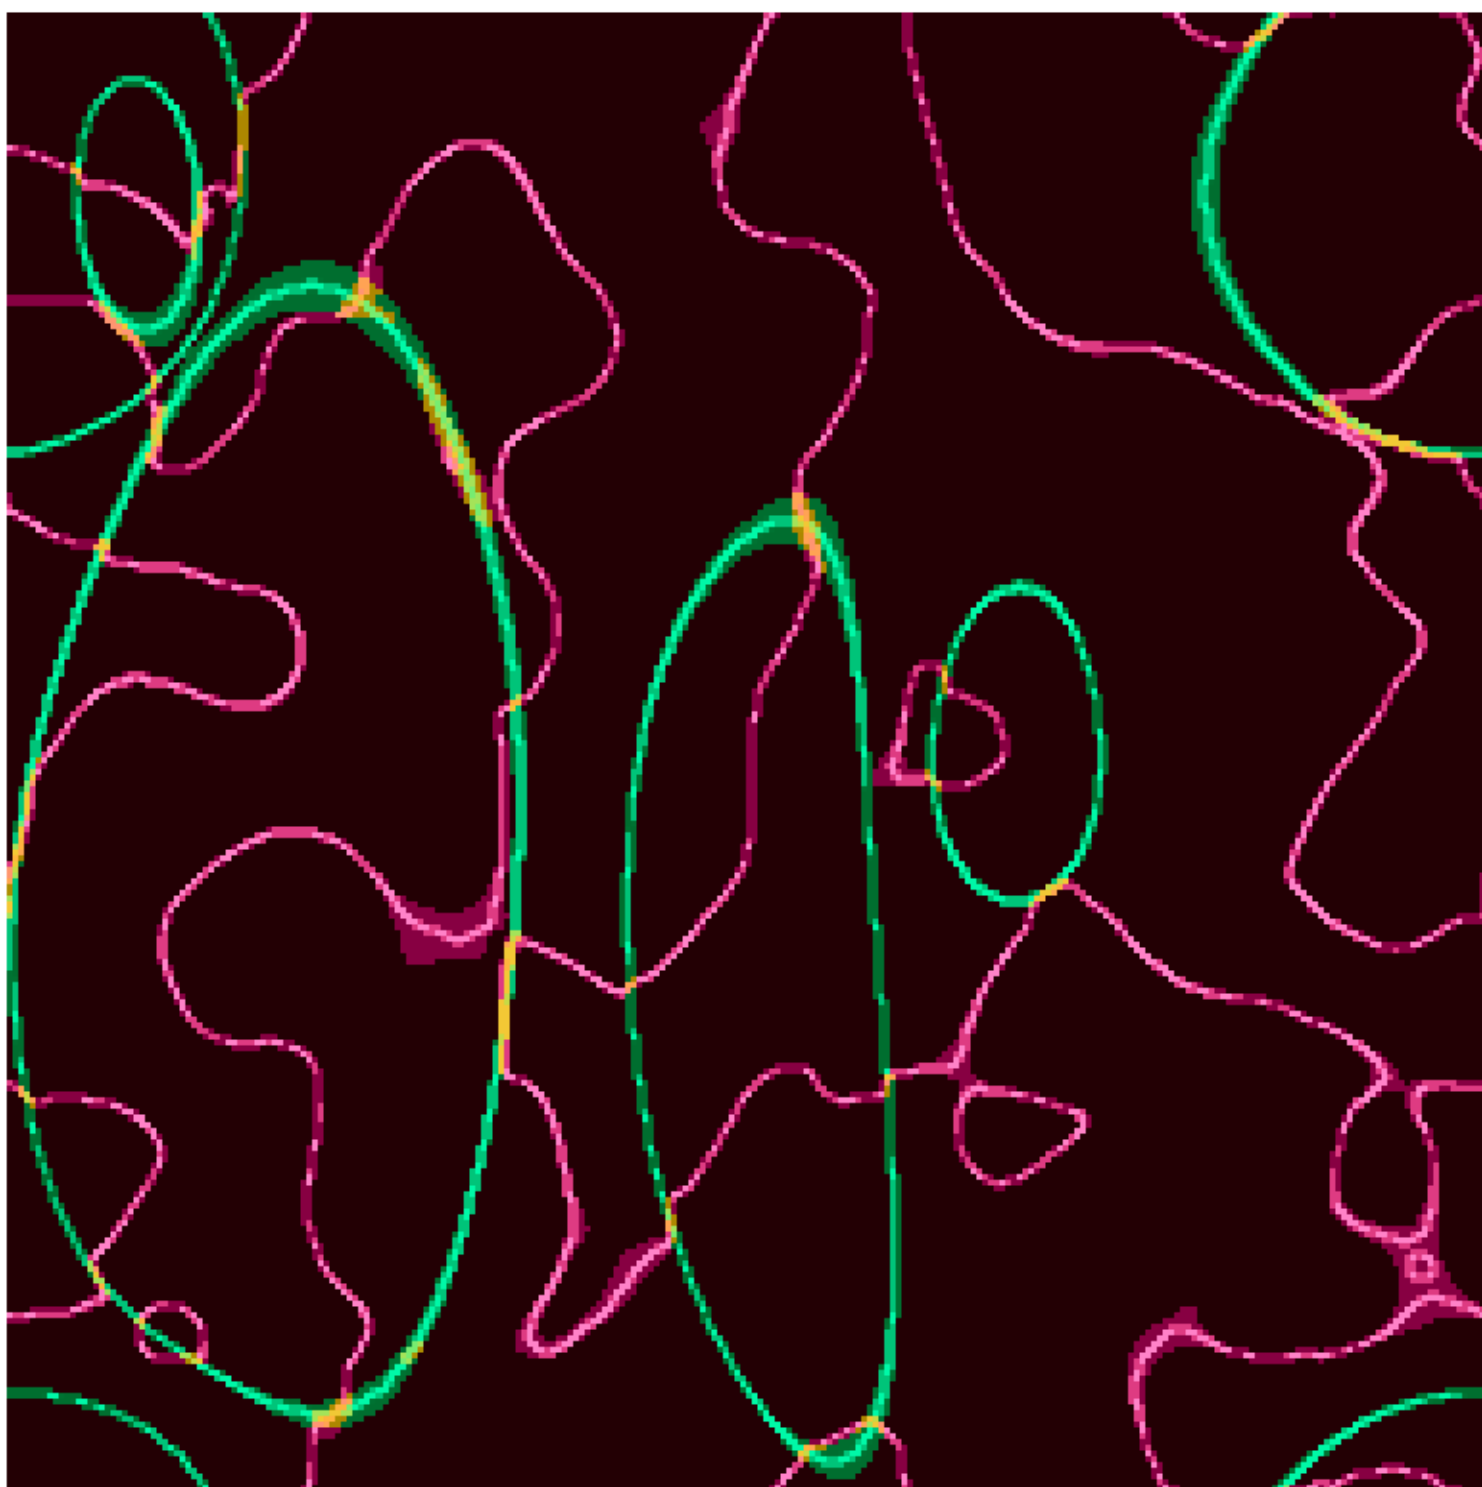

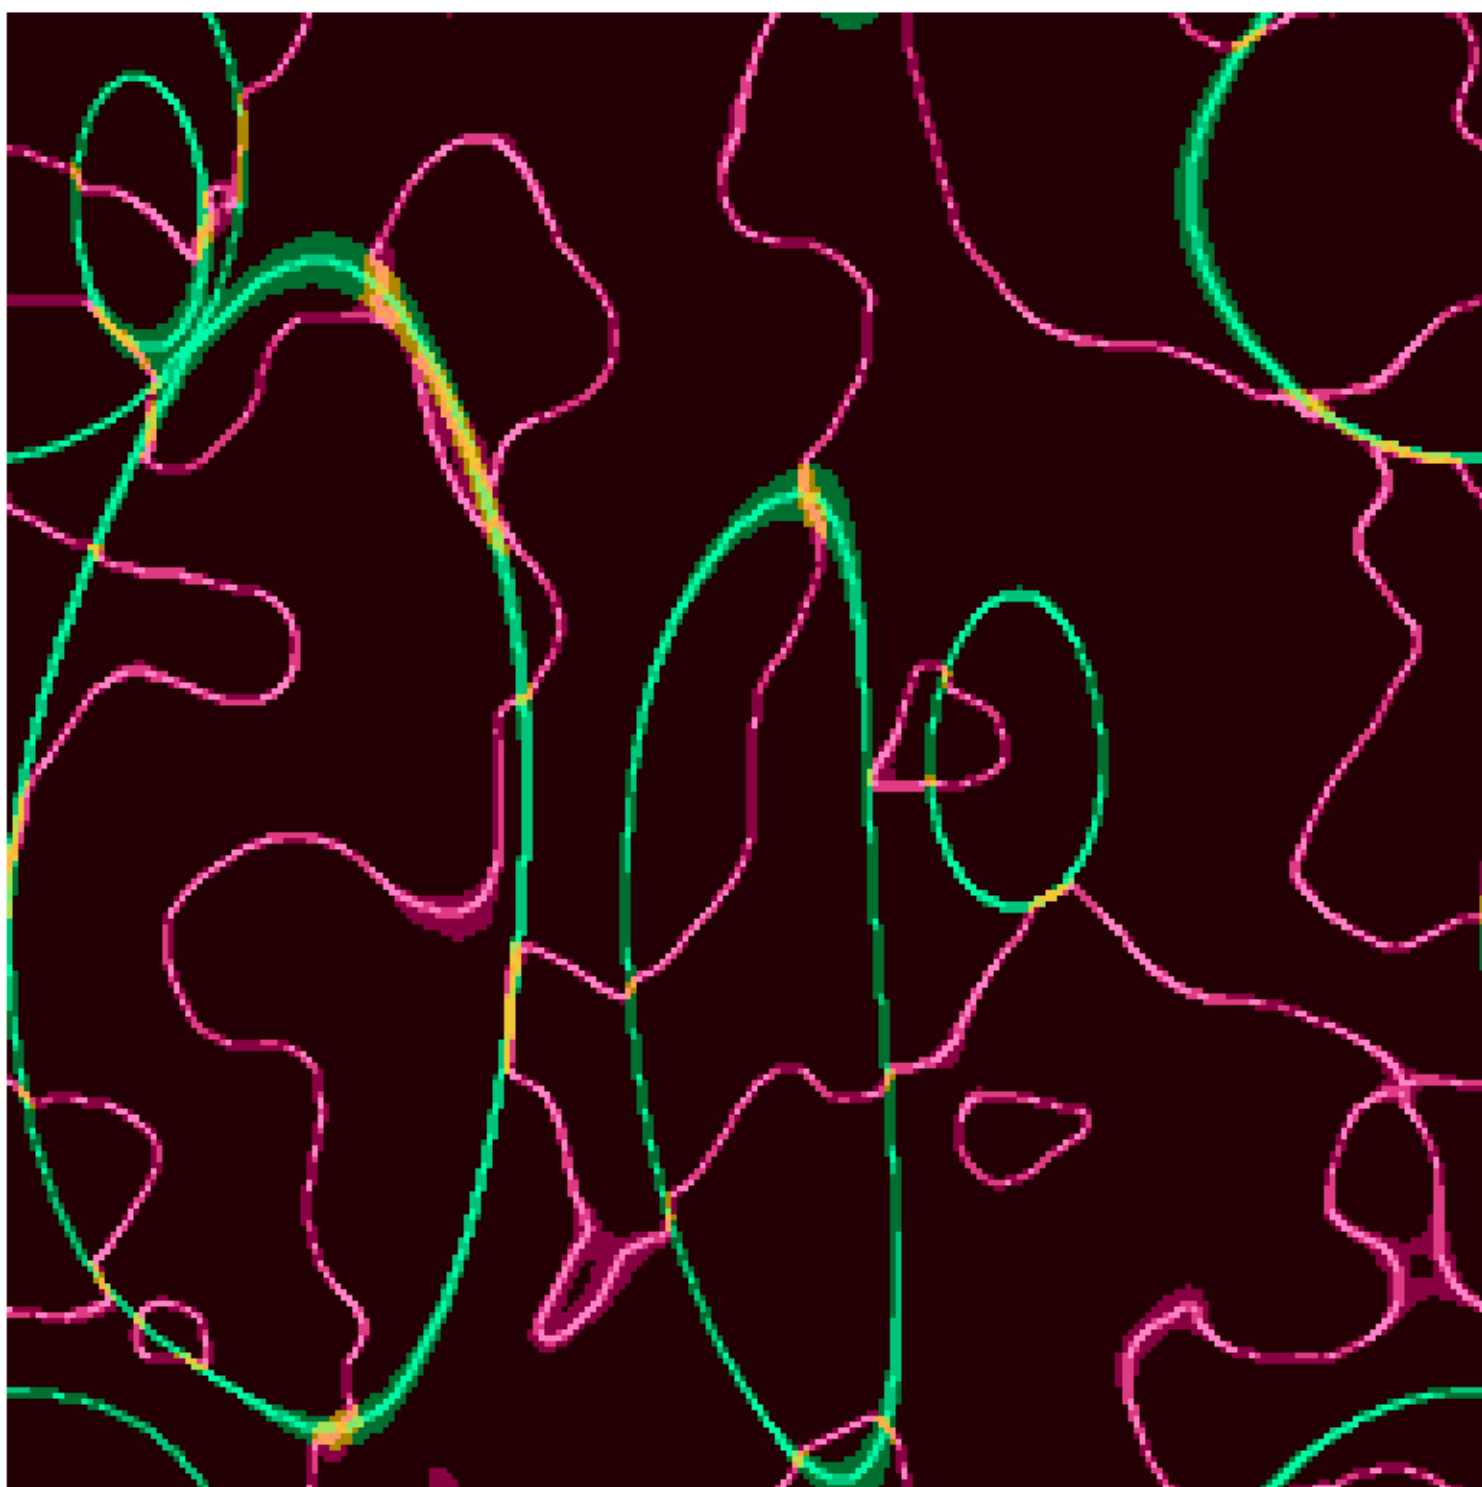



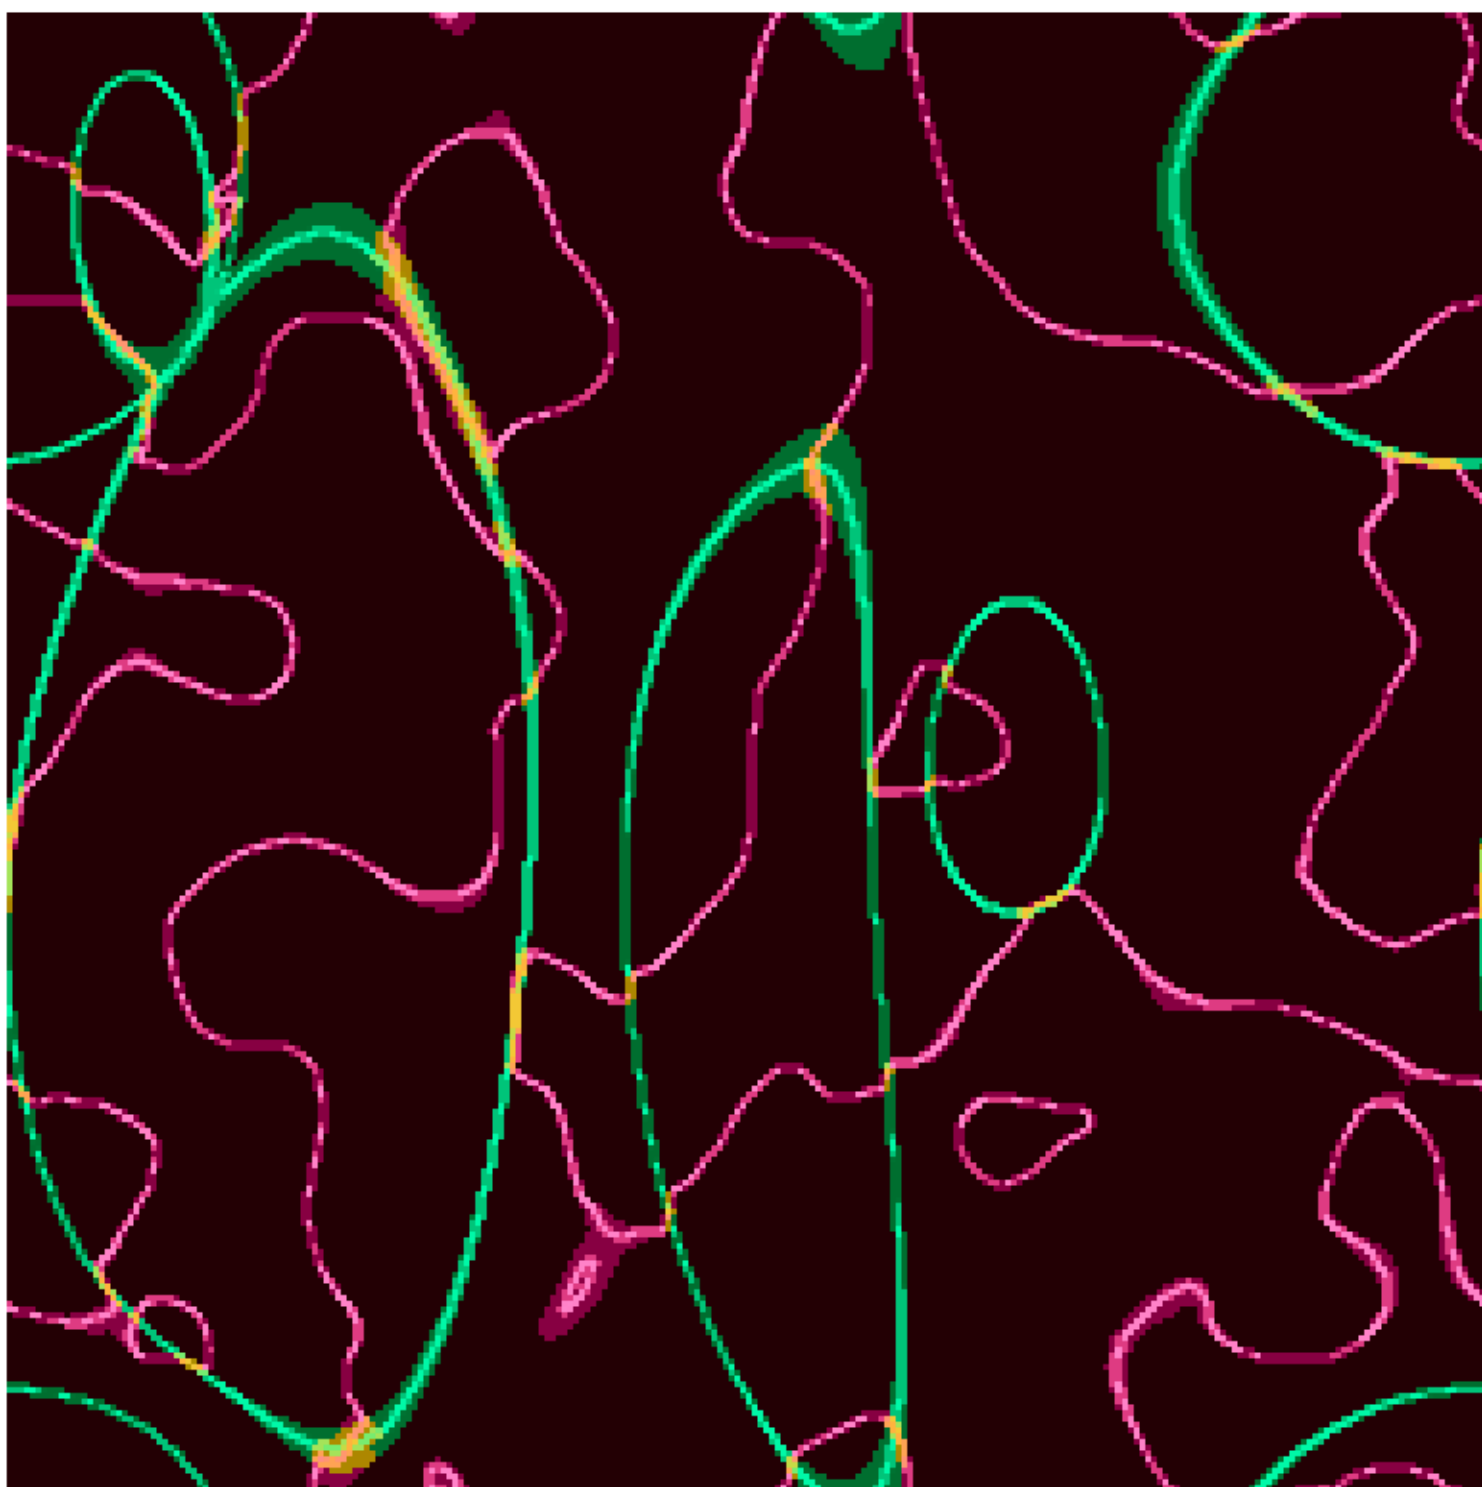

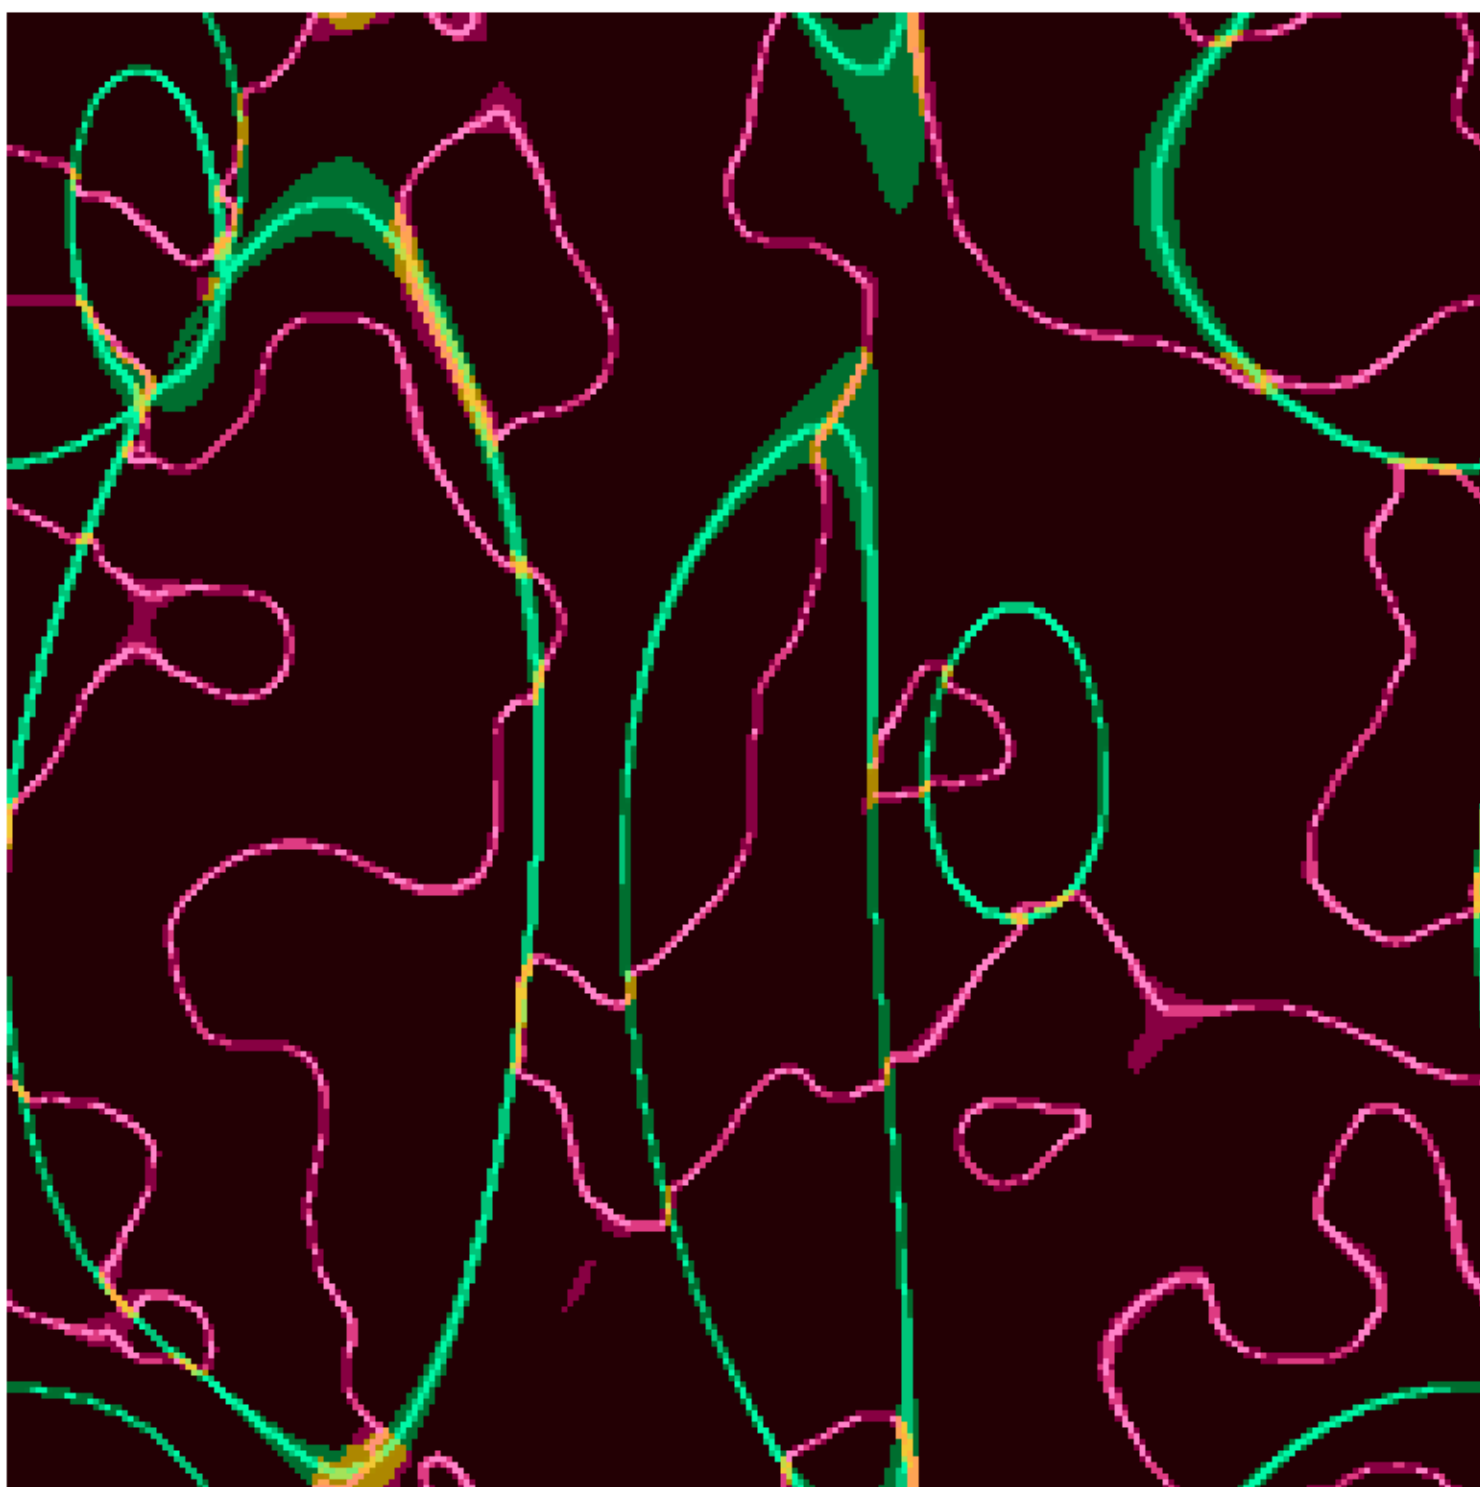

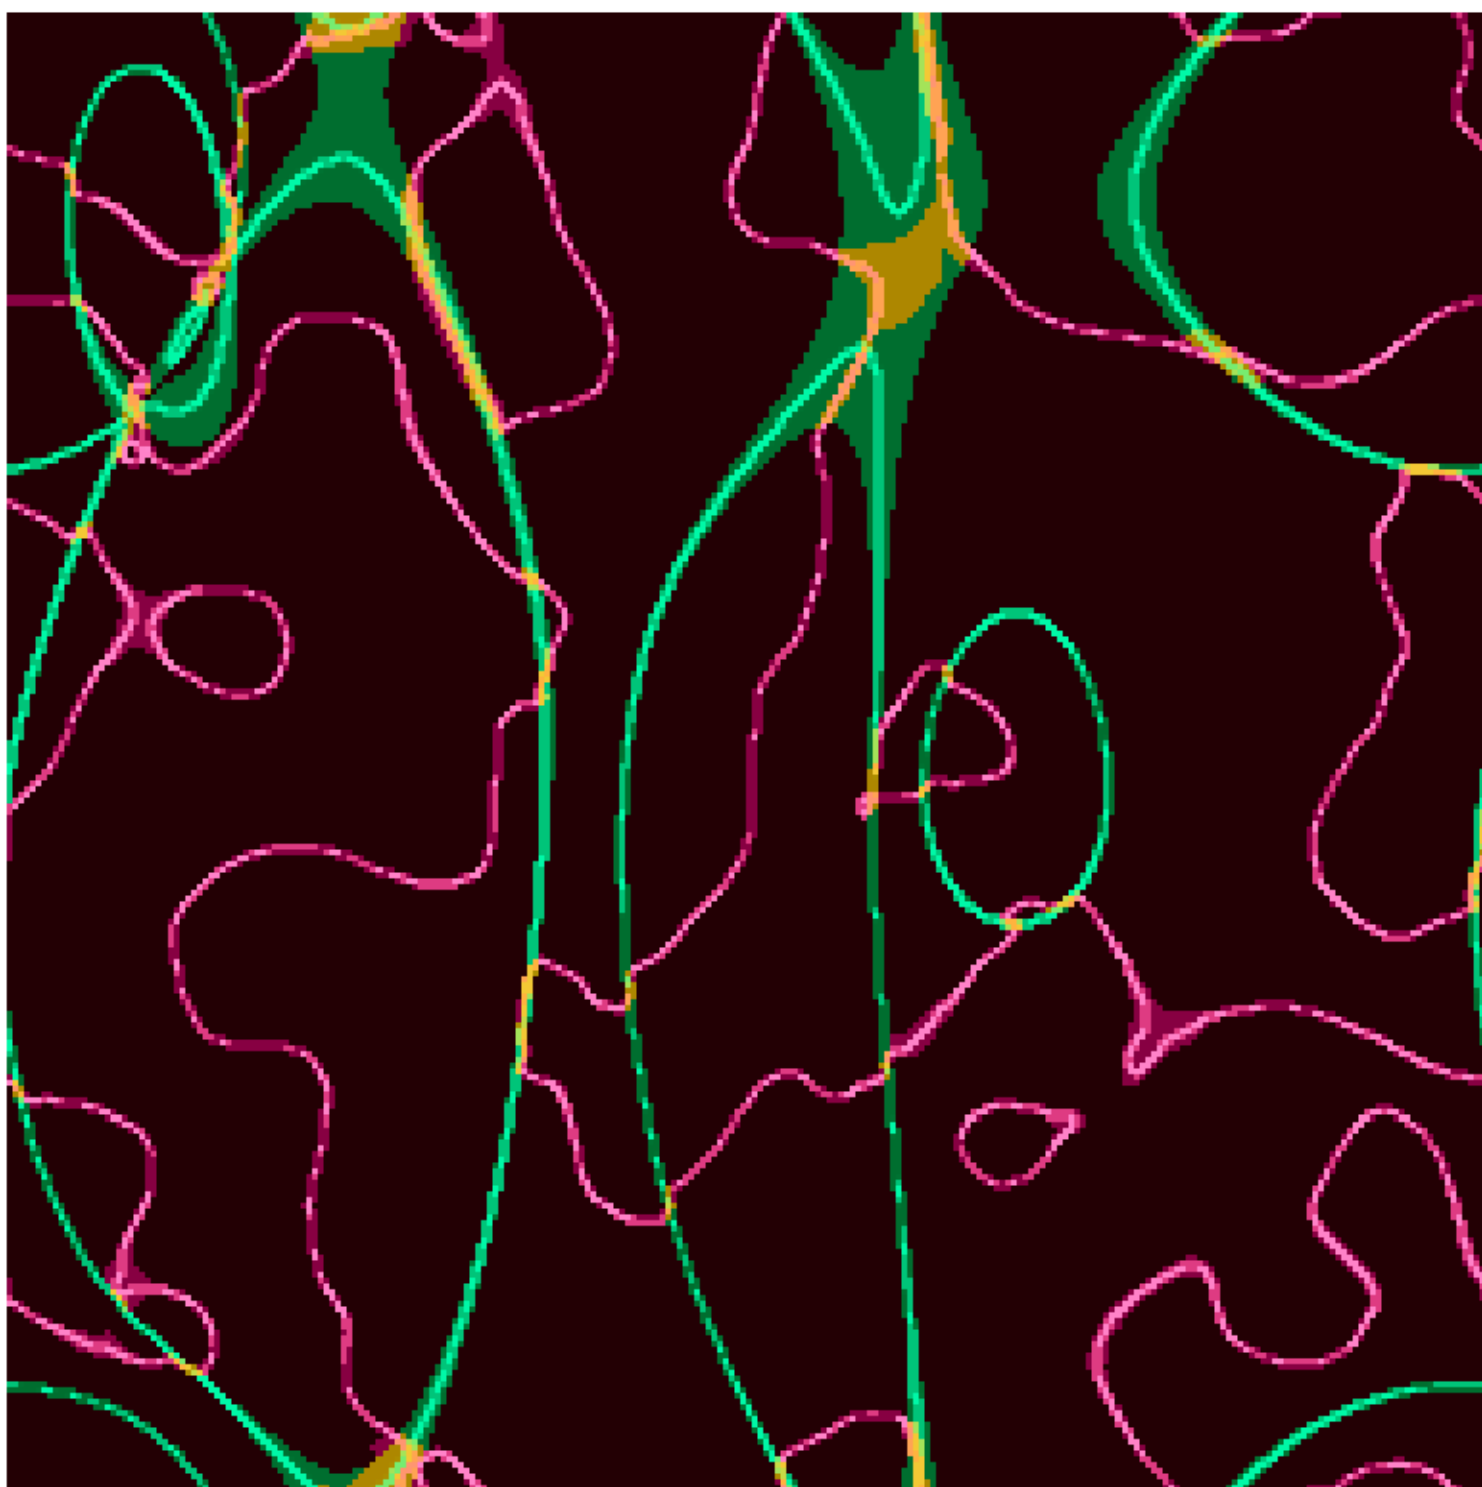

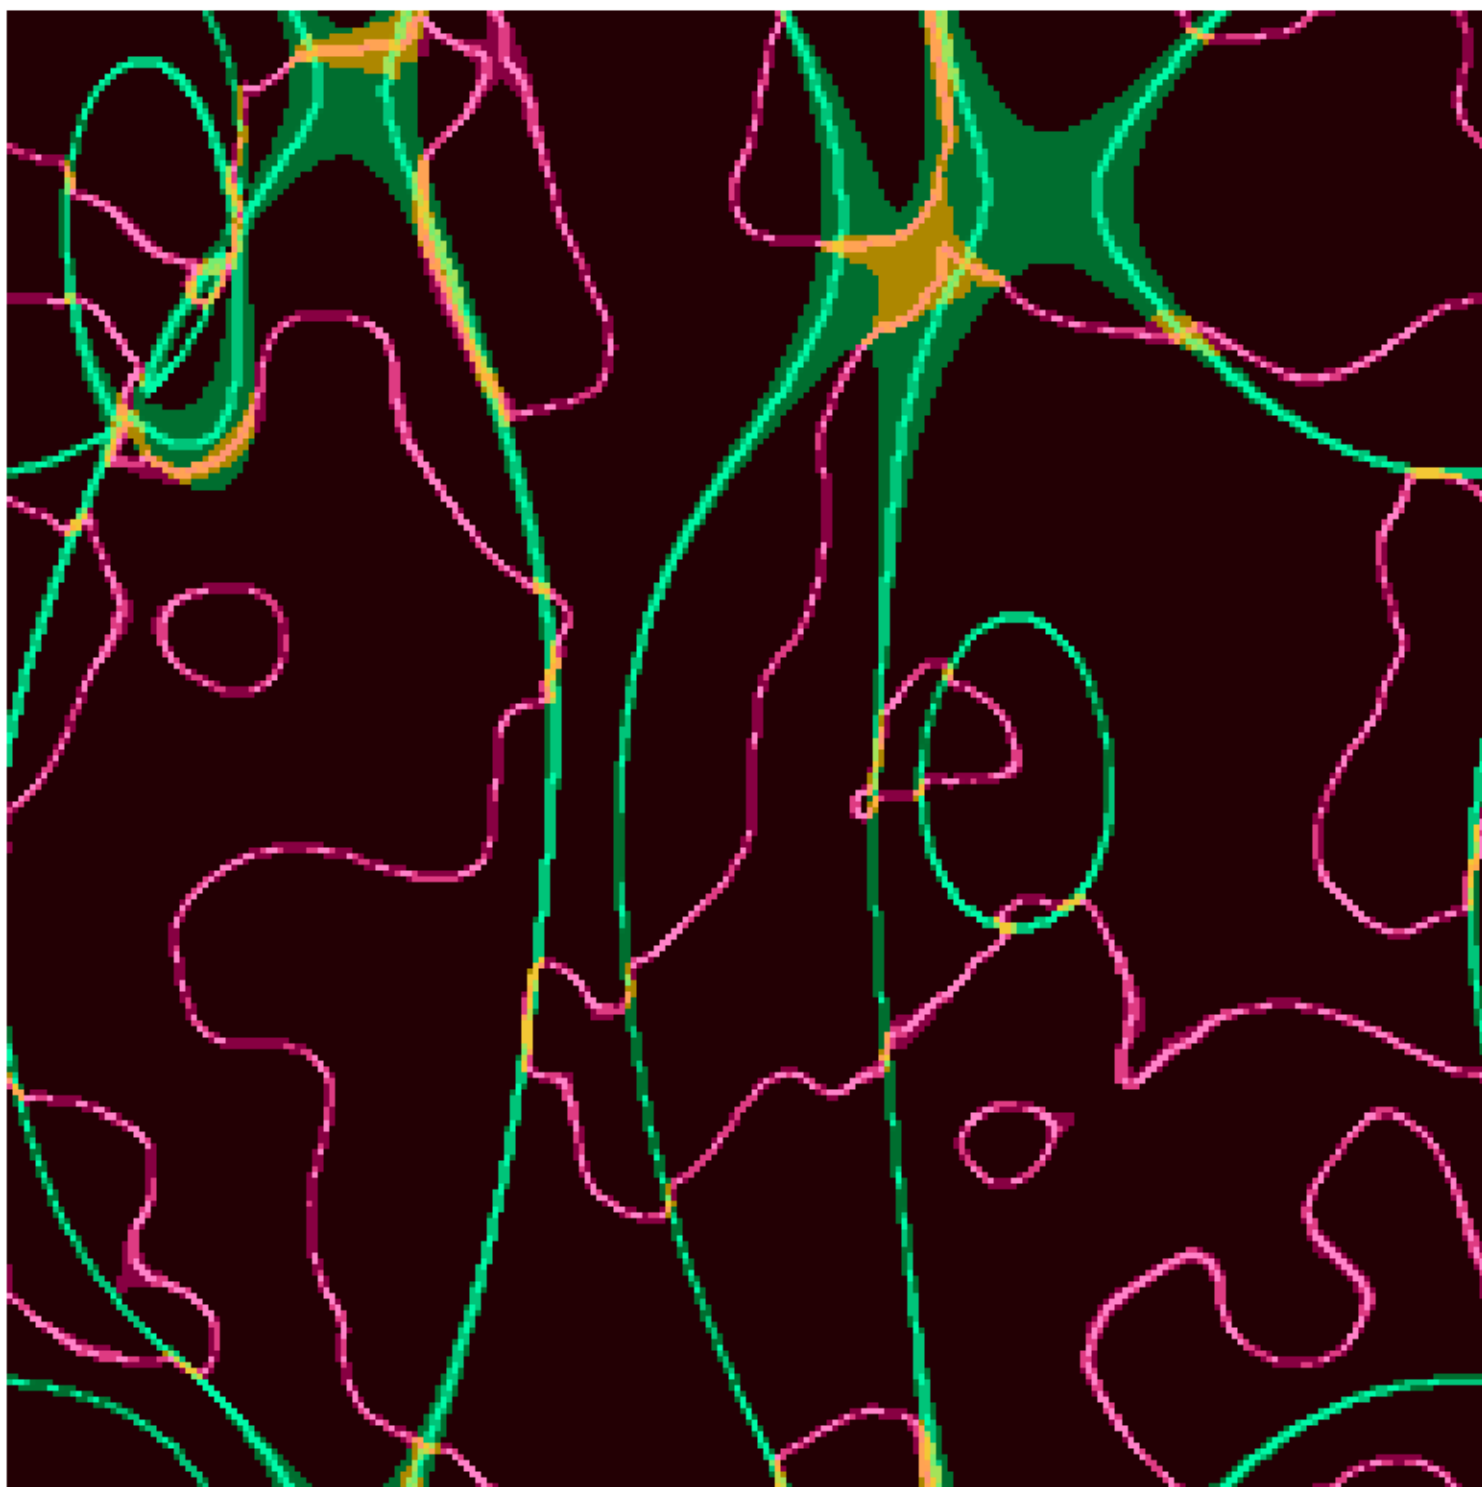

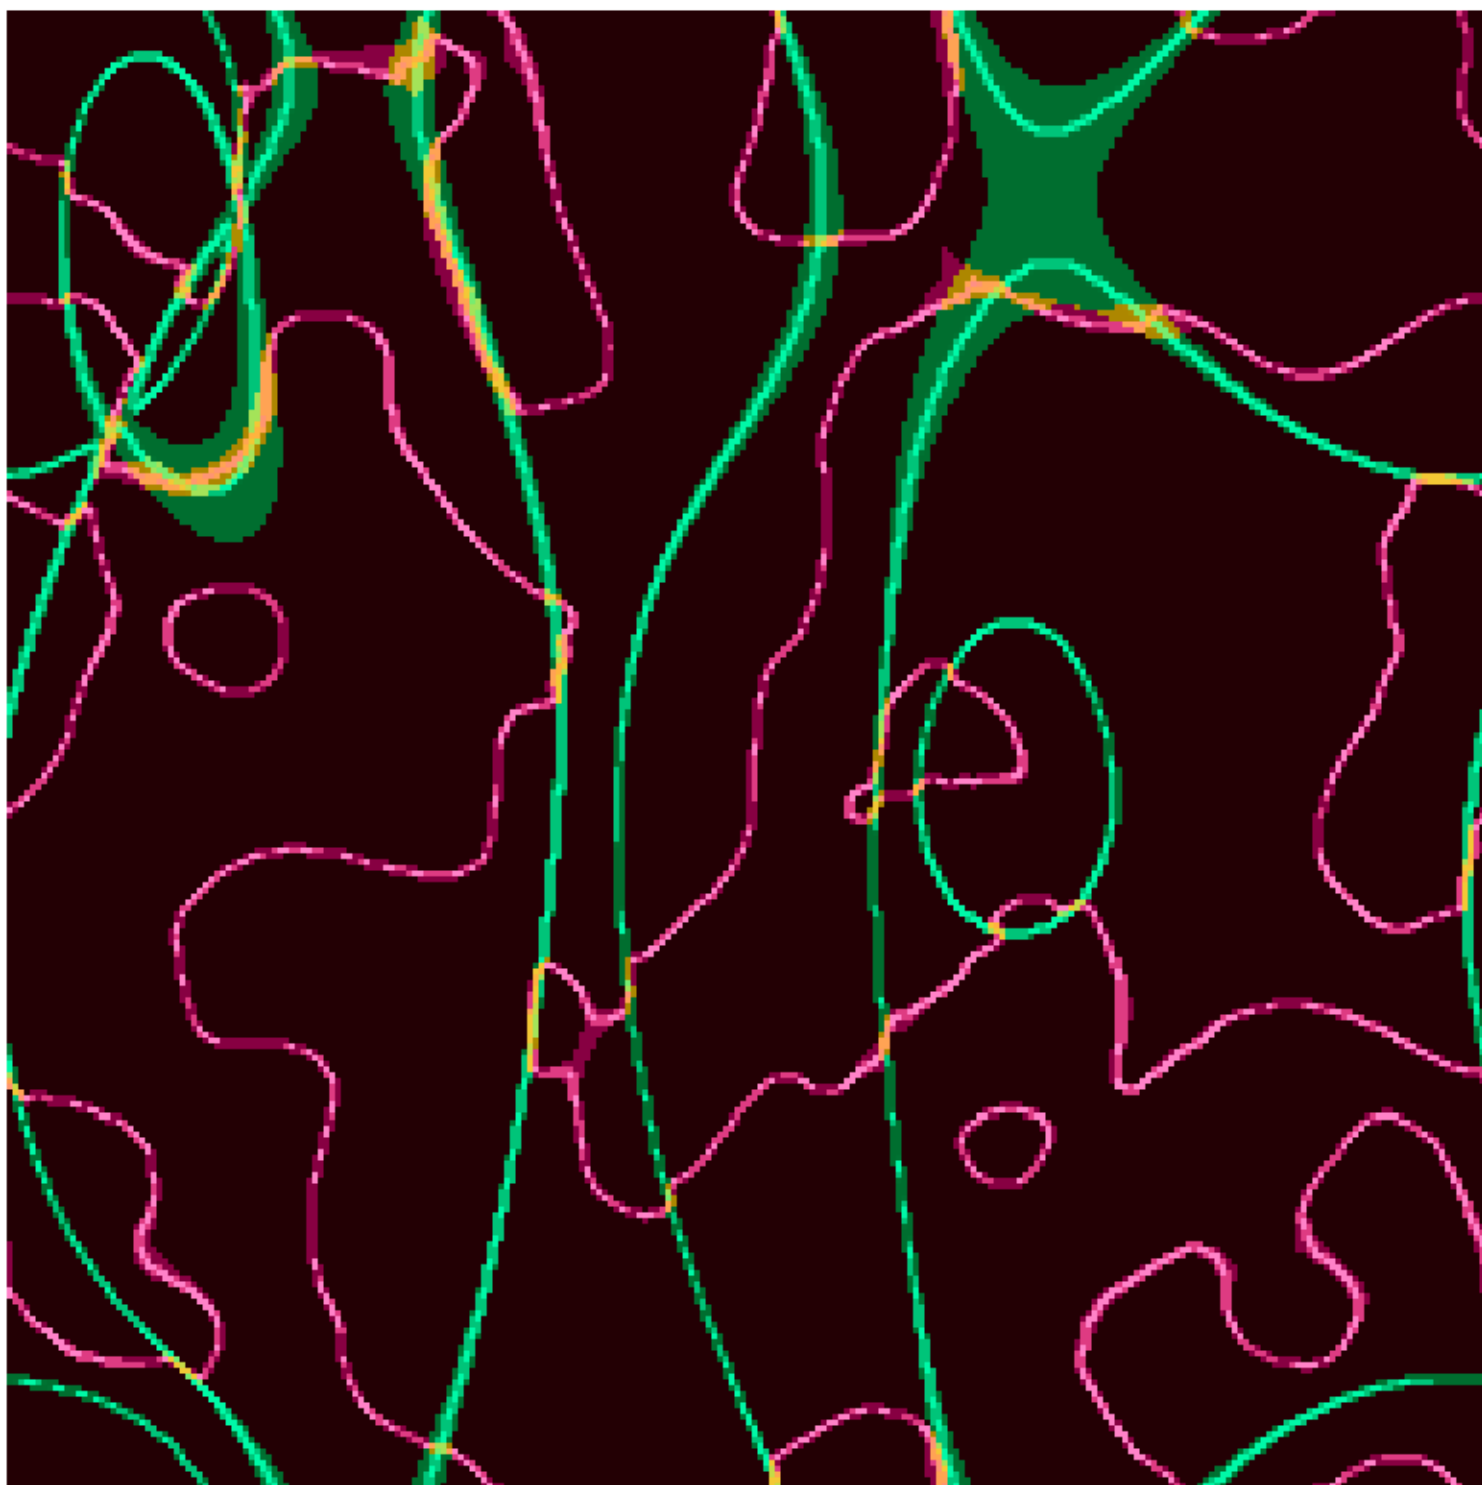

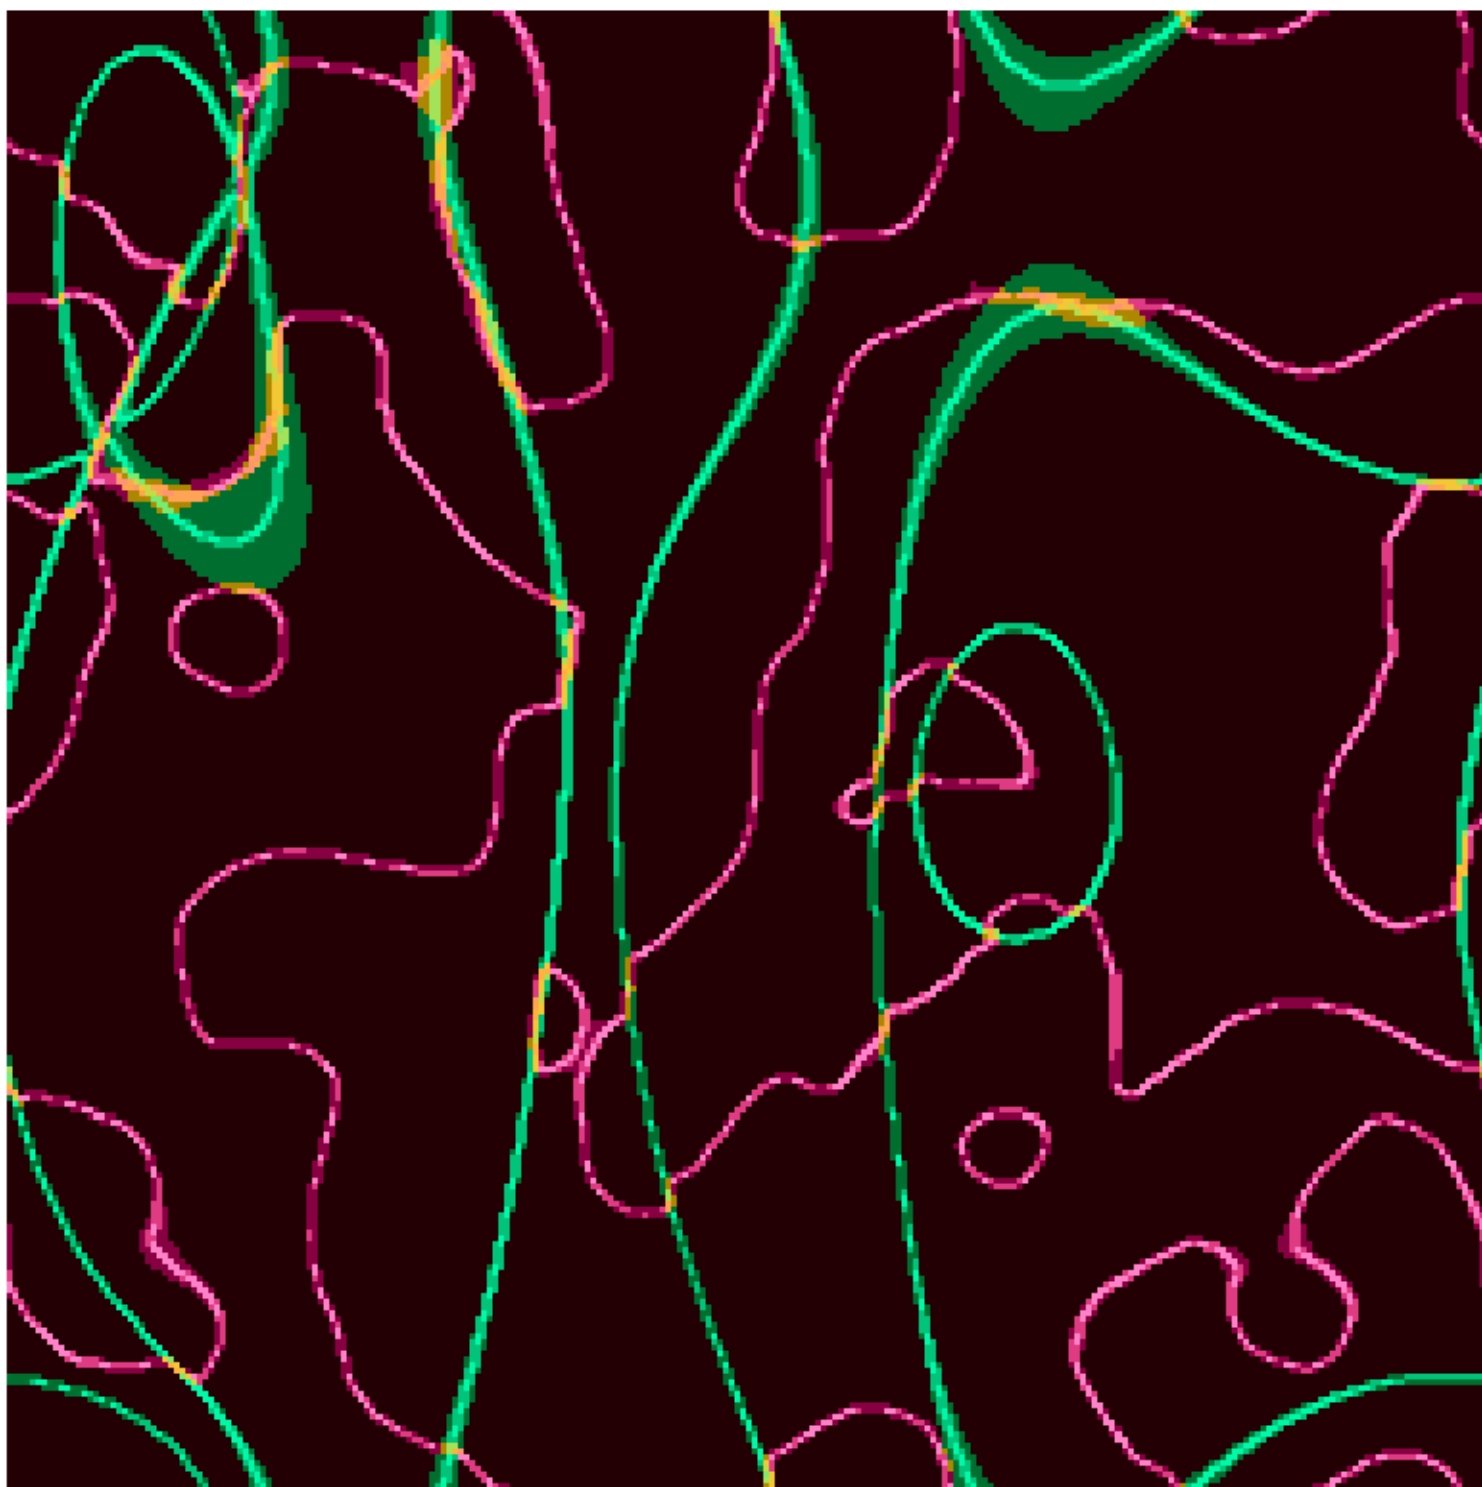

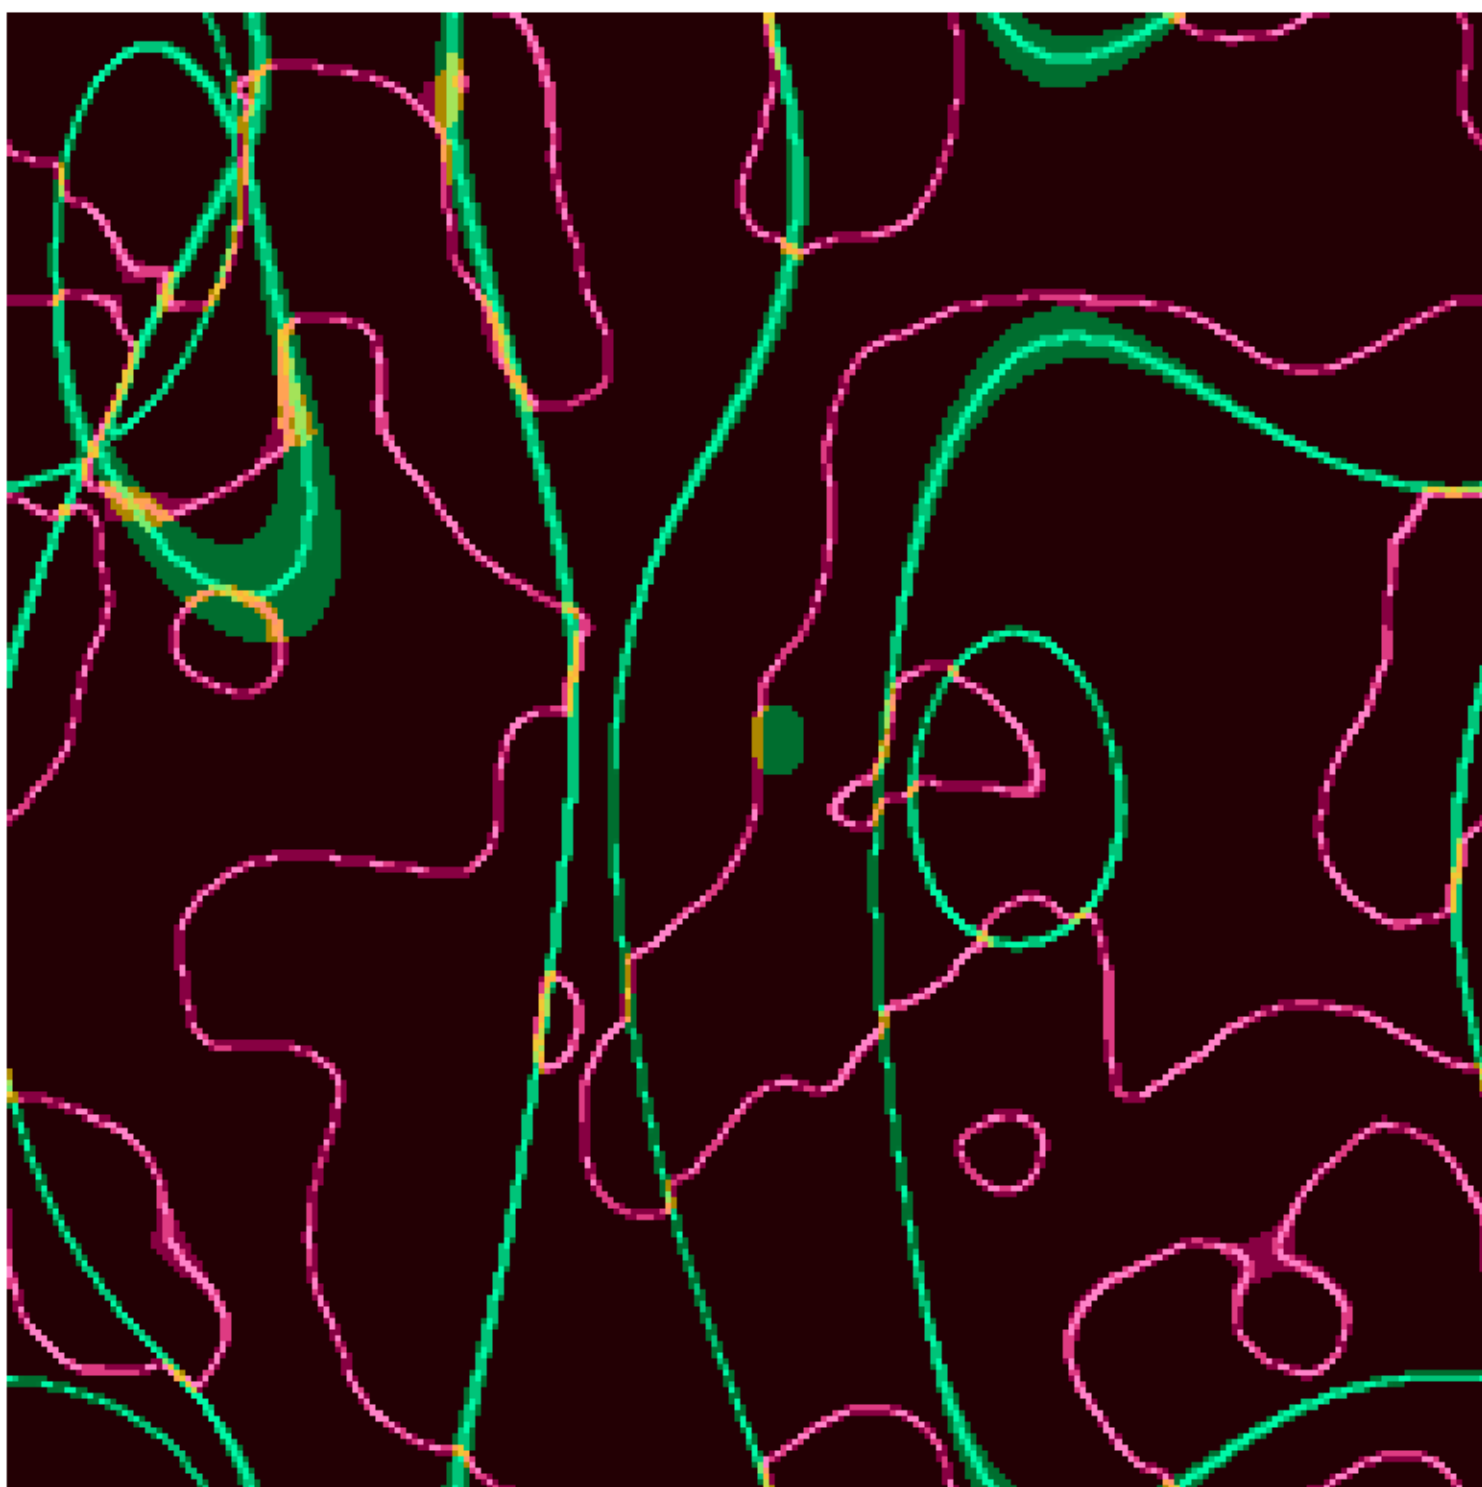

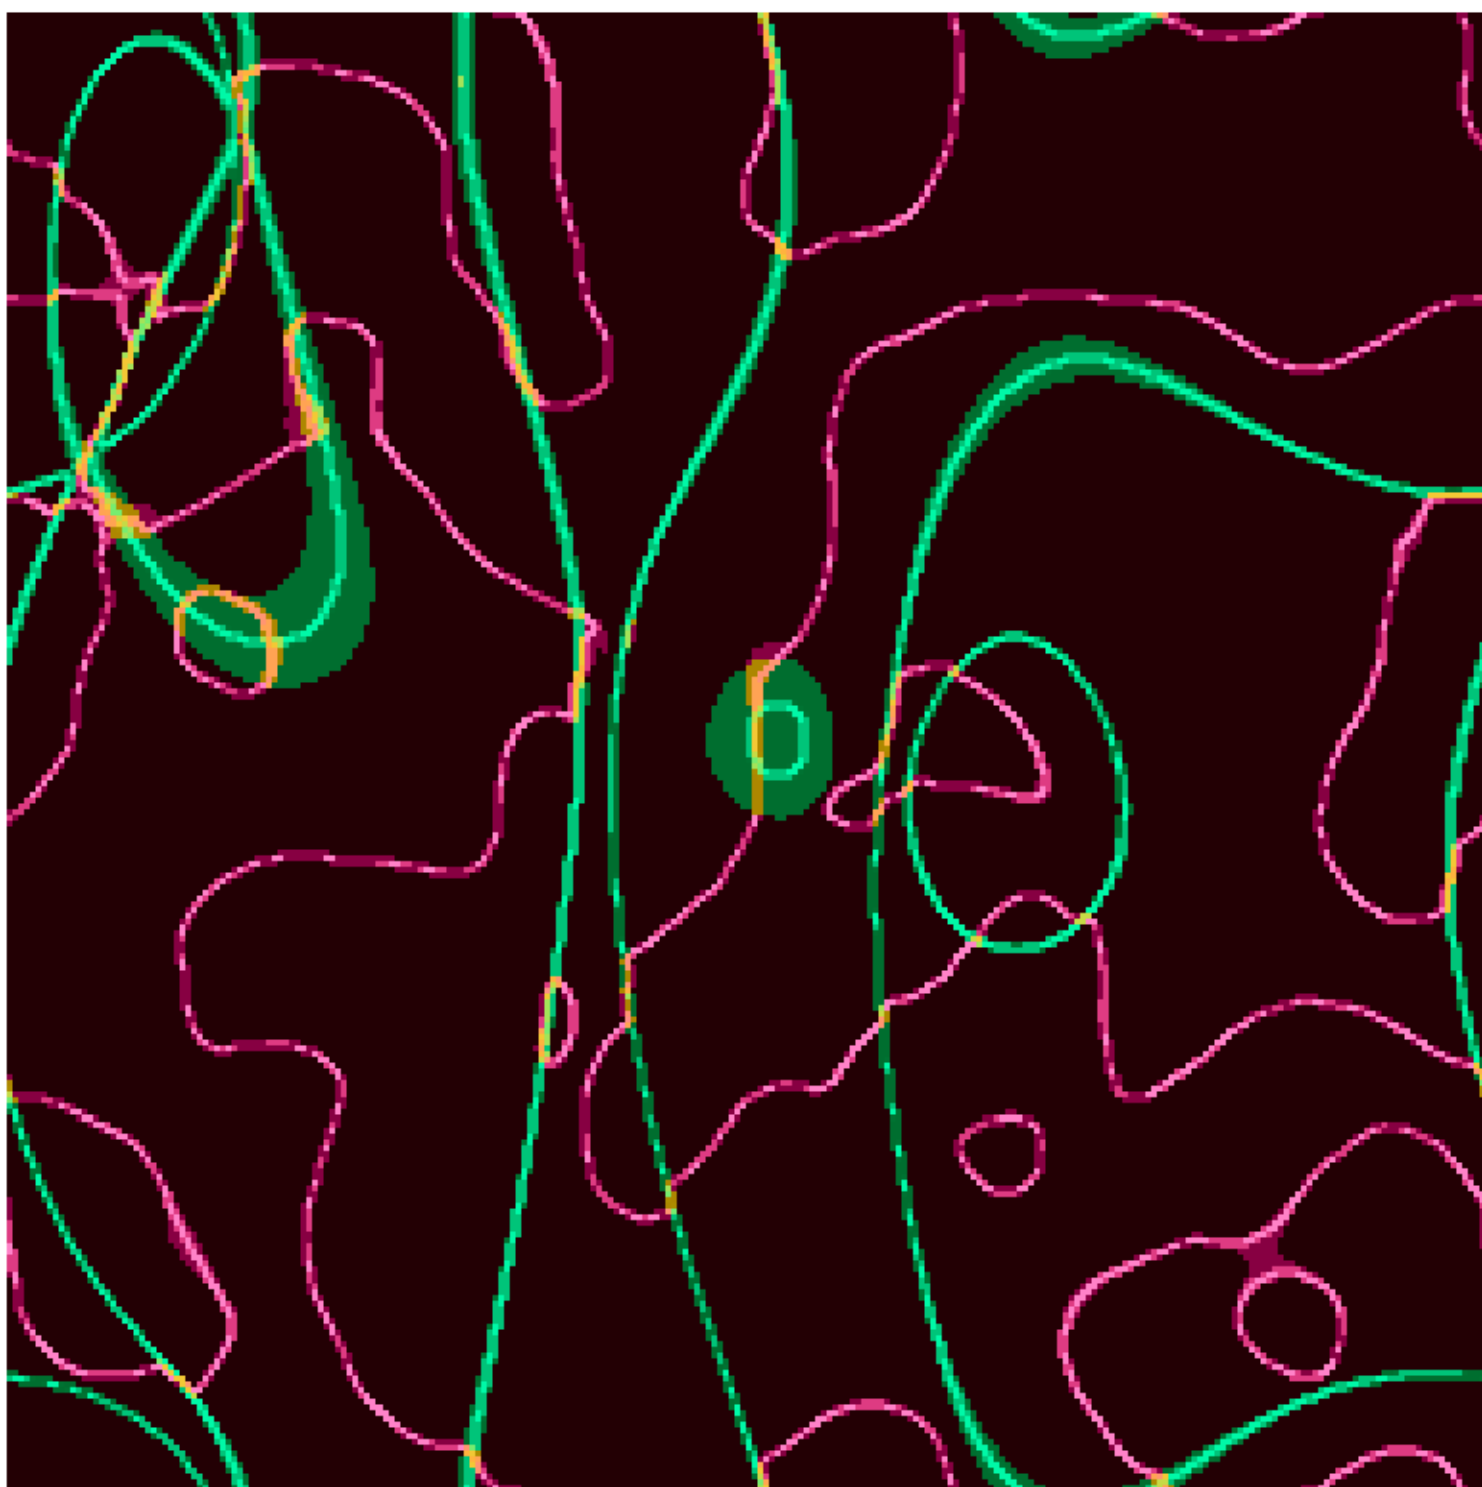



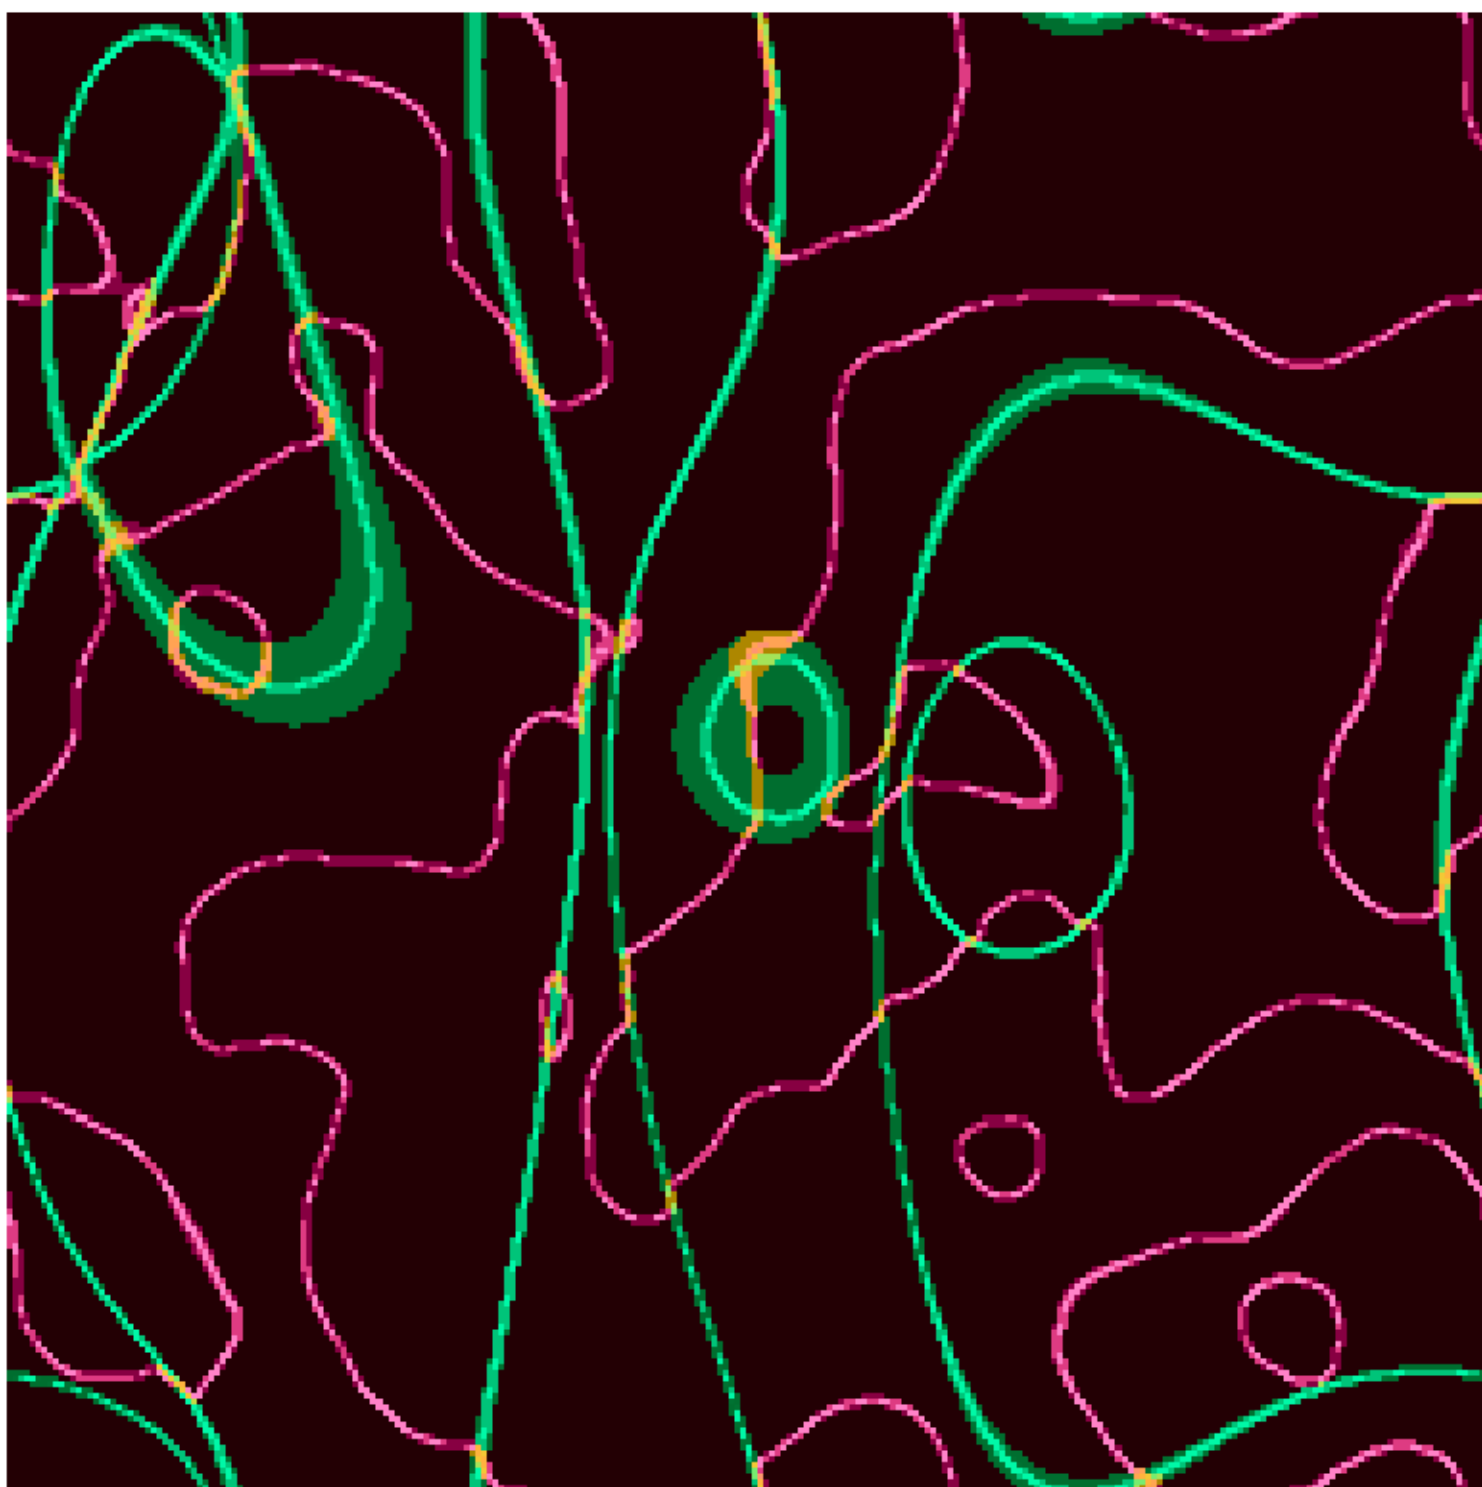

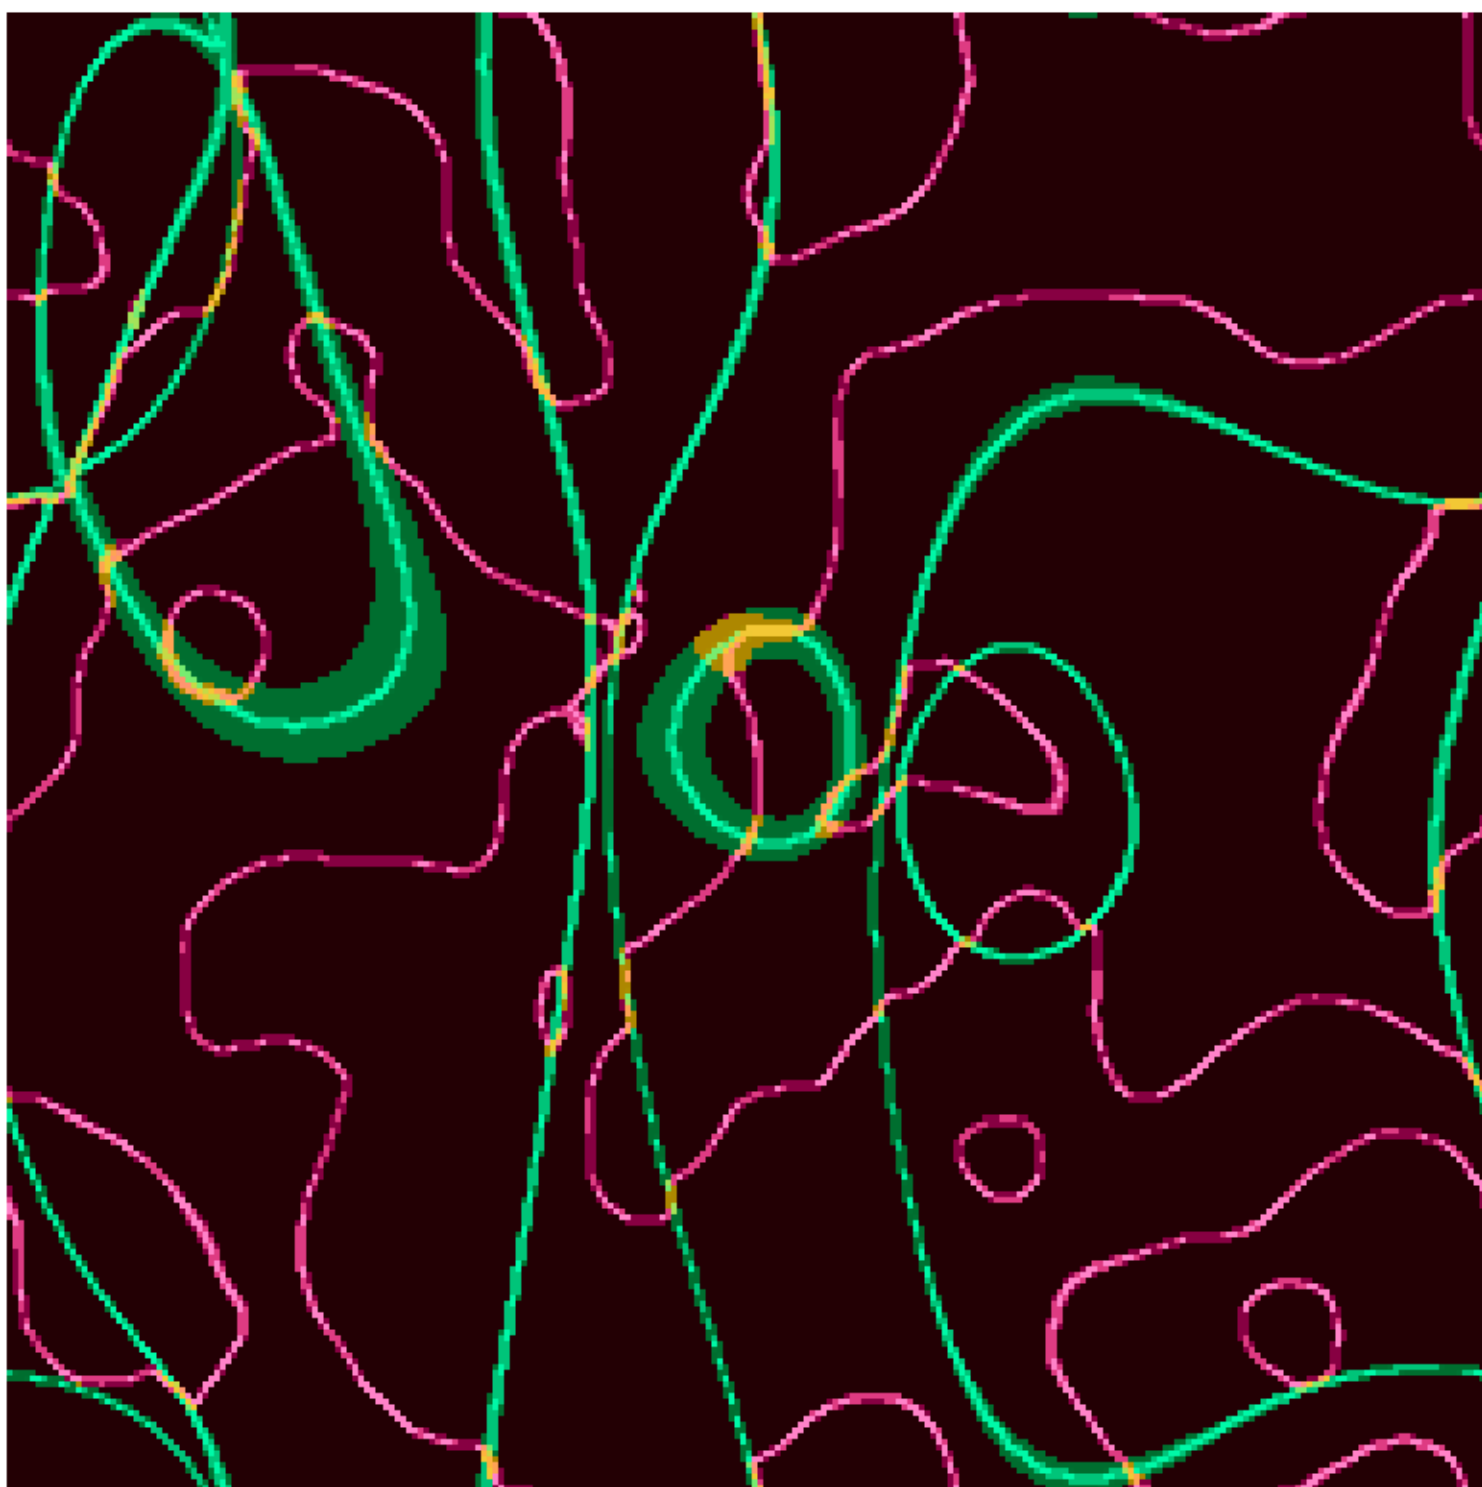

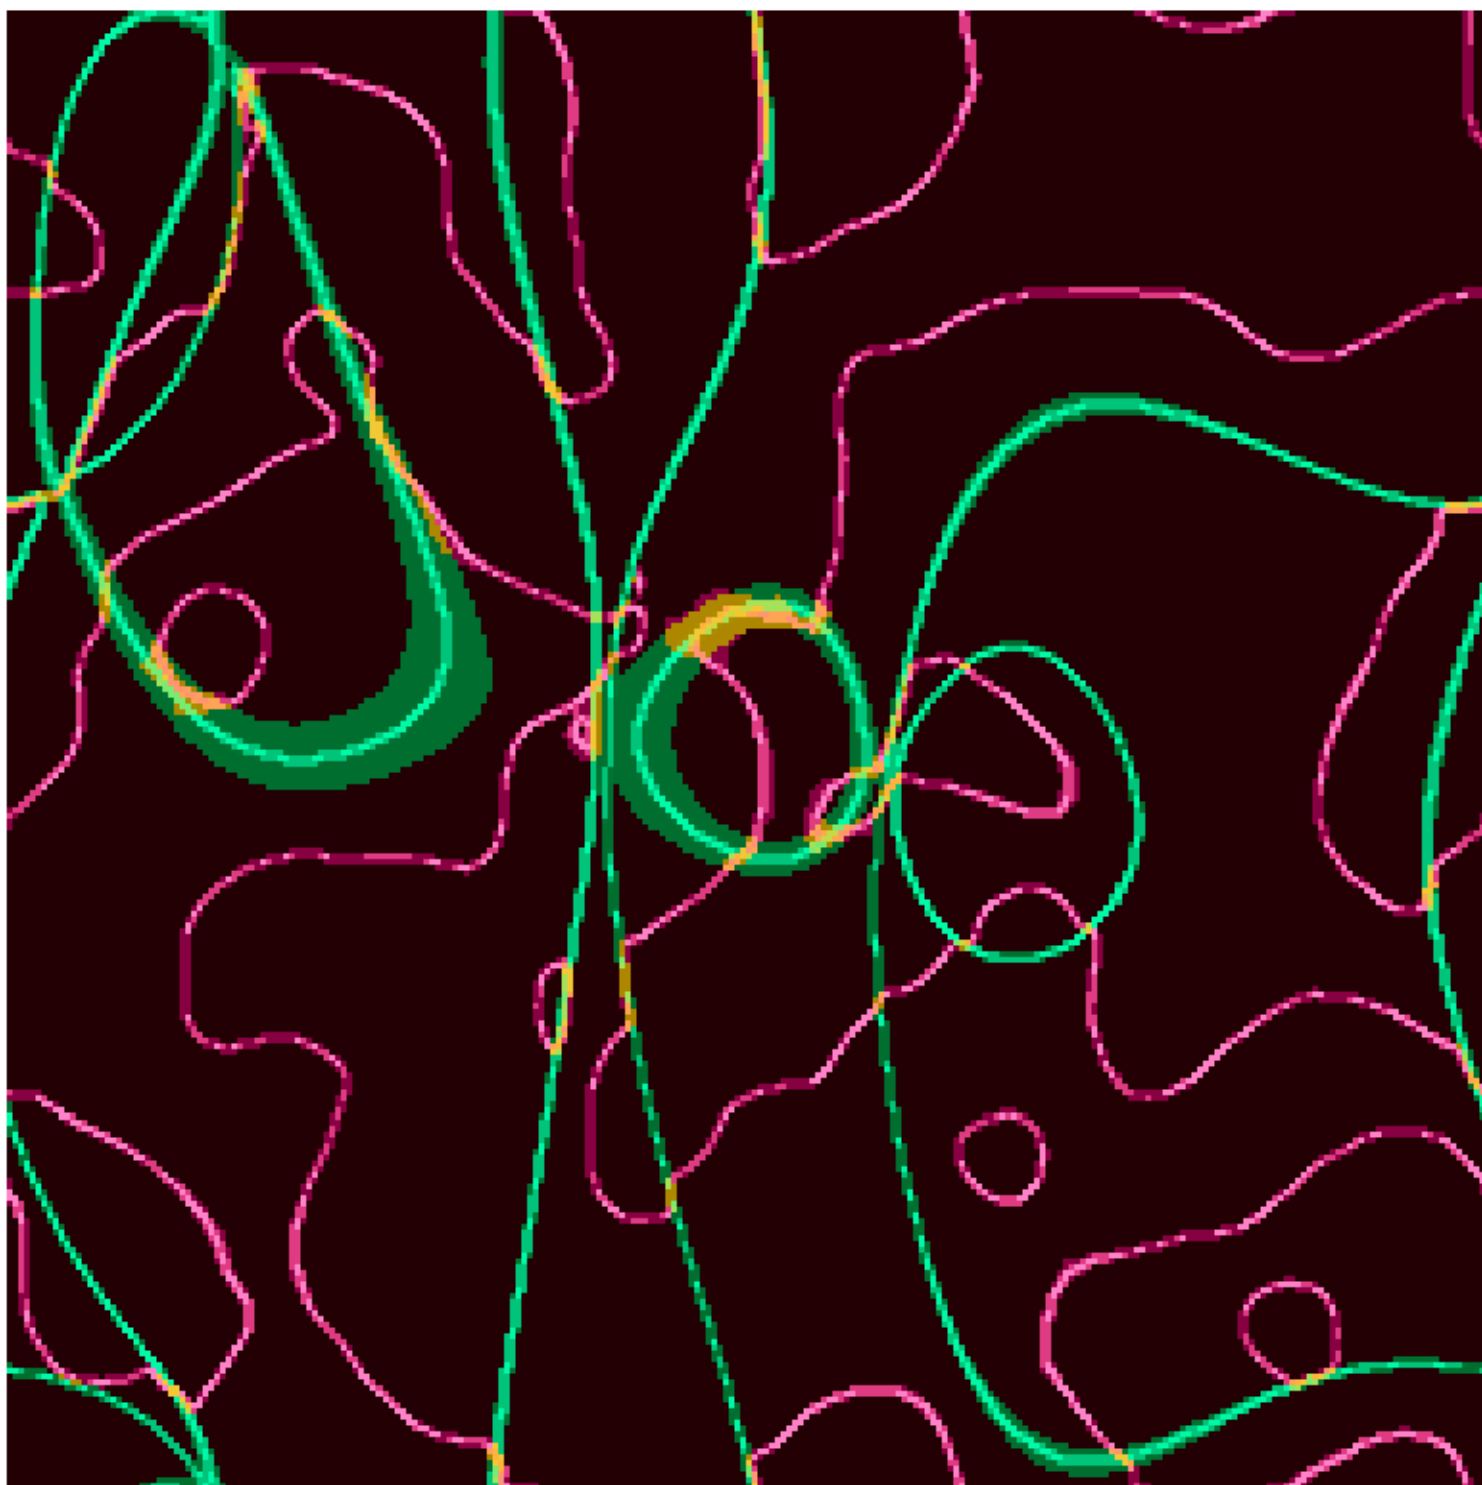

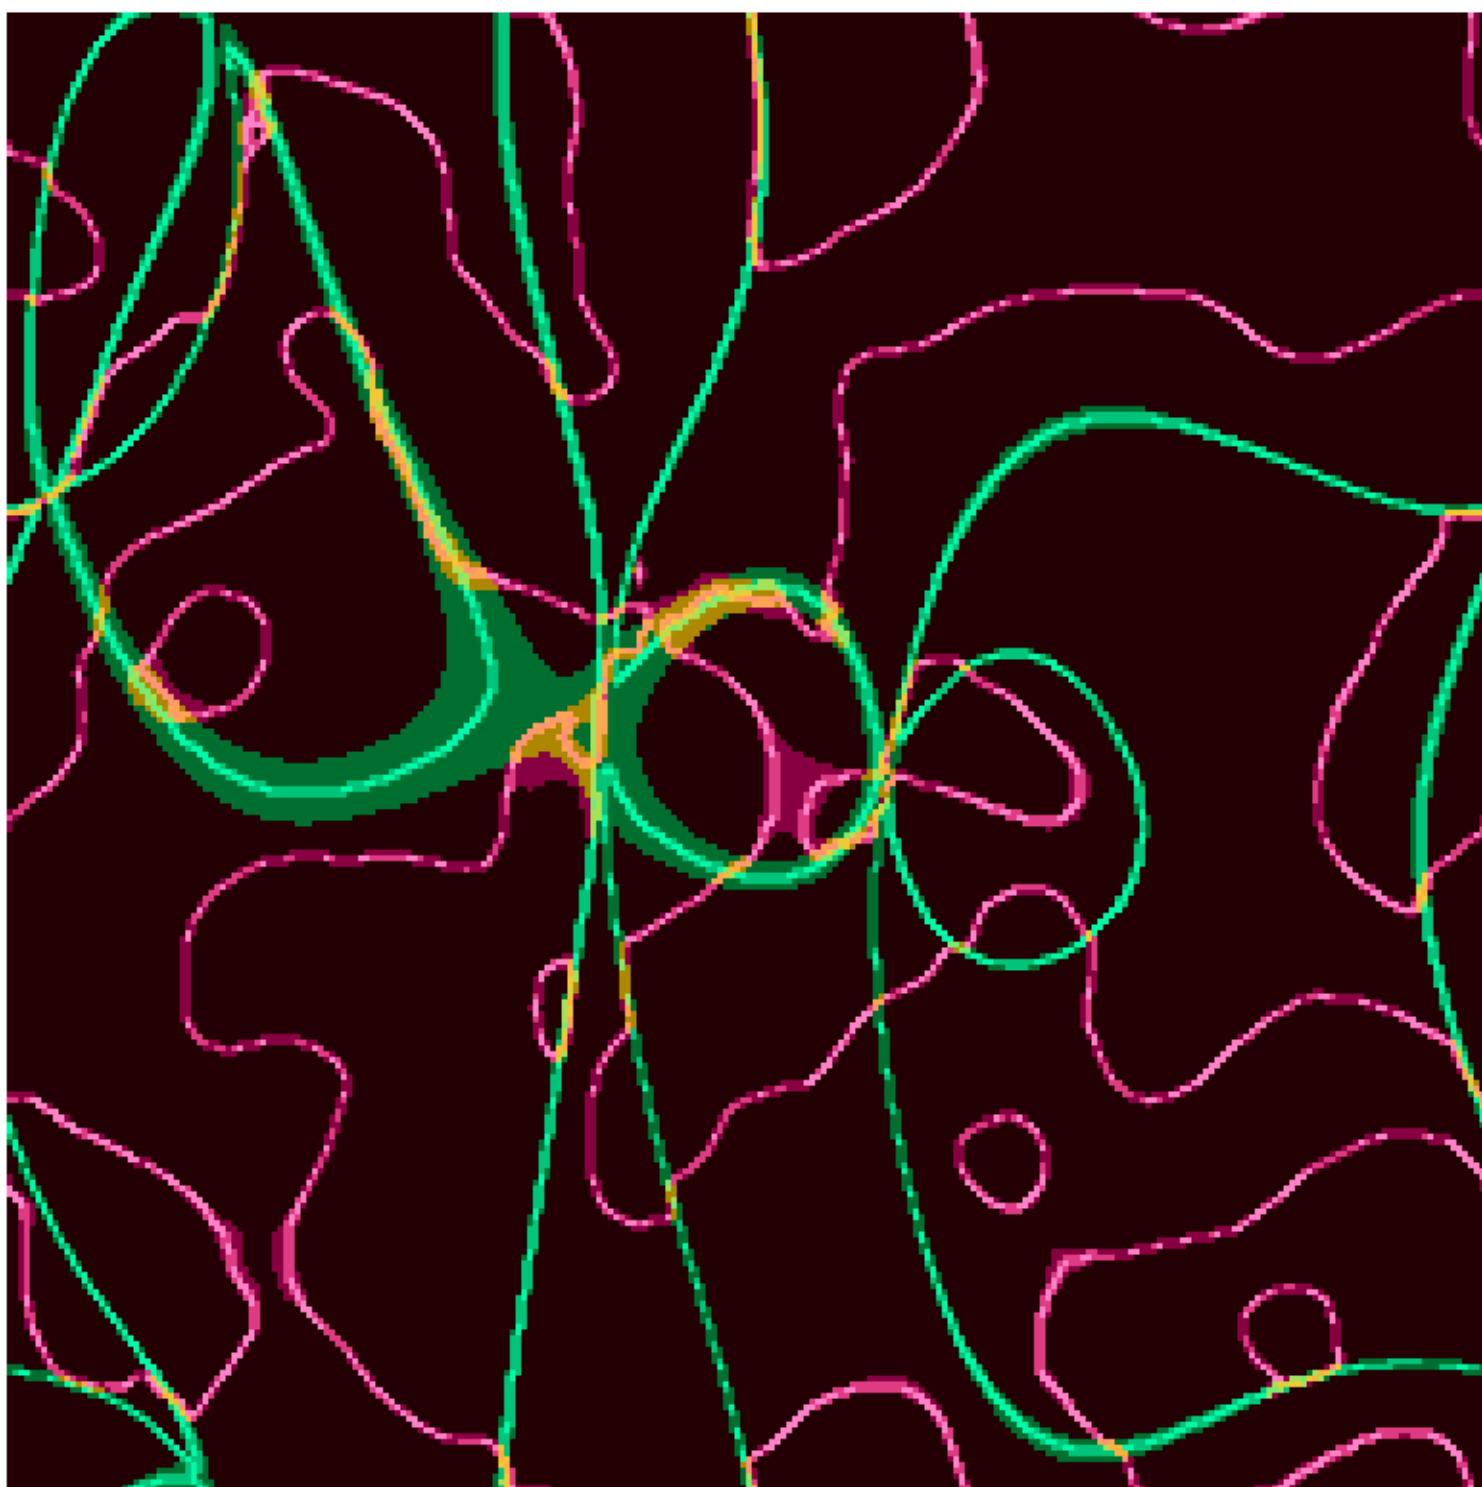

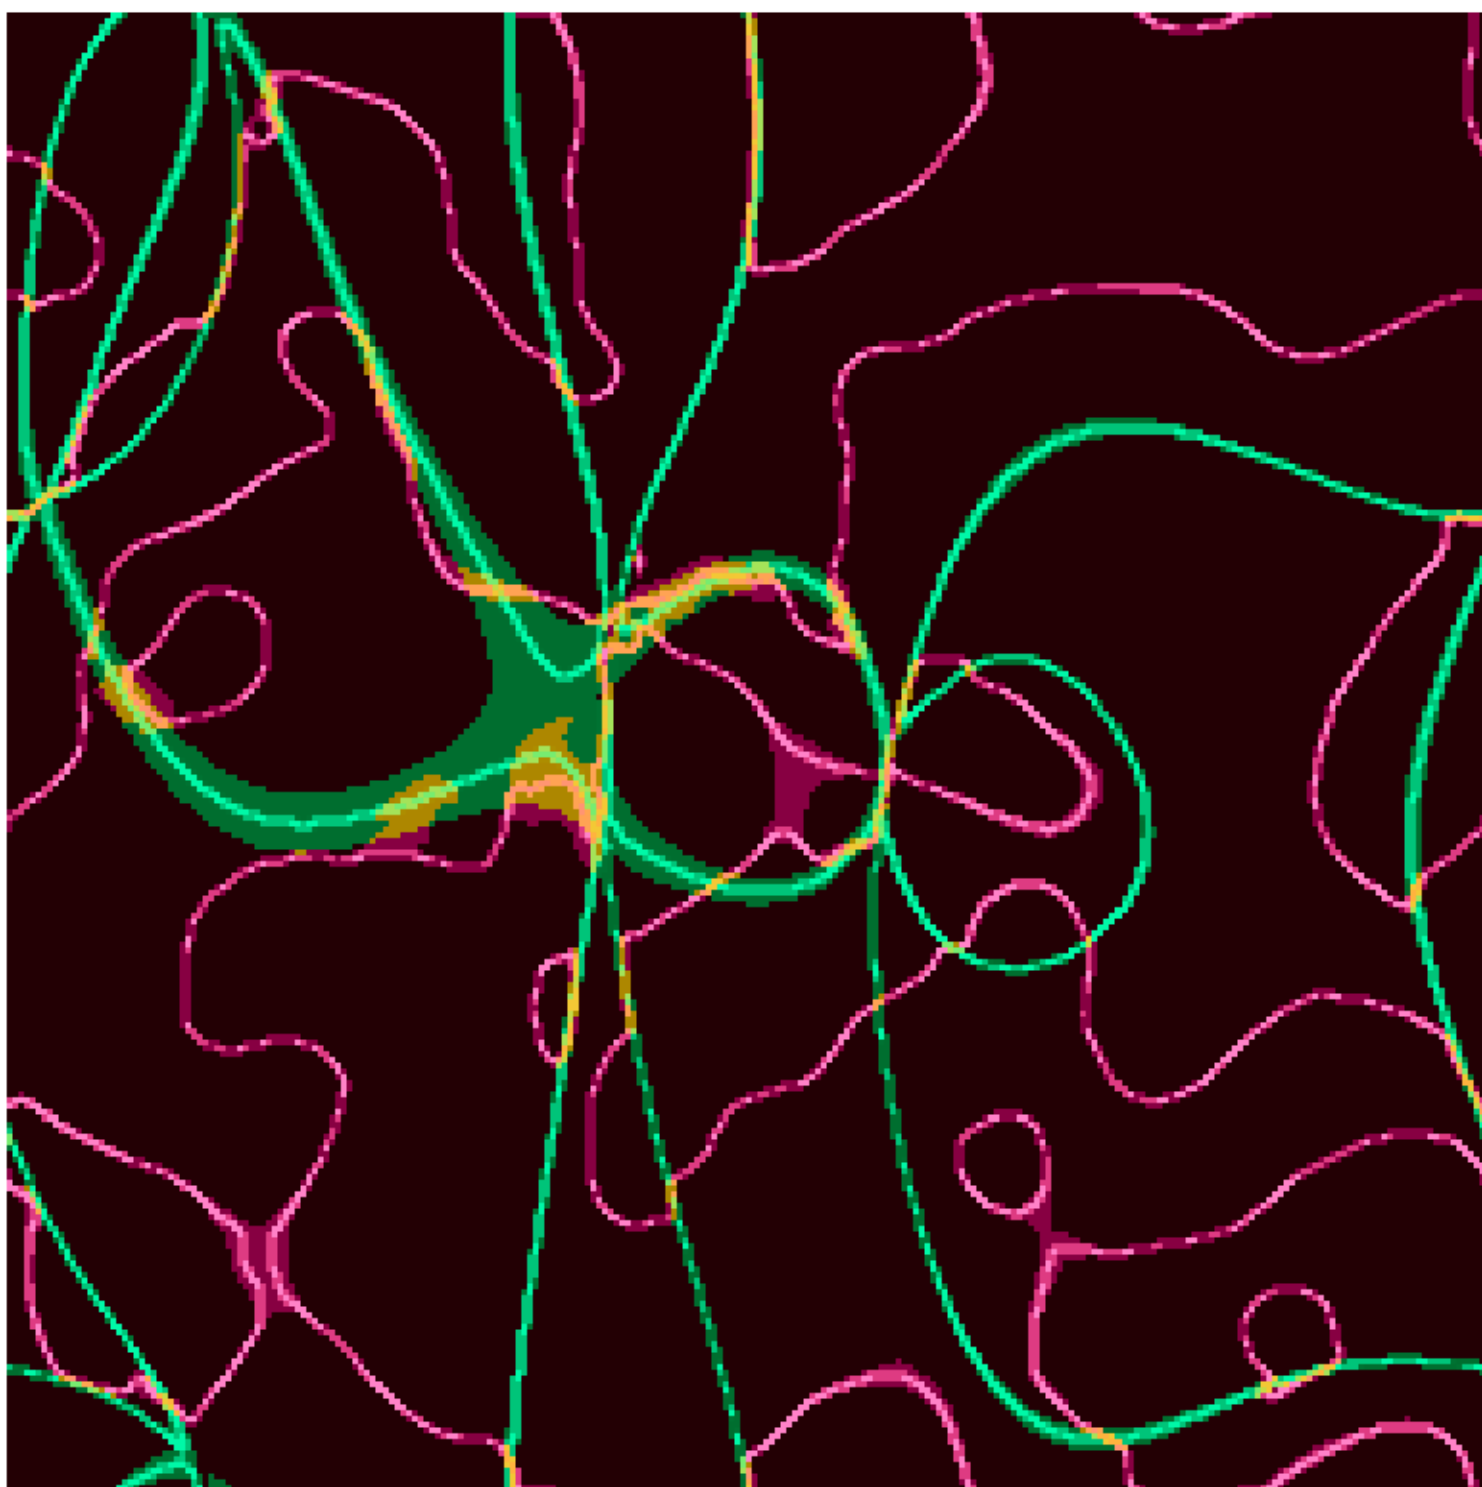

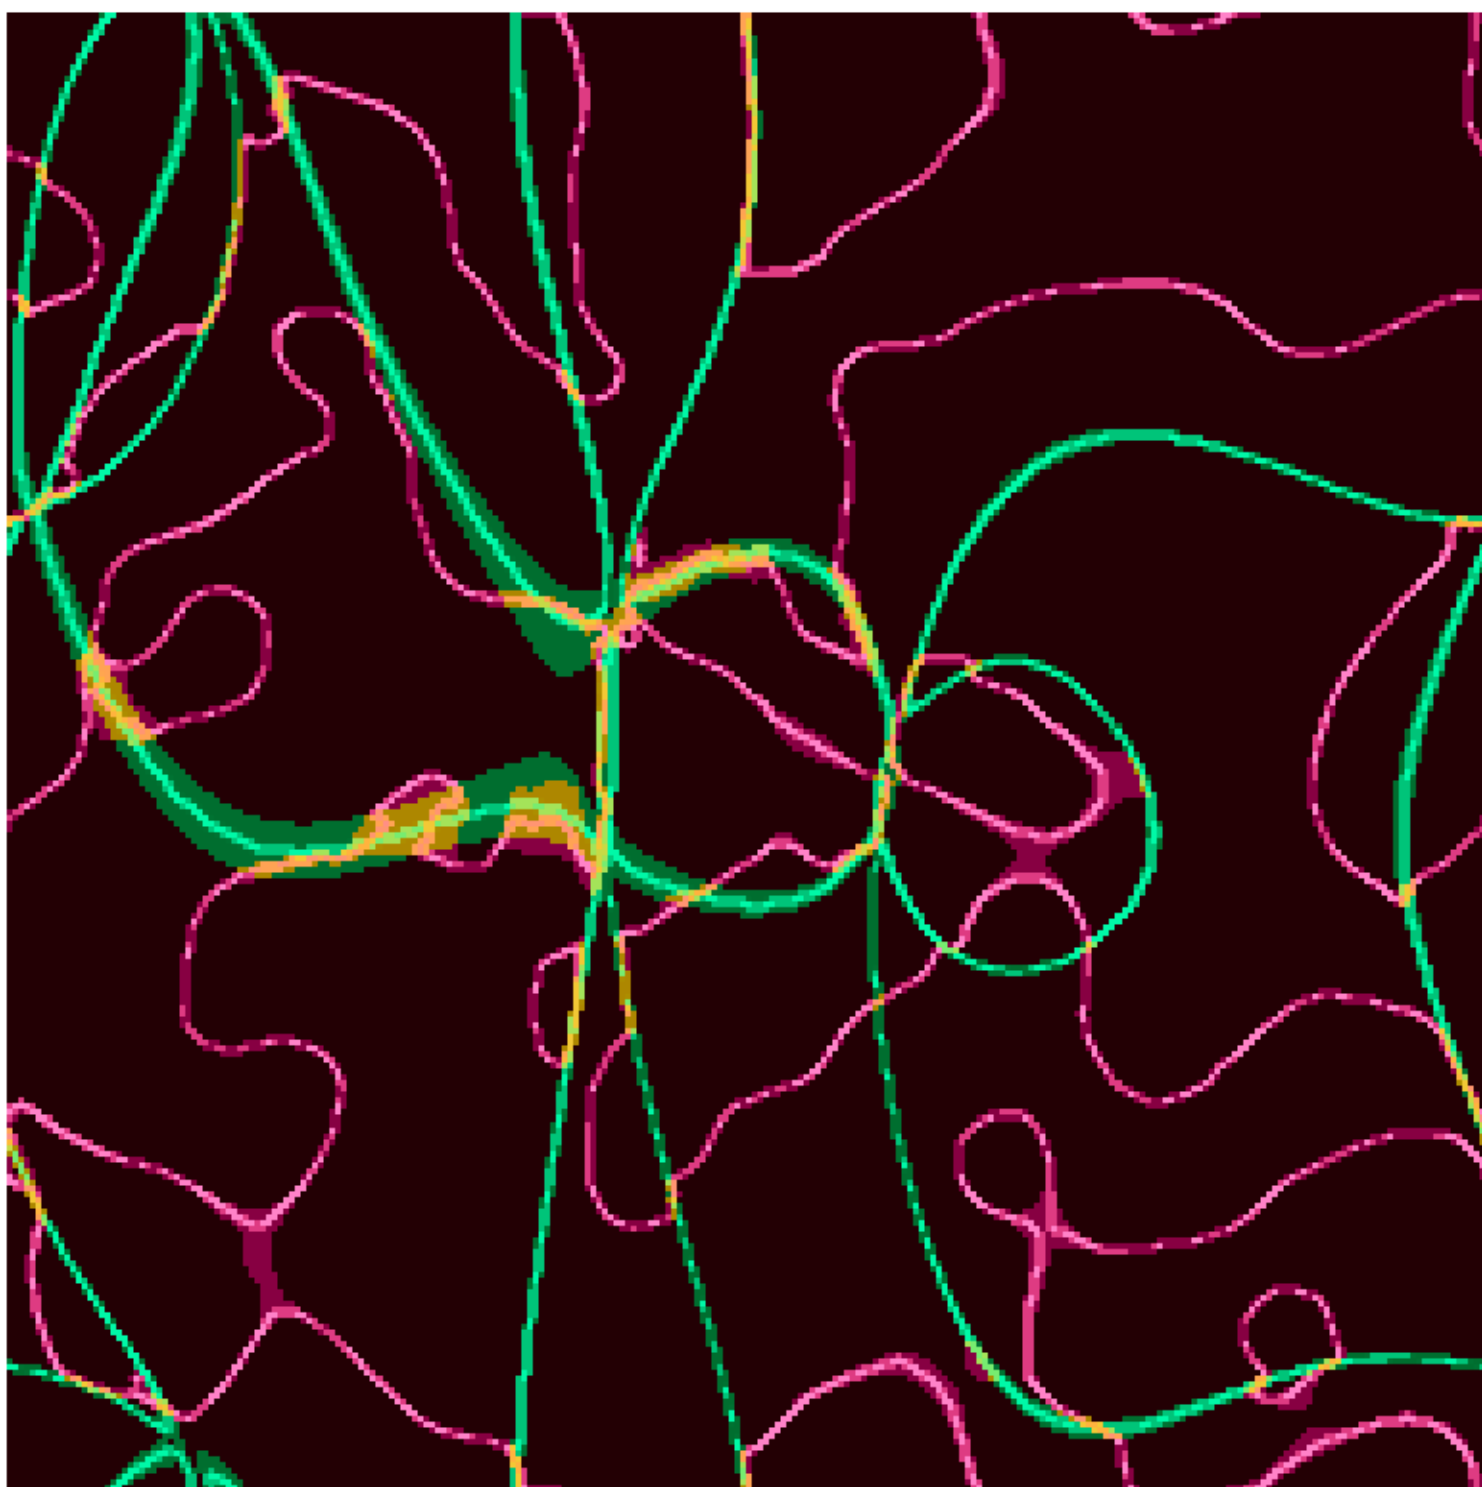

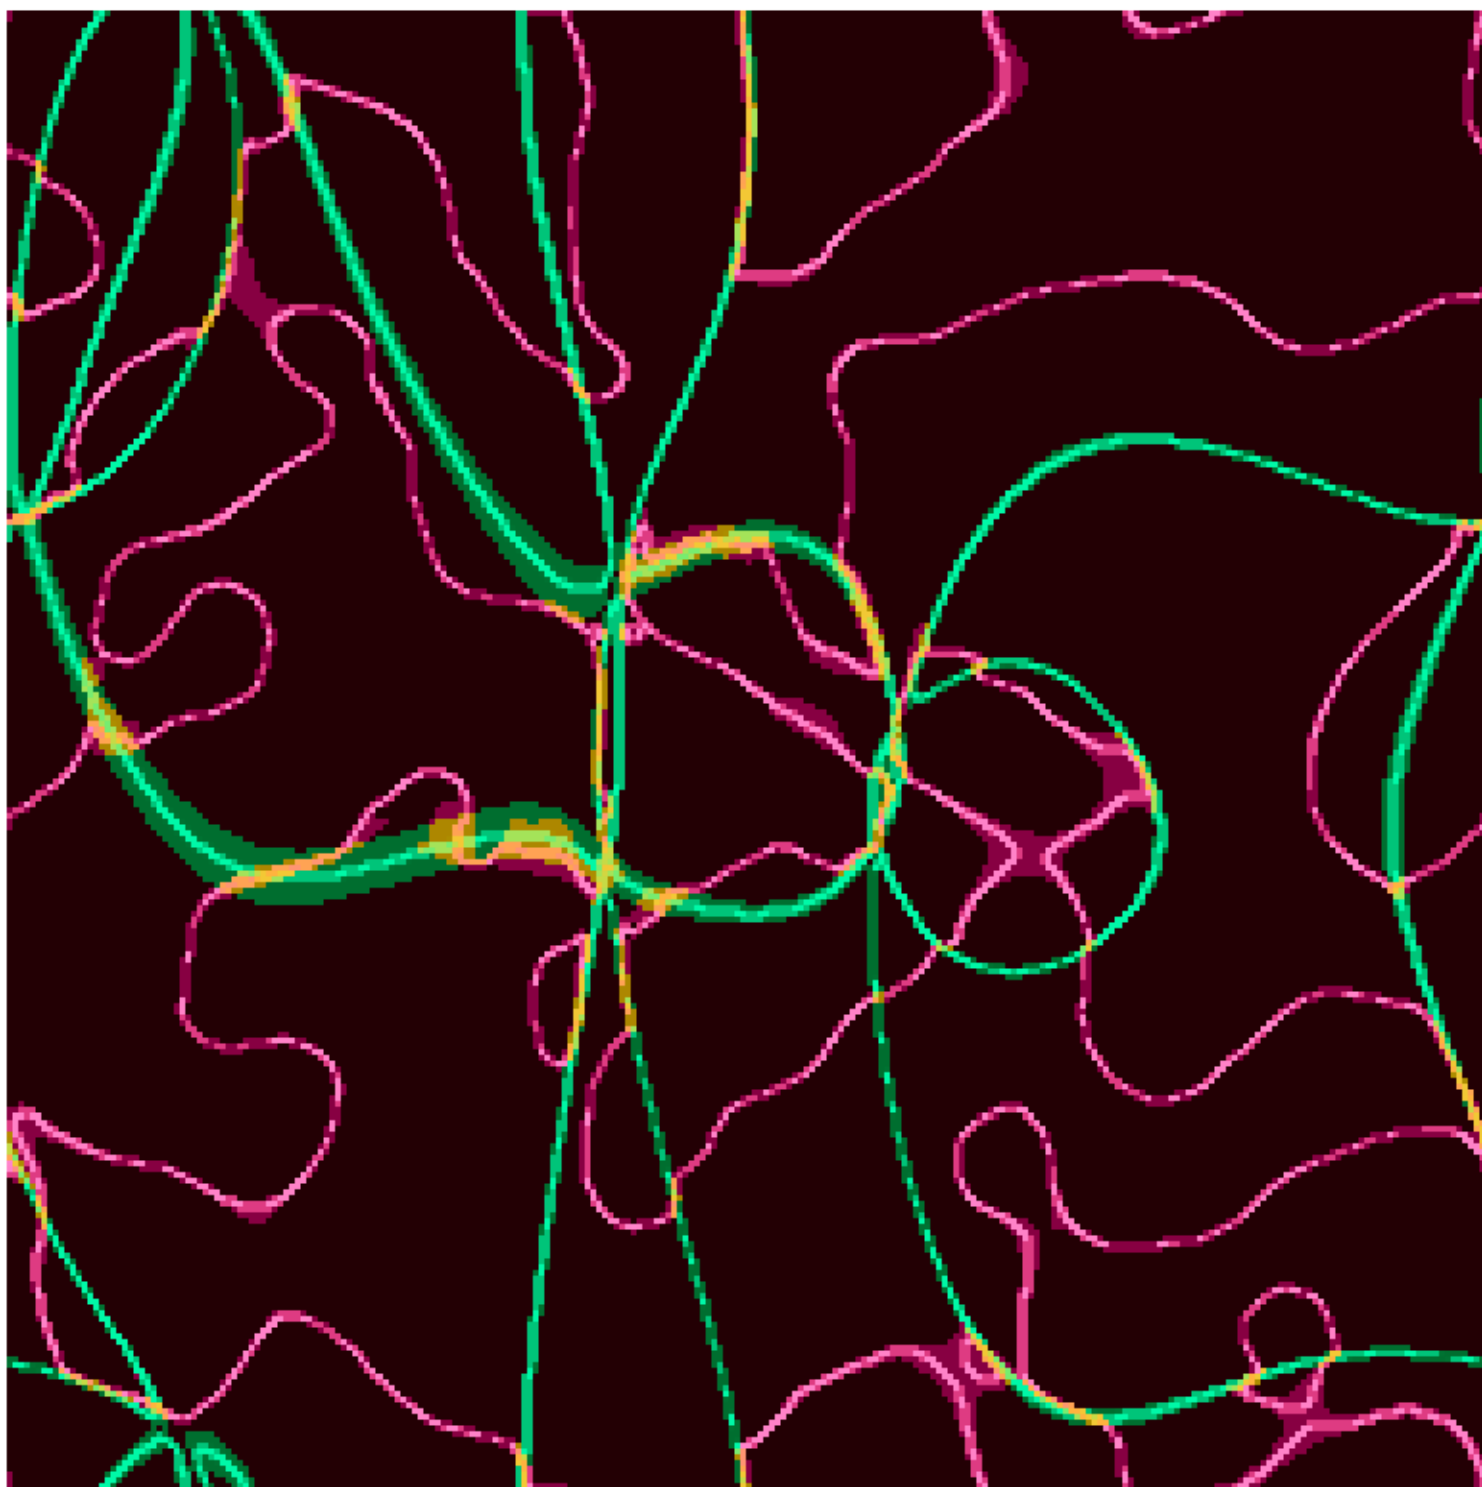

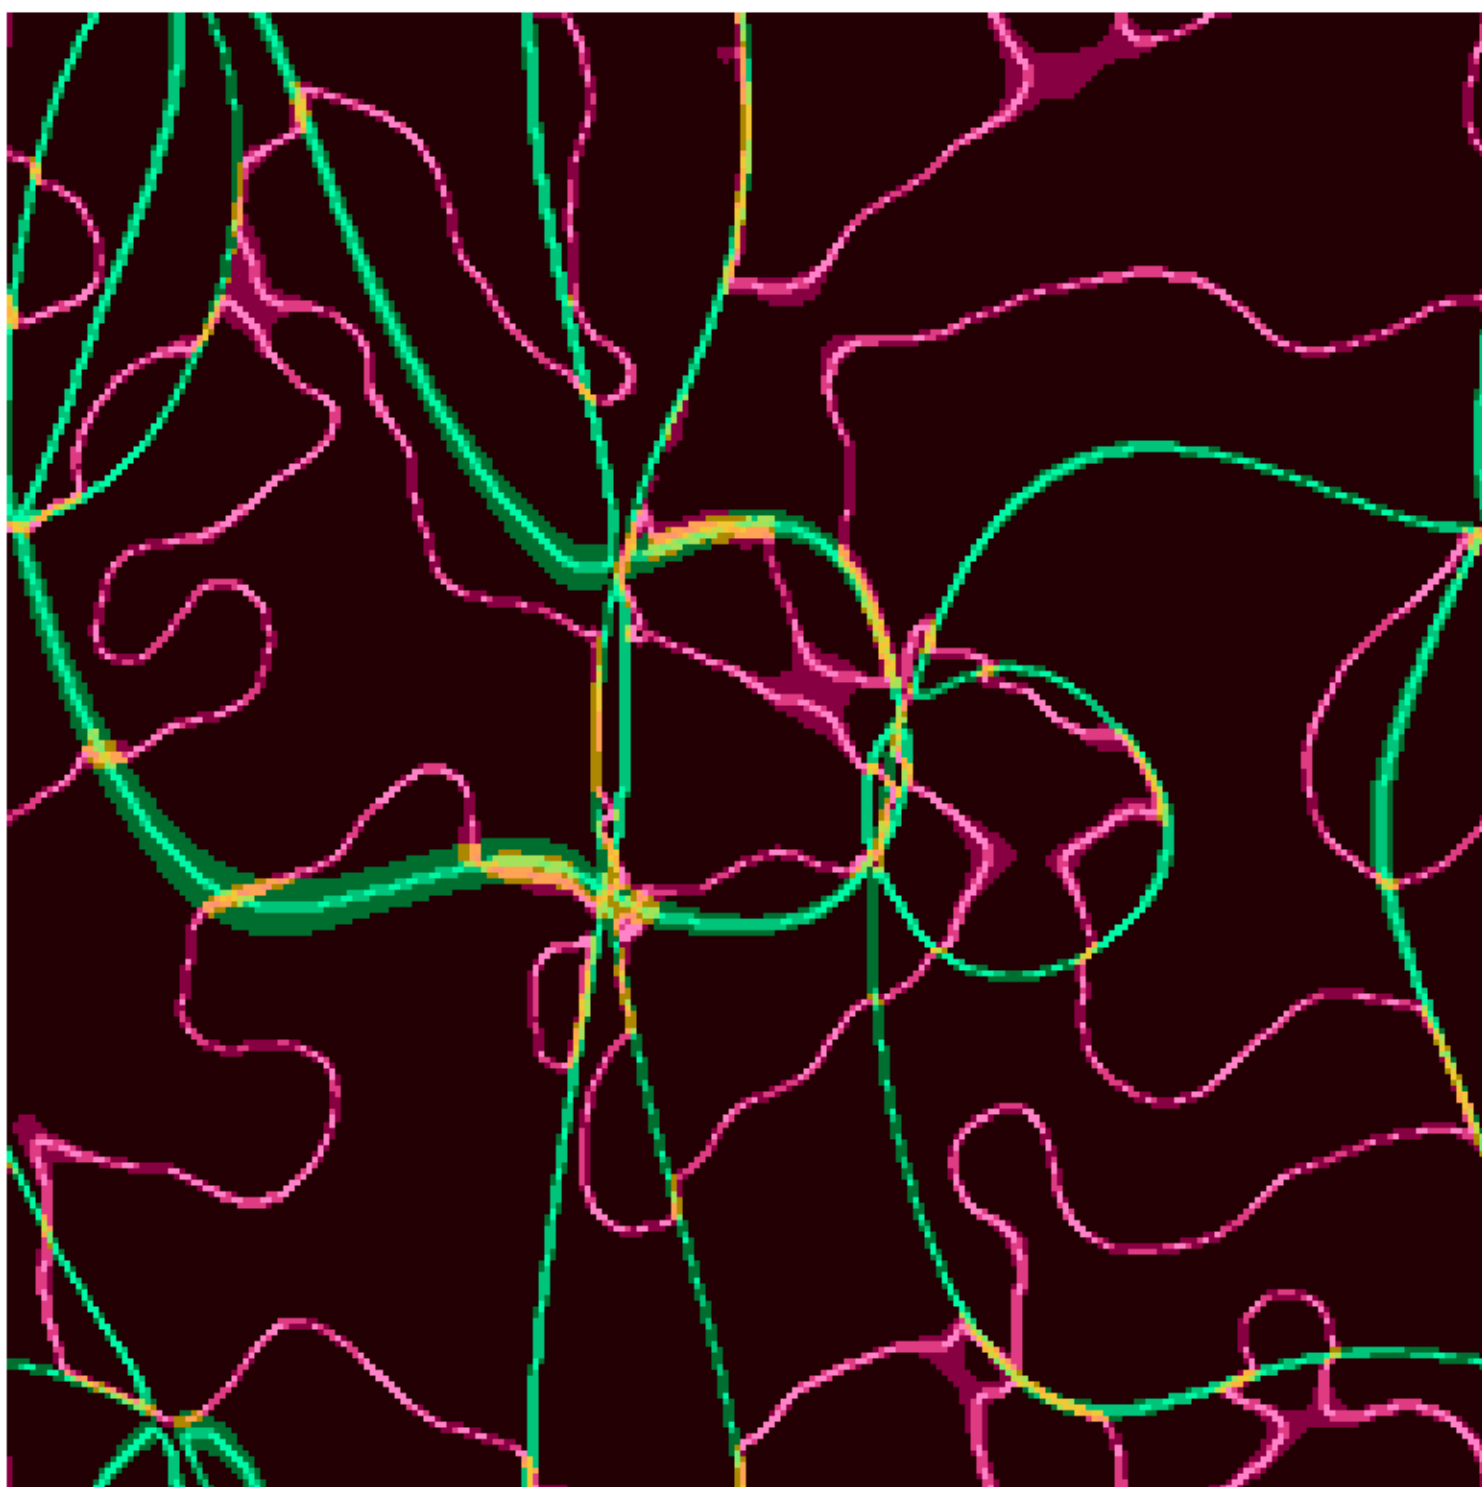



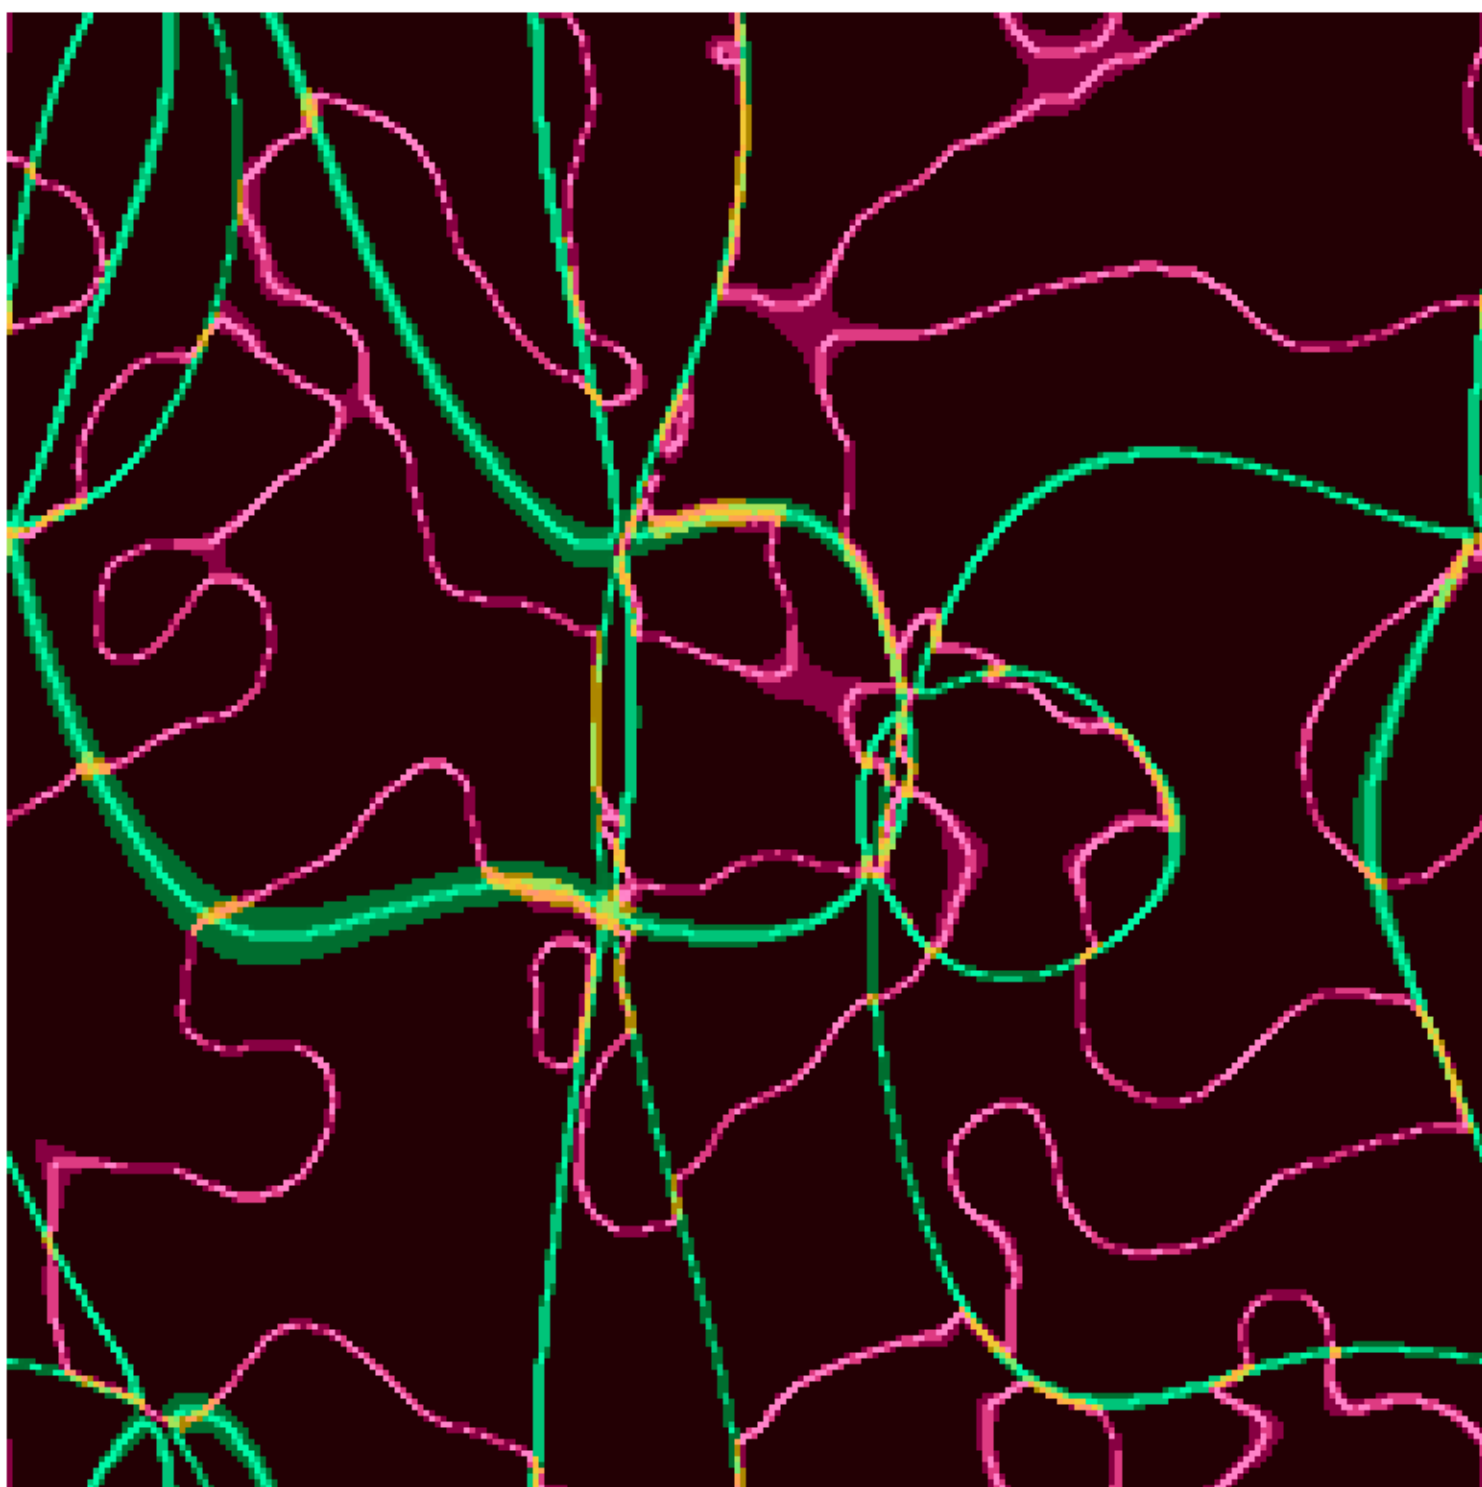

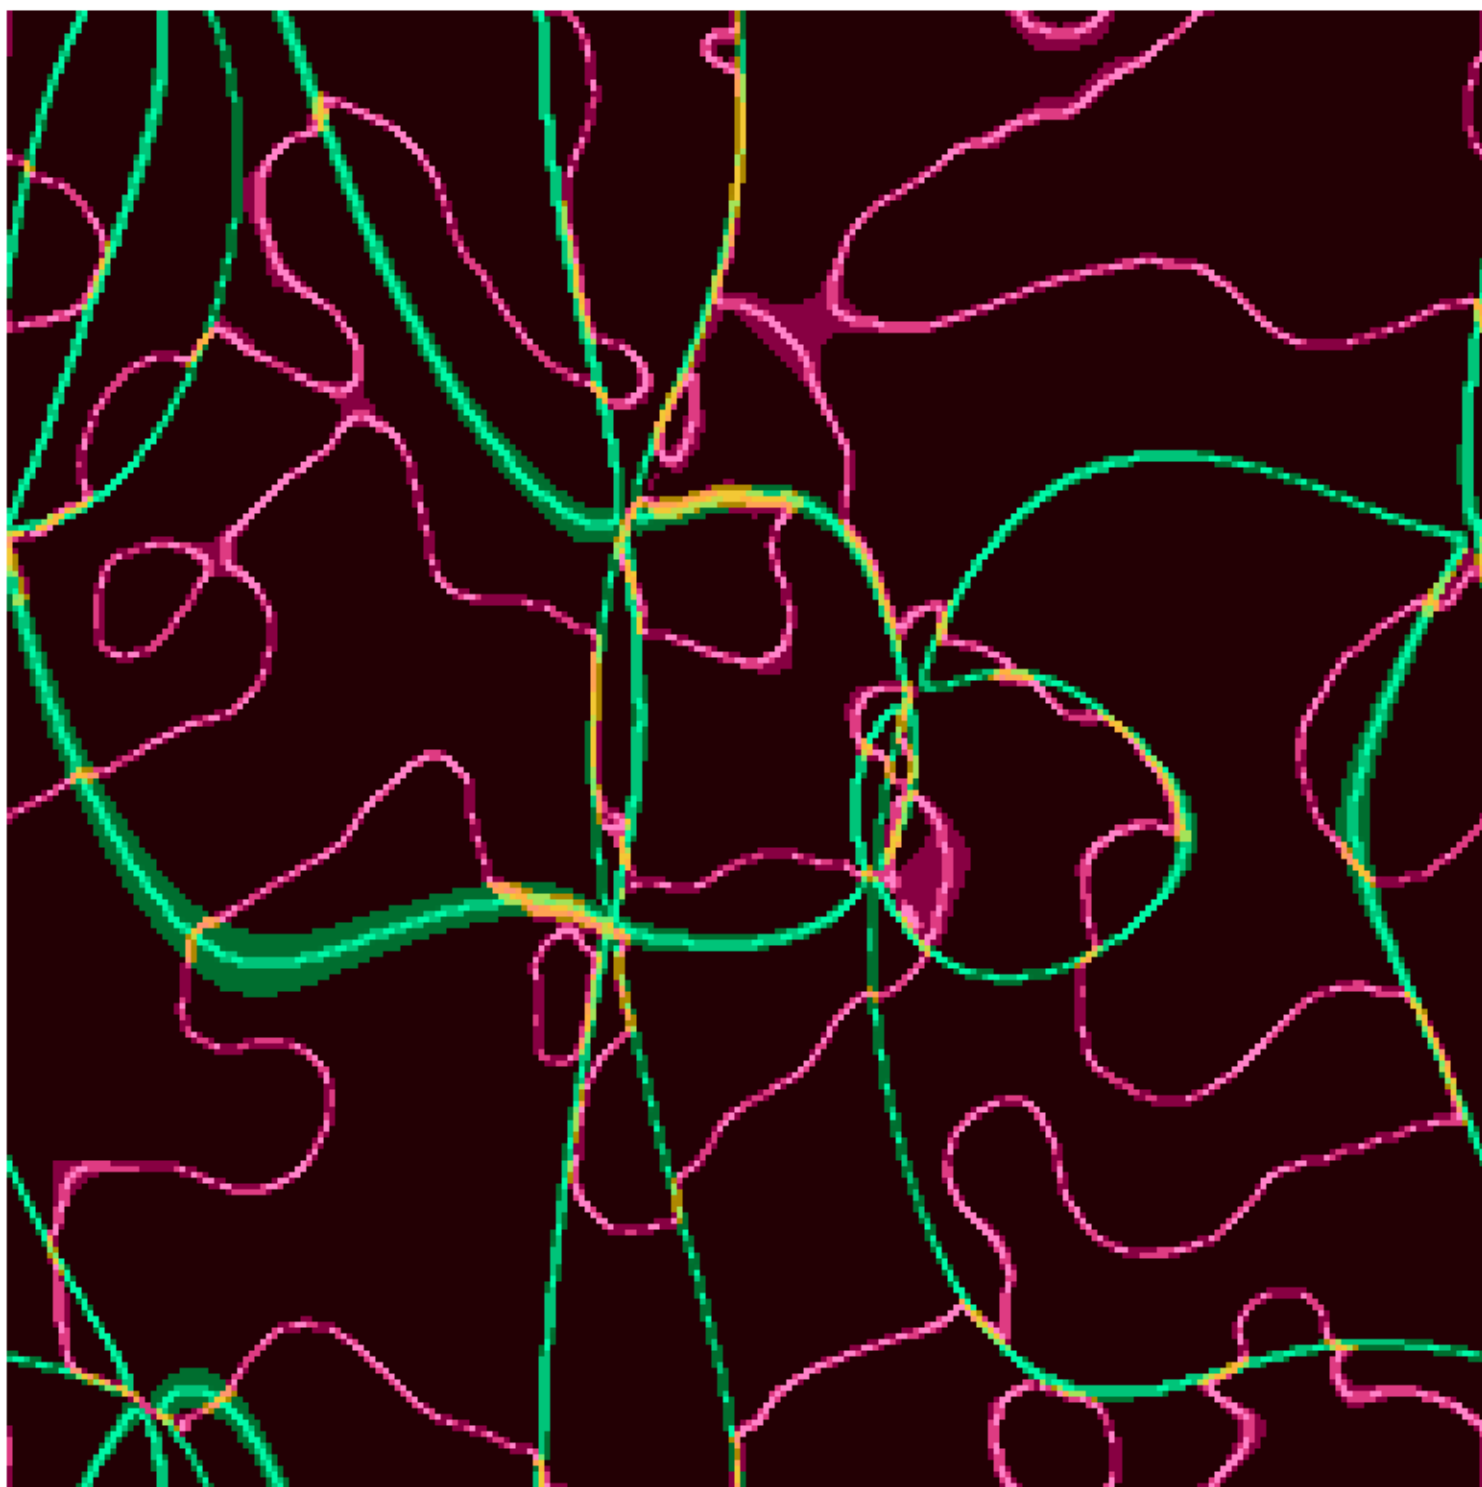

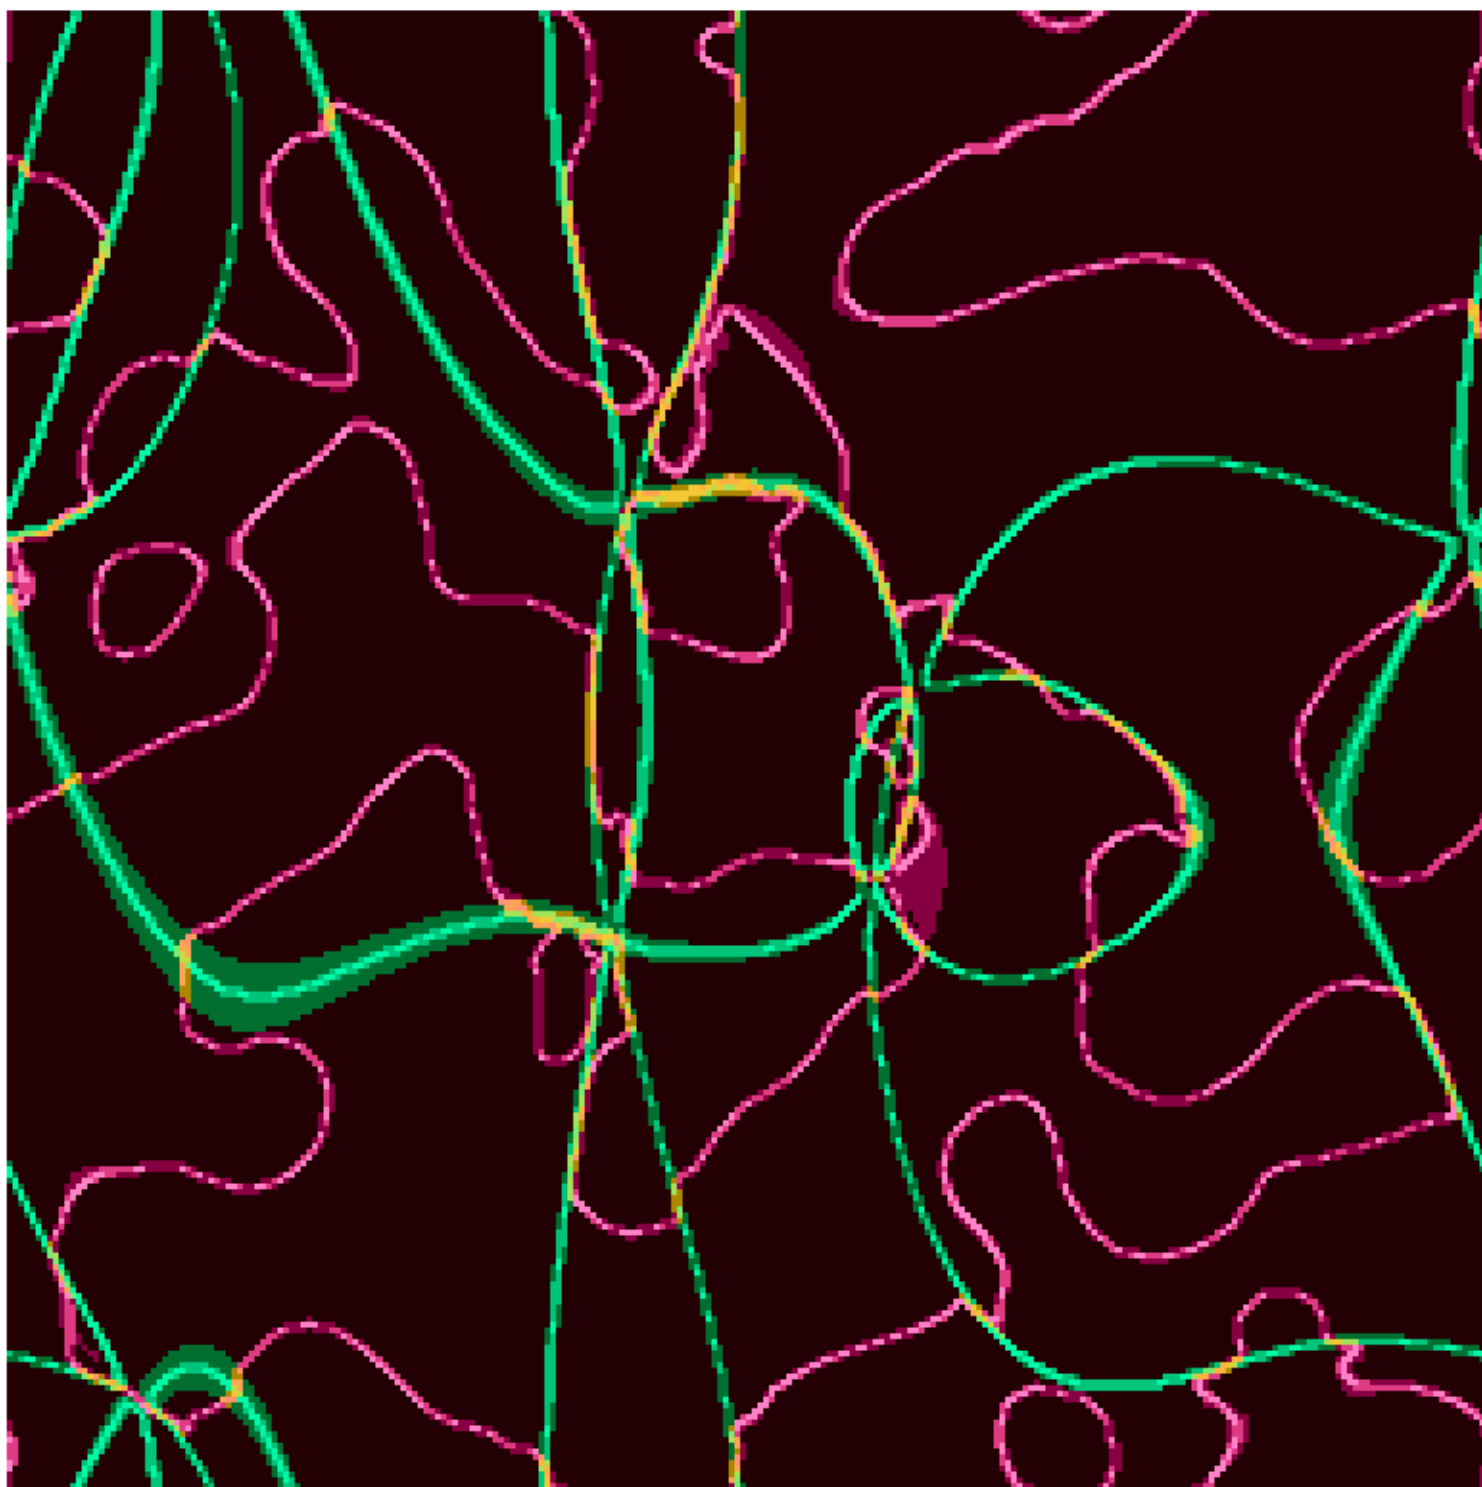

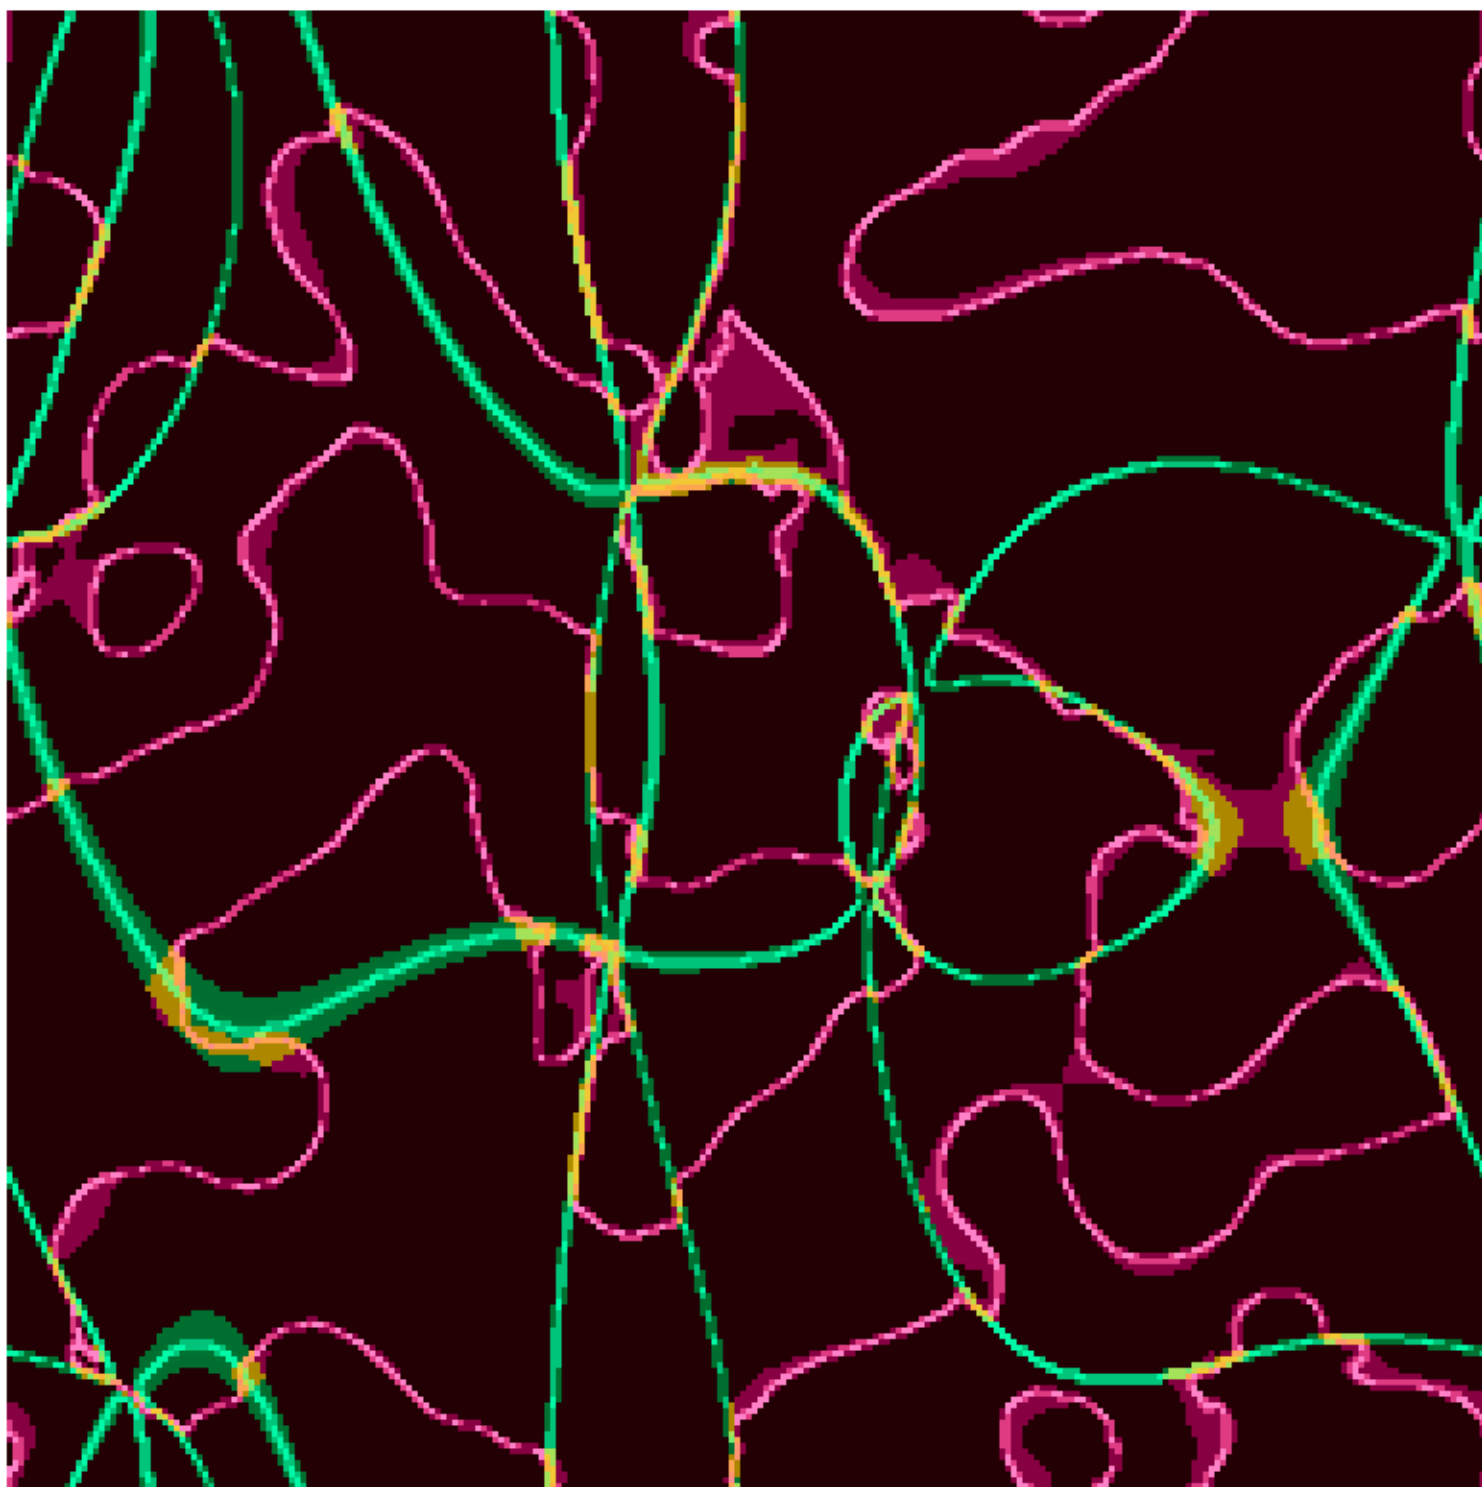

Supplement: Supplementary file 1 [file Supplemental_Data_A.pdf]
